# Supplementary material for: Controlling nanothread backbone structure through precursor design
Source: arXiv:2302.07482 source file (2023-02-15)
Supplement: Supplementary file 1 [file AtomicCoordinates.pdf]

##### SUPPORTING INFORMATION FOR #####  
CONTROLLING NANOTHREAD BACKBONE STRUCTURE THROUGH PRECURSOR DESIGN

Andrew Reynoso, Bohan Xu, and Vincent H. Crespi

#####

This file contains the coordinates and unit cell dimensions for  
206 different isolated carbon nanothreads formed by functionalized  
furan and thiophene

#####

furan\_Br\_23\_anti\_alt Energy: -208.58323001

##### cif starts

data\_furan\_Br\_23\_anti\_alt

\_publ\_section\_comment

;  
Andrew Reynoso, Bohan Xu, and Vincent H. Crespi  
;

\_cell\_length\_a 9.471752567

\_cell\_length\_b 20.0

\_cell\_length\_c 20.0

\_cell\_angle\_alpha 90.0

\_cell\_angle\_beta 90.0

\_cell\_angle\_gamma 90.0

\_symmetry\_space\_group\_name\_H-M 'P 1'

\_symmetry\_Int\_Tables\_number 1

\_symmetry\_cell\_setting triclinic

loop\_

\_atom\_site\_label

\_atom\_site\_type\_symbol

\_atom\_site\_fract\_x

\_atom\_site\_fract\_y

\_atom\_site\_fract\_z

\_atom\_site\_occupancy

|     |   |                    |                    |                    |     |
|-----|---|--------------------|--------------------|--------------------|-----|
| H1  | H | 0.9897546600000000 | 0.8979396500000000 | 0.9441384200000000 | 1.0 |
| H2  | H | 0.9803095300000000 | 0.9415471200000000 | 0.0764393500000000 | 1.0 |
| H3  | H | 0.2397446600000000 | 0.1003729300000000 | 0.0521268400000000 | 1.0 |
| H4  | H | 0.2303429300000000 | 0.0568039700000000 | 0.9198093500000000 | 1.0 |
| H5  | H | 0.4897739500000000 | 0.8979506400000000 | 0.9441119900000000 | 1.0 |
| H6  | H | 0.4802797400000000 | 0.9414965800000000 | 0.0764263200000000 | 1.0 |
| H7  | H | 0.7397959400000000 | 0.1004325500000000 | 0.0520781400000000 | 1.0 |
| H8  | H | 0.7302691300000000 | 0.0568019600000000 | 0.9197929200000000 | 1.0 |
| C9  | C | 0.0179026600000000 | 0.9455649900000000 | 0.9670696800000000 | 1.0 |
| C10 | C | 0.9351228500000000 | 0.9619760100000000 | 0.0304405800000000 | 1.0 |
| C11 | C | 0.9312873400000000 | 0.0401591100000000 | 0.0289554000000000 | 1.0 |
| C12 | C | 0.0225561300000000 | 0.0536580600000000 | 0.9651282200000000 | 1.0 |
| C13 | C | 0.2678947500000000 | 0.0527559700000000 | 0.0291776100000000 | 1.0 |
| C14 | C | 0.1851390300000000 | 0.0363644100000000 | 0.9657995200000000 | 1.0 |
| C15 | C | 0.1812725300000000 | 0.9581794000000000 | 0.9672688600000000 | 1.0 |
| C16 | C | 0.2725226300000000 | 0.9446595700000000 | 0.0310948200000000 | 1.0 |
| C17 | C | 0.5179060000000000 | 0.9455677000000000 | 0.9670652200000000 | 1.0 |
| C18 | C | 0.4351093200000000 | 0.9619480900000000 | 0.0304336300000000 | 1.0 |
| C19 | C | 0.4312644400000000 | 0.0401299500000000 | 0.0289805900000000 | 1.0 |

|      |    |                    |                    |                    |     |
|------|----|--------------------|--------------------|--------------------|-----|
| C20  | C  | 0.5225389500000000 | 0.0536597300000000 | 0.9651571800000000 | 1.0 |
| C21  | C  | 0.7679235800000000 | 0.0527974100000000 | 0.0291566200000000 | 1.0 |
| C22  | C  | 0.6851272200000000 | 0.0363732400000000 | 0.9658017900000000 | 1.0 |
| C23  | C  | 0.6812738300000000 | 0.9581872000000000 | 0.9672903600000000 | 1.0 |
| C24  | C  | 0.7725247600000000 | 0.9446996800000000 | 0.0311294000000000 | 1.0 |
| O25  | O  | 0.9734380100000000 | 0.0004589100000000 | 0.9229903700000000 | 1.0 |
| O26  | O  | 0.2234028700000000 | 0.9978490500000000 | 0.0732394200000000 | 1.0 |
| O27  | O  | 0.4734359100000000 | 0.0004737800000000 | 0.9229995200000000 | 1.0 |
| O28  | O  | 0.7234425600000000 | 0.9979165000000000 | 0.0732479100000000 | 1.0 |
| Br29 | Br | 0.9896714200000000 | 0.0879432200000000 | 0.1113341100000000 | 1.0 |
| Br30 | Br | 0.9864546000000000 | 0.1403385500000000 | 0.9246398900000000 | 1.0 |
| Br31 | Br | 0.2397357200000000 | 0.9103737700000000 | 0.8849143000000000 | 1.0 |
| Br32 | Br | 0.2365001600000000 | 0.8579647000000000 | 0.0715710700000000 | 1.0 |
| Br33 | Br | 0.4896302300000000 | 0.0878956500000000 | 0.1113720300000000 | 1.0 |
| Br34 | Br | 0.4864454800000000 | 0.1403672200000000 | 0.9247237500000000 | 1.0 |
| Br35 | Br | 0.7397693200000000 | 0.9103556500000000 | 0.8849530500000000 | 1.0 |
| Br36 | Br | 0.7364649000000000 | 0.8580554300000000 | 0.0717038700000000 | 1.0 |

##### cif ends

furan\_Br\_23\_anti\_alt\_forbid Energy: -209.44143449

##### cif starts

data\_furan\_Br\_23\_anti\_alt\_forbid

\_publ\_section\_comment

;  
Andrew Reynoso, Bohan Xu, and Vincent H. Crespi  
;

\_cell\_length\_a 10.2860132424

\_cell\_length\_b 20.0

\_cell\_length\_c 20.0

\_cell\_angle\_alpha 90.0

\_cell\_angle\_beta 90.0

\_cell\_angle\_gamma 90.0

\_symmetry\_space\_group\_name\_H-M 'P 1'

\_symmetry\_Int\_Tables\_number 1

\_symmetry\_cell\_setting triclinic

loop\_

\_atom\_site\_label

\_atom\_site\_type\_symbol

\_atom\_site\_fract\_x

\_atom\_site\_fract\_y

\_atom\_site\_fract\_z

\_atom\_site\_occupancy

|    |   |                    |                    |                    |     |
|----|---|--------------------|--------------------|--------------------|-----|
| H1 | H | 0.9542990300000000 | 0.9314434400000000 | 0.0511793700000000 | 1.0 |
|----|---|--------------------|--------------------|--------------------|-----|

|    |   |                    |                    |                    |     |
|----|---|--------------------|--------------------|--------------------|-----|
| H2 | H | 0.0695832900000000 | 0.8942408900000000 | 0.9299500200000000 | 1.0 |
|----|---|--------------------|--------------------|--------------------|-----|

|    |   |                    |                    |                    |     |
|----|---|--------------------|--------------------|--------------------|-----|
| H3 | H | 0.3305385300000000 | 0.0595851600000000 | 0.9125821100000000 | 1.0 |
|----|---|--------------------|--------------------|--------------------|-----|

|    |   |                    |                    |                    |     |
|----|---|--------------------|--------------------|--------------------|-----|
| H4 | H | 0.2153858300000000 | 0.0968107500000000 | 0.0338372700000000 | 1.0 |
|----|---|--------------------|--------------------|--------------------|-----|

|    |   |                    |                    |                    |     |
|----|---|--------------------|--------------------|--------------------|-----|
| H5 | H | 0.4539910800000000 | 0.9317157500000000 | 0.0511187400000000 | 1.0 |
|----|---|--------------------|--------------------|--------------------|-----|

|    |   |                    |                    |                    |     |
|----|---|--------------------|--------------------|--------------------|-----|
| H6 | H | 0.5694344200000000 | 0.8942042700000000 | 0.9300410300000000 | 1.0 |
|----|---|--------------------|--------------------|--------------------|-----|

|    |   |                    |                    |                    |     |
|----|---|--------------------|--------------------|--------------------|-----|
| H7 | H | 0.8309942300000000 | 0.0593065900000000 | 0.9126101600000000 | 1.0 |
|----|---|--------------------|--------------------|--------------------|-----|

|    |   |                    |                    |                    |     |
|----|---|--------------------|--------------------|--------------------|-----|
| H8 | H | 0.7154673100000000 | 0.0968452500000000 | 0.0336701100000000 | 1.0 |
|----|---|--------------------|--------------------|--------------------|-----|

|      |    |                    |                    |                    |     |
|------|----|--------------------|--------------------|--------------------|-----|
| C9   | C  | 0.0804628800000000 | 0.0515978600000000 | 0.9603385300000000 | 1.0 |
| C10  | C  | 0.9566350700000000 | 0.0350853800000000 | 0.0015376500000000 | 1.0 |
| C11  | C  | 0.9582900900000000 | 0.9562957600000000 | 0.0024223000000000 | 1.0 |
| C12  | C  | 0.0789191000000000 | 0.9391828200000000 | 0.9607208300000000 | 1.0 |
| C13  | C  | 0.2059923700000000 | 0.0518693100000000 | 0.0030711200000000 | 1.0 |
| C14  | C  | 0.3265858300000000 | 0.0347311600000000 | 0.9613373000000000 | 1.0 |
| C15  | C  | 0.3282409200000000 | 0.9559343300000000 | 0.9622441500000000 | 1.0 |
| C16  | C  | 0.2044330800000000 | 0.9394612200000000 | 0.0034770800000000 | 1.0 |
| C17  | C  | 0.5806066900000000 | 0.0516096000000000 | 0.9601285900000000 | 1.0 |
| C18  | C  | 0.4566672500000000 | 0.0352740500000000 | 0.0013343000000000 | 1.0 |
| C19  | C  | 0.4582168800000000 | 0.9564795500000000 | 0.0023261500000000 | 1.0 |
| C20  | C  | 0.5788729900000000 | 0.9391897100000000 | 0.9607399000000000 | 1.0 |
| C21  | C  | 0.7060202600000000 | 0.0518594100000000 | 0.0029719700000000 | 1.0 |
| C22  | C  | 0.8266998300000000 | 0.0345510100000000 | 0.9614043900000000 | 1.0 |
| C23  | C  | 0.8282365700000000 | 0.9557541100000000 | 0.9624015300000000 | 1.0 |
| C24  | C  | 0.7042806500000000 | 0.9394434300000000 | 0.0035890900000000 | 1.0 |
| O25  | O  | 0.0887609700000000 | 0.9962961300000000 | 0.9152923000000000 | 1.0 |
| O26  | O  | 0.1961627900000000 | 0.9947759700000000 | 0.0485006000000000 | 1.0 |
| O27  | O  | 0.5889411800000000 | 0.9962052500000000 | 0.9152130100000000 | 1.0 |
| O28  | O  | 0.6959394700000000 | 0.9948503300000000 | 0.0484972800000000 | 1.0 |
| Br29 | Br | 0.0693506400000000 | 0.1339033000000000 | 0.9082763300000000 | 1.0 |
| Br30 | Br | 0.9542285400000000 | 0.0838808000000000 | 0.0863837300000000 | 1.0 |
| Br31 | Br | 0.3305953100000000 | 0.9070204900000000 | 0.8774627500000000 | 1.0 |
| Br32 | Br | 0.2155384700000000 | 0.8572241900000000 | 0.0556396800000000 | 1.0 |
| Br33 | Br | 0.5698881500000000 | 0.1337591400000000 | 0.9078044500000000 | 1.0 |
| Br34 | Br | 0.4544162800000000 | 0.0843036600000000 | 0.0860549600000000 | 1.0 |
| Br35 | Br | 0.8304900500000000 | 0.9066474900000000 | 0.8777167600000000 | 1.0 |
| Br36 | Br | 0.7149663100000000 | 0.8573036600000000 | 0.0559235300000000 | 1.0 |

##### cif ends

furan\_Br\_23\_anti\_dir Energy: -205.16135444

##### cif starts

data\_furan\_Br\_23\_anti\_dir

\_publ\_section\_comment

;

Andrew Reynoso, Bohan Xu, and Vincent H. Crespi

;

\_cell\_length\_a 9.8043717821

\_cell\_length\_b 20.0

\_cell\_length\_c 20.0

\_cell\_angle\_alpha 90.0

\_cell\_angle\_beta 90.0

\_cell\_angle\_gamma 90.0

\_symmetry\_space\_group\_name\_H-M 'P 1'

\_symmetry\_Int\_Tables\_number 1

\_symmetry\_cell\_setting triclinic

loop\_

\_atom\_site\_label

\_atom\_site\_type\_symbol

\_atom\_site\_fract\_x

|      |    | _atom_site_fract_x | _atom_site_fract_y | _atom_site_fract_z | _atom_site_occupancy |
|------|----|--------------------|--------------------|--------------------|----------------------|
| H1   | H  | 0.9641578000000000 | 0.1019210400000000 | 0.9356495100000000 | 1.0                  |
| H2   | H  | 0.9441486500000000 | 0.0678255600000000 | 0.0722952300000000 | 1.0                  |
| H3   | H  | 0.2141176200000000 | 0.1023477800000000 | 0.0596168600000000 | 1.0                  |
| H4   | H  | 0.1941731200000000 | 0.0672760500000000 | 0.9232130200000000 | 1.0                  |
| H5   | H  | 0.4641517100000000 | 0.1019166200000000 | 0.9356402600000000 | 1.0                  |
| H6   | H  | 0.4441716200000000 | 0.0678192700000000 | 0.0722875800000000 | 1.0                  |
| H7   | H  | 0.7140961100000000 | 0.1023525000000000 | 0.0596093900000000 | 1.0                  |
| H8   | H  | 0.6941768100000000 | 0.0672775000000000 | 0.9232066100000000 | 1.0                  |
| C9   | C  | 0.9886983900000000 | 0.0567181800000000 | 0.9642679300000000 | 1.0                  |
| C10  | C  | 0.9008365100000000 | 0.0448244700000000 | 0.0273180900000000 | 1.0                  |
| C11  | C  | 0.9069004400000000 | 0.9668685000000000 | 0.0316179800000000 | 1.0                  |
| C12  | C  | 0.9983582600000000 | 0.9477904300000000 | 0.9693740600000000 | 1.0                  |
| C13  | C  | 0.2386868300000000 | 0.0569464600000000 | 0.0313197100000000 | 1.0                  |
| C14  | C  | 0.1508465800000000 | 0.0446077400000000 | 0.9683560900000000 | 1.0                  |
| C15  | C  | 0.1568981600000000 | 0.9666243100000000 | 0.9646051100000000 | 1.0                  |
| C16  | C  | 0.2483617600000000 | 0.9479836300000000 | 0.0269799700000000 | 1.0                  |
| C17  | C  | 0.4886977400000000 | 0.0567152800000000 | 0.9642591600000000 | 1.0                  |
| C18  | C  | 0.4008458900000000 | 0.0448200400000000 | 0.0273132500000000 | 1.0                  |
| C19  | C  | 0.4069077900000000 | 0.9668639500000000 | 0.0316118200000000 | 1.0                  |
| C20  | C  | 0.4983652600000000 | 0.9477872800000000 | 0.9693662900000000 | 1.0                  |
| C21  | C  | 0.7386759500000000 | 0.0569492600000000 | 0.0313152100000000 | 1.0                  |
| C22  | C  | 0.6508458800000000 | 0.0446080100000000 | 0.9683491800000000 | 1.0                  |
| C23  | C  | 0.6569038800000000 | 0.9666249500000000 | 0.9645994900000000 | 1.0                  |
| C24  | C  | 0.7483573100000000 | 0.9479869300000000 | 0.0269798600000000 | 1.0                  |
| O25  | O  | 0.9491048100000000 | 0.9991638000000000 | 0.9243738500000000 | 1.0                  |
| O26  | O  | 0.1990946700000000 | 0.9996667300000000 | 0.0716126100000000 | 1.0                  |
| O27  | O  | 0.4491069500000000 | 0.9991593700000000 | 0.9243667600000000 | 1.0                  |
| O28  | O  | 0.6990795000000000 | 0.9996710400000000 | 0.0716086400000000 | 1.0                  |
| Br29 | Br | 0.9545472500000000 | 0.9414683700000000 | 0.1246418800000000 | 1.0                  |
| Br30 | Br | 0.9629766600000000 | 0.8573210600000000 | 0.9385423800000000 | 1.0                  |
| Br31 | Br | 0.2045572400000000 | 0.9405819500000000 | 0.8717608800000000 | 1.0                  |
| Br32 | Br | 0.2129925300000000 | 0.8577248200000000 | 0.0584576100000000 | 1.0                  |
| Br33 | Br | 0.4545524700000000 | 0.9414652900000000 | 0.1246376300000000 | 1.0                  |
| Br34 | Br | 0.4629964200000000 | 0.8573169900000000 | 0.9385312200000000 | 1.0                  |
| Br35 | Br | 0.7045714900000000 | 0.9405871000000000 | 0.8717541700000000 | 1.0                  |
| Br36 | Br | 0.7129856400000000 | 0.8577288500000000 | 0.0584606400000000 | 1.0                  |

##### cif ends

furan\_Br\_23\_anti\_dir\_forbid Energy: -205.4716262

##### cif starts

data\_furan\_Br\_23\_anti\_dir\_forbid

\_publ\_section\_comment

;  
Andrew Reynoso, Bohan Xu, and Vincent H. Crespi  
;

\_cell\_length\_a 10.5578169344

\_cell\_length\_b 20.0

\_cell\_length\_c 20.0

\_cell\_angle\_alpha 90.0

\_cell\_angle\_beta 90.0  
\_cell\_angle\_gamma 90.0

\_symmetry\_space\_group\_name H-M 'P 1'  
\_symmetry\_Int\_Tables\_number 1  
\_symmetry\_cell\_setting triclinic

loop\_  
\_atom\_site\_label  
\_atom\_site\_type\_symbol  
\_atom\_site\_fract\_x  
\_atom\_site\_fract\_y  
\_atom\_site\_fract\_z  
\_atom\_site\_occupancy

|      |    |                    |                    |                    |     |
|------|----|--------------------|--------------------|--------------------|-----|
| H1   | H  | 0.1187579000000000 | 0.1279287300000000 | 0.9350220900000000 | 1.0 |
| H2   | H  | 0.0001447600000000 | 0.0943715100000000 | 0.0579973600000000 | 1.0 |
| H3   | H  | 0.8674605800000000 | 0.0939410400000000 | 0.9226459000000000 | 1.0 |
| H4   | H  | 0.7488279500000000 | 0.1282430700000000 | 0.0453949000000000 | 1.0 |
| H5   | H  | 0.2488263300000000 | 0.1282734200000000 | 0.0454086200000000 | 1.0 |
| H6   | H  | 0.3674945800000000 | 0.0939897200000000 | 0.9226606100000000 | 1.0 |
| H7   | H  | 0.6188360000000000 | 0.1278645800000000 | 0.9349799300000000 | 1.0 |
| H8   | H  | 0.5002316600000000 | 0.0944112100000000 | 0.0579972700000000 | 1.0 |
| C9   | C  | 0.1223784600000000 | 0.0839771200000000 | 0.9679980200000000 | 1.0 |
| C10  | C  | 0.9997227200000000 | 0.0703826300000000 | 0.0087368500000000 | 1.0 |
| C11  | C  | 0.9996597800000000 | 0.9920171900000000 | 0.0115602700000000 | 1.0 |
| C12  | C  | 0.1199505700000000 | 0.9703797700000000 | 0.9703290300000000 | 1.0 |
| C13  | C  | 0.2452488800000000 | 0.0841212400000000 | 0.0126997000000000 | 1.0 |
| C14  | C  | 0.3679261700000000 | 0.0702940200000000 | 0.9720619400000000 | 1.0 |
| C15  | C  | 0.3679993900000000 | 0.9919155500000000 | 0.9697186100000000 | 1.0 |
| C16  | C  | 0.2476862400000000 | 0.9705142800000000 | 0.0110490700000000 | 1.0 |
| C17  | C  | 0.7476815800000000 | 0.9704792900000000 | 0.0110821200000000 | 1.0 |
| C18  | C  | 0.8679822200000000 | 0.9918720000000000 | 0.9697238500000000 | 1.0 |
| C19  | C  | 0.6224015100000000 | 0.0839384100000000 | 0.9679898100000000 | 1.0 |
| C20  | C  | 0.4997481900000000 | 0.0704007400000000 | 0.0087437400000000 | 1.0 |
| C21  | C  | 0.4996433300000000 | 0.9920368400000000 | 0.0115888600000000 | 1.0 |
| C22  | C  | 0.6199192300000000 | 0.9703470200000000 | 0.9703810900000000 | 1.0 |
| C23  | C  | 0.7452542300000000 | 0.0840850800000000 | 0.0126959000000000 | 1.0 |
| C24  | C  | 0.8679069200000000 | 0.0702527100000000 | 0.9720533900000000 | 1.0 |
| O25  | O  | 0.1300062600000000 | 0.0256513100000000 | 0.9245948500000000 | 1.0 |
| O26  | O  | 0.2376008000000000 | 0.0260584500000000 | 0.0564469200000000 | 1.0 |
| O27  | O  | 0.6300002500000000 | 0.0255922000000000 | 0.9246166300000000 | 1.0 |
| O28  | O  | 0.7376175900000000 | 0.0260374200000000 | 0.0564636100000000 | 1.0 |
| Br29 | Br | 0.0004159700000000 | 0.9653137700000000 | 0.1062867000000000 | 1.0 |
| Br30 | Br | 0.1026455000000000 | 0.8841537500000000 | 0.9242038900000000 | 1.0 |
| Br31 | Br | 0.3672793000000000 | 0.9646478600000000 | 0.8751634200000000 | 1.0 |
| Br32 | Br | 0.2649647800000000 | 0.8845750900000000 | 0.0577048300000000 | 1.0 |
| Br33 | Br | 0.5003590900000000 | 0.9653481700000000 | 0.1063168900000000 | 1.0 |
| Br34 | Br | 0.7649562300000000 | 0.8845492300000000 | 0.0577634700000000 | 1.0 |
| Br35 | Br | 0.8671446700000000 | 0.9645596400000000 | 0.8751798200000000 | 1.0 |
| Br36 | Br | 0.6024898600000000 | 0.8840839500000000 | 0.9243289600000000 | 1.0 |

##### cif ends

furan\_Br\_23\_syn\_alt Energy: -209.64845034  
##### cif starts

data\_furan\_Br\_23\_syn\_alt

\_publ\_section\_comment

;  
Andrew Reynoso, Bohan Xu, and Vincent H. Crespi  
;

\_cell\_length\_a 10.4004989127

\_cell\_length\_b 20.0

\_cell\_length\_c 20.0

\_cell\_angle\_alpha 90.0

\_cell\_angle\_beta 90.0

\_cell\_angle\_gamma 90.0

\_symmetry\_space\_group\_name\_H-M 'P 1'

\_symmetry\_Int\_Tables\_number 1

\_symmetry\_cell\_setting triclinic

loop\_

\_atom\_site\_label

\_atom\_site\_type\_symbol

\_atom\_site\_fract\_x

\_atom\_site\_fract\_y

\_atom\_site\_fract\_z

\_atom\_site\_occupancy

|      |    |                    |                    |                    |     |
|------|----|--------------------|--------------------|--------------------|-----|
| H1   | H  | 0.9730063100000000 | 0.8928375900000000 | 0.0474322000000000 | 1.0 |
| H2   | H  | 0.0976658000000000 | 0.9290571100000000 | 0.9291255200000000 | 1.0 |
| H3   | H  | 0.2229911500000000 | 0.0949031400000000 | 0.0433053800000000 | 1.0 |
| H4   | H  | 0.3476848200000000 | 0.0539128600000000 | 0.9265823800000000 | 1.0 |
| H5   | H  | 0.4729919600000000 | 0.8927606900000000 | 0.0472642400000000 | 1.0 |
| H6   | H  | 0.5977328800000000 | 0.9290891000000000 | 0.9290246800000000 | 1.0 |
| H7   | H  | 0.7230171800000000 | 0.0948577800000000 | 0.0433018100000000 | 1.0 |
| H8   | H  | 0.8476513200000000 | 0.0538417100000000 | 0.9265469700000000 | 1.0 |
| C9   | C  | 0.9740221200000000 | 0.9399202300000000 | 0.0196304000000000 | 1.0 |
| C10  | C  | 0.0973817300000000 | 0.9529766400000000 | 0.9782326800000000 | 1.0 |
| C11  | C  | 0.0989622200000000 | 0.0315821400000000 | 0.9769448100000000 | 1.0 |
| C12  | C  | 0.9720564500000000 | 0.0472521200000000 | 0.0170813100000000 | 1.0 |
| C13  | C  | 0.2240255800000000 | 0.0467236700000000 | 0.0174506500000000 | 1.0 |
| C14  | C  | 0.3473875000000000 | 0.0319931700000000 | 0.9766139800000000 | 1.0 |
| C15  | C  | 0.3489217400000000 | 0.9533992500000000 | 0.9784927500000000 | 1.0 |
| C16  | C  | 0.2220727700000000 | 0.9393760400000000 | 0.0192995600000000 | 1.0 |
| C17  | C  | 0.4740203000000000 | 0.9398787800000000 | 0.0195262300000000 | 1.0 |
| C18  | C  | 0.5973936200000000 | 0.9529695100000000 | 0.9781512800000000 | 1.0 |
| C19  | C  | 0.5989641200000000 | 0.0315755100000000 | 0.9769313300000000 | 1.0 |
| C20  | C  | 0.4720815000000000 | 0.0472140800000000 | 0.0171082900000000 | 1.0 |
| C21  | C  | 0.7240259800000000 | 0.0466879700000000 | 0.0174340200000000 | 1.0 |
| C22  | C  | 0.8473853600000000 | 0.0319605200000000 | 0.9765954900000000 | 1.0 |
| C23  | C  | 0.8489674100000000 | 0.9533705100000000 | 0.9785240500000000 | 1.0 |
| C24  | C  | 0.7220547900000000 | 0.9393414600000000 | 0.0192549300000000 | 1.0 |
| O25  | O  | 0.9731049900000000 | 0.9954498400000000 | 0.0660515700000000 | 1.0 |
| O26  | O  | 0.2231462200000000 | 0.9931453400000000 | 0.0661009200000000 | 1.0 |
| O27  | O  | 0.4731417000000000 | 0.9953489600000000 | 0.0660147100000000 | 1.0 |
| O28  | O  | 0.7231087000000000 | 0.9930957900000000 | 0.0660737600000000 | 1.0 |
| Br29 | Br | 0.0990638300000000 | 0.0741168000000000 | 0.8886805500000000 | 1.0 |
| Br30 | Br | 0.9730007100000000 | 0.1348119200000000 | 0.0595779900000000 | 1.0 |

|      |    |                    |                    |                    |     |
|------|----|--------------------|--------------------|--------------------|-----|
| Br31 | Br | 0.3488690100000000 | 0.9073896100000000 | 0.8919816000000000 | 1.0 |
| Br32 | Br | 0.2231136300000000 | 0.8536833400000000 | 0.0654381600000000 | 1.0 |
| Br33 | Br | 0.5990498500000000 | 0.0741791000000000 | 0.8887003200000000 | 1.0 |
| Br34 | Br | 0.4730961800000000 | 0.1347046700000000 | 0.0597390700000000 | 1.0 |
| Br35 | Br | 0.8491085200000000 | 0.9072957700000000 | 0.8920456800000000 | 1.0 |
| Br36 | Br | 0.7230180900000000 | 0.8536181100000000 | 0.0653368900000000 | 1.0 |

##### cif ends

furan\_Br\_23\_syn\_alt\_forbid Energy: -206.48454169

##### cif starts

data\_furan\_Br\_23\_syn\_alt\_forbid

\_publ\_section\_comment

;  
Andrew Reynoso, Bohan Xu, and Vincent H. Crespi  
;

\_cell\_length\_a 9.6809603631

\_cell\_length\_b 20.0

\_cell\_length\_c 20.0

\_cell\_angle\_alpha 90.0

\_cell\_angle\_beta 90.0

\_cell\_angle\_gamma 90.0

\_symmetry\_space\_group\_name\_H-M 'P 1'

\_symmetry\_Int\_Tables\_number 1

\_symmetry\_cell\_setting triclinic

loop\_

\_atom\_site\_label

\_atom\_site\_type\_symbol

\_atom\_site\_fract\_x

\_atom\_site\_fract\_y

\_atom\_site\_fract\_z

\_atom\_site\_occupancy

|     |   |                    |                    |                    |     |
|-----|---|--------------------|--------------------|--------------------|-----|
| H1  | H | 0.9995521700000000 | 0.0950937000000000 | 0.0613209600000000 | 1.0 |
| H2  | H | 0.0009073900000000 | 0.0598491500000000 | 0.9259004400000000 | 1.0 |
| H3  | H | 0.2516918700000000 | 0.9315356100000000 | 0.9292869100000000 | 1.0 |
| H4  | H | 0.2531930900000000 | 0.9035004100000000 | 0.0663733600000000 | 1.0 |
| H5  | H | 0.4995397800000000 | 0.0950059200000000 | 0.0614211400000000 | 1.0 |
| H6  | H | 0.5009808500000000 | 0.0598916100000000 | 0.9259544100000000 | 1.0 |
| H7  | H | 0.7517692700000000 | 0.9315222200000000 | 0.9292530500000000 | 1.0 |
| H8  | H | 0.7531353400000000 | 0.9033988000000000 | 0.0663117000000000 | 1.0 |
| C9  | C | 0.0368680100000000 | 0.0512305500000000 | 0.0343347700000000 | 1.0 |
| C10 | C | 0.9581879600000000 | 0.0354554300000000 | 0.9700834200000000 | 1.0 |
| C11 | C | 0.9586444400000000 | 0.9572143900000000 | 0.9705180200000000 | 1.0 |
| C12 | C | 0.0478191400000000 | 0.9408888200000000 | 0.0340140500000000 | 1.0 |
| C13 | C | 0.2048687400000000 | 0.0560465000000000 | 0.0309564600000000 | 1.0 |
| C14 | C | 0.2940357100000000 | 0.0363825400000000 | 0.9684299200000000 | 1.0 |
| C15 | C | 0.2944705600000000 | 0.9582311500000000 | 0.9721073900000000 | 1.0 |
| C16 | C | 0.2158394000000000 | 0.9458786400000000 | 0.0371205400000000 | 1.0 |
| C17 | C | 0.5368502100000000 | 0.0511692800000000 | 0.0343871800000000 | 1.0 |
| C18 | C | 0.4581981800000000 | 0.0354684300000000 | 0.9701048100000000 | 1.0 |
| C19 | C | 0.4586288800000000 | 0.9572277400000000 | 0.9704835700000000 | 1.0 |

|      |    |                    |                    |                    |     |
|------|----|--------------------|--------------------|--------------------|-----|
| C20  | C  | 0.5477982200000000 | 0.9408270900000000 | 0.0339536800000000 | 1.0 |
| C21  | C  | 0.7048661100000000 | 0.0559759200000000 | 0.0310083000000000 | 1.0 |
| C22  | C  | 0.7940183400000000 | 0.0363554400000000 | 0.9684500500000000 | 1.0 |
| C23  | C  | 0.7944821400000000 | 0.9582004000000000 | 0.9720992300000000 | 1.0 |
| C24  | C  | 0.7158054200000000 | 0.9457999700000000 | 0.0370841600000000 | 1.0 |
| O25  | O  | 0.0080860900000000 | 0.9939553900000000 | 0.0764197500000000 | 1.0 |
| O26  | O  | 0.2446067600000000 | 0.0053069600000000 | 0.0761153600000000 | 1.0 |
| O27  | O  | 0.5080598900000000 | 0.9938476900000000 | 0.0764133300000000 | 1.0 |
| O28  | O  | 0.7445888000000000 | 0.0051945800000000 | 0.0761256900000000 | 1.0 |
| Br29 | Br | 0.0132976000000000 | 0.9090948700000000 | 0.8888825000000000 | 1.0 |
| Br30 | Br | 0.9997842100000000 | 0.8539916400000000 | 0.0734850400000000 | 1.0 |
| Br31 | Br | 0.2528875400000000 | 0.1449325800000000 | 0.0657127600000000 | 1.0 |
| Br32 | Br | 0.2393708100000000 | 0.0801702800000000 | 0.8843985200000000 | 1.0 |
| Br33 | Br | 0.5132361700000000 | 0.9091812600000000 | 0.8888020100000000 | 1.0 |
| Br34 | Br | 0.4996993200000000 | 0.8538802700000000 | 0.0732955500000000 | 1.0 |
| Br35 | Br | 0.7529199700000000 | 0.1448209000000000 | 0.0658581400000000 | 1.0 |
| Br36 | Br | 0.7393008400000000 | 0.0801780700000000 | 0.8844429500000000 | 1.0 |

##### cif ends

furandir23\_syn\_dir\_break Energy: -203.13042771

##### cif starts

data\_furandir23\_syn\_dir\_break

\_publ\_section\_comment

;  
Andrew Reynoso, Bohan Xu, and Vincent H. Crespi  
;

\_cell\_length\_a 10.4751111504

\_cell\_length\_b 20.0

\_cell\_length\_c 20.0

\_cell\_angle\_alpha 90.0

\_cell\_angle\_beta 90.0

\_cell\_angle\_gamma 90.0

\_symmetry\_space\_group\_name\_H-M 'P 1'

\_symmetry\_Int\_Tables\_number 1

\_symmetry\_cell\_setting triclinic

loop\_

\_atom\_site\_label

\_atom\_site\_type\_symbol

\_atom\_site\_fract\_x

\_atom\_site\_fract\_y

\_atom\_site\_fract\_z

\_atom\_site\_occupancy

|    |   |                    |                    |                    |     |
|----|---|--------------------|--------------------|--------------------|-----|
| H1 | H | 0.9963931500000000 | 0.8733787900000000 | 0.9764796900000000 | 1.0 |
|----|---|--------------------|--------------------|--------------------|-----|

|    |   |                    |                    |                    |     |
|----|---|--------------------|--------------------|--------------------|-----|
| H2 | H | 0.1381516400000000 | 0.9286318300000000 | 0.0768632700000000 | 1.0 |
|----|---|--------------------|--------------------|--------------------|-----|

|    |   |                    |                    |                    |     |
|----|---|--------------------|--------------------|--------------------|-----|
| H3 | H | 0.2461463600000000 | 0.9008707800000000 | 0.9459909800000000 | 1.0 |
|----|---|--------------------|--------------------|--------------------|-----|

|    |   |                    |                    |                    |     |
|----|---|--------------------|--------------------|--------------------|-----|
| H4 | H | 0.3632347200000000 | 0.9205138200000000 | 0.0720224500000000 | 1.0 |
|----|---|--------------------|--------------------|--------------------|-----|

|    |   |                    |                    |                    |     |
|----|---|--------------------|--------------------|--------------------|-----|
| H5 | H | 0.4891654900000000 | 0.8944192900000000 | 0.9503437900000000 | 1.0 |
|----|---|--------------------|--------------------|--------------------|-----|

|    |   |                    |                    |                    |     |
|----|---|--------------------|--------------------|--------------------|-----|
| H6 | H | 0.6109135600000000 | 0.9162573200000000 | 0.0759927300000000 | 1.0 |
|----|---|--------------------|--------------------|--------------------|-----|

|    |   |                    |                    |                    |     |
|----|---|--------------------|--------------------|--------------------|-----|
| H7 | H | 0.7525181800000000 | 0.8791607300000000 | 0.9643954200000000 | 1.0 |
|----|---|--------------------|--------------------|--------------------|-----|

|    |   |                    |                    |                    |     |
|----|---|--------------------|--------------------|--------------------|-----|
| H8 | H | 0.8683831400000000 | 0.9386810700000000 | 0.0822176700000000 | 1.0 |
|----|---|--------------------|--------------------|--------------------|-----|



|      |    |                    |                    |                    |     |
|------|----|--------------------|--------------------|--------------------|-----|
| C9   | C  | 0.9972918000000000 | 0.9259282300000000 | 0.9925393700000000 | 1.0 |
| C10  | C  | 0.1234757000000000 | 0.9487650000000000 | 0.0264666600000000 | 1.0 |
| C11  | C  | 0.1109545600000000 | 0.0260035300000000 | 0.0252566600000000 | 1.0 |
| C12  | C  | 0.9928623200000000 | 0.0315486400000000 | 0.9677561000000000 | 1.0 |
| C13  | C  | 0.2461148500000000 | 0.9426207100000000 | 0.9815369500000000 | 1.0 |
| C14  | C  | 0.3686252600000000 | 0.9492355800000000 | 0.0253952700000000 | 1.0 |
| C15  | C  | 0.3702660300000000 | 0.0275543000000000 | 0.0371451200000000 | 1.0 |
| C16  | C  | 0.2435996000000000 | 0.0495278700000000 | 0.9983677100000000 | 1.0 |
| C17  | C  | 0.4934746000000000 | 0.9372987600000000 | 0.9845349700000000 | 1.0 |
| C18  | C  | 0.6183878900000000 | 0.9418704200000000 | 0.0277239400000000 | 1.0 |
| C19  | C  | 0.6282409800000000 | 0.0197300600000000 | 0.0343489300000000 | 1.0 |
| C20  | C  | 0.5012064000000000 | 0.0445428300000000 | 0.9992115700000000 | 1.0 |
| C21  | C  | 0.7452554400000000 | 0.9280669500000000 | 0.9890672200000000 | 1.0 |
| C22  | C  | 0.8724289200000000 | 0.9494660300000000 | 0.0284987800000000 | 1.0 |
| C23  | C  | 0.8721092100000000 | 0.0292906000000000 | 0.0109650100000000 | 1.0 |
| C24  | C  | 0.7418074100000000 | 0.0325599900000000 | 0.9842679300000000 | 1.0 |
| O25  | O  | 0.9993499100000000 | 0.9681534500000000 | 0.9347726900000000 | 1.0 |
| O26  | O  | 0.2475780900000000 | 0.0049040000000000 | 0.9424856300000000 | 1.0 |
| O27  | O  | 0.4970241700000000 | 0.9980484200000000 | 0.9453185400000000 | 1.0 |
| O28  | O  | 0.7356977300000000 | 0.9799340400000000 | 0.9378467800000000 | 1.0 |
| Br29 | Br | 0.0589483000000000 | 0.0593743200000000 | 0.1134357200000000 | 1.0 |
| Br30 | Br | 0.9913204600000000 | 0.0939068200000000 | 0.8936958800000000 | 1.0 |
| Br31 | Br | 0.3648193100000000 | 0.0562497200000000 | 0.1301609300000000 | 1.0 |
| Br32 | Br | 0.2373184000000000 | 0.1448158300000000 | 0.9818375400000000 | 1.0 |
| Br33 | Br | 0.6692553200000000 | 0.0432342600000000 | 0.1268962300000000 | 1.0 |
| Br34 | Br | 0.5392743900000000 | 0.1317790800000000 | 0.9622406200000000 | 1.0 |
| Br35 | Br | 0.8533728400000000 | 0.1370044100000000 | 0.0370423400000000 | 1.0 |
| Br36 | Br | 0.7638451400000000 | 0.2533914000000000 | 0.0076084600000000 | 1.0 |

##### cif ends

furan\_Br\_23\_syn\_dir\_forbid Energy: -201.78319705

##### cif starts

data\_furan\_Br\_23\_syn\_dir\_forbid

\_publ\_section\_comment

;

Andrew Reynoso, Bohan Xu, and Vincent H. Crespi

;

\_cell\_length\_a 9.834685794

\_cell\_length\_b 20.0

\_cell\_length\_c 20.0

\_cell\_angle\_alpha 90.0

\_cell\_angle\_beta 90.0

\_cell\_angle\_gamma 90.0

\_symmetry\_space\_group\_name\_H-M 'P 1'

\_symmetry\_Int\_Tables\_number 1

\_symmetry\_cell\_setting triclinic

loop\_

\_atom\_site\_label

\_atom\_site\_type\_symbol

\_atom\_site\_fract\_x

|      |    | _atom_site_fract_x | _atom_site_fract_y | _atom_site_fract_z | _atom_site_occupancy |
|------|----|--------------------|--------------------|--------------------|----------------------|
| H1   | H  | 0.0328567300000000 | 0.1066914300000000 | 0.0371000000000000 | 1.0                  |
| H2   | H  | 0.0025324200000000 | 0.0450470600000000 | 0.9134599400000000 | 1.0                  |
| H3   | H  | 0.2543771000000000 | 0.0862248400000000 | 0.0731057400000000 | 1.0                  |
| H4   | H  | 0.2699022900000000 | 0.0753875700000000 | 0.9330738100000000 | 1.0                  |
| H5   | H  | 0.5328090900000000 | 0.1066614900000000 | 0.0371294400000000 | 1.0                  |
| H6   | H  | 0.5026012300000000 | 0.0450185000000000 | 0.9134738700000000 | 1.0                  |
| H7   | H  | 0.7543493000000000 | 0.0862140500000000 | 0.0731283000000000 | 1.0                  |
| H8   | H  | 0.7698378500000000 | 0.0753965400000000 | 0.9330929700000000 | 1.0                  |
| C9   | C  | 0.0611551900000000 | 0.0552004300000000 | 0.0237595900000000 | 1.0                  |
| C10  | C  | 0.9707953700000000 | 0.0306731400000000 | 0.9639449600000000 | 1.0                  |
| C11  | C  | 0.9413954400000000 | 0.9523003400000000 | 0.9741154400000000 | 1.0                  |
| C12  | C  | 0.0230971300000000 | 0.9478479600000000 | 0.0421181500000000 | 1.0                  |
| C13  | C  | 0.2257121900000000 | 0.0481296500000000 | 0.0362836800000000 | 1.0                  |
| C14  | C  | 0.3089787600000000 | 0.0421593300000000 | 0.9721044200000000 | 1.0                  |
| C15  | C  | 0.2831189000000000 | 0.9668977800000000 | 0.9608202000000000 | 1.0                  |
| C16  | C  | 0.1899051600000000 | 0.9394882300000000 | 0.0216462400000000 | 1.0                  |
| C17  | C  | 0.5611431100000000 | 0.0551772500000000 | 0.0237805100000000 | 1.0                  |
| C18  | C  | 0.4708199600000000 | 0.0306518900000000 | 0.9639534700000000 | 1.0                  |
| C19  | C  | 0.4414035500000000 | 0.9522781600000000 | 0.9741212000000000 | 1.0                  |
| C20  | C  | 0.5231051500000000 | 0.9478196300000000 | 0.0421226000000000 | 1.0                  |
| C21  | C  | 0.7256929100000000 | 0.0481219400000000 | 0.0363022900000000 | 1.0                  |
| C22  | C  | 0.8089456300000000 | 0.0421683500000000 | 0.9721161900000000 | 1.0                  |
| C23  | C  | 0.7831090000000000 | 0.9669052500000000 | 0.9608245300000000 | 1.0                  |
| C24  | C  | 0.6899214100000000 | 0.9394778400000000 | 0.0216503400000000 | 1.0                  |
| O25  | O  | 0.0108622900000000 | 0.0111329500000000 | 0.0738513600000000 | 1.0                  |
| O26  | O  | 0.2452210900000000 | 0.9838778600000000 | 0.0698180900000000 | 1.0                  |
| O27  | O  | 0.5108578000000000 | 0.0110980300000000 | 0.0738642200000000 | 1.0                  |
| O28  | O  | 0.7452246200000000 | 0.9838666500000000 | 0.0698261000000000 | 1.0                  |
| Br29 | Br | 0.9938811100000000 | 0.8755649500000000 | 0.9183532600000000 | 1.0                  |
| Br30 | Br | 0.9893274100000000 | 0.8905234000000000 | 0.1193018500000000 | 1.0                  |
| Br31 | Br | 0.2446557800000000 | 0.9595033800000000 | 0.8642119500000000 | 1.0                  |
| Br32 | Br | 0.2359163500000000 | 0.8446215900000000 | 0.0306790400000000 | 1.0                  |
| Br33 | Br | 0.4938725700000000 | 0.8755321600000000 | 0.9183669700000000 | 1.0                  |
| Br34 | Br | 0.4893339500000000 | 0.8904750200000000 | 0.1192920100000000 | 1.0                  |
| Br35 | Br | 0.7446190700000000 | 0.9595114700000000 | 0.8642185200000000 | 1.0                  |
| Br36 | Br | 0.7359741500000000 | 0.8446164400000000 | 0.0306756600000000 | 1.0                  |

##### cif ends

furan\_Br\_24\_anti\_alt    Energy: -205.93583488

##### cif starts

data\_furan\_Br\_24\_anti\_alt

\_publ\_section\_comment

;  
Andrew Reynoso, Bohan Xu, and Vincent H. Crespi  
;

\_cell\_length\_a    9.6314908367

\_cell\_length\_b    20.0

\_cell\_length\_c    20.0

\_cell\_angle\_alpha    90.0

\_cell\_angle\_beta 90.0  
\_cell\_angle\_gamma 90.0

\_symmetry\_space\_group\_name H-M 'P 1'  
\_symmetry\_Int\_Tables\_number 1  
\_symmetry\_cell\_setting triclinic

loop\_  
\_atom\_site\_label  
\_atom\_site\_type\_symbol  
\_atom\_site\_fract\_x  
\_atom\_site\_fract\_y  
\_atom\_site\_fract\_z  
\_atom\_site\_occupancy

|      |    |                    |                    |                    |     |
|------|----|--------------------|--------------------|--------------------|-----|
| H1   | H  | 0.4952113400000000 | 0.9285492500000000 | 0.0702043400000000 | 1.0 |
| H2   | H  | 0.5158087300000000 | 0.1083193100000000 | 0.9616979900000000 | 1.0 |
| H3   | H  | 0.7452192100000000 | 0.0715252600000000 | 0.9321974500000000 | 1.0 |
| H4   | H  | 0.2658095800000000 | 0.8917501700000000 | 0.0407085300000000 | 1.0 |
| H5   | H  | 0.9951982700000000 | 0.9285276800000000 | 0.0701956800000000 | 1.0 |
| H6   | H  | 0.0157976300000000 | 0.1083102200000000 | 0.9617071900000000 | 1.0 |
| H7   | H  | 0.2452050300000000 | 0.0715194900000000 | 0.9321937300000000 | 1.0 |
| H8   | H  | 0.7657835100000000 | 0.8917458800000000 | 0.0406976900000000 | 1.0 |
| C9   | C  | 0.4543863500000000 | 0.9566287600000000 | 0.0275563000000000 | 1.0 |
| C10  | C  | 0.4540580500000000 | 0.0332371300000000 | 0.0394682500000000 | 1.0 |
| C11  | C  | 0.5431335400000000 | 0.0579928400000000 | 0.9787721200000000 | 1.0 |
| C12  | C  | 0.5430187900000000 | 0.9501518900000000 | 0.9643207000000000 | 1.0 |
| C13  | C  | 0.7930284100000000 | 0.0499066600000000 | 0.0380814400000000 | 1.0 |
| C14  | C  | 0.7043926400000000 | 0.0434370800000000 | 0.9748395300000000 | 1.0 |
| C15  | C  | 0.7040485000000000 | 0.9668276500000000 | 0.9629276300000000 | 1.0 |
| C16  | C  | 0.7931223600000000 | 0.9420677200000000 | 0.0236222500000000 | 1.0 |
| C17  | C  | 0.0430177900000000 | 0.9501431100000000 | 0.9643176300000000 | 1.0 |
| C18  | C  | 0.9543789800000000 | 0.9566149600000000 | 0.0275515600000000 | 1.0 |
| C19  | C  | 0.9540604200000000 | 0.0332213300000000 | 0.0394708100000000 | 1.0 |
| C20  | C  | 0.0431312300000000 | 0.0579835500000000 | 0.9787748100000000 | 1.0 |
| C21  | C  | 0.2930192300000000 | 0.0499121900000000 | 0.0380799400000000 | 1.0 |
| C22  | C  | 0.2043874100000000 | 0.0434330900000000 | 0.9748381500000000 | 1.0 |
| C23  | C  | 0.2040527700000000 | 0.9668224400000000 | 0.9629304200000000 | 1.0 |
| C24  | C  | 0.2931332200000000 | 0.9420722500000000 | 0.0236283900000000 | 1.0 |
| O25  | O  | 0.9945079600000000 | 0.0097056300000000 | 0.9287010000000000 | 1.0 |
| O26  | O  | 0.7445128000000000 | 0.9903453900000000 | 0.0736920700000000 | 1.0 |
| O27  | O  | 0.4945070700000000 | 0.0097127000000000 | 0.9287010300000000 | 1.0 |
| O28  | O  | 0.2445198200000000 | 0.9903513200000000 | 0.0736941600000000 | 1.0 |
| Br29 | Br | 0.5107009900000000 | 0.8592129300000000 | 0.9304551500000000 | 1.0 |
| Br30 | Br | 0.5032041400000000 | 0.0506149200000000 | 0.1344960400000000 | 1.0 |
| Br31 | Br | 0.7607221500000000 | 0.1408309900000000 | 0.0719727700000000 | 1.0 |
| Br32 | Br | 0.2531389500000000 | 0.9493852800000000 | 0.8679032800000000 | 1.0 |
| Br33 | Br | 0.0106943300000000 | 0.8592105000000000 | 0.9304403100000000 | 1.0 |
| Br34 | Br | 0.0031941200000000 | 0.0505801400000000 | 0.1345053900000000 | 1.0 |
| Br35 | Br | 0.2606579800000000 | 0.1408304700000000 | 0.0719736600000000 | 1.0 |
| Br36 | Br | 0.7531217200000000 | 0.9493938100000000 | 0.8678985800000000 | 1.0 |

##### cif ends

furan\_Br\_24\_anti\_alt\_forbid Energy: -206.84323351  
##### cif starts

data\_furan\_Br\_24\_anti\_alt\_forbid

\_publ\_section\_comment

;  
Andrew Reynoso, Bohan Xu, and Vincent H. Crespi  
;

\_cell\_length\_a 10.427333158

\_cell\_length\_b 20.0

\_cell\_length\_c 20.0

\_cell\_angle\_alpha 90.0

\_cell\_angle\_beta 90.0

\_cell\_angle\_gamma 90.0

\_symmetry\_space\_group\_name\_H-M 'P 1'

\_symmetry\_Int\_Tables\_number 1

\_symmetry\_cell\_setting triclinic

loop\_

\_atom\_site\_label

\_atom\_site\_type\_symbol

\_atom\_site\_fract\_x

\_atom\_site\_fract\_y

\_atom\_site\_fract\_z

\_atom\_site\_occupancy

|      |    |                    |                    |                    |     |
|------|----|--------------------|--------------------|--------------------|-----|
| H1   | H  | 0.0639135400000000 | 0.8964384000000000 | 0.9287059100000000 | 1.0 |
| H2   | H  | 0.9451201600000000 | 0.0633886100000000 | 0.0476808900000000 | 1.0 |
| H3   | H  | 0.2212834900000000 | 0.0934139000000000 | 0.0353654200000000 | 1.0 |
| H4   | H  | 0.3401174500000000 | 0.9264898300000000 | 0.9163724600000000 | 1.0 |
| H5   | H  | 0.5635793500000000 | 0.8963785100000000 | 0.9291429800000000 | 1.0 |
| H6   | H  | 0.4456588400000000 | 0.0639639500000000 | 0.0474576600000000 | 1.0 |
| H7   | H  | 0.7216855300000000 | 0.0935971800000000 | 0.0348722200000000 | 1.0 |
| H8   | H  | 0.8394538500000000 | 0.9259564800000000 | 0.9165706900000000 | 1.0 |
| C9   | C  | 0.0802587400000000 | 0.0529728800000000 | 0.9629815000000000 | 1.0 |
| C10  | C  | 0.9558124000000000 | 0.0365678300000000 | 0.0002715800000000 | 1.0 |
| C11  | C  | 0.9579267500000000 | 0.9584704700000000 | 0.0051836100000000 | 1.0 |
| C12  | C  | 0.0779415800000000 | 0.9405056500000000 | 0.9604378300000000 | 1.0 |
| C13  | C  | 0.2072540400000000 | 0.0493528800000000 | 0.0036266400000000 | 1.0 |
| C14  | C  | 0.3272451600000000 | 0.0314112900000000 | 0.9588530500000000 | 1.0 |
| C15  | C  | 0.3293958600000000 | 0.9533115000000000 | 0.9637828100000000 | 1.0 |
| C16  | C  | 0.2049545500000000 | 0.9368891100000000 | 0.0010850700000000 | 1.0 |
| C17  | C  | 0.5804467400000000 | 0.0530273600000000 | 0.9626937500000000 | 1.0 |
| C18  | C  | 0.4559291900000000 | 0.0369683900000000 | 0.0001206000000000 | 1.0 |
| C19  | C  | 0.4578393900000000 | 0.9588719500000000 | 0.0052655000000000 | 1.0 |
| C20  | C  | 0.5777987800000000 | 0.9405778800000000 | 0.9606604200000000 | 1.0 |
| C21  | C  | 0.7074183700000000 | 0.0493786000000000 | 0.0033831000000000 | 1.0 |
| C22  | C  | 0.8273695900000000 | 0.0310620100000000 | 0.9587791200000000 | 1.0 |
| C23  | C  | 0.8292427700000000 | 0.9529555600000000 | 0.9639113600000000 | 1.0 |
| C24  | C  | 0.7047389500000000 | 0.9369283200000000 | 0.0013608100000000 | 1.0 |
| O25  | O  | 0.0862740500000000 | 0.9982046300000000 | 0.9160057200000000 | 1.0 |
| O26  | O  | 0.1989471200000000 | 0.9916505100000000 | 0.0480536200000000 | 1.0 |
| O27  | O  | 0.5862034500000000 | 0.9980616100000000 | 0.9159478000000000 | 1.0 |
| O28  | O  | 0.6990184700000000 | 0.9919045600000000 | 0.0481005600000000 | 1.0 |
| Br29 | Br | 0.0738321600000000 | 0.1445127500000000 | 0.9265638600000000 | 1.0 |
| Br30 | Br | 0.9575265700000000 | 0.9284109800000000 | 0.0985691700000000 | 1.0 |

|      |    |                    |                    |                    |     |
|------|----|--------------------|--------------------|--------------------|-----|
| Br31 | Br | 0.3276025000000000 | 0.0614808500000000 | 0.8654763700000000 | 1.0 |
| Br32 | Br | 0.2114206100000000 | 0.8453864600000000 | 0.0375852800000000 | 1.0 |
| Br33 | Br | 0.5748994800000000 | 0.1443686900000000 | 0.9257748300000000 | 1.0 |
| Br34 | Br | 0.4568968400000000 | 0.9292682800000000 | 0.0987956000000000 | 1.0 |
| Br35 | Br | 0.8283613500000000 | 0.0607521800000000 | 0.8652762500000000 | 1.0 |
| Br36 | Br | 0.7101865200000000 | 0.8455956500000000 | 0.0382995000000000 | 1.0 |

##### cif ends

uran\_Br\_24\_anti\_dir Energy: -208.40716986

##### cif starts

data\_uran\_Br\_24\_anti\_dir

\_publ\_section\_comment

;  
Andrew Reynoso, Bohan Xu, and Vincent H. Crespi  
;

\_cell\_length\_a 9.5185782734

\_cell\_length\_b 20.0

\_cell\_length\_c 20.0

\_cell\_angle\_alpha 90.0

\_cell\_angle\_beta 90.0

\_cell\_angle\_gamma 90.0

\_symmetry\_space\_group\_name\_H-M 'P 1'

\_symmetry\_Int\_Tables\_number 1

\_symmetry\_cell\_setting triclinic

loop\_

\_atom\_site\_label

\_atom\_site\_type\_symbol

\_atom\_site\_fract\_x

\_atom\_site\_fract\_y

\_atom\_site\_fract\_z

\_atom\_site\_occupancy

|     |   |                    |                    |                    |     |
|-----|---|--------------------|--------------------|--------------------|-----|
| H1  | H | 0.4810662400000000 | 0.0622423700000000 | 0.0720907600000000 | 1.0 |
| H2  | H | 0.4972384000000000 | 0.8993361900000000 | 0.9401885000000000 | 1.0 |
| H3  | H | 0.7310669600000000 | 0.0628078500000000 | 0.9188419200000000 | 1.0 |
| H4  | H | 0.2472579600000000 | 0.8989230800000000 | 0.0495400500000000 | 1.0 |
| H5  | H | 0.9810852000000000 | 0.0622355300000000 | 0.0720810800000000 | 1.0 |
| H6  | H | 0.9972469100000000 | 0.8993253100000000 | 0.9401883200000000 | 1.0 |
| H7  | H | 0.2310787600000000 | 0.0627931100000000 | 0.9188377900000000 | 1.0 |
| H8  | H | 0.7472473200000000 | 0.8989215600000000 | 0.0495267000000000 | 1.0 |
| C9  | C | 0.4354196100000000 | 0.0409326100000000 | 0.0266607700000000 | 1.0 |
| C10 | C | 0.4332803500000000 | 0.9626001100000000 | 0.0259825500000000 | 1.0 |
| C11 | C | 0.5214319300000000 | 0.9473223700000000 | 0.9634026500000000 | 1.0 |
| C12 | C | 0.5221599500000000 | 0.0556163900000000 | 0.9625969200000000 | 1.0 |
| C13 | C | 0.7721744700000000 | 0.0553684600000000 | 0.0282807500000000 | 1.0 |
| C14 | C | 0.6854254800000000 | 0.0411573100000000 | 0.9641132500000000 | 1.0 |
| C15 | C | 0.6832771000000000 | 0.9628231100000000 | 0.9642173700000000 | 1.0 |
| C16 | C | 0.7714324900000000 | 0.9470858200000000 | 0.0266813500000000 | 1.0 |
| C17 | C | 0.0221649900000000 | 0.0556071300000000 | 0.9625881800000000 | 1.0 |
| C18 | C | 0.9354257000000000 | 0.0409271500000000 | 0.0266533000000000 | 1.0 |
| C19 | C | 0.9332783400000000 | 0.9625948300000000 | 0.0259764600000000 | 1.0 |

|      |    |                    |                    |                    |     |
|------|----|--------------------|--------------------|--------------------|-----|
| C20  | C  | 0.0214355300000000 | 0.9473130900000000 | 0.9634007200000000 | 1.0 |
| C21  | C  | 0.2721659500000000 | 0.0553682500000000 | 0.0282803900000000 | 1.0 |
| C22  | C  | 0.1854297700000000 | 0.0411489600000000 | 0.9641099900000000 | 1.0 |
| C23  | C  | 0.1832819400000000 | 0.9628144800000000 | 0.9642216900000000 | 1.0 |
| C24  | C  | 0.2714351200000000 | 0.9470855500000000 | 0.0266888400000000 | 1.0 |
| O25  | O  | 0.9763867400000000 | 0.0016466600000000 | 0.9198716700000000 | 1.0 |
| O26  | O  | 0.7263907400000000 | 0.0010984700000000 | 0.0706129200000000 | 1.0 |
| O27  | O  | 0.4763754000000000 | 0.0016588700000000 | 0.9198783700000000 | 1.0 |
| O28  | O  | 0.2263834700000000 | 0.0011003000000000 | 0.0706151100000000 | 1.0 |
| Br29 | Br | 0.4815998600000000 | 0.1405491200000000 | 0.9193632400000000 | 1.0 |
| Br30 | Br | 0.4928377000000000 | 0.9151390200000000 | 0.1087017000000000 | 1.0 |
| Br31 | Br | 0.7316051200000000 | 0.1399941000000000 | 0.0721026300000000 | 1.0 |
| Br32 | Br | 0.2428666900000000 | 0.9159077200000000 | 0.8811869900000000 | 1.0 |
| Br33 | Br | 0.9816051100000000 | 0.1405366200000000 | 0.9193501500000000 | 1.0 |
| Br34 | Br | 0.9928291600000000 | 0.9151328200000000 | 0.1086960100000000 | 1.0 |
| Br35 | Br | 0.2315815400000000 | 0.1399974200000000 | 0.0720944000000000 | 1.0 |
| Br36 | Br | 0.7428520200000000 | 0.9159252400000000 | 0.8811765500000000 | 1.0 |

##### cif ends

furan\_Br\_24\_anti\_dir\_forbid Energy: -209.30819875

##### cif starts

data\_furan\_Br\_24\_anti\_dir\_forbid

\_publ\_section\_comment

;  
Andrew Reynoso, Bohan Xu, and Vincent H. Crespi  
;

\_cell\_length\_a 10.2916368526

\_cell\_length\_b 20.0

\_cell\_length\_c 20.0

\_cell\_angle\_alpha 90.0

\_cell\_angle\_beta 90.0

\_cell\_angle\_gamma 90.0

\_symmetry\_space\_group\_name\_H-M 'P 1'

\_symmetry\_Int\_Tables\_number 1

\_symmetry\_cell\_setting triclinic

loop\_

\_atom\_site\_label

\_atom\_site\_type\_symbol

\_atom\_site\_fract\_x

\_atom\_site\_fract\_y

\_atom\_site\_fract\_z

\_atom\_site\_occupancy

|    |   |                    |                    |                    |     |
|----|---|--------------------|--------------------|--------------------|-----|
| H1 | H | 0.0096214000000000 | 0.0636726000000000 | 0.0601974100000000 | 1.0 |
|----|---|--------------------|--------------------|--------------------|-----|

|    |   |                    |                    |                    |     |
|----|---|--------------------|--------------------|--------------------|-----|
| H2 | H | 0.1278878600000000 | 0.8993333400000000 | 0.9378853400000000 | 1.0 |
|----|---|--------------------|--------------------|--------------------|-----|

|    |   |                    |                    |                    |     |
|----|---|--------------------|--------------------|--------------------|-----|
| H3 | H | 0.3880881000000000 | 0.0641825000000000 | 0.9218723200000000 | 1.0 |
|----|---|--------------------|--------------------|--------------------|-----|

|    |   |                    |                    |                    |     |
|----|---|--------------------|--------------------|--------------------|-----|
| H4 | H | 0.2701908000000000 | 0.8989911700000000 | 0.0431224400000000 | 1.0 |
|----|---|--------------------|--------------------|--------------------|-----|

|    |   |                    |                    |                    |     |
|----|---|--------------------|--------------------|--------------------|-----|
| H5 | H | 0.5098380600000000 | 0.0639360400000000 | 0.0601528900000000 | 1.0 |
|----|---|--------------------|--------------------|--------------------|-----|

|    |   |                    |                    |                    |     |
|----|---|--------------------|--------------------|--------------------|-----|
| H6 | H | 0.6277803700000000 | 0.8991991200000000 | 0.9383179700000000 | 1.0 |
|----|---|--------------------|--------------------|--------------------|-----|

|    |   |                    |                    |                    |     |
|----|---|--------------------|--------------------|--------------------|-----|
| H7 | H | 0.8883252600000000 | 0.0639422300000000 | 0.9217522100000000 | 1.0 |
|----|---|--------------------|--------------------|--------------------|-----|

|    |   |                    |                    |                    |     |
|----|---|--------------------|--------------------|--------------------|-----|
| H8 | H | 0.7700945700000000 | 0.8991544100000000 | 0.0435134700000000 | 1.0 |
|----|---|--------------------|--------------------|--------------------|-----|

|      |    |                    |                    |                    |     |
|------|----|--------------------|--------------------|--------------------|-----|
| C9   | C  | 0.1350104300000000 | 0.0569612900000000 | 0.9696514400000000 | 1.0 |
| C10  | C  | 0.0132391600000000 | 0.0392852800000000 | 0.0112638300000000 | 1.0 |
| C11  | C  | 0.0148266600000000 | 0.9604144300000000 | 0.0102326400000000 | 1.0 |
| C12  | C  | 0.1372254100000000 | 0.9440896100000000 | 0.9689979700000000 | 1.0 |
| C13  | C  | 0.2628590700000000 | 0.0568522000000000 | 0.0124362800000000 | 1.0 |
| C14  | C  | 0.3846575700000000 | 0.0395123600000000 | 0.9706712200000000 | 1.0 |
| C15  | C  | 0.3831832700000000 | 0.9606288800000000 | 0.9713047600000000 | 1.0 |
| C16  | C  | 0.2607608400000000 | 0.9439727700000000 | 0.0123448400000000 | 1.0 |
| C17  | C  | 0.6350725300000000 | 0.0569404900000000 | 0.9695731800000000 | 1.0 |
| C18  | C  | 0.5132870300000000 | 0.0394431100000000 | 0.0112671100000000 | 1.0 |
| C19  | C  | 0.5147643900000000 | 0.9605761000000000 | 0.0103654400000000 | 1.0 |
| C20  | C  | 0.6371835200000000 | 0.9440702800000000 | 0.9692579500000000 | 1.0 |
| C21  | C  | 0.7629784800000000 | 0.0568988400000000 | 0.0123105600000000 | 1.0 |
| C22  | C  | 0.8847064100000000 | 0.0393639900000000 | 0.9705918900000000 | 1.0 |
| C23  | C  | 0.8830939500000000 | 0.9604831700000000 | 0.9713531600000000 | 1.0 |
| C24  | C  | 0.7607368300000000 | 0.9440280600000000 | 0.0125747200000000 | 1.0 |
| O25  | O  | 0.1462953000000000 | 0.0014277800000000 | 0.9245169500000000 | 1.0 |
| O26  | O  | 0.2516295700000000 | 0.0010143800000000 | 0.0572067400000000 | 1.0 |
| O27  | O  | 0.6463008900000000 | 0.0012742400000000 | 0.9245933800000000 | 1.0 |
| O28  | O  | 0.7517828200000000 | 0.0012118800000000 | 0.0572676600000000 | 1.0 |
| Br29 | Br | 0.1196472900000000 | 0.1370706400000000 | 0.9145245400000000 | 1.0 |
| Br30 | Br | 0.0117000400000000 | 0.9100501000000000 | 0.0944169800000000 | 1.0 |
| Br31 | Br | 0.2779443800000000 | 0.1365805300000000 | 0.0681226100000000 | 1.0 |
| Br32 | Br | 0.3866423300000000 | 0.9106909400000000 | 0.8868707400000000 | 1.0 |
| Br33 | Br | 0.6197896900000000 | 0.1369281600000000 | 0.9142685800000000 | 1.0 |
| Br34 | Br | 0.5113429000000000 | 0.9104575500000000 | 0.0946793500000000 | 1.0 |
| Br35 | Br | 0.7783740300000000 | 0.1368431800000000 | 0.0676601700000000 | 1.0 |
| Br36 | Br | 0.8861306900000000 | 0.9103513000000000 | 0.8870253900000000 | 1.0 |

##### cif ends

furand\_24\_synalt Energy: -209.6484631

##### cif starts

data\_furand\_24\_synalt

\_publ\_section\_comment

;

Andrew Reynoso, Bohan Xu, and Vincent H. Crespi

;

\_cell\_length\_a 10.3994472511

\_cell\_length\_b 20.0

\_cell\_length\_c 20.0

\_cell\_angle\_alpha 90.0

\_cell\_angle\_beta 90.0

\_cell\_angle\_gamma 90.0

\_symmetry\_space\_group\_name\_H-M 'P 1'

\_symmetry\_Int\_Tables\_number 1

\_symmetry\_cell\_setting triclinic

loop\_

\_atom\_site\_label

\_atom\_site\_type\_symbol

\_atom\_site\_fract\_x

|      |    | _atom_site_fract_x | _atom_site_fract_y | _atom_site_fract_z | _atom_site_occupancy |
|------|----|--------------------|--------------------|--------------------|----------------------|
| H1   | H  | 0.6370800500000000 | 0.9381912500000000 | 0.9281710000000000 | 1.0                  |
| H2   | H  | 0.5119758100000000 | 0.1005404000000000 | 0.0472287500000000 | 1.0                  |
| H3   | H  | 0.8870654700000000 | 0.0629302000000000 | 0.9294508200000000 | 1.0                  |
| H4   | H  | 0.2619698300000000 | 0.8982180800000000 | 0.0452119100000000 | 1.0                  |
| H5   | H  | 0.1371074800000000 | 0.9381843100000000 | 0.9281753600000000 | 1.0                  |
| H6   | H  | 0.0119878300000000 | 0.1005295600000000 | 0.0472431600000000 | 1.0                  |
| H7   | H  | 0.3870786600000000 | 0.0629141200000000 | 0.9294320100000000 | 1.0                  |
| H8   | H  | 0.7619778700000000 | 0.8981971800000000 | 0.0451824600000000 | 1.0                  |
| C9   | C  | 0.6375801400000000 | 0.9605581900000000 | 0.9780114700000000 | 1.0                  |
| C10  | C  | 0.6360714200000000 | 0.0391639200000000 | 0.9791427600000000 | 1.0                  |
| C11  | C  | 0.5109743900000000 | 0.0531203400000000 | 0.0200179900000000 | 1.0                  |
| C12  | C  | 0.5129377600000000 | 0.9457654100000000 | 0.0187404600000000 | 1.0                  |
| C13  | C  | 0.7629256800000000 | 0.0535193300000000 | 0.0198451200000000 | 1.0                  |
| C14  | C  | 0.8875726600000000 | 0.0395574200000000 | 0.9788272400000000 | 1.0                  |
| C15  | C  | 0.8860667800000000 | 0.9609469000000000 | 0.9783445700000000 | 1.0                  |
| C16  | C  | 0.7609732600000000 | 0.9461605500000000 | 0.0189370800000000 | 1.0                  |
| C17  | C  | 0.0129374600000000 | 0.9457597900000000 | 0.0187323500000000 | 1.0                  |
| C18  | C  | 0.1375861600000000 | 0.9605564000000000 | 0.9780136800000000 | 1.0                  |
| C19  | C  | 0.1360647500000000 | 0.0391609800000000 | 0.9791353700000000 | 1.0                  |
| C20  | C  | 0.0109784300000000 | 0.0531144900000000 | 0.0200243300000000 | 1.0                  |
| C21  | C  | 0.2629232000000000 | 0.0535312500000000 | 0.0198247400000000 | 1.0                  |
| C22  | C  | 0.3875750500000000 | 0.0395559800000000 | 0.9788139700000000 | 1.0                  |
| C23  | C  | 0.3860652200000000 | 0.9609449800000000 | 0.9783534500000000 | 1.0                  |
| C24  | C  | 0.2609721000000000 | 0.9461726300000000 | 0.0189513800000000 | 1.0                  |
| O25  | O  | 0.0118823600000000 | 0.9981410200000000 | 0.0670841000000000 | 1.0                  |
| O26  | O  | 0.7618750100000000 | 0.0001554100000000 | 0.0671164000000000 | 1.0                  |
| O27  | O  | 0.5118784500000000 | 0.9981537300000000 | 0.0670853500000000 | 1.0                  |
| O28  | O  | 0.2618699100000000 | 0.0001850000000000 | 0.0671127800000000 | 1.0                  |
| Br29 | Br | 0.5120134700000000 | 0.8588259700000000 | 0.0624687900000000 | 1.0                  |
| Br30 | Br | 0.6361692300000000 | 0.0843878500000000 | 0.8922082900000000 | 1.0                  |
| Br31 | Br | 0.7619522400000000 | 0.1395716100000000 | 0.0653091400000000 | 1.0                  |
| Br32 | Br | 0.3861299800000000 | 0.9175343300000000 | 0.8904939700000000 | 1.0                  |
| Br33 | Br | 0.0120128500000000 | 0.8588093200000000 | 0.0624383600000000 | 1.0                  |
| Br34 | Br | 0.1361045900000000 | 0.0843621300000000 | 0.8921907400000000 | 1.0                  |
| Br35 | Br | 0.2619508000000000 | 0.1395965000000000 | 0.0652602900000000 | 1.0                  |
| Br36 | Br | 0.8861536600000000 | 0.9175614800000000 | 0.8904723400000000 | 1.0                  |

##### cif ends

furan\_Br\_24\_syn\_alt\_forbid Energy: -206.39069499

##### cif starts

data\_furan\_Br\_24\_syn\_alt\_forbid

\_publ\_section\_comment

;  
Andrew Reynoso, Bohan Xu, and Vincent H. Crespi  
;

\_cell\_length\_a 9.7536512352

\_cell\_length\_b 20.0

\_cell\_length\_c 20.0

\_cell\_angle\_alpha 90.0



\_cell\_angle\_beta 90.0  
\_cell\_angle\_gamma 90.0

\_symmetry\_space\_group\_name H-M 'P 1'  
\_symmetry\_Int\_Tables\_number 1  
\_symmetry\_cell\_setting triclinic

loop\_  
\_atom\_site\_label  
\_atom\_site\_type\_symbol  
\_atom\_site\_fract\_x  
\_atom\_site\_fract\_y  
\_atom\_site\_fract\_z  
\_atom\_site\_occupancy

|      |    |                    |                    |                    |     |
|------|----|--------------------|--------------------|--------------------|-----|
| H1   | H  | 0.9059203500000000 | 0.0583239100000000 | 0.9121805600000000 | 1.0 |
| H2   | H  | 0.8959083200000000 | 0.8979471800000000 | 0.0506348800000000 | 1.0 |
| H3   | H  | 0.1577968000000000 | 0.0976471600000000 | 0.0464559900000000 | 1.0 |
| H4   | H  | 0.1478308600000000 | 0.9315653500000000 | 0.9148801000000000 | 1.0 |
| H5   | H  | 0.4058514600000000 | 0.0583524000000000 | 0.9122350300000000 | 1.0 |
| H6   | H  | 0.3959037800000000 | 0.8978857500000000 | 0.0505846000000000 | 1.0 |
| H7   | H  | 0.6578234100000000 | 0.0977046200000000 | 0.0463997100000000 | 1.0 |
| H8   | H  | 0.6478526300000000 | 0.9315708300000000 | 0.9149004900000000 | 1.0 |
| C9   | C  | 0.8600501300000000 | 0.0527828800000000 | 0.0206089900000000 | 1.0 |
| C10  | C  | 0.9446998900000000 | 0.0352196200000000 | 0.9577502900000000 | 1.0 |
| C11  | C  | 0.9457700700000000 | 0.9570254700000000 | 0.9599947500000000 | 1.0 |
| C12  | C  | 0.8614683300000000 | 0.9424039400000000 | 0.0238598000000000 | 1.0 |
| C13  | C  | 0.1922249500000000 | 0.0520988100000000 | 0.0215799300000000 | 1.0 |
| C14  | C  | 0.1079194100000000 | 0.0348016500000000 | 0.9583844900000000 | 1.0 |
| C15  | C  | 0.1089910600000000 | 0.9565772100000000 | 0.9594252600000000 | 1.0 |
| C16  | C  | 0.1936461700000000 | 0.9416862100000000 | 0.0229776200000000 | 1.0 |
| C17  | C  | 0.3600472000000000 | 0.0527432200000000 | 0.0206611900000000 | 1.0 |
| C18  | C  | 0.4444683220000000 | 0.0352248400000000 | 0.9577843900000000 | 1.0 |
| C19  | C  | 0.4457684800000000 | 0.9570299600000000 | 0.9599925900000000 | 1.0 |
| C20  | C  | 0.3614596300000000 | 0.9423610100000000 | 0.0238415100000000 | 1.0 |
| C21  | C  | 0.6922366000000000 | 0.0521424400000000 | 0.0215426500000000 | 1.0 |
| C22  | C  | 0.6078979100000000 | 0.0348149200000000 | 0.9583749500000000 | 1.0 |
| C23  | C  | 0.6089915000000000 | 0.9565915800000000 | 0.9594334200000000 | 1.0 |
| C24  | C  | 0.6936491400000000 | 0.9417308700000000 | 0.0229942400000000 | 1.0 |
| O25  | O  | 0.8944441500000000 | 0.9993028900000000 | 0.0645436100000000 | 1.0 |
| O26  | O  | 0.1592945000000000 | 0.9969652500000000 | 0.0646283700000000 | 1.0 |
| O27  | O  | 0.3944351000000000 | 0.9992329200000000 | 0.0645609600000000 | 1.0 |
| O28  | O  | 0.6593047500000000 | 0.9970326600000000 | 0.0646195200000000 | 1.0 |
| Br29 | Br | 0.9115444400000000 | 0.1388348900000000 | 0.0610368800000000 | 1.0 |
| Br30 | Br | 0.8875394800000000 | 0.9064486900000000 | 0.8801384300000000 | 1.0 |
| Br31 | Br | 0.1660953600000000 | 0.0820717600000000 | 0.8765338100000000 | 1.0 |
| Br32 | Br | 0.1421886700000000 | 0.8574500400000000 | 0.0670552600000000 | 1.0 |
| Br33 | Br | 0.4115248600000000 | 0.1387636700000000 | 0.0611617000000000 | 1.0 |
| Br34 | Br | 0.3875750500000000 | 0.9064931000000000 | 0.8801070800000000 | 1.0 |
| Br35 | Br | 0.6660223000000000 | 0.0820460300000000 | 0.8764972900000000 | 1.0 |
| Br36 | Br | 0.6422135200000000 | 0.8575058400000000 | 0.0671007200000000 | 1.0 |

##### cif ends

furan\_Br\_24\_syn\_dir Energy: -204.6917907  
##### cif starts

data\_furan\_Br\_24\_syn\_dir

\_publ\_section\_comment

;  
Andrew Reynoso, Bohan Xu, and Vincent H. Crespi  
;

\_cell\_length\_a 10.5146308184

\_cell\_length\_b 20.0

\_cell\_length\_c 20.0

\_cell\_angle\_alpha 90.0

\_cell\_angle\_beta 90.0

\_cell\_angle\_gamma 90.0

\_symmetry\_space\_group\_name\_H-M 'P 1'

\_symmetry\_Int\_Tables\_number 1

\_symmetry\_cell\_setting triclinic

loop\_

\_atom\_site\_label

\_atom\_site\_type\_symbol

\_atom\_site\_fract\_x

\_atom\_site\_fract\_y

\_atom\_site\_fract\_z

\_atom\_site\_occupancy

|      |    |                    |                    |                    |     |
|------|----|--------------------|--------------------|--------------------|-----|
| H1   | H  | 0.6170079900000000 | 0.0792179900000000 | 0.9988214100000000 | 1.0 |
| H2   | H  | 0.4986310200000000 | 0.8779680000000000 | 0.9639385000000000 | 1.0 |
| H3   | H  | 0.8235821700000000 | 0.0725417300000000 | 0.9649704800000000 | 1.0 |
| H4   | H  | 0.2611852300000000 | 0.8862306200000000 | 0.0319960100000000 | 1.0 |
| H5   | H  | 0.1175934000000000 | 0.0609354700000000 | 0.9371336700000000 | 1.0 |
| H6   | H  | 0.9732203000000000 | 0.8864244500000000 | 0.0321820000000000 | 1.0 |
| H7   | H  | 0.4108598100000000 | 0.0725192100000000 | 0.9652392900000000 | 1.0 |
| H8   | H  | 0.7359301700000000 | 0.8779798400000000 | 0.9641976200000000 | 1.0 |
| C9   | C  | 0.6172065100000000 | 0.0280254300000000 | 0.0181898300000000 | 1.0 |
| C10  | C  | 0.6172560700000000 | 0.9730090400000000 | 0.9606428800000000 | 1.0 |
| C11  | C  | 0.4920877200000000 | 0.9308493900000000 | 0.9779205700000000 | 1.0 |
| C12  | C  | 0.4882445300000000 | 0.0104501200000000 | 0.0520650900000000 | 1.0 |
| C13  | C  | 0.7463239400000000 | 0.0106806200000000 | 0.0519698000000000 | 1.0 |
| C14  | C  | 0.8568001600000000 | 0.0324579600000000 | 0.9977715700000000 | 1.0 |
| C15  | C  | 0.8726139500000000 | 0.9648520300000000 | 0.9635771400000000 | 1.0 |
| C16  | C  | 0.7424630600000000 | 0.9308984500000000 | 0.9780342700000000 | 1.0 |
| C17  | C  | 0.9897669200000000 | 0.0431764800000000 | 0.0284616100000000 | 1.0 |
| C18  | C  | 0.1173274900000000 | 0.0331004600000000 | 0.9840983800000000 | 1.0 |
| C19  | C  | 0.1172426600000000 | 0.9499584400000000 | 0.9790971300000000 | 1.0 |
| C20  | C  | 0.9894957200000000 | 0.9368565400000000 | 0.0129530200000000 | 1.0 |
| C21  | C  | 0.2447726900000000 | 0.0429897900000000 | 0.0286869200000000 | 1.0 |
| C22  | C  | 0.3776930100000000 | 0.0323496500000000 | 0.9979499200000000 | 1.0 |
| C23  | C  | 0.3618963200000000 | 0.9648167700000000 | 0.9635825400000000 | 1.0 |
| C24  | C  | 0.2449843000000000 | 0.9367202600000000 | 0.0129019000000000 | 1.0 |
| O25  | O  | 0.9919233500000000 | 0.9832988200000000 | 0.0682986900000000 | 1.0 |
| O26  | O  | 0.7462087200000000 | 0.9381934500000000 | 0.0492845800000000 | 1.0 |
| O27  | O  | 0.4884426200000000 | 0.9379695500000000 | 0.0491764800000000 | 1.0 |
| O28  | O  | 0.2425803300000000 | 0.9830090100000000 | 0.0683387800000000 | 1.0 |
| Br29 | Br | 0.4639206600000000 | 0.0314062200000000 | 0.1456400100000000 | 1.0 |
| Br30 | Br | 0.6173381900000000 | 0.0163897600000000 | 0.8727713900000000 | 1.0 |

|      |    |                    |                    |                    |     |
|------|----|--------------------|--------------------|--------------------|-----|
| Br31 | Br | 0.7707314700000000 | 0.0321740100000000 | 0.1453955600000000 | 1.0 |
| Br32 | Br | 0.3195174800000000 | 0.9782554100000000 | 0.8684988000000000 | 1.0 |
| Br33 | Br | 0.9702308500000000 | 0.1305955400000000 | 0.0726575000000000 | 1.0 |
| Br34 | Br | 0.1172199700000000 | 0.8715351100000000 | 0.9121762400000000 | 1.0 |
| Br35 | Br | 0.2643528900000000 | 0.1300698100000000 | 0.0734459600000000 | 1.0 |
| Br36 | Br | 0.9150493400000000 | 0.9781845500000000 | 0.8684824700000000 | 1.0 |

##### cif ends

furan\_Br\_24\_syn\_dir\_forbid Energy: -203.06382596

##### cif starts

data\_furan\_Br\_24\_syn\_dir\_forbid

\_publ\_section\_comment

;  
Andrew Reynoso, Bohan Xu, and Vincent H. Crespi  
;

\_cell\_length\_a 9.6032443822

\_cell\_length\_b 20.0

\_cell\_length\_c 20.0

\_cell\_angle\_alpha 90.0

\_cell\_angle\_beta 90.0

\_cell\_angle\_gamma 90.0

\_symmetry\_space\_group\_name\_H-M 'P 1'

\_symmetry\_Int\_Tables\_number 1

\_symmetry\_cell\_setting triclinic

loop\_

\_atom\_site\_label

\_atom\_site\_type\_symbol

\_atom\_site\_fract\_x

\_atom\_site\_fract\_y

\_atom\_site\_fract\_z

\_atom\_site\_occupancy

|     |   |                    |                    |                    |     |
|-----|---|--------------------|--------------------|--------------------|-----|
| H1  | H | 0.8980057900000000 | 0.0471571400000000 | 0.9022653600000000 | 1.0 |
| H2  | H | 0.9115091600000000 | 0.9093867400000000 | 0.0646472100000000 | 1.0 |
| H3  | H | 0.1347825100000000 | 0.0778604400000000 | 0.9303697400000000 | 1.0 |
| H4  | H | 0.1859779100000000 | 0.8869296000000000 | 0.0234356100000000 | 1.0 |
| H5  | H | 0.3977115600000000 | 0.0472507800000000 | 0.9023662300000000 | 1.0 |
| H6  | H | 0.4116885000000000 | 0.9092452000000000 | 0.0645342800000000 | 1.0 |
| H7  | H | 0.6345192300000000 | 0.0779848900000000 | 0.9303010000000000 | 1.0 |
| H8  | H | 0.6857745500000000 | 0.8871288100000000 | 0.0235479800000000 | 1.0 |
| C9  | C | 0.8376943500000000 | 0.0539811800000000 | 0.0130696300000000 | 1.0 |
| C10 | C | 0.9278020700000000 | 0.0294837100000000 | 0.9518949100000000 | 1.0 |
| C11 | C | 0.9612821900000000 | 0.9526551400000000 | 0.9628964400000000 | 1.0 |
| C12 | C | 0.8804889500000000 | 0.9480421500000000 | 0.0288418300000000 | 1.0 |
| C13 | C | 0.1712412200000000 | 0.0460546800000000 | 0.0328574400000000 | 1.0 |
| C14 | C | 0.0905398400000000 | 0.0423748700000000 | 0.9661244200000000 | 1.0 |
| C15 | C | 0.1215468800000000 | 0.9669151700000000 | 0.9535734100000000 | 1.0 |
| C16 | C | 0.2149366800000000 | 0.9389444200000000 | 0.0132227100000000 | 1.0 |
| C17 | C | 0.3375666600000000 | 0.0538885400000000 | 0.0131951300000000 | 1.0 |
| C18 | C | 0.4276755400000000 | 0.0295362500000000 | 0.9519613000000000 | 1.0 |
| C19 | C | 0.4613279000000000 | 0.9527094300000000 | 0.9628598200000000 | 1.0 |

|      |    |                    |                    |                    |     |
|------|----|--------------------|--------------------|--------------------|-----|
| C20  | C  | 0.3805677100000000 | 0.9479503200000000 | 0.0287988500000000 | 1.0 |
| C21  | C  | 0.6713184700000000 | 0.0462549300000000 | 0.0327856600000000 | 1.0 |
| C22  | C  | 0.5904420000000000 | 0.0425095500000000 | 0.9661110400000000 | 1.0 |
| C23  | C  | 0.6215537500000000 | 0.9670496700000000 | 0.9535773900000000 | 1.0 |
| C24  | C  | 0.7148663800000000 | 0.9391144100000000 | 0.0132740600000000 | 1.0 |
| O25  | O  | 0.8957391100000000 | 0.0119129900000000 | 0.0627937800000000 | 1.0 |
| O26  | O  | 0.1572126300000000 | 0.9813463900000000 | 0.0632506700000000 | 1.0 |
| O27  | O  | 0.3957043600000000 | 0.0117745900000000 | 0.0628536400000000 | 1.0 |
| O28  | O  | 0.6572394200000000 | 0.9815945400000000 | 0.0632622800000000 | 1.0 |
| Br29 | Br | 0.8753189500000000 | 0.1516422900000000 | 0.0092133200000000 | 1.0 |
| Br30 | Br | 0.9141026600000000 | 0.8663904400000000 | 0.9188215700000000 | 1.0 |
| Br31 | Br | 0.1335507700000000 | 0.1044226700000000 | 0.1090429300000000 | 1.0 |
| Br32 | Br | 0.1643417500000000 | 0.9586711000000000 | 0.8572030000000000 | 1.0 |
| Br33 | Br | 0.3748403200000000 | 0.1515810000000000 | 0.0094786900000000 | 1.0 |
| Br34 | Br | 0.4143653400000000 | 0.8664652000000000 | 0.9186805300000000 | 1.0 |
| Br35 | Br | 0.6338746500000000 | 0.1047715200000000 | 0.1088721000000000 | 1.0 |
| Br36 | Br | 0.6645621900000000 | 0.9588532600000000 | 0.8572232700000000 | 1.0 |

##### cif ends

furane\_Br\_3\_anti\_alt Energy: -217.44262425

##### cif starts

data\_furane\_Br\_3\_anti\_alt

\_publ\_section\_comment

;  
Andrew Reynoso, Bohan Xu, and Vincent H. Crespi  
;

\_cell\_length\_a 9.4455928731

\_cell\_length\_b 20.0

\_cell\_length\_c 20.0

\_cell\_angle\_alpha 90.0

\_cell\_angle\_beta 90.0

\_cell\_angle\_gamma 90.0

\_symmetry\_space\_group\_name\_H-M 'P 1'

\_symmetry\_Int\_Tables\_number 1

\_symmetry\_cell\_setting triclinic

loop\_

\_atom\_site\_label

\_atom\_site\_type\_symbol

\_atom\_site\_fract\_x

\_atom\_site\_fract\_y

\_atom\_site\_fract\_z

\_atom\_site\_occupancy

|    |   |                    |                    |                    |     |
|----|---|--------------------|--------------------|--------------------|-----|
| H1 | H | 0.0071620200000000 | 0.1069997300000000 | 0.9343925200000000 | 1.0 |
|----|---|--------------------|--------------------|--------------------|-----|

|    |   |                    |                    |                    |     |
|----|---|--------------------|--------------------|--------------------|-----|
| H2 | H | 0.9899048000000000 | 0.9585622500000000 | 0.0830496600000000 | 1.0 |
|----|---|--------------------|--------------------|--------------------|-----|

|    |   |                    |                    |                    |     |
|----|---|--------------------|--------------------|--------------------|-----|
| H3 | H | 0.9997160100000000 | 0.9036486400000000 | 0.9546510000000000 | 1.0 |
|----|---|--------------------|--------------------|--------------------|-----|

|    |   |                    |                    |                    |     |
|----|---|--------------------|--------------------|--------------------|-----|
| H4 | H | 0.2571536900000000 | 0.9115302500000000 | 0.0660539400000000 | 1.0 |
|----|---|--------------------|--------------------|--------------------|-----|

|    |   |                    |                    |                    |     |
|----|---|--------------------|--------------------|--------------------|-----|
| H5 | H | 0.2399065400000000 | 0.0599656500000000 | 0.9173978100000000 | 1.0 |
|----|---|--------------------|--------------------|--------------------|-----|

|    |   |                    |                    |                    |     |
|----|---|--------------------|--------------------|--------------------|-----|
| H6 | H | 0.2497235200000000 | 0.1148787100000000 | 0.0457962600000000 | 1.0 |
|----|---|--------------------|--------------------|--------------------|-----|

|    |   |                    |                    |                    |     |
|----|---|--------------------|--------------------|--------------------|-----|
| H7 | H | 0.5071603000000000 | 0.1069977600000000 | 0.9343919100000000 | 1.0 |
|----|---|--------------------|--------------------|--------------------|-----|

|    |   |                    |                    |                    |     |
|----|---|--------------------|--------------------|--------------------|-----|
| H8 | H | 0.4899033800000000 | 0.9585596700000000 | 0.0830494300000000 | 1.0 |
|----|---|--------------------|--------------------|--------------------|-----|

|      |    |                    |                    |                    |     |
|------|----|--------------------|--------------------|--------------------|-----|
| H9   | H  | 0.4997175000000000 | 0.9036468500000000 | 0.9546508600000000 | 1.0 |
| H10  | H  | 0.7571557500000000 | 0.9115318400000000 | 0.0660561200000000 | 1.0 |
| H11  | H  | 0.7399050000000000 | 0.0599634500000000 | 0.9173961000000000 | 1.0 |
| H12  | H  | 0.7497205800000000 | 0.1148799600000000 | 0.0457932400000000 | 1.0 |
| C13  | C  | 0.0304244300000000 | 0.0611868400000000 | 0.9624546900000000 | 1.0 |
| C14  | C  | 0.9402178800000000 | 0.0523191800000000 | 0.0271415400000000 | 1.0 |
| C15  | C  | 0.9433639900000000 | 0.9743547500000000 | 0.0354242700000000 | 1.0 |
| C16  | C  | 0.0269828600000000 | 0.9531211700000000 | 0.9736292900000000 | 1.0 |
| C17  | C  | 0.2804199500000000 | 0.9573413100000000 | 0.0379880700000000 | 1.0 |
| C18  | C  | 0.1902117400000000 | 0.9662107700000000 | 0.9732990600000000 | 1.0 |
| C19  | C  | 0.1933613300000000 | 0.0441744100000000 | 0.9650210500000000 | 1.0 |
| C20  | C  | 0.2769887300000000 | 0.0654086600000000 | 0.0268127300000000 | 1.0 |
| C21  | C  | 0.5304242100000000 | 0.0611850200000000 | 0.9624543300000000 | 1.0 |
| C22  | C  | 0.4402186800000000 | 0.0523175400000000 | 0.0271418200000000 | 1.0 |
| C23  | C  | 0.4433639200000000 | 0.9743529100000000 | 0.0354239200000000 | 1.0 |
| C24  | C  | 0.5269834200000000 | 0.9531194700000000 | 0.9736292200000000 | 1.0 |
| C25  | C  | 0.7804207100000000 | 0.9573422300000000 | 0.0379889500000000 | 1.0 |
| C26  | C  | 0.6902126400000000 | 0.9662097000000000 | 0.9732995100000000 | 1.0 |
| C27  | C  | 0.6933610600000000 | 0.0441732300000000 | 0.9650201000000000 | 1.0 |
| C28  | C  | 0.7769878600000000 | 0.0654093600000000 | 0.0268112500000000 | 1.0 |
| O29  | O  | 0.9818707300000000 | 0.0038524100000000 | 0.9253221700000000 | 1.0 |
| O30  | O  | 0.2318700800000000 | 0.0146745100000000 | 0.0751171100000000 | 1.0 |
| O31  | O  | 0.4818709400000000 | 0.0038505100000000 | 0.9253220700000000 | 1.0 |
| O32  | O  | 0.7318696700000000 | 0.0146760800000000 | 0.0751166100000000 | 1.0 |
| Br33 | Br | 0.9993558300000000 | 0.1077144400000000 | 0.1053977400000000 | 1.0 |
| Br34 | Br | 0.2493325400000000 | 0.9108440700000000 | 0.8950209800000000 | 1.0 |
| Br35 | Br | 0.4993574400000000 | 0.1077119400000000 | 0.1053980600000000 | 1.0 |
| Br36 | Br | 0.7493352900000000 | 0.9108416900000000 | 0.8950226200000000 | 1.0 |

##### cif ends

furandBr3antiAltforbid Energy: -218.11122357

##### cif starts

data\_furandBr3antiAltforbid

\_publ\_section\_comment

;  
Andrew Reynoso, Bohan Xu, and Vincent H. Crespi  
;

\_cell\_length\_a 10.2650636621  
\_cell\_length\_b 20.0  
\_cell\_length\_c 20.0  
\_cell\_angle\_alpha 90.0  
\_cell\_angle\_beta 90.0  
\_cell\_angle\_gamma 90.0

\_symmetry\_space\_group\_name\_H-M 'P 1'  
\_symmetry\_Int\_Tables\_number 1  
\_symmetry\_cell\_setting triclinic

loop\_  
\_atom\_site\_label  
\_atom\_site\_type\_symbol  
\_atom\_site\_fract\_x

|      |    | _atom_site_fract_x | _atom_site_fract_y | _atom_site_fract_z | _atom_site_occupancy |
|------|----|--------------------|--------------------|--------------------|----------------------|
| H1   | H  | 0.0709701300000000 | 0.0971839800000000 | 0.9302215100000000 | 1.0                  |
| H2   | H  | 0.9539313300000000 | 0.9320748200000000 | 0.0524387000000000 | 1.0                  |
| H3   | H  | 0.0693326800000000 | 0.8935363500000000 | 0.9315895000000000 | 1.0                  |
| H4   | H  | 0.3305259900000000 | 0.0583149300000000 | 0.9126242000000000 | 1.0                  |
| H5   | H  | 0.2150582400000000 | 0.0967506200000000 | 0.0334705700000000 | 1.0                  |
| H6   | H  | 0.2136332500000000 | 0.8931071700000000 | 0.0347493100000000 | 1.0                  |
| H7   | H  | 0.5706518800000000 | 0.0970895000000000 | 0.9302379900000000 | 1.0                  |
| H8   | H  | 0.4539265300000000 | 0.9319553200000000 | 0.0525288300000000 | 1.0                  |
| H9   | H  | 0.5694400900000000 | 0.8934453600000000 | 0.9317095600000000 | 1.0                  |
| H10  | H  | 0.8303906800000000 | 0.0584172600000000 | 0.9125495400000000 | 1.0                  |
| H11  | H  | 0.7149582600000000 | 0.0968138100000000 | 0.0334147000000000 | 1.0                  |
| H12  | H  | 0.7139772500000000 | 0.8931788300000000 | 0.0347973400000000 | 1.0                  |
| C13  | C  | 0.0800306300000000 | 0.0514800200000000 | 0.9603891700000000 | 1.0                  |
| C14  | C  | 0.9569313600000000 | 0.0348521200000000 | 0.0016449200000000 | 1.0                  |
| C15  | C  | 0.9581914900000000 | 0.9560550800000000 | 0.0031940000000000 | 1.0                  |
| C16  | C  | 0.0795046000000000 | 0.9390164000000000 | 0.9616155400000000 | 1.0                  |
| C17  | C  | 0.2049592000000000 | 0.0512869700000000 | 0.0034211000000000 | 1.0                  |
| C18  | C  | 0.3262951800000000 | 0.0342917300000000 | 0.9618529100000000 | 1.0                  |
| C19  | C  | 0.3275678700000000 | 0.9555023200000000 | 0.9633603400000000 | 1.0                  |
| C20  | C  | 0.2044742600000000 | 0.9388232600000000 | 0.0046038000000000 | 1.0                  |
| C21  | C  | 0.5799206500000000 | 0.0514143700000000 | 0.9604314800000000 | 1.0                  |
| C22  | C  | 0.4569251400000000 | 0.0347474100000000 | 0.0017507800000000 | 1.0                  |
| C23  | C  | 0.4582026700000000 | 0.9559528000000000 | 0.0032914100000000 | 1.0                  |
| C24  | C  | 0.5795356700000000 | 0.9389492100000000 | 0.9617085900000000 | 1.0                  |
| C25  | C  | 0.7049347000000000 | 0.0513300700000000 | 0.0033883300000000 | 1.0                  |
| C26  | C  | 0.8262510300000000 | 0.0343813800000000 | 0.9617738500000000 | 1.0                  |
| C27  | C  | 0.8275590700000000 | 0.9555892100000000 | 0.9632878500000000 | 1.0                  |
| C28  | C  | 0.7045957900000000 | 0.9388652800000000 | 0.0046245700000000 | 1.0                  |
| O29  | O  | 0.0869808600000000 | 0.9952040600000000 | 0.9154751700000000 | 1.0                  |
| O30  | O  | 0.1974997000000000 | 0.9950808500000000 | 0.0495445300000000 | 1.0                  |
| O31  | O  | 0.5868560800000000 | 0.9951190800000000 | 0.9155406500000000 | 1.0                  |
| O32  | O  | 0.6976517200000000 | 0.9951428800000000 | 0.0495381100000000 | 1.0                  |
| Br33 | Br | 0.9540075500000000 | 0.0851685600000000 | 0.0861283100000000 | 1.0                  |
| Br34 | Br | 0.3305929000000000 | 0.9053660100000000 | 0.8787736700000000 | 1.0                  |
| Br35 | Br | 0.4540163600000000 | 0.0849902600000000 | 0.0862684100000000 | 1.0                  |
| Br36 | Br | 0.8304922000000000 | 0.9054544500000000 | 0.8787028800000000 | 1.0                  |

##### cif ends

furan\_Br\_3\_anti\_dir    Energy: -217.3276032

##### cif starts

data\_furan\_Br\_3\_anti\_dir

\_publ\_section\_comment

;  
Andrew Reynoso, Bohan Xu, and Vincent H. Crespi  
;

\_cell\_length\_a    9.463007945

\_cell\_length\_b    20.0

\_cell\_length\_c    20.0

\_cell\_angle\_alpha    90.0

\_cell\_angle\_beta 90.0  
\_cell\_angle\_gamma 90.0

\_symmetry\_space\_group\_name H-M 'P 1'  
\_symmetry\_Int\_Tables\_number 1  
\_symmetry\_cell\_setting triclinic

loop\_

\_atom\_site\_label  
\_atom\_site\_type\_symbol  
\_atom\_site\_fract\_x  
\_atom\_site\_fract\_y  
\_atom\_site\_fract\_z  
\_atom\_site\_occupancy

|      |    |                    |                    |                    |     |
|------|----|--------------------|--------------------|--------------------|-----|
| H1   | H  | 0.0164737500000000 | 0.9086401300000000 | 0.9469822800000000 | 1.0 |
| H2   | H  | 0.0024977000000000 | 0.0711448200000000 | 0.0788701200000000 | 1.0 |
| H3   | H  | 0.0168892500000000 | 0.1129742600000000 | 0.9442361400000000 | 1.0 |
| H4   | H  | 0.2664559300000000 | 0.9089312400000000 | 0.0561898400000000 | 1.0 |
| H5   | H  | 0.2524963200000000 | 0.0707363100000000 | 0.9234462200000000 | 1.0 |
| H6   | H  | 0.2669040700000000 | 0.1132799900000000 | 0.0578517700000000 | 1.0 |
| H7   | H  | 0.5164748900000000 | 0.9086385000000000 | 0.9469813700000000 | 1.0 |
| H8   | H  | 0.5025043300000000 | 0.0711441600000000 | 0.0788674800000000 | 1.0 |
| H9   | H  | 0.5168889300000000 | 0.1129723500000000 | 0.9442329400000000 | 1.0 |
| H10  | H  | 0.7664560700000000 | 0.9089304300000000 | 0.0561886300000000 | 1.0 |
| H11  | H  | 0.7524980100000000 | 0.0707350000000000 | 0.9234450700000000 | 1.0 |
| H12  | H  | 0.7668968300000000 | 0.1132795700000000 | 0.0578507100000000 | 1.0 |
| C13  | C  | 0.0413572000000000 | 0.9567588400000000 | 0.9697553700000000 | 1.0 |
| C14  | C  | 0.9536334200000000 | 0.9723033400000000 | 0.0325220000000000 | 1.0 |
| C15  | C  | 0.9566705700000000 | 0.0507260800000000 | 0.0328704200000000 | 1.0 |
| C16  | C  | 0.0428253800000000 | 0.0654103600000000 | 0.9686945800000000 | 1.0 |
| C17  | C  | 0.2913518200000000 | 0.9569304800000000 | 0.0331668000000000 | 1.0 |
| C18  | C  | 0.2036360500000000 | 0.9721424500000000 | 0.9703207100000000 | 1.0 |
| C19  | C  | 0.2066716300000000 | 0.0505622500000000 | 0.9695542100000000 | 1.0 |
| C20  | C  | 0.2928279100000000 | 0.0655839600000000 | 0.0336494500000000 | 1.0 |
| C21  | C  | 0.5413578500000000 | 0.9567575500000000 | 0.9697541200000000 | 1.0 |
| C22  | C  | 0.4536347400000000 | 0.9723026100000000 | 0.0325209400000000 | 1.0 |
| C23  | C  | 0.4566732900000000 | 0.0507251700000000 | 0.0328691800000000 | 1.0 |
| C24  | C  | 0.5428260800000000 | 0.0654091200000000 | 0.9686921000000000 | 1.0 |
| C25  | C  | 0.7913509200000000 | 0.9569300700000000 | 0.0331662700000000 | 1.0 |
| C26  | C  | 0.7036366500000000 | 0.9721414000000000 | 0.9703195100000000 | 1.0 |
| C27  | C  | 0.7066718700000000 | 0.0505614200000000 | 0.9695522000000000 | 1.0 |
| C28  | C  | 0.7928244200000000 | 0.0655834000000000 | 0.0336491700000000 | 1.0 |
| O29  | O  | 0.9954840600000000 | 0.0109386400000000 | 0.9264514000000000 | 1.0 |
| O30  | O  | 0.2454737300000000 | 0.0113409900000000 | 0.0761860600000000 | 1.0 |
| O31  | O  | 0.4954843000000000 | 0.0109367400000000 | 0.9264497200000000 | 1.0 |
| O32  | O  | 0.7454695700000000 | 0.0113403800000000 | 0.0761848900000000 | 1.0 |
| Br33 | Br | 0.0128957400000000 | 0.9250734500000000 | 0.1158139300000000 | 1.0 |
| Br34 | Br | 0.2628927400000000 | 0.9244719800000000 | 0.8872744600000000 | 1.0 |
| Br35 | Br | 0.5128973700000000 | 0.9250719300000000 | 0.1158125900000000 | 1.0 |
| Br36 | Br | 0.7628945800000000 | 0.9244716100000000 | 0.8872733400000000 | 1.0 |

##### cif ends

furan\_Br\_3\_anti\_dir\_forbid Energy: -218.07003066

##### cif starts

data\_furan\_Br\_3\_anti\_dir\_forbid

\_publ\_section\_comment

;  
Andrew Reynoso, Bohan Xu, and Vincent H. Crespi  
;

\_cell\_length\_a 10.2642142407

\_cell\_length\_b 20.0

\_cell\_length\_c 20.0

\_cell\_angle\_alpha 90.0

\_cell\_angle\_beta 90.0

\_cell\_angle\_gamma 90.0

\_symmetry\_space\_group\_name\_H-M 'P 1'

\_symmetry\_Int\_Tables\_number 1

\_symmetry\_cell\_setting triclinic

loop\_

\_atom\_site\_label

\_atom\_site\_type\_symbol

\_atom\_site\_fract\_x

\_atom\_site\_fract\_y

\_atom\_site\_fract\_z

\_atom\_site\_occupancy

|     |   |                    |                    |                    |     |
|-----|---|--------------------|--------------------|--------------------|-----|
| H1  | H | 0.0165151700000000 | 0.1035572100000000 | 0.9512376800000000 | 1.0 |
| H2  | H | 0.8963511600000000 | 0.9394406400000000 | 0.0725242600000000 | 1.0 |
| H3  | H | 0.0133660900000000 | 0.8999257700000000 | 0.9512142500000000 | 1.0 |
| H4  | H | 0.1581906700000000 | 0.1029635400000000 | 0.0552976700000000 | 1.0 |
| H5  | H | 0.2783213000000000 | 0.9402502900000000 | 0.9321353600000000 | 1.0 |
| H6  | H | 0.1612822100000000 | 0.8993481100000000 | 0.0530058800000000 | 1.0 |
| H7  | H | 0.5164457400000000 | 0.1035563800000000 | 0.9513318200000000 | 1.0 |
| H8  | H | 0.3962789700000000 | 0.9393541200000000 | 0.0725199100000000 | 1.0 |
| H9  | H | 0.5134945400000000 | 0.8999189400000000 | 0.9512451700000000 | 1.0 |
| H10 | H | 0.6581620000000000 | 0.1029693600000000 | 0.0553710300000000 | 1.0 |
| H11 | H | 0.7782855500000000 | 0.9402864000000000 | 0.9321576200000000 | 1.0 |
| H12 | H | 0.6613759600000000 | 0.8993591200000000 | 0.0530517000000000 | 1.0 |
| C13 | C | 0.0254951100000000 | 0.0579793400000000 | 0.9811564900000000 | 1.0 |
| C14 | C | 0.9031741200000000 | 0.0418159000000000 | 0.0224843400000000 | 1.0 |
| C15 | C | 0.9018101600000000 | 0.9629547300000000 | 0.0231131100000000 | 1.0 |
| C16 | C | 0.0238875700000000 | 0.9455256800000000 | 0.9814801300000000 | 1.0 |
| C17 | C | 0.1492120600000000 | 0.0577261100000000 | 0.0248645400000000 | 1.0 |
| C18 | C | 0.2715577200000000 | 0.0420202500000000 | 0.9833963500000000 | 1.0 |
| C19 | C | 0.2728879600000000 | 0.9631733400000000 | 0.9818258200000000 | 1.0 |
| C20 | C | 0.1507821500000000 | 0.9452821600000000 | 0.0232504000000000 | 1.0 |
| C21 | C | 0.5254741000000000 | 0.0579692900000000 | 0.9812357700000000 | 1.0 |
| C22 | C | 0.4031412900000000 | 0.0417656000000000 | 0.0225325400000000 | 1.0 |
| C23 | C | 0.4017899100000000 | 0.9629039700000000 | 0.0231251200000000 | 1.0 |
| C24 | C | 0.5239253100000000 | 0.9455143100000000 | 0.9815239900000000 | 1.0 |
| C25 | C | 0.6492031700000000 | 0.0577346000000000 | 0.0249284400000000 | 1.0 |
| C26 | C | 0.7715240500000000 | 0.0420559700000000 | 0.9834155800000000 | 1.0 |
| C27 | C | 0.7728747200000000 | 0.9632078900000000 | 0.9818500100000000 | 1.0 |
| C28 | C | 0.6508178600000000 | 0.9452950700000000 | 0.0232986100000000 | 1.0 |
| O29 | O | 0.0316176400000000 | 0.0015990100000000 | 0.9357603400000000 | 1.0 |
| O30 | O | 0.1430591600000000 | 0.0008282900000000 | 0.0696100800000000 | 1.0 |



|      |    |                    |                    |                    |     |
|------|----|--------------------|--------------------|--------------------|-----|
| O31  | O  | 0.5316367600000000 | 0.0016037500000000 | 0.9358199000000000 | 1.0 |
| O32  | O  | 0.6430984900000000 | 0.0008318800000000 | 0.0696662800000000 | 1.0 |
| Br33 | Br | 0.9002986200000000 | 0.0919130400000000 | 0.1069860400000000 | 1.0 |
| Br34 | Br | 0.2745650900000000 | 0.0931163500000000 | 0.8994888100000000 | 1.0 |
| Br35 | Br | 0.4001480900000000 | 0.0917765600000000 | 0.1070816800000000 | 1.0 |
| Br36 | Br | 0.7744280300000000 | 0.0931588700000000 | 0.8995138900000000 | 1.0 |

##### cif ends

furan\_Br\_3\_syn\_alt Energy: -218.61418034

##### cif starts

data\_furan\_Br\_3\_syn\_alt

\_publ\_section\_comment

;  
Andrew Reynoso, Bohan Xu, and Vincent H. Crespi  
;

\_cell\_length\_a 10.3519073501

\_cell\_length\_b 20.0

\_cell\_length\_c 20.0

\_cell\_angle\_alpha 90.0

\_cell\_angle\_beta 90.0

\_cell\_angle\_gamma 90.0

\_symmetry\_space\_group\_name\_H-M 'P 1'

\_symmetry\_Int\_Tables\_number 1

\_symmetry\_cell\_setting triclinic

loop\_

\_atom\_site\_label

\_atom\_site\_type\_symbol

\_atom\_site\_fract\_x

\_atom\_site\_fract\_y

\_atom\_site\_fract\_z

\_atom\_site\_occupancy

|     |   |                    |                    |                    |     |
|-----|---|--------------------|--------------------|--------------------|-----|
| H1  | H | 0.9934588800000000 | 0.8981067800000000 | 0.0434604000000000 | 1.0 |
| H2  | H | 0.1187542300000000 | 0.0611085500000000 | 0.9251597500000000 | 1.0 |
| H3  | H | 0.9940507600000000 | 0.1021623100000000 | 0.0422909100000000 | 1.0 |
| H4  | H | 0.7434686700000000 | 0.1021771400000000 | 0.0422713300000000 | 1.0 |
| H5  | H | 0.8687452400000000 | 0.9378279400000000 | 0.9258700000000000 | 1.0 |
| H6  | H | 0.7440443700000000 | 0.8981227700000000 | 0.0434768800000000 | 1.0 |
| H7  | H | 0.4934656200000000 | 0.8981110900000000 | 0.0434558500000000 | 1.0 |
| H8  | H | 0.6187529000000000 | 0.0611107000000000 | 0.9251511800000000 | 1.0 |
| H9  | H | 0.4940505500000000 | 0.1021671600000000 | 0.0422829700000000 | 1.0 |
| H10 | H | 0.2434660400000000 | 0.1021669700000000 | 0.0422862700000000 | 1.0 |
| H11 | H | 0.3687484900000000 | 0.9378323300000000 | 0.9258643700000000 | 1.0 |
| H12 | H | 0.2440574700000000 | 0.8981124600000000 | 0.0434667900000000 | 1.0 |
| C13 | C | 0.9927102000000000 | 0.9460209400000000 | 0.0167457800000000 | 1.0 |
| C14 | C | 0.1187588900000000 | 0.9605018100000000 | 0.9764368700000000 | 1.0 |
| C15 | C | 0.1187543800000000 | 0.0391158600000000 | 0.9751701300000000 | 1.0 |
| C16 | C | 0.9948018500000000 | 0.0539481000000000 | 0.0161229200000000 | 1.0 |
| C17 | C | 0.7427093300000000 | 0.0539577100000000 | 0.0161120500000000 | 1.0 |
| C18 | C | 0.8687580000000000 | 0.0390008600000000 | 0.9759754300000000 | 1.0 |
| C19 | C | 0.8687548100000000 | 0.9603828100000000 | 0.9756288700000000 | 1.0 |

|      |    |                    |                    |                    |     |
|------|----|--------------------|--------------------|--------------------|-----|
| C20  | C  | 0.7448020300000000 | 0.9460302300000000 | 0.0167508900000000 | 1.0 |
| C21  | C  | 0.4927126900000000 | 0.9460247200000000 | 0.0167408500000000 | 1.0 |
| C22  | C  | 0.6187609100000000 | 0.9605074300000000 | 0.9764331800000000 | 1.0 |
| C23  | C  | 0.6187550300000000 | 0.0391206500000000 | 0.9751627200000000 | 1.0 |
| C24  | C  | 0.4948019300000000 | 0.0539521200000000 | 0.0161165000000000 | 1.0 |
| C25  | C  | 0.2427089500000000 | 0.0539510700000000 | 0.0161198700000000 | 1.0 |
| C26  | C  | 0.3687536500000000 | 0.0390012100000000 | 0.9759753300000000 | 1.0 |
| C27  | C  | 0.3687558600000000 | 0.9603832900000000 | 0.9756249700000000 | 1.0 |
| C28  | C  | 0.2448061900000000 | 0.9460234600000000 | 0.0167475100000000 | 1.0 |
| O29  | O  | 0.9937525200000000 | 0.0002610600000000 | 0.0641619500000000 | 1.0 |
| O30  | O  | 0.7437558100000000 | 0.0002785800000000 | 0.0641590900000000 | 1.0 |
| O31  | O  | 0.4937551700000000 | 0.0002662700000000 | 0.0641564100000000 | 1.0 |
| O32  | O  | 0.2437614000000000 | 0.0002669300000000 | 0.0641609300000000 | 1.0 |
| Br33 | Br | 0.1187741400000000 | 0.9145657100000000 | 0.8892671500000000 | 1.0 |
| Br34 | Br | 0.8687895700000000 | 0.0838169500000000 | 0.8882294700000000 | 1.0 |
| Br35 | Br | 0.6187813800000000 | 0.9145683800000000 | 0.8892647400000000 | 1.0 |
| Br36 | Br | 0.3687710900000000 | 0.0838216700000000 | 0.8882317000000000 | 1.0 |

##### cif ends

furan\_Br\_3\_syn\_alt\_forbid Energy: -215.59690138

##### cif starts

data\_furan\_Br\_3\_syn\_alt\_forbid

\_publ\_section\_comment

;  
Andrew Reynoso, Bohan Xu, and Vincent H. Crespi  
;

\_cell\_length\_a 9.617939136

\_cell\_length\_b 20.0

\_cell\_length\_c 20.0

\_cell\_angle\_alpha 90.0

\_cell\_angle\_beta 90.0

\_cell\_angle\_gamma 90.0

\_symmetry\_space\_group\_name\_H-M 'P 1'

\_symmetry\_Int\_Tables\_number 1

\_symmetry\_cell\_setting triclinic

loop\_

\_atom\_site\_label

\_atom\_site\_type\_symbol

\_atom\_site\_fract\_x

\_atom\_site\_fract\_y

\_atom\_site\_fract\_z

\_atom\_site\_occupancy

|    |   |                    |                    |                    |     |
|----|---|--------------------|--------------------|--------------------|-----|
| H1 | H | 0.8999187400000000 | 0.0982989200000000 | 0.0680794900000000 | 1.0 |
|----|---|--------------------|--------------------|--------------------|-----|

|    |   |                    |                    |                    |     |
|----|---|--------------------|--------------------|--------------------|-----|
| H2 | H | 0.9018843600000000 | 0.0627203900000000 | 0.9328204400000000 | 1.0 |
|----|---|--------------------|--------------------|--------------------|-----|

|    |   |                    |                    |                    |     |
|----|---|--------------------|--------------------|--------------------|-----|
| H3 | H | 0.8948303900000000 | 0.8958536800000000 | 0.0638624800000000 | 1.0 |
|----|---|--------------------|--------------------|--------------------|-----|

|    |   |                    |                    |                    |     |
|----|---|--------------------|--------------------|--------------------|-----|
| H4 | H | 0.1582692100000000 | 0.1011386900000000 | 0.0672113500000000 | 1.0 |
|----|---|--------------------|--------------------|--------------------|-----|

|    |   |                    |                    |                    |     |
|----|---|--------------------|--------------------|--------------------|-----|
| H5 | H | 0.1512494600000000 | 0.9386787600000000 | 0.9307377700000000 | 1.0 |
|----|---|--------------------|--------------------|--------------------|-----|

|    |   |                    |                    |                    |     |
|----|---|--------------------|--------------------|--------------------|-----|
| H6 | H | 0.1534996200000000 | 0.8986467100000000 | 0.0647462500000000 | 1.0 |
|----|---|--------------------|--------------------|--------------------|-----|

|    |   |                    |                    |                    |     |
|----|---|--------------------|--------------------|--------------------|-----|
| H7 | H | 0.3997693100000000 | 0.0983166200000000 | 0.0681357700000000 | 1.0 |
|----|---|--------------------|--------------------|--------------------|-----|

|    |   |                    |                    |                    |     |
|----|---|--------------------|--------------------|--------------------|-----|
| H8 | H | 0.4019390100000000 | 0.0628686000000000 | 0.9328547200000000 | 1.0 |
|----|---|--------------------|--------------------|--------------------|-----|

|      |    |                    |                    |                    |     |
|------|----|--------------------|--------------------|--------------------|-----|
| H9   | H  | 0.3949978700000000 | 0.8958690400000000 | 0.0637472800000000 | 1.0 |
| H10  | H  | 0.6584147500000000 | 0.1011879100000000 | 0.0672481200000000 | 1.0 |
| H11  | H  | 0.6513210700000000 | 0.9387854700000000 | 0.9307285500000000 | 1.0 |
| H12  | H  | 0.6533184800000000 | 0.8987027300000000 | 0.0647377400000000 | 1.0 |
| C13  | C  | 0.8623718600000000 | 0.0536972100000000 | 0.0417436000000000 | 1.0 |
| C14  | C  | 0.9427610900000000 | 0.0383170200000000 | 0.9773993100000000 | 1.0 |
| C15  | C  | 0.9455641300000000 | 0.9602354600000000 | 0.9765822700000000 | 1.0 |
| C16  | C  | 0.8602534200000000 | 0.9423050500000000 | 0.0398681400000000 | 1.0 |
| C17  | C  | 0.1929396600000000 | 0.0555166400000000 | 0.0417008300000000 | 1.0 |
| C18  | C  | 0.1076427100000000 | 0.0396464600000000 | 0.9778479600000000 | 1.0 |
| C19  | C  | 0.1104378100000000 | 0.9615870100000000 | 0.9761193800000000 | 1.0 |
| C20  | C  | 0.1909359300000000 | 0.9441152400000000 | 0.0398916400000000 | 1.0 |
| C21  | C  | 0.3623293800000000 | 0.0537192000000000 | 0.0417536400000000 | 1.0 |
| C22  | C  | 0.4427888100000000 | 0.0384149700000000 | 0.9774118700000000 | 1.0 |
| C23  | C  | 0.4455857400000000 | 0.9603321600000000 | 0.9765245200000000 | 1.0 |
| C24  | C  | 0.3603144800000000 | 0.9423262000000000 | 0.0398042400000000 | 1.0 |
| C25  | C  | 0.6930029700000000 | 0.0555620900000000 | 0.0417239800000000 | 1.0 |
| C26  | C  | 0.6076821100000000 | 0.0397292900000000 | 0.9778747500000000 | 1.0 |
| C27  | C  | 0.6104556600000000 | 0.9616723700000000 | 0.9761074400000000 | 1.0 |
| C28  | C  | 0.6908675500000000 | 0.9441593700000000 | 0.0399019500000000 | 1.0 |
| O29  | O  | 0.8953703700000000 | 0.9967157100000000 | 0.0827961800000000 | 1.0 |
| O30  | O  | 0.1578491800000000 | 0.9997031400000000 | 0.0827985300000000 | 1.0 |
| O31  | O  | 0.3953862100000000 | 0.9967188300000000 | 0.0827681200000000 | 1.0 |
| O32  | O  | 0.6578376300000000 | 0.9997514300000000 | 0.0828118400000000 | 1.0 |
| Br33 | Br | 0.8889498400000000 | 0.9112299600000000 | 0.8947755600000000 | 1.0 |
| Br34 | Br | 0.1641043200000000 | 0.0911405700000000 | 0.8975634000000000 | 1.0 |
| Br35 | Br | 0.3889820500000000 | 0.9114379100000000 | 0.8946502800000000 | 1.0 |
| Br36 | Br | 0.6641733900000000 | 0.0912355000000000 | 0.8975998100000000 | 1.0 |

##### cif ends

furand\_Br\_3\_syn\_dir Energy: -215.75245173

##### cif starts

data\_furand\_Br\_3\_syn\_dir

\_publ\_section\_comment

;  
Andrew Reynoso, Bohan Xu, and Vincent H. Crespi  
;

\_cell\_length\_a 10.3941383599

\_cell\_length\_b 20.0

\_cell\_length\_c 20.0

\_cell\_angle\_alpha 90.0

\_cell\_angle\_beta 90.0

\_cell\_angle\_gamma 90.0

\_symmetry\_space\_group\_name\_H-M 'P 1'

\_symmetry\_Int\_Tables\_number 1

\_symmetry\_cell\_setting triclinic

loop\_

\_atom\_site\_label

\_atom\_site\_type\_symbol

\_atom\_site\_fract\_x

|      |    | _atom_site_fract_x | _atom_site_fract_y | _atom_site_fract_z | _atom_site_occupancy |
|------|----|--------------------|--------------------|--------------------|----------------------|
| H1   | H  | 0.9823967800000000 | 0.8977133500000000 | 0.0367258500000000 | 1.0                  |
| H2   | H  | 0.1041983400000000 | 0.0711319500000000 | 0.9323286700000000 | 1.0                  |
| H3   | H  | 0.9780138700000000 | 0.1013445500000000 | 0.0532934400000000 | 1.0                  |
| H4   | H  | 0.2259793400000000 | 0.8977865000000000 | 0.0369101900000000 | 1.0                  |
| H5   | H  | 0.3414412600000000 | 0.0617612900000000 | 0.9266823500000000 | 1.0                  |
| H6   | H  | 0.2308024000000000 | 0.1014137600000000 | 0.0530889600000000 | 1.0                  |
| H7   | H  | 0.4508789500000000 | 0.9236065800000000 | 0.0809100600000000 | 1.0                  |
| H8   | H  | 0.6042886500000000 | 0.0357150900000000 | 0.9218090100000000 | 1.0                  |
| H9   | H  | 0.4925043800000000 | 0.1172658500000000 | 0.0227845600000000 | 1.0                  |
| H10  | H  | 0.7574821300000000 | 0.9236128200000000 | 0.0809326900000000 | 1.0                  |
| H11  | H  | 0.8670534100000000 | 0.0619360100000000 | 0.9268661100000000 | 1.0                  |
| H12  | H  | 0.7157583500000000 | 0.1172850900000000 | 0.0229088900000000 | 1.0                  |
| C13  | C  | 0.9794575200000000 | 0.9477985200000000 | 0.0144960500000000 | 1.0                  |
| C14  | C  | 0.1042243400000000 | 0.9665210600000000 | 0.9740743400000000 | 1.0                  |
| C15  | C  | 0.1042311800000000 | 0.0452149100000000 | 0.9806814000000000 | 1.0                  |
| C16  | C  | 0.9790314600000000 | 0.0562044400000000 | 0.0221330900000000 | 1.0                  |
| C17  | C  | 0.2289852100000000 | 0.9478135800000000 | 0.0145372200000000 | 1.0                  |
| C18  | C  | 0.3618478300000000 | 0.9670040000000000 | 0.9838695000000000 | 1.0                  |
| C19  | C  | 0.3525043900000000 | 0.0443541600000000 | 0.9783146200000000 | 1.0                  |
| C20  | C  | 0.2295385200000000 | 0.0562226100000000 | 0.0220099000000000 | 1.0                  |
| C21  | C  | 0.4726148600000000 | 0.9613664000000000 | 0.0430278600000000 | 1.0                  |
| C22  | C  | 0.6042225800000000 | 0.9573494100000000 | 0.0091791500000000 | 1.0                  |
| C23  | C  | 0.6042445600000000 | 0.0331255100000000 | 0.9763979100000000 | 1.0                  |
| C24  | C  | 0.4815004700000000 | 0.0639111100000000 | 0.0111127300000000 | 1.0                  |
| C25  | C  | 0.7357542500000000 | 0.9613801500000000 | 0.0430708800000000 | 1.0                  |
| C26  | C  | 0.8465928900000000 | 0.9670805100000000 | 0.9838929000000000 | 1.0                  |
| C27  | C  | 0.8559843100000000 | 0.0444383100000000 | 0.9784559800000000 | 1.0                  |
| C28  | C  | 0.7269084300000000 | 0.0639372700000000 | 0.0112166200000000 | 1.0                  |
| O29  | O  | 0.9806562500000000 | 0.9979211300000000 | 0.0659331800000000 | 1.0                  |
| O30  | O  | 0.2279018000000000 | 0.9980117400000000 | 0.0658923000000000 | 1.0                  |
| O31  | O  | 0.4728212200000000 | 0.0264066400000000 | 0.0724373000000000 | 1.0                  |
| O32  | O  | 0.7354725300000000 | 0.0264034700000000 | 0.0725201600000000 | 1.0                  |
| Br33 | Br | 0.1042450000000000 | 0.9302896900000000 | 0.8832796700000000 | 1.0                  |
| Br34 | Br | 0.4101093500000000 | 0.9330417200000000 | 0.8942497100000000 | 1.0                  |
| Br35 | Br | 0.6043952000000000 | 0.8561479800000000 | 0.9861003000000000 | 1.0                  |
| Br36 | Br | 0.7982940000000000 | 0.9332568400000000 | 0.8942124700000000 | 1.0                  |

##### cif ends

furan\_Br\_3\_syn\_dir\_forbid Energy: -213.25582389

##### cif starts

data\_furan\_Br\_3\_syn\_dir\_forbid

\_publ\_section\_comment

;  
Andrew Reynoso, Bohan Xu, and Vincent H. Crespi  
;

\_cell\_length\_a 9.4337564037

\_cell\_length\_b 20.0

\_cell\_length\_c 20.0

\_cell\_angle\_alpha 90.0

\_cell\_angle\_beta 90.0  
\_cell\_angle\_gamma 90.0

\_symmetry\_space\_group\_name H-M 'P 1'  
\_symmetry\_Int\_Tables\_number 1  
\_symmetry\_cell\_setting triclinic

loop\_

\_atom\_site\_label  
\_atom\_site\_type\_symbol  
\_atom\_site\_fract\_x  
\_atom\_site\_fract\_y  
\_atom\_site\_fract\_z  
\_atom\_site\_occupancy

|      |    |                    |                    |                    |     |
|------|----|--------------------|--------------------|--------------------|-----|
| H1   | H  | 0.8576649400000000 | 0.1286248000000000 | 0.0508157300000000 | 1.0 |
| H2   | H  | 0.8880407600000000 | 0.9598937600000000 | 0.9328237300000000 | 1.0 |
| H3   | H  | 0.9178434700000000 | 0.9291391200000000 | 0.0745588800000000 | 1.0 |
| H4   | H  | 0.1835058300000000 | 0.0718089300000000 | 0.1022750300000000 | 1.0 |
| H5   | H  | 0.1401461700000000 | 0.9669840100000000 | 0.9170612700000000 | 1.0 |
| H6   | H  | 0.1307385400000000 | 0.8851474000000000 | 0.0274238900000000 | 1.0 |
| H7   | H  | 0.4197487100000000 | 0.0734529400000000 | 0.0648327900000000 | 1.0 |
| H8   | H  | 0.4317567000000000 | 0.9097316900000000 | 0.9271321000000000 | 1.0 |
| H9   | H  | 0.3693081100000000 | 0.8725209600000000 | 0.0556711000000000 | 1.0 |
| H10  | H  | 0.6224266000000000 | 0.1121203000000000 | 0.0191277700000000 | 1.0 |
| H11  | H  | 0.6791298500000000 | 0.9125482700000000 | 0.9515510300000000 | 1.0 |
| H12  | H  | 0.6725563500000000 | 0.9242163900000000 | 0.0918637300000000 | 1.0 |
| C13  | C  | 0.8457179600000000 | 0.0782148300000000 | 0.0300221000000000 | 1.0 |
| C14  | C  | 0.9536690300000000 | 0.0589877200000000 | 0.9779627000000000 | 1.0 |
| C15  | C  | 0.9429721700000000 | 0.9815229000000000 | 0.9759219100000000 | 1.0 |
| C16  | C  | 0.8665337700000000 | 0.9685220200000000 | 0.0452906800000000 | 1.0 |
| C17  | C  | 0.1953883300000000 | 0.0371834900000000 | 0.0603146100000000 | 1.0 |
| C18  | C  | 0.1152004200000000 | 0.0531569200000000 | 0.9961369700000000 | 1.0 |
| C19  | C  | 0.1110212700000000 | 0.9768473400000000 | 0.9689019200000000 | 1.0 |
| C20  | C  | 0.1848120100000000 | 0.9337075300000000 | 0.0233383400000000 | 1.0 |
| C21  | C  | 0.3659721800000000 | 0.0310417100000000 | 0.0418248300000000 | 1.0 |
| C22  | C  | 0.4357958300000000 | 0.0139541000000000 | 0.9670615300000000 | 1.0 |
| C23  | C  | 0.4516749200000000 | 0.9371513000000000 | 0.9736479500000000 | 1.0 |
| C24  | C  | 0.3534891000000000 | 0.9214173000000000 | 0.0317928000000000 | 1.0 |
| C25  | C  | 0.6793225600000000 | 0.0643956500000000 | 0.0152839200000000 | 1.0 |
| C26  | C  | 0.6077342200000000 | 0.0197198800000000 | 0.9597923000000000 | 1.0 |
| C27  | C  | 0.6189930000000000 | 0.9459643600000000 | 0.9843954000000000 | 1.0 |
| C28  | C  | 0.6954936100000000 | 0.9588428600000000 | 0.0508064400000000 | 1.0 |
| O29  | O  | 0.8869693200000000 | 0.0309030200000000 | 0.0804992600000000 | 1.0 |
| O30  | O  | 0.1523502100000000 | 0.9724836300000000 | 0.0818967300000000 | 1.0 |
| O31  | O  | 0.4001102100000000 | 0.9716619600000000 | 0.0778409100000000 | 1.0 |
| O32  | O  | 0.6426026000000000 | 0.0235447300000000 | 0.0712705300000000 | 1.0 |
| Br33 | Br | 0.9402719600000000 | 0.1103244200000000 | 0.8941114100000000 | 1.0 |
| Br34 | Br | 0.2068850600000000 | 0.1456988800000000 | 0.9821082600000000 | 1.0 |
| Br35 | Br | 0.3453093600000000 | 0.0417145700000000 | 0.8820834000000000 | 1.0 |
| Br36 | Br | 0.6667522500000000 | 0.0216269800000000 | 0.8657802900000000 | 1.0 |

##### cif ends

furan\_CH3\_23\_anti\_alt Energy: -356.01525265

##### cif starts

data\_furan\_CH3\_23\_anti\_alt

\_publ\_section\_comment

;  
Andrew Reynoso, Bohan Xu, and Vincent H. Crespi  
;

\_cell\_length\_a 9.6463559461

\_cell\_length\_b 20.0

\_cell\_length\_c 20.0

\_cell\_angle\_alpha 90.0

\_cell\_angle\_beta 90.0

\_cell\_angle\_gamma 90.0

\_symmetry\_space\_group\_name\_H-M 'P 1'

\_symmetry\_Int\_Tables\_number 1

\_symmetry\_cell\_setting triclinic

loop\_

\_atom\_site\_label

\_atom\_site\_type\_symbol

\_atom\_site\_fract\_x

\_atom\_site\_fract\_y

\_atom\_site\_fract\_z

\_atom\_site\_occupancy

|     |   |                    |                    |                    |     |
|-----|---|--------------------|--------------------|--------------------|-----|
| H1  | H | 0.6151552300000000 | 0.8983597400000000 | 0.8621582700000000 | 1.0 |
| H2  | H | 0.6074574600000000 | 0.9381900500000000 | 0.1188095300000000 | 1.0 |
| H3  | H | 0.5258558500000000 | 0.0567736400000000 | 0.0785727500000000 | 1.0 |
| H4  | H | 0.5609449500000000 | 0.8489067100000000 | 0.9312570900000000 | 1.0 |
| H5  | H | 0.5473981900000000 | 0.1135141700000000 | 0.9545708600000000 | 1.0 |
| H6  | H | 0.4398289900000000 | 0.9011949500000000 | 0.8877920500000000 | 1.0 |
| H7  | H | 0.4682901400000000 | 0.8843933400000000 | 0.1002493800000000 | 1.0 |
| H8  | H | 0.6264468500000000 | 0.8740709500000000 | 0.0581909100000000 | 1.0 |
| H9  | H | 0.7019818400000000 | 0.0641357300000000 | 0.1174474100000000 | 1.0 |
| H10 | H | 0.7781159400000000 | 0.9373818700000000 | 0.0638519800000000 | 1.0 |
| H11 | H | 0.9041318700000000 | 0.1480382700000000 | 0.9490665000000000 | 1.0 |
| H12 | H | 0.7932198300000000 | 0.9185142100000000 | 0.9239491000000000 | 1.0 |
| H13 | H | 0.7525425000000000 | 0.1480099700000000 | 0.8981698700000000 | 1.0 |
| H14 | H | 0.8784847600000000 | 0.0542780600000000 | 0.1388718400000000 | 1.0 |
| H15 | H | 0.8232608900000000 | 0.1280167200000000 | 0.0981810900000000 | 1.0 |
| H16 | H | 0.7440710000000000 | 0.1760026200000000 | 0.9824238500000000 | 1.0 |
| H17 | H | 0.0893224800000000 | 0.8239886100000000 | 0.9827551600000000 | 1.0 |
| H18 | H | 0.1314673000000000 | 0.9362320300000000 | 0.1175388300000000 | 1.0 |
| H19 | H | 0.0551987100000000 | 0.0628213600000000 | 0.0636768400000000 | 1.0 |
| H20 | H | 0.9291360100000000 | 0.8518557200000000 | 0.9494568400000000 | 1.0 |
| H21 | H | 0.0401341800000000 | 0.0813546300000000 | 0.9237567400000000 | 1.0 |
| H22 | H | 0.0805758100000000 | 0.8518157200000000 | 0.8984550700000000 | 1.0 |
| H23 | H | 0.9549906300000000 | 0.9461151000000000 | 0.1390029300000000 | 1.0 |
| H24 | H | 0.0102178300000000 | 0.8722754200000000 | 0.0984907000000000 | 1.0 |
| H25 | H | 0.2254767500000000 | 0.0617098300000000 | 0.1187263000000000 | 1.0 |
| H26 | H | 0.3075675100000000 | 0.9432374500000000 | 0.0786310100000000 | 1.0 |
| H27 | H | 0.2723891000000000 | 0.1510146300000000 | 0.9311871200000000 | 1.0 |
| H28 | H | 0.2858566900000000 | 0.8864184000000000 | 0.9546718400000000 | 1.0 |
| H29 | H | 0.3935213800000000 | 0.0987090000000000 | 0.8877559600000000 | 1.0 |
| H30 | H | 0.3650694000000000 | 0.1153515900000000 | 0.1004801800000000 | 1.0 |

|     |   |                    |                    |                    |     |
|-----|---|--------------------|--------------------|--------------------|-----|
| H31 | H | 0.2072196800000000 | 0.1259974600000000 | 0.0582336300000000 | 1.0 |
| H32 | H | 0.2182131400000000 | 0.1015403500000000 | 0.8621008400000000 | 1.0 |
| C33 | C | 0.5824419500000000 | 0.9544994900000000 | 0.9528793700000000 | 1.0 |
| C34 | C | 0.5009475600000000 | 0.9594692700000000 | 0.0225048700000000 | 1.0 |
| C35 | C | 0.4982157700000000 | 0.0376777200000000 | 0.0290107000000000 | 1.0 |
| C36 | C | 0.5848302000000000 | 0.0645138700000000 | 0.9714427700000000 | 1.0 |
| C37 | C | 0.5463984900000000 | 0.8972592500000000 | 0.9059476300000000 | 1.0 |
| C38 | C | 0.5548506800000000 | 0.9120597900000000 | 0.0776431300000000 | 1.0 |
| C39 | C | 0.7534576700000000 | 0.0688698800000000 | 0.9717970000000000 | 1.0 |
| C40 | C | 0.8392219200000000 | 0.0421948300000000 | 0.0321866900000000 | 1.0 |
| C41 | C | 0.8297173800000000 | 0.9644639700000000 | 0.0238772000000000 | 1.0 |
| C42 | C | 0.7547903300000000 | 0.9587202100000000 | 0.9559838700000000 | 1.0 |
| C43 | C | 0.7921140000000000 | 0.1390379900000000 | 0.9489049000000000 | 1.0 |
| C44 | C | 0.8080489500000000 | 0.0734380000000000 | 0.1001527800000000 | 1.0 |
| C45 | C | 0.0798315300000000 | 0.9311001000000000 | 0.9719288200000000 | 1.0 |
| C46 | C | 0.9941111400000000 | 0.9579207000000000 | 0.0322730400000000 | 1.0 |
| C47 | C | 0.0035822900000000 | 0.0356343100000000 | 0.0237807400000000 | 1.0 |
| C48 | C | 0.0785108100000000 | 0.0412181100000000 | 0.9558937300000000 | 1.0 |
| C49 | C | 0.0411450700000000 | 0.8608792600000000 | 0.9491996700000000 | 1.0 |
| C50 | C | 0.0253792900000000 | 0.9268625100000000 | 0.1003111600000000 | 1.0 |
| C51 | C | 0.2508532000000000 | 0.0454363500000000 | 0.9528577300000000 | 1.0 |
| C52 | C | 0.3323691200000000 | 0.0405000900000000 | 0.0225078100000000 | 1.0 |
| C53 | C | 0.3351414100000000 | 0.9623042600000000 | 0.0290485000000000 | 1.0 |
| C54 | C | 0.2484747000000000 | 0.9354357700000000 | 0.9715217900000000 | 1.0 |
| C55 | C | 0.2869455500000000 | 0.1026509000000000 | 0.9058985200000000 | 1.0 |
| C56 | C | 0.2784748400000000 | 0.0878604600000000 | 0.0776921400000000 | 1.0 |
| O57 | O | 0.5498142300000000 | 0.0167596500000000 | 0.9207705700000000 | 1.0 |
| O58 | O | 0.7892867500000000 | 0.0200168400000000 | 0.9223288700000000 | 1.0 |
| O59 | O | 0.0440100400000000 | 0.9798523000000000 | 0.9223658000000000 | 1.0 |
| O60 | O | 0.2834921700000000 | 0.9831457800000000 | 0.9208077300000000 | 1.0 |

##### cif ends

furan\_CH3\_23\_anti\_alt\_forbid Energy: -359.58167842

##### cif starts

data\_furan\_CH3\_23\_anti\_alt\_forbid

\_publ\_section\_comment

;  
Andrew Reynoso, Bohan Xu, and Vincent H. Crespi  
;

\_cell\_length\_a 10.2873194371

\_cell\_length\_b 20.0

\_cell\_length\_c 20.0

\_cell\_angle\_alpha 90.0

\_cell\_angle\_beta 90.0

\_cell\_angle\_gamma 90.0

\_symmetry\_space\_group\_name\_H-M 'P 1'

\_symmetry\_Int\_Tables\_number 1

\_symmetry\_cell\_setting triclinic

loop\_

\_atom\_site\_label

|     | _atom_site_type_symbol | _atom_site_fract_x | _atom_site_fract_y | _atom_site_fract_z | _atom_site_occupancy |
|-----|------------------------|--------------------|--------------------|--------------------|----------------------|
| H1  | H                      | 0.9552651200000000 | 0.9337323200000000 | 0.0534042300000000 | 1.0                  |
| H2  | H                      | 0.0694741300000000 | 0.8958349100000000 | 0.9325821700000000 | 1.0                  |
| H3  | H                      | 0.3272095900000000 | 0.0592428400000000 | 0.9157415300000000 | 1.0                  |
| H4  | H                      | 0.2130549000000000 | 0.0971520000000000 | 0.0365881400000000 | 1.0                  |
| H5  | H                      | 0.4558652600000000 | 0.9334163100000000 | 0.0533438800000000 | 1.0                  |
| H6  | H                      | 0.5696259000000000 | 0.8960361800000000 | 0.9321849700000000 | 1.0                  |
| H7  | H                      | 0.8267235400000000 | 0.0595903400000000 | 0.9158068500000000 | 1.0                  |
| H8  | H                      | 0.7129174700000000 | 0.0969933300000000 | 0.0369470400000000 | 1.0                  |
| H9  | H                      | 0.4149796400000000 | 0.9355903600000000 | 0.8669145300000000 | 1.0                  |
| H10 | H                      | 0.2437605500000000 | 0.9298979100000000 | 0.8670419100000000 | 1.0                  |
| H11 | H                      | 0.3382659800000000 | 0.8650975000000000 | 0.9040535200000000 | 1.0                  |
| H12 | H                      | 0.9156406400000000 | 0.9359805200000000 | 0.8668460900000000 | 1.0                  |
| H13 | H                      | 0.7443534900000000 | 0.9306975100000000 | 0.8666343400000000 | 1.0                  |
| H14 | H                      | 0.8380125500000000 | 0.8655121400000000 | 0.9035323900000000 | 1.0                  |
| H15 | H                      | 0.1613344900000000 | 0.1279396100000000 | 0.8951392700000000 | 1.0                  |
| H16 | H                      | 0.0503927900000000 | 0.1611165500000000 | 0.9547490800000000 | 1.0                  |
| H17 | H                      | 0.9921198300000000 | 0.1151230300000000 | 0.8845561000000000 | 1.0                  |
| H18 | H                      | 0.6609211900000000 | 0.1285402800000000 | 0.8958698200000000 | 1.0                  |
| H19 | H                      | 0.5499721100000000 | 0.1611643500000000 | 0.9557700800000000 | 1.0                  |
| H20 | H                      | 0.4917045300000000 | 0.1156821200000000 | 0.8852514800000000 | 1.0                  |
| H21 | H                      | 0.0387053500000000 | 0.0630201200000000 | 0.1021594300000000 | 1.0                  |
| H22 | H                      | 0.8674756400000000 | 0.0574775100000000 | 0.1022256100000000 | 1.0                  |
| H23 | H                      | 0.9444678300000000 | 0.1278966900000000 | 0.0651092000000000 | 1.0                  |
| H24 | H                      | 0.5381971100000000 | 0.0624062100000000 | 0.1024922900000000 | 1.0                  |
| H25 | H                      | 0.3669215400000000 | 0.0570075100000000 | 0.1023110400000000 | 1.0                  |
| H26 | H                      | 0.4443349500000000 | 0.1275070200000000 | 0.0655770800000000 | 1.0                  |
| H27 | H                      | 0.2313504400000000 | 0.8318140200000000 | 0.0144080200000000 | 1.0                  |
| H28 | H                      | 0.1211942100000000 | 0.8652742300000000 | 0.0742450800000000 | 1.0                  |
| H29 | H                      | 0.2905973800000000 | 0.8777049800000000 | 0.0844589700000000 | 1.0                  |
| H30 | H                      | 0.7326522000000000 | 0.8318506100000000 | 0.0135284900000000 | 1.0                  |
| H31 | H                      | 0.6214696400000000 | 0.8645341500000000 | 0.0732856600000000 | 1.0                  |
| H32 | H                      | 0.7906179200000000 | 0.8774631600000000 | 0.0840368600000000 | 1.0                  |
| C33 | C                      | 0.0700388500000000 | 0.1182312000000000 | 0.9218889300000000 | 1.0                  |
| C34 | C                      | 0.9515137400000000 | 0.0733914100000000 | 0.0724857200000000 | 1.0                  |
| C35 | C                      | 0.3310320400000000 | 0.9195985500000000 | 0.8966813800000000 | 1.0                  |
| C36 | C                      | 0.2123515300000000 | 0.8747571500000000 | 0.0472927100000000 | 1.0                  |
| C37 | C                      | 0.5696886200000000 | 0.1185504200000000 | 0.9225642400000000 | 1.0                  |
| C38 | C                      | 0.4511665700000000 | 0.0729714300000000 | 0.0727522700000000 | 1.0                  |
| C39 | C                      | 0.8313372600000000 | 0.9200568600000000 | 0.8963822500000000 | 1.0                  |
| C40 | C                      | 0.7127771000000000 | 0.8745085600000000 | 0.0466505500000000 | 1.0                  |
| C41 | C                      | 0.0779676500000000 | 0.0543299700000000 | 0.9625602000000000 | 1.0                  |
| C42 | C                      | 0.9557216400000000 | 0.0368941700000000 | 0.0055508600000000 | 1.0                  |
| C43 | C                      | 0.9574345600000000 | 0.9581047900000000 | 0.0043342700000000 | 1.0                  |
| C44 | C                      | 0.0789744100000000 | 0.9412243200000000 | 0.9630965700000000 | 1.0                  |
| C45 | C                      | 0.2035486500000000 | 0.0517686100000000 | 0.0060690400000000 | 1.0                  |
| C46 | C                      | 0.3250822600000000 | 0.0348851200000000 | 0.9648203200000000 | 1.0                  |
| C47 | C                      | 0.3268083600000000 | 0.9560906700000000 | 0.9636207800000000 | 1.0                  |
| C48 | C                      | 0.2045501700000000 | 0.9386600200000000 | 0.0066139900000000 | 1.0                  |
| C49 | C                      | 0.5778426200000000 | 0.0543907000000000 | 0.9628170200000000 | 1.0                  |
| C50 | C                      | 0.4556469000000000 | 0.0366970800000000 | 0.0057057700000000 | 1.0                  |



|     |   |                    |                    |                    |     |
|-----|---|--------------------|--------------------|--------------------|-----|
| C51 | C | 0.4575585900000000 | 0.9579194100000000 | 0.0043284400000000 | 1.0 |
| C52 | C | 0.5790293400000000 | 0.9413056200000000 | 0.9628813300000000 | 1.0 |
| C53 | C | 0.7035062600000000 | 0.0517206500000000 | 0.0062565000000000 | 1.0 |
| C54 | C | 0.8249889300000000 | 0.0350905700000000 | 0.9648223400000000 | 1.0 |
| C55 | C | 0.8268796000000000 | 0.9563110100000000 | 0.9634423200000000 | 1.0 |
| C56 | C | 0.7046793600000000 | 0.9386348300000000 | 0.0063315800000000 | 1.0 |
| O57 | O | 0.0873279500000000 | 0.9975501200000000 | 0.9173538000000000 | 1.0 |
| O58 | O | 0.1952120700000000 | 0.9954438200000000 | 0.0518163000000000 | 1.0 |
| O59 | O | 0.5871642100000000 | 0.9978138800000000 | 0.9173480000000000 | 1.0 |
| O60 | O | 0.6953681100000000 | 0.9952202900000000 | 0.0517897500000000 | 1.0 |

##### cif ends

furán\_CH3\_23\_anti\_dir Energy: -356.76254651

##### cif starts

data\_furan\_CH3\_23\_anti\_dir

\_publ\_section\_comment

;  
Andrew Reynoso, Bohan Xu, and Vincent H. Crespi  
;

\_cell\_length\_a 9.7787931765

\_cell\_length\_b 20.0

\_cell\_length\_c 20.0

\_cell\_angle\_alpha 90.0

\_cell\_angle\_beta 90.0

\_cell\_angle\_gamma 90.0

\_symmetry\_space\_group\_name\_H-M 'P 1'

\_symmetry\_Int\_Tables\_number 1

\_symmetry\_cell\_setting triclinic

loop\_

\_atom\_site\_label

\_atom\_site\_type\_symbol

\_atom\_site\_fract\_x

\_atom\_site\_fract\_y

\_atom\_site\_fract\_z

\_atom\_site\_occupancy

|     |   |                    |                    |                    |     |
|-----|---|--------------------|--------------------|--------------------|-----|
| H1  | H | 0.6271502200000000 | 0.8840767800000000 | 0.9526629800000000 | 1.0 |
| H2  | H | 0.6321153400000000 | 0.9983305000000000 | 0.1195085400000000 | 1.0 |
| H3  | H | 0.5335549800000000 | 0.1040931100000000 | 0.0788931900000000 | 1.0 |
| H4  | H | 0.4508441800000000 | 0.9021855400000000 | 0.9505362400000000 | 1.0 |
| H5  | H | 0.5550418800000000 | 0.1467609000000000 | 0.9461186400000000 | 1.0 |
| H6  | H | 0.5556882200000000 | 0.9243623000000000 | 0.8825187100000000 | 1.0 |
| H7  | H | 0.4573362700000000 | 0.9924175800000000 | 0.1391239700000000 | 1.0 |
| H8  | H | 0.5427928000000000 | 0.9226885400000000 | 0.1042423900000000 | 1.0 |
| H9  | H | 0.7008137600000000 | 0.8989517600000000 | 0.0424971800000000 | 1.0 |
| H10 | H | 0.8821153200000000 | 0.0067346500000000 | 0.8806813500000000 | 1.0 |
| H11 | H | 0.7835724000000000 | 0.1093746600000000 | 0.9286445700000000 | 1.0 |
| H12 | H | 0.8770935000000000 | 0.8810060200000000 | 0.0389386900000000 | 1.0 |
| H13 | H | 0.8049982800000000 | 0.1425870300000000 | 0.0640972900000000 | 1.0 |
| H14 | H | 0.8059148800000000 | 0.9161935000000000 | 0.1118414200000000 | 1.0 |
| H15 | H | 0.7928750800000000 | 0.9301878200000000 | 0.8906264700000000 | 1.0 |

|     |   |                    |                    |                    |     |
|-----|---|--------------------|--------------------|--------------------|-----|
| H16 | H | 0.7073446900000000 | 0.0021592900000000 | 0.8606990800000000 | 1.0 |
| H17 | H | 0.1272684500000000 | 0.8841027800000000 | 0.9526372900000000 | 1.0 |
| H18 | H | 0.1321242600000000 | 0.9983355800000000 | 0.1195089200000000 | 1.0 |
| H19 | H | 0.0335410300000000 | 0.1040804400000000 | 0.0789066900000000 | 1.0 |
| H20 | H | 0.9509402500000000 | 0.9021622600000000 | 0.9505259200000000 | 1.0 |
| H21 | H | 0.0549878400000000 | 0.1467711000000000 | 0.9461384500000000 | 1.0 |
| H22 | H | 0.0557443400000000 | 0.9243780100000000 | 0.8825053700000000 | 1.0 |
| H23 | H | 0.9573501500000000 | 0.9924004000000000 | 0.1391232200000000 | 1.0 |
| H24 | H | 0.0428418100000000 | 0.9226819300000000 | 0.1042395100000000 | 1.0 |
| H25 | H | 0.2008357300000000 | 0.8989535600000000 | 0.0424577500000000 | 1.0 |
| H26 | H | 0.2073072800000000 | 0.0022320300000000 | 0.8606912500000000 | 1.0 |
| H27 | H | 0.2835302300000000 | 0.1094084800000000 | 0.9286450900000000 | 1.0 |
| H28 | H | 0.3771310100000000 | 0.8810296500000000 | 0.0389818300000000 | 1.0 |
| H29 | H | 0.3050225400000000 | 0.1426063200000000 | 0.0640949200000000 | 1.0 |
| H30 | H | 0.3058021800000000 | 0.9162340900000000 | 0.1118401300000000 | 1.0 |
| H31 | H | 0.3820834900000000 | 0.0068339000000000 | 0.8806589800000000 | 1.0 |
| H32 | H | 0.2929226000000000 | 0.9302606700000000 | 0.8905620200000000 | 1.0 |
| C33 | C | 0.5820128200000000 | 0.9891612200000000 | 0.9694233400000000 | 1.0 |
| C34 | C | 0.4936451900000000 | 0.0046583500000000 | 0.0336918800000000 | 1.0 |
| C35 | C | 0.4902175500000000 | 0.0831003900000000 | 0.0327250200000000 | 1.0 |
| C36 | C | 0.5789593000000000 | 0.0990474400000000 | 0.9706954600000000 | 1.0 |
| C37 | C | 0.5514039500000000 | 0.9213615500000000 | 0.9370903500000000 | 1.0 |
| C38 | C | 0.5354760900000000 | 0.9773264500000000 | 0.1028799700000000 | 1.0 |
| C39 | C | 0.8320165900000000 | 0.9870221800000000 | 0.0297480700000000 | 1.0 |
| C40 | C | 0.7436493100000000 | 0.0070084900000000 | 0.9667312700000000 | 1.0 |
| C41 | C | 0.7402250200000000 | 0.0851846300000000 | 0.9732189000000000 | 1.0 |
| C42 | C | 0.8289434000000000 | 0.0967255200000000 | 0.0362235200000000 | 1.0 |
| C43 | C | 0.8014391000000000 | 0.9170974000000000 | 0.0571988100000000 | 1.0 |
| C44 | C | 0.7855008400000000 | 0.9845952900000000 | 0.8958035200000000 | 1.0 |
| C45 | C | 0.0820250800000000 | 0.9891702900000000 | 0.9694175800000000 | 1.0 |
| C46 | C | 0.9936546500000000 | 0.0046498400000000 | 0.0336924600000000 | 1.0 |
| C47 | C | 0.9902080600000000 | 0.0830917100000000 | 0.0327358500000000 | 1.0 |
| C48 | C | 0.0789334400000000 | 0.0990565500000000 | 0.9707065800000000 | 1.0 |
| C49 | C | 0.0514732500000000 | 0.9213685000000000 | 0.9370768700000000 | 1.0 |
| C50 | C | 0.0354970100000000 | 0.9773187800000000 | 0.1028788000000000 | 1.0 |
| C51 | C | 0.3320129600000000 | 0.9870405600000000 | 0.0297398300000000 | 1.0 |
| C52 | C | 0.2436495900000000 | 0.0070343600000000 | 0.9667204600000000 | 1.0 |
| C53 | C | 0.2402061500000000 | 0.0852084100000000 | 0.9732192900000000 | 1.0 |
| C54 | C | 0.3289473500000000 | 0.0967445500000000 | 0.0362172900000000 | 1.0 |
| C55 | C | 0.3014242300000000 | 0.9171176400000000 | 0.0571954200000000 | 1.0 |
| C56 | C | 0.2854939900000000 | 0.9846618500000000 | 0.8957756900000000 | 1.0 |
| O57 | O | 0.5385898100000000 | 0.0453026700000000 | 0.9268187700000000 | 1.0 |
| O58 | O | 0.7885730600000000 | 0.0400153300000000 | 0.0762054800000000 | 1.0 |
| O59 | O | 0.0385657000000000 | 0.0453140100000000 | 0.9268234700000000 | 1.0 |
| O60 | O | 0.2885714900000000 | 0.0400348600000000 | 0.0761979700000000 | 1.0 |

##### cif ends

furan\_CH3\_23\_anti\_dir\_forbid    Energy: -357.45776164

##### cif starts

data\_furan\_CH3\_23\_anti\_dir\_forbid

\_publ\_section\_comment

;  
Andrew Reynoso, Bohan Xu, and Vincent H. Crespi

;

\_cell\_length\_a 10.4610703199  
\_cell\_length\_b 20.0  
\_cell\_length\_c 20.0  
\_cell\_angle\_alpha 90.0  
\_cell\_angle\_beta 90.0  
\_cell\_angle\_gamma 90.0

\_symmetry\_space\_group\_name\_H-M 'P 1'  
\_symmetry\_Int\_Tables\_number 1  
\_symmetry\_cell\_setting triclinic

loop\_  
\_atom\_site\_label  
\_atom\_site\_type\_symbol  
\_atom\_site\_fract\_x  
\_atom\_site\_fract\_y  
\_atom\_site\_fract\_z  
\_atom\_site\_occupancy

|     |   |                    |                    |                    |     |
|-----|---|--------------------|--------------------|--------------------|-----|
| H1  | H | 0.1619775200000000 | 0.8606460100000000 | 0.9327613800000000 | 1.0 |
| H2  | H | 0.0444196000000000 | 0.9630639500000000 | 0.1108084600000000 | 1.0 |
| H3  | H | 0.9603629100000000 | 0.0761794000000000 | 0.0614256400000000 | 1.0 |
| H4  | H | 0.9961097200000000 | 0.8579336700000000 | 0.9476642800000000 | 1.0 |
| H5  | H | 0.0777060300000000 | 0.1146908000000000 | 0.9410072700000000 | 1.0 |
| H6  | H | 0.0567664500000000 | 0.8997127800000000 | 0.8762678200000000 | 1.0 |
| H7  | H | 0.8763486700000000 | 0.9659289800000000 | 0.1110993100000000 | 1.0 |
| H8  | H | 0.9557914700000000 | 0.8913144800000000 | 0.0870926600000000 | 1.0 |
| H9  | H | 0.1290832000000000 | 0.8586890200000000 | 0.0464577800000000 | 1.0 |
| H10 | H | 0.2466551500000000 | 0.9673082000000000 | 0.8720420100000000 | 1.0 |
| H11 | H | 0.3307173500000000 | 0.0785596300000000 | 0.9253529500000000 | 1.0 |
| H12 | H | 0.2949560500000000 | 0.8564655000000000 | 0.0314850400000000 | 1.0 |
| H13 | H | 0.2133998300000000 | 0.1128369800000000 | 0.0470516700000000 | 1.0 |
| H14 | H | 0.2342847300000000 | 0.8957956500000000 | 0.1042594100000000 | 1.0 |
| H15 | H | 0.4147253000000000 | 0.9701340900000000 | 0.8718492600000000 | 1.0 |
| H16 | H | 0.3352072500000000 | 0.8947337400000000 | 0.8931952800000000 | 1.0 |
| H17 | H | 0.6619396300000000 | 0.8606465100000000 | 0.9327286800000000 | 1.0 |
| H18 | H | 0.5445146000000000 | 0.9630344800000000 | 0.1107937100000000 | 1.0 |
| H19 | H | 0.4603984300000000 | 0.0761665800000000 | 0.0614512900000000 | 1.0 |
| H20 | H | 0.4960698900000000 | 0.8579475200000000 | 0.9476183900000000 | 1.0 |
| H21 | H | 0.5776823000000000 | 0.1146986200000000 | 0.9410229600000000 | 1.0 |
| H22 | H | 0.5567596000000000 | 0.8997384200000000 | 0.8762386900000000 | 1.0 |
| H23 | H | 0.3764422300000000 | 0.9659204100000000 | 0.1111299200000000 | 1.0 |
| H24 | H | 0.4558332000000000 | 0.8912949800000000 | 0.0870880700000000 | 1.0 |
| H25 | H | 0.6291388600000000 | 0.8586400000000000 | 0.0463528900000000 | 1.0 |
| H26 | H | 0.7466459000000000 | 0.9672798900000000 | 0.8720232200000000 | 1.0 |
| H27 | H | 0.8306975700000000 | 0.0785544100000000 | 0.9253257000000000 | 1.0 |
| H28 | H | 0.7950374200000000 | 0.8564716000000000 | 0.0314566900000000 | 1.0 |
| H29 | H | 0.7134395600000000 | 0.1128222400000000 | 0.0470440200000000 | 1.0 |
| H30 | H | 0.7342035000000000 | 0.8957490800000000 | 0.1042215200000000 | 1.0 |
| H31 | H | 0.9147236300000000 | 0.9701126900000000 | 0.8718184400000000 | 1.0 |
| H32 | H | 0.8352162800000000 | 0.8947124400000000 | 0.8931901100000000 | 1.0 |
| C33 | C | 0.0824765700000000 | 0.9551115700000000 | 0.9697500500000000 | 1.0 |
| C34 | C | 0.9612910300000000 | 0.9737826700000000 | 0.0129598700000000 | 1.0 |
| C35 | C | 0.9612010600000000 | 0.0524910200000000 | 0.0118244200000000 | 1.0 |

|     |   |                    |                    |                    |     |
|-----|---|--------------------|--------------------|--------------------|-----|
| C36 | C | 0.0833714700000000 | 0.0688149100000000 | 0.9713000100000000 | 1.0 |
| C37 | C | 0.0738192600000000 | 0.8897659200000000 | 0.9292533200000000 | 1.0 |
| C38 | C | 0.9590981900000000 | 0.9459762500000000 | 0.0843073300000000 | 1.0 |
| C39 | C | 0.2086064600000000 | 0.9543621100000000 | 0.0127441800000000 | 1.0 |
| C40 | C | 0.3297845900000000 | 0.9745342700000000 | 0.9702025200000000 | 1.0 |
| C41 | C | 0.3298852100000000 | 0.0531511000000000 | 0.9740957100000000 | 1.0 |
| C42 | C | 0.2077230500000000 | 0.0680470700000000 | 0.0151755300000000 | 1.0 |
| C43 | C | 0.2172533300000000 | 0.8876598700000000 | 0.0509631000000000 | 1.0 |
| C44 | C | 0.3319570500000000 | 0.9492627000000000 | 0.8979186200000000 | 1.0 |
| C45 | C | 0.5824695800000000 | 0.9551120400000000 | 0.9697355800000000 | 1.0 |
| C46 | C | 0.4613027600000000 | 0.9737779900000000 | 0.0129687200000000 | 1.0 |
| C47 | C | 0.4612138700000000 | 0.0524886700000000 | 0.0118434300000000 | 1.0 |
| C48 | C | 0.5833671200000000 | 0.0688180900000000 | 0.9713069000000000 | 1.0 |
| C49 | C | 0.5737947100000000 | 0.8897763900000000 | 0.9292226600000000 | 1.0 |
| C50 | C | 0.4591575100000000 | 0.9459594200000000 | 0.0843126700000000 | 1.0 |
| C51 | C | 0.7086138900000000 | 0.9543514900000000 | 0.0127176900000000 | 1.0 |
| C52 | C | 0.8297883700000000 | 0.9745291500000000 | 0.9701794800000000 | 1.0 |
| C53 | C | 0.8298802400000000 | 0.0531475100000000 | 0.9740699800000000 | 1.0 |
| C54 | C | 0.7077329600000000 | 0.0680382200000000 | 0.0151626900000000 | 1.0 |
| C55 | C | 0.7172708600000000 | 0.8876351800000000 | 0.0509138500000000 | 1.0 |
| C56 | C | 0.8319617400000000 | 0.9492451400000000 | 0.8979003800000000 | 1.0 |
| O57 | O | 0.0911150500000000 | 0.0132033400000000 | 0.9252783300000000 | 1.0 |
| O58 | O | 0.1999628100000000 | 0.0108593700000000 | 0.0592166200000000 | 1.0 |
| O59 | O | 0.5910938100000000 | 0.0132122700000000 | 0.9252753500000000 | 1.0 |
| O60 | O | 0.6999862000000000 | 0.0108444500000000 | 0.0591977500000000 | 1.0 |

##### cif ends

furan\_CH3\_23\_syn\_alt Energy: -359.37958489

##### cif starts

data\_furan\_CH3\_23\_syn\_alt

\_publ\_section\_comment

;  
Andrew Reynoso, Bohan Xu, and Vincent H. Crespi  
;

\_cell\_length\_a 10.4238853323

\_cell\_length\_b 20.0

\_cell\_length\_c 20.0

\_cell\_angle\_alpha 90.0

\_cell\_angle\_beta 90.0

\_cell\_angle\_gamma 90.0

\_symmetry\_space\_group\_name\_H-M 'P 1'

\_symmetry\_Int\_Tables\_number 1

\_symmetry\_cell\_setting triclinic

loop\_

\_atom\_site\_label

\_atom\_site\_type\_symbol

\_atom\_site\_fract\_x

\_atom\_site\_fract\_y

\_atom\_site\_fract\_z

\_atom\_site\_occupancy

|     |   |                   |                   |                   |     |
|-----|---|-------------------|-------------------|-------------------|-----|
| H1  | H | 0.054917300000000 | 0.110655390000000 | 0.101407840000000 | 1.0 |
| H2  | H | 0.180795700000000 | 0.050598810000000 | 0.886712050000000 | 1.0 |
| H3  | H | 0.098826530000000 | 0.926098220000000 | 0.937495830000000 | 1.0 |
| H4  | H | 0.977326050000000 | 0.151892250000000 | 0.033362110000000 | 1.0 |
| H5  | H | 0.969873800000000 | 0.886964670000000 | 0.050584790000000 | 1.0 |
| H6  | H | 0.886270330000000 | 0.113711550000000 | 0.098393410000000 | 1.0 |
| H7  | H | 0.012247530000000 | 0.045824820000000 | 0.885077350000000 | 1.0 |
| H8  | H | 0.088360010000000 | 0.116882530000000 | 0.920026400000000 | 1.0 |
| H9  | H | 0.136008930000000 | 0.865825360000000 | 0.098757990000000 | 1.0 |
| H10 | H | 0.261987330000000 | 0.932727480000000 | 0.885353060000000 | 1.0 |
| H11 | H | 0.348941810000000 | 0.052806970000000 | 0.937319420000000 | 1.0 |
| H12 | H | 0.226915460000000 | 0.827327580000000 | 0.033859810000000 | 1.0 |
| H13 | H | 0.219985970000000 | 0.092312160000000 | 0.050294310000000 | 1.0 |
| H14 | H | 0.304665110000000 | 0.868714980000000 | 0.101770630000000 | 1.0 |
| H15 | H | 0.430582030000000 | 0.928501870000000 | 0.886774820000000 | 1.0 |
| H16 | H | 0.339102860000000 | 0.861986280000000 | 0.920350410000000 | 1.0 |
| H17 | H | 0.554861110000000 | 0.110930490000000 | 0.101189530000000 | 1.0 |
| H18 | H | 0.680916720000000 | 0.051042320000000 | 0.886871390000000 | 1.0 |
| H19 | H | 0.598839560000000 | 0.926142170000000 | 0.937483030000000 | 1.0 |
| H20 | H | 0.475950510000000 | 0.151857080000000 | 0.033366860000000 | 1.0 |
| H21 | H | 0.469979240000000 | 0.886916940000000 | 0.050608220000000 | 1.0 |
| H22 | H | 0.386148370000000 | 0.113336020000000 | 0.098670610000000 | 1.0 |
| H23 | H | 0.512458180000000 | 0.045557520000000 | 0.885028630000000 | 1.0 |
| H24 | H | 0.587300600000000 | 0.116908740000000 | 0.920119800000000 | 1.0 |
| H25 | H | 0.636104560000000 | 0.865521740000000 | 0.098464610000000 | 1.0 |
| H26 | H | 0.762014330000000 | 0.932832640000000 | 0.885310780000000 | 1.0 |
| H27 | H | 0.848867480000000 | 0.052924010000000 | 0.937353870000000 | 1.0 |
| H28 | H | 0.728032960000000 | 0.827363950000000 | 0.033756490000000 | 1.0 |
| H29 | H | 0.719931990000000 | 0.092312720000000 | 0.050399190000000 | 1.0 |
| H30 | H | 0.804694170000000 | 0.868935850000000 | 0.101887350000000 | 1.0 |
| H31 | H | 0.930620620000000 | 0.928707060000000 | 0.886728150000000 | 1.0 |
| H32 | H | 0.839296450000000 | 0.862112720000000 | 0.920262120000000 | 1.0 |
| C33 | C | 0.971063120000000 | 0.043629240000000 | 0.028717280000000 | 1.0 |
| C34 | C | 0.095860750000000 | 0.028842790000000 | 0.984381750000000 | 1.0 |
| C35 | C | 0.096453470000000 | 0.950202930000000 | 0.986624070000000 | 1.0 |
| C36 | C | 0.970982960000000 | 0.935692710000000 | 0.025662570000000 | 1.0 |
| C37 | C | 0.972500320000000 | 0.108782440000000 | 0.067415610000000 | 1.0 |
| C38 | C | 0.093994360000000 | 0.062049060000000 | 0.915583610000000 | 1.0 |
| C39 | C | 0.221020040000000 | 0.935585010000000 | 0.028857770000000 | 1.0 |
| C40 | C | 0.345866940000000 | 0.950206950000000 | 0.984505970000000 | 1.0 |
| C41 | C | 0.346468700000000 | 0.028848740000000 | 0.986517880000000 | 1.0 |
| C42 | C | 0.221003920000000 | 0.043515970000000 | 0.025504280000000 | 1.0 |
| C43 | C | 0.222264250000000 | 0.870558150000000 | 0.067766560000000 | 1.0 |
| C44 | C | 0.344064380000000 | 0.916826580000000 | 0.915788450000000 | 1.0 |
| C45 | C | 0.470996270000000 | 0.043580890000000 | 0.028743920000000 | 1.0 |
| C46 | C | 0.595827810000000 | 0.028861050000000 | 0.984427410000000 | 1.0 |
| C47 | C | 0.596468780000000 | 0.950210530000000 | 0.986629350000000 | 1.0 |
| C48 | C | 0.471010590000000 | 0.935646730000000 | 0.025683820000000 | 1.0 |
| C49 | C | 0.472112040000000 | 0.108735710000000 | 0.067440170000000 | 1.0 |
| C50 | C | 0.593815740000000 | 0.062104650000000 | 0.915645460000000 | 1.0 |
| C51 | C | 0.721074240000000 | 0.935604800000000 | 0.028826190000000 | 1.0 |
| C52 | C | 0.845880100000000 | 0.950291000000000 | 0.984473920000000 | 1.0 |
| C53 | C | 0.846462070000000 | 0.028933880000000 | 0.986538440000000 | 1.0 |
| C54 | C | 0.720985850000000 | 0.043541610000000 | 0.025557030000000 | 1.0 |
| C55 | C | 0.722573630000000 | 0.870550210000000 | 0.067687210000000 | 1.0 |

|     |   |                    |                    |                    |     |
|-----|---|--------------------|--------------------|--------------------|-----|
| C56 | C | 0.8441286300000000 | 0.9169591300000000 | 0.9157334900000000 | 1.0 |
| O57 | O | 0.9709313500000000 | 0.9879321200000000 | 0.0745872700000000 | 1.0 |
| O58 | O | 0.2209166500000000 | 0.9914147500000000 | 0.0745735800000000 | 1.0 |
| O59 | O | 0.4709126200000000 | 0.9878819100000000 | 0.0746097800000000 | 1.0 |
| O60 | O | 0.7209400100000000 | 0.9914008400000000 | 0.0745825800000000 | 1.0 |

##### cif ends

furan\_CH3\_23\_syn\_alt\_forbid    Energy: -356.01565391

##### cif starts

data\_furan\_CH3\_23\_syn\_alt\_forbid

\_publ\_section\_comment

;  
Andrew Reynoso, Bohan Xu, and Vincent H. Crespi  
;

\_cell\_length\_a    9.6696572061

\_cell\_length\_b    20.0

\_cell\_length\_c    20.0

\_cell\_angle\_alpha    90.0

\_cell\_angle\_beta    90.0

\_cell\_angle\_gamma    90.0

\_symmetry\_space\_group\_name\_H-M    'P 1'

\_symmetry\_Int\_Tables\_number 1

\_symmetry\_cell\_setting triclinic

loop\_

\_atom\_site\_label

\_atom\_site\_type\_symbol

\_atom\_site\_fract\_x

\_atom\_site\_fract\_y

\_atom\_site\_fract\_z

\_atom\_site\_occupancy

|     |   |                    |                    |                    |     |
|-----|---|--------------------|--------------------|--------------------|-----|
| H1  | H | 0.9982292500000000 | 0.0915659100000000 | 0.0719632300000000 | 1.0 |
| H2  | H | 0.9955175600000000 | 0.0667390500000000 | 0.9356151800000000 | 1.0 |
| H3  | H | 0.2544878300000000 | 0.9256190600000000 | 0.9385092900000000 | 1.0 |
| H4  | H | 0.2545812100000000 | 0.9072946100000000 | 0.0759859900000000 | 1.0 |
| H5  | H | 0.4970345900000000 | 0.0898560600000000 | 0.0730498900000000 | 1.0 |
| H6  | H | 0.4968183900000000 | 0.0671578000000000 | 0.9362398900000000 | 1.0 |
| H7  | H | 0.7558663200000000 | 0.9255753600000000 | 0.9380319300000000 | 1.0 |
| H8  | H | 0.7527969400000000 | 0.9055185300000000 | 0.0751375900000000 | 1.0 |
| H9  | H | 0.3273346900000000 | 0.0506960500000000 | 0.8641558300000000 | 1.0 |
| H10 | H | 0.2509998300000000 | 0.1198497700000000 | 0.9048577900000000 | 1.0 |
| H11 | H | 0.1493110900000000 | 0.0493027500000000 | 0.8830690800000000 | 1.0 |
| H12 | H | 0.8267053200000000 | 0.0514004300000000 | 0.8649184900000000 | 1.0 |
| H13 | H | 0.7468197700000000 | 0.1195022300000000 | 0.9058304700000000 | 1.0 |
| H14 | H | 0.6487715900000000 | 0.0479046600000000 | 0.8835192300000000 | 1.0 |
| H15 | H | 0.1024433800000000 | 0.9429846500000000 | 0.8852530900000000 | 1.0 |
| H16 | H | 0.9245105900000000 | 0.9381752200000000 | 0.8669600500000000 | 1.0 |
| H17 | H | 0.0055949400000000 | 0.8718823700000000 | 0.9102184400000000 | 1.0 |
| H18 | H | 0.6020914000000000 | 0.9417023600000000 | 0.8848259100000000 | 1.0 |
| H19 | H | 0.4240841700000000 | 0.9398406800000000 | 0.8658878000000000 | 1.0 |
| H20 | H | 0.5001495700000000 | 0.8719487700000000 | 0.9087764800000000 | 1.0 |

|     |   |                    |                    |                    |     |
|-----|---|--------------------|--------------------|--------------------|-----|
| H21 | H | 0.0853286000000000 | 0.8327971100000000 | 0.0367049400000000 | 1.0 |
| H22 | H | 0.9118949800000000 | 0.8540464200000000 | 0.0551069000000000 | 1.0 |
| H23 | H | 0.0433509000000000 | 0.8664595500000000 | 0.1163326700000000 | 1.0 |
| H24 | H | 0.5843497300000000 | 0.8316574000000000 | 0.0340683300000000 | 1.0 |
| H25 | H | 0.4103801200000000 | 0.8527500700000000 | 0.0514982200000000 | 1.0 |
| H26 | H | 0.5398941800000000 | 0.8639372200000000 | 0.1139617800000000 | 1.0 |
| H27 | H | 0.3408290800000000 | 0.1435481900000000 | 0.0470867300000000 | 1.0 |
| H28 | H | 0.2108737400000000 | 0.1343686600000000 | 0.1096604500000000 | 1.0 |
| H29 | H | 0.1669827000000000 | 0.1640874300000000 | 0.0287084100000000 | 1.0 |
| H30 | H | 0.8393369200000000 | 0.1425657200000000 | 0.0492647100000000 | 1.0 |
| H31 | H | 0.7098747100000000 | 0.1319069600000000 | 0.1118194800000000 | 1.0 |
| H32 | H | 0.6651944600000000 | 0.1629124200000000 | 0.0314590400000000 | 1.0 |
| C33 | C | 0.0322610000000000 | 0.0493441300000000 | 0.0413357600000000 | 1.0 |
| C34 | C | 0.9526347000000000 | 0.0373026600000000 | 0.9768092600000000 | 1.0 |
| C35 | C | 0.9640000000000000 | 0.9589872100000000 | 0.9719786300000000 | 1.0 |
| C36 | C | 0.0515251200000000 | 0.9392089600000000 | 0.0365473300000000 | 1.0 |
| C37 | C | 0.0026467100000000 | 0.9267499100000000 | 0.9052540900000000 | 1.0 |
| C38 | C | 0.0193914700000000 | 0.8693644900000000 | 0.0627055600000000 | 1.0 |
| C39 | C | 0.2005358900000000 | 0.0577497200000000 | 0.0335598300000000 | 1.0 |
| C40 | C | 0.2877872000000000 | 0.0349045900000000 | 0.9700608600000000 | 1.0 |
| C41 | C | 0.2984347700000000 | 0.9568275200000000 | 0.9780820900000000 | 1.0 |
| C42 | C | 0.2199097900000000 | 0.9479708800000000 | 0.0434902500000000 | 1.0 |
| C43 | C | 0.2334253800000000 | 0.1287722100000000 | 0.0561045900000000 | 1.0 |
| C44 | C | 0.2504110500000000 | 0.0648094900000000 | 0.9021252700000000 | 1.0 |
| C45 | C | 0.5315027700000000 | 0.0481357900000000 | 0.0418496100000000 | 1.0 |
| C46 | C | 0.4528876200000000 | 0.0372252600000000 | 0.9767916800000000 | 1.0 |
| C47 | C | 0.4635244900000000 | 0.9589293400000000 | 0.9712588600000000 | 1.0 |
| C48 | C | 0.5507346700000000 | 0.9380974500000000 | 0.0354621900000000 | 1.0 |
| C49 | C | 0.5009103200000000 | 0.9268749600000000 | 0.9043101900000000 | 1.0 |
| C50 | C | 0.5177141200000000 | 0.8678230600000000 | 0.0602182300000000 | 1.0 |
| C51 | C | 0.6998774400000000 | 0.0565941500000000 | 0.0344913700000000 | 1.0 |
| C52 | C | 0.7873582300000000 | 0.0345466300000000 | 0.9706428700000000 | 1.0 |
| C53 | C | 0.7987223800000000 | 0.9564398300000000 | 0.9781774700000000 | 1.0 |
| C54 | C | 0.7189976400000000 | 0.9466859500000000 | 0.0430495500000000 | 1.0 |
| C55 | C | 0.7322131600000000 | 0.1273146600000000 | 0.0581468200000000 | 1.0 |
| C56 | C | 0.7488980000000000 | 0.0644854400000000 | 0.9028378000000000 | 1.0 |
| O57 | O | 0.0073913500000000 | 0.9908007500000000 | 0.0810320000000000 | 1.0 |
| O58 | O | 0.2450545000000000 | 0.0083465000000000 | 0.0803388600000000 | 1.0 |
| O59 | O | 0.5062841500000000 | 0.9889877400000000 | 0.0806333300000000 | 1.0 |
| O60 | O | 0.7439934300000000 | 0.0065475700000000 | 0.0807204400000000 | 1.0 |

##### cif ends

furan\_CH3\_23\_syn\_dir Energy: -355.98862887

##### cif starts

data\_furan\_CH3\_23\_syn\_dir

\_publ\_section\_comment

;  
Andrew Reynoso, Bohan Xu, and Vincent H. Crespi  
;

\_cell\_length\_a 10.5099390961

\_cell\_length\_b 20.0

\_cell\_length\_c 20.0

\_cell\_angle\_alpha 90.0  
\_cell\_angle\_beta 90.0  
\_cell\_angle\_gamma 90.0

\_symmetry\_space\_group\_name\_H-M 'P 1'  
\_symmetry\_Int\_Tables\_number 1  
\_symmetry\_cell\_setting triclinic

loop\_

\_atom\_site\_label

\_atom\_site\_type\_symbol

\_atom\_site\_fract\_x

\_atom\_site\_fract\_y

\_atom\_site\_fract\_z

\_atom\_site\_occupancy

|     |   |                    |                    |                    |     |
|-----|---|--------------------|--------------------|--------------------|-----|
| H1  | H | 0.9884142100000000 | 0.8976509000000000 | 0.0849806400000000 | 1.0 |
| H2  | H | 0.1037495200000000 | 0.9362352400000000 | 0.9072699600000000 | 1.0 |
| H3  | H | 0.1042268900000000 | 0.0888582500000000 | 0.9275216300000000 | 1.0 |
| H4  | H | 0.0151591100000000 | 0.9655442100000000 | 0.1402777900000000 | 1.0 |
| H5  | H | 0.9891136700000000 | 0.1571379700000000 | 0.0342607000000000 | 1.0 |
| H6  | H | 0.8593752500000000 | 0.9474077200000000 | 0.1155770900000000 | 1.0 |
| H7  | H | 0.1873986500000000 | 0.9026731000000000 | 0.9751318700000000 | 1.0 |
| H8  | H | 0.0208336800000000 | 0.9025821300000000 | 0.9753539600000000 | 1.0 |
| H9  | H | 0.1935101200000000 | 0.9650380900000000 | 0.1401319500000000 | 1.0 |
| H10 | H | 0.2223121400000000 | 0.0104677000000000 | 0.8916851500000000 | 1.0 |
| H11 | H | 0.3756634000000000 | 0.1114168400000000 | 0.9382571500000000 | 1.0 |
| H12 | H | 0.2197191000000000 | 0.8973844600000000 | 0.0844847800000000 | 1.0 |
| H13 | H | 0.2190178800000000 | 0.1570185900000000 | 0.0345208400000000 | 1.0 |
| H14 | H | 0.3490832900000000 | 0.9468848800000000 | 0.1150897700000000 | 1.0 |
| H15 | H | 0.3838476900000000 | 0.0178282600000000 | 0.8743807600000000 | 1.0 |
| H16 | H | 0.3203895500000000 | 0.9384949300000000 | 0.8954495000000000 | 1.0 |
| H17 | H | 0.3680005700000000 | 0.8899499300000000 | 0.0186047100000000 | 1.0 |
| H18 | H | 0.6064950700000000 | 0.0245512600000000 | 0.8606668600000000 | 1.0 |
| H19 | H | 0.6038144400000000 | 0.1167551700000000 | 0.9461679900000000 | 1.0 |
| H20 | H | 0.5133692500000000 | 0.8809344100000000 | 0.9773788300000000 | 1.0 |
| H21 | H | 0.4819599700000000 | 0.1282783800000000 | 0.0702192000000000 | 1.0 |
| H22 | H | 0.5101713600000000 | 0.8902776000000000 | 0.0655231000000000 | 1.0 |
| H23 | H | 0.6859386400000000 | 0.9508697100000000 | 0.8854333200000000 | 1.0 |
| H24 | H | 0.5211748700000000 | 0.9524809100000000 | 0.8846496100000000 | 1.0 |
| H25 | H | 0.6943333100000000 | 0.8808177000000000 | 0.9784703400000000 | 1.0 |
| H26 | H | 0.8236320600000000 | 0.0173820200000000 | 0.8746073100000000 | 1.0 |
| H27 | H | 0.8325225000000000 | 0.1112538000000000 | 0.9380754600000000 | 1.0 |
| H28 | H | 0.8398347000000000 | 0.8900682300000000 | 0.0194975700000000 | 1.0 |
| H29 | H | 0.7261705700000000 | 0.1286443100000000 | 0.0699390200000000 | 1.0 |
| H30 | H | 0.6977927200000000 | 0.8909406000000000 | 0.0665292500000000 | 1.0 |
| H31 | H | 0.9853105500000000 | 0.0104077800000000 | 0.8917064500000000 | 1.0 |
| H32 | H | 0.8877084900000000 | 0.9382504600000000 | 0.8957901900000000 | 1.0 |
| C33 | C | 0.9754069000000000 | 0.9992664800000000 | 0.0421459500000000 | 1.0 |
| C34 | C | 0.1040421200000000 | 0.9987692900000000 | 0.0028681700000000 | 1.0 |
| C35 | C | 0.1040921600000000 | 0.0776093400000000 | 0.9812537200000000 | 1.0 |
| C36 | C | 0.9798868600000000 | 0.1046643200000000 | 0.0185530900000000 | 1.0 |
| C37 | C | 0.9576537500000000 | 0.9483403500000000 | 0.0980509200000000 | 1.0 |
| C38 | C | 0.1039947100000000 | 0.9326872700000000 | 0.9615584100000000 | 1.0 |
| C39 | C | 0.2327601300000000 | 0.9991441200000000 | 0.0420455700000000 | 1.0 |
| C40 | C | 0.3465260800000000 | 0.0096991800000000 | 0.9798031000000000 | 1.0 |



|     |   |                    |                    |                    |     |
|-----|---|--------------------|--------------------|--------------------|-----|
| C41 | C | 0.3584770800000000 | 0.0861810600000000 | 0.9862761200000000 | 1.0 |
| C42 | C | 0.2282614100000000 | 0.1045851600000000 | 0.0186871300000000 | 1.0 |
| C43 | C | 0.2507083800000000 | 0.9479913900000000 | 0.0977301000000000 | 1.0 |
| C44 | C | 0.3158496700000000 | 0.9921149300000000 | 0.9069120300000000 | 1.0 |
| C45 | C | 0.4762421300000000 | 0.9825267200000000 | 0.0082164800000000 | 1.0 |
| C46 | C | 0.6041150800000000 | 0.0059328100000000 | 0.9699989800000000 | 1.0 |
| C47 | C | 0.6040039000000000 | 0.0825642400000000 | 0.9892544300000000 | 1.0 |
| C48 | C | 0.4803931500000000 | 0.0883359700000000 | 0.0325834500000000 | 1.0 |
| C49 | C | 0.4666140300000000 | 0.9069971100000000 | 0.0187808500000000 | 1.0 |
| C50 | C | 0.6044314800000000 | 0.9828884300000000 | 0.8965001400000000 | 1.0 |
| C51 | C | 0.7318468700000000 | 0.9826449700000000 | 0.0085069100000000 | 1.0 |
| C52 | C | 0.8615568900000000 | 0.0096650100000000 | 0.9799784400000000 | 1.0 |
| C53 | C | 0.8496506900000000 | 0.0861843100000000 | 0.9861875600000000 | 1.0 |
| C54 | C | 0.7277131400000000 | 0.0885387300000000 | 0.0324743100000000 | 1.0 |
| C55 | C | 0.7412776500000000 | 0.9071977200000000 | 0.0195959900000000 | 1.0 |
| C56 | C | 0.8919768700000000 | 0.9919044200000000 | 0.9071033100000000 | 1.0 |
| O57 | O | 0.9743732800000000 | 0.0625890900000000 | 0.0756967100000000 | 1.0 |
| O58 | O | 0.2338242300000000 | 0.0623776600000000 | 0.0757419700000000 | 1.0 |
| O59 | O | 0.4801529800000000 | 0.0245299600000000 | 0.0670794600000000 | 1.0 |
| O60 | O | 0.7279282500000000 | 0.0248824000000000 | 0.0671998700000000 | 1.0 |

##### cif ends

furan\_CH3\_23\_syn\_dir\_forbid    Energy: -353.44475772

##### cif starts

data\_furan\_CH3\_23\_syn\_dir\_forbid

\_publ\_section\_comment

;  
Andrew Reynoso, Bohan Xu, and Vincent H. Crespi  
;

\_cell\_length\_a    9.7812103348

\_cell\_length\_b    20.0

\_cell\_length\_c    20.0

\_cell\_angle\_alpha    90.0

\_cell\_angle\_beta    90.0

\_cell\_angle\_gamma    90.0

\_symmetry\_space\_group\_name\_H-M    'P 1'

\_symmetry\_Int\_Tables\_number 1

\_symmetry\_cell\_setting triclinic

loop\_

\_atom\_site\_label

\_atom\_site\_type\_symbol

\_atom\_site\_fract\_x

\_atom\_site\_fract\_y

\_atom\_site\_fract\_z

\_atom\_site\_occupancy

|    |   |                    |                    |                    |     |
|----|---|--------------------|--------------------|--------------------|-----|
| H1 | H | 0.0275531500000000 | 0.1117647100000000 | 0.0395808800000000 | 1.0 |
|----|---|--------------------|--------------------|--------------------|-----|

|    |   |                    |                    |                    |     |
|----|---|--------------------|--------------------|--------------------|-----|
| H2 | H | 0.0013814300000000 | 0.0536145400000000 | 0.9155731600000000 | 1.0 |
|----|---|--------------------|--------------------|--------------------|-----|

|    |   |                    |                    |                    |     |
|----|---|--------------------|--------------------|--------------------|-----|
| H3 | H | 0.2537266900000000 | 0.0942062300000000 | 0.0710147000000000 | 1.0 |
|----|---|--------------------|--------------------|--------------------|-----|

|    |   |                    |                    |                    |     |
|----|---|--------------------|--------------------|--------------------|-----|
| H4 | H | 0.2634901300000000 | 0.0784074300000000 | 0.9324061000000000 | 1.0 |
|----|---|--------------------|--------------------|--------------------|-----|

|    |   |                    |                    |                    |     |
|----|---|--------------------|--------------------|--------------------|-----|
| H5 | H | 0.5275376100000000 | 0.1119406200000000 | 0.0393292700000000 | 1.0 |
|----|---|--------------------|--------------------|--------------------|-----|

|     |   |                    |                    |                    |     |
|-----|---|--------------------|--------------------|--------------------|-----|
| H6  | H | 0.5011870800000000 | 0.0536015700000000 | 0.9154496100000000 | 1.0 |
| H7  | H | 0.7535787200000000 | 0.0943785200000000 | 0.0709780800000000 | 1.0 |
| H8  | H | 0.7637092200000000 | 0.0784521300000000 | 0.9324133200000000 | 1.0 |
| H9  | H | 0.9878520000000000 | 0.8517904800000000 | 0.0877003800000000 | 1.0 |
| H10 | H | 0.8944906700000000 | 0.9203200600000000 | 0.1224040800000000 | 1.0 |
| H11 | H | 0.0705257300000000 | 0.9128040900000000 | 0.1385851700000000 | 1.0 |
| H12 | H | 0.3304944400000000 | 0.8577948900000000 | 0.0199391600000000 | 1.0 |
| H13 | H | 0.1557121300000000 | 0.8379632900000000 | 0.0149950400000000 | 1.0 |
| H14 | H | 0.2283292700000000 | 0.8595591000000000 | 0.0924613000000000 | 1.0 |
| H15 | H | 0.4877967500000000 | 0.8520700700000000 | 0.0880507900000000 | 1.0 |
| H16 | H | 0.3942416000000000 | 0.9206734000000000 | 0.1224711400000000 | 1.0 |
| H17 | H | 0.5702625100000000 | 0.9132858400000000 | 0.1387772800000000 | 1.0 |
| H18 | H | 0.8299755600000000 | 0.8577747500000000 | 0.0199670200000000 | 1.0 |
| H19 | H | 0.6550673800000000 | 0.8381199800000000 | 0.0153737600000000 | 1.0 |
| H20 | H | 0.7282968700000000 | 0.8598050300000000 | 0.0926655100000000 | 1.0 |
| H21 | H | 0.0910674300000000 | 0.8819097100000000 | 0.9350419600000000 | 1.0 |
| H22 | H | 0.9826225400000000 | 0.9142650600000000 | 0.8731162400000000 | 1.0 |
| H23 | H | 0.9187031900000000 | 0.8584632100000000 | 0.9331310800000000 | 1.0 |
| H24 | H | 0.3245664400000000 | 0.9838410400000000 | 0.8571329200000000 | 1.0 |
| H25 | H | 0.1491513400000000 | 0.9819616100000000 | 0.8759446700000000 | 1.0 |
| H26 | H | 0.2434841300000000 | 0.9062729500000000 | 0.8719966800000000 | 1.0 |
| H27 | H | 0.5913249100000000 | 0.8819680500000000 | 0.9351621800000000 | 1.0 |
| H28 | H | 0.4828944300000000 | 0.9142127300000000 | 0.8731768900000000 | 1.0 |
| H29 | H | 0.4190268200000000 | 0.8584311200000000 | 0.9332178000000000 | 1.0 |
| H30 | H | 0.8244167100000000 | 0.9840200700000000 | 0.8572155400000000 | 1.0 |
| H31 | H | 0.6490262800000000 | 0.9821553600000000 | 0.8760683400000000 | 1.0 |
| H32 | H | 0.7432673400000000 | 0.9064474700000000 | 0.8719751900000000 | 1.0 |
| C33 | C | 0.0569226100000000 | 0.0605186000000000 | 0.0255069500000000 | 1.0 |
| C34 | C | 0.9675909200000000 | 0.0362775600000000 | 0.9650247100000000 | 1.0 |
| C35 | C | 0.9446876800000000 | 0.9574190000000000 | 0.9735828200000000 | 1.0 |
| C36 | C | 0.0238575900000000 | 0.9519768000000000 | 0.0422570500000000 | 1.0 |
| C37 | C | 0.9886934700000000 | 0.9009281200000000 | 0.9260739600000000 | 1.0 |
| C38 | C | 0.9916199100000000 | 0.9049058100000000 | 0.1003988400000000 | 1.0 |
| C39 | C | 0.2233233700000000 | 0.0541066700000000 | 0.0366087900000000 | 1.0 |
| C40 | C | 0.3050181200000000 | 0.0460671800000000 | 0.9720052300000000 | 1.0 |
| C41 | C | 0.2819920600000000 | 0.9701173800000000 | 0.9619095600000000 | 1.0 |
| C42 | C | 0.1925567900000000 | 0.9442463100000000 | 0.0245917800000000 | 1.0 |
| C43 | C | 0.2472827800000000 | 0.9586323900000000 | 0.8880880100000000 | 1.0 |
| C44 | C | 0.2300153200000000 | 0.8711747100000000 | 0.0390941900000000 | 1.0 |
| C45 | C | 0.5568808200000000 | 0.0606563800000000 | 0.0253770900000000 | 1.0 |
| C46 | C | 0.4675292600000000 | 0.0363004300000000 | 0.9649354000000000 | 1.0 |
| C47 | C | 0.4447317700000000 | 0.9574502700000000 | 0.9735797600000000 | 1.0 |
| C48 | C | 0.5237680400000000 | 0.9521514500000000 | 0.0423146400000000 | 1.0 |
| C49 | C | 0.4889254600000000 | 0.9009272100000000 | 0.9261473700000000 | 1.0 |
| C50 | C | 0.4914541900000000 | 0.9052250600000000 | 0.1005751000000000 | 1.0 |
| C51 | C | 0.7232940000000000 | 0.0542351000000000 | 0.0365965300000000 | 1.0 |
| C52 | C | 0.8051093600000000 | 0.0461190500000000 | 0.9720497900000000 | 1.0 |
| C53 | C | 0.7819363400000000 | 0.9701775200000000 | 0.9619772000000000 | 1.0 |
| C54 | C | 0.6924291800000000 | 0.9443811000000000 | 0.0246883300000000 | 1.0 |
| C55 | C | 0.7471414200000000 | 0.9587781100000000 | 0.8881476300000000 | 1.0 |
| C56 | C | 0.7296937100000000 | 0.8713016300000000 | 0.0392691200000000 | 1.0 |
| O57 | O | 0.0085780600000000 | 0.0157084300000000 | 0.0746304800000000 | 1.0 |
| O58 | O | 0.2437865400000000 | 0.9920467700000000 | 0.0721673600000000 | 1.0 |
| O59 | O | 0.5084437100000000 | 0.0159486200000000 | 0.0745651700000000 | 1.0 |
| O60 | O | 0.7436795200000000 | 0.9922132500000000 | 0.0722315700000000 | 1.0 |

##### cif ends

uran\_CH3\_24\_anti\_alt Energy: -357.03903374

##### cif starts

data\_uran\_CH3\_24\_anti\_alt

\_publ\_section\_comment

;  
Andrew Reynoso, Bohan Xu, and Vincent H. Crespi  
;

\_cell\_length\_a 9.6750925622

\_cell\_length\_b 20.0

\_cell\_length\_c 20.0

\_cell\_angle\_alpha 90.0

\_cell\_angle\_beta 90.0

\_cell\_angle\_gamma 90.0

\_symmetry\_space\_group\_name\_H-M 'P 1'

\_symmetry\_Int\_Tables\_number 1

\_symmetry\_cell\_setting triclinic

loop\_

\_atom\_site\_label

\_atom\_site\_type\_symbol

\_atom\_site\_fract\_x

\_atom\_site\_fract\_y

\_atom\_site\_fract\_z

\_atom\_site\_occupancy

|     |   |                    |                    |                    |     |
|-----|---|--------------------|--------------------|--------------------|-----|
| H1  | H | 0.4907330200000000 | 0.9066845000000000 | 0.9479368700000000 | 1.0 |
| H2  | H | 0.5678921200000000 | 0.9762511400000000 | 0.1182170300000000 | 1.0 |
| H3  | H | 0.4691134300000000 | 0.0785898900000000 | 0.0677777000000000 | 1.0 |
| H4  | H | 0.5619590900000000 | 0.1695092500000000 | 0.9514105700000000 | 1.0 |
| H5  | H | 0.4937312000000000 | 0.1363738400000000 | 0.8761862700000000 | 1.0 |
| H6  | H | 0.3833371600000000 | 0.1531810000000000 | 0.9448353400000000 | 1.0 |
| H7  | H | 0.3910024100000000 | 0.9725296600000000 | 0.1378088900000000 | 1.0 |
| H8  | H | 0.4766954800000000 | 0.8997687100000000 | 0.1091579800000000 | 1.0 |
| H9  | H | 0.7407077100000000 | 0.1176585900000000 | 0.0423516800000000 | 1.0 |
| H10 | H | 0.8178863500000000 | 0.0481137300000000 | 0.8720599900000000 | 1.0 |
| H11 | H | 0.7191195100000000 | 0.9457729300000000 | 0.9224805200000000 | 1.0 |
| H12 | H | 0.8119726100000000 | 0.8548378200000000 | 0.0388347200000000 | 1.0 |
| H13 | H | 0.7437834900000000 | 0.8879728500000000 | 0.1140684500000000 | 1.0 |
| H14 | H | 0.6333554900000000 | 0.8711733200000000 | 0.0454315200000000 | 1.0 |
| H15 | H | 0.2266521900000000 | 0.1245875900000000 | 0.8811094900000000 | 1.0 |
| H16 | H | 0.1409923800000000 | 0.0518141200000000 | 0.8524660300000000 | 1.0 |
| H17 | H | 0.9907298500000000 | 0.9066856100000000 | 0.9479362200000000 | 1.0 |
| H18 | H | 0.0678961900000000 | 0.9762488600000000 | 0.1182158500000000 | 1.0 |
| H19 | H | 0.9691122500000000 | 0.0785896000000000 | 0.0677794400000000 | 1.0 |
| H20 | H | 0.0619608200000000 | 0.1695100000000000 | 0.9514131700000000 | 1.0 |
| H21 | H | 0.9937361000000000 | 0.1363753900000000 | 0.8761880500000000 | 1.0 |
| H22 | H | 0.8833384500000000 | 0.1531829400000000 | 0.9448357900000000 | 1.0 |
| H23 | H | 0.8910077100000000 | 0.9725284100000000 | 0.1378102200000000 | 1.0 |
| H24 | H | 0.9766962300000000 | 0.8997672000000000 | 0.1091569000000000 | 1.0 |
| H25 | H | 0.2407099200000000 | 0.1176591100000000 | 0.0423499400000000 | 1.0 |

|     |   |                    |                    |                    |     |
|-----|---|--------------------|--------------------|--------------------|-----|
| H26 | H | 0.3178843700000000 | 0.0481103500000000 | 0.8720595800000000 | 1.0 |
| H27 | H | 0.2191166000000000 | 0.9457732200000000 | 0.9224795300000000 | 1.0 |
| H28 | H | 0.3119779400000000 | 0.8548393200000000 | 0.0388314400000000 | 1.0 |
| H29 | H | 0.2437951500000000 | 0.8879722000000000 | 0.1140670200000000 | 1.0 |
| H30 | H | 0.1333598200000000 | 0.8711714200000000 | 0.0454327900000000 | 1.0 |
| H31 | H | 0.6409945100000000 | 0.0518172200000000 | 0.8524665000000000 | 1.0 |
| H32 | H | 0.7266521600000000 | 0.1245899200000000 | 0.8811131900000000 | 1.0 |
| C33 | C | 0.4279461600000000 | 0.9756269200000000 | 0.0318634300000000 | 1.0 |
| C34 | C | 0.4275484100000000 | 0.0531364200000000 | 0.0234188300000000 | 1.0 |
| C35 | C | 0.5149217700000000 | 0.0654092200000000 | 0.9601991200000000 | 1.0 |
| C36 | C | 0.4853896900000000 | 0.1344776500000000 | 0.9307025500000000 | 1.0 |
| C37 | C | 0.4701154600000000 | 0.9541182100000000 | 0.1031192000000000 | 1.0 |
| C38 | C | 0.5162231500000000 | 0.9560294600000000 | 0.9687799000000000 | 1.0 |
| C39 | C | 0.7662007800000000 | 0.0683187500000000 | 0.0214966700000000 | 1.0 |
| C40 | C | 0.6779298200000000 | 0.0487290100000000 | 0.9584084200000000 | 1.0 |
| C41 | C | 0.6775601900000000 | 0.9712189000000000 | 0.9668452200000000 | 1.0 |
| C42 | C | 0.7649392000000000 | 0.9589421200000000 | 0.0300630900000000 | 1.0 |
| C43 | C | 0.7354186400000000 | 0.8898707500000000 | 0.0595543300000000 | 1.0 |
| C44 | C | 0.7200981000000000 | 0.0702390400000000 | 0.8871546000000000 | 1.0 |
| C45 | C | 0.0162214500000000 | 0.9560297300000000 | 0.9687799300000000 | 1.0 |
| C46 | C | 0.9279461200000000 | 0.9756266400000000 | 0.0318641300000000 | 1.0 |
| C47 | C | 0.9275482800000000 | 0.0531366800000000 | 0.0234203600000000 | 1.0 |
| C48 | C | 0.0149211700000000 | 0.0654101600000000 | 0.9602002700000000 | 1.0 |
| C49 | C | 0.9853916300000000 | 0.1344787100000000 | 0.9307041300000000 | 1.0 |
| C50 | C | 0.9701183700000000 | 0.9541170600000000 | 0.1031189900000000 | 1.0 |
| C51 | C | 0.2662014000000000 | 0.0683193200000000 | 0.0214954300000000 | 1.0 |
| C52 | C | 0.1779292400000000 | 0.0487290200000000 | 0.9584077700000000 | 1.0 |
| C53 | C | 0.1775589300000000 | 0.9712189600000000 | 0.9668447300000000 | 1.0 |
| C54 | C | 0.2649392100000000 | 0.9589422900000000 | 0.0300622300000000 | 1.0 |
| C55 | C | 0.2354231200000000 | 0.8898704900000000 | 0.0595532100000000 | 1.0 |
| C56 | C | 0.2200961300000000 | 0.0702371400000000 | 0.8871533600000000 | 1.0 |
| O57 | O | 0.9708868400000000 | 0.0063201900000000 | 0.9211930500000000 | 1.0 |
| O58 | O | 0.7208825300000000 | 0.0180199600000000 | 0.0690760700000000 | 1.0 |
| O59 | O | 0.4708888300000000 | 0.0063191100000000 | 0.9211921800000000 | 1.0 |
| O60 | O | 0.2208826900000000 | 0.0180203700000000 | 0.0690751400000000 | 1.0 |

##### cif ends

furan\_CH3\_24\_anti\_alt\_forbid Energy: -357.87970105

##### cif starts

data\_furan\_CH3\_24\_anti\_alt\_forbid

\_publ\_section\_comment

;  
Andrew Reynoso, Bohan Xu, and Vincent H. Crespi  
;

\_cell\_length\_a 10.394963128

\_cell\_length\_b 20.0

\_cell\_length\_c 20.0

\_cell\_angle\_alpha 90.0

\_cell\_angle\_beta 90.0

\_cell\_angle\_gamma 90.0

\_symmetry\_space\_group\_name\_H-M 'P 1'

\_symmetry\_Int\_Tables\_number 1  
\_symmetry\_cell\_setting triclinic

loop\_

\_atom\_site\_label

\_atom\_site\_type\_symbol

\_atom\_site\_fract\_x

\_atom\_site\_fract\_y

\_atom\_site\_fract\_z

\_atom\_site\_occupancy

|     |   |                    |                    |                    |     |
|-----|---|--------------------|--------------------|--------------------|-----|
| H1  | H | 0.0652833000000000 | 0.9010974300000000 | 0.9252224700000000 | 1.0 |
| H2  | H | 0.9477895000000000 | 0.0598969400000000 | 0.0539353700000000 | 1.0 |
| H3  | H | 0.2180438900000000 | 0.0930153400000000 | 0.0418763700000000 | 1.0 |
| H4  | H | 0.3354326100000000 | 0.9342103400000000 | 0.9131305900000000 | 1.0 |
| H5  | H | 0.5654310800000000 | 0.9011274200000000 | 0.9250605000000000 | 1.0 |
| H6  | H | 0.4476378200000000 | 0.0597234300000000 | 0.0539522800000000 | 1.0 |
| H7  | H | 0.7178768100000000 | 0.0929719400000000 | 0.0419945800000000 | 1.0 |
| H8  | H | 0.8357024200000000 | 0.9343607400000000 | 0.9131175500000000 | 1.0 |
| H9  | H | 0.9535022100000000 | 0.8716329600000000 | 0.0736729900000000 | 1.0 |
| H10 | H | 0.8705975700000000 | 0.9438866200000000 | 0.1015190000000000 | 1.0 |
| H11 | H | 0.0402627200000000 | 0.9423362800000000 | 0.1026468100000000 | 1.0 |
| H12 | H | 0.4534397400000000 | 0.8713451700000000 | 0.0733332400000000 | 1.0 |
| H13 | H | 0.3709483300000000 | 0.9436159200000000 | 0.1014895800000000 | 1.0 |
| H14 | H | 0.5405931000000000 | 0.9418529800000000 | 0.1024647200000000 | 1.0 |
| H15 | H | 0.2901665200000000 | 0.8382710500000000 | 0.0122893000000000 | 1.0 |
| H16 | H | 0.1209636900000000 | 0.8383928300000000 | 0.0198104100000000 | 1.0 |
| H17 | H | 0.2166837900000000 | 0.8684451100000000 | 0.0863983400000000 | 1.0 |
| H18 | H | 0.7906437500000000 | 0.8383655800000000 | 0.0121086100000000 | 1.0 |
| H19 | H | 0.6214189600000000 | 0.8382699000000000 | 0.0195792500000000 | 1.0 |
| H20 | H | 0.7169465400000000 | 0.8683286100000000 | 0.0862391400000000 | 1.0 |
| H21 | H | 0.4122069400000000 | 0.0499232600000000 | 0.8654128200000000 | 1.0 |
| H22 | H | 0.3306804100000000 | 0.1225080300000000 | 0.8935023200000000 | 1.0 |
| H23 | H | 0.2425652400000000 | 0.0522248300000000 | 0.8646015300000000 | 1.0 |
| H24 | H | 0.6625861300000000 | 0.1555400200000000 | 0.9468236500000000 | 1.0 |
| H25 | H | 0.4935994600000000 | 0.1559709400000000 | 0.9556581800000000 | 1.0 |
| H26 | H | 0.5647504600000000 | 0.1257763800000000 | 0.8809406100000000 | 1.0 |
| H27 | H | 0.9120423600000000 | 0.0501942000000000 | 0.8654600600000000 | 1.0 |
| H28 | H | 0.8306095500000000 | 0.1227331400000000 | 0.8937523600000000 | 1.0 |
| H29 | H | 0.7424225400000000 | 0.0525443800000000 | 0.8646925800000000 | 1.0 |
| H30 | H | 0.1629964200000000 | 0.1554525300000000 | 0.9466308600000000 | 1.0 |
| H31 | H | 0.9940494100000000 | 0.1560789300000000 | 0.9555856200000000 | 1.0 |
| H32 | H | 0.0648745500000000 | 0.1257385700000000 | 0.8808433800000000 | 1.0 |
| C33 | C | 0.0750334400000000 | 0.1274058000000000 | 0.9352856700000000 | 1.0 |
| C34 | C | 0.9556259600000000 | 0.9264145600000000 | 0.0743886800000000 | 1.0 |
| C35 | C | 0.3276429200000000 | 0.0677388200000000 | 0.8927189800000000 | 1.0 |
| C36 | C | 0.2082577200000000 | 0.8667159700000000 | 0.0318749500000000 | 1.0 |
| C37 | C | 0.5747668000000000 | 0.1274092200000000 | 0.9353911400000000 | 1.0 |
| C38 | C | 0.4558047700000000 | 0.9261248700000000 | 0.0742284200000000 | 1.0 |
| C39 | C | 0.8275287700000000 | 0.0679644400000000 | 0.8928336000000000 | 1.0 |
| C40 | C | 0.7085749100000000 | 0.8666776000000000 | 0.0317106000000000 | 1.0 |
| C41 | C | 0.0790430700000000 | 0.0572368500000000 | 0.9664670400000000 | 1.0 |
| C42 | C | 0.9555771900000000 | 0.0365611000000000 | 0.0043122100000000 | 1.0 |
| C43 | C | 0.9574222300000000 | 0.9580202300000000 | 0.0046538000000000 | 1.0 |
| C44 | C | 0.0777336300000000 | 0.9441200200000000 | 0.9589552200000000 | 1.0 |
| C45 | C | 0.2055765900000000 | 0.0499933700000000 | 0.0081469000000000 | 1.0 |

|     |   |                    |                    |                    |     |
|-----|---|--------------------|--------------------|--------------------|-----|
| C46 | C | 0.3258668300000000 | 0.0360857600000000 | 0.9624303500000000 | 1.0 |
| C47 | C | 0.3276962300000000 | 0.9575380700000000 | 0.9627615300000000 | 1.0 |
| C48 | C | 0.2042548300000000 | 0.9368702500000000 | 0.0006403900000000 | 1.0 |
| C49 | C | 0.5789874900000000 | 0.0572164100000000 | 0.9665097600000000 | 1.0 |
| C50 | C | 0.4555478400000000 | 0.0364418000000000 | 0.0043096500000000 | 1.0 |
| C51 | C | 0.4574608700000000 | 0.9578992000000000 | 0.0045764300000000 | 1.0 |
| C52 | C | 0.5778015300000000 | 0.9441003600000000 | 0.9588619600000000 | 1.0 |
| C53 | C | 0.7055046100000000 | 0.0499902100000000 | 0.0082055200000000 | 1.0 |
| C54 | C | 0.8258392800000000 | 0.0361885400000000 | 0.9624827200000000 | 1.0 |
| C55 | C | 0.8277554100000000 | 0.9576442900000000 | 0.9627578000000000 | 1.0 |
| C56 | C | 0.7043225100000000 | 0.9368663200000000 | 0.0005608700000000 | 1.0 |
| O57 | O | 0.0855231700000000 | 0.0028265400000000 | 0.9170359600000000 | 1.0 |
| O58 | O | 0.1978183800000000 | 0.9912859400000000 | 0.0500650100000000 | 1.0 |
| O59 | O | 0.5855873900000000 | 0.0028606900000000 | 0.9170220900000000 | 1.0 |
| O60 | O | 0.6977427000000000 | 0.9912271400000000 | 0.0500447800000000 | 1.0 |

##### cif ends

furán\_CH3\_24\_anti\_dir Energy: -358.74232279

##### cif starts

data\_furan\_CH3\_24\_anti\_dir

\_publ\_section\_comment

;

Andrew Reynoso, Bohan Xu, and Vincent H. Crespi

;

\_cell\_length\_a 9.5463555734

\_cell\_length\_b 20.0

\_cell\_length\_c 20.0

\_cell\_angle\_alpha 90.0

\_cell\_angle\_beta 90.0

\_cell\_angle\_gamma 90.0

\_symmetry\_space\_group\_name\_H-M 'P 1'

\_symmetry\_Int\_Tables\_number 1

\_symmetry\_cell\_setting triclinic

loop\_

\_atom\_site\_label

\_atom\_site\_type\_symbol

\_atom\_site\_fract\_x

\_atom\_site\_fract\_y

\_atom\_site\_fract\_z

\_atom\_site\_occupancy

|    |   |                    |                    |                    |     |
|----|---|--------------------|--------------------|--------------------|-----|
| H1 | H | 0.4673405000000000 | 0.1221998700000000 | 0.9406524700000000 | 1.0 |
|----|---|--------------------|--------------------|--------------------|-----|

|    |   |                    |                    |                    |     |
|----|---|--------------------|--------------------|--------------------|-----|
| H2 | H | 0.3693509700000000 | 0.0904853100000000 | 0.1303769600000000 | 1.0 |
|----|---|--------------------|--------------------|--------------------|-----|

|    |   |                    |                    |                    |     |
|----|---|--------------------|--------------------|--------------------|-----|
| H3 | H | 0.4520431800000000 | 0.9608157300000000 | 0.0719825000000000 | 1.0 |
|----|---|--------------------|--------------------|--------------------|-----|

|    |   |                    |                    |                    |     |
|----|---|--------------------|--------------------|--------------------|-----|
| H4 | H | 0.3542162500000000 | 0.8894955600000000 | 0.9193335600000000 | 1.0 |
|----|---|--------------------|--------------------|--------------------|-----|

|    |   |                    |                    |                    |     |
|----|---|--------------------|--------------------|--------------------|-----|
| H5 | H | 0.5208109700000000 | 0.8961367600000000 | 0.8802210900000000 | 1.0 |
|----|---|--------------------|--------------------|--------------------|-----|

|    |   |                    |                    |                    |     |
|----|---|--------------------|--------------------|--------------------|-----|
| H6 | H | 0.5054194000000000 | 0.8571847900000000 | 0.9597364600000000 | 1.0 |
|----|---|--------------------|--------------------|--------------------|-----|

|    |   |                    |                    |                    |     |
|----|---|--------------------|--------------------|--------------------|-----|
| H7 | H | 0.5478769900000000 | 0.0759592700000000 | 0.1137907700000000 | 1.0 |
|----|---|--------------------|--------------------|--------------------|-----|

|    |   |                    |                    |                    |     |
|----|---|--------------------|--------------------|--------------------|-----|
| H8 | H | 0.4648817900000000 | 0.1496798700000000 | 0.0826670800000000 | 1.0 |
|----|---|--------------------|--------------------|--------------------|-----|

|    |   |                    |                    |                    |     |
|----|---|--------------------|--------------------|--------------------|-----|
| H9 | H | 0.7173504200000000 | 0.1220154000000000 | 0.0510591300000000 | 1.0 |
|----|---|--------------------|--------------------|--------------------|-----|

|     |   |                    |                    |                    |     |
|-----|---|--------------------|--------------------|--------------------|-----|
| H10 | H | 0.7977955600000000 | 0.0763221900000000 | 0.8777276200000000 | 1.0 |
|-----|---|--------------------|--------------------|--------------------|-----|

|     |   |                    |                    |                    |     |
|-----|---|--------------------|--------------------|--------------------|-----|
| H11 | H | 0.7020426500000000 | 0.9610846100000000 | 0.9191827300000000 | 1.0 |
| H12 | H | 0.7707842800000000 | 0.8957700600000000 | 0.1107409300000000 | 1.0 |
| H13 | H | 0.6042644600000000 | 0.8891968700000000 | 0.0715431700000000 | 1.0 |
| H14 | H | 0.7555895600000000 | 0.8570730400000000 | 0.0310921600000000 | 1.0 |
| H15 | H | 0.2150367300000000 | 0.1499653500000000 | 0.9091404600000000 | 1.0 |
| H16 | H | 0.1192688200000000 | 0.0910030200000000 | 0.8612512200000000 | 1.0 |
| H17 | H | 0.9673531700000000 | 0.1222099100000000 | 0.9406507400000000 | 1.0 |
| H18 | H | 0.8693378500000000 | 0.0905359200000000 | 0.1303600600000000 | 1.0 |
| H19 | H | 0.9520647200000000 | 0.9608276300000000 | 0.0719762800000000 | 1.0 |
| H20 | H | 0.8542006000000000 | 0.8894998200000000 | 0.9193405000000000 | 1.0 |
| H21 | H | 0.0207576300000000 | 0.8961637300000000 | 0.8801956000000000 | 1.0 |
| H22 | H | 0.0054520200000000 | 0.8571937900000000 | 0.9597062800000000 | 1.0 |
| H23 | H | 0.0478499900000000 | 0.0759445000000000 | 0.1137979800000000 | 1.0 |
| H24 | H | 0.9649820600000000 | 0.1496846600000000 | 0.0826449200000000 | 1.0 |
| H25 | H | 0.2173511900000000 | 0.1220062400000000 | 0.0510710800000000 | 1.0 |
| H26 | H | 0.2977871200000000 | 0.0763101000000000 | 0.8777213100000000 | 1.0 |
| H27 | H | 0.2020409400000000 | 0.9610921600000000 | 0.9191734900000000 | 1.0 |
| H28 | H | 0.2555249300000000 | 0.8570654700000000 | 0.0310543400000000 | 1.0 |
| H29 | H | 0.2707722400000000 | 0.8957359000000000 | 0.1107138600000000 | 1.0 |
| H30 | H | 0.1042341700000000 | 0.8891956200000000 | 0.0715278200000000 | 1.0 |
| H31 | H | 0.6192623400000000 | 0.0909477700000000 | 0.8612373300000000 | 1.0 |
| H32 | H | 0.7149222200000000 | 0.1499611900000000 | 0.9091133500000000 | 1.0 |
| C33 | C | 0.4049505000000000 | 0.0600653700000000 | 0.0277905700000000 | 1.0 |
| C34 | C | 0.4063123300000000 | 0.9814836900000000 | 0.0261283600000000 | 1.0 |
| C35 | C | 0.4939172900000000 | 0.9649114500000000 | 0.9622764900000000 | 1.0 |
| C36 | C | 0.4659253000000000 | 0.8982475300000000 | 0.9284750100000000 | 1.0 |
| C37 | C | 0.4515827600000000 | 0.0957999300000000 | 0.0923835000000000 | 1.0 |
| C38 | C | 0.4914330600000000 | 0.0741262500000000 | 0.9643902000000000 | 1.0 |
| C39 | C | 0.7414395800000000 | 0.0740223900000000 | 0.0271580800000000 | 1.0 |
| C40 | C | 0.6549430400000000 | 0.0601782300000000 | 0.9637126000000000 | 1.0 |
| C41 | C | 0.6563094300000000 | 0.9815909800000000 | 0.9651090400000000 | 1.0 |
| C42 | C | 0.7439305700000000 | 0.9648014000000000 | 0.0289036700000000 | 1.0 |
| C43 | C | 0.7159761700000000 | 0.8980177600000000 | 0.0624732500000000 | 1.0 |
| C44 | C | 0.7015462800000000 | 0.0961172900000000 | 0.8992241200000000 | 1.0 |
| C45 | C | 0.9914390000000000 | 0.0741346200000000 | 0.9643862500000000 | 1.0 |
| C46 | C | 0.9049531500000000 | 0.0600740000000000 | 0.0277845300000000 | 1.0 |
| C47 | C | 0.9063189500000000 | 0.9814923200000000 | 0.0261240000000000 | 1.0 |
| C48 | C | 0.9939139700000000 | 0.9649199300000000 | 0.9622683200000000 | 1.0 |
| C49 | C | 0.9659142300000000 | 0.8982595200000000 | 0.9284613700000000 | 1.0 |
| C50 | C | 0.9515955600000000 | 0.0958117600000000 | 0.0923741700000000 | 1.0 |
| C51 | C | 0.2414376000000000 | 0.0740159900000000 | 0.0271642900000000 | 1.0 |
| C52 | C | 0.1549485100000000 | 0.0601823600000000 | 0.9637137800000000 | 1.0 |
| C53 | C | 0.1563085700000000 | 0.9815951000000000 | 0.9651016400000000 | 1.0 |
| C54 | C | 0.2439202100000000 | 0.9647954200000000 | 0.0288970900000000 | 1.0 |
| C55 | C | 0.2159471800000000 | 0.8980054700000000 | 0.0624517800000000 | 1.0 |
| C56 | C | 0.2015744500000000 | 0.0961294000000000 | 0.8992330600000000 | 1.0 |
| O57 | O | 0.9495559200000000 | 0.0200501600000000 | 0.9197075600000000 | 1.0 |
| O58 | O | 0.6995696500000000 | 0.0197766600000000 | 0.0716607400000000 | 1.0 |
| O59 | O | 0.4495509200000000 | 0.0200388200000000 | 0.9197137700000000 | 1.0 |
| O60 | O | 0.1995571000000000 | 0.0197661200000000 | 0.0716595500000000 | 1.0 |

##### cif ends

furan\_CH3\_24\_anti\_dir\_forbid    Energy: -359.49211871

##### cif starts

data\_furan\_CH3\_24\_anti\_dir\_forbid

\_publ\_section\_comment

;  
Andrew Reynoso, Bohan Xu, and Vincent H. Crespi  
;

\_cell\_length\_a 10.2913470249

\_cell\_length\_b 20.0

\_cell\_length\_c 20.0

\_cell\_angle\_alpha 90.0

\_cell\_angle\_beta 90.0

\_cell\_angle\_gamma 90.0

\_symmetry\_space\_group\_name\_H-M 'P 1'

\_symmetry\_Int\_Tables\_number 1

\_symmetry\_cell\_setting triclinic

loop\_

\_atom\_site\_label

\_atom\_site\_type\_symbol

\_atom\_site\_fract\_x

\_atom\_site\_fract\_y

\_atom\_site\_fract\_z

\_atom\_site\_occupancy

|     |   |                    |                    |                    |     |
|-----|---|--------------------|--------------------|--------------------|-----|
| H1  | H | 0.8596061900000000 | 0.1098136100000000 | 0.0602760100000000 | 1.0 |
| H2  | H | 0.0631682100000000 | 0.0716923000000000 | 0.8914450400000000 | 1.0 |
| H3  | H | 0.9758802800000000 | 0.9461484000000000 | 0.9389888600000000 | 1.0 |
| H4  | H | 0.8914936600000000 | 0.8449297700000000 | 0.0413655900000000 | 1.0 |
| H5  | H | 0.9378765300000000 | 0.8947026000000000 | 0.1112390400000000 | 1.0 |
| H6  | H | 0.7717120300000000 | 0.8764943300000000 | 0.0973051800000000 | 1.0 |
| H7  | H | 0.8918224700000000 | 0.0763957000000000 | 0.8907690200000000 | 1.0 |
| H8  | H | 0.9840193200000000 | 0.1409796200000000 | 0.9295583800000000 | 1.0 |
| H9  | H | 0.2190166200000000 | 0.1105734100000000 | 0.9574598600000000 | 1.0 |
| H10 | H | 0.0154249700000000 | 0.0699059500000000 | 0.1257095000000000 | 1.0 |
| H11 | H | 0.1027532100000000 | 0.9451265500000000 | 0.0763206700000000 | 1.0 |
| H12 | H | 0.1871848000000000 | 0.8454354500000000 | 0.9725214600000000 | 1.0 |
| H13 | H | 0.1406639800000000 | 0.8961823700000000 | 0.9033777600000000 | 1.0 |
| H14 | H | 0.3068687900000000 | 0.8778081300000000 | 0.9169939100000000 | 1.0 |
| H15 | H | 0.1867675700000000 | 0.0746350000000000 | 0.1264811800000000 | 1.0 |
| H16 | H | 0.0945352100000000 | 0.1397877600000000 | 0.0886716600000000 | 1.0 |
| H17 | H | 0.3596227900000000 | 0.1098443500000000 | 0.0602236700000000 | 1.0 |
| H18 | H | 0.5632286000000000 | 0.0716532200000000 | 0.8914453200000000 | 1.0 |
| H19 | H | 0.4757945100000000 | 0.9461037800000000 | 0.9390179700000000 | 1.0 |
| H20 | H | 0.3914378400000000 | 0.8449405300000000 | 0.0415158300000000 | 1.0 |
| H21 | H | 0.4379450700000000 | 0.8947833600000000 | 0.1113170200000000 | 1.0 |
| H22 | H | 0.2717520300000000 | 0.8765910300000000 | 0.0974617300000000 | 1.0 |
| H23 | H | 0.3918743300000000 | 0.0763025000000000 | 0.8907284500000000 | 1.0 |
| H24 | H | 0.4839637300000000 | 0.1409360800000000 | 0.9295055700000000 | 1.0 |
| H25 | H | 0.7190096000000000 | 0.1106069400000000 | 0.9575062100000000 | 1.0 |
| H26 | H | 0.5153565500000000 | 0.0698756500000000 | 0.1256981800000000 | 1.0 |
| H27 | H | 0.6028516000000000 | 0.9450974100000000 | 0.0762921800000000 | 1.0 |
| H28 | H | 0.6871961100000000 | 0.8454560400000000 | 0.9723509900000000 | 1.0 |
| H29 | H | 0.6406753300000000 | 0.8962901200000000 | 0.9032689100000000 | 1.0 |
| H30 | H | 0.8068779100000000 | 0.8779039900000000 | 0.9168627400000000 | 1.0 |



|     |   |                    |                    |                    |     |
|-----|---|--------------------|--------------------|--------------------|-----|
| H31 | H | 0.6867023900000000 | 0.0745583700000000 | 0.1265068600000000 | 1.0 |
| H32 | H | 0.5945660300000000 | 0.1397512900000000 | 0.0887052500000000 | 1.0 |
| C33 | C | 0.8517767200000000 | 0.0642784800000000 | 0.0298328400000000 | 1.0 |
| C34 | C | 0.9738101800000000 | 0.0490247400000000 | 0.9873506800000000 | 1.0 |
| C35 | C | 0.9739967800000000 | 0.9701984700000000 | 0.9882337400000000 | 1.0 |
| C36 | C | 0.8525841900000000 | 0.9509749500000000 | 0.0300312900000000 | 1.0 |
| C37 | C | 0.8640119800000000 | 0.8880528500000000 | 0.0722626700000000 | 1.0 |
| C38 | C | 0.9782732400000000 | 0.0866018900000000 | 0.9210391200000000 | 1.0 |
| C39 | C | 0.2268423300000000 | 0.0645935400000000 | 0.9872262200000000 | 1.0 |
| C40 | C | 0.1048112400000000 | 0.0487128300000000 | 0.0294849800000000 | 1.0 |
| C41 | C | 0.1046252700000000 | 0.9699076500000000 | 0.0274380900000000 | 1.0 |
| C42 | C | 0.2260291700000000 | 0.9513038900000000 | 0.9853543600000000 | 1.0 |
| C43 | C | 0.2145924400000000 | 0.8889962100000000 | 0.9422259100000000 | 1.0 |
| C44 | C | 0.1003233100000000 | 0.0852857000000000 | 0.0963582900000000 | 1.0 |
| C45 | C | 0.3517834600000000 | 0.0642896700000000 | 0.0298111800000000 | 1.0 |
| C46 | C | 0.4738115700000000 | 0.0490052100000000 | 0.9873419700000000 | 1.0 |
| C47 | C | 0.4739788900000000 | 0.9701772300000000 | 0.9882538300000000 | 1.0 |
| C48 | C | 0.3525840700000000 | 0.9509870500000000 | 0.0300847900000000 | 1.0 |
| C49 | C | 0.3640252500000000 | 0.8881032100000000 | 0.0723727600000000 | 1.0 |
| C50 | C | 0.4782897000000000 | 0.0865518800000000 | 0.9210125000000000 | 1.0 |
| C51 | C | 0.7268395100000000 | 0.0646077400000000 | 0.9872442300000000 | 1.0 |
| C52 | C | 0.6048068800000000 | 0.0486964900000000 | 0.0294863600000000 | 1.0 |
| C53 | C | 0.6046462400000000 | 0.9698933600000000 | 0.0274169700000000 | 1.0 |
| C54 | C | 0.7260334300000000 | 0.9513208300000000 | 0.9853007700000000 | 1.0 |
| C55 | C | 0.7146008000000000 | 0.8890553100000000 | 0.9421109700000000 | 1.0 |
| C56 | C | 0.6002919100000000 | 0.0852457200000000 | 0.0963716400000000 | 1.0 |
| O57 | O | 0.8428576400000000 | 0.0078576400000000 | 0.0752118500000000 | 1.0 |
| O58 | O | 0.2357425100000000 | 0.0088437900000000 | 0.9410153400000000 | 1.0 |
| O59 | O | 0.3428671600000000 | 0.0078997800000000 | 0.0752256600000000 | 1.0 |
| O60 | O | 0.7357476500000000 | 0.0088877800000000 | 0.9410000800000000 | 1.0 |

##### cif ends

furan\_CH3\_24\_syn\_alt    Energy: -359.37744865

##### cif starts

data\_furan\_CH3\_24\_syn\_alt

\_publ\_section\_comment

;  
Andrew Reynoso, Bohan Xu, and Vincent H. Crespi  
;

\_cell\_length\_a    10.4223713627

\_cell\_length\_b    20.0

\_cell\_length\_c    20.0

\_cell\_angle\_alpha    90.0

\_cell\_angle\_beta    90.0

\_cell\_angle\_gamma    90.0

\_symmetry\_space\_group\_name\_H-M    'P 1'

\_symmetry\_Int\_Tables\_number    1

\_symmetry\_cell\_setting    triclinic

loop\_

\_atom\_site\_label

|     | _atom_site_type_symbol | _atom_site_fract_x | _atom_site_fract_y | _atom_site_fract_z | _atom_site_occupancy |
|-----|------------------------|--------------------|--------------------|--------------------|----------------------|
| H1  | H                      | 0.4782237500000000 | 0.8874665000000000 | 0.0542426200000000 | 1.0                  |
| H2  | H                      | 0.5169385400000000 | 0.9270603800000000 | 0.8917748700000000 | 1.0                  |
| H3  | H                      | 0.5988326500000000 | 0.0538189600000000 | 0.9417307600000000 | 1.0                  |
| H4  | H                      | 0.3929189600000000 | 0.1113907300000000 | 0.1057807200000000 | 1.0                  |
| H5  | H                      | 0.5617479800000000 | 0.1129939800000000 | 0.1043572100000000 | 1.0                  |
| H6  | H                      | 0.4741331500000000 | 0.1526337300000000 | 0.0388975700000000 | 1.0                  |
| H7  | H                      | 0.6849342400000000 | 0.9358317100000000 | 0.8888611800000000 | 1.0                  |
| H8  | H                      | 0.6160071300000000 | 0.8631859100000000 | 0.9246151400000000 | 1.0                  |
| H9  | H                      | 0.7282087600000000 | 0.0935422400000000 | 0.0543913500000000 | 1.0                  |
| H10 | H                      | 0.9348957800000000 | 0.0454114400000000 | 0.8889255300000000 | 1.0                  |
| H11 | H                      | 0.8488324500000000 | 0.9273543100000000 | 0.9416404600000000 | 1.0                  |
| H12 | H                      | 0.8117603400000000 | 0.8679266600000000 | 0.1041615000000000 | 1.0                  |
| H13 | H                      | 0.6429308800000000 | 0.8695503800000000 | 0.1056197500000000 | 1.0                  |
| H14 | H                      | 0.7240843100000000 | 0.8283991000000000 | 0.0386594900000000 | 1.0                  |
| H15 | H                      | 0.3660221300000000 | 0.1180013600000000 | 0.9248025800000000 | 1.0                  |
| H16 | H                      | 0.2669311400000000 | 0.0541846200000000 | 0.8918726100000000 | 1.0                  |
| H17 | H                      | 0.9782093700000000 | 0.8874688000000000 | 0.0542439700000000 | 1.0                  |
| H18 | H                      | 0.0169326900000000 | 0.9270545500000000 | 0.8917792900000000 | 1.0                  |
| H19 | H                      | 0.0988466900000000 | 0.0538120000000000 | 0.9417296100000000 | 1.0                  |
| H20 | H                      | 0.8929134400000000 | 0.1113959200000000 | 0.1057718600000000 | 1.0                  |
| H21 | H                      | 0.0617437000000000 | 0.1129706500000000 | 0.1043761500000000 | 1.0                  |
| H22 | H                      | 0.9741938500000000 | 0.1526387600000000 | 0.0389093800000000 | 1.0                  |
| H23 | H                      | 0.1849273500000000 | 0.9358366500000000 | 0.8888608500000000 | 1.0                  |
| H24 | H                      | 0.1160214900000000 | 0.8631838200000000 | 0.9246131700000000 | 1.0                  |
| H25 | H                      | 0.2282080100000000 | 0.0935329600000000 | 0.0543990300000000 | 1.0                  |
| H26 | H                      | 0.4349230600000000 | 0.0454027200000000 | 0.8889406100000000 | 1.0                  |
| H27 | H                      | 0.3488357600000000 | 0.9273505200000000 | 0.9416437200000000 | 1.0                  |
| H28 | H                      | 0.3117726400000000 | 0.8679296300000000 | 0.1041678100000000 | 1.0                  |
| H29 | H                      | 0.1429413400000000 | 0.8695376100000000 | 0.1056229900000000 | 1.0                  |
| H30 | H                      | 0.2241136100000000 | 0.8283900200000000 | 0.0386660900000000 | 1.0                  |
| H31 | H                      | 0.7669040300000000 | 0.0541905700000000 | 0.8918764200000000 | 1.0                  |
| H32 | H                      | 0.8660019600000000 | 0.1180074700000000 | 0.9247966200000000 | 1.0                  |
| C33 | C                      | 0.6027066800000000 | 0.9511837100000000 | 0.9887564700000000 | 1.0                  |
| C34 | C                      | 0.6018291300000000 | 0.0298309300000000 | 0.9909041800000000 | 1.0                  |
| C35 | C                      | 0.4774345800000000 | 0.0443191400000000 | 0.0333381600000000 | 1.0                  |
| C36 | C                      | 0.4764254800000000 | 0.1091551900000000 | 0.0725465500000000 | 1.0                  |
| C37 | C                      | 0.6054769300000000 | 0.9178147600000000 | 0.9200243300000000 | 1.0                  |
| C38 | C                      | 0.4773913200000000 | 0.9363834900000000 | 0.0296812300000000 | 1.0                  |
| C39 | C                      | 0.7273856200000000 | 0.0446601300000000 | 0.0297577900000000 | 1.0                  |
| C40 | C                      | 0.8527034100000000 | 0.0299206300000000 | 0.9888137800000000 | 1.0                  |
| C41 | C                      | 0.8518276200000000 | 0.9512708700000000 | 0.9908516700000000 | 1.0                  |
| C42 | C                      | 0.7274312400000000 | 0.9367199200000000 | 0.0332601300000000 | 1.0                  |
| C43 | C                      | 0.7264159800000000 | 0.8718275500000000 | 0.0723753000000000 | 1.0                  |
| C44 | C                      | 0.8554585900000000 | 0.0633871100000000 | 0.9201283400000000 | 1.0                  |
| C45 | C                      | 0.9773861700000000 | 0.9363844100000000 | 0.0296798500000000 | 1.0                  |
| C46 | C                      | 0.1027069800000000 | 0.9511789300000000 | 0.9887588400000000 | 1.0                  |
| C47 | C                      | 0.1018332200000000 | 0.0298273700000000 | 0.9909051100000000 | 1.0                  |
| C48 | C                      | 0.9774372100000000 | 0.0443209200000000 | 0.0333340800000000 | 1.0                  |
| C49 | C                      | 0.9764382200000000 | 0.1091529200000000 | 0.0725502000000000 | 1.0                  |
| C50 | C                      | 0.1054764600000000 | 0.9178126400000000 | 0.9200251200000000 | 1.0                  |

|     |   |                    |                    |                    |     |
|-----|---|--------------------|--------------------|--------------------|-----|
| C51 | C | 0.2273842800000000 | 0.0446536200000000 | 0.0297615400000000 | 1.0 |
| C52 | C | 0.3527020000000000 | 0.0299153000000000 | 0.9888183800000000 | 1.0 |
| C53 | C | 0.3518297100000000 | 0.9512662500000000 | 0.9908541200000000 | 1.0 |
| C54 | C | 0.2274327700000000 | 0.9367129100000000 | 0.0332627600000000 | 1.0 |
| C55 | C | 0.2264291800000000 | 0.8718211000000000 | 0.0723792900000000 | 1.0 |
| C56 | C | 0.3554741000000000 | 0.0633800600000000 | 0.9201329700000000 | 1.0 |
| O57 | O | 0.9775190600000000 | 0.9883428200000000 | 0.0788936300000000 | 1.0 |
| O58 | O | 0.7275115500000000 | 0.9926353400000000 | 0.0788997200000000 | 1.0 |
| O59 | O | 0.4775229000000000 | 0.9883407500000000 | 0.0788970500000000 | 1.0 |
| O60 | O | 0.2275094300000000 | 0.9926275600000000 | 0.0789035000000000 | 1.0 |

##### cif ends

furan\_CH3\_24\_syn\_alt\_forbid    Energy: -356.13288325

##### cif starts

data\_furan\_CH3\_24\_syn\_alt\_forbid

\_publ\_section\_comment

;  
Andrew Reynoso, Bohan Xu, and Vincent H. Crespi  
;

\_cell\_length\_a    9.7168383423

\_cell\_length\_b    20.0

\_cell\_length\_c    20.0

\_cell\_angle\_alpha    90.0

\_cell\_angle\_beta    90.0

\_cell\_angle\_gamma    90.0

\_symmetry\_space\_group\_name\_H-M    'P 1'

\_symmetry\_Int\_Tables\_number 1

\_symmetry\_cell\_setting triclinic

loop\_

\_atom\_site\_label

\_atom\_site\_type\_symbol

\_atom\_site\_fract\_x

\_atom\_site\_fract\_y

\_atom\_site\_fract\_z

\_atom\_site\_occupancy

|     |   |                    |                    |                    |     |
|-----|---|--------------------|--------------------|--------------------|-----|
| H1  | H | 0.9096746400000000 | 0.0682934000000000 | 0.9187026700000000 | 1.0 |
| H2  | H | 0.8828838000000000 | 0.8921882800000000 | 0.0364400800000000 | 1.0 |
| H3  | H | 0.1699715300000000 | 0.1037211000000000 | 0.0326830300000000 | 1.0 |
| H4  | H | 0.1433256000000000 | 0.9235285800000000 | 0.9212652300000000 | 1.0 |
| H5  | H | 0.4096952800000000 | 0.0683179600000000 | 0.9187010600000000 | 1.0 |
| H6  | H | 0.3829095500000000 | 0.8922069700000000 | 0.0364310300000000 | 1.0 |
| H7  | H | 0.6699973100000000 | 0.1037158900000000 | 0.0327106900000000 | 1.0 |
| H8  | H | 0.6433205300000000 | 0.9235519900000000 | 0.9212514800000000 | 1.0 |
| H9  | H | 0.0090647200000000 | 0.1033851500000000 | 0.0923447900000000 | 1.0 |
| H10 | H | 0.8324645900000000 | 0.1162836400000000 | 0.1089710100000000 | 1.0 |
| H11 | H | 0.9100012700000000 | 0.1574245600000000 | 0.0394851300000000 | 1.0 |
| H12 | H | 0.5090399400000000 | 0.1034353400000000 | 0.0923212400000000 | 1.0 |
| H13 | H | 0.3324334100000000 | 0.1162784700000000 | 0.1089752200000000 | 1.0 |
| H14 | H | 0.4098759900000000 | 0.1574515000000000 | 0.0394827500000000 | 1.0 |
| H15 | H | 0.1531369900000000 | 0.1178489000000000 | 0.8879752200000000 | 1.0 |

|     |   |                    |                    |                    |     |
|-----|---|--------------------|--------------------|--------------------|-----|
| H16 | H | 0.0784226200000000 | 0.0486122700000000 | 0.8467983200000000 | 1.0 |
| H17 | H | 0.2551969200000000 | 0.0474471700000000 | 0.8668329300000000 | 1.0 |
| H18 | H | 0.6533314500000000 | 0.1178739500000000 | 0.8880163500000000 | 1.0 |
| H19 | H | 0.5784142900000000 | 0.0487035600000000 | 0.8468172900000000 | 1.0 |
| H20 | H | 0.7551935400000000 | 0.0474180100000000 | 0.8668288300000000 | 1.0 |
| H21 | H | 0.9751139200000000 | 0.9399550100000000 | 0.8489072100000000 | 1.0 |
| H22 | H | 0.7981994000000000 | 0.9434140400000000 | 0.8683900500000000 | 1.0 |
| H23 | H | 0.8974263600000000 | 0.8729956600000000 | 0.8925026200000000 | 1.0 |
| H24 | H | 0.4750794500000000 | 0.9400283400000000 | 0.8488883200000000 | 1.0 |
| H25 | H | 0.2981731200000000 | 0.9434294000000000 | 0.8683956400000000 | 1.0 |
| H26 | H | 0.3974915500000000 | 0.8730279800000000 | 0.8924677600000000 | 1.0 |
| H27 | H | 0.1447377500000000 | 0.8386559100000000 | 0.0452851800000000 | 1.0 |
| H28 | H | 0.0436205300000000 | 0.8941699300000000 | 0.0956581200000000 | 1.0 |
| H29 | H | 0.2201840500000000 | 0.8828563700000000 | 0.1134422400000000 | 1.0 |
| H30 | H | 0.6445975700000000 | 0.8386550700000000 | 0.0452504100000000 | 1.0 |
| H31 | H | 0.5435965600000000 | 0.8941856800000000 | 0.0956627100000000 | 1.0 |
| H32 | H | 0.7201584000000000 | 0.8828053200000000 | 0.1134093500000000 | 1.0 |
| C33 | C | 0.8705173300000000 | 0.0516240300000000 | 0.0248238800000000 | 1.0 |
| C34 | C | 0.9510226300000000 | 0.0382445000000000 | 0.9598172700000000 | 1.0 |
| C35 | C | 0.9376797400000000 | 0.9599979800000000 | 0.9542775200000000 | 1.0 |
| C36 | C | 0.8510471700000000 | 0.9412825200000000 | 0.0174989100000000 | 1.0 |
| C37 | C | 0.9086883200000000 | 0.1108807600000000 | 0.0687401500000000 | 1.0 |
| C38 | C | 0.8986243200000000 | 0.9278898700000000 | 0.8875939500000000 | 1.0 |
| C39 | C | 0.2018552700000000 | 0.0539977300000000 | 0.0154873500000000 | 1.0 |
| C40 | C | 0.1152427700000000 | 0.0330286300000000 | 0.9529734200000000 | 1.0 |
| C41 | C | 0.1019360100000000 | 0.9550093200000000 | 0.9612845500000000 | 1.0 |
| C42 | C | 0.1824315600000000 | 0.9439796800000000 | 0.0267248900000000 | 1.0 |
| C43 | C | 0.1540027200000000 | 0.0628065400000000 | 0.8851833600000000 | 1.0 |
| C44 | C | 0.1445370300000000 | 0.8862945900000000 | 0.0727370200000000 | 1.0 |
| C45 | C | 0.3705036600000000 | 0.0516404800000000 | 0.0248153800000000 | 1.0 |
| C46 | C | 0.4510297200000000 | 0.0382675400000000 | 0.9598165400000000 | 1.0 |
| C47 | C | 0.4376784500000000 | 0.9600199900000000 | 0.9542689500000000 | 1.0 |
| C48 | C | 0.3510539400000000 | 0.9412990700000000 | 0.0174938900000000 | 1.0 |
| C49 | C | 0.4086381300000000 | 0.1109026900000000 | 0.0687318400000000 | 1.0 |
| C50 | C | 0.3986243000000000 | 0.9279252100000000 | 0.8875803600000000 | 1.0 |
| C51 | C | 0.7018667900000000 | 0.0539938500000000 | 0.0155029500000000 | 1.0 |
| C52 | C | 0.6152535700000000 | 0.0330449600000000 | 0.9529822700000000 | 1.0 |
| C53 | C | 0.6019332400000000 | 0.9550244700000000 | 0.9612769100000000 | 1.0 |
| C54 | C | 0.6824177300000000 | 0.9439730300000000 | 0.0267184700000000 | 1.0 |
| C55 | C | 0.6540501100000000 | 0.0628319400000000 | 0.8852000400000000 | 1.0 |
| C56 | C | 0.6444845600000000 | 0.8862829300000000 | 0.0727199300000000 | 1.0 |
| O57 | O | 0.8942686200000000 | 0.9914718700000000 | 0.0631852700000000 | 1.0 |
| O58 | O | 0.1586164600000000 | 0.0054529400000000 | 0.0629197900000000 | 1.0 |
| O59 | O | 0.3942707500000000 | 0.9914915000000000 | 0.0631785000000000 | 1.0 |
| O60 | O | 0.6586176000000000 | 0.0054410200000000 | 0.0629246800000000 | 1.0 |

##### cif ends

furan\_CH3\_24\_syn\_dir    Energy: -355.91371439

##### cif starts

data\_furan\_CH3\_24\_syn\_dir

\_publ\_section\_comment

;  
Andrew Reynoso, Bohan Xu, and Vincent H. Crespi

;

\_cell\_length\_a 10.535127043  
\_cell\_length\_b 20.0  
\_cell\_length\_c 20.0  
\_cell\_angle\_alpha 90.0  
\_cell\_angle\_beta 90.0  
\_cell\_angle\_gamma 90.0

\_symmetry\_space\_group\_name\_H-M 'P 1'  
\_symmetry\_Int\_Tables\_number 1  
\_symmetry\_cell\_setting triclinic

loop\_  
\_atom\_site\_label  
\_atom\_site\_type\_symbol  
\_atom\_site\_fract\_x  
\_atom\_site\_fract\_y  
\_atom\_site\_fract\_z  
\_atom\_site\_occupancy

|     |   |                    |                    |                    |     |
|-----|---|--------------------|--------------------|--------------------|-----|
| H1  | H | 0.4299839000000000 | 0.1193720600000000 | 0.0493543200000000 | 1.0 |
| H2  | H | 0.5706169400000000 | 0.0784743900000000 | 0.8837952900000000 | 1.0 |
| H3  | H | 0.5439407400000000 | 0.9464081700000000 | 0.9484852400000000 | 1.0 |
| H4  | H | 0.5220441100000000 | 0.9178638700000000 | 0.1348425100000000 | 1.0 |
| H5  | H | 0.3555667100000000 | 0.9187357400000000 | 0.1338056300000000 | 1.0 |
| H6  | H | 0.4381588100000000 | 0.8569363100000000 | 0.0866713100000000 | 1.0 |
| H7  | H | 0.4830738400000000 | 0.1330381300000000 | 0.9350373700000000 | 1.0 |
| H8  | H | 0.6481312800000000 | 0.1344181400000000 | 0.9384685100000000 | 1.0 |
| H9  | H | 0.6963002400000000 | 0.1059766500000000 | 0.0647414500000000 | 1.0 |
| H10 | H | 0.8969647600000000 | 0.0318888900000000 | 0.8930058200000000 | 1.0 |
| H11 | H | 0.8319842700000000 | 0.9394272700000000 | 0.9533357500000000 | 1.0 |
| H12 | H | 0.7676513800000000 | 0.8511509300000000 | 0.0337188700000000 | 1.0 |
| H13 | H | 0.6851631700000000 | 0.8693072200000000 | 0.1083415100000000 | 1.0 |
| H14 | H | 0.6011206500000000 | 0.8515847500000000 | 0.0339048200000000 | 1.0 |
| H15 | H | 0.3099300000000000 | 0.1072482900000000 | 0.8973467400000000 | 1.0 |
| H16 | H | 0.2315026400000000 | 0.0290299600000000 | 0.8917240700000000 | 1.0 |
| H17 | H | 0.9299896500000000 | 0.1193788500000000 | 0.0493193600000000 | 1.0 |
| H18 | H | 0.0706151400000000 | 0.0784277400000000 | 0.8837688300000000 | 1.0 |
| H19 | H | 0.0439287700000000 | 0.9463917800000000 | 0.9484903700000000 | 1.0 |
| H20 | H | 0.0220895300000000 | 0.9179044900000000 | 0.1348546400000000 | 1.0 |
| H21 | H | 0.8556117900000000 | 0.9187684000000000 | 0.1338409000000000 | 1.0 |
| H22 | H | 0.9381918500000000 | 0.8569528100000000 | 0.0867205000000000 | 1.0 |
| H23 | H | 0.9830536300000000 | 0.1330039400000000 | 0.9349895000000000 | 1.0 |
| H24 | H | 0.1481097700000000 | 0.1343963800000000 | 0.9384244300000000 | 1.0 |
| H25 | H | 0.1962639700000000 | 0.1059826400000000 | 0.0647273100000000 | 1.0 |
| H26 | H | 0.3970034100000000 | 0.0319044400000000 | 0.8930167300000000 | 1.0 |
| H27 | H | 0.3319777500000000 | 0.9394400600000000 | 0.9533236200000000 | 1.0 |
| H28 | H | 0.2676415300000000 | 0.8511518500000000 | 0.0336969800000000 | 1.0 |
| H29 | H | 0.1851646300000000 | 0.8692947400000000 | 0.1083258200000000 | 1.0 |
| H30 | H | 0.1011113000000000 | 0.8515887600000000 | 0.0338890500000000 | 1.0 |
| H31 | H | 0.7314624900000000 | 0.0290028300000000 | 0.8917301200000000 | 1.0 |
| H32 | H | 0.8098754400000000 | 0.1072266000000000 | 0.8973355800000000 | 1.0 |
| C33 | C | 0.5634947600000000 | 0.0517828300000000 | 0.9939611600000000 | 1.0 |
| C34 | C | 0.5596740100000000 | 0.9718470200000000 | 0.9965205600000000 | 1.0 |
| C35 | C | 0.4384404300000000 | 0.9609671100000000 | 0.0472214900000000 | 1.0 |

|     |   |                    |                    |                    |     |
|-----|---|--------------------|--------------------|--------------------|-----|
| C36 | C | 0.4394244400000000 | 0.9090874800000000 | 0.1029566600000000 | 1.0 |
| C37 | C | 0.5668546600000000 | 0.1006608300000000 | 0.9337686200000000 | 1.0 |
| C38 | C | 0.4360556700000000 | 0.0676308700000000 | 0.0308939100000000 | 1.0 |
| C39 | C | 0.6889927500000000 | 0.0592704300000000 | 0.0360538500000000 | 1.0 |
| C40 | C | 0.8132146300000000 | 0.0439054100000000 | 0.9903558600000000 | 1.0 |
| C41 | C | 0.8174840800000000 | 0.9670912000000000 | 0.0002281700000000 | 1.0 |
| C42 | C | 0.6868610900000000 | 0.9508955600000000 | 0.0330214600000000 | 1.0 |
| C43 | C | 0.6846235600000000 | 0.8769314000000000 | 0.0542115700000000 | 1.0 |
| C44 | C | 0.8120114900000000 | 0.0551710200000000 | 0.9143111600000000 | 1.0 |
| C45 | C | 0.9360562500000000 | 0.0676342200000000 | 0.0308747100000000 | 1.0 |
| C46 | C | 0.0634912300000000 | 0.0517743900000000 | 0.9939427800000000 | 1.0 |
| C47 | C | 0.0596708400000000 | 0.9718427000000000 | 0.9965188900000000 | 1.0 |
| C48 | C | 0.9384458500000000 | 0.9609718900000000 | 0.0472303000000000 | 1.0 |
| C49 | C | 0.9394548900000000 | 0.9091114000000000 | 0.1029839000000000 | 1.0 |
| C50 | C | 0.0668422100000000 | 0.1006324200000000 | 0.9337351400000000 | 1.0 |
| C51 | C | 0.1889839600000000 | 0.0592738100000000 | 0.0360419400000000 | 1.0 |
| C52 | C | 0.3132207800000000 | 0.0439130800000000 | 0.9903591400000000 | 1.0 |
| C53 | C | 0.3174814900000000 | 0.9670969300000000 | 0.0002200600000000 | 1.0 |
| C54 | C | 0.1868600100000000 | 0.9508976300000000 | 0.0330147700000000 | 1.0 |
| C55 | C | 0.1846186700000000 | 0.8769305300000000 | 0.0541975200000000 | 1.0 |
| C56 | C | 0.3120489200000000 | 0.0551898100000000 | 0.9143163000000000 | 1.0 |
| O57 | O | 0.9354757400000000 | 0.0226452500000000 | 0.0847661500000000 | 1.0 |
| O58 | O | 0.6870339300000000 | 0.0039550600000000 | 0.0830361600000000 | 1.0 |
| O59 | O | 0.4354695200000000 | 0.0226286000000000 | 0.0847739500000000 | 1.0 |
| O60 | O | 0.1870270500000000 | 0.0039600500000000 | 0.0830278600000000 | 1.0 |

##### cif ends

furan\_CH3\_24\_syn\_dir\_forbid Energy: -353.90451462

##### cif starts

data\_furan\_CH3\_24\_syn\_dir\_forbid

\_publ\_section\_comment

;  
Andrew Reynoso, Bohan Xu, and Vincent H. Crespi  
;

\_cell\_length\_a 9.6501278716

\_cell\_length\_b 20.0

\_cell\_length\_c 20.0

\_cell\_angle\_alpha 90.0

\_cell\_angle\_beta 90.0

\_cell\_angle\_gamma 90.0

\_symmetry\_space\_group\_name\_H-M 'P 1'

\_symmetry\_Int\_Tables\_number 1

\_symmetry\_cell\_setting triclinic

loop\_

\_atom\_site\_label

\_atom\_site\_type\_symbol

\_atom\_site\_fract\_x

\_atom\_site\_fract\_y

\_atom\_site\_fract\_z

\_atom\_site\_occupancy

|     |   |                    |                    |                    |     |
|-----|---|--------------------|--------------------|--------------------|-----|
| H1  | H | 0.9922127400000000 | 0.0926155700000000 | 0.0822024800000000 | 1.0 |
| H2  | H | 0.0045597100000000 | 0.1212230300000000 | 0.8865157500000000 | 1.0 |
| H3  | H | 0.9830045100000000 | 0.9660278600000000 | 0.9107527000000000 | 1.0 |
| H4  | H | 0.0604268300000000 | 0.8641120000000000 | 0.9977789700000000 | 1.0 |
| H5  | H | 0.9545264800000000 | 0.8509642900000000 | 0.0690232800000000 | 1.0 |
| H6  | H | 0.8812425900000000 | 0.8499810300000000 | 0.9878698800000000 | 1.0 |
| H7  | H | 0.8967558200000000 | 0.1419886900000000 | 0.9548340700000000 | 1.0 |
| H8  | H | 0.0741070100000000 | 0.1614409000000000 | 0.9576000900000000 | 1.0 |
| H9  | H | 0.2634270500000000 | 0.1149085300000000 | 0.0493339400000000 | 1.0 |
| H10 | H | 0.3410141400000000 | 0.0414569400000000 | 0.8815043300000000 | 1.0 |
| H11 | H | 0.2224558300000000 | 0.9389326100000000 | 0.9321692700000000 | 1.0 |
| H12 | H | 0.1247883000000000 | 0.9152980300000000 | 0.1149046100000000 | 1.0 |
| H13 | H | 0.3035177600000000 | 0.9048880400000000 | 0.1300473600000000 | 1.0 |
| H14 | H | 0.2181354300000000 | 0.8514622700000000 | 0.0717049000000000 | 1.0 |
| H15 | H | 0.1631643100000000 | 0.0414956200000000 | 0.8615725300000000 | 1.0 |
| H16 | H | 0.2450787000000000 | 0.1169496800000000 | 0.8849370800000000 | 1.0 |
| H17 | H | 0.4921742200000000 | 0.0925976300000000 | 0.0822371500000000 | 1.0 |
| H18 | H | 0.5045518800000000 | 0.1212915900000000 | 0.8865793900000000 | 1.0 |
| H19 | H | 0.4830072400000000 | 0.9660350500000000 | 0.9107658900000000 | 1.0 |
| H20 | H | 0.5605409900000000 | 0.8641264100000000 | 0.9978216800000000 | 1.0 |
| H21 | H | 0.4546070400000000 | 0.8509691100000000 | 0.0690509200000000 | 1.0 |
| H22 | H | 0.3813790600000000 | 0.8499463000000000 | 0.9878851100000000 | 1.0 |
| H23 | H | 0.3966883600000000 | 0.1419910300000000 | 0.9548946100000000 | 1.0 |
| H24 | H | 0.5740254600000000 | 0.1614640700000000 | 0.9577076600000000 | 1.0 |
| H25 | H | 0.7634746300000000 | 0.1149437800000000 | 0.0493076300000000 | 1.0 |
| H26 | H | 0.7224575500000000 | 0.9389487600000000 | 0.9321821100000000 | 1.0 |
| H27 | H | 0.6248440100000000 | 0.9153677200000000 | 0.1149571800000000 | 1.0 |
| H28 | H | 0.8035863200000000 | 0.9049691500000000 | 0.1300709200000000 | 1.0 |
| H29 | H | 0.7181576300000000 | 0.8515066100000000 | 0.0717777600000000 | 1.0 |
| H30 | H | 0.6630493100000000 | 0.0415360200000000 | 0.8615808500000000 | 1.0 |
| H31 | H | 0.7450137300000000 | 0.1169767700000000 | 0.8849449500000000 | 1.0 |
| H32 | H | 0.8409167100000000 | 0.0414755400000000 | 0.8814801700000000 | 1.0 |
| C33 | C | 0.9610624100000000 | 0.0562074800000000 | 0.0439263600000000 | 1.0 |
| C34 | C | 0.0394314000000000 | 0.0580009900000000 | 0.9770136600000000 | 1.0 |
| C35 | C | 0.0134280400000000 | 0.9808764000000000 | 0.9615393300000000 | 1.0 |
| C36 | C | 0.9250916000000000 | 0.9494478900000000 | 0.0201997100000000 | 1.0 |
| C37 | C | 0.9590069500000000 | 0.8745556180000000 | 0.0197739300000000 | 1.0 |
| C38 | C | 0.9992312800000000 | 0.1231795100000000 | 0.9411464800000000 | 1.0 |
| C39 | C | 0.2933953900000000 | 0.0648788800000000 | 0.0314343100000000 | 1.0 |
| C40 | C | 0.2029129900000000 | 0.0453466300000000 | 0.9675733200000000 | 1.0 |
| C41 | C | 0.1768045600000000 | 0.9688326200000000 | 0.9727726600000000 | 1.0 |
| C42 | C | 0.2569704700000000 | 0.9556380300000000 | 0.0389285700000000 | 1.0 |
| C43 | C | 0.2232274200000000 | 0.9024496600000000 | 0.0912384200000000 | 1.0 |
| C44 | C | 0.2410254400000000 | 0.0631965100000000 | 0.8953843000000000 | 1.0 |
| C45 | C | 0.4610423800000000 | 0.0561943600000000 | 0.0439541500000000 | 1.0 |
| C46 | C | 0.5394067700000000 | 0.0580088700000000 | 0.9770407200000000 | 1.0 |
| C47 | C | 0.5134266900000000 | 0.9808812600000000 | 0.9615528400000000 | 1.0 |
| C48 | C | 0.4251097700000000 | 0.9494335100000000 | 0.0202084500000000 | 1.0 |
| C49 | C | 0.4590937700000000 | 0.8745500500000000 | 0.0197958300000000 | 1.0 |
| C50 | C | 0.4991848300000000 | 0.1232052100000000 | 0.9412111000000000 | 1.0 |
| C51 | C | 0.7934120900000000 | 0.0649064700000000 | 0.0314177600000000 | 1.0 |
| C52 | C | 0.7028905900000000 | 0.0453649800000000 | 0.9675758900000000 | 1.0 |
| C53 | C | 0.6767979300000000 | 0.9688505600000000 | 0.9727814600000000 | 1.0 |
| C54 | C | 0.7569701000000000 | 0.9556695300000000 | 0.0389377700000000 | 1.0 |
| C55 | C | 0.7232632600000000 | 0.9025050500000000 | 0.0912797300000000 | 1.0 |

|     |   |                    |                    |                    |     |
|-----|---|--------------------|--------------------|--------------------|-----|
| C56 | C | 0.7409466100000000 | 0.0632230900000000 | 0.8953825300000000 | 1.0 |
| O57 | O | 0.9793774900000000 | 0.9909316300000000 | 0.0729710100000000 | 1.0 |
| O58 | O | 0.2416843300000000 | 0.0166985000000000 | 0.0765879600000000 | 1.0 |
| O59 | O | 0.4793675800000000 | 0.9909156400000000 | 0.0729872500000000 | 1.0 |
| O60 | O | 0.7416986000000000 | 0.0167394700000000 | 0.0765845100000000 | 1.0 |

##### cif ends

furane\_CH3\_3\_anti\_alt Energy: -292.34590661

##### cif starts

data\_furane\_CH3\_3\_anti\_alt

\_publ\_section\_comment

;  
Andrew Reynoso, Bohan Xu, and Vincent H. Crespi  
;

\_cell\_length\_a 9.4454315969

\_cell\_length\_b 20.0

\_cell\_length\_c 20.0

\_cell\_angle\_alpha 90.0

\_cell\_angle\_beta 90.0

\_cell\_angle\_gamma 90.0

\_symmetry\_space\_group\_name\_H-M 'P 1'

\_symmetry\_Int\_Tables\_number 1

\_symmetry\_cell\_setting triclinic

loop\_

\_atom\_site\_label

\_atom\_site\_type\_symbol

\_atom\_site\_fract\_x

\_atom\_site\_fract\_y

\_atom\_site\_fract\_z

\_atom\_site\_occupancy

|     |   |                    |                    |                    |     |
|-----|---|--------------------|--------------------|--------------------|-----|
| H1  | H | 0.0504280700000000 | 0.9041372900000000 | 0.9161378000000000 | 1.0 |
| H2  | H | 0.1298893800000000 | 0.9322902000000000 | 0.0948402800000000 | 1.0 |
| H3  | H | 0.0342406300000000 | 0.0537959500000000 | 0.0636405700000000 | 1.0 |
| H4  | H | 0.0439335300000000 | 0.1072211000000000 | 0.9358451900000000 | 1.0 |
| H5  | H | 0.9486324500000000 | 0.9196190800000000 | 0.1100710700000000 | 1.0 |
| H6  | H | 0.0405287400000000 | 0.8629946900000000 | 0.0575175400000000 | 1.0 |
| H7  | H | 0.3004219800000000 | 0.0992551700000000 | 0.0466047000000000 | 1.0 |
| H8  | H | 0.3798958200000000 | 0.0710884100000000 | 0.8679149100000000 | 1.0 |
| H9  | H | 0.2842523300000000 | 0.9495892200000000 | 0.8991070000000000 | 1.0 |
| H10 | H | 0.2939321500000000 | 0.8961677500000000 | 0.0269037800000000 | 1.0 |
| H11 | H | 0.1986481200000000 | 0.0837651400000000 | 0.8526798700000000 | 1.0 |
| H12 | H | 0.2905457300000000 | 0.1403890000000000 | 0.9052326700000000 | 1.0 |
| H13 | H | 0.5504138300000000 | 0.9041354200000000 | 0.9161407500000000 | 1.0 |
| H14 | H | 0.6299013600000000 | 0.9322776700000000 | 0.0948345000000000 | 1.0 |
| H15 | H | 0.5342473800000000 | 0.0537989200000000 | 0.0636402700000000 | 1.0 |
| H16 | H | 0.5439417100000000 | 0.1072203400000000 | 0.9358441500000000 | 1.0 |
| H17 | H | 0.4486402400000000 | 0.9196401000000000 | 0.1100806900000000 | 1.0 |
| H18 | H | 0.5404742400000000 | 0.8629939900000000 | 0.0575262600000000 | 1.0 |
| H19 | H | 0.8004141800000000 | 0.0992494800000000 | 0.0466015300000000 | 1.0 |
| H20 | H | 0.8798724600000000 | 0.0710535400000000 | 0.8678956400000000 | 1.0 |



|     |   |                    |                    |                    |     |
|-----|---|--------------------|--------------------|--------------------|-----|
| H21 | H | 0.7842414800000000 | 0.9495824300000000 | 0.8991046700000000 | 1.0 |
| H22 | H | 0.7939372200000000 | 0.8961635600000000 | 0.0268999200000000 | 1.0 |
| H23 | H | 0.6986295900000000 | 0.0837766300000000 | 0.8526833900000000 | 1.0 |
| H24 | H | 0.7906213900000000 | 0.1403748000000000 | 0.9052265300000000 | 1.0 |
| C25 | C | 0.0743363800000000 | 0.9498773900000000 | 0.9444188500000000 | 1.0 |
| C26 | C | 0.9866643900000000 | 0.9578513200000000 | 0.0104357800000000 | 1.0 |
| C27 | C | 0.9873555100000000 | 0.0366675700000000 | 0.0164454100000000 | 1.0 |
| C28 | C | 0.0716541600000000 | 0.0575766300000000 | 0.9549692400000000 | 1.0 |
| C29 | C | 0.0313727000000000 | 0.9160955100000000 | 0.0716533100000000 | 1.0 |
| C30 | C | 0.3243303100000000 | 0.0535089800000000 | 0.0183275100000000 | 1.0 |
| C31 | C | 0.2366672500000000 | 0.0455356200000000 | 0.9523143100000000 | 1.0 |
| C32 | C | 0.2373633800000000 | 0.9667180900000000 | 0.9463028300000000 | 1.0 |
| C33 | C | 0.3216524400000000 | 0.9458166900000000 | 0.0077801200000000 | 1.0 |
| C34 | C | 0.2813819000000000 | 0.0872876300000000 | 0.8911008300000000 | 1.0 |
| C35 | C | 0.5743291500000000 | 0.9498756300000000 | 0.9444198700000000 | 1.0 |
| C36 | C | 0.4866623400000000 | 0.9578531000000000 | 0.0104384700000000 | 1.0 |
| C37 | C | 0.4873588300000000 | 0.0366699300000000 | 0.0164463700000000 | 1.0 |
| C38 | C | 0.5716569800000000 | 0.0575759400000000 | 0.9549679700000000 | 1.0 |
| C39 | C | 0.5313660000000000 | 0.9160984300000000 | 0.0716569500000000 | 1.0 |
| C40 | C | 0.8243273800000000 | 0.0535059700000000 | 0.0183259400000000 | 1.0 |
| C41 | C | 0.7366675800000000 | 0.0455302800000000 | 0.9523109300000000 | 1.0 |
| C42 | C | 0.7373592000000000 | 0.9667132600000000 | 0.9462999900000000 | 1.0 |
| C43 | C | 0.8216524900000000 | 0.9458101700000000 | 0.0077782400000000 | 1.0 |
| C44 | C | 0.7813887800000000 | 0.0872765600000000 | 0.8910942700000000 | 1.0 |
| O45 | O | 0.0270809000000000 | 0.0070679900000000 | 0.9063650900000000 | 1.0 |
| O46 | O | 0.2770497300000000 | 0.9963241300000000 | 0.0563779800000000 | 1.0 |
| O47 | O | 0.5270752200000000 | 0.0070664800000000 | 0.9063649500000000 | 1.0 |
| O48 | O | 0.7770489800000000 | 0.9963188300000000 | 0.0563751200000000 | 1.0 |

##### cif ends

furane\_CH3\_3\_anti\_alt\_forbid Energy: -293.02630765

##### cif starts

data\_furane\_CH3\_3\_anti\_alt\_forbid

\_publ\_section\_comment

;

Andrew Reynoso, Bohan Xu, and Vincent H. Crespi

;

\_cell\_length\_a 10.2556421763

\_cell\_length\_b 20.0

\_cell\_length\_c 20.0

\_cell\_angle\_alpha 90.0

\_cell\_angle\_beta 90.0

\_cell\_angle\_gamma 90.0

\_symmetry\_space\_group\_name\_H-M 'P 1'

\_symmetry\_Int\_Tables\_number 1

\_symmetry\_cell\_setting triclinic

loop\_

\_atom\_site\_label

\_atom\_site\_type\_symbol

\_atom\_site\_fract\_x

|     |   | _atom_site_fract_y |                    | _atom_site_fract_z |     | _atom_site_occupancy |  |
|-----|---|--------------------|--------------------|--------------------|-----|----------------------|--|
| H1  | H | 0.0694035500000000 | 0.0913600900000000 | 0.9261027200000000 | 1.0 |                      |  |
| H2  | H | 0.9528201600000000 | 0.9367599100000000 | 0.0609804900000000 | 1.0 |                      |  |
| H3  | H | 0.0703794800000000 | 0.8885493300000000 | 0.9449697800000000 | 1.0 |                      |  |
| H4  | H | 0.3310714300000000 | 0.0520131900000000 | 0.9120255800000000 | 1.0 |                      |  |
| H5  | H | 0.2136267000000000 | 0.1002714900000000 | 0.0280623100000000 | 1.0 |                      |  |
| H6  | H | 0.2144790400000000 | 0.8974639900000000 | 0.0469652000000000 | 1.0 |                      |  |
| H7  | H | 0.5690391400000000 | 0.0914744000000000 | 0.9264290500000000 | 1.0 |                      |  |
| H8  | H | 0.4533624000000000 | 0.9364677300000000 | 0.0610329200000000 | 1.0 |                      |  |
| H9  | H | 0.5704886900000000 | 0.8886042900000000 | 0.9447053400000000 | 1.0 |                      |  |
| H10 | H | 0.8306890400000000 | 0.0523517300000000 | 0.9119710500000000 | 1.0 |                      |  |
| H11 | H | 0.7134400700000000 | 0.1001806900000000 | 0.0282787700000000 | 1.0 |                      |  |
| H12 | H | 0.7149423100000000 | 0.8973164200000000 | 0.0465444500000000 | 1.0 |                      |  |
| H13 | H | 0.0395298300000000 | 0.0711868600000000 | 0.0981181100000000 | 1.0 |                      |  |
| H14 | H | 0.8675948200000000 | 0.0667516400000000 | 0.0983199900000000 | 1.0 |                      |  |
| H15 | H | 0.9470180000000000 | 0.1326732700000000 | 0.0545462800000000 | 1.0 |                      |  |
| H16 | H | 0.5392617200000000 | 0.0703541300000000 | 0.0985521100000000 | 1.0 |                      |  |
| H17 | H | 0.3672819500000000 | 0.0663427900000000 | 0.0985164600000000 | 1.0 |                      |  |
| H18 | H | 0.4475415800000000 | 0.1323084900000000 | 0.0552000200000000 | 1.0 |                      |  |
| H19 | H | 0.4162245300000000 | 0.9218806200000000 | 0.8747273000000000 | 1.0 |                      |  |
| H20 | H | 0.2442880600000000 | 0.9174773200000000 | 0.8749825700000000 | 1.0 |                      |  |
| H21 | H | 0.3367990600000000 | 0.8560368100000000 | 0.9186116200000000 | 1.0 |                      |  |
| H22 | H | 0.9168413400000000 | 0.9223139100000000 | 0.8745366900000000 | 1.0 |                      |  |
| H23 | H | 0.7448395100000000 | 0.9183797300000000 | 0.8744051700000000 | 1.0 |                      |  |
| H24 | H | 0.8363637400000000 | 0.8564202000000000 | 0.9178565700000000 | 1.0 |                      |  |
| C25 | C | 0.9524897900000000 | 0.0791427100000000 | 0.0673841400000000 | 1.0 |                      |  |
| C26 | C | 0.3313550300000000 | 0.9095518000000000 | 0.9057032800000000 | 1.0 |                      |  |
| C27 | C | 0.4524348500000000 | 0.0787005000000000 | 0.0677540100000000 | 1.0 |                      |  |
| C28 | C | 0.8315922700000000 | 0.9100232600000000 | 0.9052554900000000 | 1.0 |                      |  |
| C29 | C | 0.0783600700000000 | 0.0484335300000000 | 0.9602627600000000 | 1.0 |                      |  |
| C30 | C | 0.9564939000000000 | 0.0362555000000000 | 0.0043884100000000 | 1.0 |                      |  |
| C31 | C | 0.9570279700000000 | 0.9573265700000000 | 0.0100974800000000 | 1.0 |                      |  |
| C32 | C | 0.0791125500000000 | 0.9367716700000000 | 0.9708302900000000 | 1.0 |                      |  |
| C33 | C | 0.2048572400000000 | 0.0520458400000000 | 0.0022093100000000 | 1.0 |                      |  |
| C34 | C | 0.3269040500000000 | 0.0314582700000000 | 0.9629148300000000 | 1.0 |                      |  |
| C35 | C | 0.3274428200000000 | 0.9525189900000000 | 0.9686517700000000 | 1.0 |                      |  |
| C36 | C | 0.2055878600000000 | 0.9403837700000000 | 0.0127958600000000 | 1.0 |                      |  |
| C37 | C | 0.5781987000000000 | 0.0484405900000000 | 0.9604403600000000 | 1.0 |                      |  |
| C38 | C | 0.4564703400000000 | 0.0360614400000000 | 0.0045893100000000 | 1.0 |                      |  |
| C39 | C | 0.4571655600000000 | 0.9571318000000000 | 0.0101799200000000 | 1.0 |                      |  |
| C40 | C | 0.5791421000000000 | 0.9367614400000000 | 0.9706866600000000 | 1.0 |                      |  |
| C41 | C | 0.7048105000000000 | 0.0520254400000000 | 0.0022860800000000 | 1.0 |                      |  |
| C42 | C | 0.8268189900000000 | 0.0316596900000000 | 0.9628131200000000 | 1.0 |                      |  |
| C43 | C | 0.8274968500000000 | 0.9527155100000000 | 0.9683901300000000 | 1.0 |                      |  |
| C44 | C | 0.7057502600000000 | 0.9403426100000000 | 0.0125281300000000 | 1.0 |                      |  |
| O45 | O | 0.0866407500000000 | 0.9886681800000000 | 0.9197229000000000 | 1.0 |                      |  |
| O46 | O | 0.1973503900000000 | 0.0001591000000000 | 0.0533234600000000 | 1.0 |                      |  |
| O47 | O | 0.5863719200000000 | 0.9887963700000000 | 0.9197125400000000 | 1.0 |                      |  |
| O48 | O | 0.6975927100000000 | 0.9999841300000000 | 0.0532540800000000 | 1.0 |                      |  |

##### cif ends

furan\_CH3\_3\_anti\_dir    Energy: -292.31543592

##### cif starts

data\_furan\_CH3\_3\_anti\_dir

\_publ\_section\_comment

;  
Andrew Reynoso, Bohan Xu, and Vincent H. Crespi  
;

\_cell\_length\_a 9.4557505809

\_cell\_length\_b 20.0

\_cell\_length\_c 20.0

\_cell\_angle\_alpha 90.0

\_cell\_angle\_beta 90.0

\_cell\_angle\_gamma 90.0

\_symmetry\_space\_group\_name\_H-M 'P 1'

\_symmetry\_Int\_Tables\_number 1

\_symmetry\_cell\_setting triclinic

loop\_

\_atom\_site\_label

\_atom\_site\_type\_symbol

\_atom\_site\_fract\_x

\_atom\_site\_fract\_y

\_atom\_site\_fract\_z

\_atom\_site\_occupancy

|     |   |                    |                    |                    |     |
|-----|---|--------------------|--------------------|--------------------|-----|
| H1  | H | 0.9956309400000000 | 0.0898977300000000 | 0.9217641200000000 | 1.0 |
| H2  | H | 0.8969525900000000 | 0.0571896500000000 | 0.1114883300000000 | 1.0 |
| H3  | H | 0.9834257300000000 | 0.9268205500000000 | 0.0527315100000000 | 1.0 |
| H4  | H | 0.9973561500000000 | 0.8858420500000000 | 0.9189084800000000 | 1.0 |
| H5  | H | 0.0779130500000000 | 0.0440597800000000 | 0.0957775200000000 | 1.0 |
| H6  | H | 0.9923866100000000 | 0.1172944100000000 | 0.0645160100000000 | 1.0 |
| H7  | H | 0.2456428600000000 | 0.0894380700000000 | 0.0307268100000000 | 1.0 |
| H8  | H | 0.3278875200000000 | 0.0450505400000000 | 0.8563136700000000 | 1.0 |
| H9  | H | 0.2334201200000000 | 0.9274687100000000 | 0.8983937000000000 | 1.0 |
| H10 | H | 0.2473455500000000 | 0.8853639300000000 | 0.0318625600000000 | 1.0 |
| H11 | H | 0.1469259000000000 | 0.0583199700000000 | 0.8407316700000000 | 1.0 |
| H12 | H | 0.2423986200000000 | 0.1180311000000000 | 0.8881864000000000 | 1.0 |
| H13 | H | 0.4956250600000000 | 0.0898927900000000 | 0.9217640100000000 | 1.0 |
| H14 | H | 0.3969636100000000 | 0.0571658100000000 | 0.1114962100000000 | 1.0 |
| H15 | H | 0.4834185500000000 | 0.9268163900000000 | 0.0527343200000000 | 1.0 |
| H16 | H | 0.4973571800000000 | 0.8858376100000000 | 0.9189127500000000 | 1.0 |
| H17 | H | 0.5779284800000000 | 0.0440669000000000 | 0.0957739100000000 | 1.0 |
| H18 | H | 0.4923429700000000 | 0.1172921900000000 | 0.0645265500000000 | 1.0 |
| H19 | H | 0.7456416000000000 | 0.0894412300000000 | 0.0307209300000000 | 1.0 |
| H20 | H | 0.8279041600000000 | 0.0450673100000000 | 0.8563217000000000 | 1.0 |
| H21 | H | 0.7334195000000000 | 0.9274646200000000 | 0.8983962900000000 | 1.0 |
| H22 | H | 0.7473529500000000 | 0.8853669700000000 | 0.0318669300000000 | 1.0 |
| H23 | H | 0.6469306400000000 | 0.0582793600000000 | 0.8407202700000000 | 1.0 |
| H24 | H | 0.7423065200000000 | 0.1180309300000000 | 0.8881690800000000 | 1.0 |
| C25 | C | 0.0211089700000000 | 0.0417699900000000 | 0.9451299900000000 | 1.0 |
| C26 | C | 0.9355145100000000 | 0.0274790000000000 | 0.0090286900000000 | 1.0 |
| C27 | C | 0.9370987800000000 | 0.9484104000000000 | 0.0072758700000000 | 1.0 |
| C28 | C | 0.0234903600000000 | 0.9335436600000000 | 0.9432048800000000 | 1.0 |
| C29 | C | 0.9806079700000000 | 0.0632714300000000 | 0.0739004300000000 | 1.0 |

|     |   |                    |                    |                    |     |
|-----|---|--------------------|--------------------|--------------------|-----|
| C30 | C | 0.2711141700000000 | 0.0415083200000000 | 0.0069596500000000 | 1.0 |
| C31 | C | 0.1855159900000000 | 0.0277588400000000 | 0.9429376800000000 | 1.0 |
| C32 | C | 0.1870958000000000 | 0.9486775500000000 | 0.9440294200000000 | 1.0 |
| C33 | C | 0.2734892600000000 | 0.9332678000000000 | 0.0079724900000000 | 1.0 |
| C34 | C | 0.2305990400000000 | 0.0640878100000000 | 0.8783607300000000 | 1.0 |
| C35 | C | 0.5211057200000000 | 0.0417665800000000 | 0.9451309600000000 | 1.0 |
| C36 | C | 0.4355142200000000 | 0.0274757600000000 | 0.0090313600000000 | 1.0 |
| C37 | C | 0.4370967700000000 | 0.9484070300000000 | 0.0072785700000000 | 1.0 |
| C38 | C | 0.5234896800000000 | 0.9335396600000000 | 0.9432078600000000 | 1.0 |
| C39 | C | 0.4806049000000000 | 0.0632659000000000 | 0.0739045400000000 | 1.0 |
| C40 | C | 0.7711145400000000 | 0.0415105400000000 | 0.0069561300000000 | 1.0 |
| C41 | C | 0.6855126200000000 | 0.0277564900000000 | 0.9429361300000000 | 1.0 |
| C42 | C | 0.6870953000000000 | 0.9486752700000000 | 0.9440312100000000 | 1.0 |
| C43 | C | 0.7734926100000000 | 0.9332694700000000 | 0.0079739400000000 | 1.0 |
| C44 | C | 0.7305832300000000 | 0.0640820600000000 | 0.8783554100000000 | 1.0 |
| O45 | O | 0.9765940400000000 | 0.9877525300000000 | 0.9007313500000000 | 1.0 |
| O46 | O | 0.2266063200000000 | 0.9871168500000000 | 0.0509052100000000 | 1.0 |
| O47 | O | 0.4765892800000000 | 0.9877476700000000 | 0.9007342400000000 | 1.0 |
| O48 | O | 0.7266110900000000 | 0.9871208000000000 | 0.0509045000000000 | 1.0 |

##### cif ends

furan\_CH3\_3\_anti\_dir\_forbid Energy: -293.02810247

##### cif starts

data\_furan\_CH3\_3\_anti\_dir\_forbid

\_publ\_section\_comment

;  
Andrew Reynoso, Bohan Xu, and Vincent H. Crespi  
;

\_cell\_length\_a 10.2567651642

\_cell\_length\_b 20.0

\_cell\_length\_c 20.0

\_cell\_angle\_alpha 90.0

\_cell\_angle\_beta 90.0

\_cell\_angle\_gamma 90.0

\_symmetry\_space\_group\_name\_H-M 'P 1'

\_symmetry\_Int\_Tables\_number 1

\_symmetry\_cell\_setting triclinic

loop\_

\_atom\_site\_label

\_atom\_site\_type\_symbol

\_atom\_site\_fract\_x

\_atom\_site\_fract\_y

\_atom\_site\_fract\_z

\_atom\_site\_occupancy

|    |   |                    |                    |                    |     |
|----|---|--------------------|--------------------|--------------------|-----|
| H1 | H | 0.0860209000000000 | 0.0958820500000000 | 0.9394703400000000 | 1.0 |
| H2 | H | 0.8827293000000000 | 0.0555558600000000 | 0.1077809700000000 | 1.0 |
| H3 | H | 0.9676425800000000 | 0.9297759400000000 | 0.0585462400000000 | 1.0 |
| H4 | H | 0.0839622900000000 | 0.8922126200000000 | 0.9377492200000000 | 1.0 |
| H5 | H | 0.0546102600000000 | 0.0596198600000000 | 0.1084064100000000 | 1.0 |
| H6 | H | 0.9630537900000000 | 0.1252524600000000 | 0.0708098600000000 | 1.0 |

|     |   |                    |                    |                    |     |
|-----|---|--------------------|--------------------|--------------------|-----|
| H7  | H | 0.2283337600000000 | 0.0950159900000000 | 0.0416858000000000 | 1.0 |
| H8  | H | 0.4316786700000000 | 0.0574317800000000 | 0.8727286500000000 | 1.0 |
| H9  | H | 0.3466518400000000 | 0.9309200000000000 | 0.9198467500000000 | 1.0 |
| H10 | H | 0.2303424400000000 | 0.8913470200000000 | 0.0399984000000000 | 1.0 |
| H11 | H | 0.2597917900000000 | 0.0613852700000000 | 0.8720650700000000 | 1.0 |
| H12 | H | 0.3510935500000000 | 0.1265117900000000 | 0.9106940100000000 | 1.0 |
| H13 | H | 0.5859997500000000 | 0.0958902000000000 | 0.9394821300000000 | 1.0 |
| H14 | H | 0.3826723700000000 | 0.0556045100000000 | 0.1077664000000000 | 1.0 |
| H15 | H | 0.4676946200000000 | 0.9297650900000000 | 0.0585441500000000 | 1.0 |
| H16 | H | 0.5839182700000000 | 0.8922238700000000 | 0.9377108100000000 | 1.0 |
| H17 | H | 0.5545673500000000 | 0.0594723000000000 | 0.1084579800000000 | 1.0 |
| H18 | H | 0.4633486700000000 | 0.1252314900000000 | 0.0708659500000000 | 1.0 |
| H19 | H | 0.7283379500000000 | 0.0949958700000000 | 0.0416869300000000 | 1.0 |
| H20 | H | 0.9317049100000000 | 0.0574650300000000 | 0.8727201700000000 | 1.0 |
| H21 | H | 0.8467228700000000 | 0.9309293300000000 | 0.9198175400000000 | 1.0 |
| H22 | H | 0.7303552700000000 | 0.8913261200000000 | 0.0399413900000000 | 1.0 |
| H23 | H | 0.7598149100000000 | 0.0613742000000000 | 0.8720392900000000 | 1.0 |
| H24 | H | 0.8510383800000000 | 0.1265213100000000 | 0.9106804200000000 | 1.0 |
| C25 | C | 0.0941804500000000 | 0.0498699900000000 | 0.9691451000000000 | 1.0 |
| C26 | C | 0.9722223600000000 | 0.0340743200000000 | 0.0115536200000000 | 1.0 |
| C27 | C | 0.9717303200000000 | 0.9549749400000000 | 0.0097915700000000 | 1.0 |
| C28 | C | 0.0935762200000000 | 0.9377263400000000 | 0.9682886200000000 | 1.0 |
| C29 | C | 0.9679563500000000 | 0.0707111700000000 | 0.0783568400000000 | 1.0 |
| C30 | C | 0.2201503200000000 | 0.0495145400000000 | 0.0112370700000000 | 1.0 |
| C31 | C | 0.3420839100000000 | 0.0344184300000000 | 0.9685535900000000 | 1.0 |
| C32 | C | 0.3425733800000000 | 0.9553056600000000 | 0.9690139200000000 | 1.0 |
| C33 | C | 0.2207374900000000 | 0.9373714700000000 | 0.0102329100000000 | 1.0 |
| C34 | C | 0.3463508200000000 | 0.0720883700000000 | 0.9023275200000000 | 1.0 |
| C35 | C | 0.5941721500000000 | 0.0498704500000000 | 0.9691446800000000 | 1.0 |
| C36 | C | 0.4722308000000000 | 0.0340670600000000 | 0.0115648100000000 | 1.0 |
| C37 | C | 0.4717409900000000 | 0.9549695500000000 | 0.0097918200000000 | 1.0 |
| C38 | C | 0.5935623900000000 | 0.9377282000000000 | 0.9682615300000000 | 1.0 |
| C39 | C | 0.4680042500000000 | 0.0706806700000000 | 0.0783823400000000 | 1.0 |
| C40 | C | 0.7201538800000000 | 0.0495034400000000 | 0.0112255000000000 | 1.0 |
| C41 | C | 0.8420876500000000 | 0.0344201000000000 | 0.9685344400000000 | 1.0 |
| C42 | C | 0.8425899700000000 | 0.9553079700000000 | 0.9689871000000000 | 1.0 |
| C43 | C | 0.7207439600000000 | 0.9373603300000000 | 0.0101919100000000 | 1.0 |
| C44 | C | 0.8463511800000000 | 0.0720968100000000 | 0.9023123400000000 | 1.0 |
| O45 | O | 0.1016415800000000 | 0.9939977500000000 | 0.9227107800000000 | 1.0 |
| O46 | O | 0.2126915500000000 | 0.9928759800000000 | 0.0567412300000000 | 1.0 |
| O47 | O | 0.6016075300000000 | 0.9940090700000000 | 0.9226962200000000 | 1.0 |
| O48 | O | 0.7127078000000000 | 0.9928527900000000 | 0.0567161600000000 | 1.0 |

##### cif ends

furane\_CH3\_3\_syn\_alt Energy: -293.05220959

##### cif starts

data\_furane\_CH3\_3\_syn\_alt

\_publ\_section\_comment

;  
Andrew Reynoso, Bohan Xu, and Vincent H. Crespi  
;

\_cell\_length\_a 10.3637712242

\_cell\_length\_b 20.0  
\_cell\_length\_c 20.0  
\_cell\_angle\_alpha 90.0  
\_cell\_angle\_beta 90.0  
\_cell\_angle\_gamma 90.0

\_symmetry\_space\_group\_name\_H-M 'P 1'  
\_symmetry\_Int\_Tables\_number 1  
\_symmetry\_cell\_setting triclinic

loop\_

\_atom\_site\_label  
\_atom\_site\_type\_symbol  
\_atom\_site\_fract\_x  
\_atom\_site\_fract\_y  
\_atom\_site\_fract\_z  
\_atom\_site\_occupancy

|     |   |                    |                    |                    |     |
|-----|---|--------------------|--------------------|--------------------|-----|
| H1  | H | 0.9641469600000000 | 0.9347015700000000 | 0.0731231100000000 | 1.0 |
| H2  | H | 0.0030806700000000 | 0.9749784500000000 | 0.9048489300000000 | 1.0 |
| H3  | H | 0.0879272400000000 | 0.0981715000000000 | 0.9545831400000000 | 1.0 |
| H4  | H | 0.9615529800000000 | 0.1379496700000000 | 0.0703673700000000 | 1.0 |
| H5  | H | 0.1728599200000000 | 0.9746005800000000 | 0.9049607900000000 | 1.0 |
| H6  | H | 0.0873158100000000 | 0.9066531000000000 | 0.9403512200000000 | 1.0 |
| H7  | H | 0.2142115000000000 | 0.1379155200000000 | 0.0704047900000000 | 1.0 |
| H8  | H | 0.4228763200000000 | 0.0934034900000000 | 0.9033534800000000 | 1.0 |
| H9  | H | 0.3378884500000000 | 0.9713050600000000 | 0.9562940100000000 | 1.0 |
| H10 | H | 0.2115604200000000 | 0.9346679700000000 | 0.0731165400000000 | 1.0 |
| H11 | H | 0.2531076800000000 | 0.0930207900000000 | 0.9032398300000000 | 1.0 |
| H12 | H | 0.3373306600000000 | 0.1623166200000000 | 0.9368198200000000 | 1.0 |
| H13 | H | 0.4642130900000000 | 0.9346761300000000 | 0.0731150400000000 | 1.0 |
| H14 | H | 0.5030140700000000 | 0.9748919200000000 | 0.9048754600000000 | 1.0 |
| H15 | H | 0.5878369700000000 | 0.0981665400000000 | 0.9545667200000000 | 1.0 |
| H16 | H | 0.4615523600000000 | 0.1379223000000000 | 0.0703976600000000 | 1.0 |
| H17 | H | 0.6727929900000000 | 0.9747421500000000 | 0.9049085900000000 | 1.0 |
| H18 | H | 0.5876493900000000 | 0.9066679200000000 | 0.9403182000000000 | 1.0 |
| H19 | H | 0.7141851900000000 | 0.1379577100000000 | 0.0703462100000000 | 1.0 |
| H20 | H | 0.9227721600000000 | 0.0932108100000000 | 0.9032576200000000 | 1.0 |
| H21 | H | 0.8378880400000000 | 0.9713213200000000 | 0.9562793500000000 | 1.0 |
| H22 | H | 0.7115986000000000 | 0.9347096000000000 | 0.0731198300000000 | 1.0 |
| H23 | H | 0.7529955200000000 | 0.0933418200000000 | 0.9032810800000000 | 1.0 |
| H24 | H | 0.8381008400000000 | 0.1623634100000000 | 0.9368223200000000 | 1.0 |
| C25 | C | 0.9629882700000000 | 0.9823910900000000 | 0.0457964700000000 | 1.0 |
| C26 | C | 0.0878708500000000 | 0.9958920100000000 | 0.0030481900000000 | 1.0 |
| C27 | C | 0.0878934800000000 | 0.0749183100000000 | 0.0041027200000000 | 1.0 |
| C28 | C | 0.9627518700000000 | 0.0895394300000000 | 0.0443398000000000 | 1.0 |
| C29 | C | 0.0877878000000000 | 0.9614562000000000 | 0.9348361900000000 | 1.0 |
| C30 | C | 0.2130019500000000 | 0.0895123500000000 | 0.0443652100000000 | 1.0 |
| C31 | C | 0.3378744100000000 | 0.0748474600000000 | 0.0019857700000000 | 1.0 |
| C32 | C | 0.3378842200000000 | 0.9958824400000000 | 0.0051704200000000 | 1.0 |
| C33 | C | 0.2127510800000000 | 0.9823611100000000 | 0.0457964200000000 | 1.0 |
| C34 | C | 0.3378007200000000 | 0.1073810900000000 | 0.9328458400000000 | 1.0 |
| C35 | C | 0.4630108500000000 | 0.9823700900000000 | 0.0457964400000000 | 1.0 |
| C36 | C | 0.5878781400000000 | 0.9958969000000000 | 0.0030387700000000 | 1.0 |
| C37 | C | 0.5878689200000000 | 0.0749211600000000 | 0.0040894900000000 | 1.0 |
| C38 | C | 0.4627496100000000 | 0.0895223300000000 | 0.0443529100000000 | 1.0 |

|     |   |                    |                    |                    |     |
|-----|---|--------------------|--------------------|--------------------|-----|
| C39 | C | 0.5878387800000000 | 0.9614732200000000 | 0.9348201400000000 | 1.0 |
| C40 | C | 0.7129993400000000 | 0.0895453400000000 | 0.0443231900000000 | 1.0 |
| C41 | C | 0.8378908200000000 | 0.0748740900000000 | 0.0019561500000000 | 1.0 |
| C42 | C | 0.8378837900000000 | 0.9959082900000000 | 0.0051508600000000 | 1.0 |
| C43 | C | 0.7127654800000000 | 0.9823938400000000 | 0.0457848600000000 | 1.0 |
| C44 | C | 0.8379402300000000 | 0.1074289700000000 | 0.9328256900000000 | 1.0 |
| O45 | O | 0.9628560100000000 | 0.0366113400000000 | 0.0927656600000000 | 1.0 |
| O46 | O | 0.2128707500000000 | 0.0365711700000000 | 0.0927773900000000 | 1.0 |
| O47 | O | 0.4628830800000000 | 0.0365841800000000 | 0.0927716300000000 | 1.0 |
| O48 | O | 0.7128857500000000 | 0.0366196000000000 | 0.0927516900000000 | 1.0 |

##### cif ends

furan\_CH3\_3\_syn\_alt\_forbid Energy: -289.95117586

##### cif starts

data\_furan\_CH3\_3\_syn\_alt\_forbid

\_publ\_section\_comment

;  
Andrew Reynoso, Bohan Xu, and Vincent H. Crespi  
;

\_cell\_length\_a 9.6130636243

\_cell\_length\_b 20.0

\_cell\_length\_c 20.0

\_cell\_angle\_alpha 90.0

\_cell\_angle\_beta 90.0

\_cell\_angle\_gamma 90.0

\_symmetry\_space\_group\_name\_H-M 'P 1'

\_symmetry\_Int\_Tables\_number 1

\_symmetry\_cell\_setting triclinic

loop\_

\_atom\_site\_label

\_atom\_site\_type\_symbol

\_atom\_site\_fract\_x

\_atom\_site\_fract\_y

\_atom\_site\_fract\_z

\_atom\_site\_occupancy

|     |   |                    |                    |                    |     |
|-----|---|--------------------|--------------------|--------------------|-----|
| H1  | H | 0.9036106400000000 | 0.0955177500000000 | 0.0784506200000000 | 1.0 |
| H2  | H | 0.9064812300000000 | 0.0700190100000000 | 0.9427023500000000 | 1.0 |
| H3  | H | 0.8910765700000000 | 0.8942073800000000 | 0.0625409900000000 | 1.0 |
| H4  | H | 0.1630811100000000 | 0.1030773300000000 | 0.0663746700000000 | 1.0 |
| H5  | H | 0.1476893700000000 | 0.9317549200000000 | 0.9402089200000000 | 1.0 |
| H6  | H | 0.1506864600000000 | 0.9013230100000000 | 0.0749236600000000 | 1.0 |
| H7  | H | 0.4035271000000000 | 0.0956591400000000 | 0.0783854100000000 | 1.0 |
| H8  | H | 0.4065817100000000 | 0.0700673300000000 | 0.9426708400000000 | 1.0 |
| H9  | H | 0.3911268600000000 | 0.8943351500000000 | 0.0626291100000000 | 1.0 |
| H10 | H | 0.6631510000000000 | 0.1029740300000000 | 0.0664901200000000 | 1.0 |
| H11 | H | 0.6475609600000000 | 0.9318100000000000 | 0.9401262400000000 | 1.0 |
| H12 | H | 0.6506458200000000 | 0.9012125000000000 | 0.0748021100000000 | 1.0 |
| H13 | H | 0.1602396300000000 | 0.1266696800000000 | 0.9193661900000000 | 1.0 |
| H14 | H | 0.0754372500000000 | 0.0622374800000000 | 0.8747119400000000 | 1.0 |
| H15 | H | 0.2539369000000000 | 0.0550990400000000 | 0.8925324000000000 | 1.0 |

|     |   |                    |                    |                    |     |
|-----|---|--------------------|--------------------|--------------------|-----|
| H16 | H | 0.6608117000000000 | 0.1266761900000000 | 0.9194566300000000 | 1.0 |
| H17 | H | 0.5754528800000000 | 0.0624261100000000 | 0.8747824700000000 | 1.0 |
| H18 | H | 0.7539228200000000 | 0.0549628500000000 | 0.8925188200000000 | 1.0 |
| H19 | H | 0.9784536900000000 | 0.9427813700000000 | 0.8723663100000000 | 1.0 |
| H20 | H | 0.7998897600000000 | 0.9476686400000000 | 0.8908025000000000 | 1.0 |
| H21 | H | 0.8964661100000000 | 0.8759027800000000 | 0.9145808600000000 | 1.0 |
| H22 | H | 0.4783824700000000 | 0.9426960200000000 | 0.8724076300000000 | 1.0 |
| H23 | H | 0.2998490800000000 | 0.9479441400000000 | 0.8907869200000000 | 1.0 |
| H24 | H | 0.3957728800000000 | 0.8759954300000000 | 0.9146267300000000 | 1.0 |
| C25 | C | 0.8679933400000000 | 0.0526176100000000 | 0.0487547600000000 | 1.0 |
| C26 | C | 0.9481321500000000 | 0.0404422900000000 | 0.9840011300000000 | 1.0 |
| C27 | C | 0.9402227600000000 | 0.9620566600000000 | 0.9776661700000000 | 1.0 |
| C28 | C | 0.8561023700000000 | 0.9422947900000000 | 0.0418145800000000 | 1.0 |
| C29 | C | 0.8999731400000000 | 0.9308320800000000 | 0.9105529900000000 | 1.0 |
| C30 | C | 0.1980937600000000 | 0.0557816700000000 | 0.0439088300000000 | 1.0 |
| C31 | C | 0.1140062200000000 | 0.0383769800000000 | 0.9790622800000000 | 1.0 |
| C32 | C | 0.1060814000000000 | 0.9598223800000000 | 0.9825566600000000 | 1.0 |
| C33 | C | 0.1862616400000000 | 0.9452858800000000 | 0.0468090100000000 | 1.0 |
| C34 | C | 0.1546541800000000 | 0.0719850700000000 | 0.9131669800000000 | 1.0 |
| C35 | C | 0.3679597700000000 | 0.0527272700000000 | 0.0487201900000000 | 1.0 |
| C36 | C | 0.4481566800000000 | 0.0405002400000000 | 0.9839967900000000 | 1.0 |
| C37 | C | 0.4401705400000000 | 0.9621165800000000 | 0.9776814900000000 | 1.0 |
| C38 | C | 0.3561038600000000 | 0.9423993400000000 | 0.0418696300000000 | 1.0 |
| C39 | C | 0.3997574500000000 | 0.9309151900000000 | 0.9105769200000000 | 1.0 |
| C40 | C | 0.6981316000000000 | 0.0557030500000000 | 0.0439637100000000 | 1.0 |
| C41 | C | 0.6140400300000000 | 0.0383886100000000 | 0.9790894500000000 | 1.0 |
| C42 | C | 0.6060361700000000 | 0.9598365500000000 | 0.9825212200000000 | 1.0 |
| C43 | C | 0.6862492300000000 | 0.9452049900000000 | 0.0467412700000000 | 1.0 |
| C44 | C | 0.6548091500000000 | 0.0720073400000000 | 0.9132133000000000 | 1.0 |
| O45 | O | 0.8960864500000000 | 0.9936618700000000 | 0.0873001700000000 | 1.0 |
| O46 | O | 0.1581763100000000 | 0.0027840600000000 | 0.0874880700000000 | 1.0 |
| O47 | O | 0.3960693000000000 | 0.9938099700000000 | 0.0873150200000000 | 1.0 |
| O48 | O | 0.6581949500000000 | 0.0026596200000000 | 0.0874849600000000 | 1.0 |

##### cif ends

furand\_CH3\_3\_syn\_dir Energy: -291.20462175

##### cif starts

data\_furand\_CH3\_3\_syn\_dir

\_publ\_section\_comment

;  
Andrew Reynoso, Bohan Xu, and Vincent H. Crespi  
;

\_cell\_length\_a 10.4327486946

\_cell\_length\_b 20.0

\_cell\_length\_c 20.0

\_cell\_angle\_alpha 90.0

\_cell\_angle\_beta 90.0

\_cell\_angle\_gamma 90.0

\_symmetry\_space\_group\_name\_H-M 'P 1'

\_symmetry\_Int\_Tables\_number 1

\_symmetry\_cell\_setting triclinic



| loop_                  |   |                    |                    |                    |     |
|------------------------|---|--------------------|--------------------|--------------------|-----|
| _atom_site_label       |   |                    |                    |                    |     |
| _atom_site_type_symbol |   |                    |                    |                    |     |
| _atom_site_fract_x     |   |                    |                    |                    |     |
| _atom_site_fract_y     |   |                    |                    |                    |     |
| _atom_site_fract_z     |   |                    |                    |                    |     |
| _atom_site_occupancy   |   |                    |                    |                    |     |
| H1                     | H | 0.0395667400000000 | 0.0380720000000000 | 0.1000397600000000 | 1.0 |
| H2                     | H | 0.2388972400000000 | 0.0535107300000000 | 0.9159292100000000 | 1.0 |
| H3                     | H | 0.1552976800000000 | 0.9434069900000000 | 0.9194630800000000 | 1.0 |
| H4                     | H | 0.0204410600000000 | 0.8594127200000000 | 0.0041801000000000 | 1.0 |
| H5                     | H | 0.0715811600000000 | 0.0535011800000000 | 0.9159466800000000 | 1.0 |
| H6                     | H | 0.1552442800000000 | 0.1163160100000000 | 0.9603461400000000 | 1.0 |
| H7                     | H | 0.2709927500000000 | 0.0380897400000000 | 0.1000326700000000 | 1.0 |
| H8                     | H | 0.4052370400000000 | 0.1012670500000000 | 0.9355383800000000 | 1.0 |
| H9                     | H | 0.4052687500000000 | 0.9534787900000000 | 0.9189068800000000 | 1.0 |
| H10                    | H | 0.2901116200000000 | 0.8594173000000000 | 0.0042086100000000 | 1.0 |
| H11                    | H | 0.3218143500000000 | 0.1194170700000000 | 0.0099377300000000 | 1.0 |
| H12                    | H | 0.4886933000000000 | 0.1194326700000000 | 0.0099226300000000 | 1.0 |
| H13                    | H | 0.5395564600000000 | 0.0380795200000000 | 0.1000362800000000 | 1.0 |
| H14                    | H | 0.7389011200000000 | 0.0535227300000000 | 0.9159368100000000 | 1.0 |
| H15                    | H | 0.6552881900000000 | 0.9434113600000000 | 0.9194628100000000 | 1.0 |
| H16                    | H | 0.5204469500000000 | 0.8594143100000000 | 0.0041918500000000 | 1.0 |
| H17                    | H | 0.6552527700000000 | 0.1163223300000000 | 0.9603627700000000 | 1.0 |
| H18                    | H | 0.7709989600000000 | 0.0380831300000000 | 0.1000399800000000 | 1.0 |
| H19                    | H | 0.9052417000000000 | 0.1012814300000000 | 0.9355552200000000 | 1.0 |
| H20                    | H | 0.9052627100000000 | 0.9534851100000000 | 0.9189069100000000 | 1.0 |
| H21                    | H | 0.7901122100000000 | 0.8594181100000000 | 0.0042025300000000 | 1.0 |
| H22                    | H | 0.8218186700000000 | 0.1194169200000000 | 0.0099579400000000 | 1.0 |
| H23                    | H | 0.9886983800000000 | 0.1194318600000000 | 0.0099430500000000 | 1.0 |
| H24                    | H | 0.5715839500000000 | 0.0535144900000000 | 0.9159572300000000 | 1.0 |
| C25                    | C | 0.0319433600000000 | 0.0083134200000000 | 0.0539929500000000 | 1.0 |
| C26                    | C | 0.1552706600000000 | 0.0137924000000000 | 0.0065661400000000 | 1.0 |
| C27                    | C | 0.1552788100000000 | 0.9422823100000000 | 0.9744375100000000 | 1.0 |
| C28                    | C | 0.0282141000000000 | 0.9142034400000000 | 0.0033126500000000 | 1.0 |
| C29                    | C | 0.1552484600000000 | 0.0630814200000000 | 0.9475886800000000 | 1.0 |
| C30                    | C | 0.2786034700000000 | 0.0083221000000000 | 0.0539935800000000 | 1.0 |
| C31                    | C | 0.4052728300000000 | 0.0196217100000000 | 0.0142296200000000 | 1.0 |
| C32                    | C | 0.4052750900000000 | 0.9498811300000000 | 0.9737693800000000 | 1.0 |
| C33                    | C | 0.2823359900000000 | 0.9142067900000000 | 0.0033236600000000 | 1.0 |
| C34                    | C | 0.4052563500000000 | 0.0931510800000000 | 0.9896188200000000 | 1.0 |
| C35                    | C | 0.5319415200000000 | 0.0083184600000000 | 0.0539915700000000 | 1.0 |
| C36                    | C | 0.6552729000000000 | 0.0137943200000000 | 0.0065699900000000 | 1.0 |
| C37                    | C | 0.6552780400000000 | 0.9422855200000000 | 0.9744377700000000 | 1.0 |
| C38                    | C | 0.5282163400000000 | 0.9142048300000000 | 0.0033168500000000 | 1.0 |
| C39                    | C | 0.6552547600000000 | 0.0630898600000000 | 0.9475974500000000 | 1.0 |
| C40                    | C | 0.7786053500000000 | 0.0083191600000000 | 0.0539983400000000 | 1.0 |
| C41                    | C | 0.9052741500000000 | 0.0196213000000000 | 0.0142347400000000 | 1.0 |
| C42                    | C | 0.9052735500000000 | 0.9498837200000000 | 0.9737689200000000 | 1.0 |
| C43                    | C | 0.7823361700000000 | 0.9142075700000000 | 0.0033212500000000 | 1.0 |
| C44                    | C | 0.9052604900000000 | 0.0931542500000000 | 0.9896341800000000 | 1.0 |
| O45                    | O | 0.0305123400000000 | 0.9389296600000000 | 0.0707201900000000 | 1.0 |
| O46                    | O | 0.2800398400000000 | 0.9389437300000000 | 0.0707268500000000 | 1.0 |
| O47                    | O | 0.5305130500000000 | 0.9389365000000000 | 0.0707223800000000 | 1.0 |

O48 O 0.7800403400000000 0.9389387400000000 0.0707263000000000 1.0

##### cif ends

furán\_CH3\_3\_syn\_dir\_forbid Energy: -288.37878365

##### cif starts

data\_furan\_CH3\_3\_syn\_dir\_forbid

\_publ\_section\_comment

;  
Andrew Reynoso, Bohan Xu, and Vincent H. Crespi  
;

\_cell\_length\_a 9.4586954274

\_cell\_length\_b 20.0

\_cell\_length\_c 20.0

\_cell\_angle\_alpha 90.0

\_cell\_angle\_beta 90.0

\_cell\_angle\_gamma 90.0

\_symmetry\_space\_group\_name\_H-M 'P 1'

\_symmetry\_Int\_Tables\_number 1

\_symmetry\_cell\_setting triclinic

loop\_

\_atom\_site\_label

\_atom\_site\_type\_symbol

\_atom\_site\_fract\_x

\_atom\_site\_fract\_y

\_atom\_site\_fract\_z

\_atom\_site\_occupancy

|     |   |                    |                    |                    |     |
|-----|---|--------------------|--------------------|--------------------|-----|
| H1  | H | 0.8591880300000000 | 0.1189387700000000 | 0.0659359200000000 | 1.0 |
| H2  | H | 0.8863170800000000 | 0.9559028400000000 | 0.9365850900000000 | 1.0 |
| H3  | H | 0.9201053200000000 | 0.9190230800000000 | 0.0736094900000000 | 1.0 |
| H4  | H | 0.1848671800000000 | 0.0738130700000000 | 0.1001378600000000 | 1.0 |
| H5  | H | 0.1357019900000000 | 0.9626652000000000 | 0.9187796900000000 | 1.0 |
| H6  | H | 0.1297648700000000 | 0.8854592000000000 | 0.0314498500000000 | 1.0 |
| H7  | H | 0.4235227200000000 | 0.0715327300000000 | 0.0676935400000000 | 1.0 |
| H8  | H | 0.4293814500000000 | 0.9085683600000000 | 0.9298827600000000 | 1.0 |
| H9  | H | 0.3670621100000000 | 0.8718223500000000 | 0.0579207100000000 | 1.0 |
| H10 | H | 0.6253039000000000 | 0.1050617700000000 | 0.0329726100000000 | 1.0 |
| H11 | H | 0.6784032100000000 | 0.9097199600000000 | 0.9524991300000000 | 1.0 |
| H12 | H | 0.6751273300000000 | 0.9130780600000000 | 0.0920520000000000 | 1.0 |
| H13 | H | 0.2974478500000000 | 0.1227860000000000 | 0.9810265500000000 | 1.0 |
| H14 | H | 0.1321861900000000 | 0.1589937600000000 | 0.9970889300000000 | 1.0 |
| H15 | H | 0.1728681900000000 | 0.1300111100000000 | 0.9157818400000000 | 1.0 |
| H16 | H | 0.4042194000000000 | 0.0893741500000000 | 0.8915549500000000 | 1.0 |
| H17 | H | 0.2609688800000000 | 0.0340306400000000 | 0.9012352000000000 | 1.0 |
| H18 | H | 0.4143084800000000 | 0.0065644000000000 | 0.8621142800000000 | 1.0 |
| H19 | H | 0.9596452500000000 | 0.1534295200000000 | 0.9336763000000000 | 1.0 |
| H20 | H | 0.8011010700000000 | 0.1120835600000000 | 0.9186858400000000 | 1.0 |
| H21 | H | 0.9560692600000000 | 0.0863180800000000 | 0.8760444700000000 | 1.0 |
| H22 | H | 0.7722781600000000 | 0.0156578300000000 | 0.8863012900000000 | 1.0 |
| H23 | H | 0.6354850900000000 | 0.0734240300000000 | 0.8690109500000000 | 1.0 |
| H24 | H | 0.6070287200000000 | 0.9864684200000000 | 0.8612835800000000 | 1.0 |

|     |   |                    |                    |                    |     |
|-----|---|--------------------|--------------------|--------------------|-----|
| C25 | C | 0.8484802800000000 | 0.0702096100000000 | 0.0409575200000000 | 1.0 |
| C26 | C | 0.9479002800000000 | 0.0573831400000000 | 0.9831240600000000 | 1.0 |
| C27 | C | 0.9411407800000000 | 0.9790216900000000 | 0.9788950200000000 | 1.0 |
| C28 | C | 0.8685541400000000 | 0.9608598200000000 | 0.0479853500000000 | 1.0 |
| C29 | C | 0.9143873200000000 | 0.1038871500000000 | 0.9242684300000000 | 1.0 |
| C30 | C | 0.1974771300000000 | 0.0380835300000000 | 0.0588906500000000 | 1.0 |
| C31 | C | 0.1163378700000000 | 0.0532795900000000 | 0.9941124200000000 | 1.0 |
| C32 | C | 0.1079556400000000 | 0.9758370700000000 | 0.9703528500000000 | 1.0 |
| C33 | C | 0.1838040600000000 | 0.9338116100000000 | 0.0253929000000000 | 1.0 |
| C34 | C | 0.1851296300000000 | 0.1187410000000000 | 0.9689323800000000 | 1.0 |
| C35 | C | 0.3689976100000000 | 0.0300565800000000 | 0.0429629200000000 | 1.0 |
| C36 | C | 0.4394959800000000 | 0.0135115900000000 | 0.9694672400000000 | 1.0 |
| C37 | C | 0.4525400100000000 | 0.9361113700000000 | 0.9762047400000000 | 1.0 |
| C38 | C | 0.3530003000000000 | 0.9208483100000000 | 0.0339399400000000 | 1.0 |
| C39 | C | 0.3751971300000000 | 0.0375340000000000 | 0.9032576100000000 | 1.0 |
| C40 | C | 0.6812312100000000 | 0.0574457000000000 | 0.0252163900000000 | 1.0 |
| C41 | C | 0.6120577000000000 | 0.0177198100000000 | 0.9646700200000000 | 1.0 |
| C42 | C | 0.6197171100000000 | 0.9426943900000000 | 0.9866378400000000 | 1.0 |
| C43 | C | 0.6968787700000000 | 0.9507663700000000 | 0.0535490900000000 | 1.0 |
| C44 | C | 0.6593623000000000 | 0.0247415300000000 | 0.8917625400000000 | 1.0 |
| O45 | O | 0.8896481200000000 | 0.0198763400000000 | 0.0875624900000000 | 1.0 |
| O46 | O | 0.1531963200000000 | 0.9743070400000000 | 0.0826358400000000 | 1.0 |
| O47 | O | 0.3982337600000000 | 0.9706190200000000 | 0.0802652300000000 | 1.0 |
| O48 | O | 0.6455331300000000 | 0.0135355900000000 | 0.0788165000000000 | 1.0 |

##### cif ends

furand\_Cl\_23\_anti\_alt Energy: -214.19070046

##### cif starts

data\_furand\_Cl\_23\_anti\_alt

\_publ\_section\_comment

;  
Andrew Reynoso, Bohan Xu, and Vincent H. Crespi  
;

\_cell\_length\_a 9.4498909941

\_cell\_length\_b 20.0

\_cell\_length\_c 20.0

\_cell\_angle\_alpha 90.0

\_cell\_angle\_beta 90.0

\_cell\_angle\_gamma 90.0

\_symmetry\_space\_group\_name\_H-M 'P 1'

\_symmetry\_Int\_Tables\_number 1

\_symmetry\_cell\_setting triclinic

loop\_

\_atom\_site\_label

\_atom\_site\_type\_symbol

\_atom\_site\_fract\_x

\_atom\_site\_fract\_y

\_atom\_site\_fract\_z

\_atom\_site\_occupancy

H1 H 0.5237801000000000 0.9005000800000000 0.9423097400000000 1.0

|      |    |                    |                    |                    |     |
|------|----|--------------------|--------------------|--------------------|-----|
| H2   | H  | 0.5134842600000000 | 0.9397351200000000 | 0.0761209300000000 | 1.0 |
| H3   | H  | 0.7737771400000000 | 0.0994989200000000 | 0.0576898300000000 | 1.0 |
| H4   | H  | 0.7634848900000000 | 0.0602641700000000 | 0.9238784700000000 | 1.0 |
| H5   | H  | 0.0237790600000000 | 0.9005005800000000 | 0.9423111200000000 | 1.0 |
| H6   | H  | 0.0134827600000000 | 0.9397357700000000 | 0.0761221800000000 | 1.0 |
| H7   | H  | 0.2737822000000000 | 0.0995003600000000 | 0.0576890500000000 | 1.0 |
| H8   | H  | 0.2634818500000000 | 0.0602646900000000 | 0.9238783400000000 | 1.0 |
| C9   | C  | 0.5505228600000000 | 0.9474698000000000 | 0.9669059400000000 | 1.0 |
| C10  | C  | 0.4679541200000000 | 0.9616809800000000 | 0.0308771900000000 | 1.0 |
| C11  | C  | 0.4645077300000000 | 0.0398523900000000 | 0.0322401800000000 | 1.0 |
| C12  | C  | 0.5549297300000000 | 0.0556098000000000 | 0.9682645100000000 | 1.0 |
| C13  | C  | 0.8005214400000000 | 0.0525293800000000 | 0.0330936900000000 | 1.0 |
| C14  | C  | 0.7179546000000000 | 0.0383185200000000 | 0.9691222200000000 | 1.0 |
| C15  | C  | 0.7145072900000000 | 0.9601471200000000 | 0.9677587700000000 | 1.0 |
| C16  | C  | 0.8049293500000000 | 0.9443893500000000 | 0.0317345400000000 | 1.0 |
| C17  | C  | 0.0505223100000000 | 0.9474704100000000 | 0.9669070400000000 | 1.0 |
| C18  | C  | 0.9679536500000000 | 0.9616812900000000 | 0.0308780800000000 | 1.0 |
| C19  | C  | 0.9645064400000000 | 0.0398527100000000 | 0.0322412500000000 | 1.0 |
| C20  | C  | 0.0549286700000000 | 0.0556104700000000 | 0.9682657900000000 | 1.0 |
| C21  | C  | 0.3005233300000000 | 0.0525302800000000 | 0.0330931900000000 | 1.0 |
| C22  | C  | 0.2179537400000000 | 0.0383190900000000 | 0.9691225800000000 | 1.0 |
| C23  | C  | 0.2145064000000000 | 0.9601476400000000 | 0.9677596200000000 | 1.0 |
| C24  | C  | 0.3049292900000000 | 0.9443901900000000 | 0.0317351500000000 | 1.0 |
| O25  | O  | 0.5063823600000000 | 0.0034898000000000 | 0.9245651300000000 | 1.0 |
| O26  | O  | 0.7563802200000000 | 0.9965084100000000 | 0.0754340700000000 | 1.0 |
| O27  | O  | 0.0063811000000000 | 0.0034905600000000 | 0.9245666000000000 | 1.0 |
| O28  | O  | 0.2563828200000000 | 0.9965104500000000 | 0.0754343800000000 | 1.0 |
| Cl29 | Cl | 0.5223273200000000 | 0.0805698100000000 | 0.1073961600000000 | 1.0 |
| Cl30 | Cl | 0.5211153200000000 | 0.1352738800000000 | 0.9340549100000000 | 1.0 |
| Cl31 | Cl | 0.7723273100000000 | 0.9194295500000000 | 0.8926029900000000 | 1.0 |
| Cl32 | Cl | 0.7711151600000000 | 0.8647246800000000 | 0.0659429200000000 | 1.0 |
| Cl33 | Cl | 0.0223253900000000 | 0.0805710400000000 | 0.1073967600000000 | 1.0 |
| Cl34 | Cl | 0.0211132200000000 | 0.1352748000000000 | 0.9340570200000000 | 1.0 |
| Cl35 | Cl | 0.2723252200000000 | 0.9194293900000000 | 0.8926041400000000 | 1.0 |
| Cl36 | Cl | 0.2711133400000000 | 0.8647265100000000 | 0.0659455000000000 | 1.0 |

##### cif ends

furand\_Cl\_23\_anti\_alt\_forbid Energy: -214.93212615

##### cif starts

data\_furand\_Cl\_23\_anti\_alt\_forbid

\_publ\_section\_comment

;  
Andrew Reynoso, Bohan Xu, and Vincent H. Crespi  
;

\_cell\_length\_a 10.2613971347

\_cell\_length\_b 20.0

\_cell\_length\_c 20.0

\_cell\_angle\_alpha 90.0

\_cell\_angle\_beta 90.0

\_cell\_angle\_gamma 90.0

\_symmetry\_space\_group\_name\_H-M 'P 1'

\_symmetry\_Int\_Tables\_number 1  
\_symmetry\_cell\_setting triclinic

loop\_  
\_atom\_site\_label  
\_atom\_site\_type\_symbol  
\_atom\_site\_fract\_x  
\_atom\_site\_fract\_y  
\_atom\_site\_fract\_z  
\_atom\_site\_occupancy

|      |    |                    |                    |                    |     |
|------|----|--------------------|--------------------|--------------------|-----|
| H1   | H  | 0.9542244800000000 | 0.9318273300000000 | 0.0519775600000000 | 1.0 |
| H2   | H  | 0.0698659200000000 | 0.8942932400000000 | 0.9307272800000000 | 1.0 |
| H3   | H  | 0.3307201700000000 | 0.0592317000000000 | 0.9134075000000000 | 1.0 |
| H4   | H  | 0.2150690400000000 | 0.0967946100000000 | 0.0346656700000000 | 1.0 |
| H5   | H  | 0.4544208200000000 | 0.9317935500000000 | 0.0522334200000000 | 1.0 |
| H6   | H  | 0.5697832100000000 | 0.8942753600000000 | 0.9309179400000000 | 1.0 |
| H7   | H  | 0.8305935700000000 | 0.0593566000000000 | 0.9132470100000000 | 1.0 |
| H8   | H  | 0.7151817100000000 | 0.0969055100000000 | 0.0345760200000000 | 1.0 |
| C9   | C  | 0.0807237000000000 | 0.0518137300000000 | 0.9606679100000000 | 1.0 |
| C10  | C  | 0.9567268000000000 | 0.0352855400000000 | 0.0024301800000000 | 1.0 |
| C11  | C  | 0.9583202600000000 | 0.9565333000000000 | 0.0031667400000000 | 1.0 |
| C12  | C  | 0.0789052000000000 | 0.9394083000000000 | 0.9612790900000000 | 1.0 |
| C13  | C  | 0.2060690100000000 | 0.0516859100000000 | 0.0041058900000000 | 1.0 |
| C14  | C  | 0.3266718500000000 | 0.0345716300000000 | 0.9622422300000000 | 1.0 |
| C15  | C  | 0.3283155600000000 | 0.9558140200000000 | 0.9630181800000000 | 1.0 |
| C16  | C  | 0.2042672900000000 | 0.9392762200000000 | 0.0047196400000000 | 1.0 |
| C17  | C  | 0.5805761700000000 | 0.0518158500000000 | 0.9607806400000000 | 1.0 |
| C18  | C  | 0.4567030300000000 | 0.0352341500000000 | 0.0026291000000000 | 1.0 |
| C19  | C  | 0.4583712200000000 | 0.9564800100000000 | 0.0034049500000000 | 1.0 |
| C20  | C  | 0.5788814100000000 | 0.9394048800000000 | 0.9614376100000000 | 1.0 |
| C21  | C  | 0.7061250800000000 | 0.0517712400000000 | 0.0040535600000000 | 1.0 |
| C22  | C  | 0.8266300700000000 | 0.0346794400000000 | 0.9620781500000000 | 1.0 |
| C23  | C  | 0.8282567600000000 | 0.9559229200000000 | 0.9628227000000000 | 1.0 |
| C24  | C  | 0.7044257400000000 | 0.9393564400000000 | 0.0047003500000000 | 1.0 |
| O25  | O  | 0.0889864300000000 | 0.9961586500000000 | 0.9158540700000000 | 1.0 |
| O26  | O  | 0.1959829000000000 | 0.9949315300000000 | 0.0495357700000000 | 1.0 |
| O27  | O  | 0.5887163300000000 | 0.9961458900000000 | 0.9159769800000000 | 1.0 |
| O28  | O  | 0.6963024600000000 | 0.9950277200000000 | 0.0495090300000000 | 1.0 |
| Cl29 | Cl | 0.0703419600000000 | 0.1263065700000000 | 0.9133699400000000 | 1.0 |
| Cl30 | Cl | 0.9543250400000000 | 0.0800656400000000 | 0.0790126100000000 | 1.0 |
| Cl31 | Cl | 0.3309215000000000 | 0.9109795500000000 | 0.8864645300000000 | 1.0 |
| Cl32 | Cl | 0.2146111900000000 | 0.8647633300000000 | 0.0519856600000000 | 1.0 |
| Cl33 | Cl | 0.5698161200000000 | 0.1262996400000000 | 0.9134915100000000 | 1.0 |
| Cl34 | Cl | 0.4542338900000000 | 0.0800171500000000 | 0.0792084500000000 | 1.0 |
| Cl35 | Cl | 0.8306462300000000 | 0.9111486600000000 | 0.8862395900000000 | 1.0 |
| Cl36 | Cl | 0.7151867400000000 | 0.8648764100000000 | 0.0519988400000000 | 1.0 |

##### cif ends

furandir Energy: -214.19077278

##### cif starts

furandir

\_publ\_section\_comment

;

;

```
_cell_length_a  9.4501796935
_cell_length_b  20.0
_cell_length_c  20.0
_cell_angle_alpha  90.0
_cell_angle_beta  90.0
_cell_angle_gamma  90.0
```

```
_symmetry_space_group_name_H-M  'P 1'
_symmetry_Int_Tables_number 1
_symmetry_cell_setting triclinic
```

```
loop_
_atom_site_label
_atom_site_type_symbol
_atom_site_fract_x
_atom_site_fract_y
_atom_site_fract_z
_atom_site_occupancy
H1  H  0.5237557700000000  0.9006023000000000  0.9421464300000000  1.0
H2  H  0.5134847700000000  0.9396069000000000  0.0760268400000000  1.0
H3  H  0.7737502000000000  0.0993943800000000  0.0578608800000000  1.0
H4  H  0.7634859100000000  0.0603972300000000  0.9239775400000000  1.0
H5  H  0.0237444500000000  0.9006059400000000  0.9421404800000000  1.0
H6  H  0.0134884200000000  0.9396063000000000  0.0760227800000000  1.0
H7  H  0.2737499300000000  0.0993972500000000  0.0578522100000000  1.0
H8  H  0.2634871600000000  0.0603896500000000  0.9239728500000000  1.0
C9  C  0.5505204000000000  0.9475310400000000  0.9668205200000000  1.0
C10 C  0.4679602800000000  0.9616383900000000  0.0308229500000000  1.0
C11 C  0.4645182500000000  0.0397958400000000  0.0323158700000000  1.0
C12 C  0.5549474000000000  0.0556609700000000  0.9683617500000000  1.0
C13 C  0.8005182500000000  0.0524683900000000  0.0331825700000000  1.0
C14 C  0.7179590800000000  0.0383631700000000  0.9691796100000000  1.0
C15 C  0.7145201200000000  0.9602059400000000  0.9676835300000000  1.0
C16 C  0.8049529000000000  0.9443387500000000  0.0316362900000000  1.0
C17 C  0.0505174500000000  0.9475321500000000  0.9668172700000000  1.0
C18 C  0.9679617200000000  0.9616392600000000  0.0308201300000000  1.0
C19 C  0.9645203700000000  0.0397966000000000  0.0323153500000000  1.0
C20 C  0.0549530500000000  0.0556617200000000  0.9683612700000000  1.0
C21 C  0.3005194600000000  0.0524684900000000  0.0331795200000000  1.0
C22 C  0.2179627400000000  0.0383590800000000  0.9691770700000000  1.0
C23 C  0.2145183300000000  0.9602015200000000  0.9676851100000000  1.0
C24 C  0.3049474300000000  0.9443386600000000  0.0316406200000000  1.0
O25 O  0.5064067600000000  0.0036223700000000  0.9245683400000000  1.0
O26 O  0.7564098900000000  0.9963744300000000  0.0754325000000000  1.0
O27 O  0.0064097700000000  0.0036255300000000  0.9245662800000000  1.0
O28 O  0.2564065500000000  0.9963777900000000  0.0754327600000000  1.0
Cl29 Cl  0.5222852000000000  0.0803953200000000  0.1075449300000000  1.0
Cl30 Cl  0.5211093100000000  0.1353975100000000  0.9343047800000000  1.0
Cl31 Cl  0.7722845700000000  0.9196124900000000  0.8924506400000000  1.0
Cl32 Cl  0.7711243700000000  0.8645983000000000  0.0656860000000000  1.0
Cl33 Cl  0.0222888200000000  0.0803953400000000  0.1075445100000000  1.0
Cl34 Cl  0.0211286600000000  0.1354017800000000  0.9343093200000000  1.0
```

Cl35 Cl 0.272291340000000 0.919597510000000 0.892459740000000 1.0  
Cl36 Cl 0.271113940000000 0.864602720000000 0.065699750000000 1.0

##### cif ends

furandirforbid Energy: -211.9435042

##### cif starts

data\_furandirforbid

\_publ\_section\_comment

;  
Andrew Reynoso, Bohan Xu, and Vincent H. Crespi  
;

\_cell\_length\_a 10.5045001497

\_cell\_length\_b 20.0

\_cell\_length\_c 20.0

\_cell\_angle\_alpha 90.0

\_cell\_angle\_beta 90.0

\_cell\_angle\_gamma 90.0

\_symmetry\_space\_group\_name\_H-M 'P 1'

\_symmetry\_Int\_Tables\_number 1

\_symmetry\_cell\_setting triclinic

loop\_

\_atom\_site\_label

\_atom\_site\_type\_symbol

\_atom\_site\_fract\_x

\_atom\_site\_fract\_y

\_atom\_site\_fract\_z

\_atom\_site\_occupancy

|     |   |                   |                   |                   |     |
|-----|---|-------------------|-------------------|-------------------|-----|
| H1  | H | 0.007145630000000 | 0.100316480000000 | 0.939851160000000 | 1.0 |
| H2  | H | 0.125542710000000 | 0.062413950000000 | 0.061681690000000 | 1.0 |
| H3  | H | 0.373818550000000 | 0.098672100000000 | 0.047977810000000 | 1.0 |
| H4  | H | 0.255813330000000 | 0.064397120000000 | 0.924956470000000 | 1.0 |
| H5  | H | 0.506611010000000 | 0.100048720000000 | 0.939388230000000 | 1.0 |
| H6  | H | 0.624833660000000 | 0.063137140000000 | 0.061639160000000 | 1.0 |
| H7  | H | 0.874671470000000 | 0.098418550000000 | 0.048554140000000 | 1.0 |
| H8  | H | 0.756174190000000 | 0.065247460000000 | 0.925319400000000 | 1.0 |
| C9  | C | 0.002341250000000 | 0.055209910000000 | 0.971186420000000 | 1.0 |
| C10 | C | 0.124930970000000 | 0.039844410000000 | 0.011726310000000 | 1.0 |
| C11 | C | 0.124468310000000 | 0.961466550000000 | 0.012600080000000 | 1.0 |
| C12 | C | 0.003885030000000 | 0.941918260000000 | 0.969927250000000 | 1.0 |
| C13 | C | 0.378757200000000 | 0.054526550000000 | 0.015309750000000 | 1.0 |
| C14 | C | 0.256278670000000 | 0.040375180000000 | 0.974234500000000 | 1.0 |
| C15 | C | 0.256703110000000 | 0.962061780000000 | 0.971076750000000 | 1.0 |
| C16 | C | 0.377230970000000 | 0.941247010000000 | 0.013189830000000 | 1.0 |
| C17 | C | 0.502123910000000 | 0.055165640000000 | 0.971050620000000 | 1.0 |
| C18 | C | 0.624779310000000 | 0.040330930000000 | 0.011788070000000 | 1.0 |
| C19 | C | 0.624695660000000 | 0.961981320000000 | 0.012951650000000 | 1.0 |
| C20 | C | 0.504210290000000 | 0.941872440000000 | 0.970632820000000 | 1.0 |
| C21 | C | 0.879065450000000 | 0.054513140000000 | 0.015541650000000 | 1.0 |
| C22 | C | 0.756327790000000 | 0.040917080000000 | 0.974441450000000 | 1.0 |
| C23 | C | 0.756436360000000 | 0.962641710000000 | 0.970869630000000 | 1.0 |

|      |    |                    |                    |                    |     |
|------|----|--------------------|--------------------|--------------------|-----|
| C24  | C  | 0.8769731800000000 | 0.9412608000000000 | 0.0125379800000000 | 1.0 |
| O25  | O  | 0.9942008500000000 | 0.9985476300000000 | 0.9257495500000000 | 1.0 |
| O26  | O  | 0.3868237100000000 | 0.9965323600000000 | 0.0590439400000000 | 1.0 |
| O27  | O  | 0.4942181000000000 | 0.9981616300000000 | 0.9260259800000000 | 1.0 |
| O28  | O  | 0.8870325100000000 | 0.9961761200000000 | 0.0588160400000000 | 1.0 |
| Cl29 | Cl | 0.1238589000000000 | 0.9292694200000000 | 0.0948914100000000 | 1.0 |
| Cl30 | Cl | 0.0170670400000000 | 0.8658461800000000 | 0.9258444200000000 | 1.0 |
| Cl31 | Cl | 0.2573593500000000 | 0.9322636500000000 | 0.8878848100000000 | 1.0 |
| Cl32 | Cl | 0.3639678600000000 | 0.8638810700000000 | 0.0549522200000000 | 1.0 |
| Cl33 | Cl | 0.6251540600000000 | 0.9302926100000000 | 0.0954454700000000 | 1.0 |
| Cl34 | Cl | 0.5184880000000000 | 0.8653886400000000 | 0.9273309900000000 | 1.0 |
| Cl35 | Cl | 0.7559440300000000 | 0.9335393800000000 | 0.8874212200000000 | 1.0 |
| Cl36 | Cl | 0.8627934100000000 | 0.8635161100000000 | 0.0535485700000000 | 1.0 |

##### cif ends

  furan\_Cl\_23\_syn\_alt   Energy: -215.17233386

##### cif starts

data\_furan\_Cl\_23\_syn\_alt

\_publ\_section\_comment

;  
Andrew Reynoso, Bohan Xu, and Vincent H. Crespi  
;

\_cell\_length\_a 10.3746949227

\_cell\_length\_b 20.0

\_cell\_length\_c 20.0

\_cell\_angle\_alpha 90.0

\_cell\_angle\_beta 90.0

\_cell\_angle\_gamma 90.0

\_symmetry\_space\_group\_name\_H-M 'P 1'

\_symmetry\_Int\_Tables\_number 1

\_symmetry\_cell\_setting triclinic

loop\_

\_atom\_site\_label

\_atom\_site\_type\_symbol

\_atom\_site\_fract\_x

\_atom\_site\_fract\_y

\_atom\_site\_fract\_z

\_atom\_site\_occupancy

|    |   |                    |                    |                    |     |
|----|---|--------------------|--------------------|--------------------|-----|
| H1 | H | 0.4859396300000000 | 0.8987335600000000 | 0.0463663600000000 | 1.0 |
|----|---|--------------------|--------------------|--------------------|-----|

|    |   |                    |                    |                    |     |
|----|---|--------------------|--------------------|--------------------|-----|
| H2 | H | 0.6106542200000000 | 0.9379966900000000 | 0.9288277700000000 | 1.0 |
|----|---|--------------------|--------------------|--------------------|-----|

|    |   |                    |                    |                    |     |
|----|---|--------------------|--------------------|--------------------|-----|
| H3 | H | 0.7359380200000000 | 0.1009216000000000 | 0.0471121400000000 | 1.0 |
|----|---|--------------------|--------------------|--------------------|-----|

|    |   |                    |                    |                    |     |
|----|---|--------------------|--------------------|--------------------|-----|
| H4 | H | 0.8606625100000000 | 0.0625360600000000 | 0.9292950600000000 | 1.0 |
|----|---|--------------------|--------------------|--------------------|-----|

|    |   |                    |                    |                    |     |
|----|---|--------------------|--------------------|--------------------|-----|
| H5 | H | 0.9859401000000000 | 0.8987316100000000 | 0.0463626500000000 | 1.0 |
|----|---|--------------------|--------------------|--------------------|-----|

|    |   |                    |                    |                    |     |
|----|---|--------------------|--------------------|--------------------|-----|
| H6 | H | 0.1106531500000000 | 0.9379995700000000 | 0.9288249500000000 | 1.0 |
|----|---|--------------------|--------------------|--------------------|-----|

|    |   |                    |                    |                    |     |
|----|---|--------------------|--------------------|--------------------|-----|
| H7 | H | 0.2359376100000000 | 0.1009211400000000 | 0.0471121000000000 | 1.0 |
|----|---|--------------------|--------------------|--------------------|-----|

|    |   |                    |                    |                    |     |
|----|---|--------------------|--------------------|--------------------|-----|
| H8 | H | 0.3606610500000000 | 0.0625351100000000 | 0.9292935500000000 | 1.0 |
|----|---|--------------------|--------------------|--------------------|-----|

|    |   |                    |                    |                    |     |
|----|---|--------------------|--------------------|--------------------|-----|
| C9 | C | 0.4870368400000000 | 0.9465497400000000 | 0.0198654100000000 | 1.0 |
|----|---|--------------------|--------------------|--------------------|-----|

|     |   |                    |                    |                    |     |
|-----|---|--------------------|--------------------|--------------------|-----|
| C10 | C | 0.6103264700000000 | 0.9606448600000000 | 0.9785466700000000 | 1.0 |
|-----|---|--------------------|--------------------|--------------------|-----|

|     |   |                    |                    |                    |     |
|-----|---|--------------------|--------------------|--------------------|-----|
| C11 | C | 0.6119873700000000 | 0.0391207800000000 | 0.9789265300000000 | 1.0 |
|-----|---|--------------------|--------------------|--------------------|-----|

|     |   |                    |                    |                    |     |
|-----|---|--------------------|--------------------|--------------------|-----|
| C12 | C | 0.4849795300000000 | 0.0539800100000000 | 0.0200219900000000 | 1.0 |
|-----|---|--------------------|--------------------|--------------------|-----|



|      |    |                    |                    |                    |     |
|------|----|--------------------|--------------------|--------------------|-----|
| C13  | C  | 0.7370370200000000 | 0.0533000600000000 | 0.0202620900000000 | 1.0 |
| C14  | C  | 0.8603284700000000 | 0.0395150000000000 | 0.9788426900000000 | 1.0 |
| C15  | C  | 0.8619872700000000 | 0.9610374300000000 | 0.9786335200000000 | 1.0 |
| C16  | C  | 0.7349788600000000 | 0.9458720500000000 | 0.0196151700000000 | 1.0 |
| C17  | C  | 0.9870366000000000 | 0.9465486400000000 | 0.0198632600000000 | 1.0 |
| C18  | C  | 0.1103263600000000 | 0.9606455200000000 | 0.9785448700000000 | 1.0 |
| C19  | C  | 0.1119866000000000 | 0.0391215900000000 | 0.9789268300000000 | 1.0 |
| C20  | C  | 0.9849798500000000 | 0.0539788200000000 | 0.0200238300000000 | 1.0 |
| C21  | C  | 0.2370370700000000 | 0.0532999700000000 | 0.0202615800000000 | 1.0 |
| C22  | C  | 0.3603281500000000 | 0.0395148800000000 | 0.9788415700000000 | 1.0 |
| C23  | C  | 0.3619878200000000 | 0.9610371200000000 | 0.9786339200000000 | 1.0 |
| C24  | C  | 0.2349786900000000 | 0.9458720400000000 | 0.0196137300000000 | 1.0 |
| O25  | O  | 0.4860551700000000 | 0.0007143600000000 | 0.0675329400000000 | 1.0 |
| O26  | O  | 0.7360607400000000 | 0.9987771400000000 | 0.0675232300000000 | 1.0 |
| O27  | O  | 0.9860557600000000 | 0.0007116900000000 | 0.0675328100000000 | 1.0 |
| O28  | O  | 0.2360601500000000 | 0.9987769000000000 | 0.0675225900000000 | 1.0 |
| Cl29 | Cl | 0.6120115500000000 | 0.0795951300000000 | 0.8996818000000000 | 1.0 |
| Cl30 | Cl | 0.4860073600000000 | 0.1323361300000000 | 0.0604252800000000 | 1.0 |
| Cl31 | Cl | 0.8620024900000000 | 0.9211572800000000 | 0.8990894300000000 | 1.0 |
| Cl32 | Cl | 0.7360129900000000 | 0.8672170000000000 | 0.0594325800000000 | 1.0 |
| Cl33 | Cl | 0.1120076100000000 | 0.0795981000000000 | 0.8996829600000000 | 1.0 |
| Cl34 | Cl | 0.9860086400000000 | 0.1323328500000000 | 0.0604310200000000 | 1.0 |
| Cl35 | Cl | 0.3620039000000000 | 0.9211531500000000 | 0.8990916900000000 | 1.0 |
| Cl36 | Cl | 0.2360143600000000 | 0.8672164000000000 | 0.0594304300000000 | 1.0 |

##### cif ends

furan\_Cl\_23\_syn\_alt\_forbid Energy: -212.09580831

##### cif starts

data\_furan\_Cl\_23\_syn\_alt\_forbid

\_publ\_section\_comment

;  
Andrew Reynoso, Bohan Xu, and Vincent H. Crespi  
;

\_cell\_length\_a 9.6601690909

\_cell\_length\_b 20.0

\_cell\_length\_c 20.0

\_cell\_angle\_alpha 90.0

\_cell\_angle\_beta 90.0

\_cell\_angle\_gamma 90.0

\_symmetry\_space\_group\_name\_H-M 'P 1'

\_symmetry\_Int\_Tables\_number 1

\_symmetry\_cell\_setting triclinic

loop\_

\_atom\_site\_label

\_atom\_site\_type\_symbol

\_atom\_site\_fract\_x

\_atom\_site\_fract\_y

\_atom\_site\_fract\_z

\_atom\_site\_occupancy

H1 H 0.000901820000000 0.095716460000000 0.060422030000000 1.0

|      |    |                   |                   |                   |     |
|------|----|-------------------|-------------------|-------------------|-----|
| H2   | H  | 0.000071460000000 | 0.059951560000000 | 0.924943370000000 | 1.0 |
| H3   | H  | 0.252495230000000 | 0.931642590000000 | 0.928246310000000 | 1.0 |
| H4   | H  | 0.251817710000000 | 0.902926430000000 | 0.065403040000000 | 1.0 |
| H5   | H  | 0.500889430000000 | 0.095587000000000 | 0.060571360000000 | 1.0 |
| H6   | H  | 0.500172140000000 | 0.060027170000000 | 0.925027180000000 | 1.0 |
| H7   | H  | 0.752605940000000 | 0.931610500000000 | 0.928212170000000 | 1.0 |
| H8   | H  | 0.751734320000000 | 0.902801980000000 | 0.065331960000000 | 1.0 |
| C9   | C  | 0.037188970000000 | 0.051491300000000 | 0.033691760000000 | 1.0 |
| C10  | C  | 0.958271680000000 | 0.035666160000000 | 0.969393050000000 | 1.0 |
| C11  | C  | 0.958984720000000 | 0.957413630000000 | 0.969671360000000 | 1.0 |
| C12  | C  | 0.046872170000000 | 0.941016030000000 | 0.033816160000000 | 1.0 |
| C13  | C  | 0.205813490000000 | 0.056037450000000 | 0.030829980000000 | 1.0 |
| C14  | C  | 0.293695820000000 | 0.036338160000000 | 0.967634480000000 | 1.0 |
| C15  | C  | 0.294375910000000 | 0.958179510000000 | 0.971371060000000 | 1.0 |
| C16  | C  | 0.215514900000000 | 0.945705820000000 | 0.036421730000000 | 1.0 |
| C17  | C  | 0.537152690000000 | 0.051403370000000 | 0.033765560000000 | 1.0 |
| C18  | C  | 0.458276260000000 | 0.035688560000000 | 0.969427910000000 | 1.0 |
| C19  | C  | 0.458960440000000 | 0.957438000000000 | 0.969621240000000 | 1.0 |
| C20  | C  | 0.546846780000000 | 0.940932210000000 | 0.033733740000000 | 1.0 |
| C21  | C  | 0.705791940000000 | 0.055946120000000 | 0.030886800000000 | 1.0 |
| C22  | C  | 0.793672940000000 | 0.036295550000000 | 0.967655240000000 | 1.0 |
| C23  | C  | 0.794397290000000 | 0.958135300000000 | 0.971366430000000 | 1.0 |
| C24  | C  | 0.715473970000000 | 0.945608200000000 | 0.036381440000000 | 1.0 |
| O25  | O  | 0.007746210000000 | 0.994640470000000 | 0.075877940000000 | 1.0 |
| O26  | O  | 0.244963220000000 | 0.004665180000000 | 0.075608220000000 | 1.0 |
| O27  | O  | 0.507704070000000 | 0.994491890000000 | 0.075871120000000 | 1.0 |
| O28  | O  | 0.744929940000000 | 0.004532050000000 | 0.075620790000000 | 1.0 |
| Cl29 | Cl | 0.012654290000000 | 0.914155040000000 | 0.896048340000000 | 1.0 |
| Cl30 | Cl | 0.000592280000000 | 0.862825180000000 | 0.069875340000000 | 1.0 |
| Cl31 | Cl | 0.252111080000000 | 0.135996160000000 | 0.062777940000000 | 1.0 |
| Cl32 | Cl | 0.240088520000000 | 0.075735200000000 | 0.891870750000000 | 1.0 |
| Cl33 | Cl | 0.512561000000000 | 0.914283290000000 | 0.895930250000000 | 1.0 |
| Cl34 | Cl | 0.500521390000000 | 0.862677030000000 | 0.069648650000000 | 1.0 |
| Cl35 | Cl | 0.752068950000000 | 0.135877260000000 | 0.062904300000000 | 1.0 |
| Cl36 | Cl | 0.740011180000000 | 0.075719720000000 | 0.891912540000000 | 1.0 |

##### cif ends

furandir Energy: -211.03988108

##### cif starts

data\_furandir

\_publ\_section\_comment

;  
Andrew Reynoso, Bohan Xu, and Vincent H. Crespi  
;

\_cell\_length\_a 10.5051580555

\_cell\_length\_b 20.0

\_cell\_length\_c 20.0

\_cell\_angle\_alpha 90.0

\_cell\_angle\_beta 90.0

\_cell\_angle\_gamma 90.0

\_symmetry\_space\_group\_name\_H-M 'P 1'

\_symmetry\_Int\_Tables\_number 1  
\_symmetry\_cell\_setting triclinic

loop\_  
\_atom\_site\_label  
\_atom\_site\_type\_symbol  
\_atom\_site\_fract\_x  
\_atom\_site\_fract\_y  
\_atom\_site\_fract\_z  
\_atom\_site\_occupancy

|      |    |                    |                    |                    |     |
|------|----|--------------------|--------------------|--------------------|-----|
| H1   | H  | 0.4615753100000000 | 0.0918939700000000 | 0.0547598600000000 | 1.0 |
| H2   | H  | 0.5876940400000000 | 0.0699241100000000 | 0.9322073200000000 | 1.0 |
| H3   | H  | 0.7137898600000000 | 0.0918889600000000 | 0.0547743100000000 | 1.0 |
| H4   | H  | 0.8153466500000000 | 0.0600311200000000 | 0.9224767300000000 | 1.0 |
| H5   | H  | 0.9753660700000000 | 0.1172254300000000 | 0.0107962600000000 | 1.0 |
| H6   | H  | 0.0877049200000000 | 0.0290706800000000 | 0.9151986300000000 | 1.0 |
| H7   | H  | 0.2000440700000000 | 0.1172257100000000 | 0.0107933500000000 | 1.0 |
| H8   | H  | 0.3600288200000000 | 0.0600152100000000 | 0.9224659300000000 | 1.0 |
| C9   | C  | 0.5876861900000000 | 0.0408322500000000 | 0.9787137400000000 | 1.0 |
| C10  | C  | 0.5876910100000000 | 0.9631441700000000 | 0.9659617500000000 | 1.0 |
| C11  | C  | 0.4600531600000000 | 0.9419195400000000 | 0.0052330000000000 | 1.0 |
| C12  | C  | 0.4629877800000000 | 0.0493223100000000 | 0.0202385100000000 | 1.0 |
| C13  | C  | 0.7123752600000000 | 0.0493227900000000 | 0.0202469300000000 | 1.0 |
| C14  | C  | 0.8332552000000000 | 0.0417406200000000 | 0.9732689300000000 | 1.0 |
| C15  | C  | 0.8445094600000000 | 0.9655691800000000 | 0.9765675800000000 | 1.0 |
| C16  | C  | 0.7153279600000000 | 0.9419232500000000 | 0.0052248100000000 | 1.0 |
| C17  | C  | 0.9642649500000000 | 0.0632402800000000 | 0.0026347100000000 | 1.0 |
| C18  | C  | 0.0876976600000000 | 0.0300352500000000 | 0.9698757000000000 | 1.0 |
| C19  | C  | 0.0876985300000000 | 0.9563928900000000 | 0.0059592800000000 | 1.0 |
| C20  | C  | 0.9593373200000000 | 0.9634048000000000 | 0.0427601300000000 | 1.0 |
| C21  | C  | 0.2111237000000000 | 0.0632387800000000 | 0.0026329600000000 | 1.0 |
| C22  | C  | 0.3421195800000000 | 0.0417319600000000 | 0.9732601600000000 | 1.0 |
| C23  | C  | 0.3308677300000000 | 0.9655573400000000 | 0.9765713000000000 | 1.0 |
| C24  | C  | 0.2160629200000000 | 0.9634030700000000 | 0.0427567700000000 | 1.0 |
| O25  | O  | 0.9572587300000000 | 0.0300868200000000 | 0.0660065200000000 | 1.0 |
| O26  | O  | 0.7116723300000000 | 0.9880922800000000 | 0.0603043600000000 | 1.0 |
| O27  | O  | 0.4636837500000000 | 0.9880991800000000 | 0.0603040000000000 | 1.0 |
| O28  | O  | 0.2181467300000000 | 0.0300871500000000 | 0.0660057200000000 | 1.0 |
| Cl29 | Cl | 0.5876981900000000 | 0.9387677500000000 | 0.8809888800000000 | 1.0 |
| Cl30 | Cl | 0.4475625300000000 | 0.8565717800000000 | 0.0238798300000000 | 1.0 |
| Cl31 | Cl | 0.2395431800000000 | 0.9122774300000000 | 0.1119561100000000 | 1.0 |
| Cl32 | Cl | 0.2906651900000000 | 0.9329983300000000 | 0.8969989200000000 | 1.0 |
| Cl33 | Cl | 0.0877015400000000 | 0.8720002900000000 | 0.9754401700000000 | 1.0 |
| Cl34 | Cl | 0.9358701900000000 | 0.9122821900000000 | 0.1119665500000000 | 1.0 |
| Cl35 | Cl | 0.8847327300000000 | 0.9330159400000000 | 0.8969966400000000 | 1.0 |
| Cl36 | Cl | 0.7278727700000000 | 0.8565702300000000 | 0.0238446400000000 | 1.0 |

##### cif ends

furand\_Cl\_23\_syn\_dir\_forbid Energy: -208.38123191

##### cif starts

data\_furand\_Cl\_23\_syn\_dir\_forbid

\_publ\_section\_comment

;

;

```

_cell_length_a  9.7850370148
_cell_length_b  20.0
_cell_length_c  20.0
_cell_angle_alpha  90.0
_cell_angle_beta  90.0
_cell_angle_gamma  90.0

```

```

_symmetry_space_group_name_H-M  'P 1'
_symmetry_Int_Tables_number 1
_symmetry_cell_setting triclinic

```

```

loop_
_atom_site_label
_atom_site_type_symbol
_atom_site_fract_x
_atom_site_fract_y
_atom_site_fract_z
_atom_site_occupancy
H1  H  0.0311021100000000  0.1069041000000000  0.0378852700000000  1.0
H2  H  0.0042046200000000  0.0451633500000000  0.9139175400000000  1.0
H3  H  0.2554951600000000  0.0876796800000000  0.0715685000000000  1.0
H4  H  0.2680071700000000  0.0743392400000000  0.9313970300000000  1.0
H5  H  0.5311029500000000  0.1069031800000000  0.0378868100000000  1.0
H6  H  0.5042010400000000  0.0451651100000000  0.9139182100000000  1.0
H7  H  0.7554983600000000  0.0876794800000000  0.0715660500000000  1.0
H8  H  0.7680098300000000  0.0743383200000000  0.9313943700000000  1.0
C9  C  0.0600018400000000  0.0555187300000000  0.0244168000000000  1.0
C10 C  0.9704819100000000  0.0308887100000000  0.9641567700000000  1.0
C11 C  0.9423340900000000  0.9526536400000000  0.9748168100000000  1.0
C12 C  0.0226166700000000  0.9483213500000000  0.0429973100000000  1.0
C13 C  0.2253916500000000  0.0488577200000000  0.0357731900000000  1.0
C14 C  0.3078047700000000  0.0420269600000000  0.9711163700000000  1.0
C15 C  0.2825773100000000  0.9666767800000000  0.9610520600000000  1.0
C16 C  0.1912181900000000  0.9400261100000000  0.0224327500000000  1.0
C17 C  0.5600022300000000  0.0555184900000000  0.0244168600000000  1.0
C18 C  0.4704800400000000  0.0308895300000000  0.9641574400000000  1.0
C19 C  0.4423330600000000  0.9526540500000000  0.9748164700000000  1.0
C20 C  0.5226184000000000  0.9483205000000000  0.0429962100000000  1.0
C21 C  0.7253929700000000  0.0488573000000000  0.0357705200000000  1.0
C22 C  0.8078061800000000  0.0420262900000000  0.9711143400000000  1.0
C23 C  0.7825791500000000  0.9666759400000000  0.9610506800000000  1.0
C24 C  0.6912199100000000  0.9400255200000000  0.0224308300000000  1.0
O25 O  0.0104840400000000  0.0114341000000000  0.0747675000000000  1.0
O26 O  0.2462035900000000  0.9853914000000000  0.0702151600000000  1.0
O27 O  0.5104865300000000  0.0114325900000000  0.0747674500000000  1.0
O28 O  0.7462052700000000  0.9853911300000000  0.0702132900000000  1.0
Cl29 Cl  0.9945370500000000  0.8841574000000000  0.9248654200000000  1.0
Cl30 Cl  0.9888773000000000  0.8918053400000000  0.1075639600000000  1.0
Cl31 Cl  0.2458304600000000  0.9521902200000000  0.8755300000000000  1.0
Cl32 Cl  0.2343392600000000  0.8550842100000000  0.0323074000000000  1.0
Cl33 Cl  0.4945350200000000  0.8841592100000000  0.9248630700000000  1.0
Cl34 Cl  0.4888810700000000  0.8918032400000000  0.1075620700000000  1.0

```

Cl35 Cl 0.7458348700000000 0.9521882500000000 0.8755286100000000 1.0  
Cl36 Cl 0.7343415000000000 0.8550837000000000 0.0323056600000000 1.0

##### cif ends

furane Cl 24 anti alt Energy: -212.00906462

##### cif starts

data\_furane Cl 24 anti alt

\_publ\_section\_comment

;  
Andrew Reynoso, Bohan Xu, and Vincent H. Crespi  
;

\_cell\_length\_a 9.6547452385

\_cell\_length\_b 20.0

\_cell\_length\_c 20.0

\_cell\_angle\_alpha 90.0

\_cell\_angle\_beta 90.0

\_cell\_angle\_gamma 90.0

\_symmetry\_space\_group\_name\_H-M 'P 1'

\_symmetry\_Int\_Tables\_number 1

\_symmetry\_cell\_setting triclinic

loop\_

\_atom\_site\_label

\_atom\_site\_type\_symbol

\_atom\_site\_fract\_x

\_atom\_site\_fract\_y

\_atom\_site\_fract\_z

\_atom\_site\_occupancy

|     |   |                    |                    |                    |     |
|-----|---|--------------------|--------------------|--------------------|-----|
| H1  | H | 0.5076848400000000 | 0.9320795100000000 | 0.0715024900000000 | 1.0 |
| H2  | H | 0.5285730700000000 | 0.1067219300000000 | 0.9556110400000000 | 1.0 |
| H3  | H | 0.7576817700000000 | 0.0679217600000000 | 0.9284979600000000 | 1.0 |
| H4  | H | 0.7785767600000000 | 0.8932779500000000 | 0.0443871400000000 | 1.0 |
| H5  | H | 0.0076845100000000 | 0.9320795300000000 | 0.0715003100000000 | 1.0 |
| H6  | H | 0.0285796100000000 | 0.1067226100000000 | 0.9556105000000000 | 1.0 |
| H7  | H | 0.2576879900000000 | 0.0679204800000000 | 0.9284996100000000 | 1.0 |
| H8  | H | 0.2785782900000000 | 0.8932762300000000 | 0.0443881600000000 | 1.0 |
| C9  | C | 0.4659273800000000 | 0.9578764700000000 | 0.0276302200000000 | 1.0 |
| C10 | C | 0.4662273500000000 | 0.0348237100000000 | 0.0364723800000000 | 1.0 |
| C11 | C | 0.5549242600000000 | 0.0569522800000000 | 0.9745618200000000 | 1.0 |
| C12 | C | 0.5540180100000000 | 0.9485333900000000 | 0.9645452500000000 | 1.0 |
| C13 | C | 0.7159255100000000 | 0.0421240100000000 | 0.9723701300000000 | 1.0 |
| C14 | C | 0.7162275700000000 | 0.9651768100000000 | 0.9635278100000000 | 1.0 |
| C15 | C | 0.8049264100000000 | 0.9430480500000000 | 0.0254371800000000 | 1.0 |
| C16 | C | 0.8040175600000000 | 0.0514669600000000 | 0.0354545100000000 | 1.0 |
| C17 | C | 0.9659267400000000 | 0.9578767800000000 | 0.0276281600000000 | 1.0 |
| C18 | C | 0.9662277900000000 | 0.0348240100000000 | 0.0364705600000000 | 1.0 |
| C19 | C | 0.0549276900000000 | 0.0569524600000000 | 0.9745611400000000 | 1.0 |
| C20 | C | 0.0540181100000000 | 0.9485335800000000 | 0.9645435600000000 | 1.0 |
| C21 | C | 0.2159281700000000 | 0.0421229800000000 | 0.9723711800000000 | 1.0 |
| C22 | C | 0.2162290500000000 | 0.9651756600000000 | 0.9635284300000000 | 1.0 |
| C23 | C | 0.3049268200000000 | 0.9430469000000000 | 0.0254384600000000 | 1.0 |

|      |    |                    |                    |                    |     |
|------|----|--------------------|--------------------|--------------------|-----|
| C24  | C  | 0.3040168300000000 | 0.0514655200000000 | 0.0354568200000000 | 1.0 |
| O25  | O  | 0.5078914200000000 | 0.0071331300000000 | 0.9263563200000000 | 1.0 |
| O26  | O  | 0.7578932500000000 | 0.9928666500000000 | 0.0736433500000000 | 1.0 |
| O27  | O  | 0.0078948600000000 | 0.0071340100000000 | 0.9263548600000000 | 1.0 |
| O28  | O  | 0.2578927200000000 | 0.9928650100000000 | 0.0736446900000000 | 1.0 |
| Cl29 | Cl | 0.5234733100000000 | 0.8675745500000000 | 0.9322182300000000 | 1.0 |
| Cl30 | Cl | 0.5162755900000000 | 0.0572040500000000 | 0.1195850500000000 | 1.0 |
| Cl31 | Cl | 0.7734722200000000 | 0.1324252800000000 | 0.0677826700000000 | 1.0 |
| Cl32 | Cl | 0.7662717800000000 | 0.9427980800000000 | 0.8804140700000000 | 1.0 |
| Cl33 | Cl | 0.0234706700000000 | 0.8675760500000000 | 0.9322142800000000 | 1.0 |
| Cl34 | Cl | 0.0162718100000000 | 0.0572024500000000 | 0.1195845800000000 | 1.0 |
| Cl35 | Cl | 0.2734698200000000 | 0.1324233800000000 | 0.0677856500000000 | 1.0 |
| Cl36 | Cl | 0.2662764400000000 | 0.9427957800000000 | 0.8804154000000000 | 1.0 |

##### cif ends

furan\_Cl\_24\_anti\_alt\_forbid Energy: -212.78700745

##### cif starts

data\_furan\_Cl\_24\_anti\_alt\_forbid

\_publ\_section\_comment

;  
Andrew Reynoso, Bohan Xu, and Vincent H. Crespi  
;

\_cell\_length\_a 10.4061681386

\_cell\_length\_b 20.0

\_cell\_length\_c 20.0

\_cell\_angle\_alpha 90.0

\_cell\_angle\_beta 90.0

\_cell\_angle\_gamma 90.0

\_symmetry\_space\_group\_name\_H-M 'P 1'

\_symmetry\_Int\_Tables\_number 1

\_symmetry\_cell\_setting triclinic

loop\_

\_atom\_site\_label

\_atom\_site\_type\_symbol

\_atom\_site\_fract\_x

\_atom\_site\_fract\_y

\_atom\_site\_fract\_z

\_atom\_site\_occupancy

|    |   |                    |                    |                    |     |
|----|---|--------------------|--------------------|--------------------|-----|
| H1 | H | 0.0656703300000000 | 0.8956412600000000 | 0.9302116100000000 | 1.0 |
|----|---|--------------------|--------------------|--------------------|-----|

|    |   |                    |                    |                    |     |
|----|---|--------------------|--------------------|--------------------|-----|
| H2 | H | 0.9469121900000000 | 0.0627209000000000 | 0.0488184600000000 | 1.0 |
|----|---|--------------------|--------------------|--------------------|-----|

|    |   |                    |                    |                    |     |
|----|---|--------------------|--------------------|--------------------|-----|
| H3 | H | 0.2194930600000000 | 0.0943612300000000 | 0.0353662500000000 | 1.0 |
|----|---|--------------------|--------------------|--------------------|-----|

|    |   |                    |                    |                    |     |
|----|---|--------------------|--------------------|--------------------|-----|
| H4 | H | 0.3383396200000000 | 0.9273848800000000 | 0.9166628200000000 | 1.0 |
|----|---|--------------------|--------------------|--------------------|-----|

|    |   |                    |                    |                    |     |
|----|---|--------------------|--------------------|--------------------|-----|
| H5 | H | 0.5653826800000000 | 0.8957038000000000 | 0.9303281300000000 | 1.0 |
|----|---|--------------------|--------------------|--------------------|-----|

|    |   |                    |                    |                    |     |
|----|---|--------------------|--------------------|--------------------|-----|
| H6 | H | 0.4472242800000000 | 0.0629270500000000 | 0.0488926800000000 | 1.0 |
|----|---|--------------------|--------------------|--------------------|-----|

|    |   |                    |                    |                    |     |
|----|---|--------------------|--------------------|--------------------|-----|
| H7 | H | 0.7199408600000000 | 0.0943924400000000 | 0.0351485600000000 | 1.0 |
|----|---|--------------------|--------------------|--------------------|-----|

|    |   |                    |                    |                    |     |
|----|---|--------------------|--------------------|--------------------|-----|
| H8 | H | 0.8380504600000000 | 0.9270834100000000 | 0.9166890700000000 | 1.0 |
|----|---|--------------------|--------------------|--------------------|-----|

|    |   |                    |                    |                    |     |
|----|---|--------------------|--------------------|--------------------|-----|
| C9 | C | 0.0800954700000000 | 0.0529557500000000 | 0.9627446400000000 | 1.0 |
|----|---|--------------------|--------------------|--------------------|-----|

|     |   |                    |                    |                    |     |
|-----|---|--------------------|--------------------|--------------------|-----|
| C10 | C | 0.9561432000000000 | 0.0363375000000000 | 0.0010661400000000 | 1.0 |
|-----|---|--------------------|--------------------|--------------------|-----|

|     |   |                    |                    |                    |     |
|-----|---|--------------------|--------------------|--------------------|-----|
| C11 | C | 0.9581146700000000 | 0.9582344000000000 | 0.0056692700000000 | 1.0 |
|-----|---|--------------------|--------------------|--------------------|-----|

|     |   |                    |                    |                    |     |
|-----|---|--------------------|--------------------|--------------------|-----|
| C12 | C | 0.0785234100000000 | 0.9404404000000000 | 0.9610990200000000 | 1.0 |
|-----|---|--------------------|--------------------|--------------------|-----|

|      |    |                    |                    |                    |     |
|------|----|--------------------|--------------------|--------------------|-----|
| C13  | C  | 0.2066943500000000 | 0.0495835100000000 | 0.0044454800000000 | 1.0 |
| C14  | C  | 0.3271129500000000 | 0.0318306000000000 | 0.9598824500000000 | 1.0 |
| C15  | C  | 0.3290951000000000 | 0.9537230900000000 | 0.9644373300000000 | 1.0 |
| C16  | C  | 0.2051534600000000 | 0.9370668500000000 | 0.0027649600000000 | 1.0 |
| C17  | C  | 0.5801538400000000 | 0.0530213700000000 | 0.9627190400000000 | 1.0 |
| C18  | C  | 0.4562157400000000 | 0.0365209000000000 | 0.0011379000000000 | 1.0 |
| C19  | C  | 0.4581021700000000 | 0.9584133800000000 | 0.0057629800000000 | 1.0 |
| C20  | C  | 0.5784053000000000 | 0.9405136800000000 | 0.9611766200000000 | 1.0 |
| C21  | C  | 0.7068443100000000 | 0.0495700900000000 | 0.0043250200000000 | 1.0 |
| C22  | C  | 0.8271394700000000 | 0.0316376900000000 | 0.9597405000000000 | 1.0 |
| C23  | C  | 0.8290207300000000 | 0.9535337900000000 | 0.9644153000000000 | 1.0 |
| C24  | C  | 0.7050606700000000 | 0.9370649200000000 | 0.0028114300000000 | 1.0 |
| O25  | O  | 0.0865981300000000 | 0.9972370400000000 | 0.9162820000000000 | 1.0 |
| O26  | O  | 0.1986519800000000 | 0.9927701000000000 | 0.0492420200000000 | 1.0 |
| O27  | O  | 0.5864159300000000 | 0.9972647000000000 | 0.9162938400000000 | 1.0 |
| O28  | O  | 0.6987692100000000 | 0.9928348600000000 | 0.0492169300000000 | 1.0 |
| Cl29 | Cl | 0.0744265600000000 | 0.1332298400000000 | 0.9249286900000000 | 1.0 |
| Cl30 | Cl | 0.9578624000000000 | 0.9273664200000000 | 0.0886548400000000 | 1.0 |
| Cl31 | Cl | 0.3273695700000000 | 0.0627384300000000 | 0.8769071300000000 | 1.0 |
| Cl32 | Cl | 0.2108281700000000 | 0.8567721300000000 | 0.0405491700000000 | 1.0 |
| Cl33 | Cl | 0.5748366500000000 | 0.1332819200000000 | 0.9248672500000000 | 1.0 |
| Cl34 | Cl | 0.4577120300000000 | 0.9276604700000000 | 0.0887949500000000 | 1.0 |
| Cl35 | Cl | 0.8275078300000000 | 0.0623678800000000 | 0.8766990200000000 | 1.0 |
| Cl36 | Cl | 0.7103468200000000 | 0.8568274200000000 | 0.0407173200000000 | 1.0 |

##### cif ends

furandata\_furan\_Cl\_24\_anti\_dir Energy: -214.05518301

##### cif starts

data\_furan\_Cl\_24\_anti\_dir

\_publ\_section\_comment

;  
Andrew Reynoso, Bohan Xu, and Vincent H. Crespi  
;

\_cell\_length\_a 9.4920545577

\_cell\_length\_b 20.0

\_cell\_length\_c 20.0

\_cell\_angle\_alpha 90.0

\_cell\_angle\_beta 90.0

\_cell\_angle\_gamma 90.0

\_symmetry\_space\_group\_name\_H-M 'P 1'

\_symmetry\_Int\_Tables\_number 1

\_symmetry\_cell\_setting triclinic

loop\_

\_atom\_site\_label

\_atom\_site\_type\_symbol

\_atom\_site\_fract\_x

\_atom\_site\_fract\_y

\_atom\_site\_fract\_z

\_atom\_site\_occupancy

H1 H 0.5680810100000000 0.0596609200000000 0.0766496900000000 1.0

|      |    |                    |                    |                    |     |
|------|----|--------------------|--------------------|--------------------|-----|
| H2   | H  | 0.5839826200000000 | 0.8967580100000000 | 0.9445941100000000 | 1.0 |
| H3   | H  | 0.8180520800000000 | 0.0591567500000000 | 0.9229364800000000 | 1.0 |
| H4   | H  | 0.8339727500000000 | 0.8971374100000000 | 0.0560757700000000 | 1.0 |
| H5   | H  | 0.0679749000000000 | 0.0596722900000000 | 0.0767088400000000 | 1.0 |
| H6   | H  | 0.0839442600000000 | 0.8968178200000000 | 0.9445768200000000 | 1.0 |
| H7   | H  | 0.3179948000000000 | 0.0592105700000000 | 0.9229564400000000 | 1.0 |
| H8   | H  | 0.3339420300000000 | 0.8971441700000000 | 0.0560502900000000 | 1.0 |
| C9   | C  | 0.5226252000000000 | 0.0382812700000000 | 0.0311757400000000 | 1.0 |
| C10  | C  | 0.5201485900000000 | 0.9599998700000000 | 0.0309979200000000 | 1.0 |
| C11  | C  | 0.6073046200000000 | 0.9448309600000000 | 0.9678228500000000 | 1.0 |
| C12  | C  | 0.6092118200000000 | 0.0531283000000000 | 0.9669865400000000 | 1.0 |
| C13  | C  | 0.7726114900000000 | 0.0380745700000000 | 0.9685540100000000 | 1.0 |
| C14  | C  | 0.7701632800000000 | 0.9597962700000000 | 0.9692487100000000 | 1.0 |
| C15  | C  | 0.8572932300000000 | 0.9450562800000000 | 0.0325301900000000 | 1.0 |
| C16  | C  | 0.8591840800000000 | 0.0533557000000000 | 0.0326489900000000 | 1.0 |
| C17  | C  | 0.0225908500000000 | 0.0382969500000000 | 0.0312154900000000 | 1.0 |
| C18  | C  | 0.0201461200000000 | 0.9600153400000000 | 0.0310180100000000 | 1.0 |
| C19  | C  | 0.1072822500000000 | 0.9448769700000000 | 0.9678290200000000 | 1.0 |
| C20  | C  | 0.1091993400000000 | 0.0531743500000000 | 0.9670410600000000 | 1.0 |
| C21  | C  | 0.2725994000000000 | 0.0381110600000000 | 0.9685753700000000 | 1.0 |
| C22  | C  | 0.2701371900000000 | 0.9598329700000000 | 0.9692437500000000 | 1.0 |
| C23  | C  | 0.3572896300000000 | 0.9450644100000000 | 0.0325143800000000 | 1.0 |
| C24  | C  | 0.3592343100000000 | 0.0533638100000000 | 0.0326531600000000 | 1.0 |
| O25  | O  | 0.5631944200000000 | 0.9989411100000000 | 0.9242760400000000 | 1.0 |
| O26  | O  | 0.8131467400000000 | 0.9994534100000000 | 0.0757146000000000 | 1.0 |
| O27  | O  | 0.0631553900000000 | 0.9990056500000000 | 0.9243078000000000 | 1.0 |
| O28  | O  | 0.3131971600000000 | 0.9994583200000000 | 0.0757153200000000 | 1.0 |
| Cl29 | Cl | 0.5715199500000000 | 0.1305259300000000 | 0.9287162900000000 | 1.0 |
| Cl30 | Cl | 0.5790342900000000 | 0.9176179600000000 | 0.1054074400000000 | 1.0 |
| Cl31 | Cl | 0.8214703700000000 | 0.1310139900000000 | 0.0703831300000000 | 1.0 |
| Cl32 | Cl | 0.8290992400000000 | 0.9169332800000000 | 0.8951223000000000 | 1.0 |
| Cl33 | Cl | 0.0715138100000000 | 0.1306008400000000 | 0.9288266500000000 | 1.0 |
| Cl34 | Cl | 0.0790696900000000 | 0.9176249600000000 | 0.1054146200000000 | 1.0 |
| Cl35 | Cl | 0.3216176400000000 | 0.1310194900000000 | 0.0704129000000000 | 1.0 |
| Cl36 | Cl | 0.3290284200000000 | 0.9169870200000000 | 0.8951012800000000 | 1.0 |

##### cif ends

furandirforbid Energy: -214.82652379

##### cif starts

furandirforbid

publ\_section\_comment

;  
Andrew Reynoso, Bohan Xu, and Vincent H. Crespi  
;

\_cell\_length\_a 10.2655525939

\_cell\_length\_b 20.0

\_cell\_length\_c 20.0

\_cell\_angle\_alpha 90.0

\_cell\_angle\_beta 90.0

\_cell\_angle\_gamma 90.0

\_symmetry\_space\_group\_name\_H-M 'P 1'



\_symmetry\_Int\_Tables\_number 1  
\_symmetry\_cell\_setting triclinic

loop\_  
\_atom\_site\_label  
\_atom\_site\_type\_symbol  
\_atom\_site\_fract\_x  
\_atom\_site\_fract\_y  
\_atom\_site\_fract\_z  
\_atom\_site\_occupancy

|      |    |                    |                    |                    |     |
|------|----|--------------------|--------------------|--------------------|-----|
| H1   | H  | 0.9678365000000000 | 0.0656080700000000 | 0.0624928500000000 | 1.0 |
| H2   | H  | 0.0860541500000000 | 0.8995905400000000 | 0.9424279700000000 | 1.0 |
| H3   | H  | 0.3461727000000000 | 0.0639004700000000 | 0.9239020600000000 | 1.0 |
| H4   | H  | 0.2279542800000000 | 0.9008300800000000 | 0.0479316500000000 | 1.0 |
| H5   | H  | 0.4678119400000000 | 0.0656103000000000 | 0.0624960100000000 | 1.0 |
| H6   | H  | 0.5860682200000000 | 0.8995791700000000 | 0.9424605600000000 | 1.0 |
| H7   | H  | 0.8461583200000000 | 0.0639123100000000 | 0.9239078400000000 | 1.0 |
| H8   | H  | 0.7279909100000000 | 0.9008408600000000 | 0.0479522500000000 | 1.0 |
| C9   | C  | 0.0928504600000000 | 0.0577317200000000 | 0.9717454600000000 | 1.0 |
| C10  | C  | 0.9712299500000000 | 0.0404895200000000 | 0.0139327500000000 | 1.0 |
| C11  | C  | 0.9729707900000000 | 0.9616625200000000 | 0.0142879800000000 | 1.0 |
| C12  | C  | 0.0953600400000000 | 0.9449090700000000 | 0.9727222600000000 | 1.0 |
| C13  | C  | 0.2212136800000000 | 0.0582346000000000 | 0.0148462600000000 | 1.0 |
| C14  | C  | 0.3428141800000000 | 0.0399807800000000 | 0.9730608200000000 | 1.0 |
| C15  | C  | 0.3410867900000000 | 0.9611640900000000 | 0.9746309700000000 | 1.0 |
| C16  | C  | 0.2186840700000000 | 0.9454195000000000 | 0.0165689300000000 | 1.0 |
| C17  | C  | 0.5928460700000000 | 0.0577274000000000 | 0.9717536900000000 | 1.0 |
| C18  | C  | 0.4712226200000000 | 0.0404868100000000 | 0.0139371200000000 | 1.0 |
| C19  | C  | 0.4729644400000000 | 0.9616602500000000 | 0.0143016600000000 | 1.0 |
| C20  | C  | 0.5953641200000000 | 0.9449029300000000 | 0.9727444500000000 | 1.0 |
| C21  | C  | 0.7212130500000000 | 0.0582410300000000 | 0.0148547800000000 | 1.0 |
| C22  | C  | 0.8428097900000000 | 0.0399881600000000 | 0.9730658500000000 | 1.0 |
| C23  | C  | 0.8410808200000000 | 0.9611716900000000 | 0.9746326700000000 | 1.0 |
| C24  | C  | 0.7186942000000000 | 0.9454250300000000 | 0.0165868800000000 | 1.0 |
| O25  | O  | 0.1040559600000000 | 0.0013558400000000 | 0.9274609000000000 | 1.0 |
| O26  | O  | 0.2100112400000000 | 0.0029305400000000 | 0.0604683000000000 | 1.0 |
| O27  | O  | 0.6040540000000000 | 0.0013450500000000 | 0.9274761500000000 | 1.0 |
| O28  | O  | 0.7100239200000000 | 0.0029393900000000 | 0.0604799600000000 | 1.0 |
| Cl29 | Cl | 0.0787162000000000 | 0.1301358600000000 | 0.9216291700000000 | 1.0 |
| Cl30 | Cl | 0.9695423800000000 | 0.9170845600000000 | 0.0911547600000000 | 1.0 |
| Cl31 | Cl | 0.2354109500000000 | 0.1318009500000000 | 0.0632346200000000 | 1.0 |
| Cl32 | Cl | 0.3445678300000000 | 0.9146985900000000 | 0.8988926800000000 | 1.0 |
| Cl33 | Cl | 0.5787082600000000 | 0.1301249300000000 | 0.9216280800000000 | 1.0 |
| Cl34 | Cl | 0.4695144000000000 | 0.9170931600000000 | 0.0911741200000000 | 1.0 |
| Cl35 | Cl | 0.7353971900000000 | 0.1318129100000000 | 0.0632351100000000 | 1.0 |
| Cl36 | Cl | 0.8445346200000000 | 0.9147082300000000 | 0.8988911500000000 | 1.0 |

##### cif ends

uranium\_Cl\_24\_syn\_alt Energy: -215.17225824

##### cif starts

data\_uranium\_Cl\_24\_syn\_alt

\_publ\_section\_comment

;

;

```
_cell_length_a 10.3739294022
_cell_length_b 20.0
_cell_length_c 20.0
_cell_angle_alpha 90.0
_cell_angle_beta 90.0
_cell_angle_gamma 90.0
```

```
_symmetry_space_group_name_H-M 'P 1'
_symmetry_Int_Tables_number 1
_symmetry_cell_setting triclinic
```

```
loop_
_atom_site_label
_atom_site_type_symbol
_atom_site_fract_x
_atom_site_fract_y
_atom_site_fract_z
_atom_site_occupancy
H1 H 0.6389999400000000 0.9382951900000000 0.9285810800000000 1.0
H2 H 0.5141034200000000 0.1008946900000000 0.0472969100000000 1.0
H3 H 0.8889917600000000 0.0627633200000000 0.9295140300000000 1.0
H4 H 0.7640965400000000 0.8984125900000000 0.0457912000000000 1.0
H5 H 0.1389992800000000 0.9382944200000000 0.9285816900000000 1.0
H6 H 0.0141038800000000 0.1008952700000000 0.0472953500000000 1.0
H7 H 0.3889922800000000 0.0627635600000000 0.9295151000000000 1.0
H8 H 0.2640986300000000 0.8984120200000000 0.0457913100000000 1.0
C9 C 0.6396445700000000 0.9607199200000000 0.9784008400000000 1.0
C10 C 0.6380676200000000 0.0391928900000000 0.9790725500000000 1.0
C11 C 0.5129923700000000 0.0533115300000000 0.0203736200000000 1.0
C12 C 0.5150367800000000 0.9458803500000000 0.0194925600000000 1.0
C13 C 0.8896438500000000 0.0395955600000000 0.9789926100000000 1.0
C14 C 0.8880656100000000 0.9611218700000000 0.9784910700000000 1.0
C15 C 0.7629908500000000 0.9463897500000000 0.0195771900000000 1.0
C16 C 0.7650381300000000 0.0538203500000000 0.0203015000000000 1.0
C17 C 0.1396448800000000 0.9607198900000000 0.9784012400000000 1.0
C18 C 0.1380685600000000 0.0391928500000000 0.9790726000000000 1.0
C19 C 0.0129925500000000 0.0533118900000000 0.0203726200000000 1.0
C20 C 0.0150366300000000 0.9458807600000000 0.0194930500000000 1.0
C21 C 0.3896437500000000 0.0395956000000000 0.9789935300000000 1.0
C22 C 0.3880661100000000 0.9611220500000000 0.9784909800000000 1.0
C23 C 0.2629914300000000 0.9463894600000000 0.0195775400000000 1.0
C24 C 0.2650381900000000 0.0538200900000000 0.0203021300000000 1.0
O25 O 0.5139587100000000 0.9986881100000000 0.0675219100000000 1.0
O26 O 0.7639506100000000 0.0002973500000000 0.0675398000000000 1.0
O27 O 0.0139583200000000 0.9986892700000000 0.0675217200000000 1.0
O28 O 0.2639511400000000 0.0002969500000000 0.0675401700000000 1.0
Cl29 Cl 0.5139461100000000 0.8671632400000000 0.0591792000000000 1.0
Cl30 Cl 0.6382681800000000 0.0799217800000000 0.8999568000000000 1.0
Cl31 Cl 0.7639473800000000 0.1319459400000000 0.0611396100000000 1.0
Cl32 Cl 0.8882543100000000 0.9215838000000000 0.8987743600000000 1.0
Cl33 Cl 0.0139475000000000 0.8671643000000000 0.0591810700000000 1.0
Cl34 Cl 0.1382706500000000 0.0799208200000000 0.8999564600000000 1.0
```

Cl35 Cl 0.2639479000000000 0.1319458300000000 0.0611396400000000 1.0  
Cl36 Cl 0.3882545800000000 0.9215847200000000 0.8987739300000000 1.0

##### cif ends

furand Cl24 syn alt forbid Energy: -212.0291044

##### cif starts

data\_furand Cl24 syn alt forbid

\_publ\_section\_comment

;  
Andrew Reynoso, Bohan Xu, and Vincent H. Crespi  
;

\_cell\_length\_a 9.7149560463

\_cell\_length\_b 20.0

\_cell\_length\_c 20.0

\_cell\_angle\_alpha 90.0

\_cell\_angle\_beta 90.0

\_cell\_angle\_gamma 90.0

\_symmetry\_space\_group\_name\_H-M 'P 1'

\_symmetry\_Int\_Tables\_number 1

\_symmetry\_cell\_setting triclinic

loop\_

\_atom\_site\_label

\_atom\_site\_type\_symbol

\_atom\_site\_fract\_x

\_atom\_site\_fract\_y

\_atom\_site\_fract\_z

\_atom\_site\_occupancy

|     |   |                    |                    |                    |     |
|-----|---|--------------------|--------------------|--------------------|-----|
| H1  | H | 0.9059561100000000 | 0.0581415800000000 | 0.9115981200000000 | 1.0 |
| H2  | H | 0.8954726800000000 | 0.8978990200000000 | 0.0505089700000000 | 1.0 |
| H3  | H | 0.1581585900000000 | 0.0976997200000000 | 0.0466143700000000 | 1.0 |
| H4  | H | 0.1476686900000000 | 0.9321521600000000 | 0.9140781700000000 | 1.0 |
| H5  | H | 0.4059079300000000 | 0.0581164100000000 | 0.9116204300000000 | 1.0 |
| H6  | H | 0.3954267800000000 | 0.8978479800000000 | 0.0504932100000000 | 1.0 |
| H7  | H | 0.6581442700000000 | 0.0977287700000000 | 0.0465768100000000 | 1.0 |
| H8  | H | 0.6476919600000000 | 0.9321296900000000 | 0.9141057900000000 | 1.0 |
| C9  | C | 0.8604482900000000 | 0.0530658600000000 | 0.0204889300000000 | 1.0 |
| C10 | C | 0.9444483600000000 | 0.0351617600000000 | 0.9573129600000000 | 1.0 |
| C11 | C | 0.9452983700000000 | 0.9569361800000000 | 0.9594254400000000 | 1.0 |
| C12 | C | 0.8616989200000000 | 0.9425387400000000 | 0.0238054900000000 | 1.0 |
| C13 | C | 0.1918999600000000 | 0.0520432600000000 | 0.0216768600000000 | 1.0 |
| C14 | C | 0.1082935900000000 | 0.0351439100000000 | 0.9579114300000000 | 1.0 |
| C15 | C | 0.1091386500000000 | 0.9568963400000000 | 0.9588531200000000 | 1.0 |
| C16 | C | 0.1931309200000000 | 0.9414735300000000 | 0.0226879600000000 | 1.0 |
| C17 | C | 0.3604505700000000 | 0.0530295900000000 | 0.0205143300000000 | 1.0 |
| C18 | C | 0.4444359500000000 | 0.0351385200000000 | 0.9573275600000000 | 1.0 |
| C19 | C | 0.4453038200000000 | 0.9569123500000000 | 0.9594349100000000 | 1.0 |
| C20 | C | 0.3616816700000000 | 0.9425009800000000 | 0.0238012100000000 | 1.0 |
| C21 | C | 0.6918976200000000 | 0.0520662900000000 | 0.0216564200000000 | 1.0 |
| C22 | C | 0.6082793400000000 | 0.0351334700000000 | 0.9579053300000000 | 1.0 |
| C23 | C | 0.6091447200000000 | 0.9568864800000000 | 0.9588711700000000 | 1.0 |

|      |    |                    |                    |                    |     |
|------|----|--------------------|--------------------|--------------------|-----|
| C24  | C  | 0.6931492300000000 | 0.9414969200000000 | 0.0227090500000000 | 1.0 |
| O25  | O  | 0.8948827400000000 | 0.9992053700000000 | 0.0642993500000000 | 1.0 |
| O26  | O  | 0.1587266900000000 | 0.9970103300000000 | 0.0643595800000000 | 1.0 |
| O27  | O  | 0.3948689100000000 | 0.9991545300000000 | 0.0643113900000000 | 1.0 |
| O28  | O  | 0.6587428300000000 | 0.9970476000000000 | 0.0643616100000000 | 1.0 |
| Cl29 | Cl | 0.9098325000000000 | 0.1306033100000000 | 0.0571188000000000 | 1.0 |
| Cl30 | Cl | 0.8884265400000000 | 0.9114895600000000 | 0.8874257600000000 | 1.0 |
| Cl31 | Cl | 0.1651885000000000 | 0.0777408700000000 | 0.8841941100000000 | 1.0 |
| Cl32 | Cl | 0.1437384600000000 | 0.8654399100000000 | 0.0623424900000000 | 1.0 |
| Cl33 | Cl | 0.4098445700000000 | 0.1305518400000000 | 0.0571726600000000 | 1.0 |
| Cl34 | Cl | 0.3884543100000000 | 0.9114650800000000 | 0.8874310800000000 | 1.0 |
| Cl35 | Cl | 0.6651409000000000 | 0.0777126100000000 | 0.8841722900000000 | 1.0 |
| Cl36 | Cl | 0.6437971800000000 | 0.8654746100000000 | 0.0623947600000000 | 1.0 |

##### cif ends

uran\_Cl\_24\_syn\_dir Energy: -211.1485704

##### cif starts

data\_uran\_Cl\_24\_syn\_dir

\_publ\_section\_comment

;  
Andrew Reynoso, Bohan Xu, and Vincent H. Crespi  
;

\_cell\_length\_a 10.5053019007

\_cell\_length\_b 20.0

\_cell\_length\_c 20.0

\_cell\_angle\_alpha 90.0

\_cell\_angle\_beta 90.0

\_cell\_angle\_gamma 90.0

\_symmetry\_space\_group\_name\_H-M 'P 1'

\_symmetry\_Int\_Tables\_number 1

\_symmetry\_cell\_setting triclinic

loop\_

\_atom\_site\_label

\_atom\_site\_type\_symbol

\_atom\_site\_fract\_x

\_atom\_site\_fract\_y

\_atom\_site\_fract\_z

\_atom\_site\_occupancy

|    |   |                    |                    |                    |     |
|----|---|--------------------|--------------------|--------------------|-----|
| H1 | H | 0.1459415100000000 | 0.0730666500000000 | 0.9486092800000000 | 1.0 |
|----|---|--------------------|--------------------|--------------------|-----|

|    |   |                    |                    |                    |     |
|----|---|--------------------|--------------------|--------------------|-----|
| H2 | H | 0.0200093100000000 | 0.8872660000000000 | 0.0315168800000000 | 1.0 |
|----|---|--------------------|--------------------|--------------------|-----|

|    |   |                    |                    |                    |     |
|----|---|--------------------|--------------------|--------------------|-----|
| H3 | H | 0.3574131000000000 | 0.0644330800000000 | 0.9388123600000000 | 1.0 |
|----|---|--------------------|--------------------|--------------------|-----|

|    |   |                    |                    |                    |     |
|----|---|--------------------|--------------------|--------------------|-----|
| H4 | H | 0.2582517200000000 | 0.8831831800000000 | 0.0188714500000000 | 1.0 |
|----|---|--------------------|--------------------|--------------------|-----|

|    |   |                    |                    |                    |     |
|----|---|--------------------|--------------------|--------------------|-----|
| H5 | H | 0.6102578800000000 | 0.0323580800000000 | 0.9129550800000000 | 1.0 |
|----|---|--------------------|--------------------|--------------------|-----|

|    |   |                    |                    |                    |     |
|----|---|--------------------|--------------------|--------------------|-----|
| H6 | H | 0.4909719300000000 | 0.9071447700000000 | 0.0664032200000000 | 1.0 |
|----|---|--------------------|--------------------|--------------------|-----|

|    |   |                    |                    |                    |     |
|----|---|--------------------|--------------------|--------------------|-----|
| H7 | H | 0.9246928500000000 | 0.0471154600000000 | 0.9196450400000000 | 1.0 |
|----|---|--------------------|--------------------|--------------------|-----|

|    |   |                    |                    |                    |     |
|----|---|--------------------|--------------------|--------------------|-----|
| H8 | H | 0.7777095500000000 | 0.9222701700000000 | 0.0747893600000000 | 1.0 |
|----|---|--------------------|--------------------|--------------------|-----|

|    |   |                    |                    |                    |     |
|----|---|--------------------|--------------------|--------------------|-----|
| C9 | C | 0.1369835300000000 | 0.0399167000000000 | 0.9919186900000000 | 1.0 |
|----|---|--------------------|--------------------|--------------------|-----|

|     |   |                    |                    |                    |     |
|-----|---|--------------------|--------------------|--------------------|-----|
| C10 | C | 0.1360725100000000 | 0.9634716100000000 | 0.9723933500000000 | 1.0 |
|-----|---|--------------------|--------------------|--------------------|-----|

|     |   |                    |                    |                    |     |
|-----|---|--------------------|--------------------|--------------------|-----|
| C11 | C | 0.0117879700000000 | 0.9383395800000000 | 0.0120753600000000 | 1.0 |
|-----|---|--------------------|--------------------|--------------------|-----|

|     |   |                    |                    |                    |     |
|-----|---|--------------------|--------------------|--------------------|-----|
| C12 | C | 0.0044509700000000 | 0.0456934800000000 | 0.0259347500000000 | 1.0 |
|-----|---|--------------------|--------------------|--------------------|-----|

|      |    |                    |                    |                    |     |
|------|----|--------------------|--------------------|--------------------|-----|
| C13  | C  | 0.3786696500000000 | 0.0386633500000000 | 0.9857764300000000 | 1.0 |
| C14  | C  | 0.3897421900000000 | 0.9617910600000000 | 0.9784538000000000 | 1.0 |
| C15  | C  | 0.2607278700000000 | 0.9367872500000000 | 0.0074346100000000 | 1.0 |
| C16  | C  | 0.2602617000000000 | 0.0414343900000000 | 0.0369541900000000 | 1.0 |
| C17  | C  | 0.6306098900000000 | 0.0259338700000000 | 0.9661341600000000 | 1.0 |
| C18  | C  | 0.6345262400000000 | 0.9501362800000000 | 0.9952455100000000 | 1.0 |
| C19  | C  | 0.5068300400000000 | 0.9496614900000000 | 0.0330325200000000 | 1.0 |
| C20  | C  | 0.5116481800000000 | 0.0548910300000000 | 0.0146795900000000 | 1.0 |
| C21  | C  | 0.8945483300000000 | 0.0313051400000000 | 0.9695409700000000 | 1.0 |
| C22  | C  | 0.8830047700000000 | 0.9556850700000000 | 0.9780762600000000 | 1.0 |
| C23  | C  | 0.7633515900000000 | 0.9562523100000000 | 0.0325504600000000 | 1.0 |
| C24  | C  | 0.7613284800000000 | 0.0559134500000000 | 0.9912643100000000 | 1.0 |
| O25  | O  | 0.0046498600000000 | 0.9852354500000000 | 0.0659895000000000 | 1.0 |
| O26  | O  | 0.2599668700000000 | 0.9754013800000000 | 0.0674315900000000 | 1.0 |
| O27  | O  | 0.5108396600000000 | 0.0099943300000000 | 0.0702343400000000 | 1.0 |
| O28  | O  | 0.7621210000000000 | 0.0246022800000000 | 0.0572246100000000 | 1.0 |
| Cl29 | Cl | 0.9807595000000000 | 0.1145196800000000 | 0.0782666600000000 | 1.0 |
| Cl30 | Cl | 0.1336584100000000 | 0.9510386400000000 | 0.8844502000000000 | 1.0 |
| Cl31 | Cl | 0.2659070900000000 | 0.0983964100000000 | 0.1029189300000000 | 1.0 |
| Cl32 | Cl | 0.4209210500000000 | 0.9387201300000000 | 0.8938841500000000 | 1.0 |
| Cl33 | Cl | 0.5213187900000000 | 0.1375130200000000 | 0.0431541800000000 | 1.0 |
| Cl34 | Cl | 0.6300287200000000 | 0.8661802800000000 | 0.9596685700000000 | 1.0 |
| Cl35 | Cl | 0.7681671000000000 | 0.1442953800000000 | 0.9783922300000000 | 1.0 |
| Cl36 | Cl | 0.8579716500000000 | 0.9161073400000000 | 0.8995302800000000 | 1.0 |

##### cif ends

furandata\_furan\_Cl\_24\_syn\_dir\_forbid Energy: -209.00954583

##### cif starts

data\_furan\_Cl\_24\_syn\_dir\_forbid

\_publ\_section\_comment

;  
Andrew Reynoso, Bohan Xu, and Vincent H. Crespi  
;

\_cell\_length\_a 9.6326938576

\_cell\_length\_b 20.0

\_cell\_length\_c 20.0

\_cell\_angle\_alpha 90.0

\_cell\_angle\_beta 90.0

\_cell\_angle\_gamma 90.0

\_symmetry\_space\_group\_name\_H-M 'P 1'

\_symmetry\_Int\_Tables\_number 1

\_symmetry\_cell\_setting triclinic

loop\_

\_atom\_site\_label

\_atom\_site\_type\_symbol

\_atom\_site\_fract\_x

\_atom\_site\_fract\_y

\_atom\_site\_fract\_z

\_atom\_site\_occupancy

H1 H 0.8984247200000000 0.0460919000000000 0.9022171300000000 1.0

|      |    |                    |                    |                    |     |
|------|----|--------------------|--------------------|--------------------|-----|
| H2   | H  | 0.9107798500000000 | 0.9094595500000000 | 0.0654506400000000 | 1.0 |
| H3   | H  | 0.1361212000000000 | 0.0758746600000000 | 0.9286776300000000 | 1.0 |
| H4   | H  | 0.1847705200000000 | 0.8875768700000000 | 0.0260453800000000 | 1.0 |
| H5   | H  | 0.3983179300000000 | 0.0460623400000000 | 0.9022464500000000 | 1.0 |
| H6   | H  | 0.4107323400000000 | 0.9094121800000000 | 0.0654542200000000 | 1.0 |
| H7   | H  | 0.6360376500000000 | 0.0758471800000000 | 0.9286256600000000 | 1.0 |
| H8   | H  | 0.6847940500000000 | 0.8876102300000000 | 0.0260985500000000 | 1.0 |
| C9   | C  | 0.8396472900000000 | 0.0544255200000000 | 0.0129347500000000 | 1.0 |
| C10  | C  | 0.9289607500000000 | 0.0289739400000000 | 0.9519645200000000 | 1.0 |
| C11  | C  | 0.9599362500000000 | 0.9520960100000000 | 0.9635379800000000 | 1.0 |
| C12  | C  | 0.8796173200000000 | 0.9481963300000000 | 0.0297610000000000 | 1.0 |
| C13  | C  | 0.1713544200000000 | 0.0468095700000000 | 0.0322853400000000 | 1.0 |
| C14  | C  | 0.0912962700000000 | 0.0416056500000000 | 0.9654358800000000 | 1.0 |
| C15  | C  | 0.1213908600000000 | 0.9660452800000000 | 0.9541800000000000 | 1.0 |
| C16  | C  | 0.2139596100000000 | 0.9393290300000000 | 0.0146798200000000 | 1.0 |
| C17  | C  | 0.3396217200000000 | 0.0543915100000000 | 0.0129703300000000 | 1.0 |
| C18  | C  | 0.4289191900000000 | 0.0289515300000000 | 0.9519868800000000 | 1.0 |
| C19  | C  | 0.4599202400000000 | 0.9520759900000000 | 0.9635529800000000 | 1.0 |
| C20  | C  | 0.3795980300000000 | 0.9481614500000000 | 0.0297726900000000 | 1.0 |
| C21  | C  | 0.6713692600000000 | 0.0468458700000000 | 0.0322511400000000 | 1.0 |
| C22  | C  | 0.5912645000000000 | 0.0415992600000000 | 0.9654180600000000 | 1.0 |
| C23  | C  | 0.6213738400000000 | 0.9660336700000000 | 0.9541886500000000 | 1.0 |
| C24  | C  | 0.7139728200000000 | 0.9393563100000000 | 0.0146926200000000 | 1.0 |
| O25  | O  | 0.8958530400000000 | 0.0118344200000000 | 0.0630962900000000 | 1.0 |
| O26  | O  | 0.1574408800000000 | 0.9827315300000000 | 0.0639473200000000 | 1.0 |
| O27  | O  | 0.3958384800000000 | 0.0117941300000000 | 0.0631231900000000 | 1.0 |
| O28  | O  | 0.6574760800000000 | 0.9827831800000000 | 0.0639449600000000 | 1.0 |
| Cl29 | Cl | 0.8770541900000000 | 0.1417276100000000 | 0.0145700600000000 | 1.0 |
| Cl30 | Cl | 0.9127926600000000 | 0.8773966100000000 | 0.9196811500000000 | 1.0 |
| Cl31 | Cl | 0.1349759300000000 | 0.1034861000000000 | 0.0969754900000000 | 1.0 |
| Cl32 | Cl | 0.1627414200000000 | 0.9537028300000000 | 0.8681823300000000 | 1.0 |
| Cl33 | Cl | 0.3769774700000000 | 0.1416993300000000 | 0.0146005100000000 | 1.0 |
| Cl34 | Cl | 0.4127556100000000 | 0.8773863700000000 | 0.9196821000000000 | 1.0 |
| Cl35 | Cl | 0.6349933800000000 | 0.1035498300000000 | 0.0969158200000000 | 1.0 |
| Cl36 | Cl | 0.6627304900000000 | 0.9536580800000000 | 0.8681985500000000 | 1.0 |

##### cif ends

furan\_Cl\_3\_anti\_alt Energy: -220.24925146

##### cif starts

data\_furan\_Cl\_3\_anti\_alt

\_publ\_section\_comment

;

Andrew Reynoso, Bohan Xu, and Vincent H. Crespi

;

\_cell\_length\_a 9.4346369497

\_cell\_length\_b 20.0

\_cell\_length\_c 20.0

\_cell\_angle\_alpha 90.0

\_cell\_angle\_beta 90.0

\_cell\_angle\_gamma 90.0

\_symmetry\_space\_group\_name\_H-M 'P 1'

\_symmetry\_Int\_Tables\_number 1  
\_symmetry\_cell\_setting triclinic

loop\_  
\_atom\_site\_label  
\_atom\_site\_type\_symbol  
\_atom\_site\_fract\_x  
\_atom\_site\_fract\_y  
\_atom\_site\_fract\_z  
\_atom\_site\_occupancy

|      |    |                    |                    |                    |     |
|------|----|--------------------|--------------------|--------------------|-----|
| H1   | H  | 0.0373517900000000 | 0.9074313900000000 | 0.9280331800000000 | 1.0 |
| H2   | H  | 0.0209685700000000 | 0.0659924400000000 | 0.0654945800000000 | 1.0 |
| H3   | H  | 0.0310066400000000 | 0.1116396300000000 | 0.9332325100000000 | 1.0 |
| H4   | H  | 0.2874012300000000 | 0.1117564500000000 | 0.0457865400000000 | 1.0 |
| H5   | H  | 0.2709460300000000 | 0.9531636600000000 | 0.9083605900000000 | 1.0 |
| H6   | H  | 0.2809882200000000 | 0.9075483000000000 | 0.0406337200000000 | 1.0 |
| H7   | H  | 0.5373757400000000 | 0.9074412500000000 | 0.9280122500000000 | 1.0 |
| H8   | H  | 0.5209624000000000 | 0.0659865200000000 | 0.0654926800000000 | 1.0 |
| H9   | H  | 0.5310019600000000 | 0.1116475000000000 | 0.9332361000000000 | 1.0 |
| H10  | H  | 0.7874023300000000 | 0.1117610200000000 | 0.0457965800000000 | 1.0 |
| H11  | H  | 0.7709672200000000 | 0.9531831500000000 | 0.9083561800000000 | 1.0 |
| H12  | H  | 0.7809768900000000 | 0.9075526300000000 | 0.0406267100000000 | 1.0 |
| C13  | C  | 0.0606483300000000 | 0.9551899800000000 | 0.9526543300000000 | 1.0 |
| C14  | C  | 0.9709546300000000 | 0.9685110800000000 | 0.0169298900000000 | 1.0 |
| C15  | C  | 0.9736992400000000 | 0.0470422500000000 | 0.0191768000000000 | 1.0 |
| C16  | C  | 0.0572028300000000 | 0.0636364300000000 | 0.9559745600000000 | 1.0 |
| C17  | C  | 0.3106749600000000 | 0.0639864500000000 | 0.0211834200000000 | 1.0 |
| C18  | C  | 0.2209676600000000 | 0.0506579400000000 | 0.9569112000000000 | 1.0 |
| C19  | C  | 0.2236772100000000 | 0.9721259000000000 | 0.9546747400000000 | 1.0 |
| C20  | C  | 0.3071902200000000 | 0.9555415700000000 | 0.0178750000000000 | 1.0 |
| C21  | C  | 0.5606594200000000 | 0.9551969800000000 | 0.9526421100000000 | 1.0 |
| C22  | C  | 0.4709602700000000 | 0.9685070300000000 | 0.0169190600000000 | 1.0 |
| C23  | C  | 0.4736998200000000 | 0.0470386700000000 | 0.0191724300000000 | 1.0 |
| C24  | C  | 0.5572049700000000 | 0.0636430000000000 | 0.9559736600000000 | 1.0 |
| C25  | C  | 0.8106736300000000 | 0.0639927300000000 | 0.0211892900000000 | 1.0 |
| C26  | C  | 0.7209712400000000 | 0.0506694900000000 | 0.9569144300000000 | 1.0 |
| C27  | C  | 0.7236884200000000 | 0.9721371200000000 | 0.9546705300000000 | 1.0 |
| C28  | C  | 0.8071876800000000 | 0.9555476400000000 | 0.0178747500000000 | 1.0 |
| O29  | O  | 0.0127835100000000 | 0.0095824000000000 | 0.9113840400000000 | 1.0 |
| O30  | O  | 0.2627936400000000 | 0.0096033900000000 | 0.0624624300000000 | 1.0 |
| O31  | O  | 0.5127960400000000 | 0.0095928700000000 | 0.9113763400000000 | 1.0 |
| O32  | O  | 0.7627837300000000 | 0.0096074100000000 | 0.0624633000000000 | 1.0 |
| Cl33 | Cl | 0.0292683100000000 | 0.9240975100000000 | 0.0906904900000000 | 1.0 |
| Cl34 | Cl | 0.2792514900000000 | 0.0950490500000000 | 0.8831341200000000 | 1.0 |
| Cl35 | Cl | 0.5292867700000000 | 0.9240820300000000 | 0.0906703600000000 | 1.0 |
| Cl36 | Cl | 0.7792642900000000 | 0.0950679200000000 | 0.8831428800000000 | 1.0 |

##### cif ends

furand\_Cl3\_anti\_alt\_forbid Energy: -220.84199994

##### cif starts

data\_furand\_Cl3\_anti\_alt\_forbid

\_publ\_section\_comment

;

;

```

_cell_length_a 10.245388043
_cell_length_b 20.0
_cell_length_c 20.0
_cell_angle_alpha 90.0
_cell_angle_beta 90.0
_cell_angle_gamma 90.0

```

```

_symmetry_space_group_name_H-M 'P 1'
_symmetry_Int_Tables_number 1
_symmetry_cell_setting triclinic

```

```

loop_
_atom_site_label
_atom_site_type_symbol
_atom_site_fract_x
_atom_site_fract_y
_atom_site_fract_z
_atom_site_occupancy
H1 H 0.0713748800000000 0.0979697800000000 0.9311951300000000 1.0
H2 H 0.9542898000000000 0.9321492400000000 0.0521655100000000 1.0
H3 H 0.0695461000000000 0.8943863700000000 0.9305721100000000 1.0
H4 H 0.3304251700000000 0.0587955400000000 0.9131433700000000 1.0
H5 H 0.2151751600000000 0.0965634900000000 0.0347493700000000 1.0
H6 H 0.2133544500000000 0.8929844800000000 0.0341175300000000 1.0
H7 H 0.5711174700000000 0.0979334500000000 0.9312080800000000 1.0
H8 H 0.4544069700000000 0.9321117000000000 0.0522905400000000 1.0
H9 H 0.5695564200000000 0.8943480000000000 0.9306735100000000 1.0
H10 H 0.8303837100000000 0.0588841300000000 0.9130576200000000 1.0
H11 H 0.7151734800000000 0.0966368700000000 0.0346675000000000 1.0
H12 H 0.7136561800000000 0.8930546200000000 0.0341072900000000 1.0
C13 C 0.0803792300000000 0.0519546900000000 0.9608982700000000 1.0
C14 C 0.9571927800000000 0.0351604500000000 0.0023219000000000 1.0
C15 C 0.9583506500000000 0.9562778100000000 0.0029927400000000 1.0
C16 C 0.0795269200000000 0.9395351500000000 0.9611099400000000 1.0
C17 C 0.2052116800000000 0.0514218900000000 0.0042032100000000 1.0
C18 C 0.3263893500000000 0.0346827900000000 0.9623237200000000 1.0
C19 C 0.3275726600000000 0.9558000700000000 0.9630144400000000 1.0
C20 C 0.2043641100000000 0.9390037200000000 0.0044180800000000 1.0
C21 C 0.5802839400000000 0.0519350900000000 0.9609250900000000 1.0
C22 C 0.4571933900000000 0.0351114400000000 0.0024162000000000 1.0
C23 C 0.4583850100000000 0.9562303300000000 0.0031086100000000 1.0
C24 C 0.5795269900000000 0.9395151100000000 0.9611829200000000 1.0
C25 C 0.7052235700000000 0.0514746000000000 0.0041482800000000 1.0
C26 C 0.8263748500000000 0.0347558200000000 0.9622318100000000 1.0
C27 C 0.8275502400000000 0.9558753800000000 0.9629020000000000 1.0
C28 C 0.7044679300000000 0.9390549800000000 0.0043957500000000 1.0
O29 O 0.0872949500000000 0.9961760600000000 0.9155201100000000 1.0
O30 O 0.1974277600000000 0.9947834300000000 0.0497931700000000 1.0
O31 O 0.5871371700000000 0.9961408900000000 0.9155633300000000 1.0
O32 O 0.6975988900000000 0.9948466800000000 0.0497601800000000 1.0
Cl33 Cl 0.9539312200000000 0.0801259900000000 0.0792949700000000 1.0
Cl34 Cl 0.3308746100000000 0.9108156200000000 0.8860556400000000 1.0

```



Cl35 Cl 0.4539407900000000 0.0800632000000000 0.0793935700000000 1.0  
Cl36 Cl 0.8307672300000000 0.9109409100000000 0.8859156200000000 1.0

##### cif ends

furandir Energy: -220.14842289

##### cif starts

data\_furandir

\_publ\_section\_comment

;  
Andrew Reynoso, Bohan Xu, and Vincent H. Crespi  
;

\_cell\_length\_a 9.4522460377

\_cell\_length\_b 20.0

\_cell\_length\_c 20.0

\_cell\_angle\_alpha 90.0

\_cell\_angle\_beta 90.0

\_cell\_angle\_gamma 90.0

\_symmetry\_space\_group\_name\_H-M 'P 1'

\_symmetry\_Int\_Tables\_number 1

\_symmetry\_cell\_setting triclinic

loop\_

\_atom\_site\_label

\_atom\_site\_type\_symbol

\_atom\_site\_fract\_x

\_atom\_site\_fract\_y

\_atom\_site\_fract\_z

\_atom\_site\_occupancy

|     |   |                    |                    |                    |     |
|-----|---|--------------------|--------------------|--------------------|-----|
| H1  | H | 0.0063175700000000 | 0.1089888900000000 | 0.9435410700000000 | 1.0 |
| H2  | H | 0.9928134800000000 | 0.9472089400000000 | 0.0762119700000000 | 1.0 |
| H3  | H | 0.0075013600000000 | 0.9047147100000000 | 0.9417886900000000 | 1.0 |
| H4  | H | 0.2562918900000000 | 0.1084314200000000 | 0.0552020900000000 | 1.0 |
| H5  | H | 0.2429453300000000 | 0.9479583300000000 | 0.9209329900000000 | 1.0 |
| H6  | H | 0.2575261100000000 | 0.9041542700000000 | 0.0549369800000000 | 1.0 |
| H7  | H | 0.5062779700000000 | 0.1090875600000000 | 0.9436629500000000 | 1.0 |
| H8  | H | 0.4930327700000000 | 0.9471628500000000 | 0.0761481400000000 | 1.0 |
| H9  | H | 0.5073924600000000 | 0.9048165000000000 | 0.9416552600000000 | 1.0 |
| H10 | H | 0.7562881800000000 | 0.1084664200000000 | 0.0551485300000000 | 1.0 |
| H11 | H | 0.7429103700000000 | 0.9480351500000000 | 0.9208559400000000 | 1.0 |
| H12 | H | 0.7573722500000000 | 0.9041846000000000 | 0.0548635200000000 | 1.0 |
| C13 | C | 0.0302271400000000 | 0.0609448100000000 | 0.9666973500000000 | 1.0 |
| C14 | C | 0.9432410500000000 | 0.0458044100000000 | 0.0299610000000000 | 1.0 |
| C15 | C | 0.9466332600000000 | 0.9672264500000000 | 0.0301035000000000 | 1.0 |
| C16 | C | 0.0329960400000000 | 0.9524489900000000 | 0.9660391100000000 | 1.0 |
| C17 | C | 0.2802282100000000 | 0.0606225700000000 | 0.0315702000000000 | 1.0 |
| C18 | C | 0.1932766000000000 | 0.0461019100000000 | 0.9681415500000000 | 1.0 |
| C19 | C | 0.1966879900000000 | 0.9675264400000000 | 0.9672162800000000 | 1.0 |
| C20 | C | 0.2830054100000000 | 0.9521210100000000 | 0.0311454200000000 | 1.0 |
| C21 | C | 0.5302145800000000 | 0.0610079800000000 | 0.9667409600000000 | 1.0 |
| C22 | C | 0.4432760600000000 | 0.0457943200000000 | 0.0300080100000000 | 1.0 |
| C23 | C | 0.4466973300000000 | 0.9672173100000000 | 0.0300892100000000 | 1.0 |

|      |    |                    |                    |                    |     |
|------|----|--------------------|--------------------|--------------------|-----|
| C24  | C  | 0.5329435000000000 | 0.9525104200000000 | 0.9659707100000000 | 1.0 |
| C25  | C  | 0.7802120700000000 | 0.0606521700000000 | 0.0315210400000000 | 1.0 |
| C26  | C  | 0.6932466600000000 | 0.0461465600000000 | 0.9681069500000000 | 1.0 |
| C27  | C  | 0.6966457200000000 | 0.9675764500000000 | 0.9671494200000000 | 1.0 |
| C28  | C  | 0.7829267200000000 | 0.9521502700000000 | 0.0310904800000000 | 1.0 |
| O29  | O  | 0.9857910300000000 | 0.0066543100000000 | 0.9234487500000000 | 1.0 |
| O30  | O  | 0.2357749700000000 | 0.0058949200000000 | 0.0742637800000000 | 1.0 |
| O31  | O  | 0.4857047900000000 | 0.0067628600000000 | 0.9234535700000000 | 1.0 |
| O32  | O  | 0.7357083900000000 | 0.0059275400000000 | 0.0742078300000000 | 1.0 |
| Cl33 | Cl | 0.0022722300000000 | 0.0883469000000000 | 0.1046202400000000 | 1.0 |
| Cl34 | Cl | 0.2522988100000000 | 0.0894105800000000 | 0.8939213600000000 | 1.0 |
| Cl35 | Cl | 0.5022614700000000 | 0.0882703200000000 | 0.1047115000000000 | 1.0 |
| Cl36 | Cl | 0.7522503200000000 | 0.0894335000000000 | 0.8938755000000000 | 1.0 |

##### cif ends

furan\_Cl\_3\_anti\_dir\_forbid Energy: -220.80079643

##### cif starts

data\_furan\_Cl\_3\_anti\_dir\_forbid

\_publ\_section\_comment

;  
Andrew Reynoso, Bohan Xu, and Vincent H. Crespi  
;

\_cell\_length\_a 10.2442327435

\_cell\_length\_b 20.0

\_cell\_length\_c 20.0

\_cell\_angle\_alpha 90.0

\_cell\_angle\_beta 90.0

\_cell\_angle\_gamma 90.0

\_symmetry\_space\_group\_name\_H-M 'P 1'

\_symmetry\_Int\_Tables\_number 1

\_symmetry\_cell\_setting triclinic

loop\_

\_atom\_site\_label

\_atom\_site\_type\_symbol

\_atom\_site\_fract\_x

\_atom\_site\_fract\_y

\_atom\_site\_fract\_z

\_atom\_site\_occupancy

|     |   |                    |                    |                    |     |
|-----|---|--------------------|--------------------|--------------------|-----|
| H1  | H | 0.0885413900000000 | 0.1042927500000000 | 0.9408421700000000 | 1.0 |
| H2  | H | 0.9684533900000000 | 0.9400264000000000 | 0.0620584700000000 | 1.0 |
| H3  | H | 0.0853604400000000 | 0.9007456000000000 | 0.9406241600000000 | 1.0 |
| H4  | H | 0.2299037900000000 | 0.1034874000000000 | 0.0454754900000000 | 1.0 |
| H5  | H | 0.3499545400000000 | 0.9411317500000000 | 0.9216934800000000 | 1.0 |
| H6  | H | 0.2331052700000000 | 0.8999513100000000 | 0.0425184900000000 | 1.0 |
| H7  | H | 0.5885299200000000 | 0.1042816700000000 | 0.9408183100000000 | 1.0 |
| H8  | H | 0.4684505000000000 | 0.9400305900000000 | 0.0620615500000000 | 1.0 |
| H9  | H | 0.5853649900000000 | 0.9007369800000000 | 0.9406347000000000 | 1.0 |
| H10 | H | 0.7298981500000000 | 0.1035004800000000 | 0.0454515000000000 | 1.0 |
| H11 | H | 0.8499508500000000 | 0.9411237700000000 | 0.9216959700000000 | 1.0 |
| H12 | H | 0.7331074000000000 | 0.8999636200000000 | 0.0425313600000000 | 1.0 |

|      |    |                    |                    |                    |     |
|------|----|--------------------|--------------------|--------------------|-----|
| C13  | C  | 0.0974508100000000 | 0.0586798200000000 | 0.9707256300000000 | 1.0 |
| C14  | C  | 0.9751754800000000 | 0.0425405400000000 | 0.0125262400000000 | 1.0 |
| C15  | C  | 0.9736991600000000 | 0.9636062200000000 | 0.0126681800000000 | 1.0 |
| C16  | C  | 0.0957704700000000 | 0.9462707300000000 | 0.9710160400000000 | 1.0 |
| C17  | C  | 0.2210072200000000 | 0.0583422100000000 | 0.0148880700000000 | 1.0 |
| C18  | C  | 0.3432732100000000 | 0.0428573200000000 | 0.9728322500000000 | 1.0 |
| C19  | C  | 0.3447383700000000 | 0.9639325400000000 | 0.9714497600000000 | 1.0 |
| C20  | C  | 0.2226887200000000 | 0.9459477900000000 | 0.0128445700000000 | 1.0 |
| C21  | C  | 0.5974473800000000 | 0.0586755200000000 | 0.9707117300000000 | 1.0 |
| C22  | C  | 0.4751808500000000 | 0.0425425300000000 | 0.0125238900000000 | 1.0 |
| C23  | C  | 0.4736993300000000 | 0.9636075600000000 | 0.0126698000000000 | 1.0 |
| C24  | C  | 0.5957696300000000 | 0.9462671300000000 | 0.9710200500000000 | 1.0 |
| C25  | C  | 0.7210061300000000 | 0.0583485900000000 | 0.0148726300000000 | 1.0 |
| C26  | C  | 0.8432772200000000 | 0.0428558200000000 | 0.9728245300000000 | 1.0 |
| C27  | C  | 0.8447356700000000 | 0.9639305900000000 | 0.9714491200000000 | 1.0 |
| C28  | C  | 0.7226897100000000 | 0.9459541100000000 | 0.0128484500000000 | 1.0 |
| O29  | O  | 0.1036662000000000 | 0.0024290400000000 | 0.9253729600000000 | 1.0 |
| O30  | O  | 0.2148287600000000 | 0.0013904500000000 | 0.0593576300000000 | 1.0 |
| O31  | O  | 0.6036567100000000 | 0.0024179200000000 | 0.9253683000000000 | 1.0 |
| O32  | O  | 0.7148306400000000 | 0.0014041200000000 | 0.0593522400000000 | 1.0 |
| Cl33 | Cl | 0.9719487400000000 | 0.0877526000000000 | 0.0891978900000000 | 1.0 |
| Cl34 | Cl | 0.3465098000000000 | 0.0892787100000000 | 0.8968886100000000 | 1.0 |
| Cl35 | Cl | 0.4719730900000000 | 0.0877611400000000 | 0.0891933600000000 | 1.0 |
| Cl36 | Cl | 0.8465307600000000 | 0.0892688000000000 | 0.8968765200000000 | 1.0 |

##### cif ends

furand\_Cl\_3\_syn\_alt Energy: -221.2949588

##### cif starts

data\_furand\_Cl\_3\_syn\_alt

\_publ\_section\_comment

;  
Andrew Reynoso, Bohan Xu, and Vincent H. Crespi  
;

\_cell\_length\_a 10.3378460129

\_cell\_length\_b 20.0

\_cell\_length\_c 20.0

\_cell\_angle\_alpha 90.0

\_cell\_angle\_beta 90.0

\_cell\_angle\_gamma 90.0

\_symmetry\_space\_group\_name\_H-M 'P 1'

\_symmetry\_Int\_Tables\_number 1

\_symmetry\_cell\_setting triclinic

loop\_

\_atom\_site\_label

\_atom\_site\_type\_symbol

\_atom\_site\_fract\_x

\_atom\_site\_fract\_y

\_atom\_site\_fract\_z

\_atom\_site\_occupancy

H1 H 0.0257683100000000 0.8959113600000000 0.0426538800000000 1.0

|      |    |                    |                    |                    |     |
|------|----|--------------------|--------------------|--------------------|-----|
| H2   | H  | 0.1507703800000000 | 0.0596679100000000 | 0.9253886400000000 | 1.0 |
| H3   | H  | 0.0258273100000000 | 0.0998491200000000 | 0.0430183300000000 | 1.0 |
| H4   | H  | 0.2758053500000000 | 0.0998812000000000 | 0.0430090300000000 | 1.0 |
| H5   | H  | 0.4007503200000000 | 0.9365047100000000 | 0.9251893300000000 | 1.0 |
| H6   | H  | 0.2758200100000000 | 0.8959503200000000 | 0.0427047100000000 | 1.0 |
| H7   | H  | 0.5257792500000000 | 0.8959358000000000 | 0.0426667800000000 | 1.0 |
| H8   | H  | 0.6507960300000000 | 0.0596799100000000 | 0.9253809100000000 | 1.0 |
| H9   | H  | 0.5258368600000000 | 0.0998748200000000 | 0.0429997600000000 | 1.0 |
| H10  | H  | 0.7758021400000000 | 0.0998607800000000 | 0.0430345600000000 | 1.0 |
| H11  | H  | 0.9007804700000000 | 0.9365104200000000 | 0.9251619600000000 | 1.0 |
| H12  | H  | 0.7758122300000000 | 0.8959325400000000 | 0.0426513200000000 | 1.0 |
| C13  | C  | 0.0247794300000000 | 0.9440337500000000 | 0.0162958800000000 | 1.0 |
| C14  | C  | 0.1508199300000000 | 0.9587515400000000 | 0.9756663300000000 | 1.0 |
| C15  | C  | 0.1508096300000000 | 0.0374646300000000 | 0.9753266200000000 | 1.0 |
| C16  | C  | 0.0268435900000000 | 0.0518254300000000 | 0.0164933000000000 | 1.0 |
| C17  | C  | 0.2747896100000000 | 0.0518501500000000 | 0.0164878400000000 | 1.0 |
| C18  | C  | 0.4008071600000000 | 0.0372687700000000 | 0.9757868800000000 | 1.0 |
| C19  | C  | 0.4007983200000000 | 0.9585584000000000 | 0.9751957900000000 | 1.0 |
| C20  | C  | 0.2768416700000000 | 0.9440578400000000 | 0.0163316000000000 | 1.0 |
| C21  | C  | 0.5247863200000000 | 0.9440540200000000 | 0.0163028500000000 | 1.0 |
| C22  | C  | 0.6508090700000000 | 0.9587743700000000 | 0.9756474600000000 | 1.0 |
| C23  | C  | 0.6508100200000000 | 0.0374837500000000 | 0.9753232800000000 | 1.0 |
| C24  | C  | 0.5268421400000000 | 0.0518477100000000 | 0.0164837800000000 | 1.0 |
| C25  | C  | 0.7747921500000000 | 0.0518428200000000 | 0.0164891000000000 | 1.0 |
| C26  | C  | 0.9008148000000000 | 0.0372617500000000 | 0.9757858300000000 | 1.0 |
| C27  | C  | 0.9008078900000000 | 0.9585499800000000 | 0.9751760900000000 | 1.0 |
| C28  | C  | 0.7768398900000000 | 0.9440490900000000 | 0.0162957000000000 | 1.0 |
| O29  | O  | 0.0258160600000000 | 0.9978405100000000 | 0.0640357400000000 | 1.0 |
| O30  | O  | 0.2758282100000000 | 0.9978866900000000 | 0.0640498400000000 | 1.0 |
| O31  | O  | 0.5258306300000000 | 0.9978723500000000 | 0.0640350600000000 | 1.0 |
| O32  | O  | 0.7758315800000000 | 0.9978627400000000 | 0.0640316000000000 | 1.0 |
| Cl33 | Cl | 0.1508853200000000 | 0.9181275000000000 | 0.8959130500000000 | 1.0 |
| Cl34 | Cl | 0.4008101900000000 | 0.0781397200000000 | 0.8961590700000000 | 1.0 |
| Cl35 | Cl | 0.6508094400000000 | 0.9182052000000000 | 0.8958658100000000 | 1.0 |
| Cl36 | Cl | 0.9008537300000000 | 0.0781561100000000 | 0.8961696800000000 | 1.0 |

##### cif ends

furran\_Cl\_3\_syn\_alt\_forbid Energy: -218.36472487

##### cif starts

data\_furran\_Cl\_3\_syn\_alt\_forbid

\_publ\_section\_comment

;  
Andrew Reynoso, Bohan Xu, and Vincent H. Crespi  
;

\_cell\_length\_a 9.5995830775

\_cell\_length\_b 20.0

\_cell\_length\_c 20.0

\_cell\_angle\_alpha 90.0

\_cell\_angle\_beta 90.0

\_cell\_angle\_gamma 90.0

\_symmetry\_space\_group\_name\_H-M 'P 1'

\_symmetry\_Int\_Tables\_number 1  
\_symmetry\_cell\_setting triclinic

loop\_  
\_atom\_site\_label  
\_atom\_site\_type\_symbol  
\_atom\_site\_fract\_x  
\_atom\_site\_fract\_y  
\_atom\_site\_fract\_z  
\_atom\_site\_occupancy

|      |    |                    |                    |                    |     |
|------|----|--------------------|--------------------|--------------------|-----|
| H1   | H  | 0.8997220500000000 | 0.0983854700000000 | 0.0672408200000000 | 1.0 |
| H2   | H  | 0.9027285600000000 | 0.0629145800000000 | 0.9317013700000000 | 1.0 |
| H3   | H  | 0.8955587100000000 | 0.8960087300000000 | 0.0628463700000000 | 1.0 |
| H4   | H  | 0.1576113500000000 | 0.1006814300000000 | 0.0667594600000000 | 1.0 |
| H5   | H  | 0.1505247400000000 | 0.9388835600000000 | 0.9293509800000000 | 1.0 |
| H6   | H  | 0.1536287500000000 | 0.8982841400000000 | 0.0634373100000000 | 1.0 |
| H7   | H  | 0.3996191500000000 | 0.0983817800000000 | 0.0673043000000000 | 1.0 |
| H8   | H  | 0.4027276100000000 | 0.0629978200000000 | 0.9317471800000000 | 1.0 |
| H9   | H  | 0.3956438200000000 | 0.8960081100000000 | 0.0627926400000000 | 1.0 |
| H10  | H  | 0.6577166300000000 | 0.1007210300000000 | 0.0667750500000000 | 1.0 |
| H11  | H  | 0.6505544300000000 | 0.9389508300000000 | 0.9293461200000000 | 1.0 |
| H12  | H  | 0.6535401000000000 | 0.8983254400000000 | 0.0634323600000000 | 1.0 |
| C13  | C  | 0.8623133500000000 | 0.0537586300000000 | 0.0408580200000000 | 1.0 |
| C14  | C  | 0.9428579100000000 | 0.0385294100000000 | 0.9764571800000000 | 1.0 |
| C15  | C  | 0.9450374400000000 | 0.9603095800000000 | 0.9752226400000000 | 1.0 |
| C16  | C  | 0.8605172300000000 | 0.9424392400000000 | 0.0389249900000000 | 1.0 |
| C17  | C  | 0.1926986800000000 | 0.0552011200000000 | 0.0410890000000000 | 1.0 |
| C18  | C  | 0.1081967900000000 | 0.0397610800000000 | 0.9767471000000000 | 1.0 |
| C19  | C  | 0.1103761200000000 | 0.9615495800000000 | 0.9749981500000000 | 1.0 |
| C20  | C  | 0.1909693500000000 | 0.9438920300000000 | 0.0387667900000000 | 1.0 |
| C21  | C  | 0.3622803600000000 | 0.0537608200000000 | 0.0408875000000000 | 1.0 |
| C22  | C  | 0.4428607600000000 | 0.0385833100000000 | 0.9764861100000000 | 1.0 |
| C23  | C  | 0.4450446300000000 | 0.9603643100000000 | 0.9752049500000000 | 1.0 |
| C24  | C  | 0.3605455400000000 | 0.9424438000000000 | 0.0389003900000000 | 1.0 |
| C25  | C  | 0.6927387100000000 | 0.0552343700000000 | 0.0410968500000000 | 1.0 |
| C26  | C  | 0.6081993300000000 | 0.0398158800000000 | 0.9767671300000000 | 1.0 |
| C27  | C  | 0.6103817600000000 | 0.9616048000000000 | 0.9749927600000000 | 1.0 |
| C28  | C  | 0.6909377600000000 | 0.9439267900000000 | 0.0387700200000000 | 1.0 |
| O29  | O  | 0.8956683000000000 | 0.9967799900000000 | 0.0817981400000000 | 1.0 |
| O30  | O  | 0.1576204200000000 | 0.9992572900000000 | 0.0818621300000000 | 1.0 |
| O31  | O  | 0.3956613700000000 | 0.9967677600000000 | 0.0818014500000000 | 1.0 |
| O32  | O  | 0.6576295500000000 | 0.9992949000000000 | 0.0818689700000000 | 1.0 |
| Cl33 | Cl | 0.8896383600000000 | 0.9170402700000000 | 0.9010190400000000 | 1.0 |
| Cl34 | Cl | 0.1635854500000000 | 0.0858434700000000 | 0.9042559300000000 | 1.0 |
| Cl35 | Cl | 0.3896659300000000 | 0.9171529200000000 | 0.9009658700000000 | 1.0 |
| Cl36 | Cl | 0.6635741600000000 | 0.0859251200000000 | 0.9042894300000000 | 1.0 |

##### cif ends

furandCl3\_syn\_dir Energy: -218.91292387

##### cif starts

data\_furandCl3\_syn\_dir

\_publ\_section\_comment

;

;

```

_cell_length_a 10.3997828912
_cell_length_b 20.0
_cell_length_c 20.0
_cell_angle_alpha 90.0
_cell_angle_beta 90.0
_cell_angle_gamma 90.0

```

```

_symmetry_space_group_name_H-M 'P 1'
_symmetry_Int_Tables_number 1
_symmetry_cell_setting triclinic

```

```

loop_
_atom_site_label
_atom_site_type_symbol
_atom_site_fract_x
_atom_site_fract_y
_atom_site_fract_z
_atom_site_occupancy
H1 H 0.0689036500000000 0.0877289900000000 0.0691849800000000 1.0
H2 H 0.1830429700000000 0.9344653700000000 0.9311724100000000 1.0
H3 H 0.0293108000000000 0.8889101700000000 0.0318381700000000 1.0
H4 H 0.2984299700000000 0.1063118800000000 0.0286496600000000 1.0
H5 H 0.4191797300000000 0.9250720800000000 0.9386101700000000 1.0
H6 H 0.2906508100000000 0.9047355200000000 0.0609893100000000 1.0
H7 H 0.5397552900000000 0.1063328800000000 0.0287080600000000 1.0
H8 H 0.6553960800000000 0.9345663200000000 0.9311630800000000 1.0
H9 H 0.5477749300000000 0.9047474600000000 0.0609570100000000 1.0
H10 H 0.7695853800000000 0.0878413000000000 0.0691597400000000 1.0
H11 H 0.9190880900000000 0.9587169700000000 0.9219413700000000 1.0
H12 H 0.8089387800000000 0.8889893000000000 0.0319248100000000 1.0
C13 C 0.0497625100000000 0.0458461200000000 0.0354044100000000 1.0
C14 C 0.1638026100000000 0.0339233800000000 0.9793027100000000 1.0
C15 C 0.1713570900000000 0.9562413100000000 0.9811060500000000 1.0
C16 C 0.0412206200000000 0.9406729300000000 0.0145612100000000 1.0
C17 C 0.2949763800000000 0.0546002800000000 0.0105035400000000 1.0
C18 C 0.4191602100000000 0.0324840900000000 0.9713832300000000 1.0
C19 C 0.4191784000000000 0.9546560400000000 0.9848142700000000 1.0
C20 C 0.2932644500000000 0.9473746300000000 0.0264906200000000 1.0
C21 C 0.5433059200000000 0.0546306500000000 0.0105399900000000 1.0
C22 C 0.6745282700000000 0.0340119300000000 0.9793388600000000 1.0
C23 C 0.6670157400000000 0.9563209500000000 0.9811104900000000 1.0
C24 C 0.5450971200000000 0.9474000000000000 0.0264784600000000 1.0
C25 C 0.7886284100000000 0.0459249200000000 0.0354047100000000 1.0
C26 C 0.9192008800000000 0.0465920800000000 0.9993396400000000 1.0
C27 C 0.9191600800000000 0.9677376500000000 0.9759155000000000 1.0
C28 C 0.7971000900000000 0.9407396800000000 0.0146024200000000 1.0
O29 O 0.0482350000000000 0.9845268600000000 0.0715841000000000 1.0
O30 O 0.2949631700000000 0.0087721200000000 0.0655815500000000 1.0
O31 O 0.5433377700000000 0.0087789300000000 0.0655959800000000 1.0
O32 O 0.7901014700000000 0.9846230100000000 0.0716071800000000 1.0
Cl33 Cl 0.1309729400000000 0.0601927100000000 0.8956581400000000 1.0
Cl34 Cl 0.4191473100000000 0.0569056700000000 0.8859528800000000 1.0

```

Cl35 Cl 0.7072800600000000 0.0603818000000000 0.8957232500000000 1.0  
Cl36 Cl 0.9193020100000000 0.1293299900000000 0.9598866500000000 1.0

##### cif ends

furandirforbid Energy: -216.43683922

##### cif starts

data\_furandirforbid

\_publ\_section\_comment

;  
Andrew Reynoso, Bohan Xu, and Vincent H. Crespi  
;

\_cell\_length\_a 9.4466564225

\_cell\_length\_b 20.0

\_cell\_length\_c 20.0

\_cell\_angle\_alpha 90.0

\_cell\_angle\_beta 90.0

\_cell\_angle\_gamma 90.0

\_symmetry\_space\_group\_name\_H-M 'P 1'

\_symmetry\_Int\_Tables\_number 1

\_symmetry\_cell\_setting triclinic

loop\_

\_atom\_site\_label

\_atom\_site\_type\_symbol

\_atom\_site\_fract\_x

\_atom\_site\_fract\_y

\_atom\_site\_fract\_z

\_atom\_site\_occupancy

|     |   |                    |                    |                    |     |
|-----|---|--------------------|--------------------|--------------------|-----|
| H1  | H | 0.8624188700000000 | 0.1271814800000000 | 0.0505630700000000 | 1.0 |
| H2  | H | 0.8889243600000000 | 0.9572934800000000 | 0.9328145700000000 | 1.0 |
| H3  | H | 0.9188448500000000 | 0.9275615400000000 | 0.0745231200000000 | 1.0 |
| H4  | H | 0.1784617400000000 | 0.0724908800000000 | 0.1013513800000000 | 1.0 |
| H5  | H | 0.1417316200000000 | 0.9659052600000000 | 0.9167164700000000 | 1.0 |
| H6  | H | 0.1335949500000000 | 0.8848198000000000 | 0.0279707600000000 | 1.0 |
| H7  | H | 0.4164057200000000 | 0.0749485300000000 | 0.0656235300000000 | 1.0 |
| H8  | H | 0.4303043800000000 | 0.9118975000000000 | 0.9280079700000000 | 1.0 |
| H9  | H | 0.3716588100000000 | 0.8737424600000000 | 0.0571783300000000 | 1.0 |
| H10 | H | 0.6234241700000000 | 0.1121399000000000 | 0.0266927300000000 | 1.0 |
| H11 | H | 0.6785435000000000 | 0.9168702900000000 | 0.9479044900000000 | 1.0 |
| H12 | H | 0.6738806300000000 | 0.9207164900000000 | 0.0889303400000000 | 1.0 |
| C13 | C | 0.8465474500000000 | 0.0768158200000000 | 0.0301968700000000 | 1.0 |
| C14 | C | 0.9519298100000000 | 0.0569495300000000 | 0.9766637100000000 | 1.0 |
| C15 | C | 0.9437541500000000 | 0.9794647700000000 | 0.9756277800000000 | 1.0 |
| C16 | C | 0.8683220700000000 | 0.9669334800000000 | 0.0449613200000000 | 1.0 |
| C17 | C | 0.1931970800000000 | 0.0374898000000000 | 0.0598673700000000 | 1.0 |
| C18 | C | 0.1146971500000000 | 0.0528544400000000 | 0.9948814000000000 | 1.0 |
| C19 | C | 0.1117929100000000 | 0.9759367700000000 | 0.9684286000000000 | 1.0 |
| C20 | C | 0.1862011200000000 | 0.9336922500000000 | 0.0235299600000000 | 1.0 |
| C21 | C | 0.3635418900000000 | 0.0322211700000000 | 0.0425817100000000 | 1.0 |
| C22 | C | 0.4338123000000000 | 0.0152866500000000 | 0.9687591400000000 | 1.0 |
| C23 | C | 0.4527110900000000 | 0.9386029200000000 | 0.9746869700000000 | 1.0 |

|      |    |                    |                    |                    |     |
|------|----|--------------------|--------------------|--------------------|-----|
| C24  | C  | 0.3552029300000000 | 0.9224153900000000 | 0.0329369100000000 | 1.0 |
| C25  | C  | 0.6784368800000000 | 0.0643399300000000 | 0.0193897000000000 | 1.0 |
| C26  | C  | 0.6058209600000000 | 0.0231744500000000 | 0.9622212000000000 | 1.0 |
| C27  | C  | 0.6196682800000000 | 0.9481958800000000 | 0.9832204200000000 | 1.0 |
| C28  | C  | 0.6975121800000000 | 0.9575291500000000 | 0.0498932100000000 | 1.0 |
| O29  | O  | 0.8897822400000000 | 0.0293597200000000 | 0.0800118000000000 | 1.0 |
| O30  | O  | 0.1515937900000000 | 0.9727614600000000 | 0.0816044600000000 | 1.0 |
| O31  | O  | 0.3989995300000000 | 0.9731393400000000 | 0.0789930400000000 | 1.0 |
| O32  | O  | 0.6455820100000000 | 0.0211420400000000 | 0.0739401700000000 | 1.0 |
| Cl33 | Cl | 0.9411111100000000 | 0.0996269500000000 | 0.8986274900000000 | 1.0 |
| Cl34 | Cl | 0.1967629200000000 | 0.1333585000000000 | 0.9749405000000000 | 1.0 |
| Cl35 | Cl | 0.3527894800000000 | 0.0385556200000000 | 0.8916788700000000 | 1.0 |
| Cl36 | Cl | 0.6568270500000000 | 0.0371212500000000 | 0.8786251100000000 | 1.0 |

##### cif ends

  furan\_F\_23\_anti\_alt   Energy: -229.33016416

##### cif starts

data\_furan\_F\_23\_anti\_alt

\_publ\_section\_comment

;  
Andrew Reynoso, Bohan Xu, and Vincent H. Crespi  
;

\_cell\_length\_a 9.3312422417

\_cell\_length\_b 20.0

\_cell\_length\_c 20.0

\_cell\_angle\_alpha 90.0

\_cell\_angle\_beta 90.0

\_cell\_angle\_gamma 90.0

\_symmetry\_space\_group\_name\_H-M 'P 1'

\_symmetry\_Int\_Tables\_number 1

\_symmetry\_cell\_setting triclinic

loop\_

\_atom\_site\_label

\_atom\_site\_type\_symbol

\_atom\_site\_fract\_x

\_atom\_site\_fract\_y

\_atom\_site\_fract\_z

\_atom\_site\_occupancy

|    |   |                    |                    |                    |     |
|----|---|--------------------|--------------------|--------------------|-----|
| H1 | H | 0.0263391900000000 | 0.9018776500000000 | 0.9364120200000000 | 1.0 |
|----|---|--------------------|--------------------|--------------------|-----|

|    |   |                    |                    |                    |     |
|----|---|--------------------|--------------------|--------------------|-----|
| H2 | H | 0.0141875900000000 | 0.9374022400000000 | 0.0729927700000000 | 1.0 |
|----|---|--------------------|--------------------|--------------------|-----|

|    |   |                    |                    |                    |     |
|----|---|--------------------|--------------------|--------------------|-----|
| H3 | H | 0.2763383700000000 | 0.0981230000000000 | 0.0635883000000000 | 1.0 |
|----|---|--------------------|--------------------|--------------------|-----|

|    |   |                    |                    |                    |     |
|----|---|--------------------|--------------------|--------------------|-----|
| H4 | H | 0.2641867200000000 | 0.0625974800000000 | 0.9270081500000000 | 1.0 |
|----|---|--------------------|--------------------|--------------------|-----|

|    |   |                    |                    |                    |     |
|----|---|--------------------|--------------------|--------------------|-----|
| H5 | H | 0.5263318400000000 | 0.9018793000000000 | 0.9364103400000000 | 1.0 |
|----|---|--------------------|--------------------|--------------------|-----|

|    |   |                    |                    |                    |     |
|----|---|--------------------|--------------------|--------------------|-----|
| H6 | H | 0.5141902300000000 | 0.9374038400000000 | 0.0729913700000000 | 1.0 |
|----|---|--------------------|--------------------|--------------------|-----|

|    |   |                    |                    |                    |     |
|----|---|--------------------|--------------------|--------------------|-----|
| H7 | H | 0.7763349300000000 | 0.0981210000000000 | 0.0635874600000000 | 1.0 |
|----|---|--------------------|--------------------|--------------------|-----|

|    |   |                    |                    |                    |     |
|----|---|--------------------|--------------------|--------------------|-----|
| H8 | H | 0.7641913300000000 | 0.0625952500000000 | 0.9270066000000000 | 1.0 |
|----|---|--------------------|--------------------|--------------------|-----|

|    |   |                    |                    |                    |     |
|----|---|--------------------|--------------------|--------------------|-----|
| C9 | C | 0.9664447000000000 | 0.9600573100000000 | 0.0283532500000000 | 1.0 |
|----|---|--------------------|--------------------|--------------------|-----|

|     |   |                    |                    |                    |     |
|-----|---|--------------------|--------------------|--------------------|-----|
| C10 | C | 0.9637019800000000 | 0.0378751100000000 | 0.0318789100000000 | 1.0 |
|-----|---|--------------------|--------------------|--------------------|-----|

|     |   |                    |                    |                    |     |
|-----|---|--------------------|--------------------|--------------------|-----|
| C11 | C | 0.0525623100000000 | 0.0555977000000000 | 0.9684814600000000 | 1.0 |
|-----|---|--------------------|--------------------|--------------------|-----|

|     |   |                    |                    |                    |     |
|-----|---|--------------------|--------------------|--------------------|-----|
| C12 | C | 0.0495408100000000 | 0.9481316000000000 | 0.9633445000000000 | 1.0 |
|-----|---|--------------------|--------------------|--------------------|-----|



|     |   |                    |                    |                    |     |
|-----|---|--------------------|--------------------|--------------------|-----|
| C13 | C | 0.2995405700000000 | 0.0518694700000000 | 0.0366566800000000 | 1.0 |
| C14 | C | 0.2164434200000000 | 0.0399428100000000 | 0.9716477100000000 | 1.0 |
| C15 | C | 0.2137027600000000 | 0.9621252100000000 | 0.9681219300000000 | 1.0 |
| C16 | C | 0.3025650900000000 | 0.9444033600000000 | 0.0315194000000000 | 1.0 |
| C17 | C | 0.5495382000000000 | 0.9481323000000000 | 0.9633428600000000 | 1.0 |
| C18 | C | 0.4664449600000000 | 0.9600588500000000 | 0.0283523700000000 | 1.0 |
| C19 | C | 0.4637037000000000 | 0.0378764200000000 | 0.0318779900000000 | 1.0 |
| C20 | C | 0.5525662800000000 | 0.0555978400000000 | 0.9684803700000000 | 1.0 |
| C21 | C | 0.7995395100000000 | 0.0518671600000000 | 0.0366559600000000 | 1.0 |
| C22 | C | 0.7164466200000000 | 0.0399408500000000 | 0.9716464200000000 | 1.0 |
| C23 | C | 0.7137019100000000 | 0.9621231500000000 | 0.9681215600000000 | 1.0 |
| C24 | C | 0.8025626800000000 | 0.9444014500000000 | 0.0315194300000000 | 1.0 |
| O25 | O | 0.5062018100000000 | 0.0052944200000000 | 0.9226227000000000 | 1.0 |
| O26 | O | 0.2562029900000000 | 0.9947076600000000 | 0.0773771800000000 | 1.0 |
| O27 | O | 0.0062012400000000 | 0.0052927500000000 | 0.9226238200000000 | 1.0 |
| O28 | O | 0.7562002200000000 | 0.9947059400000000 | 0.0773765700000000 | 1.0 |
| F29 | F | 0.0222296400000000 | 0.0665010300000000 | 0.0896145500000000 | 1.0 |
| F30 | F | 0.0237857900000000 | 0.1179318800000000 | 0.9430861700000000 | 1.0 |
| F31 | F | 0.7737889400000000 | 0.8820668200000000 | 0.0569142800000000 | 1.0 |
| F32 | F | 0.7722313000000000 | 0.9334964800000000 | 0.9103869600000000 | 1.0 |
| F33 | F | 0.5222320000000000 | 0.0665020300000000 | 0.0896137100000000 | 1.0 |
| F34 | F | 0.5237942300000000 | 0.1179330000000000 | 0.9430866600000000 | 1.0 |
| F35 | F | 0.2722310600000000 | 0.9334994900000000 | 0.9103861300000000 | 1.0 |
| F36 | F | 0.2737900900000000 | 0.8820691600000000 | 0.0569144400000000 | 1.0 |

##### cif ends

furan\_F\_23\_anti\_alt\_forbid Energy: -229.29114667

##### cif starts

data\_furan\_F\_23\_anti\_alt\_forbid

\_publ\_section\_comment

;  
Andrew Reynoso, Bohan Xu, and Vincent H. Crespi  
;

\_cell\_length\_a 10.1989264836

\_cell\_length\_b 20.0

\_cell\_length\_c 20.0

\_cell\_angle\_alpha 90.0

\_cell\_angle\_beta 90.0

\_cell\_angle\_gamma 90.0

\_symmetry\_space\_group\_name\_H-M 'P 1'

\_symmetry\_Int\_Tables\_number 1

\_symmetry\_cell\_setting triclinic

loop\_

\_atom\_site\_label

\_atom\_site\_type\_symbol

\_atom\_site\_fract\_x

\_atom\_site\_fract\_y

\_atom\_site\_fract\_z

\_atom\_site\_occupancy

H1 H 0.9546862000000000 0.9326296600000000 0.0572139600000000 1.0

|     |   |                    |                    |                    |     |
|-----|---|--------------------|--------------------|--------------------|-----|
| H2  | H | 0.0708166200000000 | 0.8943235300000000 | 0.9351447700000000 | 1.0 |
| H3  | H | 0.3305313200000000 | 0.0599809800000000 | 0.9174615100000000 | 1.0 |
| H4  | H | 0.2143673000000000 | 0.0982712200000000 | 0.0395296000000000 | 1.0 |
| H5  | H | 0.4548833300000000 | 0.9325259800000000 | 0.0573420200000000 | 1.0 |
| H6  | H | 0.5707977000000000 | 0.8943066600000000 | 0.9351843300000000 | 1.0 |
| H7  | H | 0.8303396900000000 | 0.0600947300000000 | 0.9173515900000000 | 1.0 |
| H8  | H | 0.7143968100000000 | 0.0982970400000000 | 0.0395115500000000 | 1.0 |
| C9  | C | 0.0814447600000000 | 0.0517048900000000 | 0.9651684800000000 | 1.0 |
| C10 | C | 0.9573365100000000 | 0.0353150400000000 | 0.0063839500000000 | 1.0 |
| C11 | C | 0.9578954200000000 | 0.9568992600000000 | 0.0081429100000000 | 1.0 |
| C12 | C | 0.0784813700000000 | 0.9396654200000000 | 0.9655627200000000 | 1.0 |
| C13 | C | 0.2067266100000000 | 0.0529373500000000 | 0.0091013500000000 | 1.0 |
| C14 | C | 0.3273234100000000 | 0.0357109100000000 | 0.9665329700000000 | 1.0 |
| C15 | C | 0.3278901300000000 | 0.9572969500000000 | 0.9682967900000000 | 1.0 |
| C16 | C | 0.2037654100000000 | 0.9409026100000000 | 0.0094947500000000 | 1.0 |
| C17 | C | 0.5813301400000000 | 0.0516868700000000 | 0.9652585200000000 | 1.0 |
| C18 | C | 0.4573444600000000 | 0.0352321400000000 | 0.0065394100000000 | 1.0 |
| C19 | C | 0.4579464800000000 | 0.9568169700000000 | 0.0082782200000000 | 1.0 |
| C20 | C | 0.5784632100000000 | 0.9396448700000000 | 0.9656102000000000 | 1.0 |
| C21 | C | 0.7067492900000000 | 0.0529648200000000 | 0.0090766600000000 | 1.0 |
| C22 | C | 0.8272691400000000 | 0.0357998500000000 | 0.9664121500000000 | 1.0 |
| C23 | C | 0.8278718400000000 | 0.9573874500000000 | 0.9681452400000000 | 1.0 |
| C24 | C | 0.7038878800000000 | 0.9409276400000000 | 0.0094244500000000 | 1.0 |
| O25 | O | 0.0899927400000000 | 0.9964850900000000 | 0.9203980000000000 | 1.0 |
| O26 | O | 0.1952019200000000 | 0.9961188200000000 | 0.0542623500000000 | 1.0 |
| O27 | O | 0.5897887100000000 | 0.9964855200000000 | 0.9204614100000000 | 1.0 |
| O28 | O | 0.6954216800000000 | 0.9961233400000000 | 0.0542214400000000 | 1.0 |
| F29 | F | 0.0716260600000000 | 0.1090380600000000 | 0.9273957700000000 | 1.0 |
| F30 | F | 0.9549340500000000 | 0.0708023500000000 | 0.0660535900000000 | 1.0 |
| F31 | F | 0.3303310700000000 | 0.9218005100000000 | 0.9086331500000000 | 1.0 |
| F32 | F | 0.2135932300000000 | 0.8835747400000000 | 0.0472674700000000 | 1.0 |
| F33 | F | 0.5712675700000000 | 0.1090330300000000 | 0.9275160900000000 | 1.0 |
| F34 | F | 0.4549283600000000 | 0.0706887500000000 | 0.0662239300000000 | 1.0 |
| F35 | F | 0.8302902900000000 | 0.9219348700000000 | 0.9084576200000000 | 1.0 |
| F36 | F | 0.7139726300000000 | 0.8835899200000000 | 0.0471693300000000 | 1.0 |

##### cif ends

furand\_F\_23\_anti\_dir    Energy: -228.3147788

##### cif starts

data\_furand\_F\_23\_anti\_dir

\_publ\_section\_comment

;  
Andrew Reynoso, Bohan Xu, and Vincent H. Crespi  
;

\_cell\_length\_a    9.4332712746

\_cell\_length\_b    20.0

\_cell\_length\_c    20.0

\_cell\_angle\_alpha    90.0

\_cell\_angle\_beta    90.0

\_cell\_angle\_gamma    90.0

\_symmetry\_space\_group\_name\_H-M    'P 1'

\_symmetry\_Int\_Tables\_number 1  
\_symmetry\_cell\_setting triclinic

loop\_  
\_atom\_site\_label  
\_atom\_site\_type\_symbol  
\_atom\_site\_fract\_x  
\_atom\_site\_fract\_y  
\_atom\_site\_fract\_z  
\_atom\_site\_occupancy

|     |   |                    |                    |                    |     |
|-----|---|--------------------|--------------------|--------------------|-----|
| H1  | H | 0.1383603000000000 | 0.1041370400000000 | 0.9412000100000000 | 1.0 |
| H2  | H | 0.1255436800000000 | 0.0605251700000000 | 0.0761283200000000 | 1.0 |
| H3  | H | 0.3883745700000000 | 0.1041402500000000 | 0.0587944100000000 | 1.0 |
| H4  | H | 0.3755491700000000 | 0.0605172100000000 | 0.9238700200000000 | 1.0 |
| H5  | H | 0.6383644200000000 | 0.1041273800000000 | 0.9411887400000000 | 1.0 |
| H6  | H | 0.6255644200000000 | 0.0605176900000000 | 0.0761193700000000 | 1.0 |
| H7  | H | 0.8883490100000000 | 0.1041415000000000 | 0.0587865200000000 | 1.0 |
| H8  | H | 0.8755578100000000 | 0.0605049400000000 | 0.9238645700000000 | 1.0 |
| C9  | C | 0.0767143600000000 | 0.0417523300000000 | 0.0300500900000000 | 1.0 |
| C10 | C | 0.0752556800000000 | 0.9640714500000000 | 0.0299893600000000 | 1.0 |
| C11 | C | 0.1615991100000000 | 0.9485028600000000 | 0.9662775700000000 | 1.0 |
| C12 | C | 0.1627949100000000 | 0.0565820800000000 | 0.9659232400000000 | 1.0 |
| C13 | C | 0.4128012500000000 | 0.0565839700000000 | 0.0340745200000000 | 1.0 |
| C14 | C | 0.3267186500000000 | 0.0417497000000000 | 0.9699481200000000 | 1.0 |
| C15 | C | 0.3252548900000000 | 0.9640679800000000 | 0.9700175900000000 | 1.0 |
| C16 | C | 0.4116004000000000 | 0.9485033800000000 | 0.0337297100000000 | 1.0 |
| C17 | C | 0.6627983400000000 | 0.0565747700000000 | 0.9659143000000000 | 1.0 |
| C18 | C | 0.5767232500000000 | 0.0417477200000000 | 0.0300450200000000 | 1.0 |
| C19 | C | 0.5752556300000000 | 0.9640664800000000 | 0.0299834100000000 | 1.0 |
| C20 | C | 0.6615996000000000 | 0.9484950500000000 | 0.9662736700000000 | 1.0 |
| C21 | C | 0.9127910600000000 | 0.0565831900000000 | 0.0340716100000000 | 1.0 |
| C22 | C | 0.8267197000000000 | 0.0417415600000000 | 0.9699444000000000 | 1.0 |
| C23 | C | 0.8252566200000000 | 0.9640600400000000 | 0.9700192600000000 | 1.0 |
| C24 | C | 0.9115994200000000 | 0.9485039100000000 | 0.0337346000000000 | 1.0 |
| O25 | O | 0.6183426700000000 | 0.0022647600000000 | 0.9225093100000000 | 1.0 |
| O26 | O | 0.3683446000000000 | 0.0022795300000000 | 0.0774869700000000 | 1.0 |
| O27 | O | 0.1183378700000000 | 0.0022741500000000 | 0.9225154800000000 | 1.0 |
| O28 | O | 0.8683343900000000 | 0.0022815200000000 | 0.0774871200000000 | 1.0 |
| F29 | F | 0.1299610100000000 | 0.9343224200000000 | 0.0869443200000000 | 1.0 |
| F30 | F | 0.1364121900000000 | 0.8878622100000000 | 0.9387991900000000 | 1.0 |
| F31 | F | 0.8864198500000000 | 0.8878680700000000 | 0.0612260200000000 | 1.0 |
| F32 | F | 0.8799656900000000 | 0.9342993600000000 | 0.9130713600000000 | 1.0 |
| F33 | F | 0.6299581700000000 | 0.9343161000000000 | 0.0869390800000000 | 1.0 |
| F34 | F | 0.6364113600000000 | 0.8878541000000000 | 0.9387951400000000 | 1.0 |
| F35 | F | 0.3799545600000000 | 0.9343117600000000 | 0.9130655900000000 | 1.0 |
| F36 | F | 0.3864124200000000 | 0.8878663600000000 | 0.0612139700000000 | 1.0 |

##### cif ends

uran\_F\_23\_anti\_dir\_forbid Energy: -228.27213818

##### cif starts

data\_uran\_F\_23\_anti\_dir\_forbid

\_publ\_section\_comment

;

;

```

_cell_length_a 10.2736618852
_cell_length_b 20.0
_cell_length_c 20.0
_cell_angle_alpha 90.0
_cell_angle_beta 90.0
_cell_angle_gamma 90.0

_symmetry_space_group_name_H-M 'P 1'
_symmetry_Int_Tables_number 1
_symmetry_cell_setting triclinic

```

```

loop_
_atom_site_label
_atom_site_type_symbol
_atom_site_fract_x
_atom_site_fract_y
_atom_site_fract_z
_atom_site_occupancy
H1 H 0.0115138400000000 0.1055310300000000 0.9410528900000000 1.0
H2 H 0.8942202300000000 0.0654156200000000 0.0628994300000000 1.0
H3 H 0.1534211800000000 0.1046378200000000 0.0458730400000000 1.0
H4 H 0.2705938500000000 0.0667042100000000 0.9232671900000000 1.0
H5 H 0.5117134700000000 0.1052942200000000 0.9406198500000000 1.0
H6 H 0.3946115200000000 0.0657736800000000 0.0627591400000000 1.0
H7 H 0.6536186900000000 0.1048917600000000 0.0454425700000000 1.0
H8 H 0.7709938800000000 0.0663091100000000 0.9231405100000000 1.0
C9 C 0.0198947800000000 0.0600536900000000 0.9715967100000000 1.0
C10 C 0.8975237600000000 0.0428857600000000 0.0129530700000000 1.0
C11 C 0.8981056500000000 0.9644388000000000 0.0119915400000000 1.0
C12 C 0.0200451600000000 0.9477692600000000 0.9694439900000000 1.0
C13 C 0.1451797900000000 0.0597069400000000 0.0145249700000000 1.0
C14 C 0.2675873500000000 0.0433526900000000 0.9728415900000000 1.0
C15 C 0.2671649700000000 0.9649007000000000 0.9725751600000000 1.0
C16 C 0.1451426600000000 0.9474017200000000 0.0146827500000000 1.0
C17 C 0.5199892900000000 0.0599742700000000 0.9714028900000000 1.0
C18 C 0.3975876200000000 0.0430826600000000 0.0128794800000000 1.0
C19 C 0.3979750700000000 0.9646372100000000 0.0121138100000000 1.0
C20 C 0.5200082200000000 0.9476784200000000 0.9698229000000000 1.0
C21 C 0.6452614300000000 0.0597918300000000 0.0143441000000000 1.0
C22 C 0.7676560000000000 0.0431461500000000 0.9727978400000000 1.0
C23 C 0.7670554600000000 0.9646969600000000 0.9727524800000000 1.0
C24 C 0.6450895200000000 0.9474873700000000 0.0150859000000000 1.0
O25 O 0.0299938600000000 0.0038828700000000 0.9255211600000000 1.0
O26 O 0.1351115400000000 0.0027271200000000 0.0595966800000000 1.0
O27 O 0.5300860400000000 0.0035664500000000 0.9256143400000000 1.0
O28 O 0.6351329800000000 0.0030498300000000 0.0597118500000000 1.0
F29 F 0.8978859200000000 0.9305751600000000 0.0720060500000000 1.0
F30 F 0.0117458600000000 0.8906790100000000 0.9327644800000000 1.0
F31 F 0.2679332300000000 0.9320452500000000 0.9120070500000000 1.0
F32 F 0.1535292900000000 0.8896618300000000 0.0503252200000000 1.0
F33 F 0.3971562700000000 0.9309781400000000 0.0722337400000000 1.0
F34 F 0.5115898100000000 0.8903760600000000 0.9334761200000000 1.0

```

F35 F 0.7672899400000000 0.9316322500000000 0.9122919800000000 1.0  
F36 F 0.6533534400000000 0.8899590900000000 0.0510753200000000 1.0

##### cif ends

furand\_F\_23\_syn\_alt Energy: -229.54291638

##### cif starts

data\_furand\_F\_23\_syn\_alt

\_publ\_section\_comment

;  
Andrew Reynoso, Bohan Xu, and Vincent H. Crespi  
;

\_cell\_length\_a 10.3036661943

\_cell\_length\_b 20.0

\_cell\_length\_c 20.0

\_cell\_angle\_alpha 90.0

\_cell\_angle\_beta 90.0

\_cell\_angle\_gamma 90.0

\_symmetry\_space\_group\_name\_H-M 'P 1'

\_symmetry\_Int\_Tables\_number 1

\_symmetry\_cell\_setting triclinic

loop\_

\_atom\_site\_label

\_atom\_site\_type\_symbol

\_atom\_site\_fract\_x

\_atom\_site\_fract\_y

\_atom\_site\_fract\_z

\_atom\_site\_occupancy

|     |   |                    |                    |                    |     |
|-----|---|--------------------|--------------------|--------------------|-----|
| H1  | H | 0.9305876700000000 | 0.8990660400000000 | 0.0471790500000000 | 1.0 |
| H2  | H | 0.0540090400000000 | 0.9386188200000000 | 0.9271295500000000 | 1.0 |
| H3  | H | 0.1805856400000000 | 0.1009397900000000 | 0.0471667600000000 | 1.0 |
| H4  | H | 0.3040078500000000 | 0.0613714600000000 | 0.9271224700000000 | 1.0 |
| H5  | H | 0.4305869300000000 | 0.8990665900000000 | 0.0471807600000000 | 1.0 |
| H6  | H | 0.5540070600000000 | 0.9386189800000000 | 0.9271309200000000 | 1.0 |
| H7  | H | 0.6805885400000000 | 0.1009404200000000 | 0.0471657500000000 | 1.0 |
| H8  | H | 0.8040064800000000 | 0.0613705500000000 | 0.9271209200000000 | 1.0 |
| C9  | C | 0.0546481900000000 | 0.9604863500000000 | 0.9773259100000000 | 1.0 |
| C10 | C | 0.0564890400000000 | 0.0386246800000000 | 0.9784070700000000 | 1.0 |
| C11 | C | 0.9294464100000000 | 0.0536384900000000 | 0.0181847600000000 | 1.0 |
| C12 | C | 0.9314806000000000 | 0.9464573300000000 | 0.0198759600000000 | 1.0 |
| C13 | C | 0.1814798000000000 | 0.0535448800000000 | 0.0198698600000000 | 1.0 |
| C14 | C | 0.3046477500000000 | 0.0395106100000000 | 0.9773217400000000 | 1.0 |
| C15 | C | 0.3064894200000000 | 0.9613725500000000 | 0.9784129400000000 | 1.0 |
| C16 | C | 0.1794469600000000 | 0.9463636200000000 | 0.0181927100000000 | 1.0 |
| C17 | C | 0.4314802800000000 | 0.9464576000000000 | 0.0198774000000000 | 1.0 |
| C18 | C | 0.5546476300000000 | 0.9604863800000000 | 0.9773272600000000 | 1.0 |
| C19 | C | 0.5564886400000000 | 0.0386247800000000 | 0.9784079400000000 | 1.0 |
| C20 | C | 0.4294466800000000 | 0.0536388100000000 | 0.0181866300000000 | 1.0 |
| C21 | C | 0.6814806300000000 | 0.0535452000000000 | 0.0198693900000000 | 1.0 |
| C22 | C | 0.8046473400000000 | 0.0395100900000000 | 0.9773204400000000 | 1.0 |
| C23 | C | 0.8064886100000000 | 0.9613722000000000 | 0.9784122600000000 | 1.0 |

|     |   |                    |                    |                    |     |
|-----|---|--------------------|--------------------|--------------------|-----|
| C24 | C | 0.6794469200000000 | 0.9463638600000000 | 0.0181933400000000 | 1.0 |
| O25 | O | 0.4304598900000000 | 0.0014844900000000 | 0.0665507000000000 | 1.0 |
| O26 | O | 0.1804594300000000 | 0.9985238900000000 | 0.0665501400000000 | 1.0 |
| O27 | O | 0.9304598600000000 | 0.0014843200000000 | 0.0665492100000000 | 1.0 |
| O28 | O | 0.6804608100000000 | 0.9985245900000000 | 0.0665502500000000 | 1.0 |
| F29 | F | 0.0574471600000000 | 0.0696639500000000 | 0.9158500700000000 | 1.0 |
| F30 | F | 0.9304355700000000 | 0.1146951900000000 | 0.0494909600000000 | 1.0 |
| F31 | F | 0.6804371500000000 | 0.8853119300000000 | 0.0495084900000000 | 1.0 |
| F32 | F | 0.8074437600000000 | 0.9303254600000000 | 0.9158588700000000 | 1.0 |
| F33 | F | 0.5574446900000000 | 0.0696640600000000 | 0.9158508600000000 | 1.0 |
| F34 | F | 0.4304369300000000 | 0.1146952500000000 | 0.0494933600000000 | 1.0 |
| F35 | F | 0.3074468300000000 | 0.9303264700000000 | 0.9158591900000000 | 1.0 |
| F36 | F | 0.1804368100000000 | 0.8853113100000000 | 0.0495071200000000 | 1.0 |

##### cif ends

uran\_F\_23\_syn\_alt\_forbid Energy: -227.16885932

##### cif starts

data\_uran\_F\_23\_syn\_alt\_forbid

\_publ\_section\_comment

;  
Andrew Reynoso, Bohan Xu, and Vincent H. Crespi  
;

\_cell\_length\_a 9.5155998925

\_cell\_length\_b 20.0

\_cell\_length\_c 20.0

\_cell\_angle\_alpha 90.0

\_cell\_angle\_beta 90.0

\_cell\_angle\_gamma 90.0

\_symmetry\_space\_group\_name\_H-M 'P 1'

\_symmetry\_Int\_Tables\_number 1

\_symmetry\_cell\_setting triclinic

loop\_

\_atom\_site\_label

\_atom\_site\_type\_symbol

\_atom\_site\_fract\_x

\_atom\_site\_fract\_y

\_atom\_site\_fract\_z

\_atom\_site\_occupancy

|    |   |                    |                    |                    |     |
|----|---|--------------------|--------------------|--------------------|-----|
| H1 | H | 0.0060826400000000 | 0.0992317600000000 | 0.0567146600000000 | 1.0 |
|----|---|--------------------|--------------------|--------------------|-----|

|    |   |                    |                    |                    |     |
|----|---|--------------------|--------------------|--------------------|-----|
| H2 | H | 0.9994257000000000 | 0.0600357800000000 | 0.9206743000000000 | 1.0 |
|----|---|--------------------|--------------------|--------------------|-----|

|    |   |                    |                    |                    |     |
|----|---|--------------------|--------------------|--------------------|-----|
| H3 | H | 0.2530880700000000 | 0.9332680600000000 | 0.9232518600000000 | 1.0 |
|----|---|--------------------|--------------------|--------------------|-----|

|    |   |                    |                    |                    |     |
|----|---|--------------------|--------------------|--------------------|-----|
| H4 | H | 0.2465634900000000 | 0.8996155300000000 | 0.0607860500000000 | 1.0 |
|----|---|--------------------|--------------------|--------------------|-----|

|    |   |                    |                    |                    |     |
|----|---|--------------------|--------------------|--------------------|-----|
| H5 | H | 0.5060115500000000 | 0.0991111800000000 | 0.0568009900000000 | 1.0 |
|----|---|--------------------|--------------------|--------------------|-----|

|    |   |                    |                    |                    |     |
|----|---|--------------------|--------------------|--------------------|-----|
| H6 | H | 0.4995334300000000 | 0.0600210000000000 | 0.9207163300000000 | 1.0 |
|----|---|--------------------|--------------------|--------------------|-----|

|    |   |                    |                    |                    |     |
|----|---|--------------------|--------------------|--------------------|-----|
| H7 | H | 0.7531923800000000 | 0.9332993500000000 | 0.9231979700000000 | 1.0 |
|----|---|--------------------|--------------------|--------------------|-----|

|    |   |                    |                    |                    |     |
|----|---|--------------------|--------------------|--------------------|-----|
| H8 | H | 0.7465957700000000 | 0.8995267800000000 | 0.0606937900000000 | 1.0 |
|----|---|--------------------|--------------------|--------------------|-----|

|    |   |                    |                    |                    |     |
|----|---|--------------------|--------------------|--------------------|-----|
| C9 | C | 0.0400881500000000 | 0.0536622200000000 | 0.0311121800000000 | 1.0 |
|----|---|--------------------|--------------------|--------------------|-----|

|     |   |                    |                    |                    |     |
|-----|---|--------------------|--------------------|--------------------|-----|
| C10 | C | 0.9595550100000000 | 0.0368923500000000 | 0.9664947800000000 | 1.0 |
|-----|---|--------------------|--------------------|--------------------|-----|

|     |   |                    |                    |                    |     |
|-----|---|--------------------|--------------------|--------------------|-----|
| C11 | C | 0.9588441900000000 | 0.9589258800000000 | 0.9681067400000000 | 1.0 |
|-----|---|--------------------|--------------------|--------------------|-----|

|     |   |                    |                    |                    |     |
|-----|---|--------------------|--------------------|--------------------|-----|
| C12 | C | 0.0432362400000000 | 0.9433185300000000 | 0.0326493100000000 | 1.0 |
|-----|---|--------------------|--------------------|--------------------|-----|

|     |   |                    |                    |                    |     |
|-----|---|--------------------|--------------------|--------------------|-----|
| C13 | C | 0.2094024300000000 | 0.0544198800000000 | 0.0303930700000000 | 1.0 |
| C14 | C | 0.2938089000000000 | 0.0361916400000000 | 0.9665565100000000 | 1.0 |
| C15 | C | 0.2930502000000000 | 0.9582267100000000 | 0.9680937000000000 | 1.0 |
| C16 | C | 0.2125454200000000 | 0.9441056700000000 | 0.0333535400000000 | 1.0 |
| C17 | C | 0.5400563300000000 | 0.0535722200000000 | 0.0311573400000000 | 1.0 |
| C18 | C | 0.4595790600000000 | 0.0368554100000000 | 0.9665082700000000 | 1.0 |
| C19 | C | 0.4588227200000000 | 0.9588864000000000 | 0.9680869100000000 | 1.0 |
| C20 | C | 0.5432494500000000 | 0.9432268400000000 | 0.0326011400000000 | 1.0 |
| C21 | C | 0.7093759100000000 | 0.0543566900000000 | 0.0304452200000000 | 1.0 |
| C22 | C | 0.7937801300000000 | 0.0362005000000000 | 0.9665829600000000 | 1.0 |
| C23 | C | 0.7930747600000000 | 0.9582333600000000 | 0.9680698300000000 | 1.0 |
| C24 | C | 0.7125507800000000 | 0.9440380800000000 | 0.0333038600000000 | 1.0 |
| O25 | O | 0.0064712500000000 | 0.9977766300000000 | 0.0737381000000000 | 1.0 |
| O26 | O | 0.2461517700000000 | 0.0016824100000000 | 0.0736709900000000 | 1.0 |
| O27 | O | 0.5064572000000000 | 0.9976444600000000 | 0.0737350600000000 | 1.0 |
| O28 | O | 0.7461347800000000 | 0.0015794400000000 | 0.0736759500000000 | 1.0 |
| F29 | F | 0.0115833700000000 | 0.9254086100000000 | 0.9121083600000000 | 1.0 |
| F30 | F | 0.9993954000000000 | 0.8847561600000000 | 0.0629391800000000 | 1.0 |
| F31 | F | 0.2532435900000000 | 0.1141673500000000 | 0.0582753400000000 | 1.0 |
| F32 | F | 0.2410638400000000 | 0.0674122500000000 | 0.9092463200000000 | 1.0 |
| F33 | F | 0.5114764700000000 | 0.9253890500000000 | 0.9120594600000000 | 1.0 |
| F34 | F | 0.4994411400000000 | 0.8846339200000000 | 0.0628427700000000 | 1.0 |
| F35 | F | 0.7531839300000000 | 0.1140849100000000 | 0.0583790800000000 | 1.0 |
| F36 | F | 0.7409739300000000 | 0.0674542900000000 | 0.9093025000000000 | 1.0 |

##### cif ends

furán\_F\_23\_syn\_dir Energy: -228.220684

##### cif starts

data\_furan\_F\_23\_syn\_dir

\_publ\_section\_comment

;  
Andrew Reynoso, Bohan Xu, and Vincent H. Crespi  
;

\_cell\_length\_a 10.4154208412

\_cell\_length\_b 20.0

\_cell\_length\_c 20.0

\_cell\_angle\_alpha 90.0

\_cell\_angle\_beta 90.0

\_cell\_angle\_gamma 90.0

\_symmetry\_space\_group\_name\_H-M 'P 1'

\_symmetry\_Int\_Tables\_number 1

\_symmetry\_cell\_setting triclinic

loop\_

\_atom\_site\_label

\_atom\_site\_type\_symbol

\_atom\_site\_fract\_x

\_atom\_site\_fract\_y

\_atom\_site\_fract\_z

\_atom\_site\_occupancy

H1 H 0.5377364000000000 0.0927232700000000 0.0698494200000000 1.0

|     |   |                    |                    |                    |     |
|-----|---|--------------------|--------------------|--------------------|-----|
| H2  | H | 0.6627448300000000 | 0.0759646500000000 | 0.9456821800000000 | 1.0 |
| H3  | H | 0.7877372400000000 | 0.0927196200000000 | 0.0698549000000000 | 1.0 |
| H4  | H | 0.9127362800000000 | 0.0759665300000000 | 0.9456841900000000 | 1.0 |
| H5  | H | 0.0377368400000000 | 0.0927169000000000 | 0.0698545700000000 | 1.0 |
| H6  | H | 0.1627375500000000 | 0.0759637000000000 | 0.9456828500000000 | 1.0 |
| H7  | H | 0.2877347800000000 | 0.0927201700000000 | 0.0698535400000000 | 1.0 |
| H8  | H | 0.4127290300000000 | 0.0759643200000000 | 0.9456814500000000 | 1.0 |
| C9  | C | 0.6627368600000000 | 0.0451581500000000 | 0.9911142100000000 | 1.0 |
| C10 | C | 0.6627268700000000 | 0.9684479800000000 | 0.9761001300000000 | 1.0 |
| C11 | C | 0.5377368900000000 | 0.9457716200000000 | 0.0139139400000000 | 1.0 |
| C12 | C | 0.5377386100000000 | 0.0512443800000000 | 0.0339171300000000 | 1.0 |
| C13 | C | 0.7877375300000000 | 0.0512423000000000 | 0.0339204800000000 | 1.0 |
| C14 | C | 0.9127340400000000 | 0.0451579900000000 | 0.9911151200000000 | 1.0 |
| C15 | C | 0.9127254400000000 | 0.9684481000000000 | 0.9760995500000000 | 1.0 |
| C16 | C | 0.7877352700000000 | 0.9457696000000000 | 0.0139139100000000 | 1.0 |
| C17 | C | 0.0377372900000000 | 0.0512411600000000 | 0.0339190500000000 | 1.0 |
| C18 | C | 0.1627352300000000 | 0.0451571800000000 | 0.9911150200000000 | 1.0 |
| C19 | C | 0.1627273400000000 | 0.9684475600000000 | 0.9761004100000000 | 1.0 |
| C20 | C | 0.0377351600000000 | 0.9457692800000000 | 0.0139114300000000 | 1.0 |
| C21 | C | 0.2877380800000000 | 0.0512426700000000 | 0.0339196000000000 | 1.0 |
| C22 | C | 0.4127338200000000 | 0.0451581800000000 | 0.9911139800000000 | 1.0 |
| C23 | C | 0.4127265400000000 | 0.9684478000000000 | 0.9761011800000000 | 1.0 |
| C24 | C | 0.2877366600000000 | 0.9457701900000000 | 0.0139154400000000 | 1.0 |
| O25 | O | 0.0377356300000000 | 0.9887955500000000 | 0.0704110500000000 | 1.0 |
| O26 | O | 0.7877361000000000 | 0.9887969800000000 | 0.0704126300000000 | 1.0 |
| O27 | O | 0.5377392500000000 | 0.9888005900000000 | 0.0704117700000000 | 1.0 |
| O28 | O | 0.2877387700000000 | 0.9887984100000000 | 0.0704133500000000 | 1.0 |
| F29 | F | 0.6627151300000000 | 0.9508584100000000 | 0.9092209100000000 | 1.0 |
| F30 | F | 0.5377724700000000 | 0.8807145900000000 | 0.0329126800000000 | 1.0 |
| F31 | F | 0.2877716200000000 | 0.8807134800000000 | 0.0329150400000000 | 1.0 |
| F32 | F | 0.4127148700000000 | 0.9508573600000000 | 0.9092221400000000 | 1.0 |
| F33 | F | 0.1627190600000000 | 0.9508592300000000 | 0.9092208500000000 | 1.0 |
| F34 | F | 0.0377705000000000 | 0.8807111400000000 | 0.0329063500000000 | 1.0 |
| F35 | F | 0.9127140600000000 | 0.9508597500000000 | 0.9092199800000000 | 1.0 |
| F36 | F | 0.7877709700000000 | 0.8807122100000000 | 0.0329115800000000 | 1.0 |

##### cif ends

furán\_F\_23\_syn\_dir\_forbid Energy: -225.59182208

##### cif starts

data\_furan\_F\_23\_syn\_dir\_forbid

\_publ\_section\_comment

;  
Andrew Reynoso, Bohan Xu, and Vincent H. Crespi  
;

\_cell\_length\_a 9.6848346968

\_cell\_length\_b 20.0

\_cell\_length\_c 20.0

\_cell\_angle\_alpha 90.0

\_cell\_angle\_beta 90.0

\_cell\_angle\_gamma 90.0

\_symmetry\_space\_group\_name\_H-M 'P 1'



\_symmetry\_Int\_Tables\_number 1  
\_symmetry\_cell\_setting triclinic

loop\_  
\_atom\_site\_label  
\_atom\_site\_type\_symbol  
\_atom\_site\_fract\_x  
\_atom\_site\_fract\_y  
\_atom\_site\_fract\_z  
\_atom\_site\_occupancy

|     |   |                    |                    |                    |     |
|-----|---|--------------------|--------------------|--------------------|-----|
| H1  | H | 0.9982928100000000 | 0.0889078300000000 | 0.0678234900000000 | 1.0 |
| H2  | H | 0.9883117200000000 | 0.0639670500000000 | 0.9270374600000000 | 1.0 |
| H3  | H | 0.2591004900000000 | 0.1137785800000000 | 0.0418182200000000 | 1.0 |
| H4  | H | 0.2343944400000000 | 0.0606759600000000 | 0.9125663400000000 | 1.0 |
| H5  | H | 0.4959692000000000 | 0.1136844200000000 | 0.0420037600000000 | 1.0 |
| H6  | H | 0.5206356300000000 | 0.0607385400000000 | 0.9126579600000000 | 1.0 |
| H7  | H | 0.7569202900000000 | 0.0890469200000000 | 0.0676743400000000 | 1.0 |
| H8  | H | 0.7667088600000000 | 0.0636680200000000 | 0.9269553300000000 | 1.0 |
| C9  | C | 0.9623841100000000 | 0.0470780300000000 | 0.0369734800000000 | 1.0 |
| C10 | C | 0.0390931500000000 | 0.0389427500000000 | 0.9691081100000000 | 1.0 |
| C11 | C | 0.0442307400000000 | 0.9614480200000000 | 0.9647437500000000 | 1.0 |
| C12 | C | 0.9615694400000000 | 0.9368433500000000 | 0.0254307300000000 | 1.0 |
| C13 | C | 0.2928914400000000 | 0.0654600200000000 | 0.0215917900000000 | 1.0 |
| C14 | C | 0.2047989300000000 | 0.0415974400000000 | 0.9619411400000000 | 1.0 |
| C15 | C | 0.2082448600000000 | 0.9638320500000000 | 0.9687017400000000 | 1.0 |
| C16 | C | 0.2905097100000000 | 0.9557622200000000 | 0.0357012100000000 | 1.0 |
| C17 | C | 0.4621509300000000 | 0.0654178900000000 | 0.0216645100000000 | 1.0 |
| C18 | C | 0.5502377000000000 | 0.0415982200000000 | 0.9620069600000000 | 1.0 |
| C19 | C | 0.5464514100000000 | 0.9638464500000000 | 0.9686769600000000 | 1.0 |
| C20 | C | 0.4640385300000000 | 0.9556956500000000 | 0.0356285900000000 | 1.0 |
| C21 | C | 0.7927750900000000 | 0.0471086100000000 | 0.0369560200000000 | 1.0 |
| C22 | C | 0.7159465000000000 | 0.0388088800000000 | 0.9691283700000000 | 1.0 |
| C23 | C | 0.7104752300000000 | 0.9612962500000000 | 0.9649267900000000 | 1.0 |
| C24 | C | 0.7931765800000000 | 0.9368564500000000 | 0.0256403000000000 | 1.0 |
| O25 | O | 0.9973145900000000 | 0.9866938300000000 | 0.0726520600000000 | 1.0 |
| O26 | O | 0.2583299600000000 | 0.0155547600000000 | 0.0704065900000000 | 1.0 |
| O27 | O | 0.4964873600000000 | 0.0154094700000000 | 0.0704169200000000 | 1.0 |
| O28 | O | 0.7578049700000000 | 0.9868349400000000 | 0.0727915600000000 | 1.0 |
| F29 | F | 0.0072971700000000 | 0.9331927500000000 | 0.9045552100000000 | 1.0 |
| F30 | F | 0.0028527400000000 | 0.8757019900000000 | 0.0474511700000000 | 1.0 |
| F31 | F | 0.2575811200000000 | 0.9261796000000000 | 0.9166163400000000 | 1.0 |
| F32 | F | 0.2524237200000000 | 0.9029800400000000 | 0.0738200100000000 | 1.0 |
| F33 | F | 0.4972687200000000 | 0.9264030300000000 | 0.9164079600000000 | 1.0 |
| F34 | F | 0.5020896900000000 | 0.9028108200000000 | 0.0736202700000000 | 1.0 |
| F35 | F | 0.7476263000000000 | 0.9328204100000000 | 0.9048701900000000 | 1.0 |
| F36 | F | 0.7521222100000000 | 0.8757993900000000 | 0.0479669500000000 | 1.0 |

##### cif ends

furand\_F\_24\_anti\_alt Energy: -228.65226943

##### cif starts

data\_furand\_F\_24\_anti\_alt

\_publ\_section\_comment

;

;

```

_cell_length_a  9.4200542805
_cell_length_b  20.0
_cell_length_c  20.0
_cell_angle_alpha  90.0
_cell_angle_beta  90.0
_cell_angle_gamma  90.0

```

```

_symmetry_space_group_name_H-M  'P 1'
_symmetry_Int_Tables_number 1
_symmetry_cell_setting triclinic

```

```

loop_
_atom_site_label
_atom_site_type_symbol
_atom_site_fract_x
_atom_site_fract_y
_atom_site_fract_z
_atom_site_occupancy
H1  H  0.9313835600000000  0.9405260400000000  0.0749310200000000  1.0
H2  H  0.9440829000000000  0.1036240900000000  0.9438468500000000  1.0
H3  H  0.1813863800000000  0.0594738800000000  0.9250700800000000  1.0
H4  H  0.6940791000000000  0.8963770500000000  0.0561539500000000  1.0
H5  H  0.4313867500000000  0.9405269100000000  0.0749315000000000  1.0
H6  H  0.4440792700000000  0.1036229900000000  0.9438443500000000  1.0
H7  H  0.6813837800000000  0.0594734400000000  0.9250673100000000  1.0
H8  H  0.1940834000000000  0.8963762200000000  0.0561547900000000  1.0
C9  C  0.8817972300000000  0.9603669100000000  0.0295211300000000  1.0
C10 C  0.8814362200000000  0.0380939200000000  0.0304321100000000  1.0
C11 C  0.9685696500000000  0.0552117900000000  0.9666552500000000  1.0
C12 C  0.9670088600000000  0.9471235300000000  0.9658244100000000  1.0
C13 C  0.2170094700000000  0.0528765000000000  0.0341765800000000  1.0
C14 C  0.1317990300000000  0.0396332400000000  0.9704799400000000  1.0
C15 C  0.1314373400000000  0.9619060600000000  0.9695686600000000  1.0
C16 C  0.2185698200000000  0.9447884100000000  0.0333460900000000  1.0
C17 C  0.4670086300000000  0.9471230900000000  0.9658244000000000  1.0
C18 C  0.3817991900000000  0.9603670400000000  0.0295215200000000  1.0
C19 C  0.3814374800000000  0.0380941700000000  0.0304320100000000  1.0
C20 C  0.4685676500000000  0.0552113700000000  0.9666537600000000  1.0
C21 C  0.7170082300000000  0.0528771300000000  0.0341742900000000  1.0
C22 C  0.6317977700000000  0.0396332600000000  0.9704775700000000  1.0
C23 C  0.6314363400000000  0.9619061800000000  0.9695672200000000  1.0
C24 C  0.7185674100000000  0.9447887600000000  0.0333449300000000  1.0
O25 O  0.4236879300000000  0.0019503100000000  0.9226347800000000  1.0
O26 O  0.1736906800000000  0.9980487700000000  0.0773659900000000  1.0
O27 O  0.9236902100000000  0.0019511700000000  0.9226350500000000  1.0
O28 O  0.6736873700000000  0.9980498400000000  0.0773642300000000  1.0
F29 F  0.9417333300000000  0.8868224800000000  0.9367112500000000  1.0
F30 F  0.9352971000000000  0.0666147900000000  0.0882752300000000  1.0
F31 F  0.1917327700000000  0.1131776900000000  0.0632899600000000  1.0
F32 F  0.6852982300000000  0.9333845400000000  0.9117247400000000  1.0
F33 F  0.4417322400000000  0.8868212300000000  0.9367127500000000  1.0
F34 F  0.4353005700000000  0.0666161600000000  0.0882741500000000  1.0

```

F35 F 0.691732940000000 0.113179170000000 0.063286280000000 1.0  
F36 F 0.185299140000000 0.933384900000000 0.911725870000000 1.0

##### cif ends

furand\_F\_24\_anti\_alt\_forbid Energy: -228.60339426

##### cif starts

data\_furand\_F\_24\_anti\_alt\_forbid

\_publ\_section\_comment

;  
Andrew Reynoso, Bohan Xu, and Vincent H. Crespi  
;

\_cell\_length\_a 10.2598914067

\_cell\_length\_b 20.0

\_cell\_length\_c 20.0

\_cell\_angle\_alpha 90.0

\_cell\_angle\_beta 90.0

\_cell\_angle\_gamma 90.0

\_symmetry\_space\_group\_name\_H-M 'P 1'

\_symmetry\_Int\_Tables\_number 1

\_symmetry\_cell\_setting triclinic

loop\_

\_atom\_site\_label

\_atom\_site\_type\_symbol

\_atom\_site\_fract\_x

\_atom\_site\_fract\_y

\_atom\_site\_fract\_z

\_atom\_site\_occupancy

|     |   |                   |                   |                   |     |
|-----|---|-------------------|-------------------|-------------------|-----|
| H1  | H | 0.071601660000000 | 0.891620990000000 | 0.938627900000000 | 1.0 |
| H2  | H | 0.955402360000000 | 0.061347640000000 | 0.054509420000000 | 1.0 |
| H3  | H | 0.213701610000000 | 0.098912650000000 | 0.036334010000000 | 1.0 |
| H4  | H | 0.329912100000000 | 0.929159790000000 | 0.920469710000000 | 1.0 |
| H5  | H | 0.571554740000000 | 0.891827710000000 | 0.938181620000000 | 1.0 |
| H6  | H | 0.454945220000000 | 0.061118510000000 | 0.054673580000000 | 1.0 |
| H7  | H | 0.713674900000000 | 0.098682610000000 | 0.036782610000000 | 1.0 |
| H8  | H | 0.830338590000000 | 0.929426320000000 | 0.920264860000000 | 1.0 |
| C9  | C | 0.080393440000000 | 0.050559970000000 | 0.964148470000000 | 1.0 |
| C10 | C | 0.958135810000000 | 0.035685840000000 | 0.006130890000000 | 1.0 |
| C11 | C | 0.957620940000000 | 0.957249670000000 | 0.008340910000000 | 1.0 |
| C12 | C | 0.079711210000000 | 0.938466610000000 | 0.966913030000000 | 1.0 |
| C13 | C | 0.205583790000000 | 0.052071350000000 | 0.008044670000000 | 1.0 |
| C14 | C | 0.327676360000000 | 0.033279370000000 | 0.966614620000000 | 1.0 |
| C15 | C | 0.327159150000000 | 0.954839660000000 | 0.968837850000000 | 1.0 |
| C16 | C | 0.204898020000000 | 0.939980430000000 | 0.010818620000000 | 1.0 |
| C17 | C | 0.580346420000000 | 0.050647170000000 | 0.964385650000000 | 1.0 |
| C18 | C | 0.458059010000000 | 0.035570650000000 | 0.006244780000000 | 1.0 |
| C19 | C | 0.457682440000000 | 0.957131430000000 | 0.008306630000000 | 1.0 |
| C20 | C | 0.579696200000000 | 0.938540130000000 | 0.966682350000000 | 1.0 |
| C21 | C | 0.705563170000000 | 0.051973140000000 | 0.008274560000000 | 1.0 |
| C22 | C | 0.827601810000000 | 0.033401210000000 | 0.966665900000000 | 1.0 |
| C23 | C | 0.827235070000000 | 0.954960120000000 | 0.968703780000000 | 1.0 |

|     |   |                    |                    |                    |     |
|-----|---|--------------------|--------------------|--------------------|-----|
| C24 | C | 0.7049410800000000 | 0.9398655400000000 | 0.0105510700000000 | 1.0 |
| O25 | O | 0.0896222200000000 | 0.9933008000000000 | 0.9203649600000000 | 1.0 |
| O26 | O | 0.1956710700000000 | 0.9972422500000000 | 0.0545927300000000 | 1.0 |
| O27 | O | 0.5895359400000000 | 0.9935698500000000 | 0.9203654600000000 | 1.0 |
| O28 | O | 0.6957042200000000 | 0.9969363100000000 | 0.0545791000000000 | 1.0 |
| F29 | F | 0.0730002400000000 | 0.1069856500000000 | 0.9256492000000000 | 1.0 |
| F30 | F | 0.9567340200000000 | 0.9266370800000000 | 0.0701975500000000 | 1.0 |
| F31 | F | 0.3285892700000000 | 0.0638985100000000 | 0.9047635500000000 | 1.0 |
| F32 | F | 0.2123002100000000 | 0.8835757900000000 | 0.0493452800000000 | 1.0 |
| F33 | F | 0.5729297900000000 | 0.1072536800000000 | 0.9261474400000000 | 1.0 |
| F34 | F | 0.4571340900000000 | 0.9263623700000000 | 0.0700902100000000 | 1.0 |
| F35 | F | 0.8281486300000000 | 0.0641968200000000 | 0.9048974000000000 | 1.0 |
| F36 | F | 0.7124218700000000 | 0.8832571900000000 | 0.0487818200000000 | 1.0 |

##### cif ends

  furan\_F\_24\_anti\_dir  Energy: -229.37626843

##### cif starts

data\_furan\_F\_24\_anti\_dir

\_publ\_section\_comment

;  
Andrew Reynoso, Bohan Xu, and Vincent H. Crespi  
;

\_cell\_length\_a  9.3349072271

\_cell\_length\_b  20.0

\_cell\_length\_c  20.0

\_cell\_angle\_alpha  90.0

\_cell\_angle\_beta  90.0

\_cell\_angle\_gamma  90.0

\_symmetry\_space\_group\_name\_H-M  'P 1'

\_symmetry\_Int\_Tables\_number  1

\_symmetry\_cell\_setting  triclinic

loop\_

\_atom\_site\_label

\_atom\_site\_type\_symbol

\_atom\_site\_fract\_x

\_atom\_site\_fract\_y

\_atom\_site\_fract\_z

\_atom\_site\_occupancy

|    |   |                    |                    |                    |     |
|----|---|--------------------|--------------------|--------------------|-----|
| H1 | H | 0.9305087900000000 | 0.0584035200000000 | 0.0770619800000000 | 1.0 |
|----|---|--------------------|--------------------|--------------------|-----|

|    |   |                    |                    |                    |     |
|----|---|--------------------|--------------------|--------------------|-----|
| H2 | H | 0.9440865000000000 | 0.8985446000000000 | 0.9399647400000000 | 1.0 |
|----|---|--------------------|--------------------|--------------------|-----|

|    |   |                    |                    |                    |     |
|----|---|--------------------|--------------------|--------------------|-----|
| H3 | H | 0.1805114900000000 | 0.0582666300000000 | 0.9228325200000000 | 1.0 |
|----|---|--------------------|--------------------|--------------------|-----|

|    |   |                    |                    |                    |     |
|----|---|--------------------|--------------------|--------------------|-----|
| H4 | H | 0.6940919300000000 | 0.8986511800000000 | 0.0602171600000000 | 1.0 |
|----|---|--------------------|--------------------|--------------------|-----|

|    |   |                    |                    |                    |     |
|----|---|--------------------|--------------------|--------------------|-----|
| H5 | H | 0.4305094100000000 | 0.0584029400000000 | 0.0770615800000000 | 1.0 |
|----|---|--------------------|--------------------|--------------------|-----|

|    |   |                    |                    |                    |     |
|----|---|--------------------|--------------------|--------------------|-----|
| H6 | H | 0.4440870900000000 | 0.8985444200000000 | 0.9399641300000000 | 1.0 |
|----|---|--------------------|--------------------|--------------------|-----|

|    |   |                    |                    |                    |     |
|----|---|--------------------|--------------------|--------------------|-----|
| H7 | H | 0.6805122700000000 | 0.0582665300000000 | 0.9228326600000000 | 1.0 |
|----|---|--------------------|--------------------|--------------------|-----|

|    |   |                    |                    |                    |     |
|----|---|--------------------|--------------------|--------------------|-----|
| H8 | H | 0.1940909700000000 | 0.8986513900000000 | 0.0602171700000000 | 1.0 |
|----|---|--------------------|--------------------|--------------------|-----|

|    |   |                    |                    |                    |     |
|----|---|--------------------|--------------------|--------------------|-----|
| C9 | C | 0.8836872800000000 | 0.0386273600000000 | 0.0309353800000000 | 1.0 |
|----|---|--------------------|--------------------|--------------------|-----|

|     |   |                    |                    |                    |     |
|-----|---|--------------------|--------------------|--------------------|-----|
| C10 | C | 0.8799645100000000 | 0.9606613700000000 | 0.0292645200000000 | 1.0 |
|-----|---|--------------------|--------------------|--------------------|-----|

|     |   |                    |                    |                    |     |
|-----|---|--------------------|--------------------|--------------------|-----|
| C11 | C | 0.9656045600000000 | 0.9461036700000000 | 0.9648944000000000 | 1.0 |
|-----|---|--------------------|--------------------|--------------------|-----|

|     |   |                    |                    |                    |     |
|-----|---|--------------------|--------------------|--------------------|-----|
| C12 | C | 0.9698455600000000 | 0.0537907500000000 | 0.9669752500000000 | 1.0 |
|-----|---|--------------------|--------------------|--------------------|-----|

|     |   |                    |                    |                    |     |
|-----|---|--------------------|--------------------|--------------------|-----|
| C13 | C | 0.2198404300000000 | 0.0538506200000000 | 0.0329282000000000 | 1.0 |
| C14 | C | 0.1336929100000000 | 0.0385695100000000 | 0.9689935600000000 | 1.0 |
| C15 | C | 0.1299682500000000 | 0.9606054400000000 | 0.9708055600000000 | 1.0 |
| C16 | C | 0.2156025000000000 | 0.9461664300000000 | 0.0352018800000000 | 1.0 |
| C17 | C | 0.4698458200000000 | 0.0537904700000000 | 0.9669749800000000 | 1.0 |
| C18 | C | 0.3836877500000000 | 0.0386268500000000 | 0.0309349400000000 | 1.0 |
| C19 | C | 0.3799644100000000 | 0.9606609900000000 | 0.0292640000000000 | 1.0 |
| C20 | C | 0.4656048900000000 | 0.9461034300000000 | 0.9648939700000000 | 1.0 |
| C21 | C | 0.7198396200000000 | 0.0538507000000000 | 0.0329284500000000 | 1.0 |
| C22 | C | 0.6336931100000000 | 0.0385693600000000 | 0.9689936200000000 | 1.0 |
| C23 | C | 0.6299686300000000 | 0.9606052500000000 | 0.9708056300000000 | 1.0 |
| C24 | C | 0.7156028000000000 | 0.9461663900000000 | 0.0352021100000000 | 1.0 |
| O25 | O | 0.4229030600000000 | 0.0011851100000000 | 0.9226043100000000 | 1.0 |
| O26 | O | 0.1728959700000000 | 0.0013228700000000 | 0.0773915900000000 | 1.0 |
| O27 | O | 0.9229022400000000 | 0.0011853300000000 | 0.9226047500000000 | 1.0 |
| O28 | O | 0.6728953400000000 | 0.0013227200000000 | 0.0773917200000000 | 1.0 |
| F29 | F | 0.9388570900000000 | 0.1144233900000000 | 0.9385516500000000 | 1.0 |
| F30 | F | 0.9395414900000000 | 0.9282318400000000 | 0.0849406300000000 | 1.0 |
| F31 | F | 0.1888427300000000 | 0.1145320400000000 | 0.0612431500000000 | 1.0 |
| F32 | F | 0.6895531200000000 | 0.9280643800000000 | 0.9151956000000000 | 1.0 |
| F33 | F | 0.4388573200000000 | 0.1144231500000000 | 0.9385514100000000 | 1.0 |
| F34 | F | 0.4395417200000000 | 0.9282310300000000 | 0.0849398500000000 | 1.0 |
| F35 | F | 0.6888409100000000 | 0.1145318300000000 | 0.0612435000000000 | 1.0 |
| F36 | F | 0.1895525500000000 | 0.9280644900000000 | 0.9151954500000000 | 1.0 |

##### cif ends

furan\_F\_24\_anti\_dir\_forbid Energy: -229.33446221

##### cif starts

data\_furan\_F\_24\_anti\_dir\_forbid

\_publ\_section\_comment

;  
Andrew Reynoso, Bohan Xu, and Vincent H. Crespi  
;

\_cell\_length\_a 10.1944078727

\_cell\_length\_b 20.0

\_cell\_length\_c 20.0

\_cell\_angle\_alpha 90.0

\_cell\_angle\_beta 90.0

\_cell\_angle\_gamma 90.0

\_symmetry\_space\_group\_name\_H-M 'P 1'

\_symmetry\_Int\_Tables\_number 1

\_symmetry\_cell\_setting triclinic

loop\_

\_atom\_site\_label

\_atom\_site\_type\_symbol

\_atom\_site\_fract\_x

\_atom\_site\_fract\_y

\_atom\_site\_fract\_z

\_atom\_site\_occupancy

H1 H 0.0225327000000000 0.0598110100000000 0.0667128900000000 1.0

|     |   |                    |                    |                    |     |
|-----|---|--------------------|--------------------|--------------------|-----|
| H2  | H | 0.1437431800000000 | 0.9003564100000000 | 0.9374078200000000 | 1.0 |
| H3  | H | 0.4030060000000000 | 0.0639734400000000 | 0.9261792700000000 | 1.0 |
| H4  | H | 0.2814932600000000 | 0.8972267000000000 | 0.0458905200000000 | 1.0 |
| H5  | H | 0.5221557300000000 | 0.0598347400000000 | 0.0667255000000000 | 1.0 |
| H6  | H | 0.6438018400000000 | 0.9003872400000000 | 0.9374994400000000 | 1.0 |
| H7  | H | 0.9026932200000000 | 0.0639320700000000 | 0.9263234600000000 | 1.0 |
| H8  | H | 0.7814157400000000 | 0.8971521300000000 | 0.0460284900000000 | 1.0 |
| C9  | C | 0.1480049700000000 | 0.0564004800000000 | 0.9754539100000000 | 1.0 |
| C10 | C | 0.0266551000000000 | 0.0375599200000000 | 0.0167808000000000 | 1.0 |
| C11 | C | 0.0286443700000000 | 0.9591224000000000 | 0.0125900100000000 | 1.0 |
| C12 | C | 0.1513953100000000 | 0.9441882600000000 | 0.9700042700000000 | 1.0 |
| C13 | C | 0.2771841400000000 | 0.0552186000000000 | 0.0169671900000000 | 1.0 |
| C14 | C | 0.3986595200000000 | 0.0388293200000000 | 0.9747136400000000 | 1.0 |
| C15 | C | 0.3966365200000000 | 0.9602784700000000 | 0.9743231000000000 | 1.0 |
| C16 | C | 0.2738194500000000 | 0.9428760100000000 | 0.0158972600000000 | 1.0 |
| C17 | C | 0.6480983400000000 | 0.0564141700000000 | 0.9756281400000000 | 1.0 |
| C18 | C | 0.5265592600000000 | 0.0375896000000000 | 0.0167982200000000 | 1.0 |
| C19 | C | 0.5285561500000000 | 0.9591524100000000 | 0.0126001100000000 | 1.0 |
| C20 | C | 0.6514267700000000 | 0.9441981800000000 | 0.9701232300000000 | 1.0 |
| C21 | C | 0.7772016100000000 | 0.0551570800000000 | 0.0172003700000000 | 1.0 |
| C22 | C | 0.8985810500000000 | 0.0387852200000000 | 0.9748611600000000 | 1.0 |
| C23 | C | 0.8965778300000000 | 0.9602341000000000 | 0.9744506100000000 | 1.0 |
| C24 | C | 0.7737949700000000 | 0.9428224700000000 | 0.0160591400000000 | 1.0 |
| O25 | O | 0.1599408700000000 | 0.0029077700000000 | 0.9280193900000000 | 1.0 |
| O26 | O | 0.2652202900000000 | 0.9990621900000000 | 0.0612194000000000 | 1.0 |
| O27 | O | 0.6601312800000000 | 0.0029392800000000 | 0.9281713300000000 | 1.0 |
| O28 | O | 0.7652050400000000 | 0.9989758200000000 | 0.0614082300000000 | 1.0 |
| F29 | F | 0.1359952600000000 | 0.1146819800000000 | 0.9396981200000000 | 1.0 |
| F30 | F | 0.0272992500000000 | 0.9211776000000000 | 0.0708827400000000 | 1.0 |
| F31 | F | 0.2890749100000000 | 0.1113352600000000 | 0.0560417400000000 | 1.0 |
| F32 | F | 0.3981451000000000 | 0.9257910400000000 | 0.9139270200000000 | 1.0 |
| F33 | F | 0.6363126700000000 | 0.1147223500000000 | 0.9398953400000000 | 1.0 |
| F34 | F | 0.5269619000000000 | 0.9212078300000000 | 0.0708900500000000 | 1.0 |
| F35 | F | 0.7891594600000000 | 0.1112309500000000 | 0.0563283400000000 | 1.0 |
| F36 | F | 0.8979222100000000 | 0.9257575500000000 | 0.9140425300000000 | 1.0 |

##### cif ends

furand\_F\_24\_syn\_alt Energy: -229.54310378

##### cif starts

data\_furand\_F\_24\_syn\_alt

\_publ\_section\_comment

;  
Andrew Reynoso, Bohan Xu, and Vincent H. Crespi  
;

\_cell\_length\_a 10.3042204584

\_cell\_length\_b 20.0

\_cell\_length\_c 20.0

\_cell\_angle\_alpha 90.0

\_cell\_angle\_beta 90.0

\_cell\_angle\_gamma 90.0

\_symmetry\_space\_group\_name\_H-M 'P 1'

\_symmetry\_Int\_Tables\_number 1  
\_symmetry\_cell\_setting triclinic

loop\_  
\_atom\_site\_label  
\_atom\_site\_type\_symbol  
\_atom\_site\_fract\_x  
\_atom\_site\_fract\_y  
\_atom\_site\_fract\_z  
\_atom\_site\_occupancy

|     |   |                    |                    |                    |     |
|-----|---|--------------------|--------------------|--------------------|-----|
| H1  | H | 0.6060302400000000 | 0.9393318800000000 | 0.9155325300000000 | 1.0 |
| H2  | H | 0.4796325700000000 | 0.1014938900000000 | 0.0358088200000000 | 1.0 |
| H3  | H | 0.8560062300000000 | 0.0621157000000000 | 0.9157867600000000 | 1.0 |
| H4  | H | 0.2296735200000000 | 0.8994665700000000 | 0.0354045700000000 | 1.0 |
| H5  | H | 0.1060657100000000 | 0.9393376100000000 | 0.9155342200000000 | 1.0 |
| H6  | H | 0.9796220000000000 | 0.1014885700000000 | 0.0358156400000000 | 1.0 |
| H7  | H | 0.3560375600000000 | 0.0621216500000000 | 0.9157839900000000 | 1.0 |
| H8  | H | 0.7296100500000000 | 0.8994666500000000 | 0.0354066700000000 | 1.0 |
| C9  | C | 0.6054714300000000 | 0.9610892400000000 | 0.9657635000000000 | 1.0 |
| C10 | C | 0.6036592700000000 | 0.0392284700000000 | 0.9669937100000000 | 1.0 |
| C11 | C | 0.4786710300000000 | 0.0541292100000000 | 0.0084629700000000 | 1.0 |
| C12 | C | 0.4806939900000000 | 0.9469330400000000 | 0.0066136100000000 | 1.0 |
| C13 | C | 0.7306830500000000 | 0.0541424100000000 | 0.0068340500000000 | 1.0 |
| C14 | C | 0.8554632400000000 | 0.0401521500000000 | 0.9659280800000000 | 1.0 |
| C15 | C | 0.8536536100000000 | 0.9620085800000000 | 0.9668397000000000 | 1.0 |
| C16 | C | 0.7286627700000000 | 0.9469400800000000 | 0.0082479600000000 | 1.0 |
| C17 | C | 0.9806927700000000 | 0.9469281500000000 | 0.0066119000000000 | 1.0 |
| C18 | C | 0.1054827200000000 | 0.9610879500000000 | 0.9657686300000000 | 1.0 |
| C19 | C | 0.1036670300000000 | 0.0392280800000000 | 0.9669990300000000 | 1.0 |
| C20 | C | 0.9786676500000000 | 0.0541263800000000 | 0.0084647700000000 | 1.0 |
| C21 | C | 0.2306994300000000 | 0.0541433000000000 | 0.0068350200000000 | 1.0 |
| C22 | C | 0.3554740300000000 | 0.0401544600000000 | 0.9659241200000000 | 1.0 |
| C23 | C | 0.3536666400000000 | 0.9620118400000000 | 0.9668365700000000 | 1.0 |
| C24 | C | 0.2286839100000000 | 0.9469407900000000 | 0.0082478500000000 | 1.0 |
| O25 | O | 0.9796909600000000 | 0.9990258500000000 | 0.0550478900000000 | 1.0 |
| O26 | O | 0.7296787100000000 | 0.0018487600000000 | 0.0550560600000000 | 1.0 |
| O27 | O | 0.4796950400000000 | 0.9990313000000000 | 0.0550482400000000 | 1.0 |
| O28 | O | 0.2297063100000000 | 0.0018487700000000 | 0.0550564800000000 | 1.0 |
| F29 | F | 0.4796993400000000 | 0.8858438100000000 | 0.0378432300000000 | 1.0 |
| F30 | F | 0.6027893900000000 | 0.0703287600000000 | 0.9044733400000000 | 1.0 |
| F31 | F | 0.7296590800000000 | 0.1151054400000000 | 0.0383074000000000 | 1.0 |
| F32 | F | 0.3527999900000000 | 0.9311671900000000 | 0.9041894100000000 | 1.0 |
| F33 | F | 0.9796953300000000 | 0.8858393300000000 | 0.0378418200000000 | 1.0 |
| F34 | F | 0.1028058800000000 | 0.0703231100000000 | 0.9044757900000000 | 1.0 |
| F35 | F | 0.2296971500000000 | 0.1151044400000000 | 0.0383122100000000 | 1.0 |
| F36 | F | 0.8527633800000000 | 0.9311706000000000 | 0.9041894400000000 | 1.0 |

##### cif ends

furand\_F\_24\_syn\_alt\_forbid Energy: -227.28111307

##### cif starts

data\_furand\_F\_24\_syn\_alt\_forbid

\_publ\_section\_comment

;

;

```

_cell_length_a  9.5125277345
_cell_length_b  20.0
_cell_length_c  20.0
_cell_angle_alpha  90.0
_cell_angle_beta  90.0
_cell_angle_gamma  90.0

```

```

_symmetry_space_group_name_H-M  'P 1'
_symmetry_Int_Tables_number 1
_symmetry_cell_setting triclinic

```

```

loop_
_atom_site_label
_atom_site_type_symbol
_atom_site_fract_x
_atom_site_fract_y
_atom_site_fract_z
_atom_site_occupancy
H1  H  0.9038654100000000  0.0570768000000000  0.9106506700000000  1.0
H2  H  0.8979188400000000  0.8994275500000000  0.0545902900000000  1.0
H3  H  0.1564840800000000  0.0986105700000000  0.0500206800000000  1.0
H4  H  0.1504907400000000  0.9345485600000000  0.9134372300000000  1.0
H5  H  0.4037994600000000  0.0570488100000000  0.9106733300000000  1.0
H6  H  0.3978642100000000  0.8993661400000000  0.0545672900000000  1.0
H7  H  0.6564545800000000  0.0986520200000000  0.0499627300000000  1.0
H8  H  0.6505198900000000  0.9345146500000000  0.9134697100000000  1.0
C9  C  0.8596610400000000  0.0540257700000000  0.0211479600000000  1.0
C10 C  0.9426505000000000  0.0356515300000000  0.9574627400000000  1.0
C11 C  0.9459799200000000  0.9577581200000000  0.9615732200000000  1.0
C12 C  0.8641600100000000  0.9437285900000000  0.0267738700000000  1.0
C13 C  0.1902302100000000  0.0530818900000000  0.0242619400000000  1.0
C14 C  0.1084041000000000  0.0360868700000000  0.9597715300000000  1.0
C15 C  0.1117285000000000  0.9580898900000000  0.9592248500000000  1.0
C16 C  0.1947070800000000  0.9426417900000000  0.0236895300000000  1.0
C17 C  0.3596692900000000  0.0539804100000000  0.0211749000000000  1.0
C18 C  0.4426333500000000  0.0356222700000000  0.9574743800000000  1.0
C19 C  0.4459837300000000  0.9577276100000000  0.9615781200000000  1.0
C20 C  0.3641382400000000  0.9436788200000000  0.0267648000000000  1.0
C21 C  0.6902252700000000  0.0531102400000000  0.0242278600000000  1.0
C22 C  0.6083881400000000  0.0360709700000000  0.9597563200000000  1.0
C23 C  0.6117342800000000  0.9580738300000000  0.9592429300000000  1.0
C24 C  0.6947262900000000  0.9426715300000000  0.0237150300000000  1.0
O25 O  0.8970252000000000  0.0016438400000000  0.0656858900000000  1.0
O26 O  0.1573422200000000  0.9970105300000000  0.0657871300000000  1.0
O27 O  0.3970175500000000  0.0015800200000000  0.0656955300000000  1.0
O28 O  0.6573547500000000  0.9970627500000000  0.0657846200000000  1.0
F29 F  0.9039050000000000  0.1138982200000000  0.0486884100000000  1.0
F30 F  0.8918969700000000  0.9220183100000000  0.9071393000000000  1.0
F31 F  0.1624241600000000  0.0692970000000000  0.9037418100000000  1.0
F32 F  0.1504131500000000  0.8840947700000000  0.0539224500000000  1.0
F33 F  0.4039352900000000  0.1138408300000000  0.0487312800000000  1.0
F34 F  0.3919367500000000  0.9219921600000000  0.9071327900000000  1.0

```



F35 F 0.6623684900000000 0.0692518700000000 0.9037010300000000 1.0  
F36 F 0.6504745500000000 0.8841360700000000 0.0539857000000000 1.0

##### cif ends

furán\_F\_24\_syn\_dir Energy: -228.58941527

##### cif starts

data\_furan\_F\_24\_syn\_dir

\_publ\_section\_comment

;  
Andrew Reynoso, Bohan Xu, and Vincent H. Crespi  
;

\_cell\_length\_a 10.4003726193

\_cell\_length\_b 20.0

\_cell\_length\_c 20.0

\_cell\_angle\_alpha 90.0

\_cell\_angle\_beta 90.0

\_cell\_angle\_gamma 90.0

\_symmetry\_space\_group\_name\_H-M 'P 1'

\_symmetry\_Int\_Tables\_number 1

\_symmetry\_cell\_setting triclinic

loop\_

\_atom\_site\_label

\_atom\_site\_type\_symbol

\_atom\_site\_fract\_x

\_atom\_site\_fract\_y

\_atom\_site\_fract\_z

\_atom\_site\_occupancy

|     |   |                    |                    |                    |     |
|-----|---|--------------------|--------------------|--------------------|-----|
| H1  | H | 0.0555477800000000 | 0.0541451400000000 | 0.9222238700000000 | 1.0 |
| H2  | H | 0.9305531400000000 | 0.9019421600000000 | 0.0542417500000000 | 1.0 |
| H3  | H | 0.3055465300000000 | 0.0541407700000000 | 0.9222261200000000 | 1.0 |
| H4  | H | 0.6805484500000000 | 0.9019380300000000 | 0.0542437300000000 | 1.0 |
| H5  | H | 0.5555483900000000 | 0.0541440500000000 | 0.9222297500000000 | 1.0 |
| H6  | H | 0.4305470200000000 | 0.9019378800000000 | 0.0542427200000000 | 1.0 |
| H7  | H | 0.8055308300000000 | 0.0541414900000000 | 0.9222266200000000 | 1.0 |
| H8  | H | 0.1805414800000000 | 0.9019443400000000 | 0.0542473200000000 | 1.0 |
| C9  | C | 0.0555482100000000 | 0.0369922900000000 | 0.9742641100000000 | 1.0 |
| C10 | C | 0.0555493500000000 | 0.9590695500000000 | 0.9817493200000000 | 1.0 |
| C11 | C | 0.9305572000000000 | 0.9476982900000000 | 0.0240404900000000 | 1.0 |
| C12 | C | 0.9305573000000000 | 0.0546360100000000 | 0.0138489600000000 | 1.0 |
| C13 | C | 0.1805579400000000 | 0.0546365100000000 | 0.0138504400000000 | 1.0 |
| C14 | C | 0.3055487000000000 | 0.0369905300000000 | 0.9742671000000000 | 1.0 |
| C15 | C | 0.3055478300000000 | 0.9590674500000000 | 0.9817522000000000 | 1.0 |
| C16 | C | 0.1805542100000000 | 0.9476991400000000 | 0.0240436500000000 | 1.0 |
| C17 | C | 0.4305578100000000 | 0.0546336900000000 | 0.0138537500000000 | 1.0 |
| C18 | C | 0.5555479000000000 | 0.0369901500000000 | 0.9742695000000000 | 1.0 |
| C19 | C | 0.5555482300000000 | 0.9590665200000000 | 0.9817521400000000 | 1.0 |
| C20 | C | 0.4305555100000000 | 0.9476953000000000 | 0.0240430900000000 | 1.0 |
| C21 | C | 0.6805569700000000 | 0.0546330200000000 | 0.0138557900000000 | 1.0 |
| C22 | C | 0.8055438900000000 | 0.0369905500000000 | 0.9742672600000000 | 1.0 |
| C23 | C | 0.8055474300000000 | 0.9590675900000000 | 0.9817506000000000 | 1.0 |

|     |   |                    |                    |                    |     |
|-----|---|--------------------|--------------------|--------------------|-----|
| C24 | C | 0.6805561800000000 | 0.9476947900000000 | 0.0240431600000000 | 1.0 |
| O25 | O | 0.4305790600000000 | 0.0054069300000000 | 0.0662662000000000 | 1.0 |
| O26 | O | 0.1805784700000000 | 0.0054122100000000 | 0.0662640300000000 | 1.0 |
| O27 | O | 0.9305803800000000 | 0.0054107400000000 | 0.0662622600000000 | 1.0 |
| O28 | O | 0.6805798100000000 | 0.0054056100000000 | 0.0662670300000000 | 1.0 |
| F29 | F | 0.9305758100000000 | 0.1170159800000000 | 0.0409116400000000 | 1.0 |
| F30 | F | 0.0555481400000000 | 0.9231032000000000 | 0.9224356000000000 | 1.0 |
| F31 | F | 0.1805766600000000 | 0.1170166400000000 | 0.0409126600000000 | 1.0 |
| F32 | F | 0.8055446200000000 | 0.9231050600000000 | 0.9224343100000000 | 1.0 |
| F33 | F | 0.4305764900000000 | 0.1170125600000000 | 0.0409188100000000 | 1.0 |
| F34 | F | 0.5555459700000000 | 0.9231025600000000 | 0.9224368500000000 | 1.0 |
| F35 | F | 0.6805766700000000 | 0.1170109900000000 | 0.0409222400000000 | 1.0 |
| F36 | F | 0.3055426500000000 | 0.9231032900000000 | 0.9224369400000000 | 1.0 |

##### cif ends

  furan\_F\_24\_syn\_dir\_forbid   Energy: -225.8734903

##### cif starts

data\_furan\_F\_24\_syn\_dir\_forbid

\_publ\_section\_comment

;  
Andrew Reynoso, Bohan Xu, and Vincent H. Crespi  
;

\_cell\_length\_a   9.6425308638

\_cell\_length\_b   20.0

\_cell\_length\_c   20.0

\_cell\_angle\_alpha   90.0

\_cell\_angle\_beta   90.0

\_cell\_angle\_gamma   90.0

\_symmetry\_space\_group\_name\_H-M   'P 1'

\_symmetry\_Int\_Tables\_number 1

\_symmetry\_cell\_setting triclinic

loop\_

\_atom\_site\_label

\_atom\_site\_type\_symbol

\_atom\_site\_fract\_x

\_atom\_site\_fract\_y

\_atom\_site\_fract\_z

\_atom\_site\_occupancy

|    |   |                    |                    |                    |     |
|----|---|--------------------|--------------------|--------------------|-----|
| H1 | H | 0.9228873000000000 | 0.0519512500000000 | 0.9006243500000000 | 1.0 |
|----|---|--------------------|--------------------|--------------------|-----|

|    |   |                    |                    |                    |     |
|----|---|--------------------|--------------------|--------------------|-----|
| H2 | H | 0.8954499500000000 | 0.9140490600000000 | 0.0634248300000000 | 1.0 |
|----|---|--------------------|--------------------|--------------------|-----|

|    |   |                    |                    |                    |     |
|----|---|--------------------|--------------------|--------------------|-----|
| H3 | H | 0.1689411500000000 | 0.0572990900000000 | 0.9206938400000000 | 1.0 |
|----|---|--------------------|--------------------|--------------------|-----|

|    |   |                    |                    |                    |     |
|----|---|--------------------|--------------------|--------------------|-----|
| H4 | H | 0.1582721400000000 | 0.8829277000000000 | 0.0399808400000000 | 1.0 |
|----|---|--------------------|--------------------|--------------------|-----|

|    |   |                    |                    |                    |     |
|----|---|--------------------|--------------------|--------------------|-----|
| H5 | H | 0.3807846600000000 | 0.0596505600000000 | 0.9210703600000000 | 1.0 |
|----|---|--------------------|--------------------|--------------------|-----|

|    |   |                    |                    |                    |     |
|----|---|--------------------|--------------------|--------------------|-----|
| H6 | H | 0.3999397000000000 | 0.8845852100000000 | 0.0396910200000000 | 1.0 |
|----|---|--------------------|--------------------|--------------------|-----|

|    |   |                    |                    |                    |     |
|----|---|--------------------|--------------------|--------------------|-----|
| H7 | H | 0.6269101200000000 | 0.0582235300000000 | 0.9029683300000000 | 1.0 |
|----|---|--------------------|--------------------|--------------------|-----|

|    |   |                    |                    |                    |     |
|----|---|--------------------|--------------------|--------------------|-----|
| H8 | H | 0.6544900900000000 | 0.9127430900000000 | 0.0588110900000000 | 1.0 |
|----|---|--------------------|--------------------|--------------------|-----|

|    |   |                    |                    |                    |     |
|----|---|--------------------|--------------------|--------------------|-----|
| C9 | C | 0.8614636300000000 | 0.0625538800000000 | 0.0088020100000000 | 1.0 |
|----|---|--------------------|--------------------|--------------------|-----|

|     |   |                    |                    |                    |     |
|-----|---|--------------------|--------------------|--------------------|-----|
| C10 | C | 0.9494855800000000 | 0.0348275000000000 | 0.9510471600000000 | 1.0 |
|-----|---|--------------------|--------------------|--------------------|-----|

|     |   |                    |                    |                    |     |
|-----|---|--------------------|--------------------|--------------------|-----|
| C11 | C | 0.9452744600000000 | 0.9575663100000000 | 0.9628700800000000 | 1.0 |
|-----|---|--------------------|--------------------|--------------------|-----|

|     |   |                    |                    |                    |     |
|-----|---|--------------------|--------------------|--------------------|-----|
| C12 | C | 0.8620641900000000 | 0.9539133300000000 | 0.0294713300000000 | 1.0 |
|-----|---|--------------------|--------------------|--------------------|-----|

|     |   |                    |                    |                    |     |
|-----|---|--------------------|--------------------|--------------------|-----|
| C13 | C | 0.1879041000000000 | 0.0417402400000000 | 0.0305833100000000 | 1.0 |
| C14 | C | 0.1140656800000000 | 0.0328693200000000 | 0.9618453900000000 | 1.0 |
| C15 | C | 0.1102810700000000 | 0.9551032400000000 | 0.9595828400000000 | 1.0 |
| C16 | C | 0.1938995500000000 | 0.9311539300000000 | 0.0202997600000000 | 1.0 |
| C17 | C | 0.3608004800000000 | 0.0428196900000000 | 0.0305971200000000 | 1.0 |
| C18 | C | 0.4354581900000000 | 0.0351238600000000 | 0.9622338000000000 | 1.0 |
| C19 | C | 0.4423696400000000 | 0.9573466400000000 | 0.9588478100000000 | 1.0 |
| C20 | C | 0.3613656400000000 | 0.9323408300000000 | 0.0201474400000000 | 1.0 |
| C21 | C | 0.6894980600000000 | 0.0634134200000000 | 0.0107298200000000 | 1.0 |
| C22 | C | 0.5997928600000000 | 0.0389721700000000 | 0.9525644000000000 | 1.0 |
| C23 | C | 0.6079350200000000 | 0.9615954400000000 | 0.9604488700000000 | 1.0 |
| C24 | C | 0.6912256600000000 | 0.9540046400000000 | 0.0274220200000000 | 1.0 |
| O25 | O | 0.8954888600000000 | 0.0163421700000000 | 0.0604406600000000 | 1.0 |
| O26 | O | 0.1552489700000000 | 0.9820448500000000 | 0.0668915200000000 | 1.0 |
| O27 | O | 0.3968111000000000 | 0.9836160800000000 | 0.0668242400000000 | 1.0 |
| O28 | O | 0.6567967400000000 | 0.0151240300000000 | 0.0606560600000000 | 1.0 |
| F29 | F | 0.9029547100000000 | 0.1252313400000000 | 0.0269997800000000 | 1.0 |
| F30 | F | 0.8965736000000000 | 0.9148347700000000 | 0.9142869700000000 | 1.0 |
| F31 | F | 0.1468002200000000 | 0.0946672000000000 | 0.0679543900000000 | 1.0 |
| F32 | F | 0.1460257900000000 | 0.9259149700000000 | 0.8993906400000000 | 1.0 |
| F33 | F | 0.3997510500000000 | 0.0963260600000000 | 0.0677789700000000 | 1.0 |
| F34 | F | 0.4043797800000000 | 0.9281549700000000 | 0.8990360500000000 | 1.0 |
| F35 | F | 0.6521491600000000 | 0.1252208500000000 | 0.0331896600000000 | 1.0 |
| F36 | F | 0.6561339800000000 | 0.9246715500000000 | 0.9073196600000000 | 1.0 |

##### cif ends

furane\_F\_3\_anti\_alt Energy: -228.01294678

##### cif starts

data\_furane\_F\_3\_anti\_alt

\_publ\_section\_comment

;  
Andrew Reynoso, Bohan Xu, and Vincent H. Crespi  
;

\_cell\_length\_a 9.3147961202

\_cell\_length\_b 20.0

\_cell\_length\_c 20.0

\_cell\_angle\_alpha 90.0

\_cell\_angle\_beta 90.0

\_cell\_angle\_gamma 90.0

\_symmetry\_space\_group\_name\_H-M 'P 1'

\_symmetry\_Int\_Tables\_number 1

\_symmetry\_cell\_setting triclinic

loop\_

\_atom\_site\_label

\_atom\_site\_type\_symbol

\_atom\_site\_fract\_x

\_atom\_site\_fract\_y

\_atom\_site\_fract\_z

\_atom\_site\_occupancy

H1 H 0.0601147400000000 0.9004937900000000 0.9336044600000000 1.0

|     |   |                    |                    |                    |     |
|-----|---|--------------------|--------------------|--------------------|-----|
| H2  | H | 0.0488138200000000 | 0.0552685700000000 | 0.0740471800000000 | 1.0 |
| H3  | H | 0.0582522900000000 | 0.1047074400000000 | 0.9413409900000000 | 1.0 |
| H4  | H | 0.3101084700000000 | 0.1021256900000000 | 0.0590053000000000 | 1.0 |
| H5  | H | 0.2988179000000000 | 0.9472760200000000 | 0.9186462400000000 | 1.0 |
| H6  | H | 0.3083195200000000 | 0.8979101800000000 | 0.0513694800000000 | 1.0 |
| H7  | H | 0.5601099500000000 | 0.9004857400000000 | 0.9336356200000000 | 1.0 |
| H8  | H | 0.5488129600000000 | 0.0553511700000000 | 0.0739913200000000 | 1.0 |
| H9  | H | 0.5583586900000000 | 0.1047011300000000 | 0.9412622300000000 | 1.0 |
| H10 | H | 0.8100933900000000 | 0.1020519600000000 | 0.0590951700000000 | 1.0 |
| H11 | H | 0.7988070300000000 | 0.9472755500000000 | 0.9186376200000000 | 1.0 |
| H12 | H | 0.8083101700000000 | 0.8978454700000000 | 0.0513268300000000 | 1.0 |
| C13 | C | 0.0834434000000000 | 0.9477239300000000 | 0.9592823800000000 | 1.0 |
| C14 | C | 0.9950185000000000 | 0.9605123700000000 | 0.0238260400000000 | 1.0 |
| C15 | C | 0.9974057500000000 | 0.0387405300000000 | 0.0276026400000000 | 1.0 |
| C16 | C | 0.0812356700000000 | 0.0562496900000000 | 0.9642663000000000 | 1.0 |
| C17 | C | 0.3334437900000000 | 0.0548837000000000 | 0.0333518600000000 | 1.0 |
| C18 | C | 0.2449898500000000 | 0.0420617800000000 | 0.9688211400000000 | 1.0 |
| C19 | C | 0.2474043800000000 | 0.9638343100000000 | 0.9650787300000000 | 1.0 |
| C20 | C | 0.3312615000000000 | 0.9463579400000000 | 0.0284124000000000 | 1.0 |
| C21 | C | 0.5834513000000000 | 0.9477277200000000 | 0.9592893900000000 | 1.0 |
| C22 | C | 0.4950129000000000 | 0.9605553800000000 | 0.0238254400000000 | 1.0 |
| C23 | C | 0.4974064800000000 | 0.0387874900000000 | 0.0275585100000000 | 1.0 |
| C24 | C | 0.5812778700000000 | 0.0562544100000000 | 0.9642281700000000 | 1.0 |
| C25 | C | 0.8334368100000000 | 0.0548320500000000 | 0.0334059900000000 | 1.0 |
| C26 | C | 0.7450265700000000 | 0.0420527200000000 | 0.9688459100000000 | 1.0 |
| C27 | C | 0.7474178500000000 | 0.9638245100000000 | 0.9650797800000000 | 1.0 |
| C28 | C | 0.8312680500000000 | 0.9463094600000000 | 0.0284042300000000 | 1.0 |
| O29 | O | 0.0382762500000000 | 0.0029787400000000 | 0.9183032400000000 | 1.0 |
| O30 | O | 0.2883200700000000 | 0.9996431400000000 | 0.0743595500000000 | 1.0 |
| O31 | O | 0.5383290500000000 | 0.0029689400000000 | 0.9182817900000000 | 1.0 |
| O32 | O | 0.7883147200000000 | 0.9995691200000000 | 0.0743767400000000 | 1.0 |
| F33 | F | 0.0541150800000000 | 0.9269846900000000 | 0.0793386600000000 | 1.0 |
| F34 | F | 0.3040275500000000 | 0.0755776900000000 | 0.9132824700000000 | 1.0 |
| F35 | F | 0.5540804000000000 | 0.9270522600000000 | 0.0793589600000000 | 1.0 |
| F36 | F | 0.8041572700000000 | 0.0755967100000000 | 0.9133462600000000 | 1.0 |

##### cif ends

furan\_F\_3\_anti\_alt\_forbid Energy: -227.890244

##### cif starts

data\_furan\_F\_3\_anti\_alt\_forbid

\_publ\_section\_comment

;

Andrew Reynoso, Bohan Xu, and Vincent H. Crespi

;

\_cell\_length\_a 10.1885870695

\_cell\_length\_b 20.0

\_cell\_length\_c 20.0

\_cell\_angle\_alpha 90.0

\_cell\_angle\_beta 90.0

\_cell\_angle\_gamma 90.0

\_symmetry\_space\_group\_name\_H-M 'P 1'

\_symmetry\_Int\_Tables\_number 1  
\_symmetry\_cell\_setting triclinic

loop\_  
\_atom\_site\_label  
\_atom\_site\_type\_symbol  
\_atom\_site\_fract\_x  
\_atom\_site\_fract\_y  
\_atom\_site\_fract\_z  
\_atom\_site\_occupancy

|     |   |                    |                    |                    |     |
|-----|---|--------------------|--------------------|--------------------|-----|
| H1  | H | 0.0731953300000000 | 0.1000953000000000 | 0.9358939000000000 | 1.0 |
| H2  | H | 0.9565537900000000 | 0.9342236500000000 | 0.0564895100000000 | 1.0 |
| H3  | H | 0.0701143900000000 | 0.8964833900000000 | 0.9327952900000000 | 1.0 |
| H4  | H | 0.3285375600000000 | 0.0597786700000000 | 0.9176070100000000 | 1.0 |
| H5  | H | 0.2148960500000000 | 0.0975428700000000 | 0.0412482900000000 | 1.0 |
| H6  | H | 0.2117222400000000 | 0.8939314200000000 | 0.0382000200000000 | 1.0 |
| H7  | H | 0.5730606100000000 | 0.1001914300000000 | 0.9362875200000000 | 1.0 |
| H8  | H | 0.4569017400000000 | 0.9338916400000000 | 0.0563897200000000 | 1.0 |
| H9  | H | 0.5700991200000000 | 0.8965980300000000 | 0.9324642700000000 | 1.0 |
| H10 | H | 0.8279615200000000 | 0.0599867900000000 | 0.9176399700000000 | 1.0 |
| H11 | H | 0.7148624800000000 | 0.0972986200000000 | 0.0415841600000000 | 1.0 |
| H12 | H | 0.7119236900000000 | 0.8936942900000000 | 0.0377714000000000 | 1.0 |
| C13 | C | 0.0813596600000000 | 0.0538769000000000 | 0.9653477700000000 | 1.0 |
| C14 | C | 0.9577608000000000 | 0.0363347100000000 | 0.0059226100000000 | 1.0 |
| C15 | C | 0.9587562900000000 | 0.9577047800000000 | 0.0069675500000000 | 1.0 |
| C16 | C | 0.0795395200000000 | 0.9410865900000000 | 0.9642516800000000 | 1.0 |
| C17 | C | 0.2054315800000000 | 0.0529270800000000 | 0.0098134700000000 | 1.0 |
| C18 | C | 0.3262343800000000 | 0.0362787700000000 | 0.9671177900000000 | 1.0 |
| C19 | C | 0.3271778200000000 | 0.9576493800000000 | 0.9681307200000000 | 1.0 |
| C20 | C | 0.2035910900000000 | 0.9401405000000000 | 0.0087279800000000 | 1.0 |
| C21 | C | 0.5813009500000000 | 0.0538693300000000 | 0.9655706200000000 | 1.0 |
| C22 | C | 0.4577477700000000 | 0.0361619800000000 | 0.0060771100000000 | 1.0 |
| C23 | C | 0.4588233700000000 | 0.9575310600000000 | 0.0069397300000000 | 1.0 |
| C24 | C | 0.5795435600000000 | 0.9410909200000000 | 0.9640769800000000 | 1.0 |
| C25 | C | 0.7054226800000000 | 0.0528022200000000 | 0.0099789600000000 | 1.0 |
| C26 | C | 0.8261267600000000 | 0.0363777400000000 | 0.9671037600000000 | 1.0 |
| C27 | C | 0.8272465000000000 | 0.9577459600000000 | 0.9680095200000000 | 1.0 |
| C28 | C | 0.7036760500000000 | 0.9400227700000000 | 0.0084967500000000 | 1.0 |
| O29 | O | 0.0890395600000000 | 0.9984483400000000 | 0.9194932800000000 | 1.0 |
| O30 | O | 0.1959213100000000 | 0.9955822000000000 | 0.0545740000000000 | 1.0 |
| O31 | O | 0.5889451800000000 | 0.9986028100000000 | 0.9195128700000000 | 1.0 |
| O32 | O | 0.6960476400000000 | 0.9952921500000000 | 0.0545450400000000 | 1.0 |
| F33 | F | 0.9541740500000000 | 0.0709037300000000 | 0.0665440300000000 | 1.0 |
| F34 | F | 0.3306388100000000 | 0.9231056200000000 | 0.9074959600000000 | 1.0 |
| F35 | F | 0.4540276700000000 | 0.0705616000000000 | 0.0667844300000000 | 1.0 |
| F36 | F | 0.8310545100000000 | 0.9233100200000000 | 0.9073254500000000 | 1.0 |

##### cif ends

furand\_F3\_anti\_dir Energy: -227.96027514

##### cif starts

data\_furand\_F3\_anti\_dir

\_publ\_section\_comment

;

;

```

_cell_length_a  9.3206475576
_cell_length_b  20.0
_cell_length_c  20.0
_cell_angle_alpha  90.0
_cell_angle_beta  90.0
_cell_angle_gamma  90.0

```

```

_symmetry_space_group_name_H-M  'P 1'
_symmetry_Int_Tables_number 1
_symmetry_cell_setting triclinic

```

```

loop_
_atom_site_label
_atom_site_type_symbol
_atom_site_fract_x
_atom_site_fract_y
_atom_site_fract_z
_atom_site_occupancy
H1  H  0.0265437000000000  0.0983017900000000  0.9373723300000000  1.0
H2  H  0.0163516700000000  0.9411343300000000  0.0751810200000000  1.0
H3  H  0.0279212300000000  0.8939739500000000  0.9415826600000000  1.0
H4  H  0.2765471300000000  0.0989549600000000  0.0580005600000000  1.0
H5  H  0.2663815500000000  0.9403076100000000  0.9219010800000000  1.0
H6  H  0.2779303900000000  0.8945908800000000  0.0559989500000000  1.0
H7  H  0.5265250500000000  0.0982986500000000  0.9373608300000000  1.0
H8  H  0.5164010600000000  0.9411348200000000  0.0751737000000000  1.0
H9  H  0.5278860800000000  0.8939724900000000  0.9415754400000000  1.0
H10 H  0.7765228800000000  0.0989646200000000  0.0579562300000000  1.0
H11 H  0.7663658200000000  0.9402932800000000  0.9218817500000000  1.0
H12 H  0.7778817500000000  0.8945997900000000  0.0559899800000000  1.0
C13 C  0.0480235800000000  0.0508833200000000  0.9626192800000000  1.0
C14 C  0.9617281800000000  0.0367350700000000  0.0266508300000000  1.0
C15 C  0.9664027800000000  0.9584927100000000  0.0286924100000000  1.0
C16 C  0.0524168100000000  0.9423307700000000  0.9648506200000000  1.0
C17 C  0.2980139900000000  0.0512611800000000  0.0332714500000000  1.0
C18 C  0.2117449500000000  0.0364256600000000  0.9693906400000000  1.0
C19 C  0.2164143900000000  0.9581651800000000  0.9681951500000000  1.0
C20 C  0.3024204500000000  0.9426956100000000  0.0322121700000000  1.0
C21 C  0.5480109500000000  0.0508820000000000  0.9626058100000000  1.0
C22 C  0.4617462800000000  0.0367361200000000  0.0266514400000000  1.0
C23 C  0.4664255800000000  0.9584930100000000  0.0286924900000000  1.0
C24 C  0.5524033400000000  0.9423290400000000  0.9648398900000000  1.0
C25 C  0.7980015200000000  0.0512663700000000  0.0332410800000000  1.0
C26 C  0.7117388500000000  0.0364195800000000  0.9693599100000000  1.0
C27 C  0.7163992200000000  0.9581598100000000  0.9681750500000000  1.0
C28 C  0.8023943400000000  0.9426975800000000  0.0321964500000000  1.0
O29 O  0.0061985500000000  0.9954711440000000  0.9202873400000000  1.0
O30 O  0.2562026300000000  0.9963125000000000  0.0762045400000000  1.0
O31 O  0.5061683900000000  0.9954684400000000  0.9202809500000000  1.0
O32 O  0.7561595600000000  0.9963224700000000  0.0761780800000000  1.0
F33 F  0.0221302300000000  0.0692363500000000  0.0825147800000000  1.0
F34 F  0.2721920400000000  0.0683235400000000  0.9131922200000000  1.0

```

F35 F 0.522175760000000 0.069244540000000 0.082505130000000 1.0  
F36 F 0.772165280000000 0.068302550000000 0.913149740000000 1.0

##### cif ends

furand\_F3\_anti\_dir\_forbid Energy: -227.82937221

##### cif starts

data\_furand\_F3\_anti\_dir\_forbid

\_publ\_section\_comment

;  
Andrew Reynoso, Bohan Xu, and Vincent H. Crespi  
;

\_cell\_length\_a 10.1848992695

\_cell\_length\_b 20.0

\_cell\_length\_c 20.0

\_cell\_angle\_alpha 90.0

\_cell\_angle\_beta 90.0

\_cell\_angle\_gamma 90.0

\_symmetry\_space\_group\_name\_H-M 'P 1'

\_symmetry\_Int\_Tables\_number 1

\_symmetry\_cell\_setting triclinic

loop\_

\_atom\_site\_label

\_atom\_site\_type\_symbol

\_atom\_site\_fract\_x

\_atom\_site\_fract\_y

\_atom\_site\_fract\_z

\_atom\_site\_occupancy

|     |   |                   |                   |                   |     |
|-----|---|-------------------|-------------------|-------------------|-----|
| H1  | H | 0.119103510000000 | 0.097994180000000 | 0.935674290000000 | 1.0 |
| H2  | H | 0.998053760000000 | 0.936844210000000 | 0.061542800000000 | 1.0 |
| H3  | H | 0.114217020000000 | 0.894451290000000 | 0.940351100000000 | 1.0 |
| H4  | H | 0.256392920000000 | 0.099033600000000 | 0.043506240000000 | 1.0 |
| H5  | H | 0.377504310000000 | 0.935368570000000 | 0.920914370000000 | 1.0 |
| H6  | H | 0.261070050000000 | 0.895436520000000 | 0.042849540000000 | 1.0 |
| H7  | H | 0.619084940000000 | 0.097970870000000 | 0.935675940000000 | 1.0 |
| H8  | H | 0.498013250000000 | 0.936857490000000 | 0.061589830000000 | 1.0 |
| H9  | H | 0.614238520000000 | 0.894427440000000 | 0.940424670000000 | 1.0 |
| H10 | H | 0.756368900000000 | 0.099058850000000 | 0.043509720000000 | 1.0 |
| H11 | H | 0.877402440000000 | 0.935397890000000 | 0.920903500000000 | 1.0 |
| H12 | H | 0.761161510000000 | 0.895463340000000 | 0.042895180000000 | 1.0 |
| C13 | C | 0.126609050000000 | 0.053141500000000 | 0.966889910000000 | 1.0 |
| C14 | C | 0.004086460000000 | 0.037400930000000 | 0.009049270000000 | 1.0 |
| C15 | C | 0.002642900000000 | 0.958750450000000 | 0.011355730000000 | 1.0 |
| C16 | C | 0.124472240000000 | 0.940459770000000 | 0.969997970000000 | 1.0 |
| C17 | C | 0.248823640000000 | 0.053580720000000 | 0.013173450000000 | 1.0 |
| C18 | C | 0.371334430000000 | 0.036988490000000 | 0.971327470000000 | 1.0 |
| C19 | C | 0.372797830000000 | 0.958308630000000 | 0.970634060000000 | 1.0 |
| C20 | C | 0.250909990000000 | 0.940858520000000 | 0.012302480000000 | 1.0 |
| C21 | C | 0.626602050000000 | 0.053130330000000 | 0.966908640000000 | 1.0 |
| C22 | C | 0.504069440000000 | 0.037396450000000 | 0.009061060000000 | 1.0 |
| C23 | C | 0.502632970000000 | 0.958746880000000 | 0.011395610000000 | 1.0 |

|     |   |                    |                    |                    |     |
|-----|---|--------------------|--------------------|--------------------|-----|
| C24 | C | 0.6244793600000000 | 0.9404486800000000 | 0.9700536800000000 | 1.0 |
| C25 | C | 0.7488210500000000 | 0.0535966100000000 | 0.0131891700000000 | 1.0 |
| C26 | C | 0.8713233900000000 | 0.0370095800000000 | 0.9713348700000000 | 1.0 |
| C27 | C | 0.8727752000000000 | 0.9583288100000000 | 0.9706295400000000 | 1.0 |
| C28 | C | 0.7509365800000000 | 0.9408745000000000 | 0.0123389200000000 | 1.0 |
| O29 | O | 0.1338333000000000 | 0.9958333400000000 | 0.9231118700000000 | 1.0 |
| O30 | O | 0.2415579100000000 | 0.9971523900000000 | 0.0580766400000000 | 1.0 |
| O31 | O | 0.6338277800000000 | 0.9958069100000000 | 0.9231490000000000 | 1.0 |
| O32 | O | 0.7415915600000000 | 0.9971773500000000 | 0.0581030800000000 | 1.0 |
| F33 | F | 0.0025820300000000 | 0.0738145700000000 | 0.0685405900000000 | 1.0 |
| F34 | F | 0.3728270700000000 | 0.0721726000000000 | 0.9110980300000000 | 1.0 |
| F35 | F | 0.5025268500000000 | 0.0738325600000000 | 0.0685407300000000 | 1.0 |
| F36 | F | 0.8728022500000000 | 0.0722040300000000 | 0.9111129000000000 | 1.0 |

##### cif ends

  furan\_F\_3\_syn\_alt  Energy: -228.15332605

##### cif starts

data\_furan\_F\_3\_syn\_alt

\_publ\_section\_comment

;  
Andrew Reynoso, Bohan Xu, and Vincent H. Crespi  
;

\_cell\_length\_a  10.2982096564

\_cell\_length\_b  20.0

\_cell\_length\_c  20.0

\_cell\_angle\_alpha  90.0

\_cell\_angle\_beta  90.0

\_cell\_angle\_gamma  90.0

\_symmetry\_space\_group\_name\_H-M  'P 1'

\_symmetry\_Int\_Tables\_number  1

\_symmetry\_cell\_setting  triclinic

loop\_

\_atom\_site\_label

\_atom\_site\_type\_symbol

\_atom\_site\_fract\_x

\_atom\_site\_fract\_y

\_atom\_site\_fract\_z

\_atom\_site\_occupancy

|     |   |                    |                    |                    |     |
|-----|---|--------------------|--------------------|--------------------|-----|
| H1  | H | 0.9913432800000000 | 0.9034765300000000 | 0.0467777200000000 | 1.0 |
| H2  | H | 0.1165594000000000 | 0.0628477500000000 | 0.9239367200000000 | 1.0 |
| H3  | H | 0.9916212400000000 | 0.1073344700000000 | 0.0415927000000000 | 1.0 |
| H4  | H | 0.2413807000000000 | 0.1072756000000000 | 0.0416741300000000 | 1.0 |
| H5  | H | 0.3665825100000000 | 0.9419353200000000 | 0.9269471000000000 | 1.0 |
| H6  | H | 0.2416971400000000 | 0.9034112000000000 | 0.0466906700000000 | 1.0 |
| H7  | H | 0.4913291600000000 | 0.9034893100000000 | 0.0467836700000000 | 1.0 |
| H8  | H | 0.6165821600000000 | 0.0628473200000000 | 0.9239342100000000 | 1.0 |
| H9  | H | 0.4916233900000000 | 0.1073472600000000 | 0.0415793600000000 | 1.0 |
| H10 | H | 0.7413924900000000 | 0.1072765100000000 | 0.0416742300000000 | 1.0 |
| H11 | H | 0.8665678400000000 | 0.9419272700000000 | 0.9269534000000000 | 1.0 |
| H12 | H | 0.7416825000000000 | 0.9034125200000000 | 0.0467010300000000 | 1.0 |



|     |   |                    |                    |                    |     |
|-----|---|--------------------|--------------------|--------------------|-----|
| C13 | C | 0.9905097300000000 | 0.9506914300000000 | 0.0188241500000000 | 1.0 |
| C14 | C | 0.1165110200000000 | 0.9648173800000000 | 0.9783195800000000 | 1.0 |
| C15 | C | 0.1165144000000000 | 0.0432021700000000 | 0.9750771000000000 | 1.0 |
| C16 | C | 0.9925023100000000 | 0.0587523100000000 | 0.0160836300000000 | 1.0 |
| C17 | C | 0.2405064400000000 | 0.0587184800000000 | 0.0161182400000000 | 1.0 |
| C18 | C | 0.3664916300000000 | 0.0425918600000000 | 0.9763545200000000 | 1.0 |
| C19 | C | 0.3665295400000000 | 0.9641440000000000 | 0.9770394800000000 | 1.0 |
| C20 | C | 0.2425359700000000 | 0.9506555400000000 | 0.0187860500000000 | 1.0 |
| C21 | C | 0.4905059700000000 | 0.9507008500000000 | 0.0188252200000000 | 1.0 |
| C22 | C | 0.6165119900000000 | 0.9648200000000000 | 0.9783236000000000 | 1.0 |
| C23 | C | 0.6165211400000000 | 0.0432048100000000 | 0.9750760300000000 | 1.0 |
| C24 | C | 0.4925025300000000 | 0.0587615200000000 | 0.0160758100000000 | 1.0 |
| C25 | C | 0.7405103000000000 | 0.0587184200000000 | 0.0161206300000000 | 1.0 |
| C26 | C | 0.8664943900000000 | 0.0425850500000000 | 0.9763596600000000 | 1.0 |
| C27 | C | 0.8665260100000000 | 0.9641371300000000 | 0.9770451100000000 | 1.0 |
| C28 | C | 0.7425317800000000 | 0.9506554800000000 | 0.0187937300000000 | 1.0 |
| O29 | O | 0.9914837600000000 | 0.0059346000000000 | 0.0651113600000000 | 1.0 |
| O30 | O | 0.2415152600000000 | 0.0058602200000000 | 0.0651112300000000 | 1.0 |
| O31 | O | 0.4914790000000000 | 0.0059483000000000 | 0.0651081700000000 | 1.0 |
| O32 | O | 0.7415131200000000 | 0.0058624100000000 | 0.0651161200000000 | 1.0 |
| F33 | F | 0.1164473300000000 | 0.9324049500000000 | 0.9159880900000000 | 1.0 |
| F34 | F | 0.3663982900000000 | 0.0718769300000000 | 0.9124926000000000 | 1.0 |
| F35 | F | 0.6164507800000000 | 0.9324037300000000 | 0.9159939400000000 | 1.0 |
| F36 | F | 0.8664104800000000 | 0.0718683600000000 | 0.9124970000000000 | 1.0 |

##### cif ends

furan\_F\_3\_syn\_alt\_forbid Energy: -225.71224735

##### cif starts

data\_furan\_F\_3\_syn\_alt\_forbid

\_publ\_section\_comment

;  
Andrew Reynoso, Bohan Xu, and Vincent H. Crespi  
;

\_cell\_length\_a 9.4899579599

\_cell\_length\_b 20.0

\_cell\_length\_c 20.0

\_cell\_angle\_alpha 90.0

\_cell\_angle\_beta 90.0

\_cell\_angle\_gamma 90.0

\_symmetry\_space\_group\_name\_H-M 'P 1'

\_symmetry\_Int\_Tables\_number 1

\_symmetry\_cell\_setting triclinic

loop\_

\_atom\_site\_label

\_atom\_site\_type\_symbol

\_atom\_site\_fract\_x

\_atom\_site\_fract\_y

\_atom\_site\_fract\_z

\_atom\_site\_occupancy

H1 H 0.8977624500000000 0.1004135800000000 0.0619910500000000 1.0

|     |   |                    |                    |                    |     |
|-----|---|--------------------|--------------------|--------------------|-----|
| H2  | H | 0.9025442700000000 | 0.0621517100000000 | 0.9259874700000000 | 1.0 |
| H3  | H | 0.9001384800000000 | 0.8980729100000000 | 0.0616026100000000 | 1.0 |
| H4  | H | 0.1529021900000000 | 0.0992096500000000 | 0.0650787300000000 | 1.0 |
| H5  | H | 0.1503638300000000 | 0.9399152300000000 | 0.9239051500000000 | 1.0 |
| H6  | H | 0.1548770400000000 | 0.8969736600000000 | 0.0585257200000000 | 1.0 |
| H7  | H | 0.3979515000000000 | 0.1002461800000000 | 0.0620555900000000 | 1.0 |
| H8  | H | 0.4023576800000000 | 0.0620099200000000 | 0.9260158400000000 | 1.0 |
| H9  | H | 0.3999270200000000 | 0.8979047000000000 | 0.0615773100000000 | 1.0 |
| H10 | H | 0.6527303000000000 | 0.0993001200000000 | 0.0648900100000000 | 1.0 |
| H11 | H | 0.6504147000000000 | 0.9397542500000000 | 0.9239963100000000 | 1.0 |
| H12 | H | 0.6550819400000000 | 0.8970543600000000 | 0.0586958000000000 | 1.0 |
| C13 | C | 0.8604213600000000 | 0.0551332500000000 | 0.0365595800000000 | 1.0 |
| C14 | C | 0.9416470700000000 | 0.0390620700000000 | 0.9720054600000000 | 1.0 |
| C15 | C | 0.9448136000000000 | 0.9610422500000000 | 0.9723025900000000 | 1.0 |
| C16 | C | 0.8627491500000000 | 0.9435184900000000 | 0.0364880300000000 | 1.0 |
| C17 | C | 0.1901542400000000 | 0.0546325000000000 | 0.0384115800000000 | 1.0 |
| C18 | C | 0.1080294100000000 | 0.0393467600000000 | 0.9736719400000000 | 1.0 |
| C19 | C | 0.1111895000000000 | 0.9613869000000000 | 0.9706846500000000 | 1.0 |
| C20 | C | 0.1923467400000000 | 0.9430810500000000 | 0.0346684300000000 | 1.0 |
| C21 | C | 0.3604835900000000 | 0.0549978200000000 | 0.0366122600000000 | 1.0 |
| C22 | C | 0.4415967200000000 | 0.0389346900000000 | 0.9720125400000000 | 1.0 |
| C23 | C | 0.4448221800000000 | 0.9609141500000000 | 0.9723275600000000 | 1.0 |
| C24 | C | 0.3626716100000000 | 0.9433830300000000 | 0.0364731400000000 | 1.0 |
| C25 | C | 0.6900977400000000 | 0.0546920200000000 | 0.0383084200000000 | 1.0 |
| C26 | C | 0.6079789000000000 | 0.0392583800000000 | 0.9736054000000000 | 1.0 |
| C27 | C | 0.6112012100000000 | 0.9612955400000000 | 0.9707363200000000 | 1.0 |
| C28 | C | 0.6924171500000000 | 0.9431350400000000 | 0.0347434800000000 | 1.0 |
| O29 | O | 0.8963505400000000 | 0.9990599900000000 | 0.0782981800000000 | 1.0 |
| O30 | O | 0.1565143700000000 | 0.9977018700000000 | 0.0783034300000000 | 1.0 |
| O31 | O | 0.3963444400000000 | 0.9988833700000000 | 0.0783168000000000 | 1.0 |
| O32 | O | 0.6565313300000000 | 0.9978193600000000 | 0.0782931600000000 | 1.0 |
| F33 | F | 0.8913320300000000 | 0.9279760800000000 | 0.9156030700000000 | 1.0 |
| F34 | F | 0.1614878000000000 | 0.0743449100000000 | 0.9181388200000000 | 1.0 |
| F35 | F | 0.3914381600000000 | 0.9278298800000000 | 0.9156151200000000 | 1.0 |
| F36 | F | 0.6613379700000000 | 0.0741677900000000 | 0.9179981200000000 | 1.0 |

##### cif ends

furand\_F\_3\_syn\_dir Energy: -227.57664629

##### cif starts

data\_furand\_F\_3\_syn\_dir

\_publ\_section\_comment

;  
Andrew Reynoso, Bohan Xu, and Vincent H. Crespi  
;

\_cell\_length\_a 10.3517876351

\_cell\_length\_b 20.0

\_cell\_length\_c 20.0

\_cell\_angle\_alpha 90.0

\_cell\_angle\_beta 90.0

\_cell\_angle\_gamma 90.0

\_symmetry\_space\_group\_name\_H-M 'P 1'

\_symmetry\_Int\_Tables\_number 1  
\_symmetry\_cell\_setting triclinic

loop\_  
\_atom\_site\_label  
\_atom\_site\_type\_symbol  
\_atom\_site\_fract\_x  
\_atom\_site\_fract\_y  
\_atom\_site\_fract\_z  
\_atom\_site\_occupancy

|     |   |                    |                    |                    |     |
|-----|---|--------------------|--------------------|--------------------|-----|
| H1  | H | 0.9581850700000000 | 0.0625547100000000 | 0.9042208400000000 | 1.0 |
| H2  | H | 0.0831773400000000 | 0.9863708300000000 | 0.0902876700000000 | 1.0 |
| H3  | H | 0.9581899000000000 | 0.8887553000000000 | 0.0109132500000000 | 1.0 |
| H4  | H | 0.2081913300000000 | 0.0625333000000000 | 0.9042120400000000 | 1.0 |
| H5  | H | 0.3332011900000000 | 0.9863710700000000 | 0.0902887800000000 | 1.0 |
| H6  | H | 0.2081907900000000 | 0.8887532400000000 | 0.0109352100000000 | 1.0 |
| H7  | H | 0.4581958400000000 | 0.0625537600000000 | 0.9042221600000000 | 1.0 |
| H8  | H | 0.5831709700000000 | 0.9863715900000000 | 0.0902932700000000 | 1.0 |
| H9  | H | 0.4581925100000000 | 0.8887552900000000 | 0.0109164200000000 | 1.0 |
| H10 | H | 0.7081889100000000 | 0.0625347200000000 | 0.9042182000000000 | 1.0 |
| H11 | H | 0.8332173400000000 | 0.9863716100000000 | 0.0902919900000000 | 1.0 |
| H12 | H | 0.7081916800000000 | 0.8887549100000000 | 0.0109432600000000 | 1.0 |
| C13 | C | 0.9581881200000000 | 0.0352821300000000 | 0.9517990500000000 | 1.0 |
| C14 | C | 0.0831925500000000 | 0.0438960300000000 | 0.9945639100000000 | 1.0 |
| C15 | C | 0.0831896900000000 | 0.9772072200000000 | 0.0361594000000000 | 1.0 |
| C16 | C | 0.9581915200000000 | 0.9436382100000000 | 0.0091974600000000 | 1.0 |
| C17 | C | 0.2081902100000000 | 0.0352720300000000 | 0.9517965700000000 | 1.0 |
| C18 | C | 0.3331905900000000 | 0.0438958500000000 | 0.9945647800000000 | 1.0 |
| C19 | C | 0.3331937000000000 | 0.9772072700000000 | 0.0361605300000000 | 1.0 |
| C20 | C | 0.2081916700000000 | 0.9436358600000000 | 0.0092079000000000 | 1.0 |
| C21 | C | 0.4581916300000000 | 0.0352816100000000 | 0.9518005700000000 | 1.0 |
| C22 | C | 0.5831918400000000 | 0.0438967400000000 | 0.9945693000000000 | 1.0 |
| C23 | C | 0.5831880500000000 | 0.9772083000000000 | 0.0361648700000000 | 1.0 |
| C24 | C | 0.4581925000000000 | 0.9436382500000000 | 0.0091998300000000 | 1.0 |
| C25 | C | 0.7081895600000000 | 0.0352732000000000 | 0.9518024500000000 | 1.0 |
| C26 | C | 0.8331921400000000 | 0.0438968900000000 | 0.9945681500000000 | 1.0 |
| C27 | C | 0.8331977800000000 | 0.9772083000000000 | 0.0361635700000000 | 1.0 |
| C28 | C | 0.7081920100000000 | 0.9436375600000000 | 0.0092145900000000 | 1.0 |
| O29 | O | 0.9581887400000000 | 0.9647424200000000 | 0.9397592000000000 | 1.0 |
| O30 | O | 0.2081921300000000 | 0.9647297100000000 | 0.9397671900000000 | 1.0 |
| O31 | O | 0.4581951400000000 | 0.9647417000000000 | 0.9397613600000000 | 1.0 |
| O32 | O | 0.7081909400000000 | 0.9647303500000000 | 0.9397737100000000 | 1.0 |
| F33 | F | 0.0832007400000000 | 0.1024321700000000 | 0.0321929700000000 | 1.0 |
| F34 | F | 0.3331872400000000 | 0.1024321800000000 | 0.0321936800000000 | 1.0 |
| F35 | F | 0.5831974700000000 | 0.1024327900000000 | 0.0321984900000000 | 1.0 |
| F36 | F | 0.8331921600000000 | 0.1024329300000000 | 0.0321973600000000 | 1.0 |

##### cif ends

uran\_F\_3\_syn\_dir\_forbid Energy: -224.86904317

##### cif starts

data\_uran\_F\_3\_syn\_dir\_forbid

\_publ\_section\_comment

;

;

```
_cell_length_a  9.5448743448
_cell_length_b  20.0
_cell_length_c  20.0
_cell_angle_alpha  90.0
_cell_angle_beta  90.0
_cell_angle_gamma  90.0
```

```
_symmetry_space_group_name_H-M  'P 1'
_symmetry_Int_Tables_number 1
_symmetry_cell_setting triclinic
```

```
loop_
_atom_site_label
_atom_site_type_symbol
_atom_site_fract_x
_atom_site_fract_y
_atom_site_fract_z
_atom_site_occupancy
H1  H  0.8621044800000000  0.1130774600000000  0.0479522300000000  1.0
H2  H  0.8594506400000000  0.9401530500000000  0.9274631100000000  1.0
H3  H  0.8816584000000000  0.9117466000000000  0.0679640200000000  1.0
H4  H  0.1316665400000000  0.0850308700000000  0.0727770000000000  1.0
H5  H  0.1109675100000000  0.9455566800000000  0.9116078900000000  1.0
H6  H  0.1229429100000000  0.8856918500000000  0.0381837600000000  1.0
H7  H  0.3753951100000000  0.0861627200000000  0.0611769300000000  1.0
H8  H  0.3934958500000000  0.9288721600000000  0.9177866200000000  1.0
H9  H  0.3631740000000000  0.8842032000000000  0.0500047200000000  1.0
H10 H  0.6177646600000000  0.1080914800000000  0.0458025400000000  1.0
H11 H  0.6429767700000000  0.9307695000000000  0.9304921400000000  1.0
H12 H  0.6363003200000000  0.9073748800000000  0.0709227100000000  1.0
C13 C  0.8289665800000000  0.0644494400000000  0.0280247200000000  1.0
C14 C  0.9153675900000000  0.0416302100000000  0.9679045500000000  1.0
C15 C  0.9126240500000000  0.9639052100000000  0.9697760700000000  1.0
C16 C  0.8393313300000000  0.9531274200000000  0.0382125800000000  1.0
C17 C  0.1628920200000000  0.0441229000000000  0.0394736100000000  1.0
C18 C  0.0810165100000000  0.0401497200000000  0.9732186800000000  1.0
C19 C  0.0799087700000000  0.9622403800000000  0.9616824900000000  1.0
C20 C  0.1637882500000000  0.9342731300000000  0.0214918800000000  1.0
C21 C  0.3338838900000000  0.0427159400000000  0.0342569100000000  1.0
C22 C  0.4149778800000000  0.0284674500000000  0.9674207000000000  1.0
C23 C  0.4238443500000000  0.9508257000000000  0.9659319500000000  1.0
C24 C  0.3335617000000000  0.9314924700000000  0.0259290400000000  1.0
C25 C  0.6606388300000000  0.0606751300000000  0.0272431400000000  1.0
C26 C  0.5816889000000000  0.0334954300000000  0.9660729000000000  1.0
C27 C  0.5908394300000000  0.9558073100000000  0.9723794100000000  1.0
C28 C  0.6689797100000000  0.9496578000000000  0.0396557200000000  1.0
O29 O  0.8702919900000000  0.0139954800000000  0.0745095500000000  1.0
O30 O  0.1282461200000000  0.9826465400000000  0.0718535200000000  1.0
O31 O  0.3687917000000000  0.9841686600000000  0.0718851500000000  1.0
O32 O  0.6286127300000000  0.0097547700000000  0.0748062600000000  1.0
F33 F  0.8814008300000000  0.0709976500000000  0.9073011200000000  1.0
F34 F  0.1315699400000000  0.0848604500000000  0.9263224800000000  1.0
```

F35 F 0.3661946900000000 0.0583634400000000 0.9098068800000000 1.0  
F36 F 0.6216938300000000 0.0608221100000000 0.9054600100000000 1.0

##### cif ends

furand\_NH2\_234\_anti\_alt Energy: -369.82946076

##### cif starts

data\_furand\_NH2\_234\_anti\_alt

\_publ\_section\_comment

;  
Andrew Reynoso, Bohan Xu, and Vincent H. Crespi  
;

\_cell\_length\_a 9.7507848692

\_cell\_length\_b 20.0

\_cell\_length\_c 20.0

\_cell\_angle\_alpha 90.0

\_cell\_angle\_beta 90.0

\_cell\_angle\_gamma 90.0

\_symmetry\_space\_group\_name\_H-M 'P 1'

\_symmetry\_Int\_Tables\_number 1

\_symmetry\_cell\_setting triclinic

loop\_

\_atom\_site\_label

\_atom\_site\_type\_symbol

\_atom\_site\_fract\_x

\_atom\_site\_fract\_y

\_atom\_site\_fract\_z

\_atom\_site\_occupancy

|     |   |                    |                    |                    |     |
|-----|---|--------------------|--------------------|--------------------|-----|
| H1  | H | 0.0518697600000000 | 0.8900360100000000 | 0.9317102900000000 | 1.0 |
| H2  | H | 0.1280785700000000 | 0.1326508600000000 | 0.9149551300000000 | 1.0 |
| H3  | H | 0.9588197600000000 | 0.1233013200000000 | 0.9336561600000000 | 1.0 |
| H4  | H | 0.9731600300000000 | 0.0461864300000000 | 0.1261128900000000 | 1.0 |
| H5  | H | 0.0508629800000000 | 0.1045549000000000 | 0.0822520900000000 | 1.0 |
| H6  | H | 0.1262393300000000 | 0.9405560200000000 | 0.0967030100000000 | 1.0 |
| H7  | H | 0.9715270700000000 | 0.9199166200000000 | 0.1186544800000000 | 1.0 |
| H8  | H | 0.3021203600000000 | 0.0852977300000000 | 0.0521086000000000 | 1.0 |
| H9  | H | 0.3782808800000000 | 0.8427917900000000 | 0.0692765600000000 | 1.0 |
| H10 | H | 0.2088839500000000 | 0.8521648100000000 | 0.0508325400000000 | 1.0 |
| H11 | H | 0.2230713100000000 | 0.9289654400000000 | 0.8579339200000000 | 1.0 |
| H12 | H | 0.3005092700000000 | 0.8705507400000000 | 0.9018051400000000 | 1.0 |
| H13 | H | 0.2212677400000000 | 0.0553602900000000 | 0.8653425200000000 | 1.0 |
| H14 | H | 0.3759823100000000 | 0.0345146300000000 | 0.8871567600000000 | 1.0 |
| H15 | H | 0.5521360500000000 | 0.8899336300000000 | 0.9317665800000000 | 1.0 |
| H16 | H | 0.4587287200000000 | 0.1229164800000000 | 0.9326759800000000 | 1.0 |
| H17 | H | 0.6281724600000000 | 0.1324109600000000 | 0.9143628500000000 | 1.0 |
| H18 | H | 0.4736927300000000 | 0.0465748300000000 | 0.1258540700000000 | 1.0 |
| H19 | H | 0.5505931600000000 | 0.1049288200000000 | 0.0816714300000000 | 1.0 |
| H20 | H | 0.4715899500000000 | 0.9202672800000000 | 0.1186227100000000 | 1.0 |
| H21 | H | 0.6263701300000000 | 0.9407795400000000 | 0.0965954300000000 | 1.0 |
| H22 | H | 0.8020875800000000 | 0.0852729000000000 | 0.0521663600000000 | 1.0 |
| H23 | H | 0.8777833400000000 | 0.8427237900000000 | 0.0693841600000000 | 1.0 |

|     |   |                    |                    |                    |     |
|-----|---|--------------------|--------------------|--------------------|-----|
| H24 | H | 0.7084629800000000 | 0.8522785900000000 | 0.0509284700000000 | 1.0 |
| H25 | H | 0.7241444600000000 | 0.9295986400000000 | 0.8577732800000000 | 1.0 |
| H26 | H | 0.7993218900000000 | 0.8704439100000000 | 0.9015946900000000 | 1.0 |
| H27 | H | 0.7221009000000000 | 0.0551578300000000 | 0.8652002400000000 | 1.0 |
| H28 | H | 0.8768752300000000 | 0.0348144600000000 | 0.8874457700000000 | 1.0 |
| C29 | C | 0.0770928700000000 | 0.9364097100000000 | 0.9581004700000000 | 1.0 |
| C30 | C | 0.9904537700000000 | 0.9473619400000000 | 0.0216885600000000 | 1.0 |
| C31 | C | 0.9890790700000000 | 0.0260968800000000 | 0.0262750100000000 | 1.0 |
| C32 | C | 0.0809824300000000 | 0.0469695900000000 | 0.9657609000000000 | 1.0 |
| C33 | C | 0.3272238100000000 | 0.0388628400000000 | 0.0257955600000000 | 1.0 |
| C34 | C | 0.2404797200000000 | 0.0278251200000000 | 0.9622865900000000 | 1.0 |
| C35 | C | 0.2390052600000000 | 0.9490894000000000 | 0.9577508800000000 | 1.0 |
| C36 | C | 0.3309728800000000 | 0.9283080700000000 | 0.0182867300000000 | 1.0 |
| C37 | C | 0.5772487500000000 | 0.9363890100000000 | 0.9580454400000000 | 1.0 |
| C38 | C | 0.4905565300000000 | 0.9474746900000000 | 0.0215995800000000 | 1.0 |
| C39 | C | 0.4890934100000000 | 0.0262194300000000 | 0.0260406800000000 | 1.0 |
| C40 | C | 0.5809406200000000 | 0.0469454000000000 | 0.9654420100000000 | 1.0 |
| C41 | C | 0.8271852900000000 | 0.0388383100000000 | 0.0258549900000000 | 1.0 |
| C42 | C | 0.7405961500000000 | 0.0278299200000000 | 0.9622370600000000 | 1.0 |
| C43 | C | 0.7391350900000000 | 0.9490892100000000 | 0.9577404400000000 | 1.0 |
| C44 | C | 0.8308688100000000 | 0.9282699100000000 | 0.0183388900000000 | 1.0 |
| N45 | N | 0.0424967200000000 | 0.9132509600000000 | 0.0814727800000000 | 1.0 |
| N46 | N | 0.0424237000000000 | 0.0539363700000000 | 0.0885219600000000 | 1.0 |
| N47 | N | 0.0579674700000000 | 0.1140712800000000 | 0.9477515500000000 | 1.0 |
| N48 | N | 0.2924083400000000 | 0.0619057700000000 | 0.9024616200000000 | 1.0 |
| N49 | N | 0.2923357300000000 | 0.9211802700000000 | 0.8955211200000000 | 1.0 |
| N50 | N | 0.3079677600000000 | 0.8612591900000000 | 0.0365124800000000 | 1.0 |
| N51 | N | 0.5425426700000000 | 0.9134791000000000 | 0.0814593700000000 | 1.0 |
| N52 | N | 0.5426783600000000 | 0.0543083600000000 | 0.0881389700000000 | 1.0 |
| N53 | N | 0.5578066700000000 | 0.1139568300000000 | 0.9471068900000000 | 1.0 |
| N54 | N | 0.7927630200000000 | 0.0619452900000000 | 0.9024926700000000 | 1.0 |
| N55 | N | 0.7926302900000000 | 0.9211548500000000 | 0.8955562200000000 | 1.0 |
| N56 | N | 0.8075932500000000 | 0.8612442400000000 | 0.0365887000000000 | 1.0 |
| O57 | O | 0.0372261600000000 | 0.9931218200000000 | 0.9170375600000000 | 1.0 |
| O58 | O | 0.2873767200000000 | 0.9822222900000000 | 0.0669378800000000 | 1.0 |
| O59 | O | 0.5374018900000000 | 0.9929946000000000 | 0.9168544100000000 | 1.0 |
| O60 | O | 0.7872268900000000 | 0.9822070800000000 | 0.0669649300000000 | 1.0 |

##### cif ends

furan\_NH2\_234\_anti\_alt\_forbid Energy: -370.81434944

##### cif starts

data\_furan\_NH2\_234\_anti\_alt\_forbid

\_publ\_section\_comment

;  
Andrew Reynoso, Bohan Xu, and Vincent H. Crespi  
;

\_cell\_length\_a 10.3483524385

\_cell\_length\_b 20.0

\_cell\_length\_c 20.0

\_cell\_angle\_alpha 90.0

\_cell\_angle\_beta 90.0

\_cell\_angle\_gamma 90.0

\_symmetry\_space\_group\_name\_H-M 'P 1'

\_symmetry\_Int\_Tables\_number 1

\_symmetry\_cell\_setting triclinic

loop\_

\_atom\_site\_label

\_atom\_site\_type\_symbol

\_atom\_site\_fract\_x

\_atom\_site\_fract\_y

\_atom\_site\_fract\_z

\_atom\_site\_occupancy

|     |   |                    |                    |                    |     |
|-----|---|--------------------|--------------------|--------------------|-----|
| H1  | H | 0.0598139400000000 | 0.0971119800000000 | 0.9304300700000000 | 1.0 |
| H2  | H | 0.2071634700000000 | 0.8959274400000000 | 0.0347914400000000 | 1.0 |
| H3  | H | 0.5597872300000000 | 0.0970355200000000 | 0.9303510900000000 | 1.0 |
| H4  | H | 0.7072456000000000 | 0.8959865700000000 | 0.0349061000000000 | 1.0 |
| H5  | H | 0.2441271100000000 | 0.0640722300000000 | 0.8722980300000000 | 1.0 |
| H6  | H | 0.4022288500000000 | 0.0652574000000000 | 0.8744650900000000 | 1.0 |
| H7  | H | 0.7441630900000000 | 0.0640904000000000 | 0.8722474200000000 | 1.0 |
| H8  | H | 0.9022849100000000 | 0.0651659500000000 | 0.8744148500000000 | 1.0 |
| H9  | H | 0.3660486700000000 | 0.9513849600000000 | 0.8628206200000000 | 1.0 |
| H10 | H | 0.2302340500000000 | 0.9098952900000000 | 0.8820778300000000 | 1.0 |
| H11 | H | 0.8652359600000000 | 0.9515203100000000 | 0.8626907400000000 | 1.0 |
| H12 | H | 0.7300088400000000 | 0.9096903600000000 | 0.8822289300000000 | 1.0 |
| H13 | H | 0.8662985100000000 | 0.9382856500000000 | 0.0954952200000000 | 1.0 |
| H14 | H | 0.0222200400000000 | 0.9251943700000000 | 0.0926956900000000 | 1.0 |
| H15 | H | 0.3660805300000000 | 0.9383893900000000 | 0.0955405100000000 | 1.0 |
| H16 | H | 0.5220328600000000 | 0.9253590900000000 | 0.0928560000000000 | 1.0 |
| H17 | H | 0.9964012000000000 | 0.0439619100000000 | 0.1031842700000000 | 1.0 |
| H18 | H | 0.8591784600000000 | 0.0847106500000000 | 0.0837167500000000 | 1.0 |
| H19 | H | 0.4966349900000000 | 0.0440817000000000 | 0.1031632300000000 | 1.0 |
| H20 | H | 0.3592639600000000 | 0.0847197000000000 | 0.0837608100000000 | 1.0 |
| H21 | H | 0.1104402200000000 | 0.1298881100000000 | 0.0563159300000000 | 1.0 |
| H22 | H | 0.2450537200000000 | 0.1523079000000000 | 0.0137551100000000 | 1.0 |
| H23 | H | 0.6104985500000000 | 0.1299915400000000 | 0.0561726200000000 | 1.0 |
| H24 | H | 0.7451261600000000 | 0.1523306300000000 | 0.0135720800000000 | 1.0 |
| H25 | H | 0.9720109100000000 | 0.8679683100000000 | 0.9093317400000000 | 1.0 |
| H26 | H | 0.0995036900000000 | 0.8377422500000000 | 0.9523993800000000 | 1.0 |
| H27 | H | 0.4719912700000000 | 0.8677984700000000 | 0.9096050100000000 | 1.0 |
| H28 | H | 0.5995077100000000 | 0.8376945800000000 | 0.9527307800000000 | 1.0 |
| C29 | C | 0.0680252000000000 | 0.0514578700000000 | 0.9607644500000000 | 1.0 |
| C30 | C | 0.9473811600000000 | 0.0369896200000000 | 0.0047198500000000 | 1.0 |
| C31 | C | 0.9453298900000000 | 0.9567261900000000 | 0.0043331000000000 | 1.0 |
| C32 | C | 0.0681019500000000 | 0.9376369300000000 | 0.9625727900000000 | 1.0 |
| C33 | C | 0.1938490900000000 | 0.0551812700000000 | 0.0037703100000000 | 1.0 |
| C34 | C | 0.3174429500000000 | 0.0383841900000000 | 0.9627904300000000 | 1.0 |
| C35 | C | 0.3163849200000000 | 0.9576515100000000 | 0.9614479700000000 | 1.0 |
| C36 | C | 0.1952546800000000 | 0.9413115700000000 | 0.0043369000000000 | 1.0 |
| C37 | C | 0.5680106500000000 | 0.0514182300000000 | 0.9607381600000000 | 1.0 |
| C38 | C | 0.4473897200000000 | 0.0370138000000000 | 0.0047384800000000 | 1.0 |
| C39 | C | 0.4453042700000000 | 0.9567529900000000 | 0.0044131000000000 | 1.0 |
| C40 | C | 0.5680742700000000 | 0.9376032600000000 | 0.9626969900000000 | 1.0 |
| C41 | C | 0.6938646100000000 | 0.0552006400000000 | 0.0037145600000000 | 1.0 |
| C42 | C | 0.8174475400000000 | 0.0383605300000000 | 0.9627489900000000 | 1.0 |
| C43 | C | 0.8163383700000000 | 0.9576365100000000 | 0.9614312800000000 | 1.0 |

|     |   |                    |                    |                    |     |
|-----|---|--------------------|--------------------|--------------------|-----|
| C44 | C | 0.6952713700000000 | 0.9413376000000000 | 0.0044073400000000 | 1.0 |
| N45 | N | 0.9386398000000000 | 0.9195104400000000 | 0.0660825900000000 | 1.0 |
| N46 | N | 0.0655009600000000 | 0.8767743200000000 | 0.9248486800000000 | 1.0 |
| N47 | N | 0.9504000000000000 | 0.0723152300000000 | 0.0679898200000000 | 1.0 |
| N48 | N | 0.3214677200000000 | 0.0766530700000000 | 0.9015449500000000 | 1.0 |
| N49 | N | 0.2018817900000000 | 0.1159770600000000 | 0.0417453500000000 | 1.0 |
| N50 | N | 0.3209811100000000 | 0.9227880700000000 | 0.8981573900000000 | 1.0 |
| N51 | N | 0.4385202300000000 | 0.9196007500000000 | 0.0661997000000000 | 1.0 |
| N52 | N | 0.5654690000000000 | 0.8766612800000000 | 0.9250978600000000 | 1.0 |
| N53 | N | 0.4504844700000000 | 0.0723854400000000 | 0.0679818600000000 | 1.0 |
| N54 | N | 0.8215431400000000 | 0.0766094000000000 | 0.9014911700000000 | 1.0 |
| N55 | N | 0.7019206700000000 | 0.1160448600000000 | 0.0416065100000000 | 1.0 |
| N56 | N | 0.8207731100000000 | 0.9227863200000000 | 0.8981234200000000 | 1.0 |
| O57 | O | 0.0739733500000000 | 0.9947905900000000 | 0.9157669900000000 | 1.0 |
| O58 | O | 0.1875593600000000 | 0.9976254400000000 | 0.0497466700000000 | 1.0 |
| O59 | O | 0.5739162800000000 | 0.9946933800000000 | 0.9158045500000000 | 1.0 |
| O60 | O | 0.6876186800000000 | 0.9976963300000000 | 0.0497569600000000 | 1.0 |

##### cif ends

furand\_NH2\_234\_anti\_dir Energy: -369.48101011

##### cif starts

data\_furand\_NH2\_234\_anti\_dir

\_publ\_section\_comment

;  
Andrew Reynoso, Bohan Xu, and Vincent H. Crespi  
;

\_cell\_length\_a 9.7216448622

\_cell\_length\_b 20.0

\_cell\_length\_c 20.0

\_cell\_angle\_alpha 90.0

\_cell\_angle\_beta 90.0

\_cell\_angle\_gamma 90.0

\_symmetry\_space\_group\_name\_H-M 'P 1'

\_symmetry\_Int\_Tables\_number 1

\_symmetry\_cell\_setting triclinic

loop\_

\_atom\_site\_label

\_atom\_site\_type\_symbol

\_atom\_site\_fract\_x

\_atom\_site\_fract\_y

\_atom\_site\_fract\_z

\_atom\_site\_occupancy

|    |   |                    |                    |                    |     |
|----|---|--------------------|--------------------|--------------------|-----|
| H1 | H | 0.9938491100000000 | 0.1157348500000000 | 0.9372009300000000 | 1.0 |
|----|---|--------------------|--------------------|--------------------|-----|

|    |   |                    |                    |                    |     |
|----|---|--------------------|--------------------|--------------------|-----|
| H2 | H | 0.8894637200000000 | 0.8763738600000000 | 0.9508132400000000 | 1.0 |
|----|---|--------------------|--------------------|--------------------|-----|

|    |   |                    |                    |                    |     |
|----|---|--------------------|--------------------|--------------------|-----|
| H3 | H | 0.0211632400000000 | 0.8794759300000000 | 0.8965727700000000 | 1.0 |
|----|---|--------------------|--------------------|--------------------|-----|

|    |   |                    |                    |                    |     |
|----|---|--------------------|--------------------|--------------------|-----|
| H4 | H | 0.0589809000000000 | 0.9678679200000000 | 0.1061528800000000 | 1.0 |
|----|---|--------------------|--------------------|--------------------|-----|

|    |   |                    |                    |                    |     |
|----|---|--------------------|--------------------|--------------------|-----|
| H5 | H | 0.9819793100000000 | 0.8974741700000000 | 0.0866820200000000 | 1.0 |
|----|---|--------------------|--------------------|--------------------|-----|

|    |   |                    |                    |                    |     |
|----|---|--------------------|--------------------|--------------------|-----|
| H6 | H | 0.0682172100000000 | 0.0726899600000000 | 0.0995616400000000 | 1.0 |
|----|---|--------------------|--------------------|--------------------|-----|

|    |   |                    |                    |                    |     |
|----|---|--------------------|--------------------|--------------------|-----|
| H7 | H | 0.9087305600000000 | 0.0856854400000000 | 0.1212170000000000 | 1.0 |
|----|---|--------------------|--------------------|--------------------|-----|

|    |   |                    |                    |                    |     |
|----|---|--------------------|--------------------|--------------------|-----|
| H8 | H | 0.2404625900000000 | 0.1155279000000000 | 0.0461728400000000 | 1.0 |
|----|---|--------------------|--------------------|--------------------|-----|



|     |   |                    |                    |                    |     |
|-----|---|--------------------|--------------------|--------------------|-----|
| H9  | H | 0.1499449300000000 | 0.8730914500000000 | 0.0336059100000000 | 1.0 |
| H10 | H | 0.2804105600000000 | 0.8823212600000000 | 0.0898730500000000 | 1.0 |
| H11 | H | 0.1774224800000000 | 0.9663926100000000 | 0.8566977300000000 | 1.0 |
| H12 | H | 0.2180260000000000 | 0.8956055600000000 | 0.8948632700000000 | 1.0 |
| H13 | H | 0.1546357200000000 | 0.0895371900000000 | 0.8640219600000000 | 1.0 |
| H14 | H | 0.3118387700000000 | 0.0633996600000000 | 0.8818159300000000 | 1.0 |
| H15 | H | 0.4902825700000000 | 0.1176778800000000 | 0.9392830800000000 | 1.0 |
| H16 | H | 0.5613155700000000 | 0.8775253700000000 | 0.9045654500000000 | 1.0 |
| H17 | H | 0.4040088600000000 | 0.8751805500000000 | 0.9434612100000000 | 1.0 |
| H18 | H | 0.5557914500000000 | 0.9705819700000000 | 0.1068471600000000 | 1.0 |
| H19 | H | 0.4936194800000000 | 0.8982505400000000 | 0.0838584500000000 | 1.0 |
| H20 | H | 0.5649254600000000 | 0.0744439900000000 | 0.0997668800000000 | 1.0 |
| H21 | H | 0.4044100200000000 | 0.0822859200000000 | 0.1223637800000000 | 1.0 |
| H22 | H | 0.7452485100000000 | 0.1167247300000000 | 0.0497412800000000 | 1.0 |
| H23 | H | 0.6510645700000000 | 0.8735504000000000 | 0.0269624700000000 | 1.0 |
| H24 | H | 0.7691918000000000 | 0.8830045500000000 | 0.0898859800000000 | 1.0 |
| H25 | H | 0.6565061600000000 | 0.9670929800000000 | 0.8591669800000000 | 1.0 |
| H26 | H | 0.8172909100000000 | 0.9658781300000000 | 0.8827638300000000 | 1.0 |
| H27 | H | 0.6528423100000000 | 0.0950336900000000 | 0.8673527000000000 | 1.0 |
| H28 | H | 0.8117018200000000 | 0.0732145100000000 | 0.8842963900000000 | 1.0 |
| C29 | C | 0.0161986900000000 | 0.0675187500000000 | 0.9609248200000000 | 1.0 |
| C30 | C | 0.9286426700000000 | 0.0549090400000000 | 0.0248922400000000 | 1.0 |
| C31 | C | 0.9291424400000000 | 0.9758077900000000 | 0.0266542600000000 | 1.0 |
| C32 | C | 0.0176679800000000 | 0.9566721800000000 | 0.9643418100000000 | 1.0 |
| C33 | C | 0.2643714700000000 | 0.0672877800000000 | 0.0228933900000000 | 1.0 |
| C34 | C | 0.1780162600000000 | 0.0534326300000000 | 0.9592745500000000 | 1.0 |
| C35 | C | 0.1792248700000000 | 0.9740209600000000 | 0.9584843700000000 | 1.0 |
| C36 | C | 0.2690171100000000 | 0.9567181200000000 | 0.0206421600000000 | 1.0 |
| C37 | C | 0.5148526400000000 | 0.0693129200000000 | 0.9621861500000000 | 1.0 |
| C38 | C | 0.4264294900000000 | 0.0547541400000000 | 0.0250607600000000 | 1.0 |
| C39 | C | 0.4295912500000000 | 0.9758108100000000 | 0.0258398700000000 | 1.0 |
| C40 | C | 0.5202238300000000 | 0.9584946600000000 | 0.9635659000000000 | 1.0 |
| C41 | C | 0.7656549300000000 | 0.0689359600000000 | 0.0247618900000000 | 1.0 |
| C42 | C | 0.6771625300000000 | 0.0572868000000000 | 0.9617298600000000 | 1.0 |
| C43 | C | 0.6800136500000000 | 0.9776660600000000 | 0.9585441700000000 | 1.0 |
| C44 | C | 0.7688240200000000 | 0.9583401900000000 | 0.0207861500000000 | 1.0 |
| N45 | N | 0.9772401200000000 | 0.0918798600000000 | 0.0829620800000000 | 1.0 |
| N46 | N | 0.9676242900000000 | 0.9478065100000000 | 0.0911835000000000 | 1.0 |
| N47 | N | 0.9890659400000000 | 0.8907680400000000 | 0.9435944200000000 | 1.0 |
| N48 | N | 0.2283109600000000 | 0.0884154500000000 | 0.9003667300000000 | 1.0 |
| N49 | N | 0.2297854300000000 | 0.9462851000000000 | 0.8961356000000000 | 1.0 |
| N50 | N | 0.2463014600000000 | 0.8906908000000000 | 0.0425078800000000 | 1.0 |
| N51 | N | 0.4714557300000000 | 0.0914241400000000 | 0.0840610500000000 | 1.0 |
| N52 | N | 0.4688596300000000 | 0.9474174300000000 | 0.0901891100000000 | 1.0 |
| N53 | N | 0.5024279800000000 | 0.8916960900000000 | 0.9441843800000000 | 1.0 |
| N54 | N | 0.7258718100000000 | 0.0949280100000000 | 0.9040456400000000 | 1.0 |
| N55 | N | 0.7218800500000000 | 0.9482931700000000 | 0.8946961000000000 | 1.0 |
| N56 | N | 0.7441845500000000 | 0.8919755100000000 | 0.0413684100000000 | 1.0 |
| O57 | O | 0.9720415100000000 | 0.0128811700000000 | 0.9179329700000000 | 1.0 |
| O58 | O | 0.2205115000000000 | 0.0127525300000000 | 0.0657261900000000 | 1.0 |
| O59 | O | 0.4733900900000000 | 0.0154337500000000 | 0.9179526600000000 | 1.0 |
| O60 | O | 0.7216165400000000 | 0.0137306300000000 | 0.0666101200000000 | 1.0 |

##### cif ends

furand\_NH2\_234\_anti\_dir\_forbid Energy: -369.8723918

##### cif starts

data\_furand\_NH2\_234\_anti\_dir\_forbid

\_publ\_section\_comment

;  
Andrew Reynoso, Bohan Xu, and Vincent H. Crespi  
;

\_cell\_length\_a 10.4239022529

\_cell\_length\_b 20.0

\_cell\_length\_c 20.0

\_cell\_angle\_alpha 90.0

\_cell\_angle\_beta 90.0

\_cell\_angle\_gamma 90.0

\_symmetry\_space\_group\_name\_H-M 'P 1'

\_symmetry\_Int\_Tables\_number 1

\_symmetry\_cell\_setting triclinic

loop\_

\_atom\_site\_label

\_atom\_site\_type\_symbol

\_atom\_site\_fract\_x

\_atom\_site\_fract\_y

\_atom\_site\_fract\_z

\_atom\_site\_occupancy

|     |   |                    |                    |                    |     |
|-----|---|--------------------|--------------------|--------------------|-----|
| H1  | H | 0.0811584700000000 | 0.1122497800000000 | 0.9332675700000000 | 1.0 |
| H2  | H | 0.1575575700000000 | 0.8677335800000000 | 0.9124545400000000 | 1.0 |
| H3  | H | 0.0128684800000000 | 0.8964272700000000 | 0.8871570900000000 | 1.0 |
| H4  | H | 0.0378913200000000 | 0.9583155000000000 | 0.0970997500000000 | 1.0 |
| H5  | H | 0.9779612300000000 | 0.8891009400000000 | 0.0649471900000000 | 1.0 |
| H6  | H | 0.0454267500000000 | 0.0811911600000000 | 0.0925946700000000 | 1.0 |
| H7  | H | 0.8904014100000000 | 0.0682432500000000 | 0.0952553000000000 | 1.0 |
| H8  | H | 0.2257192600000000 | 0.1111811900000000 | 0.0347917000000000 | 1.0 |
| H9  | H | 0.1492766900000000 | 0.8661874100000000 | 0.0502644100000000 | 1.0 |
| H10 | H | 0.2936996800000000 | 0.8944486500000000 | 0.0764777300000000 | 1.0 |
| H11 | H | 0.2687915600000000 | 0.9607001200000000 | 0.8677697100000000 | 1.0 |
| H12 | H | 0.3289637600000000 | 0.8908558700000000 | 0.8984281700000000 | 1.0 |
| H13 | H | 0.2614181600000000 | 0.0834600200000000 | 0.8748292400000000 | 1.0 |
| H14 | H | 0.4164467400000000 | 0.0705990500000000 | 0.8718983500000000 | 1.0 |
| H15 | H | 0.5811659300000000 | 0.1122705900000000 | 0.9332659600000000 | 1.0 |
| H16 | H | 0.6575322800000000 | 0.8677079900000000 | 0.9124559800000000 | 1.0 |
| H17 | H | 0.5130010600000000 | 0.8964957900000000 | 0.8870086500000000 | 1.0 |
| H18 | H | 0.5381000100000000 | 0.9582279000000000 | 0.0970282900000000 | 1.0 |
| H19 | H | 0.4777785100000000 | 0.8890810500000000 | 0.0649002300000000 | 1.0 |
| H20 | H | 0.5454572200000000 | 0.0811721800000000 | 0.0925855400000000 | 1.0 |
| H21 | H | 0.3904416000000000 | 0.0682226700000000 | 0.0952536900000000 | 1.0 |
| H22 | H | 0.7257250100000000 | 0.1111605000000000 | 0.0347924100000000 | 1.0 |
| H23 | H | 0.6492478400000000 | 0.8662081800000000 | 0.0502567600000000 | 1.0 |
| H24 | H | 0.7938207200000000 | 0.8943805600000000 | 0.0763309500000000 | 1.0 |
| H25 | H | 0.7690102700000000 | 0.9608075300000000 | 0.8676963800000000 | 1.0 |
| H26 | H | 0.8287605100000000 | 0.8908851100000000 | 0.8983695400000000 | 1.0 |
| H27 | H | 0.7614528600000000 | 0.0834958300000000 | 0.8748264900000000 | 1.0 |
| H28 | H | 0.9164881500000000 | 0.0706241200000000 | 0.8718998700000000 | 1.0 |

|     |   |                    |                    |                    |     |
|-----|---|--------------------|--------------------|--------------------|-----|
| C29 | C | 0.0910833800000000 | 0.0659291500000000 | 0.9623422300000000 | 1.0 |
| C30 | C | 0.9683693000000000 | 0.0497162900000000 | 0.0042948300000000 | 1.0 |
| C31 | C | 0.9684262200000000 | 0.9700935800000000 | 0.0034910800000000 | 1.0 |
| C32 | C | 0.0896525500000000 | 0.9509857900000000 | 0.9609780900000000 | 1.0 |
| C33 | C | 0.2157948600000000 | 0.0654842500000000 | 0.0047472000000000 | 1.0 |
| C34 | C | 0.3384985900000000 | 0.0501625200000000 | 0.9624499700000000 | 1.0 |
| C35 | C | 0.3384391500000000 | 0.9705441000000000 | 0.9615686400000000 | 1.0 |
| C36 | C | 0.2172339700000000 | 0.9505400000000000 | 0.0036923000000000 | 1.0 |
| C37 | C | 0.5910828000000000 | 0.0659415500000000 | 0.9623285900000000 | 1.0 |
| C38 | C | 0.4683789700000000 | 0.0497221800000000 | 0.0042856500000000 | 1.0 |
| C39 | C | 0.4684399600000000 | 0.9700997800000000 | 0.0034714900000000 | 1.0 |
| C40 | C | 0.5896404600000000 | 0.9510007100000000 | 0.9609248100000000 | 1.0 |
| C41 | C | 0.7157937800000000 | 0.0654726700000000 | 0.0047343400000000 | 1.0 |
| C42 | C | 0.8385093000000000 | 0.0501585900000000 | 0.9624432500000000 | 1.0 |
| C43 | C | 0.8384516600000000 | 0.9705397500000000 | 0.9615479800000000 | 1.0 |
| C44 | C | 0.7172213900000000 | 0.9505253100000000 | 0.0036378600000000 | 1.0 |
| N45 | N | 0.9625252100000000 | 0.0869270500000000 | 0.0660438300000000 | 1.0 |
| N46 | N | 0.9637339000000000 | 0.9394678000000000 | 0.0694570400000000 | 1.0 |
| N47 | N | 0.0738449800000000 | 0.8893681200000000 | 0.9265007700000000 | 1.0 |
| N48 | N | 0.3443160400000000 | 0.0886613900000000 | 0.9014945100000000 | 1.0 |
| N49 | N | 0.3430487300000000 | 0.9413172800000000 | 0.8949664900000000 | 1.0 |
| N50 | N | 0.2330137200000000 | 0.8882112600000000 | 0.0368802000000000 | 1.0 |
| N51 | N | 0.4625505100000000 | 0.0869228600000000 | 0.0660418600000000 | 1.0 |
| N52 | N | 0.4638003200000000 | 0.9394650000000000 | 0.0694328300000000 | 1.0 |
| N53 | N | 0.5738201400000000 | 0.8894009600000000 | 0.9264097800000000 | 1.0 |
| N54 | N | 0.8443480400000000 | 0.0886713100000000 | 0.9014980700000000 | 1.0 |
| N55 | N | 0.8431135700000000 | 0.9413278600000000 | 0.8949392900000000 | 1.0 |
| N56 | N | 0.7329876000000000 | 0.8881786300000000 | 0.0367870200000000 | 1.0 |
| O57 | O | 0.0995739600000000 | 0.0101687600000000 | 0.9161072500000000 | 1.0 |
| O58 | O | 0.2073095100000000 | 0.0087590600000000 | 0.0498004600000000 | 1.0 |
| O59 | O | 0.5995658200000000 | 0.0101936700000000 | 0.9160768300000000 | 1.0 |
| O60 | O | 0.7072971100000000 | 0.0087329900000000 | 0.0497678100000000 | 1.0 |

##### cif ends

furand\_NH2\_234\_syn\_alt Energy: -369.44109193

##### cif starts

data\_furand\_NH2\_234\_syn\_alt

\_publ\_section\_comment

;  
Andrew Reynoso, Bohan Xu, and Vincent H. Crespi  
;

\_cell\_length\_a 10.6466087513

\_cell\_length\_b 20.0

\_cell\_length\_c 20.0

\_cell\_angle\_alpha 90.0

\_cell\_angle\_beta 90.0

\_cell\_angle\_gamma 90.0

\_symmetry\_space\_group\_name\_H-M 'P 1'

\_symmetry\_Int\_Tables\_number 1

\_symmetry\_cell\_setting triclinic

| loop_                  |   |                    |                    |                    |     |
|------------------------|---|--------------------|--------------------|--------------------|-----|
| _atom_site_label       |   |                    |                    |                    |     |
| _atom_site_type_symbol |   |                    |                    |                    |     |
| _atom_site_fract_x     |   |                    |                    |                    |     |
| _atom_site_fract_y     |   |                    |                    |                    |     |
| _atom_site_fract_z     |   |                    |                    |                    |     |
| _atom_site_occupancy   |   |                    |                    |                    |     |
| H1                     | H | 0.0017523800000000 | 0.8819080800000000 | 0.0592911000000000 | 1.0 |
| H2                     | H | 0.0774625000000000 | 0.1076954800000000 | 0.1051904700000000 | 1.0 |
| H3                     | H | 0.9234226800000000 | 0.1078463600000000 | 0.1044053400000000 | 1.0 |
| H4                     | H | 0.2089287600000000 | 0.0548852400000000 | 0.9118988100000000 | 1.0 |
| H5                     | H | 0.1118743100000000 | 0.1112275600000000 | 0.9431746300000000 | 1.0 |
| H6                     | H | 0.1485233200000000 | 0.9494927500000000 | 0.8942826300000000 | 1.0 |
| H7                     | H | 0.0341807300000000 | 0.9004129800000000 | 0.9201998700000000 | 1.0 |
| H8                     | H | 0.2545821300000000 | 0.0884354900000000 | 0.0636970900000000 | 1.0 |
| H9                     | H | 0.1698896000000000 | 0.8620720300000000 | 0.1011804600000000 | 1.0 |
| H10                    | H | 0.3246706600000000 | 0.8587340300000000 | 0.0997736000000000 | 1.0 |
| H11                    | H | 0.3841962300000000 | 0.9383294200000000 | 0.8966688000000000 | 1.0 |
| H12                    | H | 0.2867082500000000 | 0.8854959700000000 | 0.9305757300000000 | 1.0 |
| H13                    | H | 0.3703423400000000 | 0.1024507500000000 | 0.9327145500000000 | 1.0 |
| H14                    | H | 0.4584460500000000 | 0.0415672800000000 | 0.9069652000000000 | 1.0 |
| H15                    | H | 0.5012590100000000 | 0.8849595100000000 | 0.0687864000000000 | 1.0 |
| H16                    | H | 0.4245020100000000 | 0.1145373900000000 | 0.0935467900000000 | 1.0 |
| H17                    | H | 0.5786677900000000 | 0.1147109800000000 | 0.0932696700000000 | 1.0 |
| H18                    | H | 0.7136204300000000 | 0.0490659100000000 | 0.9096120600000000 | 1.0 |
| H19                    | H | 0.6039224200000000 | 0.1019888200000000 | 0.9325584900000000 | 1.0 |
| H20                    | H | 0.6275504000000000 | 0.9421140300000000 | 0.8968509900000000 | 1.0 |
| H21                    | H | 0.5382510100000000 | 0.8850785200000000 | 0.9305881700000000 | 1.0 |
| H22                    | H | 0.7488985300000000 | 0.0890867100000000 | 0.0623028300000000 | 1.0 |
| H23                    | H | 0.6772338200000000 | 0.8599619600000000 | 0.1006321900000000 | 1.0 |
| H24                    | H | 0.8317428900000000 | 0.8638530700000000 | 0.1035512700000000 | 1.0 |
| H25                    | H | 0.8652200900000000 | 0.9527604500000000 | 0.8951611500000000 | 1.0 |
| H26                    | H | 0.7913522200000000 | 0.8885314200000000 | 0.9265584300000000 | 1.0 |
| H27                    | H | 0.8605393700000000 | 0.1082167600000000 | 0.9388549400000000 | 1.0 |
| H28                    | H | 0.9644173900000000 | 0.0540120800000000 | 0.9126579600000000 | 1.0 |
| C29                    | C | 0.0016884900000000 | 0.9318896800000000 | 0.0365918000000000 | 1.0 |
| C30                    | C | 0.1258860800000000 | 0.9473428000000000 | 0.9958783200000000 | 1.0 |
| C31                    | C | 0.1263950000000000 | 0.0268890200000000 | 0.9988258400000000 | 1.0 |
| C32                    | C | 0.0014852200000000 | 0.0399523500000000 | 0.0418040200000000 | 1.0 |
| C33                    | C | 0.2522555700000000 | 0.0392163400000000 | 0.0390193100000000 | 1.0 |
| C34                    | C | 0.3756813700000000 | 0.0236340000000000 | 0.9963067800000000 | 1.0 |
| C35                    | C | 0.3762201700000000 | 0.9440839100000000 | 0.9988468600000000 | 1.0 |
| C36                    | C | 0.2506034300000000 | 0.9308897900000000 | 0.0403984700000000 | 1.0 |
| C37                    | C | 0.5016765200000000 | 0.9325630200000000 | 0.0413745900000000 | 1.0 |
| C38                    | C | 0.6260136000000000 | 0.9443020600000000 | 0.9986906300000000 | 1.0 |
| C39                    | C | 0.6265139000000000 | 0.0239266200000000 | 0.9961573300000000 | 1.0 |
| C40                    | C | 0.5015120100000000 | 0.0405147800000000 | 0.0375193200000000 | 1.0 |
| C41                    | C | 0.7507180200000000 | 0.0395267300000000 | 0.0383045800000000 | 1.0 |
| C42                    | C | 0.8761592300000000 | 0.0262793400000000 | 0.9980854000000000 | 1.0 |
| C43                    | C | 0.8760810000000000 | 0.9469451800000000 | 0.9965195000000000 | 1.0 |
| C44                    | C | 0.7525968200000000 | 0.9311717600000000 | 0.0407194000000000 | 1.0 |
| N45                    | N | 0.1253761900000000 | 0.9156031500000000 | 0.9305250700000000 | 1.0 |
| N46                    | N | 0.1221161600000000 | 0.0610656500000000 | 0.9343439200000000 | 1.0 |
| N47                    | N | 0.0009558800000000 | 0.1029895100000000 | 0.0748007200000000 | 1.0 |
| N48                    | N | 0.3721560000000000 | 0.0513378300000000 | 0.9287406800000000 | 1.0 |

|     |   |                    |                    |                    |     |
|-----|---|--------------------|--------------------|--------------------|-----|
| N49 | N | 0.3747044200000000 | 0.9064557200000000 | 0.9363842500000000 | 1.0 |
| N50 | N | 0.2468793100000000 | 0.8674477700000000 | 0.0714213800000000 | 1.0 |
| N51 | N | 0.6243591800000000 | 0.9083293600000000 | 0.9353435900000000 | 1.0 |
| N52 | N | 0.6233482000000000 | 0.0519642500000000 | 0.9288468900000000 | 1.0 |
| N53 | N | 0.5014283500000000 | 0.1064812700000000 | 0.0642614300000000 | 1.0 |
| N54 | N | 0.8743492000000000 | 0.0579472200000000 | 0.9323778200000000 | 1.0 |
| N55 | N | 0.8732132000000000 | 0.9159054100000000 | 0.9305479800000000 | 1.0 |
| N56 | N | 0.7558719200000000 | 0.8682201100000000 | 0.0727944100000000 | 1.0 |
| O57 | O | 0.0016453700000000 | 0.9828212800000000 | 0.0866529700000000 | 1.0 |
| O58 | O | 0.2517630600000000 | 0.9871600400000000 | 0.0872439000000000 | 1.0 |
| O59 | O | 0.5017783300000000 | 0.9875021700000000 | 0.0869561700000000 | 1.0 |
| O60 | O | 0.7514855100000000 | 0.9880508600000000 | 0.0870530400000000 | 1.0 |

##### cif ends

furand\_NH2\_234\_syn\_alt\_forbid Energy: -367.37243928

##### cif starts

data\_furand\_NH2\_234\_syn\_alt\_forbid

\_publ\_section\_comment

;  
Andrew Reynoso, Bohan Xu, and Vincent H. Crespi  
;

\_cell\_length\_a 9.8434620892

\_cell\_length\_b 20.0

\_cell\_length\_c 20.0

\_cell\_angle\_alpha 90.0

\_cell\_angle\_beta 90.0

\_cell\_angle\_gamma 90.0

\_symmetry\_space\_group\_name\_H-M 'P 1'

\_symmetry\_Int\_Tables\_number 1

\_symmetry\_cell\_setting triclinic

loop\_

\_atom\_site\_label

\_atom\_site\_type\_symbol

\_atom\_site\_fract\_x

\_atom\_site\_fract\_y

\_atom\_site\_fract\_z

\_atom\_site\_occupancy

|     |   |                    |                    |                    |     |
|-----|---|--------------------|--------------------|--------------------|-----|
| H1  | H | 0.8735451000000000 | 0.1031912100000000 | 0.0332334200000000 | 1.0 |
| H2  | H | 0.1794319700000000 | 0.8880467600000000 | 0.0364922700000000 | 1.0 |
| H3  | H | 0.3735501000000000 | 0.1031942900000000 | 0.0332262300000000 | 1.0 |
| H4  | H | 0.6794362000000000 | 0.8880409000000000 | 0.0364893000000000 | 1.0 |
| H5  | H | 0.9059096900000000 | 0.0102587800000000 | 0.8590122600000000 | 1.0 |
| H6  | H | 0.0576964200000000 | 0.0973457800000000 | 0.8902556800000000 | 1.0 |
| H7  | H | 0.4058732900000000 | 0.0102367800000000 | 0.8590181100000000 | 1.0 |
| H8  | H | 0.5576852900000000 | 0.0973264200000000 | 0.8902463900000000 | 1.0 |
| H9  | H | 0.0744458300000000 | 0.9133071300000000 | 0.8761865000000000 | 1.0 |
| H10 | H | 0.5744325300000000 | 0.9132790300000000 | 0.8761992600000000 | 1.0 |
| H11 | H | 0.9117663900000000 | 0.8542961000000000 | 0.9445066700000000 | 1.0 |
| H12 | H | 0.4117271300000000 | 0.8542851200000000 | 0.9445484700000000 | 1.0 |
| H13 | H | 0.3409707000000000 | 0.8819177100000000 | 0.1148205000000000 | 1.0 |

|     |   |                    |                    |                    |     |
|-----|---|--------------------|--------------------|--------------------|-----|
| H14 | H | 0.8409835100000000 | 0.8818982200000000 | 0.1147985700000000 | 1.0 |
| H15 | H | 0.0020654900000000 | 0.8978385400000000 | 0.0998985500000000 | 1.0 |
| H16 | H | 0.5020560600000000 | 0.8978476300000000 | 0.0999169800000000 | 1.0 |
| H17 | H | 0.1592965100000000 | 0.1332623700000000 | 0.9468370600000000 | 1.0 |
| H18 | H | 0.6592766200000000 | 0.1332540900000000 | 0.9468248800000000 | 1.0 |
| H19 | H | 0.7983612400000000 | 0.0676228900000000 | 0.8912544100000000 | 1.0 |
| H20 | H | 0.2983642800000000 | 0.0676212800000000 | 0.8912561600000000 | 1.0 |
| H21 | H | 0.1640691800000000 | 0.9832980000000000 | 0.8625114100000000 | 1.0 |
| H22 | H | 0.6640109600000000 | 0.9832796200000000 | 0.8625034500000000 | 1.0 |
| H23 | H | 0.8148217000000000 | 0.9094142200000000 | 0.9033047800000000 | 1.0 |
| H24 | H | 0.3148192200000000 | 0.9094000300000000 | 0.9033190800000000 | 1.0 |
| H25 | H | 0.0512210200000000 | 0.0959764200000000 | 0.0974828600000000 | 1.0 |
| H26 | H | 0.2125615400000000 | 0.1102175700000000 | 0.1131699700000000 | 1.0 |
| H27 | H | 0.5512136900000000 | 0.0959653700000000 | 0.0974788400000000 | 1.0 |
| H28 | H | 0.7125519200000000 | 0.1102162900000000 | 0.1131639300000000 | 1.0 |
| C29 | C | 0.8433257900000000 | 0.0517197800000000 | 0.0206674300000000 | 1.0 |
| C30 | C | 0.9307733700000000 | 0.0267737000000000 | 0.9588059100000000 | 1.0 |
| C31 | C | 0.9558240400000000 | 0.9497271100000000 | 0.9694638900000000 | 1.0 |
| C32 | C | 0.8752969500000000 | 0.9425746600000000 | 0.0354535600000000 | 1.0 |
| C33 | C | 0.1776106300000000 | 0.0485760100000000 | 0.0347233600000000 | 1.0 |
| C34 | C | 0.0952194000000000 | 0.0400481700000000 | 0.9697635000000000 | 1.0 |
| C35 | C | 0.1200435200000000 | 0.9627472500000000 | 0.9599576300000000 | 1.0 |
| C36 | C | 0.2093992600000000 | 0.9390746400000000 | 0.0221699700000000 | 1.0 |
| C37 | C | 0.3433256900000000 | 0.0517219600000000 | 0.0206669500000000 | 1.0 |
| C38 | C | 0.4307673700000000 | 0.0267655400000000 | 0.9588072700000000 | 1.0 |
| C39 | C | 0.4558183400000000 | 0.9497195300000000 | 0.9694745700000000 | 1.0 |
| C40 | C | 0.3752945800000000 | 0.9425788700000000 | 0.0354655100000000 | 1.0 |
| C41 | C | 0.6776089100000000 | 0.0485707700000000 | 0.0347194000000000 | 1.0 |
| C42 | C | 0.5952148300000000 | 0.0400395900000000 | 0.9697600700000000 | 1.0 |
| C43 | C | 0.6200350000000000 | 0.9627386300000000 | 0.9599580900000000 | 1.0 |
| C44 | C | 0.7094000600000000 | 0.9390688100000000 | 0.0221652200000000 | 1.0 |
| N45 | N | 0.8970098800000000 | 0.0486916900000000 | 0.8922789300000000 | 1.0 |
| N46 | N | 0.9128630400000000 | 0.8998484100000000 | 0.9211625800000000 | 1.0 |
| N47 | N | 0.9110441500000000 | 0.8876775400000000 | 0.0775372900000000 | 1.0 |
| N48 | N | 0.1432605200000000 | 0.1046965500000000 | 0.0755176400000000 | 1.0 |
| N49 | N | 0.1402929000000000 | 0.0896292100000000 | 0.9217327900000000 | 1.0 |
| N50 | N | 0.1554131500000000 | 0.9423720100000000 | 0.8927621800000000 | 1.0 |
| N51 | N | 0.3970013800000000 | 0.0486760600000000 | 0.8922785700000000 | 1.0 |
| N52 | N | 0.4128503500000000 | 0.8998285700000000 | 0.9211871000000000 | 1.0 |
| N53 | N | 0.4110320600000000 | 0.8876868600000000 | 0.0775577600000000 | 1.0 |
| N54 | N | 0.6432501400000000 | 0.1046907600000000 | 0.0755126200000000 | 1.0 |
| N55 | N | 0.6402822500000000 | 0.0896173700000000 | 0.9217252200000000 | 1.0 |
| N56 | N | 0.6553899000000000 | 0.9423578000000000 | 0.8927624500000000 | 1.0 |
| O57 | O | 0.8938873300000000 | 0.0067376200000000 | 0.0698559600000000 | 1.0 |
| O58 | O | 0.1593127500000000 | 0.9855119300000000 | 0.0703540800000000 | 1.0 |
| O59 | O | 0.3938876500000000 | 0.0067452800000000 | 0.0698604300000000 | 1.0 |
| O60 | O | 0.6593163900000000 | 0.9855060600000000 | 0.0703505100000000 | 1.0 |

##### cif ends

  furan\_NH2\_234\_syn\_dir  Energy: -368.82055943

##### cif starts

data\_furan\_NH2\_234\_syn\_dir

\_publ\_section\_comment

;  
Andrew Reynoso, Bohan Xu, and Vincent H. Crespi  
;

\_cell\_length\_a 10.7426035291  
\_cell\_length\_b 20.0  
\_cell\_length\_c 20.0  
\_cell\_angle\_alpha 90.0  
\_cell\_angle\_beta 90.0  
\_cell\_angle\_gamma 90.0

\_symmetry\_space\_group\_name\_H-M 'P 1'  
\_symmetry\_Int\_Tables\_number 1  
\_symmetry\_cell\_setting triclinic

loop\_  
\_atom\_site\_label  
\_atom\_site\_type\_symbol  
\_atom\_site\_fract\_x  
\_atom\_site\_fract\_y  
\_atom\_site\_fract\_z  
\_atom\_site\_occupancy

|     |   |                    |                    |                    |     |
|-----|---|--------------------|--------------------|--------------------|-----|
| H1  | H | 0.9650719500000000 | 0.1161600900000000 | 0.0712360600000000 | 1.0 |
| H2  | H | 0.8744308400000000 | 0.8754879200000000 | 0.0635431600000000 | 1.0 |
| H3  | H | 0.9815938300000000 | 0.9003252000000000 | 0.1175122400000000 | 1.0 |
| H4  | H | 0.0055601700000000 | 0.9584896400000000 | 0.9079348800000000 | 1.0 |
| H5  | H | 0.1045258200000000 | 0.9007381500000000 | 0.9311480600000000 | 1.0 |
| H6  | H | 0.0019801200000000 | 0.1148476000000000 | 0.9298683700000000 | 1.0 |
| H7  | H | 0.1033533100000000 | 0.0616190600000000 | 0.8982470400000000 | 1.0 |
| H8  | H | 0.2150507900000000 | 0.1161610400000000 | 0.0712198700000000 | 1.0 |
| H9  | H | 0.1246771000000000 | 0.8753343400000000 | 0.0633128200000000 | 1.0 |
| H10 | H | 0.2308409500000000 | 0.9004745800000000 | 0.1176768100000000 | 1.0 |
| H11 | H | 0.2554878000000000 | 0.9583738000000000 | 0.9079678900000000 | 1.0 |
| H12 | H | 0.3548508600000000 | 0.9007671100000000 | 0.9311154300000000 | 1.0 |
| H13 | H | 0.2520131600000000 | 0.1148729400000000 | 0.9298719600000000 | 1.0 |
| H14 | H | 0.3532956500000000 | 0.0615960700000000 | 0.8982503500000000 | 1.0 |
| H15 | H | 0.4649958700000000 | 0.1161505900000000 | 0.0712613100000000 | 1.0 |
| H16 | H | 0.3744345100000000 | 0.8754857000000000 | 0.0635217500000000 | 1.0 |
| H17 | H | 0.4816597600000000 | 0.9002911000000000 | 0.1174673200000000 | 1.0 |
| H18 | H | 0.5055560900000000 | 0.9585771000000000 | 0.9079061700000000 | 1.0 |
| H19 | H | 0.6045473900000000 | 0.9008247000000000 | 0.9310639400000000 | 1.0 |
| H20 | H | 0.5019518800000000 | 0.1148978400000000 | 0.9299206400000000 | 1.0 |
| H21 | H | 0.6034518300000000 | 0.0617541400000000 | 0.8982833100000000 | 1.0 |
| H22 | H | 0.7150747100000000 | 0.1161485700000000 | 0.0712775000000000 | 1.0 |
| H23 | H | 0.6246801000000000 | 0.8753189700000000 | 0.0632342700000000 | 1.0 |
| H24 | H | 0.7307634600000000 | 0.9004556200000000 | 0.1176394200000000 | 1.0 |
| H25 | H | 0.7555183700000000 | 0.9584579500000000 | 0.9079467000000000 | 1.0 |
| H26 | H | 0.8547368100000000 | 0.9007883300000000 | 0.9311014800000000 | 1.0 |
| H27 | H | 0.7520453300000000 | 0.1149739100000000 | 0.9299460500000000 | 1.0 |
| H28 | H | 0.8531634400000000 | 0.0616473000000000 | 0.8982568100000000 | 1.0 |
| C29 | C | 0.9652264800000000 | 0.0693988900000000 | 0.0424616900000000 | 1.0 |
| C30 | C | 0.0900556900000000 | 0.0577828200000000 | 0.9999674000000000 | 1.0 |
| C31 | C | 0.0901219600000000 | 0.9783598100000000 | 0.9963689700000000 | 1.0 |
| C32 | C | 0.9639339400000000 | 0.9612834400000000 | 0.0378822100000000 | 1.0 |
| C33 | C | 0.2152223700000000 | 0.0693994000000000 | 0.0424476900000000 | 1.0 |

|     |   |                    |                    |                    |     |
|-----|---|--------------------|--------------------|--------------------|-----|
| C34 | C | 0.3400483200000000 | 0.0577827000000000 | 0.9999677900000000 | 1.0 |
| C35 | C | 0.3401304600000000 | 0.9783550100000000 | 0.9963598600000000 | 1.0 |
| C36 | C | 0.2139329400000000 | 0.9612917800000000 | 0.0378911500000000 | 1.0 |
| C37 | C | 0.4652051300000000 | 0.0693973200000000 | 0.0424737900000000 | 1.0 |
| C38 | C | 0.5900556100000000 | 0.0578147700000000 | 0.9999970300000000 | 1.0 |
| C39 | C | 0.5901228900000000 | 0.9783907700000000 | 0.9963524700000000 | 1.0 |
| C40 | C | 0.4639362400000000 | 0.9612819700000000 | 0.0378651900000000 | 1.0 |
| C41 | C | 0.7152280700000000 | 0.0694011800000000 | 0.0424821000000000 | 1.0 |
| C42 | C | 0.8400511700000000 | 0.0577961100000000 | 0.9999839900000000 | 1.0 |
| C43 | C | 0.8401309900000000 | 0.9783691400000000 | 0.9963603400000000 | 1.0 |
| C44 | C | 0.7139297700000000 | 0.9612968600000000 | 0.0378717100000000 | 1.0 |
| N45 | N | 0.0892458400000000 | 0.0944004400000000 | 0.9368868100000000 | 1.0 |
| N46 | N | 0.0930780500000000 | 0.9514988100000000 | 0.9284961000000000 | 1.0 |
| N47 | N | 0.9626864400000000 | 0.8954546300000000 | 0.0676579500000000 | 1.0 |
| N48 | N | 0.3392515100000000 | 0.0943931200000000 | 0.9368849600000000 | 1.0 |
| N49 | N | 0.3430775900000000 | 0.9515056100000000 | 0.9284849100000000 | 1.0 |
| N50 | N | 0.2127163900000000 | 0.8954817800000000 | 0.0677496700000000 | 1.0 |
| N51 | N | 0.5892488400000000 | 0.0944907400000000 | 0.9369504800000000 | 1.0 |
| N52 | N | 0.5930819000000000 | 0.9515864800000000 | 0.9284570400000000 | 1.0 |
| N53 | N | 0.4627019900000000 | 0.8954424600000000 | 0.0676164300000000 | 1.0 |
| N54 | N | 0.8392418200000000 | 0.0944314900000000 | 0.9369139400000000 | 1.0 |
| N55 | N | 0.8430814300000000 | 0.9515354600000000 | 0.9284783200000000 | 1.0 |
| N56 | N | 0.7127075800000000 | 0.8954733800000000 | 0.0677037600000000 | 1.0 |
| O57 | O | 0.9641011500000000 | 0.0135189400000000 | 0.0871852400000000 | 1.0 |
| O58 | O | 0.2141132800000000 | 0.0135224300000000 | 0.0871788500000000 | 1.0 |
| O59 | O | 0.4640867500000000 | 0.0135052000000000 | 0.0871824400000000 | 1.0 |
| O60 | O | 0.7141125400000000 | 0.0135026900000000 | 0.0871851100000000 | 1.0 |

##### cif ends

furand\_NH2\_234\_syn\_dir\_forbid Energy: -366.62391285

##### cif starts

data\_furand\_NH2\_234\_syn\_dir\_forbid

\_publ\_section\_comment

;  
Andrew Reynoso, Bohan Xu, and Vincent H. Crespi  
;

\_cell\_length\_a 9.9303281537

\_cell\_length\_b 20.0

\_cell\_length\_c 20.0

\_cell\_angle\_alpha 90.0

\_cell\_angle\_beta 90.0

\_cell\_angle\_gamma 90.0

\_symmetry\_space\_group\_name\_H-M 'P 1'

\_symmetry\_Int\_Tables\_number 1

\_symmetry\_cell\_setting triclinic

loop\_

\_atom\_site\_label

\_atom\_site\_type\_symbol

\_atom\_site\_fract\_x

\_atom\_site\_fract\_y



|     |   | _atom_site_fract_z |                      |                    |     |  |
|-----|---|--------------------|----------------------|--------------------|-----|--|
|     |   |                    | _atom_site_occupancy |                    |     |  |
| H1  | H | 0.8719477400000000 | 0.1068501500000000   | 0.0269038000000000 | 1.0 |  |
| H2  | H | 0.1493687200000000 | 0.0913525000000000   | 0.0615472900000000 | 1.0 |  |
| H3  | H | 0.3719422900000000 | 0.1069270800000000   | 0.0268134500000000 | 1.0 |  |
| H4  | H | 0.6493525100000000 | 0.0912657100000000   | 0.0616244000000000 | 1.0 |  |
| H5  | H | 0.9089544100000000 | 0.0075750000000000   | 0.8554610000000000 | 1.0 |  |
| H6  | H | 0.0563423000000000 | 0.0950538500000000   | 0.8825532900000000 | 1.0 |  |
| H7  | H | 0.4091965200000000 | 0.0076634500000000   | 0.8554083100000000 | 1.0 |  |
| H8  | H | 0.5564260900000000 | 0.0951816200000000   | 0.8826257000000000 | 1.0 |  |
| H9  | H | 0.0707030400000000 | 0.9122123000000000   | 0.8746042900000000 | 1.0 |  |
| H10 | H | 0.5706343600000000 | 0.9122223800000000   | 0.8745847500000000 | 1.0 |  |
| H11 | H | 0.9169484300000000 | 0.8546528600000000   | 0.9441687800000000 | 1.0 |  |
| H12 | H | 0.4169325100000000 | 0.8546737300000000   | 0.9442517600000000 | 1.0 |  |
| H13 | H | 0.0698736300000000 | 0.8708681100000000   | 0.0560764400000000 | 1.0 |  |
| H14 | H | 0.5698435100000000 | 0.8708155200000000   | 0.0559835500000000 | 1.0 |  |
| H15 | H | 0.9484923200000000 | 0.9216561000000000   | 0.1261723800000000 | 1.0 |  |
| H16 | H | 0.4490794300000000 | 0.9218041800000000   | 0.1260977200000000 | 1.0 |  |
| H17 | H | 0.1635322900000000 | 0.1328166300000000   | 0.9347859300000000 | 1.0 |  |
| H18 | H | 0.6635979400000000 | 0.1328673000000000   | 0.9349254900000000 | 1.0 |  |
| H19 | H | 0.7984420000000000 | 0.0643645300000000   | 0.8849482400000000 | 1.0 |  |
| H20 | H | 0.2984812700000000 | 0.0643493000000000   | 0.8848939100000000 | 1.0 |  |
| H21 | H | 0.1681470400000000 | 0.9789916600000000   | 0.8593623100000000 | 1.0 |  |
| H22 | H | 0.6680488200000000 | 0.9790103100000000   | 0.8593043800000000 | 1.0 |  |
| H23 | H | 0.8126202100000000 | 0.9080002700000000   | 0.9049573700000000 | 1.0 |  |
| H24 | H | 0.3126061400000000 | 0.9079866700000000   | 0.9049910400000000 | 1.0 |  |
| H25 | H | 0.1878545200000000 | 0.8406371200000000   | 0.0035935500000000 | 1.0 |  |
| H26 | H | 0.6874821700000000 | 0.8406533500000000   | 0.0032845000000000 | 1.0 |  |
| H27 | H | 0.8242960100000000 | 0.8720746600000000   | 0.0959143800000000 | 1.0 |  |
| H28 | H | 0.3244265800000000 | 0.8723040500000000   | 0.0961509400000000 | 1.0 |  |
| C29 | C | 0.8422033500000000 | 0.0550969500000000   | 0.0153662000000000 | 1.0 |  |
| C30 | C | 0.9309947200000000 | 0.0278802200000000   | 0.9548234000000000 | 1.0 |  |
| C31 | C | 0.9556235600000000 | 0.9513777900000000   | 0.9685907100000000 | 1.0 |  |
| C32 | C | 0.8769144600000000 | 0.9476722100000000   | 0.0359528400000000 | 1.0 |  |
| C33 | C | 0.1774108200000000 | 0.0495854900000000   | 0.0286624500000000 | 1.0 |  |
| C34 | C | 0.0950948300000000 | 0.0409544800000000   | 0.9642494100000000 | 1.0 |  |
| C35 | C | 0.1183112200000000 | 0.9634213800000000   | 0.9571619800000000 | 1.0 |  |
| C36 | C | 0.2061578000000000 | 0.9398660000000000   | 0.0204245800000000 | 1.0 |  |
| C37 | C | 0.3422140500000000 | 0.0551616000000000   | 0.0153159700000000 | 1.0 |  |
| C38 | C | 0.4310148800000000 | 0.0279155700000000   | 0.9547971800000000 | 1.0 |  |
| C39 | C | 0.4556239800000000 | 0.9514146400000000   | 0.9685811800000000 | 1.0 |  |
| C40 | C | 0.3769698700000000 | 0.9477457000000000   | 0.0359664600000000 | 1.0 |  |
| C41 | C | 0.6773896000000000 | 0.0495285000000000   | 0.0287003900000000 | 1.0 |  |
| C42 | C | 0.5951041500000000 | 0.0409731700000000   | 0.9642627600000000 | 1.0 |  |
| C43 | C | 0.6183011900000000 | 0.9634440800000000   | 0.9571210000000000 | 1.0 |  |
| C44 | C | 0.7061139000000000 | 0.9398217100000000   | 0.0203530900000000 | 1.0 |  |
| N45 | N | 0.8970717300000000 | 0.0470180100000000   | 0.8873376700000000 | 1.0 |  |
| N46 | N | 0.9111873800000000 | 0.9004715100000000   | 0.9216454400000000 | 1.0 |  |
| N47 | N | 0.9114487600000000 | 0.8981175900000000   | 0.0847761100000000 | 1.0 |  |
| N48 | N | 0.1394767300000000 | 0.0879570700000000   | 0.9134262600000000 | 1.0 |  |
| N49 | N | 0.1531352700000000 | 0.9396252400000000   | 0.8910592000000000 | 1.0 |  |
| N50 | N | 0.1709403000000000 | 0.8732274900000000   | 0.0419857900000000 | 1.0 |  |
| N51 | N | 0.3971601300000000 | 0.0470760700000000   | 0.8873084400000000 | 1.0 |  |
| N52 | N | 0.4111796800000000 | 0.9004701800000000   | 0.9216821800000000 | 1.0 |  |
| N53 | N | 0.4116011600000000 | 0.8982352200000000   | 0.0848151300000000 | 1.0 |  |

|     |   |                    |                    |                    |     |
|-----|---|--------------------|--------------------|--------------------|-----|
| N54 | N | 0.6395275300000000 | 0.0880386200000000 | 0.9135059600000000 | 1.0 |
| N55 | N | 0.6530753900000000 | 0.9396494300000000 | 0.8910114500000000 | 1.0 |
| N56 | N | 0.6708587800000000 | 0.8731422000000000 | 0.0417955000000000 | 1.0 |
| O57 | O | 0.8919149600000000 | 0.0123844400000000 | 0.0663464000000000 | 1.0 |
| O58 | O | 0.1580566000000000 | 0.9892660900000000 | 0.0664613600000000 | 1.0 |
| O59 | O | 0.3919579600000000 | 0.0124853700000000 | 0.0663170900000000 | 1.0 |
| O60 | O | 0.6579989700000000 | 0.9891730500000000 | 0.0664411300000000 | 1.0 |

##### cif ends

furam\_NH2\_23\_anti\_alt Energy: -323.05894175

##### cif starts

data\_furam\_NH2\_23\_anti\_alt

\_publ\_section\_comment

;  
Andrew Reynoso, Bohan Xu, and Vincent H. Crespi  
;

\_cell\_length\_a 9.411732042

\_cell\_length\_b 20.0

\_cell\_length\_c 20.0

\_cell\_angle\_alpha 90.0

\_cell\_angle\_beta 90.0

\_cell\_angle\_gamma 90.0

\_symmetry\_space\_group\_name\_H-M 'P 1'

\_symmetry\_Int\_Tables\_number 1

\_symmetry\_cell\_setting triclinic

loop\_

\_atom\_site\_label

\_atom\_site\_type\_symbol

\_atom\_site\_fract\_x

\_atom\_site\_fract\_y

\_atom\_site\_fract\_z

\_atom\_site\_occupancy

|     |   |                    |                    |                    |     |
|-----|---|--------------------|--------------------|--------------------|-----|
| H1  | H | 0.3638403500000000 | 0.8838772800000000 | 0.9378991200000000 | 1.0 |
| H2  | H | 0.3535894500000000 | 0.9275919800000000 | 0.0685122300000000 | 1.0 |
| H3  | H | 0.4369778200000000 | 0.0347534700000000 | 0.1046628000000000 | 1.0 |
| H4  | H | 0.2764577600000000 | 0.0625842400000000 | 0.1185965900000000 | 1.0 |
| H5  | H | 0.2682402100000000 | 0.1229256700000000 | 0.9326793200000000 | 1.0 |
| H6  | H | 0.4156788900000000 | 0.1138641200000000 | 0.8865791300000000 | 1.0 |
| H7  | H | 0.6122886800000000 | 0.0878011700000000 | 0.0474625800000000 | 1.0 |
| H8  | H | 0.6028300600000000 | 0.0438403000000000 | 0.9155009900000000 | 1.0 |
| H9  | H | 0.6901839200000000 | 0.9339196200000000 | 0.8819183800000000 | 1.0 |
| H10 | H | 0.5277636400000000 | 0.9092941400000000 | 0.8663047800000000 | 1.0 |
| H11 | H | 0.1871371800000000 | 0.8478540800000000 | 0.0830310100000000 | 1.0 |
| H12 | H | 0.0861832900000000 | 0.8328403400000000 | 0.0168070000000000 | 1.0 |
| H13 | H | 0.8638376400000000 | 0.8838781100000000 | 0.9378992800000000 | 1.0 |
| H14 | H | 0.8535934400000000 | 0.9275966000000000 | 0.0685117500000000 | 1.0 |
| H15 | H | 0.9369751900000000 | 0.0347565300000000 | 0.1046621600000000 | 1.0 |
| H16 | H | 0.7764597000000000 | 0.0625951700000000 | 0.1185914700000000 | 1.0 |
| H17 | H | 0.7682469100000000 | 0.1229257700000000 | 0.9326693300000000 | 1.0 |
| H18 | H | 0.9156931900000000 | 0.1138627800000000 | 0.8865748700000000 | 1.0 |

|     |   |                    |                    |                    |     |
|-----|---|--------------------|--------------------|--------------------|-----|
| H19 | H | 0.1122875600000000 | 0.0877974200000000 | 0.0474657200000000 | 1.0 |
| H20 | H | 0.1028373200000000 | 0.0438405400000000 | 0.9155022400000000 | 1.0 |
| H21 | H | 0.1901842500000000 | 0.9339193500000000 | 0.8819170200000000 | 1.0 |
| H22 | H | 0.0277620700000000 | 0.9092980100000000 | 0.8663017100000000 | 1.0 |
| H23 | H | 0.5861961300000000 | 0.8328411100000000 | 0.0168153900000000 | 1.0 |
| H24 | H | 0.6871383800000000 | 0.8478631800000000 | 0.0830415500000000 | 1.0 |
| C25 | C | 0.3050750900000000 | 0.9485519600000000 | 0.0232151800000000 | 1.0 |
| C26 | C | 0.3047031500000000 | 0.0271142800000000 | 0.0241817000000000 | 1.0 |
| C27 | C | 0.3933145700000000 | 0.0429239900000000 | 0.9593010000000000 | 1.0 |
| C28 | C | 0.3895818300000000 | 0.9323671600000000 | 0.9605006600000000 | 1.0 |
| C29 | C | 0.6397344100000000 | 0.0397579100000000 | 0.0244566000000000 | 1.0 |
| C30 | C | 0.5550710700000000 | 0.0237264700000000 | 0.9614107800000000 | 1.0 |
| C31 | C | 0.5542431600000000 | 0.9451976900000000 | 0.9607453100000000 | 1.0 |
| C32 | C | 0.6424891100000000 | 0.9298058500000000 | 0.0255297900000000 | 1.0 |
| C33 | C | 0.8895812400000000 | 0.9323681600000000 | 0.9604998600000000 | 1.0 |
| C34 | C | 0.8050762600000000 | 0.9485550300000000 | 0.0232147100000000 | 1.0 |
| C35 | C | 0.8047045200000000 | 0.0271173900000000 | 0.0241790600000000 | 1.0 |
| C36 | C | 0.8933168500000000 | 0.0429248000000000 | 0.9592983700000000 | 1.0 |
| C37 | C | 0.1397328600000000 | 0.0397549900000000 | 0.0244583200000000 | 1.0 |
| C38 | C | 0.0550731800000000 | 0.0237261300000000 | 0.9614106300000000 | 1.0 |
| C39 | C | 0.0542430000000000 | 0.9451976200000000 | 0.9607434900000000 | 1.0 |
| C40 | C | 0.1424878100000000 | 0.9298027800000000 | 0.0255273900000000 | 1.0 |
| N41 | N | 0.3560250300000000 | 0.0616527400000000 | 0.0839439400000000 | 1.0 |
| N42 | N | 0.3709487000000000 | 0.1071947300000000 | 0.9324260300000000 | 1.0 |
| N43 | N | 0.6055190000000000 | 0.9090118400000000 | 0.9018989100000000 | 1.0 |
| N44 | N | 0.6076851700000000 | 0.8664322900000000 | 0.0538161900000000 | 1.0 |
| N45 | N | 0.8560286200000000 | 0.0616573800000000 | 0.0839400000000000 | 1.0 |
| N46 | N | 0.8709557300000000 | 0.1071950700000000 | 0.9324208300000000 | 1.0 |
| N47 | N | 0.1055165400000000 | 0.9090125900000000 | 0.9018962400000000 | 1.0 |
| N48 | N | 0.1076821300000000 | 0.8664278600000000 | 0.0538098000000000 | 1.0 |
| O49 | O | 0.8461209200000000 | 0.9860581300000000 | 0.9153728200000000 | 1.0 |
| O50 | O | 0.5960646500000000 | 0.9854542700000000 | 0.0688717300000000 | 1.0 |
| O51 | O | 0.3461190800000000 | 0.9860575800000000 | 0.9153748000000000 | 1.0 |
| O52 | O | 0.0960613000000000 | 0.9854503200000000 | 0.0688714500000000 | 1.0 |

##### cif ends

furand\_NH2\_23\_anti\_alt\_forbid Energy: -322.97169644

##### cif starts

data\_furand\_NH2\_23\_anti\_alt\_forbid

\_publ\_section\_comment

;  
Andrew Reynoso, Bohan Xu, and Vincent H. Crespi  
;

\_cell\_length\_a 10.2488704913

\_cell\_length\_b 20.0

\_cell\_length\_c 20.0

\_cell\_angle\_alpha 90.0

\_cell\_angle\_beta 90.0

\_cell\_angle\_gamma 90.0

\_symmetry\_space\_group\_name\_H-M 'P 1'

\_symmetry\_Int\_Tables\_number 1

\_symmetry\_cell\_setting triclinic

loop\_

\_atom\_site\_label

\_atom\_site\_type\_symbol

\_atom\_site\_fract\_x

\_atom\_site\_fract\_y

\_atom\_site\_fract\_z

\_atom\_site\_occupancy

|     |   |                    |                    |                    |     |
|-----|---|--------------------|--------------------|--------------------|-----|
| H1  | H | 0.9498423700000000 | 0.9335874300000000 | 0.0535737000000000 | 1.0 |
| H2  | H | 0.0606069700000000 | 0.8968040600000000 | 0.9307735000000000 | 1.0 |
| H3  | H | 0.3201647100000000 | 0.0594571700000000 | 0.9153066900000000 | 1.0 |
| H4  | H | 0.2081057900000000 | 0.0968081100000000 | 0.0381897600000000 | 1.0 |
| H5  | H | 0.4499953100000000 | 0.9334700800000000 | 0.0535664000000000 | 1.0 |
| H6  | H | 0.5605992500000000 | 0.8968809200000000 | 0.9306710500000000 | 1.0 |
| H7  | H | 0.8199538000000000 | 0.0595503200000000 | 0.9153180100000000 | 1.0 |
| H8  | H | 0.7081006100000000 | 0.0967467300000000 | 0.0383261700000000 | 1.0 |
| H9  | H | 0.9451939100000000 | 0.1206436800000000 | 0.0632774500000000 | 1.0 |
| H10 | H | 0.4449847900000000 | 0.1205136500000000 | 0.0634613300000000 | 1.0 |
| H11 | H | 0.1476165600000000 | 0.1302512700000000 | 0.9073718100000000 | 1.0 |
| H12 | H | 0.6474152400000000 | 0.1304175100000000 | 0.9076110100000000 | 1.0 |
| H13 | H | 0.3118415000000000 | 0.8731036000000000 | 0.9052936600000000 | 1.0 |
| H14 | H | 0.8117725600000000 | 0.8732404900000000 | 0.9051192600000000 | 1.0 |
| H15 | H | 0.2811991800000000 | 0.8762170200000000 | 0.0738459400000000 | 1.0 |
| H16 | H | 0.7813287500000000 | 0.8760627400000000 | 0.0736192600000000 | 1.0 |
| H17 | H | 0.9911412400000000 | 0.1161470100000000 | 0.8949166400000000 | 1.0 |
| H18 | H | 0.4908921100000000 | 0.1163412200000000 | 0.8952410500000000 | 1.0 |
| H19 | H | 0.8750025400000000 | 0.0552807700000000 | 0.0989375600000000 | 1.0 |
| H20 | H | 0.3748072200000000 | 0.0550836100000000 | 0.0990110400000000 | 1.0 |
| H21 | H | 0.2572255800000000 | 0.9409452200000000 | 0.8683172200000000 | 1.0 |
| H22 | H | 0.7573411800000000 | 0.9411608000000000 | 0.8682207500000000 | 1.0 |
| H23 | H | 0.1238968900000000 | 0.8630684500000000 | 0.0629848900000000 | 1.0 |
| H24 | H | 0.6240001500000000 | 0.8629483500000000 | 0.0627991700000000 | 1.0 |
| C25 | C | 0.0725159600000000 | 0.0548551700000000 | 0.9641698600000000 | 1.0 |
| C26 | C | 0.9496146900000000 | 0.0364297800000000 | 0.0060616300000000 | 1.0 |
| C27 | C | 0.9512942600000000 | 0.9579170000000000 | 0.0043322300000000 | 1.0 |
| C28 | C | 0.0721947400000000 | 0.9414032300000000 | 0.9620725600000000 | 1.0 |
| C29 | C | 0.1982839000000000 | 0.0517011200000000 | 0.0074266800000000 | 1.0 |
| C30 | C | 0.3186778800000000 | 0.0350277700000000 | 0.9645153500000000 | 1.0 |
| C31 | C | 0.3207754600000000 | 0.9566035500000000 | 0.9630927000000000 | 1.0 |
| C32 | C | 0.1982880000000000 | 0.9382794200000000 | 0.0056016600000000 | 1.0 |
| C33 | C | 0.5724657600000000 | 0.0548835400000000 | 0.9642944300000000 | 1.0 |
| C34 | C | 0.4495852600000000 | 0.0363693900000000 | 0.0061467500000000 | 1.0 |
| C35 | C | 0.4513234200000000 | 0.9578629300000000 | 0.0043539500000000 | 1.0 |
| C36 | C | 0.5721927800000000 | 0.9414382500000000 | 0.9620272100000000 | 1.0 |
| C37 | C | 0.6982834500000000 | 0.0516795300000000 | 0.0075049300000000 | 1.0 |
| C38 | C | 0.8186304300000000 | 0.0350827600000000 | 0.9645103800000000 | 1.0 |
| C39 | C | 0.8207729400000000 | 0.9566632200000000 | 0.9630349100000000 | 1.0 |
| C40 | C | 0.6983180300000000 | 0.9382651700000000 | 0.0055224800000000 | 1.0 |
| N41 | N | 0.0624232900000000 | 0.1175740600000000 | 0.9304989700000000 | 1.0 |
| N42 | N | 0.9518516700000000 | 0.0701080300000000 | 0.0700561400000000 | 1.0 |
| N43 | N | 0.3291905600000000 | 0.9230802900000000 | 0.8988219500000000 | 1.0 |
| N44 | N | 0.2083724800000000 | 0.8755490000000000 | 0.0390869500000000 | 1.0 |
| N45 | N | 0.5622912100000000 | 0.1176700600000000 | 0.9307626300000000 | 1.0 |
| N46 | N | 0.4516834400000000 | 0.0699721200000000 | 0.0701782200000000 | 1.0 |

|     |   |                    |                    |                    |     |
|-----|---|--------------------|--------------------|--------------------|-----|
| N47 | N | 0.8292291100000000 | 0.9232170400000000 | 0.8987270600000000 | 1.0 |
| N48 | N | 0.7084392000000000 | 0.8754775900000000 | 0.0388946300000000 | 1.0 |
| O49 | O | 0.0820254700000000 | 0.9983264500000000 | 0.9176881900000000 | 1.0 |
| O50 | O | 0.1902042700000000 | 0.9949670900000000 | 0.0521103500000000 | 1.0 |
| O51 | O | 0.5819445300000000 | 0.9984260400000000 | 0.9177171200000000 | 1.0 |
| O52 | O | 0.6902765200000000 | 0.9948894100000000 | 0.0521171500000000 | 1.0 |

##### cif ends

uran\_NH2\_23\_anti\_dir Energy: -322.65947546

##### cif starts

data\_uran\_NH2\_23\_anti\_dir

\_publ\_section\_comment

;  
Andrew Reynoso, Bohan Xu, and Vincent H. Crespi  
;

\_cell\_length\_a 9.5813754893

\_cell\_length\_b 20.0

\_cell\_length\_c 20.0

\_cell\_angle\_alpha 90.0

\_cell\_angle\_beta 90.0

\_cell\_angle\_gamma 90.0

\_symmetry\_space\_group\_name\_H-M 'P 1'

\_symmetry\_Int\_Tables\_number 1

\_symmetry\_cell\_setting triclinic

loop\_

\_atom\_site\_label

\_atom\_site\_type\_symbol

\_atom\_site\_fract\_x

\_atom\_site\_fract\_y

\_atom\_site\_fract\_z

\_atom\_site\_occupancy

|     |   |                    |                    |                    |     |
|-----|---|--------------------|--------------------|--------------------|-----|
| H1  | H | 0.4612096700000000 | 0.1336715800000000 | 0.9361496600000000 | 1.0 |
| H2  | H | 0.4464095400000000 | 0.0982795700000000 | 0.0708197000000000 | 1.0 |
| H3  | H | 0.5331392400000000 | 0.9958801500000000 | 0.1125025300000000 | 1.0 |
| H4  | H | 0.4665345800000000 | 0.9225656300000000 | 0.0943292600000000 | 1.0 |
| H5  | H | 0.5362399100000000 | 0.8929628200000000 | 0.9151563300000000 | 1.0 |
| H6  | H | 0.3709946000000000 | 0.8943310900000000 | 0.9487349800000000 | 1.0 |
| H7  | H | 0.7116850800000000 | 0.1359720100000000 | 0.0560203800000000 | 1.0 |
| H8  | H | 0.6960317900000000 | 0.0950530600000000 | 0.9220685200000000 | 1.0 |
| H9  | H | 0.7926723000000000 | 0.9860614900000000 | 0.8898170400000000 | 1.0 |
| H10 | H | 0.6299268300000000 | 0.9799606200000000 | 0.8666782400000000 | 1.0 |
| H11 | H | 0.2493988900000000 | 0.9047839200000000 | 0.0988260400000000 | 1.0 |
| H12 | H | 0.1250782100000000 | 0.8929767200000000 | 0.0385444500000000 | 1.0 |
| H13 | H | 0.9611972700000000 | 0.1336908600000000 | 0.9361704800000000 | 1.0 |
| H14 | H | 0.9463924900000000 | 0.0982782900000000 | 0.0708336200000000 | 1.0 |
| H15 | H | 0.0331791100000000 | 0.9958651600000000 | 0.1124916200000000 | 1.0 |
| H16 | H | 0.9665221600000000 | 0.9225580300000000 | 0.0943233000000000 | 1.0 |
| H17 | H | 0.0362363100000000 | 0.8929978800000000 | 0.9151234500000000 | 1.0 |
| H18 | H | 0.8709813200000000 | 0.8943590200000000 | 0.9486827300000000 | 1.0 |
| H19 | H | 0.2117038200000000 | 0.1359738600000000 | 0.0560238000000000 | 1.0 |

|     |   |                    |                    |                    |     |
|-----|---|--------------------|--------------------|--------------------|-----|
| H20 | H | 0.1960154100000000 | 0.0950725100000000 | 0.9220694000000000 | 1.0 |
| H21 | H | 0.2926856900000000 | 0.9860654400000000 | 0.8898163800000000 | 1.0 |
| H22 | H | 0.1299408700000000 | 0.9800046600000000 | 0.8666625500000000 | 1.0 |
| H23 | H | 0.6250928700000000 | 0.8929728600000000 | 0.0385682900000000 | 1.0 |
| H24 | H | 0.7493962000000000 | 0.9047973400000000 | 0.0988544000000000 | 1.0 |
| C25 | C | 0.3992303400000000 | 0.0746878700000000 | 0.0267025300000000 | 1.0 |
| C26 | C | 0.4034835500000000 | 0.9973568100000000 | 0.0320350700000000 | 1.0 |
| C27 | C | 0.4935100200000000 | 0.9759523100000000 | 0.9703265300000000 | 1.0 |
| C28 | C | 0.4857595600000000 | 0.0869644200000000 | 0.9625340400000000 | 1.0 |
| C29 | C | 0.7354269600000000 | 0.0884784600000000 | 0.0309282300000000 | 1.0 |
| C30 | C | 0.6488279300000000 | 0.0739231000000000 | 0.9674568300000000 | 1.0 |
| C31 | C | 0.6535655500000000 | 0.9956428500000000 | 0.9654746800000000 | 1.0 |
| C32 | C | 0.7423958700000000 | 0.9780410500000000 | 0.0283556200000000 | 1.0 |
| C33 | C | 0.9857505100000000 | 0.0869781400000000 | 0.9625447400000000 | 1.0 |
| C34 | C | 0.8992251700000000 | 0.0746897000000000 | 0.0267115900000000 | 1.0 |
| C35 | C | 0.9034874600000000 | 0.9973572500000000 | 0.0320366700000000 | 1.0 |
| C36 | C | 0.9935006600000000 | 0.9759652900000000 | 0.9703175800000000 | 1.0 |
| C37 | C | 0.2354324500000000 | 0.0884814800000000 | 0.0309263800000000 | 1.0 |
| C38 | C | 0.1488215800000000 | 0.0739353100000000 | 0.9674572600000000 | 1.0 |
| C39 | C | 0.1535586200000000 | 0.9956552200000000 | 0.9654647300000000 | 1.0 |
| C40 | C | 0.2423909300000000 | 0.9780436600000000 | 0.0283432200000000 | 1.0 |
| N41 | N | 0.4438719500000000 | 0.9722807000000000 | 0.0978059600000000 | 1.0 |
| N42 | N | 0.4723000700000000 | 0.9092174500000000 | 0.9524170500000000 | 1.0 |
| N43 | N | 0.6992932100000000 | 0.9647663500000000 | 0.9025393100000000 | 1.0 |
| N44 | N | 0.7201733400000000 | 0.9121659300000000 | 0.0505807400000000 | 1.0 |
| N45 | N | 0.9438950100000000 | 0.9722765100000000 | 0.0978021400000000 | 1.0 |
| N46 | N | 0.9722904600000000 | 0.9092343000000000 | 0.9523905200000000 | 1.0 |
| N47 | N | 0.1992819400000000 | 0.9647871700000000 | 0.9025251600000000 | 1.0 |
| N48 | N | 0.2201630200000000 | 0.9121655400000000 | 0.0505563000000000 | 1.0 |
| O49 | O | 0.9458651100000000 | 0.0309601600000000 | 0.9207069600000000 | 1.0 |
| O50 | O | 0.6938229500000000 | 0.0339730300000000 | 0.0735719400000000 | 1.0 |
| O51 | O | 0.4458819900000000 | 0.0309395900000000 | 0.9207037600000000 | 1.0 |
| O52 | O | 0.1938236200000000 | 0.0339738100000000 | 0.0735662800000000 | 1.0 |

##### cif ends

  furan\_NH2\_23\_anti\_dir\_forbid   Energy: -322.12253578

##### cif starts

data\_furan\_NH2\_23\_anti\_dir\_forbid

\_publ\_section\_comment

;  
Andrew Reynoso, Bohan Xu, and Vincent H. Crespi  
;

\_cell\_length\_a   10.4113843815

\_cell\_length\_b   20.0

\_cell\_length\_c   20.0

\_cell\_angle\_alpha   90.0

\_cell\_angle\_beta   90.0

\_cell\_angle\_gamma   90.0

\_symmetry\_space\_group\_name\_H-M   'P 1'

\_symmetry\_Int\_Tables\_number 1

\_symmetry\_cell\_setting triclinic

| loop_                  |   |                    |                    |                    |     |
|------------------------|---|--------------------|--------------------|--------------------|-----|
| _atom_site_label       |   |                    |                    |                    |     |
| _atom_site_type_symbol |   |                    |                    |                    |     |
| _atom_site_fract_x     |   |                    |                    |                    |     |
| _atom_site_fract_y     |   |                    |                    |                    |     |
| _atom_site_fract_z     |   |                    |                    |                    |     |
| _atom_site_occupancy   |   |                    |                    |                    |     |
| H1                     | H | 0.0852348600000000 | 0.1320135200000000 | 0.9457825600000000 | 1.0 |
| H2                     | H | 0.9682704500000000 | 0.0954942500000000 | 0.0669604300000000 | 1.0 |
| H3                     | H | 0.0381113200000000 | 0.9828756200000000 | 0.1136865100000000 | 1.0 |
| H4                     | H | 0.9816173600000000 | 0.9126207200000000 | 0.0821008700000000 | 1.0 |
| H5                     | H | 0.1561708200000000 | 0.8875959000000000 | 0.9304291800000000 | 1.0 |
| H6                     | H | 0.0118494300000000 | 0.9168559800000000 | 0.9048119900000000 | 1.0 |
| H7                     | H | 0.2225690500000000 | 0.1321757600000000 | 0.0515499200000000 | 1.0 |
| H8                     | H | 0.3395626400000000 | 0.0952898900000000 | 0.9304925400000000 | 1.0 |
| H9                     | H | 0.2695177400000000 | 0.9825962100000000 | 0.8840908100000000 | 1.0 |
| H10                    | H | 0.3259977000000000 | 0.9124042700000000 | 0.9158055200000000 | 1.0 |
| H11                    | H | 0.1516116300000000 | 0.8878914100000000 | 0.0677995900000000 | 1.0 |
| H12                    | H | 0.2960967400000000 | 0.9171662300000000 | 0.0931301900000000 | 1.0 |
| H13                    | H | 0.5852264900000000 | 0.1320639600000000 | 0.9458441900000000 | 1.0 |
| H14                    | H | 0.4682330700000000 | 0.0954428200000000 | 0.0669765300000000 | 1.0 |
| H15                    | H | 0.5382993400000000 | 0.9828395000000000 | 0.1136231800000000 | 1.0 |
| H16                    | H | 0.4817708700000000 | 0.9125871300000000 | 0.0820681000000000 | 1.0 |
| H17                    | H | 0.6561862400000000 | 0.8877666100000000 | 0.9300911700000000 | 1.0 |
| H18                    | H | 0.5116463200000000 | 0.9169576000000000 | 0.9047548900000000 | 1.0 |
| H19                    | H | 0.7225583700000000 | 0.1321297700000000 | 0.0516103000000000 | 1.0 |
| H20                    | H | 0.8395286200000000 | 0.0953462100000000 | 0.9305104400000000 | 1.0 |
| H21                    | H | 0.7697026500000000 | 0.9826466100000000 | 0.8840251400000000 | 1.0 |
| H22                    | H | 0.8261402500000000 | 0.9124474800000000 | 0.9157611900000000 | 1.0 |
| H23                    | H | 0.6516103800000000 | 0.8877180100000000 | 0.0674422800000000 | 1.0 |
| H24                    | H | 0.7958763200000000 | 0.9170568300000000 | 0.0930733700000000 | 1.0 |
| C25                    | C | 0.0922008200000000 | 0.0865342300000000 | 0.9765932300000000 | 1.0 |
| C26                    | C | 0.9694826300000000 | 0.0707993900000000 | 0.0178903100000000 | 1.0 |
| C27                    | C | 0.9695450700000000 | 0.9927351600000000 | 0.0197767100000000 | 1.0 |
| C28                    | C | 0.0905848400000000 | 0.9722039600000000 | 0.9772670900000000 | 1.0 |
| C29                    | C | 0.2155955500000000 | 0.0865999500000000 | 0.0208795600000000 | 1.0 |
| C30                    | C | 0.3383109700000000 | 0.0707340000000000 | 0.9796313300000000 | 1.0 |
| C31                    | C | 0.3382207600000000 | 0.9926618200000000 | 0.9779479500000000 | 1.0 |
| C32                    | C | 0.2171971700000000 | 0.9722659500000000 | 0.0205551600000000 | 1.0 |
| C33                    | C | 0.5921930900000000 | 0.0865543400000000 | 0.9766119800000000 | 1.0 |
| C34                    | C | 0.4694791200000000 | 0.0707761200000000 | 0.0178919300000000 | 1.0 |
| C35                    | C | 0.4695746600000000 | 0.9927094000000000 | 0.0197479600000000 | 1.0 |
| C36                    | C | 0.5905979600000000 | 0.9722230300000000 | 0.9771834900000000 | 1.0 |
| C37                    | C | 0.7155912300000000 | 0.0865820600000000 | 0.0208983000000000 | 1.0 |
| C38                    | C | 0.8383142100000000 | 0.0707601200000000 | 0.9796334600000000 | 1.0 |
| C39                    | C | 0.8382533100000000 | 0.9926913100000000 | 0.9779178100000000 | 1.0 |
| C40                    | C | 0.7172141300000000 | 0.9722498600000000 | 0.0204713400000000 | 1.0 |
| N41                    | N | 0.9648066300000000 | 0.9628263800000000 | 0.0862150800000000 | 1.0 |
| N42                    | N | 0.0728608000000000 | 0.9099166300000000 | 0.9442388800000000 | 1.0 |
| N43                    | N | 0.3428507500000000 | 0.9625960400000000 | 0.9115774800000000 | 1.0 |
| N44                    | N | 0.2349229800000000 | 0.9100895100000000 | 0.0537909600000000 | 1.0 |
| N45                    | N | 0.4649469600000000 | 0.9627908900000000 | 0.0861858600000000 | 1.0 |
| N46                    | N | 0.5728719500000000 | 0.9099708000000000 | 0.9440886700000000 | 1.0 |
| N47                    | N | 0.8429859600000000 | 0.9626413100000000 | 0.9115435100000000 | 1.0 |

|     |   |                    |                    |                    |     |
|-----|---|--------------------|--------------------|--------------------|-----|
| N48 | N | 0.7349276400000000 | 0.9100342200000000 | 0.0536361800000000 | 1.0 |
| O49 | O | 0.1027782000000000 | 0.0301973800000000 | 0.9314967600000000 | 1.0 |
| O50 | O | 0.2050233200000000 | 0.0304023400000000 | 0.0661442200000000 | 1.0 |
| O51 | O | 0.6027698200000000 | 0.0302564200000000 | 0.9314657500000000 | 1.0 |
| O52 | O | 0.7050211300000000 | 0.0303450300000000 | 0.0661140600000000 | 1.0 |

##### cif ends

furand\_NH2\_23\_synalt Energy: -322.99171837

##### cif starts

data\_furand\_NH2\_23\_synalt

\_publ\_section\_comment

;  
Andrew Reynoso, Bohan Xu, and Vincent H. Crespi  
;

\_cell\_length\_a 10.3793103005

\_cell\_length\_b 20.0

\_cell\_length\_c 20.0

\_cell\_angle\_alpha 90.0

\_cell\_angle\_beta 90.0

\_cell\_angle\_gamma 90.0

\_symmetry\_space\_group\_name\_H-M 'P 1'

\_symmetry\_Int\_Tables\_number 1

\_symmetry\_cell\_setting triclinic

loop\_

\_atom\_site\_label

\_atom\_site\_type\_symbol

\_atom\_site\_fract\_x

\_atom\_site\_fract\_y

\_atom\_site\_fract\_z

\_atom\_site\_occupancy

|     |   |                    |                    |                    |     |
|-----|---|--------------------|--------------------|--------------------|-----|
| H1  | H | 0.4784022000000000 | 0.8759687500000000 | 0.0192568400000000 | 1.0 |
| H2  | H | 0.6003579900000000 | 0.9428059100000000 | 0.9182200600000000 | 1.0 |
| H3  | H | 0.6744855200000000 | 0.0744134800000000 | 0.9047152300000000 | 1.0 |
| H4  | H | 0.5818944700000000 | 0.1230382600000000 | 0.9502238800000000 | 1.0 |
| H5  | H | 0.5542801600000000 | 0.0835133500000000 | 0.1144760100000000 | 1.0 |
| H6  | H | 0.3977737800000000 | 0.0916257100000000 | 0.1077373600000000 | 1.0 |
| H7  | H | 0.7270679300000000 | 0.0749270400000000 | 0.0697271500000000 | 1.0 |
| H8  | H | 0.8585178300000000 | 0.0642338200000000 | 0.9490113800000000 | 1.0 |
| H9  | H | 0.8991517000000000 | 0.9731837200000000 | 0.8715910300000000 | 1.0 |
| H10 | H | 0.7711937300000000 | 0.9247216800000000 | 0.8807309300000000 | 1.0 |
| H11 | H | 0.3094126300000000 | 0.8448829500000000 | 0.0474697400000000 | 1.0 |
| H12 | H | 0.1512991600000000 | 0.8454218900000000 | 0.0498602000000000 | 1.0 |
| H13 | H | 0.9784143800000000 | 0.8760329800000000 | 0.0194747500000000 | 1.0 |
| H14 | H | 0.1001928100000000 | 0.9427506400000000 | 0.9182646800000000 | 1.0 |
| H15 | H | 0.1746737700000000 | 0.0743018900000000 | 0.9046754400000000 | 1.0 |
| H16 | H | 0.0821815000000000 | 0.1230220300000000 | 0.9501408100000000 | 1.0 |
| H17 | H | 0.0542128100000000 | 0.0837928500000000 | 0.1143084600000000 | 1.0 |
| H18 | H | 0.8977036000000000 | 0.0918927700000000 | 0.1075149200000000 | 1.0 |
| H19 | H | 0.2270388100000000 | 0.0748692700000000 | 0.0698015800000000 | 1.0 |
| H20 | H | 0.3585675000000000 | 0.0642879200000000 | 0.9491268100000000 | 1.0 |



|     |   |                    |                    |                    |     |
|-----|---|--------------------|--------------------|--------------------|-----|
| H21 | H | 0.3992274400000000 | 0.9733342200000000 | 0.8716020100000000 | 1.0 |
| H22 | H | 0.2710310000000000 | 0.9250271400000000 | 0.8806428100000000 | 1.0 |
| H23 | H | 0.6512662600000000 | 0.8454980800000000 | 0.0499821400000000 | 1.0 |
| H24 | H | 0.8093740200000000 | 0.8449031400000000 | 0.0475141600000000 | 1.0 |
| C25 | C | 0.6035126700000000 | 0.9534752100000000 | 0.9719343800000000 | 1.0 |
| C26 | C | 0.6034011600000000 | 0.0295875800000000 | 0.9896852800000000 | 1.0 |
| C27 | C | 0.4784700900000000 | 0.0341240300000000 | 0.0354570100000000 | 1.0 |
| C28 | C | 0.4793222300000000 | 0.9296528500000000 | 0.0078986500000000 | 1.0 |
| C29 | C | 0.7292081500000000 | 0.0335275400000000 | 0.0335688500000000 | 1.0 |
| C30 | C | 0.8539638800000000 | 0.0296516400000000 | 0.9914320400000000 | 1.0 |
| C31 | C | 0.8547815900000000 | 0.9536968100000000 | 0.9703234100000000 | 1.0 |
| C32 | C | 0.7287448800000000 | 0.9280558700000000 | 0.0075263100000000 | 1.0 |
| C33 | C | 0.9793246900000000 | 0.9296938000000000 | 0.0080051800000000 | 1.0 |
| C34 | C | 0.1034857500000000 | 0.9534613500000000 | 0.9719679200000000 | 1.0 |
| C35 | C | 0.1034356000000000 | 0.0295862500000000 | 0.9896704200000000 | 1.0 |
| C36 | C | 0.9784601000000000 | 0.0342098900000000 | 0.0353838000000000 | 1.0 |
| C37 | C | 0.2292034600000000 | 0.0334960800000000 | 0.0336128400000000 | 1.0 |
| C38 | C | 0.3539755800000000 | 0.0296539700000000 | 0.9915022100000000 | 1.0 |
| C39 | C | 0.3547616800000000 | 0.9537291100000000 | 0.9702875100000000 | 1.0 |
| C40 | C | 0.2287552900000000 | 0.9280395600000000 | 0.0075019000000000 | 1.0 |
| N41 | N | 0.5927161600000000 | 0.0751668200000000 | 0.9330383900000000 | 1.0 |
| N42 | N | 0.4810712700000000 | 0.0889477800000000 | 0.0808842800000000 | 1.0 |
| N43 | N | 0.8593511800000000 | 0.9361052600000000 | 0.8997797500000000 | 1.0 |
| N44 | N | 0.7289607500000000 | 0.8585739400000000 | 0.0217286800000000 | 1.0 |
| N45 | N | 0.0928977900000000 | 0.0751316200000000 | 0.9329912500000000 | 1.0 |
| N46 | N | 0.9810242000000000 | 0.0891321700000000 | 0.0806914400000000 | 1.0 |
| N47 | N | 0.3592479700000000 | 0.9362487900000000 | 0.8997156700000000 | 1.0 |
| N48 | N | 0.2290283900000000 | 0.8585482300000000 | 0.0216572500000000 | 1.0 |
| O49 | O | 0.9788792600000000 | 0.9688102800000000 | 0.0677370900000000 | 1.0 |
| O50 | O | 0.7291080200000000 | 0.9706006200000000 | 0.0674075100000000 | 1.0 |
| O51 | O | 0.4788922700000000 | 0.9686658200000000 | 0.0676975900000000 | 1.0 |
| O52 | O | 0.2291089400000000 | 0.9705456500000000 | 0.0674089800000000 | 1.0 |

##### cif ends

furand\_NH2\_23\_syn\_alt\_forbid Energy: -320.14446403

##### cif starts

data\_furand\_NH2\_23\_syn\_alt\_forbid

\_publ\_section\_comment

;  
Andrew Reynoso, Bohan Xu, and Vincent H. Crespi  
;

\_cell\_length\_a 9.7138095413

\_cell\_length\_b 20.0

\_cell\_length\_c 20.0

\_cell\_angle\_alpha 90.0

\_cell\_angle\_beta 90.0

\_cell\_angle\_gamma 90.0

\_symmetry\_space\_group\_name\_H-M 'P 1'

\_symmetry\_Int\_Tables\_number 1

\_symmetry\_cell\_setting triclinic

| loop_ |   | _atom_site_label       |                    |                    |     |  |
|-------|---|------------------------|--------------------|--------------------|-----|--|
|       |   | _atom_site_type_symbol |                    |                    |     |  |
|       |   | _atom_site_fract_x     |                    |                    |     |  |
|       |   | _atom_site_fract_y     |                    |                    |     |  |
|       |   | _atom_site_fract_z     |                    |                    |     |  |
|       |   | _atom_site_occupancy   |                    |                    |     |  |
| H1    | H | 0.0080640500000000     | 0.0961145100000000 | 0.0629689700000000 | 1.0 |  |
| H2    | H | 0.0029211500000000     | 0.0580205300000000 | 0.9288336000000000 | 1.0 |  |
| H3    | H | 0.2497969400000000     | 0.9314968200000000 | 0.9322764700000000 | 1.0 |  |
| H4    | H | 0.2446746600000000     | 0.9007615200000000 | 0.0682832700000000 | 1.0 |  |
| H5    | H | 0.5080644100000000     | 0.0961006500000000 | 0.0629843600000000 | 1.0 |  |
| H6    | H | 0.5029318400000000     | 0.0580180700000000 | 0.9288434400000000 | 1.0 |  |
| H7    | H | 0.7498081000000000     | 0.9314959800000000 | 0.9322648300000000 | 1.0 |  |
| H8    | H | 0.7446858800000000     | 0.9007510500000000 | 0.0682709400000000 | 1.0 |  |
| H9    | H | 0.0089295000000000     | 0.8711310000000000 | 0.9233623500000000 | 1.0 |  |
| H10   | H | 0.5607210200000000     | 0.8669225600000000 | 0.1093708600000000 | 1.0 |  |
| H11   | H | 0.5089083800000000     | 0.8711224600000000 | 0.9233778700000000 | 1.0 |  |
| H12   | H | 0.0606108100000000     | 0.8669577200000000 | 0.1094008100000000 | 1.0 |  |
| H13   | H | 0.1922012200000000     | 0.1320916100000000 | 0.1021954700000000 | 1.0 |  |
| H14   | H | 0.2437651600000000     | 0.1178261500000000 | 0.9166680000000000 | 1.0 |  |
| H15   | H | 0.6922374300000000     | 0.1320772200000000 | 0.1022072700000000 | 1.0 |  |
| H16   | H | 0.7437137100000000     | 0.1178253300000000 | 0.9166723000000000 | 1.0 |  |
| H17   | H | 0.9572352000000000     | 0.9312736800000000 | 0.8737589700000000 | 1.0 |  |
| H18   | H | 0.4572040700000000     | 0.9312573200000000 | 0.8737673100000000 | 1.0 |  |
| H19   | H | 0.2955910700000000     | 0.0551085900000000 | 0.8703975700000000 | 1.0 |  |
| H20   | H | 0.7955717000000000     | 0.0551183400000000 | 0.8703953400000000 | 1.0 |  |
| H21   | H | 0.3434310300000000     | 0.1282535200000000 | 0.0647124100000000 | 1.0 |  |
| H22   | H | 0.8434339100000000     | 0.1282525400000000 | 0.0646903900000000 | 1.0 |  |
| H23   | H | 0.9093011700000000     | 0.8687803000000000 | 0.0718403100000000 | 1.0 |  |
| H24   | H | 0.4093241300000000     | 0.8687866400000000 | 0.0718976700000000 | 1.0 |  |
| C25   | C | 0.0400622100000000     | 0.0502928800000000 | 0.0370698700000000 | 1.0 |  |
| C26   | C | 0.9586262200000000     | 0.0344702600000000 | 0.9733934400000000 | 1.0 |  |
| C27   | C | 0.9598810900000000     | 0.9562125000000000 | 0.9733300400000000 | 1.0 |  |
| C28   | C | 0.0449141200000000     | 0.9394813500000000 | 0.0381806600000000 | 1.0 |  |
| C29   | C | 0.2077979300000000     | 0.0558126700000000 | 0.0350055200000000 | 1.0 |  |
| C30   | C | 0.2928304300000000     | 0.0355785400000000 | 0.9711659000000000 | 1.0 |  |
| C31   | C | 0.2940803700000000     | 0.9574417100000000 | 0.9754881900000000 | 1.0 |  |
| C32   | C | 0.2126551700000000     | 0.9451053100000000 | 0.0399328600000000 | 1.0 |  |
| C33   | C | 0.5400632500000000     | 0.0502826900000000 | 0.0370801100000000 | 1.0 |  |
| C34   | C | 0.4586294000000000     | 0.0344657800000000 | 0.9734016500000000 | 1.0 |  |
| C35   | C | 0.4598728300000000     | 0.9562079000000000 | 0.9733350000000000 | 1.0 |  |
| C36   | C | 0.5449114400000000     | 0.9394711100000000 | 0.0381817600000000 | 1.0 |  |
| C37   | C | 0.7077972600000000     | 0.0558042700000000 | 0.0350067100000000 | 1.0 |  |
| C38   | C | 0.7928251300000000     | 0.0355773900000000 | 0.9711617500000000 | 1.0 |  |
| C39   | C | 0.7940820400000000     | 0.9574407300000000 | 0.9754799100000000 | 1.0 |  |
| C40   | C | 0.7126564300000000     | 0.9450963700000000 | 0.0399239500000000 | 1.0 |  |
| N41   | N | 0.0155271400000000     | 0.9215740800000000 | 0.9151368600000000 | 1.0 |  |
| N42   | N | 0.0122158800000000     | 0.8750763400000000 | 0.0648522300000000 | 1.0 |  |
| N43   | N | 0.2405044600000000     | 0.1215746600000000 | 0.0581276500000000 | 1.0 |  |
| N44   | N | 0.2372218200000000     | 0.0670128400000000 | 0.9111742800000000 | 1.0 |  |
| N45   | N | 0.5155095400000000     | 0.9215634500000000 | 0.9151431800000000 | 1.0 |  |
| N46   | N | 0.5122261200000000     | 0.8750645600000000 | 0.0648516600000000 | 1.0 |  |
| N47   | N | 0.7405046600000000     | 0.1215640600000000 | 0.0581295000000000 | 1.0 |  |
| N48   | N | 0.7372019300000000     | 0.0670111600000000 | 0.9111743700000000 | 1.0 |  |

|     |   |                    |                    |                    |     |
|-----|---|--------------------|--------------------|--------------------|-----|
| O49 | O | 0.0079468900000000 | 0.9954699400000000 | 0.0803313700000000 | 1.0 |
| O50 | O | 0.2447726500000000 | 0.0022020900000000 | 0.0801390300000000 | 1.0 |
| O51 | O | 0.5079539300000000 | 0.9954555400000000 | 0.0803376300000000 | 1.0 |
| O52 | O | 0.7447792100000000 | 0.0021892600000000 | 0.0801346000000000 | 1.0 |

##### cif ends

furand\_NH2\_23\_syn\_dir Energy: -321.81327906

##### cif starts

data\_furand\_NH2\_23\_syn\_dir

\_publ\_section\_comment

;  
Andrew Reynoso, Bohan Xu, and Vincent H. Crespi  
;

\_cell\_length\_a 10.6313881477

\_cell\_length\_b 20.0

\_cell\_length\_c 20.0

\_cell\_angle\_alpha 90.0

\_cell\_angle\_beta 90.0

\_cell\_angle\_gamma 90.0

\_symmetry\_space\_group\_name\_H-M 'P 1'

\_symmetry\_Int\_Tables\_number 1

\_symmetry\_cell\_setting triclinic

loop\_

\_atom\_site\_label

\_atom\_site\_type\_symbol

\_atom\_site\_fract\_x

\_atom\_site\_fract\_y

\_atom\_site\_fract\_z

\_atom\_site\_occupancy

|     |   |                    |                    |                    |     |
|-----|---|--------------------|--------------------|--------------------|-----|
| H1  | H | 0.3617627800000000 | 0.1369198500000000 | 0.0526840200000000 | 1.0 |
| H2  | H | 0.4868227100000000 | 0.1010991100000000 | 0.9338367500000000 | 1.0 |
| H3  | H | 0.4018833000000000 | 0.9793400700000000 | 0.8908121400000000 | 1.0 |
| H4  | H | 0.4962916200000000 | 0.9198996500000000 | 0.9153791000000000 | 1.0 |
| H5  | H | 0.2705565800000000 | 0.8962676400000000 | 0.0471570000000000 | 1.0 |
| H6  | H | 0.3774367200000000 | 0.9218488700000000 | 0.1014896800000000 | 1.0 |
| H7  | H | 0.6117627800000000 | 0.1369539500000000 | 0.0527004200000000 | 1.0 |
| H8  | H | 0.7368418800000000 | 0.1011365200000000 | 0.9338512200000000 | 1.0 |
| H9  | H | 0.6519280300000000 | 0.9795576000000000 | 0.8907594400000000 | 1.0 |
| H10 | H | 0.7461649400000000 | 0.9200097200000000 | 0.9152554200000000 | 1.0 |
| H11 | H | 0.1268462500000000 | 0.9220333800000000 | 0.1016419800000000 | 1.0 |
| H12 | H | 0.0206922500000000 | 0.8962029100000000 | 0.0470423800000000 | 1.0 |
| H13 | H | 0.8618584000000000 | 0.1369717200000000 | 0.0526919900000000 | 1.0 |
| H14 | H | 0.9868463500000000 | 0.1011048200000000 | 0.9338252900000000 | 1.0 |
| H15 | H | 0.9019833500000000 | 0.9795605000000000 | 0.8907547700000000 | 1.0 |
| H16 | H | 0.9958779400000000 | 0.9199192200000000 | 0.9153675700000000 | 1.0 |
| H17 | H | 0.7705316100000000 | 0.8963334900000000 | 0.0472082100000000 | 1.0 |
| H18 | H | 0.8773692400000000 | 0.9219798200000000 | 0.1015351300000000 | 1.0 |
| H19 | H | 0.1118996600000000 | 0.1369575500000000 | 0.0526401900000000 | 1.0 |
| H20 | H | 0.2368969000000000 | 0.1010470800000000 | 0.9338015600000000 | 1.0 |
| H21 | H | 0.1519203800000000 | 0.9792944600000000 | 0.8908166100000000 | 1.0 |

|     |   |                    |                    |                    |     |
|-----|---|--------------------|--------------------|--------------------|-----|
| H22 | H | 0.2461075200000000 | 0.9197834000000000 | 0.9154883700000000 | 1.0 |
| H23 | H | 0.5207735200000000 | 0.8961688400000000 | 0.0469376700000000 | 1.0 |
| H24 | H | 0.6266719700000000 | 0.9220598000000000 | 0.1016333500000000 | 1.0 |
| C25 | C | 0.4867648400000000 | 0.0769590300000000 | 0.9831951300000000 | 1.0 |
| C26 | C | 0.4869679000000000 | 0.9987302000000000 | 0.9792079500000000 | 1.0 |
| C27 | C | 0.3609503700000000 | 0.9818851400000000 | 0.0212281500000000 | 1.0 |
| C28 | C | 0.3615926300000000 | 0.0899528000000000 | 0.0241763600000000 | 1.0 |
| C29 | C | 0.6115878400000000 | 0.0899931200000000 | 0.0241829200000000 | 1.0 |
| C30 | C | 0.7367706900000000 | 0.0769936300000000 | 0.9832087300000000 | 1.0 |
| C31 | C | 0.7369665900000000 | 0.9987639700000000 | 0.9792058000000000 | 1.0 |
| C32 | C | 0.6109437400000000 | 0.9819299500000000 | 0.0212234800000000 | 1.0 |
| C33 | C | 0.8616193200000000 | 0.0900030000000000 | 0.0241864700000000 | 1.0 |
| C34 | C | 0.9867840300000000 | 0.0769731700000000 | 0.9831882000000000 | 1.0 |
| C35 | C | 0.9869634300000000 | 0.9987460400000000 | 0.9792166600000000 | 1.0 |
| C36 | C | 0.8609421500000000 | 0.9819319300000000 | 0.0212281100000000 | 1.0 |
| C37 | C | 0.1116328900000000 | 0.0899812400000000 | 0.0241487800000000 | 1.0 |
| C38 | C | 0.2367890400000000 | 0.0769246600000000 | 0.9831684000000000 | 1.0 |
| C39 | C | 0.2369642200000000 | 0.9986894000000000 | 0.9792220200000000 | 1.0 |
| C40 | C | 0.1109383100000000 | 0.9819174200000000 | 0.0212456000000000 | 1.0 |
| N41 | N | 0.4898200500000000 | 0.9709130900000000 | 0.9116375100000000 | 1.0 |
| N42 | N | 0.3597206400000000 | 0.9163315700000000 | 0.0515672100000000 | 1.0 |
| N43 | N | 0.7398146500000000 | 0.9710317200000000 | 0.9115990200000000 | 1.0 |
| N44 | N | 0.6097331900000000 | 0.9164020800000000 | 0.0516497500000000 | 1.0 |
| N45 | N | 0.9898002200000000 | 0.9709475600000000 | 0.9116378300000000 | 1.0 |
| N46 | N | 0.8596993100000000 | 0.9164024200000000 | 0.0516162200000000 | 1.0 |
| N47 | N | 0.2397974400000000 | 0.9707980100000000 | 0.9116805800000000 | 1.0 |
| N48 | N | 0.1096995700000000 | 0.9163959600000000 | 0.0516769500000000 | 1.0 |
| O49 | O | 0.8606787900000000 | 0.0346777800000000 | 0.0701526700000000 | 1.0 |
| O50 | O | 0.6106758400000000 | 0.0346552000000000 | 0.0701431400000000 | 1.0 |
| O51 | O | 0.3606699700000000 | 0.0346277500000000 | 0.0701516300000000 | 1.0 |
| O52 | O | 0.1106896600000000 | 0.0346691700000000 | 0.0701404200000000 | 1.0 |

##### cif ends

furan\_NH2\_23\_syn\_dir\_forbid Energy: -319.47305128

##### cif starts

data\_furan\_NH2\_23\_syn\_dir\_forbid

\_publ\_section\_comment

;  
Andrew Reynoso, Bohan Xu, and Vincent H. Crespi  
;

\_cell\_length\_a 9.8028141759

\_cell\_length\_b 20.0

\_cell\_length\_c 20.0

\_cell\_angle\_alpha 90.0

\_cell\_angle\_beta 90.0

\_cell\_angle\_gamma 90.0

\_symmetry\_space\_group\_name\_H-M 'P 1'

\_symmetry\_Int\_Tables\_number 1

\_symmetry\_cell\_setting triclinic

loop\_

|     | _atom_site_label       |                    |                    |                    |     |
|-----|------------------------|--------------------|--------------------|--------------------|-----|
|     | _atom_site_type_symbol |                    |                    |                    |     |
|     | _atom_site_fract_x     |                    |                    |                    |     |
|     | _atom_site_fract_y     |                    |                    |                    |     |
|     | _atom_site_fract_z     |                    |                    |                    |     |
|     | _atom_site_occupancy   |                    |                    |                    |     |
| H1  | H                      | 0.0232115800000000 | 0.1095446300000000 | 0.0400954900000000 | 1.0 |
| H2  | H                      | 0.0015375300000000 | 0.0473789900000000 | 0.9159786300000000 | 1.0 |
| H3  | H                      | 0.2520208200000000 | 0.0952642100000000 | 0.0665613400000000 | 1.0 |
| H4  | H                      | 0.2612575500000000 | 0.0718660800000000 | 0.9285592200000000 | 1.0 |
| H5  | H                      | 0.5232447700000000 | 0.1095559500000000 | 0.0400952000000000 | 1.0 |
| H6  | H                      | 0.5015186500000000 | 0.0473968300000000 | 0.9159802000000000 | 1.0 |
| H7  | H                      | 0.7520500200000000 | 0.0952631200000000 | 0.0665463600000000 | 1.0 |
| H8  | H                      | 0.7612661400000000 | 0.0718471700000000 | 0.9285455100000000 | 1.0 |
| H9  | H                      | 0.0170156500000000 | 0.8607785300000000 | 0.9593281400000000 | 1.0 |
| H10 | H                      | 0.1441159700000000 | 0.9240962900000000 | 0.8987243600000000 | 1.0 |
| H11 | H                      | 0.5169915400000000 | 0.8607909700000000 | 0.9593232900000000 | 1.0 |
| H12 | H                      | 0.6441079900000000 | 0.9240959800000000 | 0.8987248600000000 | 1.0 |
| H13 | H                      | 0.0204339700000000 | 0.9134340000000000 | 0.1379165600000000 | 1.0 |
| H14 | H                      | 0.1478836600000000 | 0.8523734600000000 | 0.0656576000000000 | 1.0 |
| H15 | H                      | 0.5203999000000000 | 0.9134587600000000 | 0.1379211000000000 | 1.0 |
| H16 | H                      | 0.6478590600000000 | 0.8523836200000000 | 0.0656709900000000 | 1.0 |
| H17 | H                      | 0.8875452800000000 | 0.8880704100000000 | 0.0903611900000000 | 1.0 |
| H18 | H                      | 0.3875338800000000 | 0.8880837000000000 | 0.0903586200000000 | 1.0 |
| H19 | H                      | 0.2708017800000000 | 0.8508118000000000 | 0.0054387100000000 | 1.0 |
| H20 | H                      | 0.7707582400000000 | 0.8508032800000000 | 0.0054442700000000 | 1.0 |
| H21 | H                      | 0.9103377000000000 | 0.8916512000000000 | 0.9013453400000000 | 1.0 |
| H22 | H                      | 0.4103325800000000 | 0.8916773500000000 | 0.9013356800000000 | 1.0 |
| H23 | H                      | 0.7645020900000000 | 0.9730202800000000 | 0.8625712800000000 | 1.0 |
| H24 | H                      | 0.2644331500000000 | 0.9730666200000000 | 0.8625759400000000 | 1.0 |
| C25 | C                      | 0.0532767100000000 | 0.0584278700000000 | 0.0260883600000000 | 1.0 |
| C26 | C                      | 0.9649640700000000 | 0.0327943200000000 | 0.9658514600000000 | 1.0 |
| C27 | C                      | 0.9440721200000000 | 0.9546091200000000 | 0.9775540200000000 | 1.0 |
| C28 | C                      | 0.0227072600000000 | 0.9501479000000000 | 0.0447868700000000 | 1.0 |
| C29 | C                      | 0.2202194400000000 | 0.0532164300000000 | 0.0349012000000000 | 1.0 |
| C30 | C                      | 0.3016905100000000 | 0.0419049700000000 | 0.9702129200000000 | 1.0 |
| C31 | C                      | 0.2795924500000000 | 0.9656947700000000 | 0.9645440300000000 | 1.0 |
| C32 | C                      | 0.1926699900000000 | 0.9430554600000000 | 0.0272501600000000 | 1.0 |
| C33 | C                      | 0.5532902600000000 | 0.0584370100000000 | 0.0260862200000000 | 1.0 |
| C34 | C                      | 0.4649577800000000 | 0.0328084600000000 | 0.9658544100000000 | 1.0 |
| C35 | C                      | 0.4440650800000000 | 0.9546229000000000 | 0.9775540300000000 | 1.0 |
| C36 | C                      | 0.5227017900000000 | 0.9501587100000000 | 0.0447873000000000 | 1.0 |
| C37 | C                      | 0.7202326200000000 | 0.0532143900000000 | 0.0348918200000000 | 1.0 |
| C38 | C                      | 0.8016980400000000 | 0.0418922000000000 | 0.9702037300000000 | 1.0 |
| C39 | C                      | 0.7795999800000000 | 0.9656806900000000 | 0.9645436800000000 | 1.0 |
| C40 | C                      | 0.6926703500000000 | 0.9430544100000000 | 0.0272510900000000 | 1.0 |
| N41 | N                      | 0.9919709800000000 | 0.9025091300000000 | 0.9325465700000000 | 1.0 |
| N42 | N                      | 0.9909654900000000 | 0.8984380500000000 | 0.0913092900000000 | 1.0 |
| N43 | N                      | 0.2463772400000000 | 0.9389716600000000 | 0.8994120600000000 | 1.0 |
| N44 | N                      | 0.2311670400000000 | 0.8762351400000000 | 0.0449786300000000 | 1.0 |
| N45 | N                      | 0.4919598200000000 | 0.9025252200000000 | 0.9325442900000000 | 1.0 |
| N46 | N                      | 0.4909521100000000 | 0.8984538900000000 | 0.0913137300000000 | 1.0 |
| N47 | N                      | 0.7463858900000000 | 0.9389440700000000 | 0.8994175800000000 | 1.0 |
| N48 | N                      | 0.7311525700000000 | 0.8762338200000000 | 0.0449867700000000 | 1.0 |
| O49 | O                      | 0.0076329100000000 | 0.0139221800000000 | 0.0766826100000000 | 1.0 |

|     |   |                    |                    |                    |     |
|-----|---|--------------------|--------------------|--------------------|-----|
| O50 | O | 0.2433328000000000 | 0.9933412400000000 | 0.0732853600000000 | 1.0 |
| O51 | O | 0.5076421800000000 | 0.0139341300000000 | 0.0766823900000000 | 1.0 |
| O52 | O | 0.7433376400000000 | 0.9933418000000000 | 0.0732812700000000 | 1.0 |

##### cif ends

furand\_NH2\_24\_anti\_alt Energy: -322.4690387

##### cif starts

data\_furand\_NH2\_24\_anti\_alt

\_publ\_section\_comment

;  
Andrew Reynoso, Bohan Xu, and Vincent H. Crespi  
;

\_cell\_length\_a 9.6633596179

\_cell\_length\_b 20.0

\_cell\_length\_c 20.0

\_cell\_angle\_alpha 90.0

\_cell\_angle\_beta 90.0

\_cell\_angle\_gamma 90.0

\_symmetry\_space\_group\_name\_H-M 'P 1'

\_symmetry\_Int\_Tables\_number 1

\_symmetry\_cell\_setting triclinic

loop\_

\_atom\_site\_label

\_atom\_site\_type\_symbol

\_atom\_site\_fract\_x

\_atom\_site\_fract\_y

\_atom\_site\_fract\_z

\_atom\_site\_occupancy

|     |   |                    |                    |                    |     |
|-----|---|--------------------|--------------------|--------------------|-----|
| H1  | H | 0.5212518700000000 | 0.9405387800000000 | 0.0745771800000000 | 1.0 |
| H2  | H | 0.5008187800000000 | 0.1038529600000000 | 0.9433986800000000 | 1.0 |
| H3  | H | 0.5404454900000000 | 0.0421852800000000 | 0.1326696800000000 | 1.0 |
| H4  | H | 0.4193111300000000 | 0.0872739300000000 | 0.0931465500000000 | 1.0 |
| H5  | H | 0.4192975800000000 | 0.8675044500000000 | 0.9121772400000000 | 1.0 |
| H6  | H | 0.5410436700000000 | 0.8483622800000000 | 0.9718206200000000 | 1.0 |
| H7  | H | 0.7712413500000000 | 0.0617355400000000 | 0.9213183200000000 | 1.0 |
| H8  | H | 0.7508095300000000 | 0.8984095900000000 | 0.0524849000000000 | 1.0 |
| H9  | H | 0.7903956100000000 | 0.9600807100000000 | 0.8632241500000000 | 1.0 |
| H10 | H | 0.6693052400000000 | 0.9149805200000000 | 0.9027631600000000 | 1.0 |
| H11 | H | 0.2910959500000000 | 0.1539027500000000 | 0.0241087000000000 | 1.0 |
| H12 | H | 0.1693111500000000 | 0.1347527500000000 | 0.0837328700000000 | 1.0 |
| H13 | H | 0.0212538600000000 | 0.9405388800000000 | 0.0745778600000000 | 1.0 |
| H14 | H | 0.0008183500000000 | 0.1038521100000000 | 0.9433981100000000 | 1.0 |
| H15 | H | 0.0404461900000000 | 0.0421856000000000 | 0.1326697200000000 | 1.0 |
| H16 | H | 0.9193106400000000 | 0.0872736300000000 | 0.0931465400000000 | 1.0 |
| H17 | H | 0.9192988500000000 | 0.8675025000000000 | 0.9121793900000000 | 1.0 |
| H18 | H | 0.0410476300000000 | 0.8483621700000000 | 0.9718220800000000 | 1.0 |
| H19 | H | 0.2712414600000000 | 0.0617369200000000 | 0.9213185800000000 | 1.0 |
| H20 | H | 0.2508113300000000 | 0.8984098300000000 | 0.0524841400000000 | 1.0 |
| H21 | H | 0.2903925900000000 | 0.9600834600000000 | 0.8632236600000000 | 1.0 |
| H22 | H | 0.1693051200000000 | 0.9149815700000000 | 0.9027625600000000 | 1.0 |

|     |   |                    |                    |                    |     |
|-----|---|--------------------|--------------------|--------------------|-----|
| H23 | H | 0.6693119200000000 | 0.1347528800000000 | 0.0837322900000000 | 1.0 |
| H24 | H | 0.7910963700000000 | 0.1539022500000000 | 0.0241077500000000 | 1.0 |
| C25 | C | 0.5648137200000000 | 0.9619595800000000 | 0.0285738200000000 | 1.0 |
| C26 | C | 0.5634011800000000 | 0.0399509700000000 | 0.0309186800000000 | 1.0 |
| C27 | C | 0.4761213700000000 | 0.0555009500000000 | 0.9666391500000000 | 1.0 |
| C28 | C | 0.4774074300000000 | 0.9456463300000000 | 0.9669363500000000 | 1.0 |
| C29 | C | 0.7274200600000000 | 0.0566202200000000 | 0.0289575000000000 | 1.0 |
| C30 | C | 0.8148151300000000 | 0.0403093700000000 | 0.9673151300000000 | 1.0 |
| C31 | C | 0.8133942500000000 | 0.9623171900000000 | 0.9649734600000000 | 1.0 |
| C32 | C | 0.7261175900000000 | 0.9467624900000000 | 0.0292446200000000 | 1.0 |
| C33 | C | 0.9774076600000000 | 0.9456456200000000 | 0.9669371500000000 | 1.0 |
| C34 | C | 0.0648145000000000 | 0.9619595500000000 | 0.0285741700000000 | 1.0 |
| C35 | C | 0.0634012400000000 | 0.0399509300000000 | 0.0309187000000000 | 1.0 |
| C36 | C | 0.9761209600000000 | 0.0555003900000000 | 0.9666391500000000 | 1.0 |
| C37 | C | 0.2274203300000000 | 0.0566205400000000 | 0.0289575700000000 | 1.0 |
| C38 | C | 0.3148153300000000 | 0.0403102300000000 | 0.9673151200000000 | 1.0 |
| C39 | C | 0.3133940500000000 | 0.9623184600000000 | 0.9649728500000000 | 1.0 |
| C40 | C | 0.2261189200000000 | 0.9467628400000000 | 0.0292442500000000 | 1.0 |
| N41 | N | 0.5069447400000000 | 0.8823998100000000 | 0.9378573700000000 | 1.0 |
| N42 | N | 0.5206403100000000 | 0.0721449800000000 | 0.0926951700000000 | 1.0 |
| N43 | N | 0.7569635000000000 | 0.1198568400000000 | 0.0580547300000000 | 1.0 |
| N44 | N | 0.7706268300000000 | 0.9301191600000000 | 0.9032005000000000 | 1.0 |
| N45 | N | 0.0069459500000000 | 0.8823989400000000 | 0.9378588100000000 | 1.0 |
| N46 | N | 0.0206399900000000 | 0.0721449500000000 | 0.0926951100000000 | 1.0 |
| N47 | N | 0.2569631300000000 | 0.1198570600000000 | 0.0580553600000000 | 1.0 |
| N48 | N | 0.2706261600000000 | 0.9301209400000000 | 0.9031995100000000 | 1.0 |
| O49 | O | 0.0205633800000000 | 0.0027010000000000 | 0.9224760900000000 | 1.0 |
| O50 | O | 0.7705683700000000 | 0.9995537000000000 | 0.0734126700000000 | 1.0 |
| O51 | O | 0.5205632400000000 | 0.0027017600000000 | 0.9224758500000000 | 1.0 |
| O52 | O | 0.2705690400000000 | 0.9995538700000000 | 0.0734123900000000 | 1.0 |

##### cif ends

furan\_NH2\_24\_anti\_alt\_forbid Energy: -323.37629868

##### cif starts

data\_furan\_NH2\_24\_anti\_alt\_forbid

\_publ\_section\_comment

;  
Andrew Reynoso, Bohan Xu, and Vincent H. Crespi  
;

\_cell\_length\_a 10.2759177608

\_cell\_length\_b 20.0

\_cell\_length\_c 20.0

\_cell\_angle\_alpha 90.0

\_cell\_angle\_beta 90.0

\_cell\_angle\_gamma 90.0

\_symmetry\_space\_group\_name\_H-M 'P 1'

\_symmetry\_Int\_Tables\_number 1

\_symmetry\_cell\_setting triclinic

loop\_

\_atom\_site\_label

|     | _atom_site_type_symbol | _atom_site_fract_x | _atom_site_fract_y | _atom_site_fract_z | _atom_site_occupancy |
|-----|------------------------|--------------------|--------------------|--------------------|----------------------|
| H1  | H                      | 0.0511872000000000 | 0.9005991400000000 | 0.9246000600000000 | 1.0                  |
| H2  | H                      | 0.9343574900000000 | 0.0589195400000000 | 0.0552616800000000 | 1.0                  |
| H3  | H                      | 0.2091052400000000 | 0.0930778000000000 | 0.0432062600000000 | 1.0                  |
| H4  | H                      | 0.3255763900000000 | 0.9346783900000000 | 0.9125438300000000 | 1.0                  |
| H5  | H                      | 0.5513773900000000 | 0.9005295000000000 | 0.9244075400000000 | 1.0                  |
| H6  | H                      | 0.4343478000000000 | 0.0587070000000000 | 0.0551903300000000 | 1.0                  |
| H7  | H                      | 0.7086220200000000 | 0.0930647800000000 | 0.0432583100000000 | 1.0                  |
| H8  | H                      | 0.8260052800000000 | 0.9349576000000000 | 0.9124774400000000 | 1.0                  |
| H9  | H                      | 0.8663049500000000 | 0.9382364600000000 | 0.0936103600000000 | 1.0                  |
| H10 | H                      | 0.0249519400000000 | 0.9383633600000000 | 0.0937869200000000 | 1.0                  |
| H11 | H                      | 0.3667061800000000 | 0.9379577700000000 | 0.0935707700000000 | 1.0                  |
| H12 | H                      | 0.5253367800000000 | 0.9380227800000000 | 0.0935876500000000 | 1.0                  |
| H13 | H                      | 0.7830130500000000 | 0.8575029600000000 | 0.0490189200000000 | 1.0                  |
| H14 | H                      | 0.6161354300000000 | 0.8536069900000000 | 0.0482496500000000 | 1.0                  |
| H15 | H                      | 0.2824935200000000 | 0.8574156700000000 | 0.0492633600000000 | 1.0                  |
| H16 | H                      | 0.1155861900000000 | 0.8538549700000000 | 0.0486199400000000 | 1.0                  |
| H17 | H                      | 0.1444517800000000 | 0.1399312000000000 | 0.9193457400000000 | 1.0                  |
| H18 | H                      | 0.9775440000000000 | 0.1362988300000000 | 0.9186892700000000 | 1.0                  |
| H19 | H                      | 0.6441256100000000 | 0.1399260400000000 | 0.9193216700000000 | 1.0                  |
| H20 | H                      | 0.4772504100000000 | 0.1360336700000000 | 0.9184710900000000 | 1.0                  |
| H21 | H                      | 0.2348915200000000 | 0.0553427300000000 | 0.8740544600000000 | 1.0                  |
| H22 | H                      | 0.3935329700000000 | 0.0552869400000000 | 0.8740660400000000 | 1.0                  |
| H23 | H                      | 0.7350632200000000 | 0.0556233800000000 | 0.8740732400000000 | 1.0                  |
| H24 | H                      | 0.8936963300000000 | 0.0557478200000000 | 0.8742100400000000 | 1.0                  |
| C25 | C                      | 0.0669869500000000 | 0.0593295500000000 | 0.9690069800000000 | 1.0                  |
| C26 | C                      | 0.9436736200000000 | 0.0366764300000000 | 0.0053122900000000 | 1.0                  |
| C27 | C                      | 0.9461865500000000 | 0.9581526400000000 | 0.0038192500000000 | 1.0                  |
| C28 | C                      | 0.0658817000000000 | 0.9438337000000000 | 0.9576882900000000 | 1.0                  |
| C29 | C                      | 0.1943019900000000 | 0.0498403300000000 | 0.0101345500000000 | 1.0                  |
| C30 | C                      | 0.3139281900000000 | 0.0354835100000000 | 0.9639440500000000 | 1.0                  |
| C31 | C                      | 0.3164167300000000 | 0.9569532500000000 | 0.9624871100000000 | 1.0                  |
| C32 | C                      | 0.1931478200000000 | 0.9343516300000000 | 0.9988588800000000 | 1.0                  |
| C33 | C                      | 0.5668885300000000 | 0.0592403800000000 | 0.9689220300000000 | 1.0                  |
| C34 | C                      | 0.4436700000000000 | 0.0364911300000000 | 0.0052311300000000 | 1.0                  |
| C35 | C                      | 0.4462512700000000 | 0.9579668800000000 | 0.0037169300000000 | 1.0                  |
| C36 | C                      | 0.5659645600000000 | 0.9437492800000000 | 0.9575303900000000 | 1.0                  |
| C37 | C                      | 0.6941412500000000 | 0.0498487400000000 | 0.0101197700000000 | 1.0                  |
| C38 | C                      | 0.8139366600000000 | 0.0356653300000000 | 0.9639966400000000 | 1.0                  |
| C39 | C                      | 0.8165307100000000 | 0.9571429200000000 | 0.9624424600000000 | 1.0                  |
| C40 | C                      | 0.6932715500000000 | 0.9343514100000000 | 0.9986869500000000 | 1.0                  |
| N41 | N                      | 0.0617775800000000 | 0.1244049500000000 | 0.9427043400000000 | 1.0                  |
| N42 | N                      | 0.9457837200000000 | 0.9219794800000000 | 0.0672850200000000 | 1.0                  |
| N43 | N                      | 0.3142312700000000 | 0.0716432000000000 | 0.9004711400000000 | 1.0                  |
| N44 | N                      | 0.1982822000000000 | 0.8692960900000000 | 0.0252213400000000 | 1.0                  |
| N45 | N                      | 0.5614447700000000 | 0.1243117500000000 | 0.9426162700000000 | 1.0                  |
| N46 | N                      | 0.4460509000000000 | 0.9217147900000000 | 0.0671341300000000 | 1.0                  |
| N47 | N                      | 0.8142512600000000 | 0.0719443000000000 | 0.9005955900000000 | 1.0                  |
| N48 | N                      | 0.6987684100000000 | 0.8692633400000000 | 0.0249414800000000 | 1.0                  |
| O49 | O                      | 0.0744536200000000 | 0.0029717900000000 | 0.9167254000000000 | 1.0                  |
| O50 | O                      | 0.1857228800000000 | 0.9907179500000000 | 0.0511090800000000 | 1.0                  |



O51 O 0.5744932700000000 0.0029188200000000 0.9166168800000000 1.0  
O52 O 0.6856129500000000 0.9906659700000000 0.0510189400000000 1.0

##### cif ends

furand\_NH2\_24\_anti\_dir Energy: -323.22730042

##### cif starts

data\_furand\_NH2\_24\_anti\_dir

\_publ\_section\_comment

;  
Andrew Reynoso, Bohan Xu, and Vincent H. Crespi  
;

\_cell\_length\_a 9.4494238838

\_cell\_length\_b 20.0

\_cell\_length\_c 20.0

\_cell\_angle\_alpha 90.0

\_cell\_angle\_beta 90.0

\_cell\_angle\_gamma 90.0

\_symmetry\_space\_group\_name\_H-M 'P 1'

\_symmetry\_Int\_Tables\_number 1

\_symmetry\_cell\_setting triclinic

loop\_

\_atom\_site\_label

\_atom\_site\_type\_symbol

\_atom\_site\_fract\_x

\_atom\_site\_fract\_y

\_atom\_site\_fract\_z

\_atom\_site\_occupancy

|     |   |                    |                    |                    |     |
|-----|---|--------------------|--------------------|--------------------|-----|
| H1  | H | 0.4816966100000000 | 0.0541442100000000 | 0.0716825300000000 | 1.0 |
| H2  | H | 0.4988516900000000 | 0.8867843500000000 | 0.9470012700000000 | 1.0 |
| H3  | H | 0.5709168200000000 | 0.9471836000000000 | 0.1105232700000000 | 1.0 |
| H4  | H | 0.4097294200000000 | 0.9215460000000000 | 0.1268300000000000 | 1.0 |
| H5  | H | 0.5418434500000000 | 0.1178128300000000 | 0.8894730900000000 | 1.0 |
| H6  | H | 0.3967878100000000 | 0.1267095200000000 | 0.9380743900000000 | 1.0 |
| H7  | H | 0.7316672400000000 | 0.0479374300000000 | 0.9183514600000000 | 1.0 |
| H8  | H | 0.7487977100000000 | 0.8911696200000000 | 0.0560815100000000 | 1.0 |
| H9  | H | 0.8210876400000000 | 0.9381001800000000 | 0.8883561200000000 | 1.0 |
| H10 | H | 0.6596856400000000 | 0.9116667900000000 | 0.8739813600000000 | 1.0 |
| H11 | H | 0.1467901900000000 | 0.1310475800000000 | 0.0457667100000000 | 1.0 |
| H12 | H | 0.2919678000000000 | 0.1260854400000000 | 0.0948574900000000 | 1.0 |
| H13 | H | 0.9816928600000000 | 0.0541450800000000 | 0.0716838300000000 | 1.0 |
| H14 | H | 0.9988500600000000 | 0.8867862300000000 | 0.9470009700000000 | 1.0 |
| H15 | H | 0.0709176000000000 | 0.9471851100000000 | 0.1105236600000000 | 1.0 |
| H16 | H | 0.9097292300000000 | 0.9215485500000000 | 0.1268311600000000 | 1.0 |
| H17 | H | 0.0418430600000000 | 0.1178161200000000 | 0.8894759000000000 | 1.0 |
| H18 | H | 0.8967881900000000 | 0.1267122300000000 | 0.9380782900000000 | 1.0 |
| H19 | H | 0.2316648600000000 | 0.0479391500000000 | 0.9183525000000000 | 1.0 |
| H20 | H | 0.2487979400000000 | 0.8911685300000000 | 0.0560794900000000 | 1.0 |
| H21 | H | 0.3210862900000000 | 0.9381014700000000 | 0.8883554400000000 | 1.0 |
| H22 | H | 0.1596822700000000 | 0.9116714300000000 | 0.8739796400000000 | 1.0 |
| H23 | H | 0.7919581700000000 | 0.1260891800000000 | 0.0948545700000000 | 1.0 |

|     |   |                    |                    |                    |     |
|-----|---|--------------------|--------------------|--------------------|-----|
| H24 | H | 0.6467853000000000 | 0.1310485100000000 | 0.0457601100000000 | 1.0 |
| C25 | C | 0.4358882800000000 | 0.0317653700000000 | 0.0264432900000000 | 1.0 |
| C26 | C | 0.4360885400000000 | 0.9532682600000000 | 0.0308345700000000 | 1.0 |
| C27 | C | 0.5223217600000000 | 0.9363096000000000 | 0.9675926700000000 | 1.0 |
| C28 | C | 0.5239015700000000 | 0.0468180300000000 | 0.9629744800000000 | 1.0 |
| C29 | C | 0.7738890300000000 | 0.0493995800000000 | 0.0273238800000000 | 1.0 |
| C30 | C | 0.6858802500000000 | 0.0293001900000000 | 0.9652609700000000 | 1.0 |
| C31 | C | 0.6860617700000000 | 0.9507036300000000 | 0.9671982900000000 | 1.0 |
| C32 | C | 0.7723411600000000 | 0.9388815400000000 | 0.0315985300000000 | 1.0 |
| C33 | C | 0.0239008100000000 | 0.0468196100000000 | 0.9629760400000000 | 1.0 |
| C34 | C | 0.9358869000000000 | 0.0317665500000000 | 0.0264445500000000 | 1.0 |
| C35 | C | 0.9360878900000000 | 0.9532692900000000 | 0.0308353400000000 | 1.0 |
| C36 | C | 0.0223207100000000 | 0.9363110500000000 | 0.9675930600000000 | 1.0 |
| C37 | C | 0.2738910700000000 | 0.0493990100000000 | 0.0273247600000000 | 1.0 |
| C38 | C | 0.1858796400000000 | 0.0293013800000000 | 0.9652618200000000 | 1.0 |
| C39 | C | 0.1860608300000000 | 0.9507046700000000 | 0.9671977800000000 | 1.0 |
| C40 | C | 0.2723415400000000 | 0.9388809500000000 | 0.0315974300000000 | 1.0 |
| N41 | N | 0.4989513300000000 | 0.1108505700000000 | 0.9356114700000000 | 1.0 |
| N42 | N | 0.4877934400000000 | 0.9207002600000000 | 0.0915870200000000 | 1.0 |
| N43 | N | 0.7489491200000000 | 0.1154251400000000 | 0.0494525100000000 | 1.0 |
| N44 | N | 0.7376633000000000 | 0.9133477300000000 | 0.9092446200000000 | 1.0 |
| N45 | N | 0.9989511600000000 | 0.1108527800000000 | 0.9356141700000000 | 1.0 |
| N46 | N | 0.9877930600000000 | 0.9207018100000000 | 0.0915877400000000 | 1.0 |
| N47 | N | 0.2489544000000000 | 0.1154241500000000 | 0.0494557300000000 | 1.0 |
| N48 | N | 0.2376597600000000 | 0.9133499500000000 | 0.9092430900000000 | 1.0 |
| O49 | O | 0.9780463300000000 | 0.9883725400000000 | 0.9208751800000000 | 1.0 |
| O50 | O | 0.7280640000000000 | 0.9945213900000000 | 0.0739776100000000 | 1.0 |
| O51 | O | 0.4780475200000000 | 0.9883704900000000 | 0.9208741600000000 | 1.0 |
| O52 | O | 0.2280659500000000 | 0.9945203400000000 | 0.0739775100000000 | 1.0 |

##### cif ends

uran\_NH2\_24\_anti\_dir\_forbid Energy: -322.30084891

##### cif starts

data\_uran\_NH2\_24\_anti\_dir\_forbid

\_publ\_section\_comment

;  
Andrew Reynoso, Bohan Xu, and Vincent H. Crespi  
;

\_cell\_length\_a 10.245148985

\_cell\_length\_b 20.0

\_cell\_length\_c 20.0

\_cell\_angle\_alpha 90.0

\_cell\_angle\_beta 90.0

\_cell\_angle\_gamma 90.0

\_symmetry\_space\_group\_name\_H-M 'P 1'

\_symmetry\_Int\_Tables\_number 1

\_symmetry\_cell\_setting triclinic

loop\_

\_atom\_site\_label

\_atom\_site\_type\_symbol

|     |   | _atom_site_fract_x | _atom_site_fract_y | _atom_site_fract_z | _atom_site_occupancy |
|-----|---|--------------------|--------------------|--------------------|----------------------|
| H1  | H | 0.8887495500000000 | 0.0592330900000000 | 0.0682338800000000 | 1.0                  |
| H2  | H | 0.0082720200000000 | 0.8959904100000000 | 0.9457604200000000 | 1.0                  |
| H3  | H | 0.9580820700000000 | 0.9417483900000000 | 0.1151932400000000 | 1.0                  |
| H4  | H | 0.9065805300000000 | 0.8728277000000000 | 0.0791304000000000 | 1.0                  |
| H5  | H | 0.0760725400000000 | 0.1190159300000000 | 0.9046207200000000 | 1.0                  |
| H6  | H | 0.9876395400000000 | 0.1540303800000000 | 0.9643253100000000 | 1.0                  |
| H7  | H | 0.7714839300000000 | 0.0595349500000000 | 0.9300411300000000 | 1.0                  |
| H8  | H | 0.6519607700000000 | 0.8957548700000000 | 0.0517959900000000 | 1.0                  |
| H9  | H | 0.7021374800000000 | 0.9422783200000000 | 0.8825651800000000 | 1.0                  |
| H10 | H | 0.7536604500000000 | 0.8731926500000000 | 0.9183052100000000 | 1.0                  |
| H11 | H | 0.5842030100000000 | 0.1185524900000000 | 0.0939615800000000 | 1.0                  |
| H12 | H | 0.6723580600000000 | 0.1538846200000000 | 0.0343509900000000 | 1.0                  |
| H13 | H | 0.0842522700000000 | 0.1184878700000000 | 0.0940204400000000 | 1.0                  |
| H14 | H | 0.3887383500000000 | 0.0592364000000000 | 0.0682337800000000 | 1.0                  |
| H15 | H | 0.5082740600000000 | 0.8959957900000000 | 0.9457598900000000 | 1.0                  |
| H16 | H | 0.4580788700000000 | 0.9417603800000000 | 0.1151937400000000 | 1.0                  |
| H17 | H | 0.4065761500000000 | 0.8728365100000000 | 0.0791381600000000 | 1.0                  |
| H18 | H | 0.5762223200000000 | 0.1191476300000000 | 0.9047664600000000 | 1.0                  |
| H19 | H | 0.4872922400000000 | 0.1540090500000000 | 0.9643666600000000 | 1.0                  |
| H20 | H | 0.2714853400000000 | 0.0595346300000000 | 0.9300354600000000 | 1.0                  |
| H21 | H | 0.1519696900000000 | 0.8957584100000000 | 0.0517955500000000 | 1.0                  |
| H22 | H | 0.2021396700000000 | 0.9422682300000000 | 0.8825636600000000 | 1.0                  |
| H23 | H | 0.2536956900000000 | 0.8731901200000000 | 0.9183074600000000 | 1.0                  |
| H24 | H | 0.1721645000000000 | 0.1539026800000000 | 0.0343630900000000 | 1.0                  |
| C25 | C | 0.0158470100000000 | 0.0537652200000000 | 0.9768954400000000 | 1.0                  |
| C26 | C | 0.8947642900000000 | 0.0349213200000000 | 0.0191551900000000 | 1.0                  |
| C27 | C | 0.8959920000000000 | 0.9563295500000000 | 0.0197244900000000 | 1.0                  |
| C28 | C | 0.0181220600000000 | 0.9409605300000000 | 0.9768636600000000 | 1.0                  |
| C29 | C | 0.6443814600000000 | 0.0536658800000000 | 0.0213610500000000 | 1.0                  |
| C30 | C | 0.7654660600000000 | 0.0350111400000000 | 0.9790147400000000 | 1.0                  |
| C31 | C | 0.7642497400000000 | 0.9564225500000000 | 0.9780947800000000 | 1.0                  |
| C32 | C | 0.6421216400000000 | 0.9408616000000000 | 0.0208916100000000 | 1.0                  |
| C33 | C | 0.5158515100000000 | 0.0537711800000000 | 0.9769033200000000 | 1.0                  |
| C34 | C | 0.3947632400000000 | 0.0349249700000000 | 0.0191547300000000 | 1.0                  |
| C35 | C | 0.3959922600000000 | 0.9563341200000000 | 0.0197245900000000 | 1.0                  |
| C36 | C | 0.5181242800000000 | 0.9409650200000000 | 0.9768645300000000 | 1.0                  |
| C37 | C | 0.1443778000000000 | 0.0536664200000000 | 0.0213537600000000 | 1.0                  |
| C38 | C | 0.2654678800000000 | 0.0350138100000000 | 0.9790099800000000 | 1.0                  |
| C39 | C | 0.2642533900000000 | 0.9564243200000000 | 0.9780925200000000 | 1.0                  |
| C40 | C | 0.1421240700000000 | 0.9408625800000000 | 0.0208883600000000 | 1.0                  |
| N41 | N | 0.9975511000000000 | 0.1123192800000000 | 0.9354268000000000 | 1.0                  |
| N42 | N | 0.8880509500000000 | 0.9227954500000000 | 0.0841526300000000 | 1.0                  |
| N43 | N | 0.6626792900000000 | 0.1120425800000000 | 0.0630837200000000 | 1.0                  |
| N44 | N | 0.7721780200000000 | 0.9231841000000000 | 0.9135139100000000 | 1.0                  |
| N45 | N | 0.4975571000000000 | 0.1123332500000000 | 0.9354502300000000 | 1.0                  |
| N46 | N | 0.3880472000000000 | 0.9228047800000000 | 0.0841551500000000 | 1.0                  |
| N47 | N | 0.1626589600000000 | 0.1120414700000000 | 0.0630831000000000 | 1.0                  |
| N48 | N | 0.2721879500000000 | 0.9231837300000000 | 0.9135134500000000 | 1.0                  |
| O49 | O | 0.0271671100000000 | 0.9974562400000000 | 0.9317580900000000 | 1.0                  |
| O50 | O | 0.6330753000000000 | 0.9971588400000000 | 0.0662481900000000 | 1.0                  |
| O51 | O | 0.5271742800000000 | 0.9974626800000000 | 0.9317620600000000 | 1.0                  |

O52 O 0.1330741200000000 0.9971621700000000 0.0662426100000000 1.0

##### cif ends

furan\_NH2\_24\_syn\_alt Energy: -322.77725163

##### cif starts

data\_furan\_NH2\_24\_syn\_alt

\_publ\_section\_comment

;  
Andrew Reynoso, Bohan Xu, and Vincent H. Crespi  
;

\_cell\_length\_a 10.3705796023

\_cell\_length\_b 20.0

\_cell\_length\_c 20.0

\_cell\_angle\_alpha 90.0

\_cell\_angle\_beta 90.0

\_cell\_angle\_gamma 90.0

\_symmetry\_space\_group\_name\_H-M 'P 1'

\_symmetry\_Int\_Tables\_number 1

\_symmetry\_cell\_setting triclinic

loop\_

\_atom\_site\_label

\_atom\_site\_type\_symbol

\_atom\_site\_fract\_x

\_atom\_site\_fract\_y

\_atom\_site\_fract\_z

\_atom\_site\_occupancy

|     |   |                    |                    |                    |     |
|-----|---|--------------------|--------------------|--------------------|-----|
| H1  | H | 0.6476186800000000 | 0.9347003900000000 | 0.9333561700000000 | 1.0 |
| H2  | H | 0.5230943900000000 | 0.1032259300000000 | 0.0427665000000000 | 1.0 |
| H3  | H | 0.7220812900000000 | 0.0491521200000000 | 0.8832296300000000 | 1.0 |
| H4  | H | 0.6570721600000000 | 0.1167876300000000 | 0.9145444400000000 | 1.0 |
| H5  | H | 0.4493662200000000 | 0.8747681100000000 | 0.0862469700000000 | 1.0 |
| H6  | H | 0.6064524900000000 | 0.8813936800000000 | 0.0929435200000000 | 1.0 |
| H7  | H | 0.8974003000000000 | 0.0585865900000000 | 0.9294451500000000 | 1.0 |
| H8  | H | 0.7787105500000000 | 0.8957082300000000 | 0.0460390600000000 | 1.0 |
| H9  | H | 0.9639640400000000 | 0.9498963900000000 | 0.8847540000000000 | 1.0 |
| H10 | H | 0.8290636400000000 | 0.9094164900000000 | 0.9013751700000000 | 1.0 |
| H11 | H | 0.2770123200000000 | 0.1581950200000000 | 0.0142185500000000 | 1.0 |
| H12 | H | 0.2137270000000000 | 0.1267331600000000 | 0.0836128800000000 | 1.0 |
| H13 | H | 0.1453761000000000 | 0.9287224200000000 | 0.9415983700000000 | 1.0 |
| H14 | H | 0.0320457400000000 | 0.1079096400000000 | 0.0358730700000000 | 1.0 |
| H15 | H | 0.2286221300000000 | 0.0481019900000000 | 0.8824175500000000 | 1.0 |
| H16 | H | 0.1287196400000000 | 0.1078007200000000 | 0.9039521200000000 | 1.0 |
| H17 | H | 0.9462222100000000 | 0.8902154100000000 | 0.1008663200000000 | 1.0 |
| H18 | H | 0.1037372600000000 | 0.8845835500000000 | 0.0977770600000000 | 1.0 |
| H19 | H | 0.4087704800000000 | 0.0558229900000000 | 0.9275270200000000 | 1.0 |
| H20 | H | 0.2789631900000000 | 0.9027985100000000 | 0.0581046800000000 | 1.0 |
| H21 | H | 0.4680992600000000 | 0.9318620500000000 | 0.8901501800000000 | 1.0 |
| H22 | H | 0.3122238500000000 | 0.9209206500000000 | 0.8990027700000000 | 1.0 |
| H23 | H | 0.8557528000000000 | 0.1246380800000000 | 0.0820448400000000 | 1.0 |
| H24 | H | 0.6976196600000000 | 0.1222343500000000 | 0.0837241300000000 | 1.0 |

|     |   |                    |                    |                    |     |
|-----|---|--------------------|--------------------|--------------------|-----|
| C25 | C | 0.6522832200000000 | 0.9595114100000000 | 0.9822648800000000 | 1.0 |
| C26 | C | 0.6525037600000000 | 0.0375439800000000 | 0.9790265500000000 | 1.0 |
| C27 | C | 0.5269600400000000 | 0.0535924700000000 | 0.0195534400000000 | 1.0 |
| C28 | C | 0.5286899800000000 | 0.9451420300000000 | 0.0257660400000000 | 1.0 |
| C29 | C | 0.7781004200000000 | 0.0536568100000000 | 0.0223075900000000 | 1.0 |
| C30 | C | 0.9015799000000000 | 0.0382647200000000 | 0.9802685500000000 | 1.0 |
| C31 | C | 0.9046807600000000 | 0.9597437900000000 | 0.9825735700000000 | 1.0 |
| C32 | C | 0.7779270300000000 | 0.9450056800000000 | 0.0219199600000000 | 1.0 |
| C33 | C | 0.0273524200000000 | 0.9486035700000000 | 0.0302397300000000 | 1.0 |
| C34 | C | 0.1517032700000000 | 0.9584399400000000 | 0.9875033400000000 | 1.0 |
| C35 | C | 0.1517818500000000 | 0.0359874300000000 | 0.9768104500000000 | 1.0 |
| C36 | C | 0.0278713900000000 | 0.0562888800000000 | 0.0169538900000000 | 1.0 |
| C37 | C | 0.2794727300000000 | 0.0560434900000000 | 0.0185036000000000 | 1.0 |
| C38 | C | 0.4037296500000000 | 0.0369923000000000 | 0.9789564600000000 | 1.0 |
| C39 | C | 0.4014782900000000 | 0.9580003300000000 | 0.9834119200000000 | 1.0 |
| C40 | C | 0.2775733300000000 | 0.9484517000000000 | 0.0277003000000000 | 1.0 |
| N41 | N | 0.5318206500000000 | 0.8828776000000000 | 0.0598161400000000 | 1.0 |
| N42 | N | 0.6473119800000000 | 0.0659377200000000 | 0.9118310600000000 | 1.0 |
| N43 | N | 0.7758658200000000 | 0.1176394000000000 | 0.0531373700000000 | 1.0 |
| N44 | N | 0.9165095100000000 | 0.9227583100000000 | 0.9202558900000000 | 1.0 |
| N45 | N | 0.0230632500000000 | 0.8893578800000000 | 0.0690572600000000 | 1.0 |
| N46 | N | 0.1442997800000000 | 0.0573973200000000 | 0.9070968600000000 | 1.0 |
| N47 | N | 0.2854100900000000 | 0.1212183200000000 | 0.0491038500000000 | 1.0 |
| N48 | N | 0.3984576500000000 | 0.9175818400000000 | 0.9231548700000000 | 1.0 |
| O49 | O | 0.0281243100000000 | 0.0098837800000000 | 0.0709282900000000 | 1.0 |
| O50 | O | 0.7781340000000000 | 0.9976595400000000 | 0.0701599300000000 | 1.0 |
| O51 | O | 0.5281091000000000 | 0.0030863100000000 | 0.0700759600000000 | 1.0 |
| O52 | O | 0.2791994100000000 | 0.0061093200000000 | 0.0702961000000000 | 1.0 |

##### cif ends

furand\_NH2\_24\_syn\_alt\_forbid Energy: -319.89431337

##### cif starts

data\_furand\_NH2\_24\_syn\_alt\_forbid

\_publ\_section\_comment

;

Andrew Reynoso, Bohan Xu, and Vincent H. Crespi

;

\_cell\_length\_a 9.6625551199

\_cell\_length\_b 20.0

\_cell\_length\_c 20.0

\_cell\_angle\_alpha 90.0

\_cell\_angle\_beta 90.0

\_cell\_angle\_gamma 90.0

\_symmetry\_space\_group\_name\_H-M 'P 1'

\_symmetry\_Int\_Tables\_number 1

\_symmetry\_cell\_setting triclinic

loop\_

\_atom\_site\_label

\_atom\_site\_type\_symbol

\_atom\_site\_fract\_x

|     |   | _atom_site_fract_y |                    | _atom_site_fract_z |     | _atom_site_occupancy |  |
|-----|---|--------------------|--------------------|--------------------|-----|----------------------|--|
| H1  | H | 0.9023647100000000 | 0.0601242000000000 | 0.9107076000000000 | 1.0 |                      |  |
| H2  | H | 0.8789280200000000 | 0.8936457000000000 | 0.0403782700000000 | 1.0 |                      |  |
| H3  | H | 0.1602195300000000 | 0.1028757800000000 | 0.0283649500000000 | 1.0 |                      |  |
| H4  | H | 0.1370211700000000 | 0.9199794100000000 | 0.9207816400000000 | 1.0 |                      |  |
| H5  | H | 0.4023641700000000 | 0.0601189200000000 | 0.9107056200000000 | 1.0 |                      |  |
| H6  | H | 0.3789219100000000 | 0.8936459700000000 | 0.0403826000000000 | 1.0 |                      |  |
| H7  | H | 0.6602130100000000 | 0.1028717900000000 | 0.0283670900000000 | 1.0 |                      |  |
| H8  | H | 0.6370200500000000 | 0.9199774100000000 | 0.9207804400000000 | 1.0 |                      |  |
| H9  | H | 0.8785563500000000 | 0.8809211200000000 | 0.8893592300000000 | 1.0 |                      |  |
| H10 | H | 0.8790336700000000 | 0.1528183100000000 | 0.0329002700000000 | 1.0 |                      |  |
| H11 | H | 0.3785519400000000 | 0.8809160200000000 | 0.8893621400000000 | 1.0 |                      |  |
| H12 | H | 0.8076188800000000 | 0.9549051000000000 | 0.8714926200000000 | 1.0 |                      |  |
| H13 | H | 0.8711893700000000 | 0.1093590600000000 | 0.1023114000000000 | 1.0 |                      |  |
| H14 | H | 0.3788969200000000 | 0.1528170200000000 | 0.0329547000000000 | 1.0 |                      |  |
| H15 | H | 0.3713210300000000 | 0.1093079000000000 | 0.1023400700000000 | 1.0 |                      |  |
| H16 | H | 0.3076218500000000 | 0.9549009000000000 | 0.8714918700000000 | 1.0 |                      |  |
| H17 | H | 0.1640259100000000 | 0.0995484000000000 | 0.8794696100000000 | 1.0 |                      |  |
| H18 | H | 0.0970043000000000 | 0.0311430400000000 | 0.8483130300000000 | 1.0 |                      |  |
| H19 | H | 0.6640529100000000 | 0.0995539400000000 | 0.8794844100000000 | 1.0 |                      |  |
| H20 | H | 0.5970057500000000 | 0.0311611100000000 | 0.8483129700000000 | 1.0 |                      |  |
| H21 | H | 0.0467562400000000 | 0.8960132800000000 | 0.0885378200000000 | 1.0 |                      |  |
| H22 | H | 0.2096033500000000 | 0.8833756600000000 | 0.1063862200000000 | 1.0 |                      |  |
| H23 | H | 0.5467642800000000 | 0.8960043100000000 | 0.0885359600000000 | 1.0 |                      |  |
| H24 | H | 0.7096145000000000 | 0.8833614500000000 | 0.1063774900000000 | 1.0 |                      |  |
| C25 | C | 0.8658639500000000 | 0.0523682900000000 | 0.0189503000000000 | 1.0 |                      |  |
| C26 | C | 0.9457074100000000 | 0.0353697300000000 | 0.9548785100000000 | 1.0 |                      |  |
| C27 | C | 0.9324470500000000 | 0.9574175700000000 | 0.9539137000000000 | 1.0 |                      |  |
| C28 | C | 0.8463916000000000 | 0.9416038300000000 | 0.0186748800000000 | 1.0 |                      |  |
| C29 | C | 0.1957262700000000 | 0.0534283700000000 | 0.0118233900000000 | 1.0 |                      |  |
| C30 | C | 0.1106015000000000 | 0.0291712400000000 | 0.9497662400000000 | 1.0 |                      |  |
| C31 | C | 0.0972878000000000 | 0.9520471100000000 | 0.9607480500000000 | 1.0 |                      |  |
| C32 | C | 0.1787836700000000 | 0.9431326400000000 | 0.0262505000000000 | 1.0 |                      |  |
| C33 | C | 0.3658657200000000 | 0.0523680800000000 | 0.0189488800000000 | 1.0 |                      |  |
| C34 | C | 0.4457078100000000 | 0.0353662100000000 | 0.9548772900000000 | 1.0 |                      |  |
| C35 | C | 0.4324471700000000 | 0.9574144000000000 | 0.9539144900000000 | 1.0 |                      |  |
| C36 | C | 0.3463899100000000 | 0.9416033700000000 | 0.0186761700000000 | 1.0 |                      |  |
| C37 | C | 0.6957233600000000 | 0.0534253900000000 | 0.0118254700000000 | 1.0 |                      |  |
| C38 | C | 0.6106009800000000 | 0.0291698400000000 | 0.9497670300000000 | 1.0 |                      |  |
| C39 | C | 0.5972897200000000 | 0.9520450400000000 | 0.9607471200000000 | 1.0 |                      |  |
| C40 | C | 0.6787866700000000 | 0.9431291500000000 | 0.0262489500000000 | 1.0 |                      |  |
| N41 | N | 0.9147054300000000 | 0.1104422400000000 | 0.0556434000000000 | 1.0 |                      |  |
| N42 | N | 0.8945555500000000 | 0.9313716200000000 | 0.8885755900000000 | 1.0 |                      |  |
| N43 | N | 0.1637153000000000 | 0.0485621400000000 | 0.8840892400000000 | 1.0 |                      |  |
| N44 | N | 0.1413151600000000 | 0.8872972200000000 | 0.0675458000000000 | 1.0 |                      |  |
| N45 | N | 0.4147097000000000 | 0.1104408900000000 | 0.0556456900000000 | 1.0 |                      |  |
| N46 | N | 0.3945545300000000 | 0.9313662800000000 | 0.8885775100000000 | 1.0 |                      |  |
| N47 | N | 0.6637216200000000 | 0.0485669400000000 | 0.8840932600000000 | 1.0 |                      |  |
| N48 | N | 0.6413205600000000 | 0.8872901900000000 | 0.0675401400000000 | 1.0 |                      |  |
| O49 | O | 0.8908470500000000 | 0.9948491800000000 | 0.0609983800000000 | 1.0 |                      |  |
| O50 | O | 0.1533441500000000 | 0.0062503400000000 | 0.0606407000000000 | 1.0 |                      |  |
| O51 | O | 0.3908459800000000 | 0.9948500300000000 | 0.0609976700000000 | 1.0 |                      |  |
| O52 | O | 0.6533424300000000 | 0.0062453300000000 | 0.0606416600000000 | 1.0 |                      |  |

##### cif ends

uran\_NH2\_24\_syn\_dir Energy: -321.71968443

##### cif starts

data\_uran\_NH2\_24\_syn\_dir

\_publ\_section\_comment

;  
Andrew Reynoso, Bohan Xu, and Vincent H. Crespi  
;

\_cell\_length\_a 10.626025915

\_cell\_length\_b 20.0

\_cell\_length\_c 20.0

\_cell\_angle\_alpha 90.0

\_cell\_angle\_beta 90.0

\_cell\_angle\_gamma 90.0

\_symmetry\_space\_group\_name\_H-M 'P 1'

\_symmetry\_Int\_Tables\_number 1

\_symmetry\_cell\_setting triclinic

loop\_

\_atom\_site\_label

\_atom\_site\_type\_symbol

\_atom\_site\_fract\_x

\_atom\_site\_fract\_y

\_atom\_site\_fract\_z

\_atom\_site\_occupancy

|     |   |                    |                    |                    |     |
|-----|---|--------------------|--------------------|--------------------|-----|
| H1  | H | 0.5224020800000000 | 0.0543676800000000 | 0.9289762000000000 | 1.0 |
| H2  | H | 0.3985230900000000 | 0.8960303500000000 | 0.0528139700000000 | 1.0 |
| H3  | H | 0.4393316000000000 | 0.9300463000000000 | 0.8950195100000000 | 1.0 |
| H4  | H | 0.5344338200000000 | 0.8724501600000000 | 0.9233177800000000 | 1.0 |
| H5  | H | 0.4122706700000000 | 0.1105767400000000 | 0.1013217300000000 | 1.0 |
| H6  | H | 0.3075957000000000 | 0.1369857300000000 | 0.0460825100000000 | 1.0 |
| H7  | H | 0.7724144000000000 | 0.0543694900000000 | 0.9289863400000000 | 1.0 |
| H8  | H | 0.6485135800000000 | 0.8960261100000000 | 0.0528079600000000 | 1.0 |
| H9  | H | 0.6893318400000000 | 0.9300548700000000 | 0.8950206300000000 | 1.0 |
| H10 | H | 0.7844326400000000 | 0.8724547100000000 | 0.9233138900000000 | 1.0 |
| H11 | H | 0.0575927200000000 | 0.1369727300000000 | 0.0461176900000000 | 1.0 |
| H12 | H | 0.1622964600000000 | 0.1105524300000000 | 0.1013399800000000 | 1.0 |
| H13 | H | 0.0223906100000000 | 0.0543756800000000 | 0.9289875600000000 | 1.0 |
| H14 | H | 0.8985228100000000 | 0.8960186200000000 | 0.0528013100000000 | 1.0 |
| H15 | H | 0.9393331300000000 | 0.9300611600000000 | 0.8950130300000000 | 1.0 |
| H16 | H | 0.0344213700000000 | 0.8724577200000000 | 0.9233060600000000 | 1.0 |
| H17 | H | 0.9122519400000000 | 0.1105455200000000 | 0.1013550000000000 | 1.0 |
| H18 | H | 0.8076028900000000 | 0.1369774100000000 | 0.0461110300000000 | 1.0 |
| H19 | H | 0.2723887100000000 | 0.0543637900000000 | 0.9289797000000000 | 1.0 |
| H20 | H | 0.1485107000000000 | 0.8960196000000000 | 0.0528009600000000 | 1.0 |
| H21 | H | 0.1893391600000000 | 0.9300464400000000 | 0.8950208400000000 | 1.0 |
| H22 | H | 0.2844350000000000 | 0.8724463700000000 | 0.9233226100000000 | 1.0 |
| H23 | H | 0.6622356600000000 | 0.1105603500000000 | 0.1013360600000000 | 1.0 |
| H24 | H | 0.5576050300000000 | 0.1369897100000000 | 0.0460821400000000 | 1.0 |
| C25 | C | 0.5231183600000000 | 0.0339949700000000 | 0.9799569400000000 | 1.0 |

|     |   |                    |                    |                    |     |
|-----|---|--------------------|--------------------|--------------------|-----|
| C26 | C | 0.5238293600000000 | 0.9557131600000000 | 0.9821143400000000 | 1.0 |
| C27 | C | 0.3982259400000000 | 0.9432960100000000 | 0.0246163300000000 | 1.0 |
| C28 | C | 0.3975023700000000 | 0.0514934000000000 | 0.0203073800000000 | 1.0 |
| C29 | C | 0.6474965400000000 | 0.0514910700000000 | 0.0203111800000000 | 1.0 |
| C30 | C | 0.7731252900000000 | 0.0339926200000000 | 0.9799655200000000 | 1.0 |
| C31 | C | 0.7738333600000000 | 0.9557126900000000 | 0.9821171100000000 | 1.0 |
| C32 | C | 0.6482220700000000 | 0.9432940500000000 | 0.0246140100000000 | 1.0 |
| C33 | C | 0.8975027400000000 | 0.0514871600000000 | 0.0203227600000000 | 1.0 |
| C34 | C | 0.0231152400000000 | 0.0339959300000000 | 0.9799655600000000 | 1.0 |
| C35 | C | 0.0238285700000000 | 0.9557136900000000 | 0.9821123000000000 | 1.0 |
| C36 | C | 0.8982260800000000 | 0.9432894700000000 | 0.0246123200000000 | 1.0 |
| C37 | C | 0.1474967700000000 | 0.0514876100000000 | 0.0203158200000000 | 1.0 |
| C38 | C | 0.2731191500000000 | 0.0339902600000000 | 0.9799602100000000 | 1.0 |
| C39 | C | 0.2738328800000000 | 0.9557103800000000 | 0.9821173600000000 | 1.0 |
| C40 | C | 0.1482213300000000 | 0.9432901300000000 | 0.0246113200000000 | 1.0 |
| N41 | N | 0.3964732500000000 | 0.1166448000000000 | 0.0512815300000000 | 1.0 |
| N42 | N | 0.5271748700000000 | 0.9231114100000000 | 0.9165352700000000 | 1.0 |
| N43 | N | 0.6464691500000000 | 0.1166386600000000 | 0.0512934200000000 | 1.0 |
| N44 | N | 0.7771740800000000 | 0.9231163800000000 | 0.9165359800000000 | 1.0 |
| N45 | N | 0.8964741100000000 | 0.1166301000000000 | 0.0513149200000000 | 1.0 |
| N46 | N | 0.0271744000000000 | 0.9231203000000000 | 0.9165288100000000 | 1.0 |
| N47 | N | 0.1464712400000000 | 0.1166315200000000 | 0.0513027300000000 | 1.0 |
| N48 | N | 0.2771782500000000 | 0.9231074100000000 | 0.9165393800000000 | 1.0 |
| O49 | O | 0.8973240800000000 | 0.9983094200000000 | 0.0699246900000000 | 1.0 |
| O50 | O | 0.6473032900000000 | 0.9983197400000000 | 0.0699199700000000 | 1.0 |
| O51 | O | 0.3973231500000000 | 0.9983239300000000 | 0.0699194000000000 | 1.0 |
| O52 | O | 0.1473054700000000 | 0.9983120400000000 | 0.0699209600000000 | 1.0 |

##### cif ends

uran\_NH2\_24\_syn\_dir\_forbid Energy: -318.94616279

##### cif starts

data\_uran\_NH2\_24\_syn\_dir\_forbid

\_publ\_section\_comment

;  
Andrew Reynoso, Bohan Xu, and Vincent H. Crespi  
;

\_cell\_length\_a 9.7342496342

\_cell\_length\_b 20.0

\_cell\_length\_c 20.0

\_cell\_angle\_alpha 90.0

\_cell\_angle\_beta 90.0

\_cell\_angle\_gamma 90.0

\_symmetry\_space\_group\_name\_H-M 'P 1'

\_symmetry\_Int\_Tables\_number 1

\_symmetry\_cell\_setting triclinic

loop\_

\_atom\_site\_label

\_atom\_site\_type\_symbol

\_atom\_site\_fract\_x

\_atom\_site\_fract\_y



|     |   | _atom_site_fract_z |                      |                    |     |  |
|-----|---|--------------------|----------------------|--------------------|-----|--|
|     |   |                    | _atom_site_occupancy |                    |     |  |
| H1  | H | 0.9014511900000000 | 0.0428619000000000   | 0.9054802900000000 | 1.0 |  |
| H2  | H | 0.9095702300000000 | 0.9071969100000000   | 0.0691154100000000 | 1.0 |  |
| H3  | H | 0.1430305400000000 | 0.0669187700000000   | 0.9242291200000000 | 1.0 |  |
| H4  | H | 0.1812070100000000 | 0.8887262100000000   | 0.0382694600000000 | 1.0 |  |
| H5  | H | 0.4025292700000000 | 0.0427079300000000   | 0.9049755900000000 | 1.0 |  |
| H6  | H | 0.4096102000000000 | 0.9077632800000000   | 0.0692663800000000 | 1.0 |  |
| H7  | H | 0.6440498800000000 | 0.0667971700000000   | 0.9245041400000000 | 1.0 |  |
| H8  | H | 0.6812490700000000 | 0.8881826400000000   | 0.0379019000000000 | 1.0 |  |
| H9  | H | 0.9093315000000000 | 0.8516111400000000   | 0.9478009600000000 | 1.0 |  |
| H10 | H | 0.0759676100000000 | 0.9075578900000000   | 0.8760851500000000 | 1.0 |  |
| H11 | H | 0.4093484300000000 | 0.8515621800000000   | 0.9479036700000000 | 1.0 |  |
| H12 | H | 0.5759231600000000 | 0.9074602400000000   | 0.8759505800000000 | 1.0 |  |
| H13 | H | 0.9871508400000000 | 0.1278438600000000   | 0.0434827000000000 | 1.0 |  |
| H14 | H | 0.1035384500000000 | 0.0811682700000000   | 0.1183243900000000 | 1.0 |  |
| H15 | H | 0.4875173400000000 | 0.1279801000000000   | 0.0431222400000000 | 1.0 |  |
| H16 | H | 0.6003631600000000 | 0.0802051200000000   | 0.1182177200000000 | 1.0 |  |
| H17 | H | 0.1633165500000000 | 0.9771063100000000   | 0.8588812700000000 | 1.0 |  |
| H18 | H | 0.6632831700000000 | 0.9770228200000000   | 0.8588065800000000 | 1.0 |  |
| H19 | H | 0.8161918300000000 | 0.9048293500000000   | 0.9018621300000000 | 1.0 |  |
| H20 | H | 0.3159981600000000 | 0.9047649800000000   | 0.9019938500000000 | 1.0 |  |
| H21 | H | 0.8598067300000000 | 0.1528288600000000   | 0.9912434400000000 | 1.0 |  |
| H22 | H | 0.3627728700000000 | 0.1527348300000000   | 0.9894040900000000 | 1.0 |  |
| H23 | H | 0.2301037500000000 | 0.1286271200000000   | 0.0845237800000000 | 1.0 |  |
| H24 | H | 0.7292526100000000 | 0.1274138200000000   | 0.0861282600000000 | 1.0 |  |
| C25 | C | 0.8486777500000000 | 0.0546933000000000   | 0.0162452300000000 | 1.0 |  |
| C26 | C | 0.9350921100000000 | 0.0265762500000000   | 0.9553241700000000 | 1.0 |  |
| C27 | C | 0.9564366500000000 | 0.9489401300000000   | 0.9668437300000000 | 1.0 |  |
| C28 | C | 0.8779704300000000 | 0.9460983700000000   | 0.0334865200000000 | 1.0 |  |
| C29 | C | 0.1775503700000000 | 0.0484192800000000   | 0.0306407800000000 | 1.0 |  |
| C30 | C | 0.0979098200000000 | 0.0364715800000000   | 0.9644752300000000 | 1.0 |  |
| C31 | C | 0.1215253600000000 | 0.9602859000000000   | 0.9580615100000000 | 1.0 |  |
| C32 | C | 0.2116317100000000 | 0.9389543600000000   | 0.0213520100000000 | 1.0 |  |
| C33 | C | 0.3490475600000000 | 0.0549963800000000   | 0.0156054900000000 | 1.0 |  |
| C34 | C | 0.4355782300000000 | 0.0265298600000000   | 0.9549503800000000 | 1.0 |  |
| C35 | C | 0.4565138200000000 | 0.9489246700000000   | 0.9667527300000000 | 1.0 |  |
| C36 | C | 0.3780321900000000 | 0.9464730000000000   | 0.0334317700000000 | 1.0 |  |
| C37 | C | 0.6772923300000000 | 0.0479433300000000   | 0.0309581500000000 | 1.0 |  |
| C38 | C | 0.5983168900000000 | 0.0362636200000000   | 0.9645195400000000 | 1.0 |  |
| C39 | C | 0.6216599400000000 | 0.9600816400000000   | 0.9579873500000000 | 1.0 |  |
| C40 | C | 0.7116076400000000 | 0.9385076500000000   | 0.0212404600000000 | 1.0 |  |
| N41 | N | 0.8830987600000000 | 0.1232872200000000   | 0.0312644300000000 | 1.0 |  |
| N42 | N | 0.9138479700000000 | 0.8956080800000000   | 0.9217632700000000 | 1.0 |  |
| N43 | N | 0.1414125200000000 | 0.1017082500000000   | 0.0753931500000000 | 1.0 |  |
| N44 | N | 0.1575712900000000 | 0.9377355000000000   | 0.8911255200000000 | 1.0 |  |
| N45 | N | 0.3838085900000000 | 0.1237072500000000   | 0.0300969100000000 | 1.0 |  |
| N46 | N | 0.4137280400000000 | 0.8955282300000000   | 0.9218124800000000 | 1.0 |  |
| N47 | N | 0.6405169600000000 | 0.1009802200000000   | 0.0758943200000000 | 1.0 |  |
| N48 | N | 0.6575408100000000 | 0.9376092900000000   | 0.8910014600000000 | 1.0 |  |
| O49 | O | 0.8972977400000000 | 0.0094094100000000   | 0.0665174300000000 | 1.0 |  |
| O50 | O | 0.1608393300000000 | 0.9868467700000000   | 0.0673221900000000 | 1.0 |  |
| O51 | O | 0.3975935400000000 | 0.0099710200000000   | 0.0661267200000000 | 1.0 |  |
| O52 | O | 0.6604963600000000 | 0.9861661300000000   | 0.0673509300000000 | 1.0 |  |

##### cif ends

uran\_NH2\_34\_anti\_dir Energy: -321.54813121

##### cif starts

data\_uran\_NH2\_34\_anti\_dir

\_publ\_section\_comment

;  
Andrew Reynoso, Bohan Xu, and Vincent H. Crespi  
;

\_cell\_length\_a 9.5470954992

\_cell\_length\_b 20.0

\_cell\_length\_c 20.0

\_cell\_angle\_alpha 90.0

\_cell\_angle\_beta 90.0

\_cell\_angle\_gamma 90.0

\_symmetry\_space\_group\_name\_H-M 'P 1'

\_symmetry\_Int\_Tables\_number 1

\_symmetry\_cell\_setting triclinic

loop\_

\_atom\_site\_label

\_atom\_site\_type\_symbol

\_atom\_site\_fract\_x

\_atom\_site\_fract\_y

\_atom\_site\_fract\_z

\_atom\_site\_occupancy

|     |   |                    |                    |                    |     |
|-----|---|--------------------|--------------------|--------------------|-----|
| H1  | H | 0.9195056600000000 | 0.1062443300000000 | 0.9225515400000000 | 1.0 |
| H2  | H | 0.9194344500000000 | 0.9006383200000000 | 0.9252335400000000 | 1.0 |
| H3  | H | 0.9915930500000000 | 0.0579427200000000 | 0.0891189200000000 | 1.0 |
| H4  | H | 0.8303289100000000 | 0.0807912200000000 | 0.1050682000000000 | 1.0 |
| H5  | H | 0.9922524700000000 | 0.9528715000000000 | 0.0901331500000000 | 1.0 |
| H6  | H | 0.8306009000000000 | 0.9316671700000000 | 0.1072615700000000 | 1.0 |
| H7  | H | 0.1693984000000000 | 0.1075984300000000 | 0.0312705600000000 | 1.0 |
| H8  | H | 0.1695705300000000 | 0.9019938000000000 | 0.0338227600000000 | 1.0 |
| H9  | H | 0.0804743100000000 | 0.0770588600000000 | 0.8493214500000000 | 1.0 |
| H10 | H | 0.2419245700000000 | 0.0552274700000000 | 0.8661497600000000 | 1.0 |
| H11 | H | 0.2418261900000000 | 0.9502417800000000 | 0.8674260600000000 | 1.0 |
| H12 | H | 0.0803821400000000 | 0.9279261400000000 | 0.8512105100000000 | 1.0 |
| H13 | H | 0.4194729100000000 | 0.1062636100000000 | 0.9226088200000000 | 1.0 |
| H14 | H | 0.4194741200000000 | 0.9006568200000000 | 0.9251742800000000 | 1.0 |
| H15 | H | 0.4916836700000000 | 0.0579183100000000 | 0.0890892800000000 | 1.0 |
| H16 | H | 0.3303472100000000 | 0.0805508000000000 | 0.1051616100000000 | 1.0 |
| H17 | H | 0.4922216600000000 | 0.9528133500000000 | 0.0901351700000000 | 1.0 |
| H18 | H | 0.3306023900000000 | 0.9315069400000000 | 0.1072053200000000 | 1.0 |
| H19 | H | 0.6694036000000000 | 0.1076386500000000 | 0.0312333200000000 | 1.0 |
| H20 | H | 0.6695596700000000 | 0.9020346800000000 | 0.0338468600000000 | 1.0 |
| H21 | H | 0.5803809700000000 | 0.0770488400000000 | 0.8493160100000000 | 1.0 |
| H22 | H | 0.7418668500000000 | 0.0552624900000000 | 0.8661180000000000 | 1.0 |
| H23 | H | 0.7418306700000000 | 0.9502651100000000 | 0.8674092000000000 | 1.0 |
| H24 | H | 0.5804023700000000 | 0.9278934400000000 | 0.8512207900000000 | 1.0 |
| C25 | C | 0.9445899100000000 | 0.0585638900000000 | 0.9468356700000000 | 1.0 |
| C26 | C | 0.8570071700000000 | 0.0453075200000000 | 0.0103458400000000 | 1.0 |

|     |   |                    |                    |                    |     |
|-----|---|--------------------|--------------------|--------------------|-----|
| C27 | C | 0.8570104000000000 | 0.9638596600000000 | 0.0114068900000000 | 1.0 |
| C28 | C | 0.9445935300000000 | 0.9489285000000000 | 0.9482634200000000 | 1.0 |
| C29 | C | 0.1945763400000000 | 0.0593285100000000 | 0.0082073500000000 | 1.0 |
| C30 | C | 0.1070004900000000 | 0.0444386800000000 | 0.9450476600000000 | 1.0 |
| C31 | C | 0.1070014500000000 | 0.9629946500000000 | 0.9460691200000000 | 1.0 |
| C32 | C | 0.1946124600000000 | 0.9496926400000000 | 0.0095640100000000 | 1.0 |
| C33 | C | 0.4445850900000000 | 0.0585716400000000 | 0.9468633100000000 | 1.0 |
| C34 | C | 0.3570007500000000 | 0.0452728200000000 | 0.0103691100000000 | 1.0 |
| C35 | C | 0.3570159900000000 | 0.9638241500000000 | 0.0113873500000000 | 1.0 |
| C36 | C | 0.4446055100000000 | 0.9489345900000000 | 0.9482377000000000 | 1.0 |
| C37 | C | 0.6945862300000000 | 0.0593592000000000 | 0.0081878600000000 | 1.0 |
| C38 | C | 0.6069959600000000 | 0.0444532000000000 | 0.9450406300000000 | 1.0 |
| C39 | C | 0.6070164400000000 | 0.9630088300000000 | 0.9460651900000000 | 1.0 |
| C40 | C | 0.6946096600000000 | 0.9497255300000000 | 0.0095743800000000 | 1.0 |
| N41 | N | 0.9062047300000000 | 0.0811473700000000 | 0.0691283000000000 | 1.0 |
| N42 | N | 0.9059962900000000 | 0.9295675700000000 | 0.0711394100000000 | 1.0 |
| N43 | N | 0.1561140300000000 | 0.0787444500000000 | 0.8853433700000000 | 1.0 |
| N44 | N | 0.1560719100000000 | 0.9271957600000000 | 0.8872400600000000 | 1.0 |
| N45 | N | 0.4061469400000000 | 0.0810720200000000 | 0.0691846700000000 | 1.0 |
| N46 | N | 0.4060281000000000 | 0.9294950200000000 | 0.0710948400000000 | 1.0 |
| N47 | N | 0.6560465400000000 | 0.0787604900000000 | 0.8853251900000000 | 1.0 |
| N48 | N | 0.6561113700000000 | 0.9272053900000000 | 0.8872418600000000 | 1.0 |
| O49 | O | 0.8995544700000000 | 0.0031811600000000 | 0.9040941300000000 | 1.0 |
| O50 | O | 0.1495573200000000 | 0.0050450000000000 | 0.0523418000000000 | 1.0 |
| O51 | O | 0.3995563700000000 | 0.0032057100000000 | 0.9040960300000000 | 1.0 |
| O52 | O | 0.6495524700000000 | 0.0050894100000000 | 0.0523355700000000 | 1.0 |

##### cif ends

uran\_NH2\_34\_anti\_dir\_forbid Energy: -322.09081287

##### cif starts

data\_uran\_NH2\_34\_anti\_dir\_forbid

\_publ\_section\_comment

;

Andrew Reynoso, Bohan Xu, and Vincent H. Crespi

;

\_cell\_length\_a 10.2478229698

\_cell\_length\_b 20.0

\_cell\_length\_c 20.0

\_cell\_angle\_alpha 90.0

\_cell\_angle\_beta 90.0

\_cell\_angle\_gamma 90.0

\_symmetry\_space\_group\_name\_H-M 'P 1'

\_symmetry\_Int\_Tables\_number 1

\_symmetry\_cell\_setting triclinic

loop\_

\_atom\_site\_label

\_atom\_site\_type\_symbol

\_atom\_site\_fract\_x

\_atom\_site\_fract\_y

\_atom\_site\_fract\_z

|     | atom | site               | occupancy          |                    |     |  |  |
|-----|------|--------------------|--------------------|--------------------|-----|--|--|
| H1  | H    | 0.1758922000000000 | 0.1066650300000000 | 0.9476737400000000 | 1.0 |  |  |
| H2  | H    | 0.1811088400000000 | 0.9027780000000000 | 0.9449282500000000 | 1.0 |  |  |
| H3  | H    | 0.1436297300000000 | 0.0754938500000000 | 0.1071625700000000 | 1.0 |  |  |
| H4  | H    | 0.9871610700000000 | 0.0594017500000000 | 0.1103043600000000 | 1.0 |  |  |
| H5  | H    | 0.1337969300000000 | 0.9468361100000000 | 0.1131417100000000 | 1.0 |  |  |
| H6  | H    | 0.0673124400000000 | 0.8798647100000000 | 0.0795924600000000 | 1.0 |  |  |
| H7  | H    | 0.3283841900000000 | 0.1069868800000000 | 0.0467584200000000 | 1.0 |  |  |
| H8  | H    | 0.3231808200000000 | 0.9031200200000000 | 0.0508357900000000 | 1.0 |  |  |
| H9  | H    | 0.3606630200000000 | 0.0747457400000000 | 0.8874457600000000 | 1.0 |  |  |
| H10 | H    | 0.5171386700000000 | 0.0586470600000000 | 0.8844493600000000 | 1.0 |  |  |
| H11 | H    | 0.3704571300000000 | 0.9460509000000000 | 0.8823342100000000 | 1.0 |  |  |
| H12 | H    | 0.4370640400000000 | 0.8793272500000000 | 0.9163186400000000 | 1.0 |  |  |
| H13 | H    | 0.6758912400000000 | 0.1066663400000000 | 0.9476769400000000 | 1.0 |  |  |
| H14 | H    | 0.6811109000000000 | 0.9027796800000000 | 0.9449247500000000 | 1.0 |  |  |
| H15 | H    | 0.6436291200000000 | 0.0754960600000000 | 0.1071624600000000 | 1.0 |  |  |
| H16 | H    | 0.4871653000000000 | 0.0593922400000000 | 0.1103073100000000 | 1.0 |  |  |
| H17 | H    | 0.6338054300000000 | 0.9468275400000000 | 0.1131380300000000 | 1.0 |  |  |
| H18 | H    | 0.5672996500000000 | 0.8798615300000000 | 0.0795884400000000 | 1.0 |  |  |
| H19 | H    | 0.8283836700000000 | 0.1069852900000000 | 0.0467614900000000 | 1.0 |  |  |
| H20 | H    | 0.8231808800000000 | 0.9031181700000000 | 0.0508329900000000 | 1.0 |  |  |
| H21 | H    | 0.8606615900000000 | 0.0747388500000000 | 0.8874443400000000 | 1.0 |  |  |
| H22 | H    | 0.0171443700000000 | 0.0586572600000000 | 0.8844526100000000 | 1.0 |  |  |
| H23 | H    | 0.8704729600000000 | 0.9460606900000000 | 0.8823299400000000 | 1.0 |  |  |
| H24 | H    | 0.9370413500000000 | 0.8793289200000000 | 0.9163173700000000 | 1.0 |  |  |
| C25 | C    | 0.1885337700000000 | 0.0606951100000000 | 0.9769506200000000 | 1.0 |  |  |
| C26 | C    | 0.0665596900000000 | 0.0432280500000000 | 0.0192174700000000 | 1.0 |  |  |
| C27 | C    | 0.0672111300000000 | 0.9626959800000000 | 0.0186425700000000 | 1.0 |  |  |
| C28 | C    | 0.1894128700000000 | 0.9477656900000000 | 0.9761734500000000 | 1.0 |  |  |
| C29 | C    | 0.3157201700000000 | 0.0608272000000000 | 0.0177841500000000 | 1.0 |  |  |
| C30 | C    | 0.4376815300000000 | 0.0430841500000000 | 0.9756243700000000 | 1.0 |  |  |
| C31 | C    | 0.4370429400000000 | 0.9625576500000000 | 0.9767291100000000 | 1.0 |  |  |
| C32 | C    | 0.3148562400000000 | 0.9479052100000000 | 0.0193011700000000 | 1.0 |  |  |
| C33 | C    | 0.6885331300000000 | 0.0606956200000000 | 0.9769526300000000 | 1.0 |  |  |
| C34 | C    | 0.5665591600000000 | 0.0432267800000000 | 0.0192184100000000 | 1.0 |  |  |
| C35 | C    | 0.5672113500000000 | 0.9626948400000000 | 0.0186414600000000 | 1.0 |  |  |
| C36 | C    | 0.6894135200000000 | 0.9477661900000000 | 0.9761716800000000 | 1.0 |  |  |
| C37 | C    | 0.8157194000000000 | 0.0608263400000000 | 0.0177860800000000 | 1.0 |  |  |
| C38 | C    | 0.9376808000000000 | 0.0430847100000000 | 0.9756250100000000 | 1.0 |  |  |
| C39 | C    | 0.9370436700000000 | 0.9625582500000000 | 0.9767290700000000 | 1.0 |  |  |
| C40 | C    | 0.8148565300000000 | 0.9479045000000000 | 0.0192999100000000 | 1.0 |  |  |
| N41 | N    | 0.0585056300000000 | 0.0800828500000000 | 0.0810616800000000 | 1.0 |  |  |
| N42 | N    | 0.0589082200000000 | 0.9305955600000000 | 0.0835740300000000 | 1.0 |  |  |
| N43 | N    | 0.4457621600000000 | 0.0795217300000000 | 0.9135345300000000 | 1.0 |  |  |
| N44 | N    | 0.4453670200000000 | 0.9300352700000000 | 0.9120091700000000 | 1.0 |  |  |
| N45 | N    | 0.5585015100000000 | 0.0800794800000000 | 0.0810635700000000 | 1.0 |  |  |
| N46 | N    | 0.5589093600000000 | 0.9305927900000000 | 0.0835720900000000 | 1.0 |  |  |
| N47 | N    | 0.9457558200000000 | 0.0795236700000000 | 0.9135357800000000 | 1.0 |  |  |
| N48 | N    | 0.9453695200000000 | 0.9300359400000000 | 0.9120089500000000 | 1.0 |  |  |
| O49 | O    | 0.1959332400000000 | 0.0046732900000000 | 0.9308159900000000 | 1.0 |  |  |
| O50 | O    | 0.3083384700000000 | 0.0051031800000000 | 0.0642866500000000 | 1.0 |  |  |
| O51 | O    | 0.6959336200000000 | 0.0046752700000000 | 0.9308161200000000 | 1.0 |  |  |
| O52 | O    | 0.8083378900000000 | 0.0051010200000000 | 0.0642869900000000 | 1.0 |  |  |

##### cif ends

furand\_NH2\_34\_syn\_dir Energy: -320.81767075

##### cif starts

data\_furand\_NH2\_34\_syn\_dir

\_publ\_section\_comment

;  
Andrew Reynoso, Bohan Xu, and Vincent H. Crespi  
;

\_cell\_length\_a 10.6158099445

\_cell\_length\_b 20.0

\_cell\_length\_c 20.0

\_cell\_angle\_alpha 90.0

\_cell\_angle\_beta 90.0

\_cell\_angle\_gamma 90.0

\_symmetry\_space\_group\_name\_H-M 'P 1'

\_symmetry\_Int\_Tables\_number 1

\_symmetry\_cell\_setting triclinic

loop\_

\_atom\_site\_label

\_atom\_site\_type\_symbol

\_atom\_site\_fract\_x

\_atom\_site\_fract\_y

\_atom\_site\_fract\_z

\_atom\_site\_occupancy

|     |   |                    |                    |                    |     |
|-----|---|--------------------|--------------------|--------------------|-----|
| H1  | H | 0.0221771200000000 | 0.0572315600000000 | 0.1067548800000000 | 1.0 |
| H2  | H | 0.0219189600000000 | 0.8653201600000000 | 0.0392941600000000 | 1.0 |
| H3  | H | 0.0575509200000000 | 0.0967158000000000 | 0.9708854800000000 | 1.0 |
| H4  | H | 0.1599951300000000 | 0.0549924100000000 | 0.9250326400000000 | 1.0 |
| H5  | H | 0.0616471200000000 | 0.9537309400000000 | 0.9047338600000000 | 1.0 |
| H6  | H | 0.1623843600000000 | 0.8918579000000000 | 0.9090609000000000 | 1.0 |
| H7  | H | 0.2721803000000000 | 0.0572314100000000 | 0.1067544800000000 | 1.0 |
| H8  | H | 0.2719197400000000 | 0.8653184000000000 | 0.0392924600000000 | 1.0 |
| H9  | H | 0.3075546000000000 | 0.0967174500000000 | 0.9708885900000000 | 1.0 |
| H10 | H | 0.4099900100000000 | 0.0549933900000000 | 0.9250304000000000 | 1.0 |
| H11 | H | 0.5221772700000000 | 0.0572320300000000 | 0.1067556200000000 | 1.0 |
| H12 | H | 0.5219194700000000 | 0.8653210200000000 | 0.0392934000000000 | 1.0 |
| H13 | H | 0.5575521700000000 | 0.0967178900000000 | 0.9708865000000000 | 1.0 |
| H14 | H | 0.6599968600000000 | 0.0549944400000000 | 0.9250334600000000 | 1.0 |
| H15 | H | 0.5616466500000000 | 0.9537342200000000 | 0.9047339200000000 | 1.0 |
| H16 | H | 0.6623833500000000 | 0.8918610500000000 | 0.9090591500000000 | 1.0 |
| H17 | H | 0.7721830000000000 | 0.0572316900000000 | 0.1067540300000000 | 1.0 |
| H18 | H | 0.7719175300000000 | 0.8653185700000000 | 0.0392920400000000 | 1.0 |
| H19 | H | 0.8075567800000000 | 0.0967161800000000 | 0.9708859000000000 | 1.0 |
| H20 | H | 0.9099901700000000 | 0.0549887200000000 | 0.9250287100000000 | 1.0 |
| H21 | H | 0.3116509600000000 | 0.9537292500000000 | 0.9047333100000000 | 1.0 |
| H22 | H | 0.4123899800000000 | 0.8918578600000000 | 0.9090580400000000 | 1.0 |
| H23 | H | 0.8116520700000000 | 0.9537309400000000 | 0.9047328600000000 | 1.0 |
| H24 | H | 0.9123880000000000 | 0.8918579700000000 | 0.9090567600000000 | 1.0 |
| C25 | C | 0.0225197300000000 | 0.0209100000000000 | 0.0655764800000000 | 1.0 |
| C26 | C | 0.1471322000000000 | 0.0221242800000000 | 0.0215322200000000 | 1.0 |
| C27 | C | 0.1472834400000000 | 0.9463851600000000 | 0.9950998500000000 | 1.0 |

|     |   |                    |                    |                    |     |
|-----|---|--------------------|--------------------|--------------------|-----|
| C28 | C | 0.0219327700000000 | 0.9195731300000000 | 0.0298776900000000 | 1.0 |
| C29 | C | 0.2725200400000000 | 0.0209101100000000 | 0.0655754500000000 | 1.0 |
| C30 | C | 0.3971394300000000 | 0.0221242400000000 | 0.0215313900000000 | 1.0 |
| C31 | C | 0.3972923700000000 | 0.9463850700000000 | 0.9950980200000000 | 1.0 |
| C32 | C | 0.2719320400000000 | 0.9195714500000000 | 0.0298781200000000 | 1.0 |
| C33 | C | 0.5225198000000000 | 0.0209106100000000 | 0.0655770900000000 | 1.0 |
| C34 | C | 0.6471323500000000 | 0.0221251900000000 | 0.0215325800000000 | 1.0 |
| C35 | C | 0.6472833600000000 | 0.9463863400000000 | 0.9950995600000000 | 1.0 |
| C36 | C | 0.5219330400000000 | 0.9195739900000000 | 0.0298775200000000 | 1.0 |
| C37 | C | 0.7725207600000000 | 0.0209102600000000 | 0.0655750500000000 | 1.0 |
| C38 | C | 0.8971396600000000 | 0.0221234500000000 | 0.0215305800000000 | 1.0 |
| C39 | C | 0.8972923000000000 | 0.9463843300000000 | 0.9950977600000000 | 1.0 |
| C40 | C | 0.7719313800000000 | 0.9195716300000000 | 0.0298776700000000 | 1.0 |
| N41 | N | 0.1460871200000000 | 0.0752282800000000 | 0.9715144700000000 | 1.0 |
| N42 | N | 0.1503854500000000 | 0.9409440300000000 | 0.9221419600000000 | 1.0 |
| N43 | N | 0.3960885400000000 | 0.0752290300000000 | 0.9715136600000000 | 1.0 |
| N44 | N | 0.4003924600000000 | 0.9409431200000000 | 0.9221391000000000 | 1.0 |
| N45 | N | 0.6460879500000000 | 0.0752296600000000 | 0.9715153000000000 | 1.0 |
| N46 | N | 0.6503850900000000 | 0.9409469000000000 | 0.9221415700000000 | 1.0 |
| N47 | N | 0.8960897000000000 | 0.0752263900000000 | 0.9715109100000000 | 1.0 |
| N48 | N | 0.9003925800000000 | 0.9409430900000000 | 0.9221387600000000 | 1.0 |
| O49 | O | 0.0220876800000000 | 0.9543691500000000 | 0.0922033800000000 | 1.0 |
| O50 | O | 0.2720939600000000 | 0.9543670800000000 | 0.0922026000000000 | 1.0 |
| O51 | O | 0.5220882200000000 | 0.9543695500000000 | 0.0922034900000000 | 1.0 |
| O52 | O | 0.7720940400000000 | 0.9543672300000000 | 0.0922022300000000 | 1.0 |

##### cif ends

furand\_NH2\_34\_syn\_dir\_forbid    Energy: -318.38606418

##### cif starts

data\_furand\_NH2\_34\_syn\_dir\_forbid

\_publ\_section\_comment

;  
Andrew Reynoso, Bohan Xu, and Vincent H. Crespi  
;

\_cell\_length\_a    9.8233560806  
\_cell\_length\_b    20.0  
\_cell\_length\_c    20.0  
\_cell\_angle\_alpha    90.0  
\_cell\_angle\_beta    90.0  
\_cell\_angle\_gamma    90.0

\_symmetry\_space\_group\_name\_H-M    'P 1'  
\_symmetry\_Int\_Tables\_number 1  
\_symmetry\_cell\_setting triclinic

loop\_  
\_atom\_site\_label  
\_atom\_site\_type\_symbol  
\_atom\_site\_fract\_x  
\_atom\_site\_fract\_y  
\_atom\_site\_fract\_z  
\_atom\_site\_occupancy

|     |   |                    |                    |                    |     |
|-----|---|--------------------|--------------------|--------------------|-----|
| H1  | H | 0.8825516500000000 | 0.1033077100000000 | 0.0351418600000000 | 1.0 |
| H2  | H | 0.9065081700000000 | 0.9031872900000000 | 0.0628699000000000 | 1.0 |
| H3  | H | 0.1531785900000000 | 0.0898931600000000 | 0.0637927900000000 | 1.0 |
| H4  | H | 0.1774886300000000 | 0.8903047300000000 | 0.0322527400000000 | 1.0 |
| H5  | H | 0.3825361800000000 | 0.1032921800000000 | 0.0351670600000000 | 1.0 |
| H6  | H | 0.4065171600000000 | 0.9031656200000000 | 0.0628407000000000 | 1.0 |
| H7  | H | 0.6531971200000000 | 0.0899208400000000 | 0.0637814900000000 | 1.0 |
| H8  | H | 0.6774773600000000 | 0.8903262400000000 | 0.0322740600000000 | 1.0 |
| H9  | H | 0.9838428700000000 | 0.0773855800000000 | 0.8704371300000000 | 1.0 |
| H10 | H | 0.2450964900000000 | 0.0827178400000000 | 0.8983587300000000 | 1.0 |
| H11 | H | 0.4838337500000000 | 0.0773964300000000 | 0.8704388400000000 | 1.0 |
| H12 | H | 0.7451029500000000 | 0.0827117900000000 | 0.8983495400000000 | 1.0 |
| H13 | H | 0.0003825100000000 | 0.8951228900000000 | 0.8853902800000000 | 1.0 |
| H14 | H | 0.2585393200000000 | 0.9259528800000000 | 0.8858025300000000 | 1.0 |
| H15 | H | 0.5004074500000000 | 0.8951715500000000 | 0.8853531400000000 | 1.0 |
| H16 | H | 0.7585556100000000 | 0.9259425200000000 | 0.8858192000000000 | 1.0 |
| H17 | H | 0.1458290400000000 | 0.9812264600000000 | 0.8545263100000000 | 1.0 |
| H18 | H | 0.6459356900000000 | 0.9812591900000000 | 0.8545386000000000 | 1.0 |
| H19 | H | 0.8882780300000000 | 0.8601803500000000 | 0.9381138300000000 | 1.0 |
| H20 | H | 0.3883075600000000 | 0.8601970800000000 | 0.9380558700000000 | 1.0 |
| H21 | H | 0.8888045500000000 | 0.0088068100000000 | 0.8589120500000000 | 1.0 |
| H22 | H | 0.3887770000000000 | 0.0088251400000000 | 0.8589186800000000 | 1.0 |
| H23 | H | 0.1397684000000000 | 0.1381139700000000 | 0.9344668600000000 | 1.0 |
| H24 | H | 0.6397871900000000 | 0.1381198300000000 | 0.9344488400000000 | 1.0 |
| C25 | C | 0.8494986000000000 | 0.0534873100000000 | 0.0184228300000000 | 1.0 |
| C26 | C | 0.9376618600000000 | 0.0302681900000000 | 0.9556905300000000 | 1.0 |
| C27 | C | 0.9601369100000000 | 0.9523357400000000 | 0.9648948400000000 | 1.0 |
| C28 | C | 0.8778551500000000 | 0.9445996100000000 | 0.0295804300000000 | 1.0 |
| C29 | C | 0.1827350200000000 | 0.0490938000000000 | 0.0299314500000000 | 1.0 |
| C30 | C | 0.1021101100000000 | 0.0425409700000000 | 0.9643450200000000 | 1.0 |
| C31 | C | 0.1247215600000000 | 0.9648253700000000 | 0.9545102400000000 | 1.0 |
| C32 | C | 0.2111948200000000 | 0.9405245900000000 | 0.0170543700000000 | 1.0 |
| C33 | C | 0.3494923600000000 | 0.0534763200000000 | 0.0184318500000000 | 1.0 |
| C34 | C | 0.4376635400000000 | 0.0302768700000000 | 0.9556940300000000 | 1.0 |
| C35 | C | 0.4601412800000000 | 0.9523436400000000 | 0.9648821500000000 | 1.0 |
| C36 | C | 0.3778553700000000 | 0.9445858400000000 | 0.0295626700000000 | 1.0 |
| C37 | C | 0.6827444500000000 | 0.0491142200000000 | 0.0299283000000000 | 1.0 |
| C38 | C | 0.6021156100000000 | 0.0425515300000000 | 0.9643442600000000 | 1.0 |
| C39 | C | 0.6247332800000000 | 0.9648366100000000 | 0.9545135000000000 | 1.0 |
| C40 | C | 0.7111938700000000 | 0.9405423100000000 | 0.0170680200000000 | 1.0 |
| N41 | N | 0.9013033700000000 | 0.0501582800000000 | 0.8882990400000000 | 1.0 |
| N42 | N | 0.9155714400000000 | 0.9038983900000000 | 0.9153595000000000 | 1.0 |
| N43 | N | 0.1448580600000000 | 0.0911481800000000 | 0.9143995300000000 | 1.0 |
| N44 | N | 0.1584692200000000 | 0.9429693500000000 | 0.8877699500000000 | 1.0 |
| N45 | N | 0.4012940500000000 | 0.0501742200000000 | 0.8883067200000000 | 1.0 |
| N46 | N | 0.4155882400000000 | 0.9039282100000000 | 0.9153235200000000 | 1.0 |
| N47 | N | 0.6448669000000000 | 0.0911496600000000 | 0.9143902900000000 | 1.0 |
| N48 | N | 0.6585058000000000 | 0.9429895700000000 | 0.8877739500000000 | 1.0 |
| O49 | O | 0.8978013400000000 | 0.0053904800000000 | 0.0656955700000000 | 1.0 |
| O50 | O | 0.1622302100000000 | 0.9874852700000000 | 0.0650906400000000 | 1.0 |
| O51 | O | 0.3977976900000000 | 0.0053684800000000 | 0.0656938100000000 | 1.0 |
| O52 | O | 0.6622307500000000 | 0.9875122300000000 | 0.0650954200000000 | 1.0 |

##### cif ends

furan\_NH2\_3\_anti\_alt Energy: -274.55527589

##### cif starts

data\_furan\_NH2\_3\_anti\_alt

\_publ\_section\_comment

;  
Andrew Reynoso, Bohan Xu, and Vincent H. Crespi  
;

\_cell\_length\_a 9.3892363918

\_cell\_length\_b 20.0

\_cell\_length\_c 20.0

\_cell\_angle\_alpha 90.0

\_cell\_angle\_beta 90.0

\_cell\_angle\_gamma 90.0

\_symmetry\_space\_group\_name\_H-M 'P 1'

\_symmetry\_Int\_Tables\_number 1

\_symmetry\_cell\_setting triclinic

loop\_

\_atom\_site\_label

\_atom\_site\_type\_symbol

\_atom\_site\_fract\_x

\_atom\_site\_fract\_y

\_atom\_site\_fract\_z

\_atom\_site\_occupancy

|     |   |                    |                    |                    |     |
|-----|---|--------------------|--------------------|--------------------|-----|
| H1  | H | 0.0122859800000000 | 0.9177761700000000 | 0.9223036600000000 | 1.0 |
| H2  | H | 0.9991365900000000 | 0.0715743500000000 | 0.0651097900000000 | 1.0 |
| H3  | H | 0.0097943800000000 | 0.1222211400000000 | 0.9356815900000000 | 1.0 |
| H4  | H | 0.9238083500000000 | 0.9321969000000000 | 0.1065296100000000 | 1.0 |
| H5  | H | 0.0842024600000000 | 0.9613555400000000 | 0.0941675200000000 | 1.0 |
| H6  | H | 0.2623203100000000 | 0.1165852500000000 | 0.0485433500000000 | 1.0 |
| H7  | H | 0.2491343600000000 | 0.9627584300000000 | 0.9057745500000000 | 1.0 |
| H8  | H | 0.2598389600000000 | 0.9121321400000000 | 0.0352190000000000 | 1.0 |
| H9  | H | 0.1736972800000000 | 0.1022754200000000 | 0.8644013600000000 | 1.0 |
| H10 | H | 0.3340228500000000 | 0.0729472300000000 | 0.8766267000000000 | 1.0 |
| H11 | H | 0.5122963900000000 | 0.9177755200000000 | 0.9222970500000000 | 1.0 |
| H12 | H | 0.4991574300000000 | 0.0716008600000000 | 0.0650733700000000 | 1.0 |
| H13 | H | 0.5098436800000000 | 0.1222200000000000 | 0.9356372000000000 | 1.0 |
| H14 | H | 0.4237775800000000 | 0.9322161700000000 | 0.1065122800000000 | 1.0 |
| H15 | H | 0.5841668000000000 | 0.9613924300000000 | 0.0941704400000000 | 1.0 |
| H16 | H | 0.7622916900000000 | 0.1165604100000000 | 0.0485732400000000 | 1.0 |
| H17 | H | 0.7491568900000000 | 0.9627524500000000 | 0.9057756400000000 | 1.0 |
| H18 | H | 0.7598229400000000 | 0.9121131000000000 | 0.0352142200000000 | 1.0 |
| H19 | H | 0.6738091200000000 | 0.1023173700000000 | 0.8644152400000000 | 1.0 |
| H20 | H | 0.8340991100000000 | 0.0729460500000000 | 0.8766491000000000 | 1.0 |
| C21 | C | 0.0372266500000000 | 0.9642596300000000 | 0.9490105900000000 | 1.0 |
| C22 | C | 0.9501357200000000 | 0.9746032600000000 | 0.0147018700000000 | 1.0 |
| C23 | C | 0.9504333200000000 | 0.0540605600000000 | 0.0184262200000000 | 1.0 |
| C24 | C | 0.0358093500000000 | 0.0730731200000000 | 0.9565697200000000 | 1.0 |
| C25 | C | 0.2872489500000000 | 0.0700934900000000 | 0.0218494600000000 | 1.0 |
| C26 | C | 0.2001261500000000 | 0.0597330500000000 | 0.9561742800000000 | 1.0 |
| C27 | C | 0.2004261700000000 | 0.9802730100000000 | 0.9524560600000000 | 1.0 |
| C28 | C | 0.2858235200000000 | 0.9612755100000000 | 0.0143130300000000 | 1.0 |



|     |   |                    |                    |                    |     |
|-----|---|--------------------|--------------------|--------------------|-----|
| C29 | C | 0.5372363600000000 | 0.9642615500000000 | 0.9489989900000000 | 1.0 |
| C30 | C | 0.4501400700000000 | 0.9746184900000000 | 0.0146874400000000 | 1.0 |
| C31 | C | 0.4504416400000000 | 0.0540766900000000 | 0.0183973900000000 | 1.0 |
| C32 | C | 0.5358308300000000 | 0.0730745600000000 | 0.9565408600000000 | 1.0 |
| C33 | C | 0.7872365600000000 | 0.0700762100000000 | 0.0218692100000000 | 1.0 |
| C34 | C | 0.7001506100000000 | 0.0597296700000000 | 0.9561773200000000 | 1.0 |
| C35 | C | 0.7004401500000000 | 0.9802681200000000 | 0.9524544400000000 | 1.0 |
| C36 | C | 0.7858180300000000 | 0.9612592000000000 | 0.0143164100000000 | 1.0 |
| N37 | N | 0.0029170700000000 | 0.9360009500000000 | 0.0717439900000000 | 1.0 |
| N38 | N | 0.2528890700000000 | 0.0983384000000000 | 0.8991282700000000 | 1.0 |
| N39 | N | 0.5029083900000000 | 0.9360261700000000 | 0.0717387700000000 | 1.0 |
| N40 | N | 0.7529743600000000 | 0.0983440600000000 | 0.8991499500000000 | 1.0 |
| O41 | O | 0.9917442300000000 | 0.0208845900000000 | 0.9089543000000000 | 1.0 |
| O42 | O | 0.2417897200000000 | 0.0134810200000000 | 0.0619231400000000 | 1.0 |
| O43 | O | 0.4917762600000000 | 0.0208826300000000 | 0.9089311300000000 | 1.0 |
| O44 | O | 0.7417706600000000 | 0.0134581300000000 | 0.0619292900000000 | 1.0 |

##### cif ends

furan\_NH2\_3\_anti\_alt\_forbid Energy: -274.89770505

##### cif starts

data\_furan\_NH2\_3\_anti\_alt\_forbid

\_publ\_section\_comment

;  
Andrew Reynoso, Bohan Xu, and Vincent H. Crespi  
;

\_cell\_length\_a 10.2140572404

\_cell\_length\_b 20.0

\_cell\_length\_c 20.0

\_cell\_angle\_alpha 90.0

\_cell\_angle\_beta 90.0

\_cell\_angle\_gamma 90.0

\_symmetry\_space\_group\_name\_H-M 'P 1'

\_symmetry\_Int\_Tables\_number 1

\_symmetry\_cell\_setting triclinic

loop\_

\_atom\_site\_label

\_atom\_site\_type\_symbol

\_atom\_site\_fract\_x

\_atom\_site\_fract\_y

\_atom\_site\_fract\_z

\_atom\_site\_occupancy

|    |   |                    |                    |                    |     |
|----|---|--------------------|--------------------|--------------------|-----|
| H1 | H | 0.0755980500000000 | 0.0945865400000000 | 0.9264194200000000 | 1.0 |
|----|---|--------------------|--------------------|--------------------|-----|

|    |   |                    |                    |                    |     |
|----|---|--------------------|--------------------|--------------------|-----|
| H2 | H | 0.9594370800000000 | 0.9355127300000000 | 0.0566024400000000 | 1.0 |
|----|---|--------------------|--------------------|--------------------|-----|

|    |   |                    |                    |                    |     |
|----|---|--------------------|--------------------|--------------------|-----|
| H3 | H | 0.0798273700000000 | 0.8905091500000000 | 0.9399978600000000 | 1.0 |
|----|---|--------------------|--------------------|--------------------|-----|

|    |   |                    |                    |                    |     |
|----|---|--------------------|--------------------|--------------------|-----|
| H4 | H | 0.3395063400000000 | 0.0569127100000000 | 0.9120363000000000 | 1.0 |
|----|---|--------------------|--------------------|--------------------|-----|

|    |   |                    |                    |                    |     |
|----|---|--------------------|--------------------|--------------------|-----|
| H5 | H | 0.2189986800000000 | 0.1019550600000000 | 0.0286302000000000 | 1.0 |
|----|---|--------------------|--------------------|--------------------|-----|

|    |   |                    |                    |                    |     |
|----|---|--------------------|--------------------|--------------------|-----|
| H6 | H | 0.2232256100000000 | 0.8978756700000000 | 0.0422229400000000 | 1.0 |
|----|---|--------------------|--------------------|--------------------|-----|

|    |   |                    |                    |                    |     |
|----|---|--------------------|--------------------|--------------------|-----|
| H7 | H | 0.5756625900000000 | 0.0945330300000000 | 0.9263141300000000 | 1.0 |
|----|---|--------------------|--------------------|--------------------|-----|

|    |   |                    |                    |                    |     |
|----|---|--------------------|--------------------|--------------------|-----|
| H8 | H | 0.4593153500000000 | 0.9355967800000000 | 0.0566401300000000 | 1.0 |
|----|---|--------------------|--------------------|--------------------|-----|

|    |   |                    |                    |                    |     |
|----|---|--------------------|--------------------|--------------------|-----|
| H9 | H | 0.5797609400000000 | 0.8904743100000000 | 0.9401097200000000 | 1.0 |
|----|---|--------------------|--------------------|--------------------|-----|

|     |   |                    |                    |                    |     |
|-----|---|--------------------|--------------------|--------------------|-----|
| H10 | H | 0.8396341900000000 | 0.0568866100000000 | 0.9120335200000000 | 1.0 |
| H11 | H | 0.7190873200000000 | 0.1019869500000000 | 0.0285399900000000 | 1.0 |
| H12 | H | 0.7231769800000000 | 0.8979194900000000 | 0.0423132500000000 | 1.0 |
| H13 | H | 0.2581557400000000 | 0.9252514600000000 | 0.8767868500000000 | 1.0 |
| H14 | H | 0.7580538600000000 | 0.9252117900000000 | 0.8768183100000000 | 1.0 |
| H15 | H | 0.8809231000000000 | 0.0661502900000000 | 0.0906101300000000 | 1.0 |
| H16 | H | 0.3809879900000000 | 0.0663099300000000 | 0.0905583700000000 | 1.0 |
| H17 | H | 0.4177629200000000 | 0.9265403500000000 | 0.8779322200000000 | 1.0 |
| H18 | H | 0.9176625100000000 | 0.9264376900000000 | 0.8779404900000000 | 1.0 |
| H19 | H | 0.0405346400000000 | 0.0668959400000000 | 0.0920149600000000 | 1.0 |
| H20 | H | 0.5405952700000000 | 0.0669667000000000 | 0.0919681500000000 | 1.0 |
| C21 | C | 0.0861065900000000 | 0.0507998400000000 | 0.9591838500000000 | 1.0 |
| C22 | C | 0.9643631200000000 | 0.0370245800000000 | 0.0033294000000000 | 1.0 |
| C23 | C | 0.9644819700000000 | 0.9573871500000000 | 0.0063250900000000 | 1.0 |
| C24 | C | 0.0867003000000000 | 0.9381699200000000 | 0.9670754200000000 | 1.0 |
| C25 | C | 0.2121898900000000 | 0.0542903500000000 | 0.0015571700000000 | 1.0 |
| C26 | C | 0.3344293700000000 | 0.0350656300000000 | 0.9623226100000000 | 1.0 |
| C27 | C | 0.3345492100000000 | 0.9554244500000000 | 0.9653336600000000 | 1.0 |
| C28 | C | 0.2127748800000000 | 0.9416597300000000 | 0.0094527000000000 | 1.0 |
| C29 | C | 0.5861328600000000 | 0.0507865100000000 | 0.9591365300000000 | 1.0 |
| C30 | C | 0.4643800400000000 | 0.0370706600000000 | 0.0033020800000000 | 1.0 |
| C31 | C | 0.4644562600000000 | 0.9574343000000000 | 0.0063496900000000 | 1.0 |
| C32 | C | 0.5866790300000000 | 0.9381607600000000 | 0.9671367700000000 | 1.0 |
| C33 | C | 0.7122182900000000 | 0.0543013200000000 | 0.0015102900000000 | 1.0 |
| C34 | C | 0.8344584700000000 | 0.0350286900000000 | 0.9623120100000000 | 1.0 |
| C35 | C | 0.8345342800000000 | 0.9553863200000000 | 0.9653443800000000 | 1.0 |
| C36 | C | 0.7127628900000000 | 0.9416734200000000 | 0.0094998900000000 | 1.0 |
| N37 | N | 0.9614859400000000 | 0.0782528800000000 | 0.0628243600000000 | 1.0 |
| N38 | N | 0.3375286100000000 | 0.9141777100000000 | 0.9058549100000000 | 1.0 |
| N39 | N | 0.4615769200000000 | 0.0783452600000000 | 0.0627648200000000 | 1.0 |
| N40 | N | 0.8374247000000000 | 0.9141158800000000 | 0.9058801400000000 | 1.0 |
| O41 | O | 0.0941541600000000 | 0.9918188700000000 | 0.9170919400000000 | 1.0 |
| O42 | O | 0.2047164100000000 | 0.0006455100000000 | 0.0515387400000000 | 1.0 |
| O43 | O | 0.5941590600000000 | 0.9917618000000000 | 0.9171028900000000 | 1.0 |
| O44 | O | 0.7047240700000000 | 0.0006967100000000 | 0.0515353100000000 | 1.0 |

##### cif ends

furand\_NH2\_3\_anti\_dir Energy: -274.24488237

##### cif starts

data\_furand\_NH2\_3\_anti\_dir

\_publ\_section\_comment

;  
Andrew Reynoso, Bohan Xu, and Vincent H. Crespi  
;

\_cell\_length\_a 9.4196108531

\_cell\_length\_b 20.0

\_cell\_length\_c 20.0

\_cell\_angle\_alpha 90.0

\_cell\_angle\_beta 90.0

\_cell\_angle\_gamma 90.0

\_symmetry\_space\_group\_name\_H-M 'P 1'

\_symmetry\_Int\_Tables\_number 1  
\_symmetry\_cell\_setting triclinic

loop\_

\_atom\_site\_label

\_atom\_site\_type\_symbol

\_atom\_site\_fract\_x

\_atom\_site\_fract\_y

\_atom\_site\_fract\_z

\_atom\_site\_occupancy

|     |   |                    |                    |                    |     |
|-----|---|--------------------|--------------------|--------------------|-----|
| H1  | H | 0.9872108700000000 | 0.0954320100000000 | 0.9871937300000000 | 1.0 |
| H2  | H | 0.9737370400000000 | 0.8871175100000000 | 0.0037504100000000 | 1.0 |
| H3  | H | 0.9848298800000000 | 0.9280364700000000 | 0.8695272800000000 | 1.0 |
| H4  | H | 0.9827206100000000 | 0.0274212600000000 | 0.1173890900000000 | 1.0 |
| H5  | H | 0.0626232200000000 | 0.9567817800000000 | 0.0948914100000000 | 1.0 |
| H6  | H | 0.2382754600000000 | 0.0332203800000000 | 0.0779394000000000 | 1.0 |
| H7  | H | 0.2233779600000000 | 0.9723614800000000 | 0.8776874100000000 | 1.0 |
| H8  | H | 0.2363041300000000 | 0.8626000800000000 | 0.9655657900000000 | 1.0 |
| H9  | H | 0.1486414400000000 | 0.1129558900000000 | 0.9117747000000000 | 1.0 |
| H10 | H | 0.3099518300000000 | 0.0829331600000000 | 0.9095939800000000 | 1.0 |
| H11 | H | 0.4872109600000000 | 0.0954316000000000 | 0.9871943300000000 | 1.0 |
| H12 | H | 0.4737362500000000 | 0.8871171000000000 | 0.0037504000000000 | 1.0 |
| H13 | H | 0.4848299500000000 | 0.9280362600000000 | 0.8695273800000000 | 1.0 |
| H14 | H | 0.4827202400000000 | 0.0274208900000000 | 0.1173887300000000 | 1.0 |
| H15 | H | 0.5626237300000000 | 0.9567817500000000 | 0.0948908800000000 | 1.0 |
| H16 | H | 0.7382755000000000 | 0.0332208400000000 | 0.0779394000000000 | 1.0 |
| H17 | H | 0.7233779100000000 | 0.9723608900000000 | 0.8776876100000000 | 1.0 |
| H18 | H | 0.7363053000000000 | 0.8625998500000000 | 0.9655663600000000 | 1.0 |
| H19 | H | 0.6486424300000000 | 0.1129553300000000 | 0.9117742700000000 | 1.0 |
| H20 | H | 0.8099521800000000 | 0.0829319800000000 | 0.9095940600000000 | 1.0 |
| C21 | C | 0.0120624200000000 | 0.0424784500000000 | 0.9791145500000000 | 1.0 |
| C22 | C | 0.9256021100000000 | 0.9941163700000000 | 0.0237443200000000 | 1.0 |
| C23 | C | 0.9255280700000000 | 0.9298653000000000 | 0.9779477200000000 | 1.0 |
| C24 | C | 0.0114926300000000 | 0.9533930900000000 | 0.9165902600000000 | 1.0 |
| C25 | C | 0.2615364600000000 | 0.0065265100000000 | 0.0314205600000000 | 1.0 |
| C26 | C | 0.1754231400000000 | 0.0306496200000000 | 0.9704508700000000 | 1.0 |
| C27 | C | 0.1751571600000000 | 0.9639117400000000 | 0.9269299500000000 | 1.0 |
| C28 | C | 0.2613798500000000 | 0.9158824800000000 | 0.9716122800000000 | 1.0 |
| C29 | C | 0.5120622300000000 | 0.0424781300000000 | 0.9791145300000000 | 1.0 |
| C30 | C | 0.4256017400000000 | 0.9941159400000000 | 0.0237442600000000 | 1.0 |
| C31 | C | 0.4255276100000000 | 0.9298650400000000 | 0.9779477500000000 | 1.0 |
| C32 | C | 0.5114924000000000 | 0.9533928400000000 | 0.9165903500000000 | 1.0 |
| C33 | C | 0.7615365900000000 | 0.0065266700000000 | 0.0314206300000000 | 1.0 |
| C34 | C | 0.6754228800000000 | 0.0306493200000000 | 0.9704508700000000 | 1.0 |
| C35 | C | 0.6751569100000000 | 0.9639113400000000 | 0.9269301400000000 | 1.0 |
| C36 | C | 0.7613803500000000 | 0.9158824000000000 | 0.9716125300000000 | 1.0 |
| N37 | N | 0.9702195000000000 | 0.9830839700000000 | 0.0928545300000000 | 1.0 |
| N38 | N | 0.2270734100000000 | 0.0930518500000000 | 0.9408253400000000 | 1.0 |
| N39 | N | 0.4702191900000000 | 0.9830834300000000 | 0.0928544500000000 | 1.0 |
| N40 | N | 0.7270737400000000 | 0.0930512800000000 | 0.9408252000000000 | 1.0 |
| O41 | O | 0.9670840000000000 | 0.0230669200000000 | 0.9116764000000000 | 1.0 |
| O42 | O | 0.2166353700000000 | 0.9371364900000000 | 0.0375781200000000 | 1.0 |
| O43 | O | 0.4670839400000000 | 0.0230667300000000 | 0.9116763200000000 | 1.0 |
| O44 | O | 0.7166364000000000 | 0.9371365700000000 | 0.0375784300000000 | 1.0 |

##### cif ends

furan\_NH2\_3\_anti\_dir\_forbid Energy: -274.59510947

##### cif starts

data\_furan\_NH2\_3\_anti\_dir\_forbid

\_publ\_section\_comment

;  
Andrew Reynoso, Bohan Xu, and Vincent H. Crespi  
;

\_cell\_length\_a 10.2230154482

\_cell\_length\_b 20.0

\_cell\_length\_c 20.0

\_cell\_angle\_alpha 90.0

\_cell\_angle\_beta 90.0

\_cell\_angle\_gamma 90.0

\_symmetry\_space\_group\_name\_H-M 'P 1'

\_symmetry\_Int\_Tables\_number 1

\_symmetry\_cell\_setting triclinic

loop\_

\_atom\_site\_label

\_atom\_site\_type\_symbol

\_atom\_site\_fract\_x

\_atom\_site\_fract\_y

\_atom\_site\_fract\_z

\_atom\_site\_occupancy

|     |   |                    |                    |                    |     |
|-----|---|--------------------|--------------------|--------------------|-----|
| H1  | H | 0.0704555300000000 | 0.0974710500000000 | 0.9304147700000000 | 1.0 |
| H2  | H | 0.9559340300000000 | 0.9332488500000000 | 0.0528742100000000 | 1.0 |
| H3  | H | 0.0692235000000000 | 0.8934144000000000 | 0.9314028500000000 | 1.0 |
| H4  | H | 0.9559171500000000 | 0.1204794300000000 | 0.0609381700000000 | 1.0 |
| H5  | H | 0.0229373600000000 | 0.0548625600000000 | 0.0974681100000000 | 1.0 |
| H6  | H | 0.2148608400000000 | 0.0977724900000000 | 0.0328093900000000 | 1.0 |
| H7  | H | 0.3293250300000000 | 0.9327985600000000 | 0.9113558100000000 | 1.0 |
| H8  | H | 0.2160419100000000 | 0.8937154000000000 | 0.0330702800000000 | 1.0 |
| H9  | H | 0.3293942800000000 | 0.1199677600000000 | 0.9021272900000000 | 1.0 |
| H10 | H | 0.2623119700000000 | 0.0541305600000000 | 0.8660214000000000 | 1.0 |
| H11 | H | 0.5701041500000000 | 0.0959142300000000 | 0.9294977000000000 | 1.0 |
| H12 | H | 0.4525133500000000 | 0.9307178900000000 | 0.0499322300000000 | 1.0 |
| H13 | H | 0.5723700300000000 | 0.8923544300000000 | 0.9296376300000000 | 1.0 |
| H14 | H | 0.5354404000000000 | 0.0619307000000000 | 0.0918662000000000 | 1.0 |
| H15 | H | 0.3763722500000000 | 0.0560283100000000 | 0.0923735000000000 | 1.0 |
| H16 | H | 0.7151267500000000 | 0.0962733600000000 | 0.0336412300000000 | 1.0 |
| H17 | H | 0.8328299200000000 | 0.9303111700000000 | 0.9143001500000000 | 1.0 |
| H18 | H | 0.7129849800000000 | 0.8927185400000000 | 0.0348466800000000 | 1.0 |
| H19 | H | 0.7499068900000000 | 0.0612583900000000 | 0.8715381800000000 | 1.0 |
| H20 | H | 0.9089740000000000 | 0.0553487900000000 | 0.8710736000000000 | 1.0 |
| C21 | C | 0.0799111700000000 | 0.0516852900000000 | 0.9603695100000000 | 1.0 |
| C22 | C | 0.9576567100000000 | 0.0357514600000000 | 0.0031595800000000 | 1.0 |
| C23 | C | 0.9577875200000000 | 0.9567345300000000 | 0.0032745800000000 | 1.0 |
| C24 | C | 0.0789436900000000 | 0.9393070500000000 | 0.9613015300000000 | 1.0 |
| C25 | C | 0.2053932400000000 | 0.0518070700000000 | 0.0031327400000000 | 1.0 |
| C26 | C | 0.3276369300000000 | 0.0356016900000000 | 0.9604340600000000 | 1.0 |

|     |   |                    |                    |                    |     |
|-----|---|--------------------|--------------------|--------------------|-----|
| C27 | C | 0.3274991700000000 | 0.9565851000000000 | 0.9608113200000000 | 1.0 |
| C28 | C | 0.2063399300000000 | 0.9394253200000000 | 0.0028910200000000 | 1.0 |
| C29 | C | 0.5802400800000000 | 0.0506566300000000 | 0.9600127000000000 | 1.0 |
| C30 | C | 0.4583834800000000 | 0.0347310700000000 | 0.0025696800000000 | 1.0 |
| C31 | C | 0.4573461400000000 | 0.9551386600000000 | 0.0007996900000000 | 1.0 |
| C32 | C | 0.5800442600000000 | 0.9379312400000000 | 0.9602755200000000 | 1.0 |
| C33 | C | 0.7050451700000000 | 0.0508116000000000 | 0.0034253400000000 | 1.0 |
| C34 | C | 0.8269339700000000 | 0.0346203700000000 | 0.9610040000000000 | 1.0 |
| C35 | C | 0.8279709000000000 | 0.9550409100000000 | 0.9632774400000000 | 1.0 |
| C36 | C | 0.7052721400000000 | 0.9380877200000000 | 0.0039050000000000 | 1.0 |
| N37 | N | 0.9483774300000000 | 0.0699046000000000 | 0.0670462600000000 | 1.0 |
| N38 | N | 0.3368999600000000 | 0.0693545100000000 | 0.8963346300000000 | 1.0 |
| N39 | N | 0.4536758000000000 | 0.0724121000000000 | 0.0643724900000000 | 1.0 |
| N40 | N | 0.8316697000000000 | 0.0719120700000000 | 0.8989674500000000 | 1.0 |
| O41 | O | 0.0870010100000000 | 0.9952070600000000 | 0.9145198800000000 | 1.0 |
| O42 | O | 0.1982851600000000 | 0.9956092100000000 | 0.0493265800000000 | 1.0 |
| O43 | O | 0.5892564500000000 | 0.9941759700000000 | 0.9145823800000000 | 1.0 |
| O44 | O | 0.6960357400000000 | 0.9946338600000000 | 0.0492234600000000 | 1.0 |

##### cif ends

furand\_NH2\_3\_syn\_alt Energy: -274.35207259

##### cif starts

data\_furand\_NH2\_3\_syn\_alt

\_publ\_section\_comment

;  
Andrew Reynoso, Bohan Xu, and Vincent H. Crespi  
;

\_cell\_length\_a 10.3352342651

\_cell\_length\_b 20.0

\_cell\_length\_c 20.0

\_cell\_angle\_alpha 90.0

\_cell\_angle\_beta 90.0

\_cell\_angle\_gamma 90.0

\_symmetry\_space\_group\_name\_H-M 'P 1'

\_symmetry\_Int\_Tables\_number 1

\_symmetry\_cell\_setting triclinic

loop\_

\_atom\_site\_label

\_atom\_site\_type\_symbol

\_atom\_site\_fract\_x

\_atom\_site\_fract\_y

\_atom\_site\_fract\_z

\_atom\_site\_occupancy

|    |   |                    |                    |                    |     |
|----|---|--------------------|--------------------|--------------------|-----|
| H1 | H | 0.9798065800000000 | 0.9468118800000000 | 0.1023525400000000 | 1.0 |
|----|---|--------------------|--------------------|--------------------|-----|

|    |   |                    |                    |                    |     |
|----|---|--------------------|--------------------|--------------------|-----|
| H2 | H | 0.1028331500000000 | 0.0454128200000000 | 0.9256783200000000 | 1.0 |
|----|---|--------------------|--------------------|--------------------|-----|

|    |   |                    |                    |                    |     |
|----|---|--------------------|--------------------|--------------------|-----|
| H3 | H | 0.9761264900000000 | 0.1306622400000000 | 0.0144403700000000 | 1.0 |
|----|---|--------------------|--------------------|--------------------|-----|

|    |   |                    |                    |                    |     |
|----|---|--------------------|--------------------|--------------------|-----|
| H4 | H | 0.1828745900000000 | 0.9095267700000000 | 0.9431477800000000 | 1.0 |
|----|---|--------------------|--------------------|--------------------|-----|

|    |   |                    |                    |                    |     |
|----|---|--------------------|--------------------|--------------------|-----|
| H5 | H | 0.0238625800000000 | 0.9099576700000000 | 0.9424804900000000 | 1.0 |
|----|---|--------------------|--------------------|--------------------|-----|

|    |   |                    |                    |                    |     |
|----|---|--------------------|--------------------|--------------------|-----|
| H6 | H | 0.2297432700000000 | 0.1306675700000000 | 0.0144299700000000 | 1.0 |
|----|---|--------------------|--------------------|--------------------|-----|

|    |   |                    |                    |                    |     |
|----|---|--------------------|--------------------|--------------------|-----|
| H7 | H | 0.3530258400000000 | 0.9312397600000000 | 0.9802922800000000 | 1.0 |
|----|---|--------------------|--------------------|--------------------|-----|

|     |   |                    |                    |                    |     |
|-----|---|--------------------|--------------------|--------------------|-----|
| H8  | H | 0.2261881300000000 | 0.9468440600000000 | 0.1023682100000000 | 1.0 |
| H9  | H | 0.2728614200000000 | 0.0303730200000000 | 0.8854622100000000 | 1.0 |
| H10 | H | 0.4318733300000000 | 0.0291574100000000 | 0.8853491200000000 | 1.0 |
| H11 | H | 0.4798035500000000 | 0.9468166000000000 | 0.1023534400000000 | 1.0 |
| H12 | H | 0.6028382800000000 | 0.0454116500000000 | 0.9256778800000000 | 1.0 |
| H13 | H | 0.4761279100000000 | 0.1306639600000000 | 0.0144353200000000 | 1.0 |
| H14 | H | 0.6828653900000000 | 0.9095268400000000 | 0.9431464500000000 | 1.0 |
| H15 | H | 0.5238538100000000 | 0.9099585100000000 | 0.9424847700000000 | 1.0 |
| H16 | H | 0.7297437100000000 | 0.1306668700000000 | 0.0144312400000000 | 1.0 |
| H17 | H | 0.8530215700000000 | 0.9312382400000000 | 0.9802939200000000 | 1.0 |
| H18 | H | 0.7261839700000000 | 0.9468441000000000 | 0.1023704000000000 | 1.0 |
| H19 | H | 0.7728620000000000 | 0.0303680900000000 | 0.8854653800000000 | 1.0 |
| H20 | H | 0.9318733600000000 | 0.0291536600000000 | 0.8853517200000000 | 1.0 |
| C21 | C | 0.9779640200000000 | 0.9786515600000000 | 0.0576329800000000 | 1.0 |
| C22 | C | 0.1029561800000000 | 0.9731378100000000 | 0.0134939200000000 | 1.0 |
| C23 | C | 0.1029452600000000 | 0.0456522900000000 | 0.9805709400000000 | 1.0 |
| C24 | C | 0.9779672100000000 | 0.0758655400000000 | 0.0111444300000000 | 1.0 |
| C25 | C | 0.2279528000000000 | 0.0758697600000000 | 0.0111122900000000 | 1.0 |
| C26 | C | 0.3529712200000000 | 0.0449698000000000 | 0.9791345700000000 | 1.0 |
| C27 | C | 0.3529681500000000 | 0.9738247600000000 | 0.0149271200000000 | 1.0 |
| C28 | C | 0.2279792900000000 | 0.9786513800000000 | 0.0576235300000000 | 1.0 |
| C29 | C | 0.4779630600000000 | 0.9786544700000000 | 0.0576327400000000 | 1.0 |
| C30 | C | 0.6029556000000000 | 0.9731383300000000 | 0.0134948900000000 | 1.0 |
| C31 | C | 0.6029465700000000 | 0.0456521400000000 | 0.9805700900000000 | 1.0 |
| C32 | C | 0.4779678200000000 | 0.0758669500000000 | 0.0111416100000000 | 1.0 |
| C33 | C | 0.7279527300000000 | 0.0758689400000000 | 0.0111133400000000 | 1.0 |
| C34 | C | 0.8529714300000000 | 0.0449683000000000 | 0.9791367000000000 | 1.0 |
| C35 | C | 0.8529669400000000 | 0.9738235900000000 | 0.0149294100000000 | 1.0 |
| C36 | C | 0.7279780900000000 | 0.9786509300000000 | 0.0576252800000000 | 1.0 |
| N37 | N | 0.1029403000000000 | 0.9129091700000000 | 0.9727513700000000 | 1.0 |
| N38 | N | 0.3530233200000000 | 0.0510568600000000 | 0.9066796600000000 | 1.0 |
| N39 | N | 0.6029368600000000 | 0.9129090400000000 | 0.9727532700000000 | 1.0 |
| N40 | N | 0.8530238300000000 | 0.0510538000000000 | 0.9066815700000000 | 1.0 |
| O41 | O | 0.9779815600000000 | 0.0476830900000000 | 0.0771097600000000 | 1.0 |
| O42 | O | 0.2279811900000000 | 0.0476902500000000 | 0.0770784700000000 | 1.0 |
| O43 | O | 0.4779807600000000 | 0.0476864700000000 | 0.0771075600000000 | 1.0 |
| O44 | O | 0.7279799100000000 | 0.0476900600000000 | 0.0770796700000000 | 1.0 |

##### cif ends

furan\_NH2\_3\_syn\_alt\_forbid Energy: -271.531983

##### cif starts

data\_furan\_NH2\_3\_syn\_alt\_forbid

\_publ\_section\_comment

;  
Andrew Reynoso, Bohan Xu, and Vincent H. Crespi  
;

\_cell\_length\_a 9.5655070801

\_cell\_length\_b 20.0

\_cell\_length\_c 20.0

\_cell\_angle\_alpha 90.0

\_cell\_angle\_beta 90.0

\_cell\_angle\_gamma 90.0

\_symmetry\_space\_group\_name\_H-M 'P 1'

\_symmetry\_Int\_Tables\_number 1

\_symmetry\_cell\_setting triclinic

loop\_

\_atom\_site\_label

\_atom\_site\_type\_symbol

\_atom\_site\_fract\_x

\_atom\_site\_fract\_y

\_atom\_site\_fract\_z

\_atom\_site\_occupancy

|     |   |                    |                    |                    |     |
|-----|---|--------------------|--------------------|--------------------|-----|
| H1  | H | 0.8887806300000000 | 0.1037895100000000 | 0.0621491000000000 | 1.0 |
| H2  | H | 0.9032293200000000 | 0.9289078300000000 | 0.9394187400000000 | 1.0 |
| H3  | H | 0.8992347500000000 | 0.9019088800000000 | 0.0751158300000000 | 1.0 |
| H4  | H | 0.1467259500000000 | 0.0979566200000000 | 0.0727316100000000 | 1.0 |
| H5  | H | 0.1426635400000000 | 0.0676673800000000 | 0.9377335700000000 | 1.0 |
| H6  | H | 0.1571029000000000 | 0.8958153600000000 | 0.0646806700000000 | 1.0 |
| H7  | H | 0.3888198400000000 | 0.1037838600000000 | 0.0621313200000000 | 1.0 |
| H8  | H | 0.4032209300000000 | 0.9288712900000000 | 0.9394385700000000 | 1.0 |
| H9  | H | 0.3991930400000000 | 0.9019047400000000 | 0.0751366200000000 | 1.0 |
| H10 | H | 0.6466835100000000 | 0.0979470400000000 | 0.0727130000000000 | 1.0 |
| H11 | H | 0.6426591200000000 | 0.0676307700000000 | 0.9377154500000000 | 1.0 |
| H12 | H | 0.6571412500000000 | 0.8958059100000000 | 0.0646950400000000 | 1.0 |
| H13 | H | 0.9689309100000000 | 0.0684851800000000 | 0.8797272600000000 | 1.0 |
| H14 | H | 0.4689014000000000 | 0.0684097400000000 | 0.8797038700000000 | 1.0 |
| H15 | H | 0.0769620200000000 | 0.9265522700000000 | 0.8814886800000000 | 1.0 |
| H16 | H | 0.5769314100000000 | 0.9264816600000000 | 0.8815115000000000 | 1.0 |
| H17 | H | 0.8035675700000000 | 0.0533468100000000 | 0.8958327300000000 | 1.0 |
| H18 | H | 0.3035343400000000 | 0.0533131400000000 | 0.8958372600000000 | 1.0 |
| H19 | H | 0.2422666700000000 | 0.9423346200000000 | 0.8971105200000000 | 1.0 |
| H20 | H | 0.7422336100000000 | 0.9422976600000000 | 0.8971061700000000 | 1.0 |
| C21 | C | 0.8527573500000000 | 0.0561546500000000 | 0.0409534100000000 | 1.0 |
| C22 | C | 0.9364999900000000 | 0.0372899700000000 | 0.9765322800000000 | 1.0 |
| C23 | C | 0.9436675400000000 | 0.9582384400000000 | 0.9814545200000000 | 1.0 |
| C24 | C | 0.8631917600000000 | 0.9451906300000000 | 0.0461148000000000 | 1.0 |
| C25 | C | 0.1827382000000000 | 0.0539775200000000 | 0.0447896600000000 | 1.0 |
| C26 | C | 0.1022551900000000 | 0.0393618200000000 | 0.9804711800000000 | 1.0 |
| C27 | C | 0.1094292100000000 | 0.9602144900000000 | 0.9774648100000000 | 1.0 |
| C28 | C | 0.1931384000000000 | 0.9429210100000000 | 0.0423353000000000 | 1.0 |
| C29 | C | 0.3527701400000000 | 0.0561475500000000 | 0.0409476000000000 | 1.0 |
| C30 | C | 0.4364976000000000 | 0.0372643700000000 | 0.9765248300000000 | 1.0 |
| C31 | C | 0.4436650200000000 | 0.9582132400000000 | 0.9814647100000000 | 1.0 |
| C32 | C | 0.3631791500000000 | 0.9451840800000000 | 0.0461254000000000 | 1.0 |
| C33 | C | 0.6827235800000000 | 0.0539686300000000 | 0.0447810000000000 | 1.0 |
| C34 | C | 0.6022526100000000 | 0.0393352700000000 | 0.9804607600000000 | 1.0 |
| C35 | C | 0.6094260100000000 | 0.9601880200000000 | 0.9774709600000000 | 1.0 |
| C36 | C | 0.6931504600000000 | 0.9429118300000000 | 0.0423392000000000 | 1.0 |
| N37 | N | 0.8936976000000000 | 0.0717659100000000 | 0.9156992600000000 | 1.0 |
| N38 | N | 0.1522964400000000 | 0.9242851600000000 | 0.9174861400000000 | 1.0 |
| N39 | N | 0.3936921600000000 | 0.0717243600000000 | 0.9156839300000000 | 1.0 |
| N40 | N | 0.6522862500000000 | 0.9242431100000000 | 0.9175006600000000 | 1.0 |
| O41 | O | 0.8923273700000000 | 0.0038176500000000 | 0.0852620800000000 | 1.0 |
| O42 | O | 0.1535587000000000 | 0.9963243700000000 | 0.0853515200000000 | 1.0 |
| O43 | O | 0.3923298600000000 | 0.0038158100000000 | 0.0852637600000000 | 1.0 |

O44 O 0.6535601700000000 0.9963169200000000 0.0853486100000000 1.0

##### cif ends

furam\_NH2\_3\_syn\_dir Energy: -273.99207534

##### cif starts

data\_furam\_NH2\_3\_syn\_dir

\_publ\_section\_comment

;  
Andrew Reynoso, Bohan Xu, and Vincent H. Crespi  
;

\_cell\_length\_a 10.4822739223

\_cell\_length\_b 20.0

\_cell\_length\_c 20.0

\_cell\_angle\_alpha 90.0

\_cell\_angle\_beta 90.0

\_cell\_angle\_gamma 90.0

\_symmetry\_space\_group\_name\_H-M 'P 1'

\_symmetry\_Int\_Tables\_number 1

\_symmetry\_cell\_setting triclinic

loop\_

\_atom\_site\_label

\_atom\_site\_type\_symbol

\_atom\_site\_fract\_x

\_atom\_site\_fract\_y

\_atom\_site\_fract\_z

\_atom\_site\_occupancy

|     |   |                    |                    |                    |     |
|-----|---|--------------------|--------------------|--------------------|-----|
| H1  | H | 0.0295403600000000 | 0.0319860200000000 | 0.1015341700000000 | 1.0 |
| H2  | H | 0.1544986200000000 | 0.9602988200000000 | 0.9135175000000000 | 1.0 |
| H3  | H | 0.0294395400000000 | 0.8618736300000000 | 0.9900259100000000 | 1.0 |
| H4  | H | 0.1660277700000000 | 0.1191272300000000 | 0.0021040600000000 | 1.0 |
| H5  | H | 0.0690579900000000 | 0.0841373200000000 | 0.9485498200000000 | 1.0 |
| H6  | H | 0.2795369600000000 | 0.0319882000000000 | 0.1015328200000000 | 1.0 |
| H7  | H | 0.4044901600000000 | 0.9603001200000000 | 0.9135160300000000 | 1.0 |
| H8  | H | 0.2794410000000000 | 0.8618733100000000 | 0.9900284900000000 | 1.0 |
| H9  | H | 0.4160511100000000 | 0.1191279000000000 | 0.0021113600000000 | 1.0 |
| H10 | H | 0.3190580500000000 | 0.0841472400000000 | 0.9485584500000000 | 1.0 |
| H11 | H | 0.5295416800000000 | 0.0319840100000000 | 0.1015328100000000 | 1.0 |
| H12 | H | 0.6545056000000000 | 0.9602982400000000 | 0.9135159700000000 | 1.0 |
| H13 | H | 0.5294400800000000 | 0.8618735600000000 | 0.9900212100000000 | 1.0 |
| H14 | H | 0.6660237500000000 | 0.1191271800000000 | 0.0021010500000000 | 1.0 |
| H15 | H | 0.5690581500000000 | 0.0841358200000000 | 0.9485463000000000 | 1.0 |
| H16 | H | 0.7795330000000000 | 0.0319905000000000 | 0.1015318900000000 | 1.0 |
| H17 | H | 0.9044933300000000 | 0.9602996800000000 | 0.9135179100000000 | 1.0 |
| H18 | H | 0.7794420600000000 | 0.8618734200000000 | 0.9900307600000000 | 1.0 |
| H19 | H | 0.9160507800000000 | 0.1191283400000000 | 0.0021127000000000 | 1.0 |
| H20 | H | 0.8190598600000000 | 0.0841477500000000 | 0.9485584700000000 | 1.0 |
| C21 | C | 0.0295045200000000 | 0.0062025600000000 | 0.0529323900000000 | 1.0 |
| C22 | C | 0.1548932900000000 | 0.0175698500000000 | 0.0101176000000000 | 1.0 |
| C23 | C | 0.1544630600000000 | 0.9510228000000000 | 0.9676857100000000 | 1.0 |
| C24 | C | 0.0294625400000000 | 0.9166929800000000 | 0.9937039900000000 | 1.0 |



|     |   |                    |                    |                    |     |
|-----|---|--------------------|--------------------|--------------------|-----|
| C25 | C | 0.2795041800000000 | 0.0062035600000000 | 0.0529317200000000 | 1.0 |
| C26 | C | 0.4048930200000000 | 0.0175705900000000 | 0.0101180300000000 | 1.0 |
| C27 | C | 0.4044617400000000 | 0.9510238700000000 | 0.9676841900000000 | 1.0 |
| C28 | C | 0.2794630100000000 | 0.9166928000000000 | 0.9937049400000000 | 1.0 |
| C29 | C | 0.5295049300000000 | 0.0062015600000000 | 0.0529304900000000 | 1.0 |
| C30 | C | 0.6548933900000000 | 0.0175697800000000 | 0.0101158500000000 | 1.0 |
| C31 | C | 0.6544653100000000 | 0.9510226000000000 | 0.9676842500000000 | 1.0 |
| C32 | C | 0.5294630100000000 | 0.9166928300000000 | 0.9937008000000000 | 1.0 |
| C33 | C | 0.7795028400000000 | 0.0062046600000000 | 0.0529314200000000 | 1.0 |
| C34 | C | 0.9048926400000000 | 0.0175711500000000 | 0.0101192400000000 | 1.0 |
| C35 | C | 0.9044625100000000 | 0.9510238200000000 | 0.9676861400000000 | 1.0 |
| C36 | C | 0.7794634400000000 | 0.9166929700000000 | 0.9937061200000000 | 1.0 |
| N37 | N | 0.1584293100000000 | 0.0790956000000000 | 0.9703354700000000 | 1.0 |
| N38 | N | 0.4084310800000000 | 0.0790992400000000 | 0.9703406000000000 | 1.0 |
| N39 | N | 0.6584288700000000 | 0.0790950700000000 | 0.9703328800000000 | 1.0 |
| N40 | N | 0.9084317900000000 | 0.0790997800000000 | 0.9703417800000000 | 1.0 |
| O41 | O | 0.0291870600000000 | 0.9355148900000000 | 0.0633659200000000 | 1.0 |
| O42 | O | 0.2791876000000000 | 0.9355159100000000 | 0.0633665000000000 | 1.0 |
| O43 | O | 0.5291870700000000 | 0.9355136100000000 | 0.0633628900000000 | 1.0 |
| O44 | O | 0.7791859500000000 | 0.9355172300000000 | 0.0633673800000000 | 1.0 |

##### cif ends

furan\_NH2\_3\_syn\_dir\_forbid Energy: -271.21315485

##### cif starts

data\_furan\_NH2\_3\_syn\_dir\_forbid

\_publ\_section\_comment

;  
Andrew Reynoso, Bohan Xu, and Vincent H. Crespi  
;

\_cell\_length\_a 9.5114045397

\_cell\_length\_b 20.0

\_cell\_length\_c 20.0

\_cell\_angle\_alpha 90.0

\_cell\_angle\_beta 90.0

\_cell\_angle\_gamma 90.0

\_symmetry\_space\_group\_name\_H-M 'P 1'

\_symmetry\_Int\_Tables\_number 1

\_symmetry\_cell\_setting triclinic

loop\_

\_atom\_site\_label

\_atom\_site\_type\_symbol

\_atom\_site\_fract\_x

\_atom\_site\_fract\_y

\_atom\_site\_fract\_z

\_atom\_site\_occupancy

|    |   |                    |                    |                    |     |
|----|---|--------------------|--------------------|--------------------|-----|
| H1 | H | 0.8692007700000000 | 0.1198276200000000 | 0.0567935000000000 | 1.0 |
|----|---|--------------------|--------------------|--------------------|-----|

|    |   |                    |                    |                    |     |
|----|---|--------------------|--------------------|--------------------|-----|
| H2 | H | 0.8871460900000000 | 0.9496422300000000 | 0.9353098900000000 | 1.0 |
|----|---|--------------------|--------------------|--------------------|-----|

|    |   |                    |                    |                    |     |
|----|---|--------------------|--------------------|--------------------|-----|
| H3 | H | 0.9180620500000000 | 0.9196463300000000 | 0.0751693600000000 | 1.0 |
|----|---|--------------------|--------------------|--------------------|-----|

|    |   |                    |                    |                    |     |
|----|---|--------------------|--------------------|--------------------|-----|
| H4 | H | 0.1721457100000000 | 0.0774679500000000 | 0.0948863000000000 | 1.0 |
|----|---|--------------------|--------------------|--------------------|-----|

|    |   |                    |                    |                    |     |
|----|---|--------------------|--------------------|--------------------|-----|
| H5 | H | 0.1380516300000000 | 0.9597431300000000 | 0.9169348700000000 | 1.0 |
|----|---|--------------------|--------------------|--------------------|-----|

|     |   |                    |                    |                    |     |
|-----|---|--------------------|--------------------|--------------------|-----|
| H6  | H | 0.1375370600000000 | 0.8856219300000000 | 0.0333417200000000 | 1.0 |
| H7  | H | 0.4128819600000000 | 0.0785906500000000 | 0.0647127000000000 | 1.0 |
| H8  | H | 0.4277842900000000 | 0.9136092200000000 | 0.9299593200000000 | 1.0 |
| H9  | H | 0.3743906000000000 | 0.8776149500000000 | 0.0602680200000000 | 1.0 |
| H10 | H | 0.6283072300000000 | 0.1077132800000000 | 0.0407060500000000 | 1.0 |
| H11 | H | 0.6754453900000000 | 0.9188144100000000 | 0.9460205600000000 | 1.0 |
| H12 | H | 0.6735280700000000 | 0.9116970100000000 | 0.0860623000000000 | 1.0 |
| H13 | H | 0.9682898800000000 | 0.0685624500000000 | 0.8764781400000000 | 1.0 |
| H14 | H | 0.0888244400000000 | 0.1356696400000000 | 0.9346710300000000 | 1.0 |
| H15 | H | 0.3403893800000000 | 0.0000114600000000 | 0.8793101000000000 | 1.0 |
| H16 | H | 0.6888449300000000 | 0.0095134100000000 | 0.8735522500000000 | 1.0 |
| H17 | H | 0.2979896300000000 | 0.0747058400000000 | 0.9127127600000000 | 1.0 |
| H18 | H | 0.5516359400000000 | 0.0596649100000000 | 0.8778820700000000 | 1.0 |
| H19 | H | 0.8120149900000000 | 0.0898935400000000 | 0.9057198100000000 | 1.0 |
| H20 | H | 0.2185856700000000 | 0.1403924000000000 | 0.9910268700000000 | 1.0 |
| C21 | C | 0.8481366700000000 | 0.0702611400000000 | 0.0353320800000000 | 1.0 |
| C22 | C | 0.9435587400000000 | 0.0521223000000000 | 0.9770295400000000 | 1.0 |
| C23 | C | 0.9416104900000000 | 0.9739051400000000 | 0.9771651500000000 | 1.0 |
| C24 | C | 0.8694235200000000 | 0.9601888600000000 | 0.0464539300000000 | 1.0 |
| C25 | C | 0.1908649500000000 | 0.0406462200000000 | 0.0551288200000000 | 1.0 |
| C26 | C | 0.1098782700000000 | 0.0515602900000000 | 0.9897862800000000 | 1.0 |
| C27 | C | 0.1086396200000000 | 0.9729174200000000 | 0.9683357400000000 | 1.0 |
| C28 | C | 0.1870497700000000 | 0.9346414700000000 | 0.0250221400000000 | 1.0 |
| C29 | C | 0.3619458000000000 | 0.0355182800000000 | 0.0409615100000000 | 1.0 |
| C30 | C | 0.4345982200000000 | 0.0177384800000000 | 0.9696542900000000 | 1.0 |
| C31 | C | 0.4533822500000000 | 0.9410045400000000 | 0.9761200000000000 | 1.0 |
| C32 | C | 0.3562671600000000 | 0.9254769100000000 | 0.0346576500000000 | 1.0 |
| C33 | C | 0.6798587300000000 | 0.0601346400000000 | 0.0281315400000000 | 1.0 |
| C34 | C | 0.6086623800000000 | 0.0254499000000000 | 0.9670355900000000 | 1.0 |
| C35 | C | 0.6196098200000000 | 0.9490233600000000 | 0.9834854200000000 | 1.0 |
| C36 | C | 0.6983638200000000 | 0.9517725100000000 | 0.0505005800000000 | 1.0 |
| N37 | N | 0.9189952200000000 | 0.0903673300000000 | 0.9164040300000000 | 1.0 |
| N38 | N | 0.1707377600000000 | 0.1101308200000000 | 0.9568656400000000 | 1.0 |
| N39 | N | 0.3770595600000000 | 0.0392835600000000 | 0.9065174200000000 | 1.0 |
| N40 | N | 0.6474822800000000 | 0.0480898000000000 | 0.9006301100000000 | 1.0 |
| O41 | O | 0.8926209100000000 | 0.0212623600000000 | 0.0830096600000000 | 1.0 |
| O42 | O | 0.1520681800000000 | 0.9768843600000000 | 0.0805531200000000 | 1.0 |
| O43 | O | 0.3956388600000000 | 0.9775415300000000 | 0.0798034400000000 | 1.0 |
| O44 | O | 0.6498494100000000 | 0.0132658100000000 | 0.0799614300000000 | 1.0 |

##### cif ends

furand\_OH\_234\_anti\_alt    Energy: -307.07134706

##### cif starts

data\_furand\_OH\_234\_anti\_alt

\_publ\_section\_comment

;  
Andrew Reynoso, Bohan Xu, and Vincent H. Crespi  
;

\_cell\_length\_a    9.4939371627

\_cell\_length\_b    20.0

\_cell\_length\_c    20.0

\_cell\_angle\_alpha    90.0

\_cell\_angle\_beta 90.0  
\_cell\_angle\_gamma 90.0

\_symmetry\_space\_group\_name H-M 'P 1'  
\_symmetry\_Int\_Tables\_number 1  
\_symmetry\_cell\_setting triclinic

loop\_

\_atom\_site\_label  
\_atom\_site\_type\_symbol  
\_atom\_site\_fract\_x  
\_atom\_site\_fract\_y  
\_atom\_site\_fract\_z  
\_atom\_site\_occupancy

|     |   |                    |                    |                    |     |
|-----|---|--------------------|--------------------|--------------------|-----|
| H1  | H | 0.9821860200000000 | 0.1024086000000000 | 0.9215591100000000 | 1.0 |
| H2  | H | 0.8733670700000000 | 0.8862522400000000 | 0.9251077700000000 | 1.0 |
| H3  | H | 0.8890142200000000 | 0.1186257000000000 | 0.0836834800000000 | 1.0 |
| H4  | H | 0.0367078300000000 | 0.9815887000000000 | 0.1035366000000000 | 1.0 |
| H5  | H | 0.2322069900000000 | 0.9108293600000000 | 0.0588397600000000 | 1.0 |
| H6  | H | 0.1233401400000000 | 0.1269823300000000 | 0.0553317500000000 | 1.0 |
| H7  | H | 0.1390187400000000 | 0.8946530300000000 | 0.8967135000000000 | 1.0 |
| H8  | H | 0.2866453100000000 | 0.0316538400000000 | 0.8768652700000000 | 1.0 |
| H9  | H | 0.4821872100000000 | 0.1024189800000000 | 0.9215697000000000 | 1.0 |
| H10 | H | 0.3733663400000000 | 0.8862634600000000 | 0.9250902900000000 | 1.0 |
| H11 | H | 0.3890045500000000 | 0.1186086300000000 | 0.0836998000000000 | 1.0 |
| H12 | H | 0.5366311000000000 | 0.9816149000000000 | 0.1035556500000000 | 1.0 |
| H13 | H | 0.7321835000000000 | 0.9108427800000000 | 0.0588508800000000 | 1.0 |
| H14 | H | 0.6233536800000000 | 0.1269937000000000 | 0.0553253100000000 | 1.0 |
| H15 | H | 0.6390248200000000 | 0.8946624600000000 | 0.8967067400000000 | 1.0 |
| H16 | H | 0.7866085700000000 | 0.0316421500000000 | 0.8768537800000000 | 1.0 |
| C17 | C | 0.0000659000000000 | 0.9484711900000000 | 0.9646084900000000 | 1.0 |
| C18 | C | 0.9150222000000000 | 0.9717638700000000 | 0.0268076100000000 | 1.0 |
| C19 | C | 0.9145421400000000 | 0.0507332300000000 | 0.0161094200000000 | 1.0 |
| C20 | C | 0.0022303500000000 | 0.0573950700000000 | 0.9511785700000000 | 1.0 |
| C21 | C | 0.2500575300000000 | 0.0647777900000000 | 0.0158153500000000 | 1.0 |
| C22 | C | 0.1650129900000000 | 0.0414908800000000 | 0.9536123300000000 | 1.0 |
| C23 | C | 0.1645490200000000 | 0.9625248100000000 | 0.9643055700000000 | 1.0 |
| C24 | C | 0.2522447800000000 | 0.9558504700000000 | 0.0292305000000000 | 1.0 |
| C25 | C | 0.5000682800000000 | 0.9484746500000000 | 0.9646025500000000 | 1.0 |
| C26 | C | 0.4150249300000000 | 0.9717610500000000 | 0.0268024200000000 | 1.0 |
| C27 | C | 0.4145415900000000 | 0.0507304600000000 | 0.0161123900000000 | 1.0 |
| C28 | C | 0.5022321000000000 | 0.0574003400000000 | 0.9511828800000000 | 1.0 |
| C29 | C | 0.7500609400000000 | 0.0647827900000000 | 0.0158105200000000 | 1.0 |
| C30 | C | 0.6650135600000000 | 0.0414939900000000 | 0.9536114900000000 | 1.0 |
| C31 | C | 0.6645492200000000 | 0.9625282700000000 | 0.9643065500000000 | 1.0 |
| C32 | C | 0.7522369100000000 | 0.9558579600000000 | 0.0292365900000000 | 1.0 |
| O33 | O | 0.9563465300000000 | 0.9988807500000000 | 0.9151092500000000 | 1.0 |
| O34 | O | 0.9738600200000000 | 0.8849701800000000 | 0.9405135600000000 | 1.0 |
| O35 | O | 0.9647945900000000 | 0.9494164100000000 | 0.0889986000000000 | 1.0 |
| O36 | O | 0.9681135100000000 | 0.0890990500000000 | 0.0705745600000000 | 1.0 |
| O37 | O | 0.2063527400000000 | 0.0143566000000000 | 0.0653057000000000 | 1.0 |
| O38 | O | 0.2238393400000000 | 0.1282680300000000 | 0.0399293900000000 | 1.0 |
| O39 | O | 0.2147695300000000 | 0.0638362700000000 | 0.8914210700000000 | 1.0 |
| O40 | O | 0.2181175000000000 | 0.9241702000000000 | 0.9098352700000000 | 1.0 |
| O41 | O | 0.4563502700000000 | 0.9988895900000000 | 0.9151072700000000 | 1.0 |

|     |   |                    |                    |                    |     |
|-----|---|--------------------|--------------------|--------------------|-----|
| O42 | O | 0.4738588200000000 | 0.8849778200000000 | 0.9404970300000000 | 1.0 |
| O43 | O | 0.4648050100000000 | 0.9494124000000000 | 0.0889923300000000 | 1.0 |
| O44 | O | 0.4681122400000000 | 0.0890902500000000 | 0.0705816400000000 | 1.0 |
| O45 | O | 0.7063494100000000 | 0.0143695200000000 | 0.0653043400000000 | 1.0 |
| O46 | O | 0.7238422000000000 | 0.1282783400000000 | 0.0399156700000000 | 1.0 |
| O47 | O | 0.7147645400000000 | 0.0638356100000000 | 0.8914175200000000 | 1.0 |
| O48 | O | 0.7181291200000000 | 0.9241736700000000 | 0.9098393700000000 | 1.0 |

##### cif ends

furan\_OH\_234\_anti\_alt\_forbid Energy: -307.41447632

##### cif starts

data\_furan\_OH\_234\_anti\_alt\_forbid

\_publ\_section\_comment

;  
Andrew Reynoso, Bohan Xu, and Vincent H. Crespi  
;

\_cell\_length\_a 10.2041665247

\_cell\_length\_b 20.0

\_cell\_length\_c 20.0

\_cell\_angle\_alpha 90.0

\_cell\_angle\_beta 90.0

\_cell\_angle\_gamma 90.0

\_symmetry\_space\_group\_name\_H-M 'P 1'

\_symmetry\_Int\_Tables\_number 1

\_symmetry\_cell\_setting triclinic

loop\_

\_atom\_site\_label

\_atom\_site\_type\_symbol

\_atom\_site\_fract\_x

\_atom\_site\_fract\_y

\_atom\_site\_fract\_z

\_atom\_site\_occupancy

|     |   |                    |                    |                    |     |
|-----|---|--------------------|--------------------|--------------------|-----|
| H1  | H | 0.0657391300000000 | 0.0990290400000000 | 0.9372935900000000 | 1.0 |
| H2  | H | 0.2114904900000000 | 0.8898515600000000 | 0.0318492800000000 | 1.0 |
| H3  | H | 0.5656803800000000 | 0.0990357000000000 | 0.9372180200000000 | 1.0 |
| H4  | H | 0.7114039700000000 | 0.8898837700000000 | 0.0318397700000000 | 1.0 |
| H5  | H | 0.0331405300000000 | 0.0821983100000000 | 0.0822766100000000 | 1.0 |
| H6  | H | 0.2886669000000000 | 0.1052386500000000 | 0.0727301000000000 | 1.0 |
| H7  | H | 0.5332837100000000 | 0.0821846600000000 | 0.0822454800000000 | 1.0 |
| H8  | H | 0.7887306300000000 | 0.1052805300000000 | 0.0726102500000000 | 1.0 |
| H9  | H | 0.3412483400000000 | 0.0394415900000000 | 0.8695189100000000 | 1.0 |
| H10 | H | 0.8421920100000000 | 0.0394482400000000 | 0.8695093000000000 | 1.0 |
| H11 | H | 0.9884967100000000 | 0.8836453800000000 | 0.8964439600000000 | 1.0 |
| H12 | H | 0.2439297600000000 | 0.9067769200000000 | 0.8868107900000000 | 1.0 |
| H13 | H | 0.4885189000000000 | 0.8836923400000000 | 0.8963641800000000 | 1.0 |
| H14 | H | 0.7439658900000000 | 0.9067284300000000 | 0.8868099000000000 | 1.0 |
| H15 | H | 0.9351083100000000 | 0.9493860600000000 | 0.0995885100000000 | 1.0 |
| H16 | H | 0.4356769700000000 | 0.9494476400000000 | 0.0995971100000000 | 1.0 |
| C17 | C | 0.0752143100000000 | 0.0521564000000000 | 0.9651685800000000 | 1.0 |
| C18 | C | 0.9539508400000000 | 0.0332976200000000 | 0.0070640900000000 | 1.0 |

|     |   |                    |                    |                    |     |
|-----|---|--------------------|--------------------|--------------------|-----|
| C19 | C | 0.9533689100000000 | 0.9535261100000000 | 0.0038163400000000 | 1.0 |
| C20 | C | 0.0763396700000000 | 0.9383649200000000 | 0.9606729200000000 | 1.0 |
| C21 | C | 0.2008097200000000 | 0.0505102400000000 | 0.0085067400000000 | 1.0 |
| C22 | C | 0.3237385600000000 | 0.0353697400000000 | 0.9653249800000000 | 1.0 |
| C23 | C | 0.3231782000000000 | 0.9556150800000000 | 0.9620478200000000 | 1.0 |
| C24 | C | 0.2019544000000000 | 0.9367263200000000 | 0.0039815400000000 | 1.0 |
| C25 | C | 0.5752006400000000 | 0.0521701500000000 | 0.9651022100000000 | 1.0 |
| C26 | C | 0.4539790200000000 | 0.0333125500000000 | 0.0070479800000000 | 1.0 |
| C27 | C | 0.4533971800000000 | 0.9535429500000000 | 0.0037950800000000 | 1.0 |
| C28 | C | 0.5763316700000000 | 0.9383883600000000 | 0.9606244400000000 | 1.0 |
| C29 | C | 0.7008248700000000 | 0.0505400400000000 | 0.0084168800000000 | 1.0 |
| C30 | C | 0.8237781400000000 | 0.0353553800000000 | 0.9652706700000000 | 1.0 |
| C31 | C | 0.8231912400000000 | 0.9555941300000000 | 0.9620308900000000 | 1.0 |
| C32 | C | 0.7019322000000000 | 0.9367442800000000 | 0.0039445900000000 | 1.0 |
| O33 | O | 0.9507365700000000 | 0.9171939300000000 | 0.0636081500000000 | 1.0 |
| O34 | O | 0.0746623400000000 | 0.8823412300000000 | 0.9192828400000000 | 1.0 |
| O35 | O | 0.9465580000000000 | 0.0629927000000000 | 0.0714590900000000 | 1.0 |
| O36 | O | 0.3262723800000000 | 0.0716862100000000 | 0.9055257000000000 | 1.0 |
| O37 | O | 0.2024924700000000 | 0.1065353000000000 | 0.0499021400000000 | 1.0 |
| O38 | O | 0.3305027500000000 | 0.9260045500000000 | 0.8976080000000000 | 1.0 |
| O39 | O | 0.0830758100000000 | 0.9978184900000000 | 0.9182397900000000 | 1.0 |
| O40 | O | 0.1940911100000000 | 0.9910515900000000 | 0.0509196300000000 | 1.0 |
| O41 | O | 0.4508112400000000 | 0.9172173200000000 | 0.0635945500000000 | 1.0 |
| O42 | O | 0.5746447400000000 | 0.8823596000000000 | 0.9192355400000000 | 1.0 |
| O43 | O | 0.4466799400000000 | 0.0629913100000000 | 0.0714528500000000 | 1.0 |
| O44 | O | 0.8263872700000000 | 0.0716499400000000 | 0.9054618000000000 | 1.0 |
| O45 | O | 0.7025422500000000 | 0.1065800900000000 | 0.0497875200000000 | 1.0 |
| O46 | O | 0.8305604500000000 | 0.9259220300000000 | 0.8976225000000000 | 1.0 |
| O47 | O | 0.5830481800000000 | 0.9978254400000000 | 0.9181899000000000 | 1.0 |
| O48 | O | 0.6940863600000000 | 0.9910934100000000 | 0.0508622000000000 | 1.0 |

##### cif ends

furan\_OH\_234\_anti\_dir Energy: -306.4253078

##### cif starts

data\_furan\_OH\_234\_anti\_dir

\_publ\_section\_comment

;  
Andrew Reynoso, Bohan Xu, and Vincent H. Crespi  
;

\_cell\_length\_a 9.5632564062

\_cell\_length\_b 20.0

\_cell\_length\_c 20.0

\_cell\_angle\_alpha 90.0

\_cell\_angle\_beta 90.0

\_cell\_angle\_gamma 90.0

\_symmetry\_space\_group\_name\_H-M 'P 1'

\_symmetry\_Int\_Tables\_number 1

\_symmetry\_cell\_setting triclinic

loop\_

\_atom\_site\_label

|     | _atom_site_type_symbol | _atom_site_fract_x | _atom_site_fract_y | _atom_site_fract_z | _atom_site_occupancy |
|-----|------------------------|--------------------|--------------------|--------------------|----------------------|
| H1  | H                      | 0.9643782700000000 | 0.8894622500000000 | 0.9403802900000000 | 1.0                  |
| H2  | H                      | 0.0418238900000000 | 0.1146985000000000 | 0.9016708000000000 | 1.0                  |
| H3  | H                      | 0.9925850000000000 | 0.9611737700000000 | 0.1126403000000000 | 1.0                  |
| H4  | H                      | 0.0390322000000000 | 0.0846475500000000 | 0.0834818400000000 | 1.0                  |
| H5  | H                      | 0.2235445700000000 | 0.8824334500000000 | 0.0469415800000000 | 1.0                  |
| H6  | H                      | 0.2915921800000000 | 0.1070903900000000 | 0.0966889000000000 | 1.0                  |
| H7  | H                      | 0.1403116900000000 | 0.9321206700000000 | 0.8694432600000000 | 1.0                  |
| H8  | H                      | 0.2859709300000000 | 0.0292786500000000 | 0.8926252500000000 | 1.0                  |
| H9  | H                      | 0.4747360400000000 | 0.8926002900000000 | 0.9294665100000000 | 1.0                  |
| H10 | H                      | 0.3678304000000000 | 0.1178345700000000 | 0.9378082200000000 | 1.0                  |
| H11 | H                      | 0.4191638000000000 | 0.9268238600000000 | 0.1172529100000000 | 1.0                  |
| H12 | H                      | 0.5471228000000000 | 0.0292782100000000 | 0.0989054600000000 | 1.0                  |
| H13 | H                      | 0.7149874900000000 | 0.8936469600000000 | 0.0541055700000000 | 1.0                  |
| H14 | H                      | 0.6295864800000000 | 0.1291616400000000 | 0.0388209200000000 | 1.0                  |
| H15 | H                      | 0.7478124400000000 | 0.9630189300000000 | 0.8782157400000000 | 1.0                  |
| H16 | H                      | 0.7862103300000000 | 0.0864002400000000 | 0.9073171900000000 | 1.0                  |
| C17 | C                      | 0.9962389000000000 | 0.0467529800000000 | 0.9647143000000000 | 1.0                  |
| C18 | C                      | 0.9065797200000000 | 0.0326960000000000 | 0.0275636300000000 | 1.0                  |
| C19 | C                      | 0.9015880000000000 | 0.9532363200000000 | 0.0275545800000000 | 1.0                  |
| C20 | C                      | 0.9894382800000000 | 0.9370994400000000 | 0.9645481100000000 | 1.0                  |
| C21 | C                      | 0.2456774400000000 | 0.0409180100000000 | 0.0318701700000000 | 1.0                  |
| C22 | C                      | 0.1578238000000000 | 0.0291544300000000 | 0.9677098600000000 | 1.0                  |
| C23 | C                      | 0.1525926300000000 | 0.9498709500000000 | 0.9649062100000000 | 1.0                  |
| C24 | C                      | 0.2438668200000000 | 0.9317293000000000 | 0.0252847900000000 | 1.0                  |
| C25 | C                      | 0.4938832400000000 | 0.0482513600000000 | 0.9657711900000000 | 1.0                  |
| C26 | C                      | 0.4083630300000000 | 0.0256360800000000 | 0.0286541300000000 | 1.0                  |
| C27 | C                      | 0.4063790900000000 | 0.9468703300000000 | 0.0223256500000000 | 1.0                  |
| C28 | C                      | 0.4932547500000000 | 0.9382724100000000 | 0.9580977000000000 | 1.0                  |
| C29 | C                      | 0.7450519000000000 | 0.0510681400000000 | 0.0249589500000000 | 1.0                  |
| C30 | C                      | 0.6571869000000000 | 0.0329501500000000 | 0.9622796400000000 | 1.0                  |
| C31 | C                      | 0.6553748500000000 | 0.9537014600000000 | 0.9627822000000000 | 1.0                  |
| C32 | C                      | 0.7386294000000000 | 0.9402591700000000 | 0.0280574600000000 | 1.0                  |
| O33 | O                      | 0.9517821800000000 | 0.9919778300000000 | 0.9206736000000000 | 1.0                  |
| O34 | O                      | 0.9680267500000000 | 0.1079211400000000 | 0.9352883300000000 | 1.0                  |
| O35 | O                      | 0.9543275600000000 | 0.0572340700000000 | 0.0891107400000000 | 1.0                  |
| O36 | O                      | 0.9515558600000000 | 0.9241191300000000 | 0.0868880000000000 | 1.0                  |
| O37 | O                      | 0.2033397500000000 | 0.9834257000000000 | 0.0723584300000000 | 1.0                  |
| O38 | O                      | 0.2165923300000000 | 0.1010319900000000 | 0.0633707500000000 | 1.0                  |
| O39 | O                      | 0.2124049700000000 | 0.0602608100000000 | 0.9094671100000000 | 1.0                  |
| O40 | O                      | 0.2066493900000000 | 0.9219750600000000 | 0.9051933900000000 | 1.0                  |
| O41 | O                      | 0.4489337500000000 | 0.9958814200000000 | 0.9185215200000000 | 1.0                  |
| O42 | O                      | 0.4692266600000000 | 0.1126966700000000 | 0.9444266900000000 | 1.0                  |
| O43 | O                      | 0.4554349100000000 | 0.0513771400000000 | 0.0903730800000000 | 1.0                  |
| O44 | O                      | 0.4670278400000000 | 0.9120696200000000 | 0.0766862400000000 | 1.0                  |
| O45 | O                      | 0.6969734400000000 | 0.9966441500000000 | 0.0700156500000000 | 1.0                  |
| O46 | O                      | 0.7234424800000000 | 0.1138906100000000 | 0.0507001500000000 | 1.0                  |
| O47 | O                      | 0.7023237200000000 | 0.0587588600000000 | 0.9006406600000000 | 1.0                  |
| O48 | O                      | 0.7128533200000000 | 0.9249716200000000 | 0.9045798800000000 | 1.0                  |

##### cif ends

furandiol\_234\_anti\_dir\_forbid Energy: -307.23987299

##### cif starts

data\_furandiol\_234\_anti\_dir\_forbid

\_publ\_section\_comment

;  
Andrew Reynoso, Bohan Xu, and Vincent H. Crespi  
;

\_cell\_length\_a 10.2129597849

\_cell\_length\_b 20.0

\_cell\_length\_c 20.0

\_cell\_angle\_alpha 90.0

\_cell\_angle\_beta 90.0

\_cell\_angle\_gamma 90.0

\_symmetry\_space\_group\_name\_H-M 'P 1'

\_symmetry\_Int\_Tables\_number 1

\_symmetry\_cell\_setting triclinic

loop\_

\_atom\_site\_label

\_atom\_site\_type\_symbol

\_atom\_site\_fract\_x

\_atom\_site\_fract\_y

\_atom\_site\_fract\_z

\_atom\_site\_occupancy

|     |   |                    |                    |                    |     |
|-----|---|--------------------|--------------------|--------------------|-----|
| H1  | H | 0.0988323600000000 | 0.8865481200000000 | 0.9425796800000000 | 1.0 |
| H2  | H | 0.0215686400000000 | 0.1026262900000000 | 0.9092848700000000 | 1.0 |
| H3  | H | 0.9851249200000000 | 0.9523676100000000 | 0.1119405500000000 | 1.0 |
| H4  | H | 0.0680202300000000 | 0.0850968100000000 | 0.0843739700000000 | 1.0 |
| H5  | H | 0.2467599900000000 | 0.8872546600000000 | 0.0465069700000000 | 1.0 |
| H6  | H | 0.3241888700000000 | 0.1038723300000000 | 0.0766967800000000 | 1.0 |
| H7  | H | 0.3610057300000000 | 0.9506224700000000 | 0.8762679500000000 | 1.0 |
| H8  | H | 0.2777314300000000 | 0.0836849600000000 | 0.9018778700000000 | 1.0 |
| H9  | H | 0.5990886800000000 | 0.8864990400000000 | 0.9427032800000000 | 1.0 |
| H10 | H | 0.5214511200000000 | 0.1026180900000000 | 0.9093639900000000 | 1.0 |
| H11 | H | 0.4818488300000000 | 0.9522303900000000 | 0.1119081300000000 | 1.0 |
| H12 | H | 0.5679528800000000 | 0.0847839200000000 | 0.0846241600000000 | 1.0 |
| H13 | H | 0.7467392600000000 | 0.8873620100000000 | 0.0467565500000000 | 1.0 |
| H14 | H | 0.8241833500000000 | 0.1039452100000000 | 0.0766874300000000 | 1.0 |
| H15 | H | 0.8597287300000000 | 0.9504577400000000 | 0.8763827500000000 | 1.0 |
| H16 | H | 0.7776717000000000 | 0.0836420500000000 | 0.9018729500000000 | 1.0 |
| C17 | C | 0.1100125300000000 | 0.0455093000000000 | 0.9709646300000000 | 1.0 |
| C18 | C | 0.9878359000000000 | 0.0294538800000000 | 0.0139450600000000 | 1.0 |
| C19 | C | 0.9880241400000000 | 0.9496851400000000 | 0.0154212200000000 | 1.0 |
| C20 | C | 0.1101419200000000 | 0.9316633100000000 | 0.9730534800000000 | 1.0 |
| C21 | C | 0.2356940200000000 | 0.0458286700000000 | 0.0158913800000000 | 1.0 |
| C22 | C | 0.3578718600000000 | 0.0291278200000000 | 0.9731630000000000 | 1.0 |
| C23 | C | 0.3576639500000000 | 0.9493529300000000 | 0.9728217700000000 | 1.0 |
| C24 | C | 0.2355022300000000 | 0.9319426700000000 | 0.0154027500000000 | 1.0 |
| C25 | C | 0.6100132000000000 | 0.0455064800000000 | 0.9710156200000000 | 1.0 |
| C26 | C | 0.4878117000000000 | 0.0294015000000000 | 0.0139760200000000 | 1.0 |
| C27 | C | 0.4879705500000000 | 0.9496320100000000 | 0.0154057800000000 | 1.0 |

|     |   |                    |                    |                    |     |
|-----|---|--------------------|--------------------|--------------------|-----|
| C28 | C | 0.6102080900000000 | 0.9316359800000000 | 0.9731653100000000 | 1.0 |
| C29 | C | 0.7356861300000000 | 0.0458704000000000 | 0.0159320000000000 | 1.0 |
| C30 | C | 0.8578486600000000 | 0.0291350600000000 | 0.9731851200000000 | 1.0 |
| C31 | C | 0.8576416900000000 | 0.9493516800000000 | 0.9729496000000000 | 1.0 |
| C32 | C | 0.7355021500000000 | 0.9320036600000000 | 0.0155862100000000 | 1.0 |
| O33 | O | 0.1183191200000000 | 0.9881858200000000 | 0.9275204900000000 | 1.0 |
| O34 | O | 0.1078275300000000 | 0.1032597200000000 | 0.9321021100000000 | 1.0 |
| O35 | O | 0.9822527600000000 | 0.0637540600000000 | 0.0760820100000000 | 1.0 |
| O36 | O | 0.9828061800000000 | 0.9175683600000000 | 0.0776122500000000 | 1.0 |
| O37 | O | 0.2274002600000000 | 0.9891073700000000 | 0.0601598700000000 | 1.0 |
| O38 | O | 0.2378909400000000 | 0.1041311500000000 | 0.0539103700000000 | 1.0 |
| O39 | O | 0.3635223300000000 | 0.0625149100000000 | 0.9105376400000000 | 1.0 |
| O40 | O | 0.3629797800000000 | 0.9163318100000000 | 0.9111069000000000 | 1.0 |
| O41 | O | 0.6183810000000000 | 0.9881410500000000 | 0.9275940900000000 | 1.0 |
| O42 | O | 0.6077668400000000 | 0.1032334100000000 | 0.9321302300000000 | 1.0 |
| O43 | O | 0.4820707000000000 | 0.0636530300000000 | 0.0761335700000000 | 1.0 |
| O44 | O | 0.4827984400000000 | 0.9174381100000000 | 0.0775577200000000 | 1.0 |
| O45 | O | 0.7273570000000000 | 0.9892164600000000 | 0.0602430600000000 | 1.0 |
| O46 | O | 0.7378841100000000 | 0.1042052000000000 | 0.0539080800000000 | 1.0 |
| O47 | O | 0.8634458800000000 | 0.0624547600000000 | 0.9105222400000000 | 1.0 |
| O48 | O | 0.8629634200000000 | 0.9162476200000000 | 0.9112741200000000 | 1.0 |

##### cif ends

furan\_OH\_234\_syn\_alt Energy: -307.17920962

##### cif starts

data\_furan\_OH\_234\_syn\_alt

\_publ\_section\_comment

;  
Andrew Reynoso, Bohan Xu, and Vincent H. Crespi  
;

\_cell\_length\_a 10.3600598045

\_cell\_length\_b 20.0

\_cell\_length\_c 20.0

\_cell\_angle\_alpha 90.0

\_cell\_angle\_beta 90.0

\_cell\_angle\_gamma 90.0

\_symmetry\_space\_group\_name\_H-M 'P 1'

\_symmetry\_Int\_Tables\_number 1

\_symmetry\_cell\_setting triclinic

loop\_

\_atom\_site\_label

\_atom\_site\_type\_symbol

\_atom\_site\_fract\_x

\_atom\_site\_fract\_y

\_atom\_site\_fract\_z

\_atom\_site\_occupancy

|    |   |                    |                    |                    |     |
|----|---|--------------------|--------------------|--------------------|-----|
| H1 | H | 0.9791947300000000 | 0.1039313900000000 | 0.0681271700000000 | 1.0 |
|----|---|--------------------|--------------------|--------------------|-----|

|    |   |                    |                    |                    |     |
|----|---|--------------------|--------------------|--------------------|-----|
| H2 | H | 0.9178917000000000 | 0.8784082800000000 | 0.0883549900000000 | 1.0 |
|----|---|--------------------|--------------------|--------------------|-----|

|    |   |                    |                    |                    |     |
|----|---|--------------------|--------------------|--------------------|-----|
| H3 | H | 0.1906174200000000 | 0.0874634200000000 | 0.9186722000000000 | 1.0 |
|----|---|--------------------|--------------------|--------------------|-----|

|    |   |                    |                    |                    |     |
|----|---|--------------------|--------------------|--------------------|-----|
| H4 | H | 0.0254208500000000 | 0.9374029700000000 | 0.9075596400000000 | 1.0 |
|----|---|--------------------|--------------------|--------------------|-----|



|     |   |                    |                    |                    |     |
|-----|---|--------------------|--------------------|--------------------|-----|
| H5  | H | 0.2288401100000000 | 0.8992594700000000 | 0.0533581400000000 | 1.0 |
| H6  | H | 0.1678574500000000 | 0.1194508100000000 | 0.1057812600000000 | 1.0 |
| H7  | H | 0.2763852500000000 | 0.9373699300000000 | 0.9074083800000000 | 1.0 |
| H8  | H | 0.4403855300000000 | 0.0867415600000000 | 0.9181069900000000 | 1.0 |
| H9  | H | 0.4792815200000000 | 0.1039462000000000 | 0.0681700400000000 | 1.0 |
| H10 | H | 0.4179451800000000 | 0.8785609600000000 | 0.0885626300000000 | 1.0 |
| H11 | H | 0.6905144900000000 | 0.0873336300000000 | 0.9185418800000000 | 1.0 |
| H12 | H | 0.5254207800000000 | 0.9373646900000000 | 0.9076222700000000 | 1.0 |
| H13 | H | 0.7288211700000000 | 0.8993725900000000 | 0.0535773300000000 | 1.0 |
| H14 | H | 0.7762479700000000 | 0.9372189700000000 | 0.9075062900000000 | 1.0 |
| H15 | H | 0.9404922200000000 | 0.0866687500000000 | 0.9180434600000000 | 1.0 |
| H16 | H | 0.6676401900000000 | 0.1199690400000000 | 0.1051786800000000 | 1.0 |
| C17 | C | 0.9837898200000000 | 0.9489007500000000 | 0.0316040700000000 | 1.0 |
| C18 | C | 0.1085432500000000 | 0.9666483500000000 | 0.9906080300000000 | 1.0 |
| C19 | C | 0.1072763600000000 | 0.0466403200000000 | 0.9967491100000000 | 1.0 |
| C20 | C | 0.9828361500000000 | 0.0576283800000000 | 0.0387892600000000 | 1.0 |
| C21 | C | 0.2339333700000000 | 0.0579304100000000 | 0.0395107900000000 | 1.0 |
| C22 | C | 0.3580872500000000 | 0.0462905800000000 | 0.9964515900000000 | 1.0 |
| C23 | C | 0.3577110000000000 | 0.9662482100000000 | 0.9910045800000000 | 1.0 |
| C24 | C | 0.2326249700000000 | 0.9492943400000000 | 0.0309785500000000 | 1.0 |
| C25 | C | 0.4837659800000000 | 0.9489252100000000 | 0.0316383400000000 | 1.0 |
| C26 | C | 0.6085416600000000 | 0.9666271300000000 | 0.9906625600000000 | 1.0 |
| C27 | C | 0.6072631300000000 | 0.0466261000000000 | 0.9966966200000000 | 1.0 |
| C28 | C | 0.4828668800000000 | 0.0576496400000000 | 0.0388127500000000 | 1.0 |
| C29 | C | 0.7339736000000000 | 0.0579985900000000 | 0.0393772500000000 | 1.0 |
| C30 | C | 0.8581116500000000 | 0.0462329700000000 | 0.9963665900000000 | 1.0 |
| C31 | C | 0.8576917700000000 | 0.9661994400000000 | 0.9910279100000000 | 1.0 |
| C32 | C | 0.7326223500000000 | 0.9493481200000000 | 0.0310728300000000 | 1.0 |
| O33 | O | 0.9835002200000000 | 0.0005424600000000 | 0.0821376100000000 | 1.0 |
| O34 | O | 0.9923375600000000 | 0.8857659900000000 | 0.0594316500000000 | 1.0 |
| O35 | O | 0.1147410300000000 | 0.9404246100000000 | 0.9252247000000000 | 1.0 |
| O36 | O | 0.1014933200000000 | 0.0827246600000000 | 0.9362038700000000 | 1.0 |
| O37 | O | 0.2334945300000000 | 0.9995478800000000 | 0.0820855600000000 | 1.0 |
| O38 | O | 0.2424137400000000 | 0.1163889500000000 | 0.0761659600000000 | 1.0 |
| O39 | O | 0.3512419900000000 | 0.0816163200000000 | 0.9354984000000000 | 1.0 |
| O40 | O | 0.3651461000000000 | 0.9394079400000000 | 0.9258633200000000 | 1.0 |
| O41 | O | 0.4835164000000000 | 0.0005669100000000 | 0.0821604900000000 | 1.0 |
| O42 | O | 0.4922230700000000 | 0.8858008200000000 | 0.0594942400000000 | 1.0 |
| O43 | O | 0.6147332100000000 | 0.9403119700000000 | 0.9253192000000000 | 1.0 |
| O44 | O | 0.6014033700000000 | 0.0825929200000000 | 0.9360816900000000 | 1.0 |
| O45 | O | 0.7335044200000000 | 0.9997053300000000 | 0.0820805300000000 | 1.0 |
| O46 | O | 0.7425729400000000 | 0.1165550700000000 | 0.0758623500000000 | 1.0 |
| O47 | O | 0.8513089300000000 | 0.0814370900000000 | 0.9353450400000000 | 1.0 |
| O48 | O | 0.8650388100000000 | 0.9392637000000000 | 0.9259284600000000 | 1.0 |

##### cif ends

furan\_OH\_234\_syn\_alt\_forbid    Energy: -304.69086835

##### cif starts

data\_furan\_OH\_234\_syn\_alt\_forbid

\_publ\_section\_comment

;  
Andrew Reynoso, Bohan Xu, and Vincent H. Crespi  
;

\_cell\_length\_a 9.7487085239  
\_cell\_length\_b 20.0  
\_cell\_length\_c 20.0  
\_cell\_angle\_alpha 90.0  
\_cell\_angle\_beta 90.0  
\_cell\_angle\_gamma 90.0

\_symmetry\_space\_group\_name\_H-M 'P 1'  
\_symmetry\_Int\_Tables\_number 1  
\_symmetry\_cell\_setting triclinic

loop\_  
\_atom\_site\_label  
\_atom\_site\_type\_symbol  
\_atom\_site\_fract\_x  
\_atom\_site\_fract\_y  
\_atom\_site\_fract\_z  
\_atom\_site\_occupancy

|     |   |                    |                    |                    |     |
|-----|---|--------------------|--------------------|--------------------|-----|
| H1  | H | 0.9009103700000000 | 0.0980795300000000 | 0.0442089700000000 | 1.0 |
| H2  | H | 0.1747283800000000 | 0.8918052800000000 | 0.0486266700000000 | 1.0 |
| H3  | H | 0.4009488800000000 | 0.0980718000000000 | 0.0441838300000000 | 1.0 |
| H4  | H | 0.6747704700000000 | 0.8918019300000000 | 0.0486570800000000 | 1.0 |
| H5  | H | 0.0794120900000000 | 0.0798456700000000 | 0.8810632500000000 | 1.0 |
| H6  | H | 0.5793810400000000 | 0.0797764200000000 | 0.8810318200000000 | 1.0 |
| H7  | H | 0.8149489200000000 | 0.0660800400000000 | 0.8943554500000000 | 1.0 |
| H8  | H | 0.3149338300000000 | 0.0660652800000000 | 0.8943609800000000 | 1.0 |
| H9  | H | 0.2058943200000000 | 0.1145109800000000 | 0.1008313900000000 | 1.0 |
| H10 | H | 0.7058493900000000 | 0.1145397300000000 | 0.1007834700000000 | 1.0 |
| H11 | H | 0.8728185800000000 | 0.8780920000000000 | 0.1047590400000000 | 1.0 |
| H12 | H | 0.3727470200000000 | 0.8781083700000000 | 0.1047969300000000 | 1.0 |
| H13 | H | 0.8242351800000000 | 0.9149960200000000 | 0.8988866600000000 | 1.0 |
| H14 | H | 0.3242335400000000 | 0.9149853100000000 | 0.8988943300000000 | 1.0 |
| H15 | H | 0.0838950800000000 | 0.9103364400000000 | 0.8806898400000000 | 1.0 |
| H16 | H | 0.5838670600000000 | 0.9102683000000000 | 0.8807229800000000 | 1.0 |
| C17 | C | 0.8656264900000000 | 0.0504710600000000 | 0.0230681200000000 | 1.0 |
| C18 | C | 0.9498416900000000 | 0.0309599400000000 | 0.9598464300000000 | 1.0 |
| C19 | C | 0.9597798400000000 | 0.9512577600000000 | 0.9642758600000000 | 1.0 |
| C20 | C | 0.8781020300000000 | 0.9385545100000000 | 0.0291976500000000 | 1.0 |
| C21 | C | 0.1972481500000000 | 0.0505687800000000 | 0.0283078400000000 | 1.0 |
| C22 | C | 0.1150898100000000 | 0.0355663600000000 | 0.9643197800000000 | 1.0 |
| C23 | C | 0.1249808600000000 | 0.9563275000000000 | 0.9624595700000000 | 1.0 |
| C24 | C | 0.2095513600000000 | 0.9387034000000000 | 0.0258235100000000 | 1.0 |
| C25 | C | 0.3656344400000000 | 0.0504608400000000 | 0.0230627600000000 | 1.0 |
| C26 | C | 0.4498293600000000 | 0.0309208400000000 | 0.9598386100000000 | 1.0 |
| C27 | C | 0.4597725300000000 | 0.9512208200000000 | 0.9642967200000000 | 1.0 |
| C28 | C | 0.3780892900000000 | 0.9385460300000000 | 0.0292174200000000 | 1.0 |
| C29 | C | 0.6972393000000000 | 0.0505616200000000 | 0.0282889000000000 | 1.0 |
| C30 | C | 0.6150848300000000 | 0.0355287200000000 | 0.9643024500000000 | 1.0 |
| C31 | C | 0.6249693500000000 | 0.9562891100000000 | 0.9624728100000000 | 1.0 |
| C32 | C | 0.7095593000000000 | 0.9386960600000000 | 0.0258327100000000 | 1.0 |
| O33 | O | 0.9070159500000000 | 0.9981124500000000 | 0.0673632000000000 | 1.0 |
| O34 | O | 0.9167574700000000 | 0.0579634400000000 | 0.8975594100000000 | 1.0 |
| O35 | O | 0.9248701600000000 | 0.9115319900000000 | 0.9093893000000000 | 1.0 |
| O36 | O | 0.9248860800000000 | 0.8823551700000000 | 0.0633008100000000 | 1.0 |

|     |   |                    |                    |                    |     |
|-----|---|--------------------|--------------------|--------------------|-----|
| O37 | O | 0.1700008600000000 | 0.9924879800000000 | 0.0687567600000000 | 1.0 |
| O38 | O | 0.1512453100000000 | 0.1080065800000000 | 0.0604818900000000 | 1.0 |
| O39 | O | 0.1620436300000000 | 0.0734712700000000 | 0.9096696700000000 | 1.0 |
| O40 | O | 0.1693376700000000 | 0.9280505000000000 | 0.9018697000000000 | 1.0 |
| O41 | O | 0.4070156600000000 | 0.9981112500000000 | 0.0673696700000000 | 1.0 |
| O42 | O | 0.4167297500000000 | 0.0578942500000000 | 0.8975409300000000 | 1.0 |
| O43 | O | 0.4248464200000000 | 0.9114686900000000 | 0.9094289900000000 | 1.0 |
| O44 | O | 0.4248313900000000 | 0.8823525200000000 | 0.0633433300000000 | 1.0 |
| O45 | O | 0.6700060000000000 | 0.9924898400000000 | 0.0687528800000000 | 1.0 |
| O46 | O | 0.6511980600000000 | 0.1080057000000000 | 0.0604397500000000 | 1.0 |
| O47 | O | 0.6620242300000000 | 0.0734067900000000 | 0.9096325700000000 | 1.0 |
| O48 | O | 0.6693187500000000 | 0.9279782200000000 | 0.9018981500000000 | 1.0 |

##### cif ends

furan\_OH\_234\_syn\_dir Energy: -307.8164034

##### cif starts

data\_furan\_OH\_234\_syn\_dir

\_publ\_section\_comment

;  
Andrew Reynoso, Bohan Xu, and Vincent H. Crespi  
;

\_cell\_length\_a 10.378277656

\_cell\_length\_b 20.0

\_cell\_length\_c 20.0

\_cell\_angle\_alpha 90.0

\_cell\_angle\_beta 90.0

\_cell\_angle\_gamma 90.0

\_symmetry\_space\_group\_name\_H-M 'P 1'

\_symmetry\_Int\_Tables\_number 1

\_symmetry\_cell\_setting triclinic

loop\_

\_atom\_site\_label

\_atom\_site\_type\_symbol

\_atom\_site\_fract\_x

\_atom\_site\_fract\_y

\_atom\_site\_fract\_z

\_atom\_site\_occupancy

|     |   |                    |                    |                    |     |
|-----|---|--------------------|--------------------|--------------------|-----|
| H1  | H | 0.9772947000000000 | 0.9133689100000000 | 0.0710383400000000 | 1.0 |
| H2  | H | 0.0609208600000000 | 0.1408270700000000 | 0.0249321500000000 | 1.0 |
| H3  | H | 0.0202910800000000 | 0.8990933200000000 | 0.9197507600000000 | 1.0 |
| H4  | H | 0.1846474800000000 | 0.0428756100000000 | 0.8789383700000000 | 1.0 |
| H5  | H | 0.2273205800000000 | 0.9133569100000000 | 0.0710313500000000 | 1.0 |
| H6  | H | 0.3108969400000000 | 0.1408217700000000 | 0.0249689900000000 | 1.0 |
| H7  | H | 0.2702746100000000 | 0.8991013000000000 | 0.9197379500000000 | 1.0 |
| H8  | H | 0.4346565800000000 | 0.0429129500000000 | 0.8789573000000000 | 1.0 |
| H9  | H | 0.4773261900000000 | 0.9133327200000000 | 0.0710006900000000 | 1.0 |
| H10 | H | 0.5608967600000000 | 0.1408171800000000 | 0.0250063100000000 | 1.0 |
| H11 | H | 0.5202962100000000 | 0.8991251500000000 | 0.9197084700000000 | 1.0 |
| H12 | H | 0.6846204200000000 | 0.0429181600000000 | 0.8789509500000000 | 1.0 |
| H13 | H | 0.7272935600000000 | 0.9133398800000000 | 0.0710071200000000 | 1.0 |

|     |   |                    |                    |                    |     |
|-----|---|--------------------|--------------------|--------------------|-----|
| H14 | H | 0.8109212000000000 | 0.1408210600000000 | 0.0249727000000000 | 1.0 |
| H15 | H | 0.7703143000000000 | 0.8991113900000000 | 0.9197202700000000 | 1.0 |
| H16 | H | 0.9346129100000000 | 0.0428787900000000 | 0.8789371700000000 | 1.0 |
| C17 | C | 0.9773996700000000 | 0.0569531800000000 | 0.0024243800000000 | 1.0 |
| C18 | C | 0.1023039400000000 | 0.0312204200000000 | 0.9663783800000000 | 1.0 |
| C19 | C | 0.1026792600000000 | 0.9542574600000000 | 0.9886184400000000 | 1.0 |
| C20 | C | 0.9773990300000000 | 0.9522463600000000 | 0.0322769500000000 | 1.0 |
| C21 | C | 0.2273940200000000 | 0.0569504400000000 | 0.0024342100000000 | 1.0 |
| C22 | C | 0.3523015900000000 | 0.0312321300000000 | 0.9663885500000000 | 1.0 |
| C23 | C | 0.3526778500000000 | 0.9542620500000000 | 0.9886051100000000 | 1.0 |
| C24 | C | 0.2274070400000000 | 0.9522403300000000 | 0.0322755100000000 | 1.0 |
| C25 | C | 0.4773922100000000 | 0.0569505900000000 | 0.0024561500000000 | 1.0 |
| C26 | C | 0.6022975000000000 | 0.0312421400000000 | 0.9663929400000000 | 1.0 |
| C27 | C | 0.6026793000000000 | 0.9542684100000000 | 0.9885951700000000 | 1.0 |
| C28 | C | 0.4774080900000000 | 0.9522302400000000 | 0.0322589800000000 | 1.0 |
| C29 | C | 0.7273984200000000 | 0.0569521600000000 | 0.0024486700000000 | 1.0 |
| C30 | C | 0.8522964400000000 | 0.0312291600000000 | 0.9663828100000000 | 1.0 |
| C31 | C | 0.8526794200000000 | 0.9542628900000000 | 0.9886079000000000 | 1.0 |
| C32 | C | 0.7273988400000000 | 0.9522342300000000 | 0.0322615200000000 | 1.0 |
| O33 | O | 0.9774921400000000 | 0.0170678900000000 | 0.0626904400000000 | 1.0 |
| O34 | O | 0.9719731000000000 | 0.1247704600000000 | 0.0160637100000000 | 1.0 |
| O35 | O | 0.0957178300000000 | 0.0437730700000000 | 0.8970837700000000 | 1.0 |
| O36 | O | 0.1090728300000000 | 0.9066715100000000 | 0.9365055000000000 | 1.0 |
| O37 | O | 0.2274929700000000 | 0.0170587200000000 | 0.0626957400000000 | 1.0 |
| O38 | O | 0.2219548500000000 | 0.1247653400000000 | 0.0160832900000000 | 1.0 |
| O39 | O | 0.3457224700000000 | 0.0438112600000000 | 0.8970981600000000 | 1.0 |
| O40 | O | 0.3590640700000000 | 0.9066955100000000 | 0.9364740300000000 | 1.0 |
| O41 | O | 0.4774953100000000 | 0.0170373000000000 | 0.0627021100000000 | 1.0 |
| O42 | O | 0.4719509700000000 | 0.1247581000000000 | 0.0161375300000000 | 1.0 |
| O43 | O | 0.5957002500000000 | 0.0438411700000000 | 0.8971058900000000 | 1.0 |
| O44 | O | 0.6090800400000000 | 0.9067113400000000 | 0.9364549900000000 | 1.0 |
| O45 | O | 0.7274950900000000 | 0.0170437800000000 | 0.0626991500000000 | 1.0 |
| O46 | O | 0.7219695400000000 | 0.1247613900000000 | 0.0161212400000000 | 1.0 |
| O47 | O | 0.8456920600000000 | 0.0437965400000000 | 0.8970900800000000 | 1.0 |
| O48 | O | 0.8590892700000000 | 0.9066895300000000 | 0.9364828100000000 | 1.0 |

##### cif ends

furan\_OH\_234\_syn\_dir\_forbid Energy: -305.26181801

##### cif starts

data\_furan\_OH\_234\_syn\_dir\_forbid

\_publ\_section\_comment

;  
Andrew Reynoso, Bohan Xu, and Vincent H. Crespi  
;

\_cell\_length\_a 9.7644131197

\_cell\_length\_b 20.0

\_cell\_length\_c 20.0

\_cell\_angle\_alpha 90.0

\_cell\_angle\_beta 90.0

\_cell\_angle\_gamma 90.0

\_symmetry\_space\_group\_name\_H-M 'P 1'

\_symmetry\_Int\_Tables\_number 1  
\_symmetry\_cell\_setting triclinic

loop\_

\_atom\_site\_label

\_atom\_site\_type\_symbol

\_atom\_site\_fract\_x

\_atom\_site\_fract\_y

\_atom\_site\_fract\_z

\_atom\_site\_occupancy

|     |   |                    |                    |                    |     |
|-----|---|--------------------|--------------------|--------------------|-----|
| H1  | H | 0.8912639000000000 | 0.1048073900000000 | 0.0348484800000000 | 1.0 |
| H2  | H | 0.1564232700000000 | 0.0982180800000000 | 0.0516876100000000 | 1.0 |
| H3  | H | 0.3912145800000000 | 0.1048518100000000 | 0.0348346800000000 | 1.0 |
| H4  | H | 0.6564805300000000 | 0.0981888500000000 | 0.0517735600000000 | 1.0 |
| H5  | H | 0.8086536700000000 | 0.0590492500000000 | 0.8898210800000000 | 1.0 |
| H6  | H | 0.0740531200000000 | 0.0730177000000000 | 0.8761315900000000 | 1.0 |
| H7  | H | 0.3086957600000000 | 0.0590579700000000 | 0.8897982100000000 | 1.0 |
| H8  | H | 0.5741192800000000 | 0.0731303700000000 | 0.8761842900000000 | 1.0 |
| H9  | H | 0.0773021300000000 | 0.9025574800000000 | 0.8884070900000000 | 1.0 |
| H10 | H | 0.5773243400000000 | 0.9026361700000000 | 0.8883562900000000 | 1.0 |
| H11 | H | 0.8185908400000000 | 0.9087380000000000 | 0.9077049700000000 | 1.0 |
| H12 | H | 0.3185779300000000 | 0.9087439800000000 | 0.9077154500000000 | 1.0 |
| H13 | H | 0.2447839900000000 | 0.8644835300000000 | 0.0828674400000000 | 1.0 |
| H14 | H | 0.7447277400000000 | 0.8644154000000000 | 0.0827759600000000 | 1.0 |
| H15 | H | 0.0061555800000000 | 0.8830246800000000 | 0.0780560200000000 | 1.0 |
| H16 | H | 0.5062028000000000 | 0.8830469900000000 | 0.0780186300000000 | 1.0 |
| C17 | C | 0.8571613000000000 | 0.0549492400000000 | 0.0189972200000000 | 1.0 |
| C18 | C | 0.9424190500000000 | 0.0291527800000000 | 0.9579379100000000 | 1.0 |
| C19 | C | 0.9547874300000000 | 0.9504560500000000 | 0.9698848500000000 | 1.0 |
| C20 | C | 0.8748092800000000 | 0.9443586600000000 | 0.0364100000000000 | 1.0 |
| C21 | C | 0.1894835300000000 | 0.0527168800000000 | 0.0256636700000000 | 1.0 |
| C22 | C | 0.1079656500000000 | 0.0348365100000000 | 0.9625884400000000 | 1.0 |
| C23 | C | 0.1195377800000000 | 0.9561182600000000 | 0.9650329000000000 | 1.0 |
| C24 | C | 0.2042796300000000 | 0.9412390800000000 | 0.0294120300000000 | 1.0 |
| C25 | C | 0.3571494800000000 | 0.0549875800000000 | 0.0189803800000000 | 1.0 |
| C26 | C | 0.4424375900000000 | 0.0292016300000000 | 0.9579392200000000 | 1.0 |
| C27 | C | 0.4547959400000000 | 0.9504993900000000 | 0.9698676100000000 | 1.0 |
| C28 | C | 0.3748277000000000 | 0.9443956700000000 | 0.0364068100000000 | 1.0 |
| C29 | C | 0.6894913700000000 | 0.0527023200000000 | 0.0257090600000000 | 1.0 |
| C30 | C | 0.6079728800000000 | 0.0348834500000000 | 0.9626181000000000 | 1.0 |
| C31 | C | 0.6195550600000000 | 0.9561610700000000 | 0.9650071100000000 | 1.0 |
| C32 | C | 0.7042811800000000 | 0.9412234400000000 | 0.0293816000000000 | 1.0 |
| O33 | O | 0.8994501500000000 | 0.0078692800000000 | 0.0683008900000000 | 1.0 |
| O34 | O | 0.9097026300000000 | 0.0497511000000000 | 0.8930947000000000 | 1.0 |
| O35 | O | 0.9177449100000000 | 0.9044893600000000 | 0.9203672900000000 | 1.0 |
| O36 | O | 0.9054387600000000 | 0.8931743600000000 | 0.0799014900000000 | 1.0 |
| O37 | O | 0.1631101100000000 | 0.9973630400000000 | 0.0692783000000000 | 1.0 |
| O38 | O | 0.1549057100000000 | 0.0706612000000000 | 0.9063477200000000 | 1.0 |
| O39 | O | 0.1618836600000000 | 0.9245608600000000 | 0.9058278000000000 | 1.0 |
| O40 | O | 0.1630546000000000 | 0.8811684500000000 | 0.0580864700000000 | 1.0 |
| O41 | O | 0.3994496000000000 | 0.0079162400000000 | 0.0682881400000000 | 1.0 |
| O42 | O | 0.4097653200000000 | 0.0498301500000000 | 0.8931001700000000 | 1.0 |
| O43 | O | 0.4177628700000000 | 0.9045477400000000 | 0.9203368300000000 | 1.0 |
| O44 | O | 0.4055006100000000 | 0.8932273200000000 | 0.0799077800000000 | 1.0 |
| O45 | O | 0.6631037700000000 | 0.9973187700000000 | 0.0692851200000000 | 1.0 |

|     |   |                    |                    |                    |     |
|-----|---|--------------------|--------------------|--------------------|-----|
| O46 | O | 0.6549417600000000 | 0.0707693200000000 | 0.9064189000000000 | 1.0 |
| O47 | O | 0.6618978500000000 | 0.9246411600000000 | 0.9057808300000000 | 1.0 |
| O48 | O | 0.6630230700000000 | 0.8811261000000000 | 0.0579926800000000 | 1.0 |

##### cif ends

furant\_OH\_23\_anti\_alt Energy: -279.99497604

##### cif starts

data\_furant\_OH\_23\_anti\_alt

\_publ\_section\_comment

;  
Andrew Reynoso, Bohan Xu, and Vincent H. Crespi  
;

\_cell\_length\_a 9.3863569574  
\_cell\_length\_b 20.0  
\_cell\_length\_c 20.0  
\_cell\_angle\_alpha 90.0  
\_cell\_angle\_beta 90.0  
\_cell\_angle\_gamma 90.0

\_symmetry\_space\_group\_name\_H-M 'P 1'  
\_symmetry\_Int\_Tables\_number 1  
\_symmetry\_cell\_setting triclinic

loop\_  
\_atom\_site\_label  
\_atom\_site\_type\_symbol  
\_atom\_site\_fract\_x  
\_atom\_site\_fract\_y  
\_atom\_site\_fract\_z  
\_atom\_site\_occupancy

|     |   |                    |                    |                    |     |
|-----|---|--------------------|--------------------|--------------------|-----|
| H1  | H | 0.5191187600000000 | 0.8775296300000000 | 0.9755503600000000 | 1.0 |
| H2  | H | 0.5097701800000000 | 0.9555135000000000 | 0.0907186500000000 | 1.0 |
| H3  | H | 0.5858416600000000 | 0.0893506500000000 | 0.8765174700000000 | 1.0 |
| H4  | H | 0.4678842100000000 | 0.0818681600000000 | 0.1069765400000000 | 1.0 |
| H5  | H | 0.7691140700000000 | 0.1040333300000000 | 0.0290067700000000 | 1.0 |
| H6  | H | 0.7597668000000000 | 0.0260694900000000 | 0.9138193800000000 | 1.0 |
| H7  | H | 0.8358174300000000 | 0.8922112600000000 | 0.1280111400000000 | 1.0 |
| H8  | H | 0.7177268300000000 | 0.8997107400000000 | 0.8975424100000000 | 1.0 |
| H9  | H | 0.0191279900000000 | 0.8775242200000000 | 0.9755486700000000 | 1.0 |
| H10 | H | 0.0097677200000000 | 0.9555051700000000 | 0.0907166200000000 | 1.0 |
| H11 | H | 0.0857952500000000 | 0.0893199600000000 | 0.8764931100000000 | 1.0 |
| H12 | H | 0.9680260800000000 | 0.0818050200000000 | 0.1070040700000000 | 1.0 |
| H13 | H | 0.2691033400000000 | 0.1040354900000000 | 0.0289956100000000 | 1.0 |
| H14 | H | 0.2597657900000000 | 0.0260659100000000 | 0.9138163000000000 | 1.0 |
| H15 | H | 0.3358195500000000 | 0.8922216100000000 | 0.1280192100000000 | 1.0 |
| H16 | H | 0.2178327300000000 | 0.8997411900000000 | 0.8975286000000000 | 1.0 |
| C17 | C | 0.5434337600000000 | 0.9300719900000000 | 0.9851416700000000 | 1.0 |
| C18 | C | 0.4595758200000000 | 0.9626004800000000 | 0.0415479800000000 | 1.0 |
| C19 | C | 0.4580942600000000 | 0.0381004900000000 | 0.0203083300000000 | 1.0 |
| C20 | C | 0.5470236600000000 | 0.0347296100000000 | 0.9543686000000000 | 1.0 |
| C21 | C | 0.7934245900000000 | 0.0514892100000000 | 0.0194024100000000 | 1.0 |
| C22 | C | 0.7095645700000000 | 0.0189740800000000 | 0.9629879900000000 | 1.0 |

|     |   |                    |                    |                    |     |
|-----|---|--------------------|--------------------|--------------------|-----|
| C23 | C | 0.7081034600000000 | 0.9434694400000000 | 0.9842154500000000 | 1.0 |
| C24 | C | 0.7970437800000000 | 0.9468279300000000 | 0.0501515500000000 | 1.0 |
| C25 | C | 0.0434375200000000 | 0.9300674900000000 | 0.9851400100000000 | 1.0 |
| C26 | C | 0.9595764700000000 | 0.9625959900000000 | 0.0415454700000000 | 1.0 |
| C27 | C | 0.9580964600000000 | 0.0380962400000000 | 0.0203078500000000 | 1.0 |
| C28 | C | 0.0470209500000000 | 0.0347236800000000 | 0.9543660000000000 | 1.0 |
| C29 | C | 0.2934220400000000 | 0.0514906700000000 | 0.0193978400000000 | 1.0 |
| C30 | C | 0.2095653500000000 | 0.0189704900000000 | 0.9629853000000000 | 1.0 |
| C31 | C | 0.2081076500000000 | 0.9434674500000000 | 0.9842170800000000 | 1.0 |
| C32 | C | 0.2970447200000000 | 0.9468313400000000 | 0.0501548400000000 | 1.0 |
| O33 | O | 0.5020886700000000 | 0.9702605600000000 | 0.9272444400000000 | 1.0 |
| O34 | O | 0.5181116100000000 | 0.0859998200000000 | 0.0645477600000000 | 1.0 |
| O35 | O | 0.5138537600000000 | 0.0871388100000000 | 0.9115572100000000 | 1.0 |
| O36 | O | 0.7520844100000000 | 0.0112862600000000 | 0.0772892300000000 | 1.0 |
| O37 | O | 0.7680576300000000 | 0.8955805000000000 | 0.9399465500000000 | 1.0 |
| O38 | O | 0.7638775000000000 | 0.8944056500000000 | 0.0929471700000000 | 1.0 |
| O39 | O | 0.0020916600000000 | 0.9702548900000000 | 0.9272434400000000 | 1.0 |
| O40 | O | 0.0181199700000000 | 0.0859951800000000 | 0.0645466300000000 | 1.0 |
| O41 | O | 0.0138455400000000 | 0.0871300000000000 | 0.9115517300000000 | 1.0 |
| O42 | O | 0.2520811800000000 | 0.0112919600000000 | 0.0772873900000000 | 1.0 |
| O43 | O | 0.2680706400000000 | 0.8955760300000000 | 0.9399529700000000 | 1.0 |
| O44 | O | 0.2638769700000000 | 0.8944131400000000 | 0.0929554300000000 | 1.0 |

##### cif ends

furand\_OH\_23\_anti\_alt\_forbid Energy: -279.74781406

##### cif starts

data\_furand\_OH\_23\_anti\_alt\_forbid

\_publ\_section\_comment

;  
Andrew Reynoso, Bohan Xu, and Vincent H. Crespi  
;

\_cell\_length\_a 10.2269559119

\_cell\_length\_b 20.0

\_cell\_length\_c 20.0

\_cell\_angle\_alpha 90.0

\_cell\_angle\_beta 90.0

\_cell\_angle\_gamma 90.0

\_symmetry\_space\_group\_name\_H-M 'P 1'

\_symmetry\_Int\_Tables\_number 1

\_symmetry\_cell\_setting triclinic

loop\_

\_atom\_site\_label

\_atom\_site\_type\_symbol

\_atom\_site\_fract\_x

\_atom\_site\_fract\_y

\_atom\_site\_fract\_z

\_atom\_site\_occupancy

|    |   |                    |                    |                    |     |
|----|---|--------------------|--------------------|--------------------|-----|
| H1 | H | 0.9570662200000000 | 0.9356111700000000 | 0.0566712000000000 | 1.0 |
|----|---|--------------------|--------------------|--------------------|-----|

|    |   |                    |                    |                    |     |
|----|---|--------------------|--------------------|--------------------|-----|
| H2 | H | 0.0650102800000000 | 0.8942294500000000 | 0.9344176700000000 | 1.0 |
|----|---|--------------------|--------------------|--------------------|-----|

|    |   |                    |                    |                    |     |
|----|---|--------------------|--------------------|--------------------|-----|
| H3 | H | 0.3227613900000000 | 0.0565275800000000 | 0.9125966300000000 | 1.0 |
|----|---|--------------------|--------------------|--------------------|-----|

|     |   |                    |                    |                    |     |
|-----|---|--------------------|--------------------|--------------------|-----|
| H4  | H | 0.2147827300000000 | 0.0978823600000000 | 0.0348615700000000 | 1.0 |
| H5  | H | 0.4571089600000000 | 0.9355411800000000 | 0.0566319300000000 | 1.0 |
| H6  | H | 0.5650870300000000 | 0.8942352500000000 | 0.9343780100000000 | 1.0 |
| H7  | H | 0.8227456600000000 | 0.0565637900000000 | 0.9126035000000000 | 1.0 |
| H8  | H | 0.7147374300000000 | 0.0978914300000000 | 0.0348651900000000 | 1.0 |
| H9  | H | 0.9634114100000000 | 0.1189077900000000 | 0.0549962900000000 | 1.0 |
| H10 | H | 0.4634681000000000 | 0.1188964600000000 | 0.0549431000000000 | 1.0 |
| H11 | H | 0.0079080400000000 | 0.1075107700000000 | 0.8906975300000000 | 1.0 |
| H12 | H | 0.5079191500000000 | 0.1074835500000000 | 0.8906672100000000 | 1.0 |
| H13 | H | 0.3161115600000000 | 0.8732178600000000 | 0.9142590800000000 | 1.0 |
| H14 | H | 0.8160668400000000 | 0.8732284200000000 | 0.9143100900000000 | 1.0 |
| H15 | H | 0.2719152000000000 | 0.8845858300000000 | 0.0785762800000000 | 1.0 |
| H16 | H | 0.7719856700000000 | 0.8846052000000000 | 0.0785394500000000 | 1.0 |
| C17 | C | 0.0786094600000000 | 0.0523269100000000 | 0.9614546800000000 | 1.0 |
| C18 | C | 0.9543793200000000 | 0.0364591600000000 | 0.0035788000000000 | 1.0 |
| C19 | C | 0.9558844900000000 | 0.9582567800000000 | 0.0066981000000000 | 1.0 |
| C20 | C | 0.0757769600000000 | 0.9400390000000000 | 0.9639362600000000 | 1.0 |
| C21 | C | 0.2040443900000000 | 0.0520772800000000 | 0.0053338000000000 | 1.0 |
| C22 | C | 0.3239402800000000 | 0.0338655900000000 | 0.9625599300000000 | 1.0 |
| C23 | C | 0.3254327700000000 | 0.9556622000000000 | 0.9656703300000000 | 1.0 |
| C24 | C | 0.2012270500000000 | 0.9397896300000000 | 0.0078098300000000 | 1.0 |
| C25 | C | 0.5785858300000000 | 0.0523245300000000 | 0.9614558900000000 | 1.0 |
| C26 | C | 0.4543756200000000 | 0.0364308100000000 | 0.0035771700000000 | 1.0 |
| C27 | C | 0.4558898900000000 | 0.9582273200000000 | 0.0066777500000000 | 1.0 |
| C28 | C | 0.5757963000000000 | 0.9400406500000000 | 0.9639095700000000 | 1.0 |
| C29 | C | 0.7040227400000000 | 0.0520882100000000 | 0.0053338000000000 | 1.0 |
| C30 | C | 0.8239357100000000 | 0.0338946200000000 | 0.9625634900000000 | 1.0 |
| C31 | C | 0.8254464500000000 | 0.9556871800000000 | 0.9656767300000000 | 1.0 |
| C32 | C | 0.7012358800000000 | 0.9398030200000000 | 0.0077971800000000 | 1.0 |
| O33 | O | 0.0764214100000000 | 0.1115272400000000 | 0.9244666900000000 | 1.0 |
| O34 | O | 0.9504080200000000 | 0.0716220900000000 | 0.0648310800000000 | 1.0 |
| O35 | O | 0.3293723400000000 | 0.9204868600000000 | 0.9044273500000000 | 1.0 |
| O36 | O | 0.2034458600000000 | 0.8805755200000000 | 0.0447830700000000 | 1.0 |
| O37 | O | 0.0866415200000000 | 0.9953579500000000 | 0.9175456800000000 | 1.0 |
| O38 | O | 0.1932069000000000 | 0.9967537300000000 | 0.0517206800000000 | 1.0 |
| O39 | O | 0.5763201500000000 | 0.1115421900000000 | 0.9244940000000000 | 1.0 |
| O40 | O | 0.4503998700000000 | 0.0716216900000000 | 0.0648133700000000 | 1.0 |
| O41 | O | 0.8294167200000000 | 0.9204859200000000 | 0.9044487000000000 | 1.0 |
| O42 | O | 0.7034929200000000 | 0.8805817400000000 | 0.0447595900000000 | 1.0 |
| O43 | O | 0.5866478200000000 | 0.9953735300000000 | 0.9175315500000000 | 1.0 |
| O44 | O | 0.6931783000000000 | 0.9967604700000000 | 0.0517156600000000 | 1.0 |

##### cif ends

furand\_OH\_23\_anti\_dir Energy: -280.95335489

##### cif starts

data\_furand\_OH\_23\_anti\_dir

\_publ\_section\_comment

;  
Andrew Reynoso, Bohan Xu, and Vincent H. Crespi  
;

\_cell\_length\_a 9.4335347466

\_cell\_length\_b 20.0



\_cell\_length\_c 20.0  
\_cell\_angle\_alpha 90.0  
\_cell\_angle\_beta 90.0  
\_cell\_angle\_gamma 90.0

\_symmetry\_space\_group\_name\_H-M 'P 1'  
\_symmetry\_Int\_Tables\_number 1  
\_symmetry\_cell\_setting triclinic

loop\_

\_atom\_site\_label  
\_atom\_site\_type\_symbol  
\_atom\_site\_fract\_x  
\_atom\_site\_fract\_y  
\_atom\_site\_fract\_z  
\_atom\_site\_occupancy

|     |   |                    |                    |                    |     |
|-----|---|--------------------|--------------------|--------------------|-----|
| H1  | H | 0.9893938800000000 | 0.1375124000000000 | 0.9438269500000000 | 1.0 |
| H2  | H | 0.9741935700000000 | 0.0948486400000000 | 0.0782056800000000 | 1.0 |
| H3  | H | 0.0641040100000000 | 0.9119209000000000 | 0.9112594700000000 | 1.0 |
| H4  | H | 0.0650491300000000 | 0.9431546800000000 | 0.0878163500000000 | 1.0 |
| H5  | H | 0.2397899700000000 | 0.1385056900000000 | 0.0561747200000000 | 1.0 |
| H6  | H | 0.2243740200000000 | 0.0933416200000000 | 0.9226106500000000 | 1.0 |
| H7  | H | 0.3141599300000000 | 0.9132218300000000 | 0.0926015600000000 | 1.0 |
| H8  | H | 0.3146313200000000 | 0.9412981100000000 | 0.9159975800000000 | 1.0 |
| H9  | H | 0.4895605900000000 | 0.1371861900000000 | 0.9435118000000000 | 1.0 |
| H10 | H | 0.4747594600000000 | 0.0946861100000000 | 0.0779980700000000 | 1.0 |
| H11 | H | 0.5637664000000000 | 0.9114269400000000 | 0.9113845400000000 | 1.0 |
| H12 | H | 0.5650389500000000 | 0.9431524300000000 | 0.0878571300000000 | 1.0 |
| H13 | H | 0.7391013700000000 | 0.1385122800000000 | 0.0559385000000000 | 1.0 |
| H14 | H | 0.7246170500000000 | 0.0928664900000000 | 0.9224738400000000 | 1.0 |
| H15 | H | 0.8143130800000000 | 0.9137476500000000 | 0.0933886900000000 | 1.0 |
| H16 | H | 0.8150588600000000 | 0.9411057300000000 | 0.9161320000000000 | 1.0 |
| C17 | C | 0.0142777300000000 | 0.0895963300000000 | 0.9678591800000000 | 1.0 |
| C18 | C | 0.9281738700000000 | 0.0748395500000000 | 0.0320451500000000 | 1.0 |
| C19 | C | 0.9265554000000000 | 0.9964042100000000 | 0.0333539900000000 | 1.0 |
| C20 | C | 0.0108859300000000 | 0.9810040100000000 | 0.9690689400000000 | 1.0 |
| C21 | C | 0.2644687900000000 | 0.0901424100000000 | 0.0330121000000000 | 1.0 |
| C22 | C | 0.1782490400000000 | 0.0742428500000000 | 0.9691306500000000 | 1.0 |
| C23 | C | 0.1764767800000000 | 0.9958097800000000 | 0.9693519600000000 | 1.0 |
| C24 | C | 0.2608976100000000 | 0.9815534300000000 | 0.0338495400000000 | 1.0 |
| C25 | C | 0.5143973400000000 | 0.0893202500000000 | 0.9676536500000000 | 1.0 |
| C26 | C | 0.4283875500000000 | 0.0746961900000000 | 0.0319112300000000 | 1.0 |
| C27 | C | 0.4264884100000000 | 0.9962575100000000 | 0.0332387000000000 | 1.0 |
| C28 | C | 0.5108635700000000 | 0.9807370700000000 | 0.9690441800000000 | 1.0 |
| C29 | C | 0.7641929100000000 | 0.0901162600000000 | 0.0329368500000000 | 1.0 |
| C30 | C | 0.6783045700000000 | 0.0739478100000000 | 0.9690241500000000 | 1.0 |
| C31 | C | 0.6765107000000000 | 0.9954830300000000 | 0.9694599500000000 | 1.0 |
| C32 | C | 0.7609280600000000 | 0.9815200000000000 | 0.0340603300000000 | 1.0 |
| O33 | O | 0.9663015900000000 | 0.0358116700000000 | 0.9251644100000000 | 1.0 |
| O34 | O | 0.9697427700000000 | 0.9634629700000000 | 0.0926751700000000 | 1.0 |
| O35 | O | 0.9803654100000000 | 0.9195786000000000 | 0.9408388400000000 | 1.0 |
| O36 | O | 0.2165056100000000 | 0.0371937800000000 | 0.0767413700000000 | 1.0 |
| O37 | O | 0.2194475500000000 | 0.9616247600000000 | 0.9106958300000000 | 1.0 |
| O38 | O | 0.2302082000000000 | 0.9206282700000000 | 0.0631116000000000 | 1.0 |
| O39 | O | 0.4664599100000000 | 0.0354805700000000 | 0.9250360200000000 | 1.0 |

|     |   |                    |                    |                    |     |
|-----|---|--------------------|--------------------|--------------------|-----|
| O40 | O | 0.4693882600000000 | 0.9631537000000000 | 0.0925113100000000 | 1.0 |
| O41 | O | 0.4800984400000000 | 0.9192860700000000 | 0.9409239500000000 | 1.0 |
| O42 | O | 0.7162880900000000 | 0.0372434600000000 | 0.0767650000000000 | 1.0 |
| O43 | O | 0.7195576400000000 | 0.9611478600000000 | 0.9109163100000000 | 1.0 |
| O44 | O | 0.7305304800000000 | 0.9207338100000000 | 0.0636774700000000 | 1.0 |

##### cif ends

furan\_OH\_23\_anti\_dir\_forbid Energy: -280.9883261

##### cif starts

data\_furan\_OH\_23\_anti\_dir\_forbid

\_publ\_section\_comment

;  
Andrew Reynoso, Bohan Xu, and Vincent H. Crespi  
;

\_cell\_length\_a 10.2212999757

\_cell\_length\_b 20.0

\_cell\_length\_c 20.0

\_cell\_angle\_alpha 90.0

\_cell\_angle\_beta 90.0

\_cell\_angle\_gamma 90.0

\_symmetry\_space\_group\_name\_H-M 'P 1'

\_symmetry\_Int\_Tables\_number 1

\_symmetry\_cell\_setting triclinic

loop\_

\_atom\_site\_label

\_atom\_site\_type\_symbol

\_atom\_site\_fract\_x

\_atom\_site\_fract\_y

\_atom\_site\_fract\_z

\_atom\_site\_occupancy

|     |   |                    |                    |                    |     |
|-----|---|--------------------|--------------------|--------------------|-----|
| H1  | H | 0.0848658200000000 | 0.1062087900000000 | 0.9415452900000000 | 1.0 |
| H2  | H | 0.9684714200000000 | 0.0663814200000000 | 0.0630274200000000 | 1.0 |
| H3  | H | 0.0051055200000000 | 0.8891317300000000 | 0.9113656400000000 | 1.0 |
| H4  | H | 0.0549046500000000 | 0.9072211400000000 | 0.0835320900000000 | 1.0 |
| H5  | H | 0.2328261000000000 | 0.1066685200000000 | 0.0438000000000000 | 1.0 |
| H6  | H | 0.3492668000000000 | 0.0657697200000000 | 0.9226943800000000 | 1.0 |
| H7  | H | 0.3126338700000000 | 0.8898453700000000 | 0.0758823900000000 | 1.0 |
| H8  | H | 0.2628159000000000 | 0.9064516300000000 | 0.9035628800000000 | 1.0 |
| H9  | H | 0.5848794400000000 | 0.1062167800000000 | 0.9415666200000000 | 1.0 |
| H10 | H | 0.4684403700000000 | 0.0663746100000000 | 0.0630300300000000 | 1.0 |
| H11 | H | 0.5050970500000000 | 0.8891403500000000 | 0.9113585100000000 | 1.0 |
| H12 | H | 0.5549103600000000 | 0.9072203000000000 | 0.0835327500000000 | 1.0 |
| H13 | H | 0.7328204400000000 | 0.1066550600000000 | 0.0438293100000000 | 1.0 |
| H14 | H | 0.8492393700000000 | 0.0657833400000000 | 0.9227077000000000 | 1.0 |
| H15 | H | 0.8126366300000000 | 0.8898321500000000 | 0.0758679100000000 | 1.0 |
| H16 | H | 0.7628235000000000 | 0.9064794500000000 | 0.9035409400000000 | 1.0 |
| C17 | C | 0.0954629000000000 | 0.0607436900000000 | 0.9720230100000000 | 1.0 |
| C18 | C | 0.9732766100000000 | 0.0428552300000000 | 0.0135695200000000 | 1.0 |
| C19 | C | 0.9740118000000000 | 0.9637365200000000 | 0.0136536300000000 | 1.0 |
| C20 | C | 0.0962279700000000 | 0.9473810100000000 | 0.9705681200000000 | 1.0 |

|     |   |                    |                    |                    |     |
|-----|---|--------------------|--------------------|--------------------|-----|
| C21 | C | 0.2222353100000000 | 0.0609330300000000 | 0.0137282300000000 | 1.0 |
| C22 | C | 0.3444313900000000 | 0.0426754800000000 | 0.9723546100000000 | 1.0 |
| C23 | C | 0.3436950600000000 | 0.9635610900000000 | 0.9729587300000000 | 1.0 |
| C24 | C | 0.2214785800000000 | 0.9475862000000000 | 0.0161920100000000 | 1.0 |
| C25 | C | 0.5954661300000000 | 0.0607459200000000 | 0.9720370600000000 | 1.0 |
| C26 | C | 0.4732703100000000 | 0.0428518800000000 | 0.0135711800000000 | 1.0 |
| C27 | C | 0.4740115700000000 | 0.9637335900000000 | 0.0136530200000000 | 1.0 |
| C28 | C | 0.5962291400000000 | 0.9473825900000000 | 0.9705642900000000 | 1.0 |
| C29 | C | 0.7222331300000000 | 0.0609264700000000 | 0.0137471600000000 | 1.0 |
| C30 | C | 0.8444250100000000 | 0.0426803700000000 | 0.9723647800000000 | 1.0 |
| C31 | C | 0.8436959700000000 | 0.9635657500000000 | 0.9729574000000000 | 1.0 |
| C32 | C | 0.7214797500000000 | 0.9475791600000000 | 0.0161869900000000 | 1.0 |
| O33 | O | 0.1059541800000000 | 0.0046700100000000 | 0.9264170000000000 | 1.0 |
| O34 | O | 0.9682273100000000 | 0.9267877300000000 | 0.0740749500000000 | 1.0 |
| O35 | O | 0.0932439900000000 | 0.8893788700000000 | 0.9325450800000000 | 1.0 |
| O36 | O | 0.2117514300000000 | 0.0052705600000000 | 0.0598334700000000 | 1.0 |
| O37 | O | 0.3494899300000000 | 0.9261003800000000 | 0.9128556900000000 | 1.0 |
| O38 | O | 0.2244717800000000 | 0.8899226700000000 | 0.0547260000000000 | 1.0 |
| O39 | O | 0.6059619100000000 | 0.0046793600000000 | 0.9264223800000000 | 1.0 |
| O40 | O | 0.4682325300000000 | 0.9267839000000000 | 0.0740739000000000 | 1.0 |
| O41 | O | 0.5932422900000000 | 0.8893879200000000 | 0.9325306200000000 | 1.0 |
| O42 | O | 0.7117511700000000 | 0.0052542900000000 | 0.0598407400000000 | 1.0 |
| O43 | O | 0.8495029200000000 | 0.9261132100000000 | 0.9128497000000000 | 1.0 |
| O44 | O | 0.7244778200000000 | 0.8899070000000000 | 0.0547080700000000 | 1.0 |

##### cif ends

furand\_OH\_23\_syn\_alt Energy: -280.15159537

##### cif starts

data\_furand\_OH\_23\_syn\_alt

\_publ\_section\_comment

;  
Andrew Reynoso, Bohan Xu, and Vincent H. Crespi  
;

\_cell\_length\_a 10.3303542182

\_cell\_length\_b 20.0

\_cell\_length\_c 20.0

\_cell\_angle\_alpha 90.0

\_cell\_angle\_beta 90.0

\_cell\_angle\_gamma 90.0

\_symmetry\_space\_group\_name\_H-M 'P 1'

\_symmetry\_Int\_Tables\_number 1

\_symmetry\_cell\_setting triclinic

loop\_

\_atom\_site\_label

\_atom\_site\_type\_symbol

\_atom\_site\_fract\_x

\_atom\_site\_fract\_y

\_atom\_site\_fract\_z

\_atom\_site\_occupancy

H1 H 0.9623794600000000 0.9010715400000000 0.0474641100000000 1.0

|     |   |                    |                    |                    |     |
|-----|---|--------------------|--------------------|--------------------|-----|
| H2  | H | 0.0902749100000000 | 0.9419564900000000 | 0.9296934300000000 | 1.0 |
| H3  | H | 0.8996665400000000 | 0.1242544600000000 | 0.0819709500000000 | 1.0 |
| H4  | H | 0.0802781800000000 | 0.1184204500000000 | 0.9190714200000000 | 1.0 |
| H5  | H | 0.2123678400000000 | 0.1045445100000000 | 0.0472368200000000 | 1.0 |
| H6  | H | 0.3394048500000000 | 0.0631134200000000 | 0.9291591300000000 | 1.0 |
| H7  | H | 0.1491725400000000 | 0.8813187300000000 | 0.0819809000000000 | 1.0 |
| H8  | H | 0.3314435600000000 | 0.8865426400000000 | 0.9200243200000000 | 1.0 |
| H9  | H | 0.4622885000000000 | 0.9018778100000000 | 0.0485973100000000 | 1.0 |
| H10 | H | 0.5893258900000000 | 0.9415697700000000 | 0.9300085700000000 | 1.0 |
| H11 | H | 0.3983711800000000 | 0.1263317100000000 | 0.0791465300000000 | 1.0 |
| H12 | H | 0.5816173600000000 | 0.1181105500000000 | 0.9185703600000000 | 1.0 |
| H13 | H | 0.7122328200000000 | 0.1043729400000000 | 0.0474030700000000 | 1.0 |
| H14 | H | 0.8401712200000000 | 0.0634652900000000 | 0.9296412700000000 | 1.0 |
| H15 | H | 0.6489535200000000 | 0.8806433600000000 | 0.0811856600000000 | 1.0 |
| H16 | H | 0.8304810900000000 | 0.8870614100000000 | 0.9191467900000000 | 1.0 |
| C17 | C | 0.9659737500000000 | 0.9493028000000000 | 0.0212992000000000 | 1.0 |
| C18 | C | 0.0897085000000000 | 0.9638071700000000 | 0.9798770100000000 | 1.0 |
| C19 | C | 0.0904408500000000 | 0.0418271800000000 | 0.9794356800000000 | 1.0 |
| C20 | C | 0.9649819500000000 | 0.0568050000000000 | 0.0212283800000000 | 1.0 |
| C21 | C | 0.2160085300000000 | 0.0562665900000000 | 0.0211399000000000 | 1.0 |
| C22 | C | 0.3395600600000000 | 0.0416674100000000 | 0.9795169800000000 | 1.0 |
| C23 | C | 0.3405858100000000 | 0.9636541000000000 | 0.9797210800000000 | 1.0 |
| C24 | C | 0.2149552300000000 | 0.9487738700000000 | 0.0213550500000000 | 1.0 |
| C25 | C | 0.4659719100000000 | 0.9497870200000000 | 0.0218375000000000 | 1.0 |
| C26 | C | 0.5895386900000000 | 0.9637496400000000 | 0.9800420400000000 | 1.0 |
| C27 | C | 0.5906544900000000 | 0.0417497700000000 | 0.9791873000000000 | 1.0 |
| C28 | C | 0.4649987800000000 | 0.0572721600000000 | 0.0205448000000000 | 1.0 |
| C29 | C | 0.7159602400000000 | 0.0561455300000000 | 0.0212430600000000 | 1.0 |
| C30 | C | 0.8397153800000000 | 0.0416760900000000 | 0.9798461100000000 | 1.0 |
| C31 | C | 0.8404971600000000 | 0.9636718900000000 | 0.9794618700000000 | 1.0 |
| C32 | C | 0.7149862500000000 | 0.9486422900000000 | 0.0212234600000000 | 1.0 |
| O33 | O | 0.9656105600000000 | 0.0029098700000000 | 0.0691777700000000 | 1.0 |
| O34 | O | 0.0901705900000000 | 0.0701783700000000 | 0.9143971100000000 | 1.0 |
| O35 | O | 0.9733097900000000 | 0.1191222800000000 | 0.0519152100000000 | 1.0 |
| O36 | O | 0.2156234900000000 | 0.0027999500000000 | 0.0691530600000000 | 1.0 |
| O37 | O | 0.3410503700000000 | 0.9347582000000000 | 0.9149208600000000 | 1.0 |
| O38 | O | 0.2232030600000000 | 0.8865312600000000 | 0.0521925400000000 | 1.0 |
| O39 | O | 0.4656128300000000 | 0.0039307300000000 | 0.0691225400000000 | 1.0 |
| O40 | O | 0.5912004500000000 | 0.0698345400000000 | 0.9140435100000000 | 1.0 |
| O41 | O | 0.4734246100000000 | 0.1200419600000000 | 0.0502718100000000 | 1.0 |
| O42 | O | 0.7155861200000000 | 0.0025621500000000 | 0.0691530800000000 | 1.0 |
| O43 | O | 0.8404221200000000 | 0.9352959800000000 | 0.9144376400000000 | 1.0 |
| O44 | O | 0.7234843600000000 | 0.8862904900000000 | 0.0518186600000000 | 1.0 |

##### cif ends

furan\_OH\_23\_syn\_alt\_forbid Energy: -277.60172584

##### cif starts

data\_furan\_OH\_23\_syn\_alt\_forbid

\_publ\_section\_comment

;  
 Andrew Reynoso, Bohan Xu, and Vincent H. Crespi  
 ;

\_cell\_length\_a 9.5614916636  
\_cell\_length\_b 20.0  
\_cell\_length\_c 20.0  
\_cell\_angle\_alpha 90.0  
\_cell\_angle\_beta 90.0  
\_cell\_angle\_gamma 90.0

\_symmetry\_space\_group\_name\_H-M 'P 1'  
\_symmetry\_Int\_Tables\_number 1  
\_symmetry\_cell\_setting triclinic

loop\_  
\_atom\_site\_label  
\_atom\_site\_type\_symbol  
\_atom\_site\_fract\_x  
\_atom\_site\_fract\_y  
\_atom\_site\_fract\_z  
\_atom\_site\_occupancy

|     |   |                    |                    |                    |     |
|-----|---|--------------------|--------------------|--------------------|-----|
| H1  | H | 0.0033026200000000 | 0.0975479000000000 | 0.0619486300000000 | 1.0 |
| H2  | H | 0.0029730300000000 | 0.0556671600000000 | 0.9281211900000000 | 1.0 |
| H3  | H | 0.2489587300000000 | 0.9331040000000000 | 0.9317446900000000 | 1.0 |
| H4  | H | 0.2492078500000000 | 0.8992224400000000 | 0.0678602100000000 | 1.0 |
| H5  | H | 0.5031768800000000 | 0.0970512700000000 | 0.0623905600000000 | 1.0 |
| H6  | H | 0.5034793500000000 | 0.0557041400000000 | 0.9283576600000000 | 1.0 |
| H7  | H | 0.7493997700000000 | 0.9331467300000000 | 0.9315374600000000 | 1.0 |
| H8  | H | 0.7491629900000000 | 0.8987422200000000 | 0.0674820800000000 | 1.0 |
| H9  | H | 0.9799785300000000 | 0.8776013200000000 | 0.9188171900000000 | 1.0 |
| H10 | H | 0.5500964800000000 | 0.8714142700000000 | 0.1091518500000000 | 1.0 |
| H11 | H | 0.4796415600000000 | 0.8776500100000000 | 0.9185069700000000 | 1.0 |
| H12 | H | 0.0500952000000000 | 0.8721749700000000 | 0.1097685200000000 | 1.0 |
| H13 | H | 0.2023433700000000 | 0.1271234200000000 | 0.1020556600000000 | 1.0 |
| H14 | H | 0.2726592300000000 | 0.1103075700000000 | 0.9120785700000000 | 1.0 |
| H15 | H | 0.7023013600000000 | 0.1264391800000000 | 0.1026941500000000 | 1.0 |
| H16 | H | 0.7722870700000000 | 0.1104026500000000 | 0.9123940600000000 | 1.0 |
| C17 | C | 0.0410486200000000 | 0.0515815100000000 | 0.0380600800000000 | 1.0 |
| C18 | C | 0.9604314100000000 | 0.0339954600000000 | 0.9740561300000000 | 1.0 |
| C19 | C | 0.9583895300000000 | 0.9560261700000000 | 0.9755837000000000 | 1.0 |
| C20 | C | 0.0416574100000000 | 0.9407995100000000 | 0.0411510600000000 | 1.0 |
| C21 | C | 0.2108017300000000 | 0.0544360500000000 | 0.0377510600000000 | 1.0 |
| C22 | C | 0.2941398000000000 | 0.0352889600000000 | 0.9732742300000000 | 1.0 |
| C23 | C | 0.2918909600000000 | 0.9573760900000000 | 0.9762687600000000 | 1.0 |
| C24 | C | 0.2114409700000000 | 0.9436768100000000 | 0.0412738500000000 | 1.0 |
| C25 | C | 0.5409624500000000 | 0.0511958000000000 | 0.0383057500000000 | 1.0 |
| C26 | C | 0.4605361700000000 | 0.0339184600000000 | 0.9741466700000000 | 1.0 |
| C27 | C | 0.4582918500000000 | 0.9559484600000000 | 0.9754705600000000 | 1.0 |
| C28 | C | 0.5416348800000000 | 0.9404065100000000 | 0.0409064900000000 | 1.0 |
| C29 | C | 0.7107448700000000 | 0.0540774200000000 | 0.0380287300000000 | 1.0 |
| C30 | C | 0.7940159500000000 | 0.0352415600000000 | 0.9734043000000000 | 1.0 |
| C31 | C | 0.7919875500000000 | 0.9573179400000000 | 0.9761965200000000 | 1.0 |
| C32 | C | 0.7113897500000000 | 0.9433018000000000 | 0.0410759100000000 | 1.0 |
| O33 | O | 0.0064790500000000 | 0.9970655200000000 | 0.0818725900000000 | 1.0 |
| O34 | O | 0.0116470300000000 | 0.9238913700000000 | 0.9175299800000000 | 1.0 |
| O35 | O | 0.9946156700000000 | 0.8808881400000000 | 0.0697961100000000 | 1.0 |
| O36 | O | 0.2459860200000000 | 0.0007253400000000 | 0.0817626100000000 | 1.0 |
| O37 | O | 0.2579183400000000 | 0.1159626300000000 | 0.0627272300000000 | 1.0 |

|     |   |                    |                    |                    |     |
|-----|---|--------------------|--------------------|--------------------|-----|
| O38 | O | 0.2411516100000000 | 0.0639929000000000 | 0.9134071100000000 | 1.0 |
| O39 | O | 0.5064098400000000 | 0.9964664300000000 | 0.0818799100000000 | 1.0 |
| O40 | O | 0.5112460700000000 | 0.9239529700000000 | 0.9172803800000000 | 1.0 |
| O41 | O | 0.4945721900000000 | 0.8803422800000000 | 0.0692407500000000 | 1.0 |
| O42 | O | 0.7459250700000000 | 0.0001666200000000 | 0.0818087700000000 | 1.0 |
| O43 | O | 0.7578061200000000 | 0.1154942300000000 | 0.0632829800000000 | 1.0 |
| O44 | O | 0.7407004200000000 | 0.0640997300000000 | 0.9136741400000000 | 1.0 |

##### cif ends

  furan\_OH\_23\_syn\_dir   Energy: -281.25163687

##### cif starts

data\_furan\_OH\_23\_syn\_dir

\_publ\_section\_comment

;  
Andrew Reynoso, Bohan Xu, and Vincent H. Crespi  
;

\_cell\_length\_a 10.3699368648

\_cell\_length\_b 20.0

\_cell\_length\_c 20.0

\_cell\_angle\_alpha 90.0

\_cell\_angle\_beta 90.0

\_cell\_angle\_gamma 90.0

\_symmetry\_space\_group\_name\_H-M 'P 1'

\_symmetry\_Int\_Tables\_number 1

\_symmetry\_cell\_setting triclinic

loop\_

\_atom\_site\_label

\_atom\_site\_type\_symbol

\_atom\_site\_fract\_x

\_atom\_site\_fract\_y

\_atom\_site\_fract\_z

\_atom\_site\_occupancy

|     |   |                    |                    |                    |     |
|-----|---|--------------------|--------------------|--------------------|-----|
| H1  | H | 0.0020172800000000 | 0.1125488000000000 | 0.0242720500000000 | 1.0 |
| H2  | H | 0.1267471500000000 | 0.0503851600000000 | 0.9159372700000000 | 1.0 |
| H3  | H | 0.0853946400000000 | 0.8892646600000000 | 0.0854667100000000 | 1.0 |
| H4  | H | 0.2104693700000000 | 0.9073022100000000 | 0.9143660100000000 | 1.0 |
| H5  | H | 0.2519364200000000 | 0.1125800000000000 | 0.0241434200000000 | 1.0 |
| H6  | H | 0.3769568700000000 | 0.0503994900000000 | 0.9159435700000000 | 1.0 |
| H7  | H | 0.3354316200000000 | 0.8893033000000000 | 0.0854861600000000 | 1.0 |
| H8  | H | 0.4604096700000000 | 0.9073473800000000 | 0.9143072000000000 | 1.0 |
| H9  | H | 0.5018629400000000 | 0.1125381600000000 | 0.0242996900000000 | 1.0 |
| H10 | H | 0.6269483500000000 | 0.0505085700000000 | 0.9160340600000000 | 1.0 |
| H11 | H | 0.5854479900000000 | 0.8891902900000000 | 0.0853671200000000 | 1.0 |
| H12 | H | 0.7104443100000000 | 0.9074318400000000 | 0.9142392700000000 | 1.0 |
| H13 | H | 0.7519469900000000 | 0.1125034500000000 | 0.0244361500000000 | 1.0 |
| H14 | H | 0.8767296700000000 | 0.0504904700000000 | 0.9160282200000000 | 1.0 |
| H15 | H | 0.8354000200000000 | 0.8891444400000000 | 0.0853436900000000 | 1.0 |
| H16 | H | 0.9605088700000000 | 0.9073916700000000 | 0.9142947300000000 | 1.0 |
| C17 | C | 0.0019246800000000 | 0.0604288300000000 | 0.0069326800000000 | 1.0 |
| C18 | C | 0.1269223100000000 | 0.0386138300000000 | 0.9695782500000000 | 1.0 |

|     |   |                    |                    |                    |     |
|-----|---|--------------------|--------------------|--------------------|-----|
| C19 | C | 0.1267759000000000 | 0.9613874800000000 | 0.9840620500000000 | 1.0 |
| C20 | C | 0.0016794300000000 | 0.9545361700000000 | 0.0283367200000000 | 1.0 |
| C21 | C | 0.2519066600000000 | 0.0604418600000000 | 0.0068560300000000 | 1.0 |
| C22 | C | 0.3769686800000000 | 0.0386180200000000 | 0.9695820700000000 | 1.0 |
| C23 | C | 0.3767747800000000 | 0.9613909800000000 | 0.9840523500000000 | 1.0 |
| C24 | C | 0.2516845600000000 | 0.9545660800000000 | 0.0283521300000000 | 1.0 |
| C25 | C | 0.5018914100000000 | 0.0604228400000000 | 0.0069453400000000 | 1.0 |
| C26 | C | 0.6269685700000000 | 0.0386581400000000 | 0.9696575800000000 | 1.0 |
| C27 | C | 0.6267784500000000 | 0.9614105000000000 | 0.9840255900000000 | 1.0 |
| C28 | C | 0.5016867200000000 | 0.9545225600000000 | 0.0283171700000000 | 1.0 |
| C29 | C | 0.7519106100000000 | 0.0604077000000000 | 0.0070237000000000 | 1.0 |
| C30 | C | 0.8769213400000000 | 0.0386527800000000 | 0.9696542500000000 | 1.0 |
| C31 | C | 0.8767819100000000 | 0.9614073100000000 | 0.9840361200000000 | 1.0 |
| C32 | C | 0.7516796200000000 | 0.9544887200000000 | 0.0282977000000000 | 1.0 |
| O33 | O | 0.0016937800000000 | 0.0167167000000000 | 0.0642307800000000 | 1.0 |
| O34 | O | 0.1208381100000000 | 0.9172113100000000 | 0.9286231100000000 | 1.0 |
| O35 | O | 0.9963380900000000 | 0.8994683200000000 | 0.0702916800000000 | 1.0 |
| O36 | O | 0.2516783800000000 | 0.0167808400000000 | 0.0641926200000000 | 1.0 |
| O37 | O | 0.3707944900000000 | 0.9172290900000000 | 0.9286016400000000 | 1.0 |
| O38 | O | 0.2463590500000000 | 0.8995394100000000 | 0.0703593400000000 | 1.0 |
| O39 | O | 0.5016564100000000 | 0.0166932100000000 | 0.0642307600000000 | 1.0 |
| O40 | O | 0.6208163300000000 | 0.9173374000000000 | 0.9285020700000000 | 1.0 |
| O41 | O | 0.4963702200000000 | 0.8994419800000000 | 0.0702544100000000 | 1.0 |
| O42 | O | 0.7516729900000000 | 0.0166229500000000 | 0.0642688700000000 | 1.0 |
| O43 | O | 0.8708683700000000 | 0.9173232400000000 | 0.9285211800000000 | 1.0 |
| O44 | O | 0.7463405800000000 | 0.8993620800000000 | 0.0701768800000000 | 1.0 |

##### cif ends

furan\_OH\_23\_syn\_dir\_forbid Energy: -278.65356354

##### cif starts

data\_furan\_OH\_23\_syn\_dir\_forbid

\_publ\_section\_comment

;

Andrew Reynoso, Bohan Xu, and Vincent H. Crespi

;

\_cell\_length\_a 9.6782744253

\_cell\_length\_b 20.0

\_cell\_length\_c 20.0

\_cell\_angle\_alpha 90.0

\_cell\_angle\_beta 90.0

\_cell\_angle\_gamma 90.0

\_symmetry\_space\_group\_name\_H-M 'P 1'

\_symmetry\_Int\_Tables\_number 1

\_symmetry\_cell\_setting triclinic

loop\_

\_atom\_site\_label

\_atom\_site\_type\_symbol

\_atom\_site\_fract\_x

\_atom\_site\_fract\_y

\_atom\_site\_fract\_z

|     | atom | site               | occupancy          |                    |     |  |  |
|-----|------|--------------------|--------------------|--------------------|-----|--|--|
| H1  | H    | 0.0258528800000000 | 0.1082540600000000 | 0.0427812200000000 | 1.0 |  |  |
| H2  | H    | 0.0144646800000000 | 0.0466826000000000 | 0.9165073300000000 | 1.0 |  |  |
| H3  | H    | 0.2631062700000000 | 0.1017053200000000 | 0.0558812900000000 | 1.0 |  |  |
| H4  | H    | 0.2675799900000000 | 0.0586598700000000 | 0.9213045600000000 | 1.0 |  |  |
| H5  | H    | 0.5259536600000000 | 0.1078759200000000 | 0.0434440700000000 | 1.0 |  |  |
| H6  | H    | 0.5151113100000000 | 0.0468478800000000 | 0.9168309200000000 | 1.0 |  |  |
| H7  | H    | 0.7633576400000000 | 0.1012694900000000 | 0.0562919800000000 | 1.0 |  |  |
| H8  | H    | 0.7669299900000000 | 0.0586562800000000 | 0.9215229000000000 | 1.0 |  |  |
| H9  | H    | 0.9286854000000000 | 0.8954976500000000 | 0.9052568900000000 | 1.0 |  |  |
| H10 | H    | 0.1651515900000000 | 0.9118312800000000 | 0.9135358300000000 | 1.0 |  |  |
| H11 | H    | 0.4283895100000000 | 0.8957378300000000 | 0.9050315500000000 | 1.0 |  |  |
| H12 | H    | 0.6653431800000000 | 0.9118787200000000 | 0.9132834400000000 | 1.0 |  |  |
| H13 | H    | 0.9107133500000000 | 0.8870088200000000 | 0.0865725300000000 | 1.0 |  |  |
| H14 | H    | 0.1727307200000000 | 0.8686223000000000 | 0.0906315400000000 | 1.0 |  |  |
| H15 | H    | 0.4106606500000000 | 0.8867921400000000 | 0.0864608400000000 | 1.0 |  |  |
| H16 | H    | 0.6730652900000000 | 0.8680462500000000 | 0.0902433000000000 | 1.0 |  |  |
| C17 | C    | 0.0592584600000000 | 0.0582779800000000 | 0.0266950300000000 | 1.0 |  |  |
| C18 | C    | 0.9745688500000000 | 0.0323234700000000 | 0.9658179800000000 | 1.0 |  |  |
| C19 | C    | 0.9638596300000000 | 0.9548295300000000 | 0.9786019900000000 | 1.0 |  |  |
| C20 | C    | 0.0432233800000000 | 0.9489127600000000 | 0.0455835500000000 | 1.0 |  |  |
| C21 | C    | 0.2282662300000000 | 0.0559823000000000 | 0.0306596800000000 | 1.0 |  |  |
| C22 | C    | 0.3090918500000000 | 0.0367449800000000 | 0.9673995600000000 | 1.0 |  |  |
| C23 | C    | 0.2984222600000000 | 0.9590730800000000 | 0.9716104000000000 | 1.0 |  |  |
| C24 | C    | 0.2143462200000000 | 0.9451008700000000 | 0.0370336800000000 | 1.0 |  |  |
| C25 | C    | 0.5593272400000000 | 0.0579866700000000 | 0.0270845400000000 | 1.0 |  |  |
| C26 | C    | 0.4747954000000000 | 0.0323450100000000 | 0.9660190100000000 | 1.0 |  |  |
| C27 | C    | 0.4639516400000000 | 0.9548205000000000 | 0.9785320000000000 | 1.0 |  |  |
| C28 | C    | 0.5433995800000000 | 0.9485204900000000 | 0.0454474800000000 | 1.0 |  |  |
| C29 | C    | 0.7283508800000000 | 0.0556554700000000 | 0.0309318400000000 | 1.0 |  |  |
| C30 | C    | 0.8088507500000000 | 0.0366419900000000 | 0.9674827600000000 | 1.0 |  |  |
| C31 | C    | 0.7983999600000000 | 0.9589632700000000 | 0.9715620600000000 | 1.0 |  |  |
| C32 | C    | 0.7143990700000000 | 0.9447450700000000 | 0.0369043800000000 | 1.0 |  |  |
| O33 | O    | 0.0200249600000000 | 0.0119033800000000 | 0.0774462000000000 | 1.0 |  |  |
| O34 | O    | 0.0120685000000000 | 0.9067613600000000 | 0.9323214200000000 | 1.0 |  |  |
| O35 | O    | 0.0124297100000000 | 0.8973451700000000 | 0.0887129500000000 | 1.0 |  |  |
| O36 | O    | 0.2571516000000000 | 0.0014705700000000 | 0.0756976500000000 | 1.0 |  |  |
| O37 | O    | 0.2660545200000000 | 0.9242442600000000 | 0.9127802500000000 | 1.0 |  |  |
| O38 | O    | 0.2555933000000000 | 0.8848539700000000 | 0.0657407400000000 | 1.0 |  |  |
| O39 | O    | 0.5201583700000000 | 0.0113508900000000 | 0.0776146000000000 | 1.0 |  |  |
| O40 | O    | 0.5119624700000000 | 0.9069834500000000 | 0.9319741400000000 | 1.0 |  |  |
| O41 | O    | 0.5125785900000000 | 0.8967195300000000 | 0.0882849300000000 | 1.0 |  |  |
| O42 | O    | 0.7572862100000000 | 0.0009651600000000 | 0.0757572100000000 | 1.0 |  |  |
| O43 | O    | 0.7662957400000000 | 0.9241714000000000 | 0.9126702500000000 | 1.0 |  |  |
| O44 | O    | 0.7558349000000000 | 0.8844015800000000 | 0.0653744900000000 | 1.0 |  |  |

##### cif ends

furan\_OH\_245\_anti\_alt    Energy: -308.03683502

##### cif starts

data\_furan\_OH\_245\_anti\_alt

\_publ\_section\_comment

;  
Andrew Reynoso, Bohan Xu, and Vincent H. Crespi



;

\_cell\_length\_a 9.4279736135  
\_cell\_length\_b 20.0  
\_cell\_length\_c 20.0  
\_cell\_angle\_alpha 90.0  
\_cell\_angle\_beta 90.0  
\_cell\_angle\_gamma 90.0

\_symmetry\_space\_group\_name\_H-M 'P 1'  
\_symmetry\_Int\_Tables\_number 1  
\_symmetry\_cell\_setting triclinic

loop\_  
\_atom\_site\_label  
\_atom\_site\_type\_symbol  
\_atom\_site\_fract\_x  
\_atom\_site\_fract\_y  
\_atom\_site\_fract\_z  
\_atom\_site\_occupancy

|     |   |                    |                    |                    |     |
|-----|---|--------------------|--------------------|--------------------|-----|
| H1  | H | 0.9716874600000000 | 0.9347215600000000 | 0.0918131800000000 | 1.0 |
| H2  | H | 0.8768509900000000 | 0.8739203700000000 | 0.9396762900000000 | 1.0 |
| H3  | H | 0.0601275800000000 | 0.0873685500000000 | 0.0926166500000000 | 1.0 |
| H4  | H | 0.0465647100000000 | 0.1137612600000000 | 0.9124637800000000 | 1.0 |
| H5  | H | 0.2212394300000000 | 0.0419350300000000 | 0.9318956600000000 | 1.0 |
| H6  | H | 0.3081025900000000 | 0.1173941200000000 | 0.0942441300000000 | 1.0 |
| H7  | H | 0.1446195800000000 | 0.8796180900000000 | 0.9159506700000000 | 1.0 |
| H8  | H | 0.2958244200000000 | 0.8650881400000000 | 0.1133317300000000 | 1.0 |
| H9  | H | 0.4716875300000000 | 0.9347215900000000 | 0.0918110500000000 | 1.0 |
| H10 | H | 0.3768414500000000 | 0.8739241900000000 | 0.9396748800000000 | 1.0 |
| H11 | H | 0.5601302400000000 | 0.0873668900000000 | 0.0926166100000000 | 1.0 |
| H12 | H | 0.5465187000000000 | 0.1137433200000000 | 0.9124366300000000 | 1.0 |
| H13 | H | 0.7212430500000000 | 0.0419288300000000 | 0.9318935300000000 | 1.0 |
| H14 | H | 0.8080975800000000 | 0.1173993300000000 | 0.0942374100000000 | 1.0 |
| H15 | H | 0.6446226600000000 | 0.8796077200000000 | 0.9159593700000000 | 1.0 |
| H16 | H | 0.7957883300000000 | 0.8651108500000000 | 0.1133633800000000 | 1.0 |
| C17 | C | 0.0050078500000000 | 0.9333561700000000 | 0.9825010100000000 | 1.0 |
| C18 | C | 0.9224710200000000 | 0.9529045500000000 | 0.0455383000000000 | 1.0 |
| C19 | C | 0.9225255000000000 | 0.0309230700000000 | 0.0415311100000000 | 1.0 |
| C20 | C | 0.0098912600000000 | 0.0425330400000000 | 0.9757970800000000 | 1.0 |
| C21 | C | 0.2564637700000000 | 0.0445014000000000 | 0.0408685900000000 | 1.0 |
| C22 | C | 0.1729092800000000 | 0.0246132200000000 | 0.9786916500000000 | 1.0 |
| C23 | C | 0.1713383700000000 | 0.9467506200000000 | 0.9836208500000000 | 1.0 |
| C24 | C | 0.2589699100000000 | 0.9356670200000000 | 0.0493503300000000 | 1.0 |
| C25 | C | 0.5050068100000000 | 0.9333554700000000 | 0.9824997900000000 | 1.0 |
| C26 | C | 0.4224712800000000 | 0.9529043100000000 | 0.0455359700000000 | 1.0 |
| C27 | C | 0.4225268300000000 | 0.0309227300000000 | 0.0415301400000000 | 1.0 |
| C28 | C | 0.5098930800000000 | 0.0425321000000000 | 0.9757954000000000 | 1.0 |
| C29 | C | 0.7564642600000000 | 0.0445017800000000 | 0.0408665300000000 | 1.0 |
| C30 | C | 0.6729115500000000 | 0.0246102300000000 | 0.9786903000000000 | 1.0 |
| C31 | C | 0.6713377500000000 | 0.9467471100000000 | 0.9836231700000000 | 1.0 |
| C32 | C | 0.7589664700000000 | 0.9356685100000000 | 0.0493553200000000 | 1.0 |
| O33 | O | 0.9618883600000000 | 0.9864480800000000 | 0.9358722300000000 | 1.0 |
| O34 | O | 0.9783514900000000 | 0.8711843300000000 | 0.9551851100000000 | 1.0 |
| O35 | O | 0.9642923700000000 | 0.0677780600000000 | 0.0986330600000000 | 1.0 |

|     |   |                    |                    |                    |     |
|-----|---|--------------------|--------------------|--------------------|-----|
| O36 | O | 0.9765438800000000 | 0.1034331400000000 | 0.9467780300000000 | 1.0 |
| O37 | O | 0.2118175600000000 | 0.9924471600000000 | 0.0885665700000000 | 1.0 |
| O38 | O | 0.2244804200000000 | 0.1074124300000000 | 0.0653034200000000 | 1.0 |
| O39 | O | 0.2236308300000000 | 0.9103391100000000 | 0.9274927500000000 | 1.0 |
| O40 | O | 0.2254528800000000 | 0.8751794800000000 | 0.0791017200000000 | 1.0 |
| O41 | O | 0.4618899800000000 | 0.9864478800000000 | 0.9358708300000000 | 1.0 |
| O42 | O | 0.4783422000000000 | 0.8711843900000000 | 0.9551842400000000 | 1.0 |
| O43 | O | 0.4642946800000000 | 0.0677753000000000 | 0.0986331300000000 | 1.0 |
| O44 | O | 0.4765440300000000 | 0.1034324500000000 | 0.9467767600000000 | 1.0 |
| O45 | O | 0.7118158800000000 | 0.9924510700000000 | 0.0885671600000000 | 1.0 |
| O46 | O | 0.7244772800000000 | 0.1074139300000000 | 0.0652975700000000 | 1.0 |
| O47 | O | 0.7236324200000000 | 0.9103308500000000 | 0.9274984700000000 | 1.0 |
| O48 | O | 0.7254473200000000 | 0.8751844400000000 | 0.0791140600000000 | 1.0 |

##### cif ends

uran\_OH\_245\_anti\_alt\_forbid Energy: -307.91389667

##### cif starts

data\_uran\_OH\_245\_anti\_alt\_forbid

\_publ\_section\_comment

;  
Andrew Reynoso, Bohan Xu, and Vincent H. Crespi  
;

\_cell\_length\_a 10.2394900285

\_cell\_length\_b 20.0

\_cell\_length\_c 20.0

\_cell\_angle\_alpha 90.0

\_cell\_angle\_beta 90.0

\_cell\_angle\_gamma 90.0

\_symmetry\_space\_group\_name\_H-M 'P 1'

\_symmetry\_Int\_Tables\_number 1

\_symmetry\_cell\_setting triclinic

loop\_

\_atom\_site\_label

\_atom\_site\_type\_symbol

\_atom\_site\_fract\_x

\_atom\_site\_fract\_y

\_atom\_site\_fract\_z

\_atom\_site\_occupancy

|     |   |                    |                    |                    |     |
|-----|---|--------------------|--------------------|--------------------|-----|
| H1  | H | 0.9529787400000000 | 0.0605573900000000 | 0.0520289900000000 | 1.0 |
| H2  | H | 0.3211289400000000 | 0.9304918500000000 | 0.9159881000000000 | 1.0 |
| H3  | H | 0.4533874300000000 | 0.0607825000000000 | 0.0519447700000000 | 1.0 |
| H4  | H | 0.8207964100000000 | 0.9302139300000000 | 0.9160899400000000 | 1.0 |
| H5  | H | 0.0322329100000000 | 0.9024564300000000 | 0.0767458700000000 | 1.0 |
| H6  | H | 0.5320377000000000 | 0.9027120200000000 | 0.0769692900000000 | 1.0 |
| H7  | H | 0.2922635400000000 | 0.8825041200000000 | 0.0677271800000000 | 1.0 |
| H8  | H | 0.7922632200000000 | 0.8826330700000000 | 0.0679360900000000 | 1.0 |
| H9  | H | 0.2418388200000000 | 0.0886204000000000 | 0.8913151500000000 | 1.0 |
| H10 | H | 0.7422292000000000 | 0.0882945900000000 | 0.8909485800000000 | 1.0 |
| H11 | H | 0.9819042300000000 | 0.1085432100000000 | 0.9002971100000000 | 1.0 |
| H12 | H | 0.4818031300000000 | 0.1084149800000000 | 0.9000964600000000 | 1.0 |

|     |   |                    |                    |                    |     |
|-----|---|--------------------|--------------------|--------------------|-----|
| H13 | H | 0.9939652100000000 | 0.8782632100000000 | 0.8981134200000000 | 1.0 |
| H14 | H | 0.4931652300000000 | 0.8776859800000000 | 0.8990031300000000 | 1.0 |
| H15 | H | 0.2802259500000000 | 0.1127339800000000 | 0.0699619100000000 | 1.0 |
| H16 | H | 0.7813672000000000 | 0.1135340600000000 | 0.0687207100000000 | 1.0 |
| C17 | C | 0.0738695800000000 | 0.0524549300000000 | 0.9611563900000000 | 1.0 |
| C18 | C | 0.9524406400000000 | 0.0350444500000000 | 0.0034635900000000 | 1.0 |
| C19 | C | 0.9517041900000000 | 0.9561287900000000 | 0.0047180300000000 | 1.0 |
| C20 | C | 0.0746296800000000 | 0.9377186700000000 | 0.9622289600000000 | 1.0 |
| C21 | C | 0.1995414900000000 | 0.0533412100000000 | 0.0058083100000000 | 1.0 |
| C22 | C | 0.3224379600000000 | 0.0349304800000000 | 0.9633094100000000 | 1.0 |
| C23 | C | 0.3216964500000000 | 0.9560100600000000 | 0.9645500700000000 | 1.0 |
| C24 | C | 0.2002884800000000 | 0.9386128400000000 | 0.0068815700000000 | 1.0 |
| C25 | C | 0.5738854300000000 | 0.0523858000000000 | 0.9609652500000000 | 1.0 |
| C26 | C | 0.4525319800000000 | 0.0351468000000000 | 0.0034482600000000 | 1.0 |
| C27 | C | 0.4516815000000000 | 0.9562370800000000 | 0.0048148700000000 | 1.0 |
| C28 | C | 0.5745588400000000 | 0.9376536100000000 | 0.9624145500000000 | 1.0 |
| C29 | C | 0.6996069300000000 | 0.0534084000000000 | 0.0055673900000000 | 1.0 |
| C30 | C | 0.8224793800000000 | 0.0348034300000000 | 0.9631733800000000 | 1.0 |
| C31 | C | 0.8216263500000000 | 0.9558885500000000 | 0.9645660100000000 | 1.0 |
| C32 | C | 0.7002572900000000 | 0.9386813700000000 | 0.0070324300000000 | 1.0 |
| O33 | O | 0.0698259600000000 | 0.1091585000000000 | 0.9214829000000000 | 1.0 |
| O34 | O | 0.9455008600000000 | 0.9210662500000000 | 0.0662408600000000 | 1.0 |
| O35 | O | 0.0714035500000000 | 0.8784667600000000 | 0.9265619100000000 | 1.0 |
| O36 | O | 0.3285973200000000 | 0.0700323900000000 | 0.9018094700000000 | 1.0 |
| O37 | O | 0.2028477400000000 | 0.1126015100000000 | 0.0414636000000000 | 1.0 |
| O38 | O | 0.2043278100000000 | 0.8819138000000000 | 0.0465584100000000 | 1.0 |
| O39 | O | 0.0871436300000000 | 0.9938869200000000 | 0.9176851600000000 | 1.0 |
| O40 | O | 0.1870245000000000 | 0.9971796700000000 | 0.0503500500000000 | 1.0 |
| O41 | O | 0.5698717300000000 | 0.1089578000000000 | 0.9211210900000000 | 1.0 |
| O42 | O | 0.4452892100000000 | 0.9212613900000000 | 0.0663840900000000 | 1.0 |
| O43 | O | 0.5712298500000000 | 0.8782579600000000 | 0.9269962700000000 | 1.0 |
| O44 | O | 0.8289511200000000 | 0.0697588900000000 | 0.9015945600000000 | 1.0 |
| O45 | O | 0.7029811900000000 | 0.1128099300000000 | 0.0409682500000000 | 1.0 |
| O46 | O | 0.7042310600000000 | 0.8821003800000000 | 0.0468752400000000 | 1.0 |
| O47 | O | 0.5870416300000000 | 0.9936750800000000 | 0.9176690400000000 | 1.0 |
| O48 | O | 0.6871148700000000 | 0.9973836200000000 | 0.0503186500000000 | 1.0 |

##### cif ends

furand\_OH\_245\_anti\_dir Energy: -307.83975724

##### cif starts

data\_furand\_OH\_245\_anti\_dir

\_publ\_section\_comment

;  
Andrew Reynoso, Bohan Xu, and Vincent H. Crespi  
;

\_cell\_length\_a 9.4533413692

\_cell\_length\_b 20.0

\_cell\_length\_c 20.0

\_cell\_angle\_alpha 90.0

\_cell\_angle\_beta 90.0

\_cell\_angle\_gamma 90.0

\_symmetry\_space\_group\_name\_H-M 'P 1'  
\_symmetry\_Int\_Tables\_number 1  
\_symmetry\_cell\_setting triclinic

loop\_

\_atom\_site\_label  
\_atom\_site\_type\_symbol  
\_atom\_site\_fract\_x  
\_atom\_site\_fract\_y  
\_atom\_site\_fract\_z  
\_atom\_site\_occupancy

|     |   |                    |                    |                    |     |
|-----|---|--------------------|--------------------|--------------------|-----|
| H1  | H | 0.9812624200000000 | 0.0685590300000000 | 0.0637323500000000 | 1.0 |
| H2  | H | 0.0499037400000000 | 0.1343499200000000 | 0.8930743100000000 | 1.0 |
| H3  | H | 0.0714390000000000 | 0.9160529100000000 | 0.0768322600000000 | 1.0 |
| H4  | H | 0.0781168100000000 | 0.8775887300000000 | 0.9050217200000000 | 1.0 |
| H5  | H | 0.2288999200000000 | 0.0678496400000000 | 0.9126184300000000 | 1.0 |
| H6  | H | 0.3008717100000000 | 0.1360624100000000 | 0.0835540100000000 | 1.0 |
| H7  | H | 0.3218230300000000 | 0.9556316900000000 | 0.8867213600000000 | 1.0 |
| H8  | H | 0.3204281500000000 | 0.8847224400000000 | 0.0803471500000000 | 1.0 |
| H9  | H | 0.4811729500000000 | 0.0685430900000000 | 0.0637750700000000 | 1.0 |
| H10 | H | 0.5497976200000000 | 0.1344141500000000 | 0.8931273300000000 | 1.0 |
| H11 | H | 0.5714642200000000 | 0.9160280700000000 | 0.0767939700000000 | 1.0 |
| H12 | H | 0.5781931000000000 | 0.8777007500000000 | 0.9049293000000000 | 1.0 |
| H13 | H | 0.7288543200000000 | 0.0679205100000000 | 0.9126396200000000 | 1.0 |
| H14 | H | 0.8010260500000000 | 0.1360739000000000 | 0.0835714300000000 | 1.0 |
| H15 | H | 0.8218251300000000 | 0.9557960000000000 | 0.8867102200000000 | 1.0 |
| H16 | H | 0.8203645700000000 | 0.8847288600000000 | 0.0803349900000000 | 1.0 |
| C17 | C | 0.0173967100000000 | 0.0616087000000000 | 0.9549789100000000 | 1.0 |
| C18 | C | 0.9327061000000000 | 0.0466558700000000 | 0.0189579600000000 | 1.0 |
| C19 | C | 0.9344427300000000 | 0.9683830200000000 | 0.0215942200000000 | 1.0 |
| C20 | C | 0.0215819700000000 | 0.9507261700000000 | 0.9582547200000000 | 1.0 |
| C21 | C | 0.2685982600000000 | 0.0631812100000000 | 0.0217467500000000 | 1.0 |
| C22 | C | 0.1812485600000000 | 0.0470480100000000 | 0.9581731900000000 | 1.0 |
| C23 | C | 0.1840872400000000 | 0.9693867700000000 | 0.9578712400000000 | 1.0 |
| C24 | C | 0.2692096600000000 | 0.9538504800000000 | 0.0220402600000000 | 1.0 |
| C25 | C | 0.5173737700000000 | 0.0616493100000000 | 0.9550165100000000 | 1.0 |
| C26 | C | 0.4326720400000000 | 0.0466539600000000 | 0.0189799000000000 | 1.0 |
| C27 | C | 0.4344454300000000 | 0.9683781300000000 | 0.0215862700000000 | 1.0 |
| C28 | C | 0.5215958900000000 | 0.9507706900000000 | 0.9582320900000000 | 1.0 |
| C29 | C | 0.7686400300000000 | 0.0632113500000000 | 0.0217555300000000 | 1.0 |
| C30 | C | 0.6812382000000000 | 0.0471005600000000 | 0.9581950400000000 | 1.0 |
| C31 | C | 0.6840960200000000 | 0.9694408300000000 | 0.9578668300000000 | 1.0 |
| C32 | C | 0.7692078200000000 | 0.9538805200000000 | 0.0220377900000000 | 1.0 |
| O33 | O | 0.9736118200000000 | 0.0044232600000000 | 0.9122977900000000 | 1.0 |
| O34 | O | 0.9792707500000000 | 0.1219397500000000 | 0.9263384800000000 | 1.0 |
| O35 | O | 0.9766184700000000 | 0.9366414100000000 | 0.0816477000000000 | 1.0 |
| O36 | O | 0.9966252900000000 | 0.8878613300000000 | 0.9340320700000000 | 1.0 |
| O37 | O | 0.2240083900000000 | 0.0088203900000000 | 0.0655078400000000 | 1.0 |
| O38 | O | 0.2339280300000000 | 0.1251131600000000 | 0.0481295500000000 | 1.0 |
| O39 | O | 0.2283357900000000 | 0.9378733000000000 | 0.8984776100000000 | 1.0 |
| O40 | O | 0.2376383600000000 | 0.8927932100000000 | 0.0505891900000000 | 1.0 |
| O41 | O | 0.4735977900000000 | 0.0044844500000000 | 0.9123105400000000 | 1.0 |
| O42 | O | 0.4792169800000000 | 0.1219946300000000 | 0.9264116900000000 | 1.0 |
| O43 | O | 0.4766548500000000 | 0.9366284600000000 | 0.0816275800000000 | 1.0 |
| O44 | O | 0.4966823900000000 | 0.8879230300000000 | 0.9339481100000000 | 1.0 |

|     |   |                    |                    |                    |     |
|-----|---|--------------------|--------------------|--------------------|-----|
| O45 | O | 0.7240374000000000 | 0.0088507500000000 | 0.0655152100000000 | 1.0 |
| O46 | O | 0.7340562600000000 | 0.1251488400000000 | 0.0481502000000000 | 1.0 |
| O47 | O | 0.7283825800000000 | 0.9379670000000000 | 0.8984587800000000 | 1.0 |
| O48 | O | 0.7375978900000000 | 0.8928179100000000 | 0.0505692000000000 | 1.0 |

##### cif ends

furan\_OH\_245\_anti\_dir\_forbid    Energy: -307.97136233

##### cif starts

data\_furan\_OH\_245\_anti\_dir\_forbid

\_publ\_section\_comment

;  
Andrew Reynoso, Bohan Xu, and Vincent H. Crespi  
;

\_cell\_length\_a    10.2298208752

\_cell\_length\_b    20.0

\_cell\_length\_c    20.0

\_cell\_angle\_alpha    90.0

\_cell\_angle\_beta    90.0

\_cell\_angle\_gamma    90.0

\_symmetry\_space\_group\_name\_H-M    'P 1'

\_symmetry\_Int\_Tables\_number 1

\_symmetry\_cell\_setting triclinic

loop\_

\_atom\_site\_label

\_atom\_site\_type\_symbol

\_atom\_site\_fract\_x

\_atom\_site\_fract\_y

\_atom\_site\_fract\_z

\_atom\_site\_occupancy

|     |   |                    |                    |                    |     |
|-----|---|--------------------|--------------------|--------------------|-----|
| H1  | H | 0.9757731100000000 | 0.0664765300000000 | 0.0759773000000000 | 1.0 |
| H2  | H | 0.1396835000000000 | 0.1521881300000000 | 0.9626514300000000 | 1.0 |
| H3  | H | 0.0583566700000000 | 0.9078734500000000 | 0.0987412500000000 | 1.0 |
| H4  | H | 0.0093838700000000 | 0.8873904200000000 | 0.9269406700000000 | 1.0 |
| H5  | H | 0.3544892700000000 | 0.0647206800000000 | 0.9354757600000000 | 1.0 |
| H6  | H | 0.3189018500000000 | 0.1281591400000000 | 0.0791548900000000 | 1.0 |
| H7  | H | 0.2662517600000000 | 0.9046589500000000 | 0.9186913100000000 | 1.0 |
| H8  | H | 0.3159347200000000 | 0.8909731200000000 | 0.0915475900000000 | 1.0 |
| H9  | H | 0.4757674300000000 | 0.0664788900000000 | 0.0759705900000000 | 1.0 |
| H10 | H | 0.6397171700000000 | 0.1521839000000000 | 0.9626395100000000 | 1.0 |
| H11 | H | 0.5583505400000000 | 0.9078792300000000 | 0.0987416000000000 | 1.0 |
| H12 | H | 0.5093848200000000 | 0.8873904700000000 | 0.9269380600000000 | 1.0 |
| H13 | H | 0.8544951400000000 | 0.0647213800000000 | 0.9354836000000000 | 1.0 |
| H14 | H | 0.8188681100000000 | 0.1281401900000000 | 0.0791949800000000 | 1.0 |
| H15 | H | 0.7662535100000000 | 0.9046600600000000 | 0.9186935700000000 | 1.0 |
| H16 | H | 0.8159314200000000 | 0.8909694400000000 | 0.0915488200000000 | 1.0 |
| C17 | C | 0.0979557400000000 | 0.0608197600000000 | 0.9840129400000000 | 1.0 |
| C18 | C | 0.9767203000000000 | 0.0421211600000000 | 0.0267808700000000 | 1.0 |
| C19 | C | 0.9773896100000000 | 0.9634087700000000 | 0.0280116000000000 | 1.0 |
| C20 | C | 0.0999290700000000 | 0.9469134700000000 | 0.9851657200000000 | 1.0 |
| C21 | C | 0.2267937500000000 | 0.0617354900000000 | 0.0259104000000000 | 1.0 |

|     |   |                    |                    |                    |     |
|-----|---|--------------------|--------------------|--------------------|-----|
| C22 | C | 0.3487292700000000 | 0.0415220200000000 | 0.9849602800000000 | 1.0 |
| C23 | C | 0.3473870700000000 | 0.9626436100000000 | 0.9873627300000000 | 1.0 |
| C24 | C | 0.2249287300000000 | 0.9479524100000000 | 0.0309462100000000 | 1.0 |
| C25 | C | 0.5979595700000000 | 0.0608200400000000 | 0.9840116200000000 | 1.0 |
| C26 | C | 0.4767190800000000 | 0.0421228100000000 | 0.0267747600000000 | 1.0 |
| C27 | C | 0.4773881400000000 | 0.9634106500000000 | 0.0280079400000000 | 1.0 |
| C28 | C | 0.5999301300000000 | 0.9469131100000000 | 0.9851645200000000 | 1.0 |
| C29 | C | 0.7267908500000000 | 0.0617337300000000 | 0.0259150900000000 | 1.0 |
| C30 | C | 0.8487305700000000 | 0.0415214800000000 | 0.9849673500000000 | 1.0 |
| C31 | C | 0.8473878300000000 | 0.9626430000000000 | 0.9873668700000000 | 1.0 |
| C32 | C | 0.7249269000000000 | 0.9479502500000000 | 0.0309477800000000 | 1.0 |
| O33 | O | 0.1105647700000000 | 0.0036781700000000 | 0.9403805800000000 | 1.0 |
| O34 | O | 0.0822520000000000 | 0.1176547600000000 | 0.9445476000000000 | 1.0 |
| O35 | O | 0.9716909900000000 | 0.9271827600000000 | 0.0888312500000000 | 1.0 |
| O36 | O | 0.0974666400000000 | 0.8883870500000000 | 0.9480749200000000 | 1.0 |
| O37 | O | 0.2140149300000000 | 0.0069897700000000 | 0.0730096000000000 | 1.0 |
| O38 | O | 0.2322607800000000 | 0.1228107700000000 | 0.0594345600000000 | 1.0 |
| O39 | O | 0.3532481200000000 | 0.9236430800000000 | 0.9284029100000000 | 1.0 |
| O40 | O | 0.2275365700000000 | 0.8912378700000000 | 0.0707258000000000 | 1.0 |
| O41 | O | 0.6105730000000000 | 0.0036778500000000 | 0.9403796100000000 | 1.0 |
| O42 | O | 0.5822599700000000 | 0.1176557600000000 | 0.9445468500000000 | 1.0 |
| O43 | O | 0.4716860300000000 | 0.9271890000000000 | 0.0888298200000000 | 1.0 |
| O44 | O | 0.5974663600000000 | 0.8883868200000000 | 0.9480732700000000 | 1.0 |
| O45 | O | 0.7140057200000000 | 0.0069864000000000 | 0.0730117100000000 | 1.0 |
| O46 | O | 0.7322515000000000 | 0.1228065700000000 | 0.0594432800000000 | 1.0 |
| O47 | O | 0.8532504400000000 | 0.9236440900000000 | 0.9284063100000000 | 1.0 |
| O48 | O | 0.7275334300000000 | 0.8912355100000000 | 0.0707269500000000 | 1.0 |

##### cif ends

furan\_OH\_245\_syn\_alt    Energy: -308.4301575

##### cif starts

data\_furan\_OH\_245\_syn\_alt

\_publ\_section\_comment

;

Andrew Reynoso, Bohan Xu, and Vincent H. Crespi

;

\_cell\_length\_a    10.3831149879

\_cell\_length\_b    20.0

\_cell\_length\_c    20.0

\_cell\_angle\_alpha    90.0

\_cell\_angle\_beta    90.0

\_cell\_angle\_gamma    90.0

\_symmetry\_space\_group\_name\_H-M    'P 1'

\_symmetry\_Int\_Tables\_number    1

\_symmetry\_cell\_setting    triclinic

loop\_

\_atom\_site\_label

\_atom\_site\_type\_symbol

\_atom\_site\_fract\_x

\_atom\_site\_fract\_y

|     |   | _atom_site_fract_z |                      |                    |     |  |
|-----|---|--------------------|----------------------|--------------------|-----|--|
|     |   |                    | _atom_site_occupancy |                    |     |  |
| H1  | H | 0.1059750100000000 | 0.9319055300000000   | 0.9258401500000000 | 1.0 |  |
| H2  | H | 0.0642887300000000 | 0.8647185100000000   | 0.0618912800000000 | 1.0 |  |
| H3  | H | 0.1063405000000000 | 0.1093308700000000   | 0.9159192500000000 | 1.0 |  |
| H4  | H | 0.0632734400000000 | 0.1207389500000000   | 0.0633653200000000 | 1.0 |  |
| H5  | H | 0.3557282700000000 | 0.0543060000000000   | 0.9254638100000000 | 1.0 |  |
| H6  | H | 0.3142939600000000 | 0.1222401700000000   | 0.0611981500000000 | 1.0 |  |
| H7  | H | 0.3563952400000000 | 0.8768361500000000   | 0.9165931400000000 | 1.0 |  |
| H8  | H | 0.3132882300000000 | 0.8662327200000000   | 0.0640218800000000 | 1.0 |  |
| H9  | H | 0.6058683300000000 | 0.9317723800000000   | 0.9260127400000000 | 1.0 |  |
| H10 | H | 0.5642460100000000 | 0.8649852000000000   | 0.0622900400000000 | 1.0 |  |
| H11 | H | 0.6064883200000000 | 0.1091512100000000   | 0.9155830600000000 | 1.0 |  |
| H12 | H | 0.5633149600000000 | 0.1209925600000000   | 0.0629840200000000 | 1.0 |  |
| H13 | H | 0.8561064900000000 | 0.0543354100000000   | 0.9255355000000000 | 1.0 |  |
| H14 | H | 0.8142076000000000 | 0.1222694200000000   | 0.0612052000000000 | 1.0 |  |
| H15 | H | 0.8564709600000000 | 0.8768809900000000   | 0.9165001900000000 | 1.0 |  |
| H16 | H | 0.8133528200000000 | 0.8662781000000000   | 0.0640901200000000 | 1.0 |  |
| C17 | C | 0.9815906000000000 | 0.9395154800000000   | 0.0173696600000000 | 1.0 |  |
| C18 | C | 0.1059342100000000 | 0.9544426400000000   | 0.9756973600000000 | 1.0 |  |
| C19 | C | 0.1059317800000000 | 0.0320983300000000   | 0.9752827700000000 | 1.0 |  |
| C20 | C | 0.9797261600000000 | 0.0471212800000000   | 0.0171655500000000 | 1.0 |  |
| C21 | C | 0.2315862000000000 | 0.0471802800000000   | 0.0171114900000000 | 1.0 |  |
| C22 | C | 0.3558908200000000 | 0.0320714600000000   | 0.9754555900000000 | 1.0 |  |
| C23 | C | 0.3559815900000000 | 0.9544163600000000   | 0.9755084900000000 | 1.0 |  |
| C24 | C | 0.2297414100000000 | 0.9395745300000000   | 0.0173973500000000 | 1.0 |  |
| C25 | C | 0.4815867100000000 | 0.9396588800000000   | 0.0175289000000000 | 1.0 |  |
| C26 | C | 0.6059161200000000 | 0.9544383600000000   | 0.9758085000000000 | 1.0 |  |
| C27 | C | 0.6059750500000000 | 0.0320926800000000   | 0.9751840000000000 | 1.0 |  |
| C28 | C | 0.4797346800000000 | 0.0472660600000000   | 0.0169873000000000 | 1.0 |  |
| C29 | C | 0.7315856900000000 | 0.0472392800000000   | 0.0170476700000000 | 1.0 |  |
| C30 | C | 0.8559623400000000 | 0.0320599900000000   | 0.9755081200000000 | 1.0 |  |
| C31 | C | 0.8559121800000000 | 0.9544044200000000   | 0.9754920700000000 | 1.0 |  |
| C32 | C | 0.7297317400000000 | 0.9396325800000000   | 0.0175027000000000 | 1.0 |  |
| O33 | O | 0.9805877300000000 | 0.9934253900000000   | 0.0652003900000000 | 1.0 |  |
| O34 | O | 0.9756701900000000 | 0.8769320200000000   | 0.0477262000000000 | 1.0 |  |
| O35 | O | 0.1058399100000000 | 0.0608513300000000   | 0.9106529500000000 | 1.0 |  |
| O36 | O | 0.9752387500000000 | 0.1099028400000000   | 0.0473260500000000 | 1.0 |  |
| O37 | O | 0.2305896400000000 | 0.9934791800000000   | 0.0651890100000000 | 1.0 |  |
| O38 | O | 0.2256510900000000 | 0.1098921600000000   | 0.0471931400000000 | 1.0 |  |
| O39 | O | 0.3561083900000000 | 0.9252838600000000   | 0.9110476100000000 | 1.0 |  |
| O40 | O | 0.2252902000000000 | 0.8769118400000000   | 0.0478125100000000 | 1.0 |  |
| O41 | O | 0.4805774000000000 | 0.9937292100000000   | 0.0651873200000000 | 1.0 |  |
| O42 | O | 0.4756366600000000 | 0.8771900200000000   | 0.0481101100000000 | 1.0 |  |
| O43 | O | 0.6060521200000000 | 0.0606564500000000   | 0.9104712600000000 | 1.0 |  |
| O44 | O | 0.4752790700000000 | 0.1101536900000000   | 0.0469357000000000 | 1.0 |  |
| O45 | O | 0.7305799800000000 | 0.9936239000000000   | 0.0652037300000000 | 1.0 |  |
| O46 | O | 0.7256281700000000 | 0.1100044500000000   | 0.0470275100000000 | 1.0 |  |
| O47 | O | 0.8557265800000000 | 0.9253331800000000   | 0.9110034500000000 | 1.0 |  |
| O48 | O | 0.7252811600000000 | 0.8770403900000000   | 0.0480530000000000 | 1.0 |  |

##### cif ends

furan\_OH\_245\_syn\_alt\_forbid    Energy: -305.59741677

##### cif starts

data\_furan\_OH\_245\_syn\_alt\_forbid

\_publ\_section\_comment

;  
Andrew Reynoso, Bohan Xu, and Vincent H. Crespi  
;

\_cell\_length\_a 9.7535164262

\_cell\_length\_b 20.0

\_cell\_length\_c 20.0

\_cell\_angle\_alpha 90.0

\_cell\_angle\_beta 90.0

\_cell\_angle\_gamma 90.0

\_symmetry\_space\_group\_name\_H-M 'P 1'

\_symmetry\_Int\_Tables\_number 1

\_symmetry\_cell\_setting triclinic

loop\_

\_atom\_site\_label

\_atom\_site\_type\_symbol

\_atom\_site\_fract\_x

\_atom\_site\_fract\_y

\_atom\_site\_fract\_z

\_atom\_site\_occupancy

|     |   |                    |                    |                    |     |
|-----|---|--------------------|--------------------|--------------------|-----|
| H1  | H | 0.9044094700000000 | 0.0471530600000000 | 0.9095767300000000 | 1.0 |
| H2  | H | 0.1533715700000000 | 0.9314577900000000 | 0.9176711900000000 | 1.0 |
| H3  | H | 0.4044992500000000 | 0.0471206400000000 | 0.9095112800000000 | 1.0 |
| H4  | H | 0.6532411100000000 | 0.9314676900000000 | 0.9175934300000000 | 1.0 |
| H5  | H | 0.2390084400000000 | 0.8640368700000000 | 0.0809599500000000 | 1.0 |
| H6  | H | 0.7389412600000000 | 0.8638772300000000 | 0.0808023900000000 | 1.0 |
| H7  | H | 0.9220978300000000 | 0.8683816800000000 | 0.9180013700000000 | 1.0 |
| H8  | H | 0.4221313300000000 | 0.8683585500000000 | 0.9180698800000000 | 1.0 |
| H9  | H | 0.1354468300000000 | 0.1096356200000000 | 0.9010571100000000 | 1.0 |
| H10 | H | 0.6355003500000000 | 0.1096578600000000 | 0.9011174700000000 | 1.0 |
| H11 | H | 0.8186504100000000 | 0.1366616900000000 | 0.0618415300000000 | 1.0 |
| H12 | H | 0.3187438200000000 | 0.1367943700000000 | 0.0616824100000000 | 1.0 |
| H13 | H | 0.5028734800000000 | 0.8815096600000000 | 0.0738506100000000 | 1.0 |
| H14 | H | 0.0028573400000000 | 0.8814594500000000 | 0.0738293500000000 | 1.0 |
| H15 | H | 0.0548741900000000 | 0.1184160300000000 | 0.0572362400000000 | 1.0 |
| H16 | H | 0.5548408600000000 | 0.1183607000000000 | 0.0572466800000000 | 1.0 |
| C17 | C | 0.8594723200000000 | 0.0529714100000000 | 0.0193596700000000 | 1.0 |
| C18 | C | 0.9425099400000000 | 0.0294909800000000 | 0.9578853500000000 | 1.0 |
| C19 | C | 0.9507189000000000 | 0.9523526900000000 | 0.9656145600000000 | 1.0 |
| C20 | C | 0.8695787200000000 | 0.9427037100000000 | 0.0324766800000000 | 1.0 |
| C21 | C | 0.1881660000000000 | 0.0520072400000000 | 0.0248218300000000 | 1.0 |
| C22 | C | 0.1070445000000000 | 0.0331396300000000 | 0.9599575900000000 | 1.0 |
| C23 | C | 0.1152614300000000 | 0.9556742900000000 | 0.9630470000000000 | 1.0 |
| C24 | C | 0.1982747300000000 | 0.9409845400000000 | 0.0271952100000000 | 1.0 |
| C25 | C | 0.3594803800000000 | 0.0530520500000000 | 0.0192824400000000 | 1.0 |
| C26 | C | 0.4425232700000000 | 0.0294932000000000 | 0.9578467400000000 | 1.0 |
| C27 | C | 0.4506979000000000 | 0.9523597900000000 | 0.9656362300000000 | 1.0 |
| C28 | C | 0.3696117500000000 | 0.9428010600000000 | 0.0325367700000000 | 1.0 |
| C29 | C | 0.6881316100000000 | 0.0519146900000000 | 0.0248804300000000 | 1.0 |
| C30 | C | 0.6070543300000000 | 0.0331248600000000 | 0.9599687900000000 | 1.0 |



|     |   |                    |                    |                    |     |
|-----|---|--------------------|--------------------|--------------------|-----|
| C31 | C | 0.6152312900000000 | 0.9556569300000000 | 0.9630043400000000 | 1.0 |
| C32 | C | 0.6982665100000000 | 0.9408869300000000 | 0.0271193600000000 | 1.0 |
| O33 | O | 0.8966595000000000 | 0.0036359900000000 | 0.0679476700000000 | 1.0 |
| O34 | O | 0.9005320500000000 | 0.1168192100000000 | 0.0396281000000000 | 1.0 |
| O35 | O | 0.8959518700000000 | 0.9149699700000000 | 0.9115480100000000 | 1.0 |
| O36 | O | 0.9004542800000000 | 0.8879581900000000 | 0.0716751800000000 | 1.0 |
| O37 | O | 0.1610568100000000 | 0.9966094200000000 | 0.0684318800000000 | 1.0 |
| O38 | O | 0.1572788700000000 | 0.1116827600000000 | 0.0560066700000000 | 1.0 |
| O39 | O | 0.1617938900000000 | 0.0626293400000000 | 0.9012119000000000 | 1.0 |
| O40 | O | 0.1571871600000000 | 0.8805787100000000 | 0.0561452400000000 | 1.0 |
| O41 | O | 0.3966929500000000 | 0.0037820300000000 | 0.0679282000000000 | 1.0 |
| O42 | O | 0.4005889200000000 | 0.1169262200000000 | 0.0394610000000000 | 1.0 |
| O43 | O | 0.3958342200000000 | 0.9149275600000000 | 0.9116276400000000 | 1.0 |
| O44 | O | 0.4004918500000000 | 0.8881130600000000 | 0.0718126200000000 | 1.0 |
| O45 | O | 0.6610233500000000 | 0.9964577700000000 | 0.0684194800000000 | 1.0 |
| O46 | O | 0.6572285500000000 | 0.1115424500000000 | 0.0561472600000000 | 1.0 |
| O47 | O | 0.6618903500000000 | 0.0626576300000000 | 0.9012639000000000 | 1.0 |
| O48 | O | 0.6571423200000000 | 0.8804411400000000 | 0.0559875200000000 | 1.0 |

##### cif ends

furan\_OH\_245\_syn\_dir Energy: -308.90830487

##### cif starts

data\_furan\_OH\_245\_syn\_dir

\_publ\_section\_comment

;  
Andrew Reynoso, Bohan Xu, and Vincent H. Crespi  
;

\_cell\_length\_a 10.3947989135

\_cell\_length\_b 20.0

\_cell\_length\_c 20.0

\_cell\_angle\_alpha 90.0

\_cell\_angle\_beta 90.0

\_cell\_angle\_gamma 90.0

\_symmetry\_space\_group\_name\_H-M 'P 1'

\_symmetry\_Int\_Tables\_number 1

\_symmetry\_cell\_setting triclinic

loop\_

\_atom\_site\_label

\_atom\_site\_type\_symbol

\_atom\_site\_fract\_x

\_atom\_site\_fract\_y

\_atom\_site\_fract\_z

\_atom\_site\_occupancy

|    |   |                    |                    |                    |     |
|----|---|--------------------|--------------------|--------------------|-----|
| H1 | H | 0.1592057500000000 | 0.0476664700000000 | 0.9188587300000000 | 1.0 |
|----|---|--------------------|--------------------|--------------------|-----|

|    |   |                    |                    |                    |     |
|----|---|--------------------|--------------------|--------------------|-----|
| H2 | H | 0.1170241100000000 | 0.1342921600000000 | 0.0436585200000000 | 1.0 |
|----|---|--------------------|--------------------|--------------------|-----|

|    |   |                    |                    |                    |     |
|----|---|--------------------|--------------------|--------------------|-----|
| H3 | H | 0.0760717200000000 | 0.9035537800000000 | 0.9122177900000000 | 1.0 |
|----|---|--------------------|--------------------|--------------------|-----|

|    |   |                    |                    |                    |     |
|----|---|--------------------|--------------------|--------------------|-----|
| H4 | H | 0.9511316400000000 | 0.8797048400000000 | 0.0820559000000000 | 1.0 |
|----|---|--------------------|--------------------|--------------------|-----|

|    |   |                    |                    |                    |     |
|----|---|--------------------|--------------------|--------------------|-----|
| H5 | H | 0.4091366300000000 | 0.0476365300000000 | 0.9188262300000000 | 1.0 |
|----|---|--------------------|--------------------|--------------------|-----|

|    |   |                    |                    |                    |     |
|----|---|--------------------|--------------------|--------------------|-----|
| H6 | H | 0.3670459100000000 | 0.1343120100000000 | 0.0436066700000000 | 1.0 |
|----|---|--------------------|--------------------|--------------------|-----|

|    |   |                    |                    |                    |     |
|----|---|--------------------|--------------------|--------------------|-----|
| H7 | H | 0.3260712000000000 | 0.9035419700000000 | 0.9122364500000000 | 1.0 |
|----|---|--------------------|--------------------|--------------------|-----|

|     |   |                    |                    |                    |     |
|-----|---|--------------------|--------------------|--------------------|-----|
| H8  | H | 0.2011357900000000 | 0.8797126800000000 | 0.0820716000000000 | 1.0 |
| H9  | H | 0.6592214100000000 | 0.0476211700000000 | 0.9187987500000000 | 1.0 |
| H10 | H | 0.6170480400000000 | 0.1343426700000000 | 0.0435202400000000 | 1.0 |
| H11 | H | 0.5760537800000000 | 0.9035284500000000 | 0.9122443200000000 | 1.0 |
| H12 | H | 0.4511487700000000 | 0.8797695100000000 | 0.0821211300000000 | 1.0 |
| H13 | H | 0.9092898500000000 | 0.0476483100000000 | 0.9188315000000000 | 1.0 |
| H14 | H | 0.8670260300000000 | 0.1343256500000000 | 0.0435674000000000 | 1.0 |
| H15 | H | 0.8260426000000000 | 0.9035406200000000 | 0.9122301200000000 | 1.0 |
| H16 | H | 0.7011363500000000 | 0.8797641000000000 | 0.0821034500000000 | 1.0 |
| C17 | C | 0.0338476100000000 | 0.0542733400000000 | 0.0098963500000000 | 1.0 |
| C18 | C | 0.1590854800000000 | 0.0331061700000000 | 0.9717381200000000 | 1.0 |
| C19 | C | 0.1593049400000000 | 0.9556692600000000 | 0.9834966700000000 | 1.0 |
| C20 | C | 0.0344077500000000 | 0.9473184800000000 | 0.0275793400000000 | 1.0 |
| C21 | C | 0.2838485100000000 | 0.0542793600000000 | 0.0098897800000000 | 1.0 |
| C22 | C | 0.4090684100000000 | 0.0331011300000000 | 0.9717124800000000 | 1.0 |
| C23 | C | 0.4093029800000000 | 0.9556686000000000 | 0.9835057200000000 | 1.0 |
| C24 | C | 0.2844100800000000 | 0.9473270300000000 | 0.0275910500000000 | 1.0 |
| C25 | C | 0.5338505500000000 | 0.0542982000000000 | 0.0098361200000000 | 1.0 |
| C26 | C | 0.6590896300000000 | 0.0330982500000000 | 0.9716883200000000 | 1.0 |
| C27 | C | 0.6593029400000000 | 0.9556688900000000 | 0.9834999700000000 | 1.0 |
| C28 | C | 0.5344144200000000 | 0.9473566600000000 | 0.0276004400000000 | 1.0 |
| C29 | C | 0.7838496500000000 | 0.0542923700000000 | 0.0098419300000000 | 1.0 |
| C30 | C | 0.9091070700000000 | 0.0331025700000000 | 0.9717147400000000 | 1.0 |
| C31 | C | 0.9093039400000000 | 0.9556688900000000 | 0.9834917500000000 | 1.0 |
| C32 | C | 0.7844112500000000 | 0.9473484800000000 | 0.0275892400000000 | 1.0 |
| O33 | O | 0.0342860900000000 | 0.0079321200000000 | 0.0656974400000000 | 1.0 |
| O34 | O | 0.0285163200000000 | 0.1203173300000000 | 0.0312854300000000 | 1.0 |
| O35 | O | 0.1653403400000000 | 0.9134318400000000 | 0.9266896500000000 | 1.0 |
| O36 | O | 0.0398086100000000 | 0.8904539100000000 | 0.0670502500000000 | 1.0 |
| O37 | O | 0.2842998900000000 | 0.0079473000000000 | 0.0656983200000000 | 1.0 |
| O38 | O | 0.2785254400000000 | 0.1203261500000000 | 0.0312684500000000 | 1.0 |
| O39 | O | 0.4153409700000000 | 0.9134007600000000 | 0.9267215500000000 | 1.0 |
| O40 | O | 0.2898131600000000 | 0.8904719200000000 | 0.0670753500000000 | 1.0 |
| O41 | O | 0.5343075600000000 | 0.0080013000000000 | 0.0656721800000000 | 1.0 |
| O42 | O | 0.5285315700000000 | 0.1203611400000000 | 0.0311665800000000 | 1.0 |
| O43 | O | 0.6653258000000000 | 0.9133842500000000 | 0.9267282900000000 | 1.0 |
| O44 | O | 0.5398263000000000 | 0.8905311000000000 | 0.0671252100000000 | 1.0 |
| O45 | O | 0.7842921500000000 | 0.0079861600000000 | 0.0656712100000000 | 1.0 |
| O46 | O | 0.7785217800000000 | 0.1203529600000000 | 0.0311805100000000 | 1.0 |
| O47 | O | 0.9153171600000000 | 0.9134148900000000 | 0.9266971400000000 | 1.0 |
| O48 | O | 0.7898144600000000 | 0.8905113900000000 | 0.0670981200000000 | 1.0 |

##### cif ends

furan\_OH\_245\_syn\_dir\_forbid Energy: -306.26930867

##### cif starts

data\_furan\_OH\_245\_syn\_dir\_forbid

\_publ\_section\_comment

;  
Andrew Reynoso, Bohan Xu, and Vincent H. Crespi  
;

\_cell\_length\_a 9.7567283817

\_cell\_length\_b 20.0

\_cell\_length\_c 20.0  
\_cell\_angle\_alpha 90.0  
\_cell\_angle\_beta 90.0  
\_cell\_angle\_gamma 90.0

\_symmetry\_space\_group\_name\_H-M 'P 1'  
\_symmetry\_Int\_Tables\_number 1  
\_symmetry\_cell\_setting triclinic

loop\_  
\_atom\_site\_label  
\_atom\_site\_type\_symbol  
\_atom\_site\_fract\_x  
\_atom\_site\_fract\_y  
\_atom\_site\_fract\_z  
\_atom\_site\_occupancy

|     |   |                    |                    |                    |     |
|-----|---|--------------------|--------------------|--------------------|-----|
| H1  | H | 0.8958985800000000 | 0.0442780000000000 | 0.9107261700000000 | 1.0 |
| H2  | H | 0.1406460300000000 | 0.0575135300000000 | 0.9181310000000000 | 1.0 |
| H3  | H | 0.3958870600000000 | 0.0442987300000000 | 0.9107455800000000 | 1.0 |
| H4  | H | 0.6406338900000000 | 0.0575394200000000 | 0.9181439200000000 | 1.0 |
| H5  | H | 0.8087540700000000 | 0.1371472300000000 | 0.0612545600000000 | 1.0 |
| H6  | H | 0.0463387800000000 | 0.1177759000000000 | 0.0584328600000000 | 1.0 |
| H7  | H | 0.3087506200000000 | 0.1371290000000000 | 0.0612921800000000 | 1.0 |
| H8  | H | 0.5463569900000000 | 0.1177712200000000 | 0.0584720700000000 | 1.0 |
| H9  | H | 0.9978766500000000 | 0.8801417900000000 | 0.0765885500000000 | 1.0 |
| H10 | H | 0.2359037700000000 | 0.8606952300000000 | 0.0798973200000000 | 1.0 |
| H11 | H | 0.4978817700000000 | 0.8801043800000000 | 0.0765337800000000 | 1.0 |
| H12 | H | 0.7359182000000000 | 0.8607138300000000 | 0.0799018300000000 | 1.0 |
| H13 | H | 0.9807226500000000 | 0.8934826300000000 | 0.8951771500000000 | 1.0 |
| H14 | H | 0.2434730500000000 | 0.9100849700000000 | 0.9046334000000000 | 1.0 |
| H15 | H | 0.4807472200000000 | 0.8935663200000000 | 0.8951147000000000 | 1.0 |
| H16 | H | 0.7434799800000000 | 0.9100869100000000 | 0.9046372800000000 | 1.0 |
| C17 | C | 0.8501916500000000 | 0.0528233300000000 | 0.0206125000000000 | 1.0 |
| C18 | C | 0.9344013700000000 | 0.0279945900000000 | 0.9595833200000000 | 1.0 |
| C19 | C | 0.9457641000000000 | 0.9504933700000000 | 0.9704115600000000 | 1.0 |
| C20 | C | 0.8661829800000000 | 0.9428183000000000 | 0.0370389400000000 | 1.0 |
| C21 | C | 0.1787352000000000 | 0.0507549600000000 | 0.0268981800000000 | 1.0 |
| C22 | C | 0.0984995200000000 | 0.0331810200000000 | 0.9627286400000000 | 1.0 |
| C23 | C | 0.1107594700000000 | 0.9553660200000000 | 0.9641947900000000 | 1.0 |
| C24 | C | 0.1950477300000000 | 0.9392094800000000 | 0.0289735000000000 | 1.0 |
| C25 | C | 0.3501969000000000 | 0.0528126100000000 | 0.0206328200000000 | 1.0 |
| C26 | C | 0.4344031000000000 | 0.0280067800000000 | 0.9595970700000000 | 1.0 |
| C27 | C | 0.4457622900000000 | 0.9505036300000000 | 0.9703987900000000 | 1.0 |
| C28 | C | 0.3661710500000000 | 0.9427973600000000 | 0.0370222400000000 | 1.0 |
| C29 | C | 0.6787355800000000 | 0.0507625800000000 | 0.0269038400000000 | 1.0 |
| C30 | C | 0.5984916500000000 | 0.0331981100000000 | 0.9627376000000000 | 1.0 |
| C31 | C | 0.6107723700000000 | 0.9553846500000000 | 0.9641892100000000 | 1.0 |
| C32 | C | 0.6950645400000000 | 0.9392195700000000 | 0.0289687600000000 | 1.0 |
| O33 | O | 0.8892607600000000 | 0.0051777900000000 | 0.0703897200000000 | 1.0 |
| O34 | O | 0.8901879100000000 | 0.1173993600000000 | 0.0385562800000000 | 1.0 |
| O35 | O | 0.8983344000000000 | 0.9039315400000000 | 0.9226779200000000 | 1.0 |
| O36 | O | 0.8969385100000000 | 0.8900718300000000 | 0.0785384400000000 | 1.0 |
| O37 | O | 0.1534796500000000 | 0.9937513400000000 | 0.0698402800000000 | 1.0 |
| O38 | O | 0.1476402100000000 | 0.1087917700000000 | 0.0607418600000000 | 1.0 |
| O39 | O | 0.1437264000000000 | 0.9227238700000000 | 0.9042900100000000 | 1.0 |

|     |   |                    |                    |                    |     |
|-----|---|--------------------|--------------------|--------------------|-----|
| O40 | O | 0.1541995600000000 | 0.8778951800000000 | 0.0554365000000000 | 1.0 |
| O41 | O | 0.3892520100000000 | 0.0051467000000000 | 0.0703946400000000 | 1.0 |
| O42 | O | 0.3901985700000000 | 0.1173778700000000 | 0.0386088900000000 | 1.0 |
| O43 | O | 0.3983560300000000 | 0.9039724600000000 | 0.9226314200000000 | 1.0 |
| O44 | O | 0.3969416000000000 | 0.8900309100000000 | 0.0784934800000000 | 1.0 |
| O45 | O | 0.6534851200000000 | 0.9937552100000000 | 0.0698415300000000 | 1.0 |
| O46 | O | 0.6476620300000000 | 0.1087950700000000 | 0.0607620900000000 | 1.0 |
| O47 | O | 0.6437552100000000 | 0.9227672900000000 | 0.9042733700000000 | 1.0 |
| O48 | O | 0.6542307000000000 | 0.8778965500000000 | 0.0554144700000000 | 1.0 |

##### cif ends

furand\_OH\_24\_anti\_alt    Energy: -280.88914473

##### cif starts

data\_furand\_OH\_24\_anti\_alt

\_publ\_section\_comment

;  
Andrew Reynoso, Bohan Xu, and Vincent H. Crespi  
;

\_cell\_length\_a    9.4592667167

\_cell\_length\_b    20.0

\_cell\_length\_c    20.0

\_cell\_angle\_alpha    90.0

\_cell\_angle\_beta    90.0

\_cell\_angle\_gamma    90.0

\_symmetry\_space\_group\_name\_H-M    'P 1'

\_symmetry\_Int\_Tables\_number 1

\_symmetry\_cell\_setting triclinic

loop\_

\_atom\_site\_label

\_atom\_site\_type\_symbol

\_atom\_site\_fract\_x

\_atom\_site\_fract\_y

\_atom\_site\_fract\_z

\_atom\_site\_occupancy

|     |   |                    |                    |                    |     |
|-----|---|--------------------|--------------------|--------------------|-----|
| H1  | H | 0.0004693000000000 | 0.9556924500000000 | 0.0838037200000000 | 1.0 |
| H2  | H | 0.0138429900000000 | 0.0898272800000000 | 0.9223248000000000 | 1.0 |
| H3  | H | 0.0975786100000000 | 0.8594674200000000 | 0.9338849000000000 | 1.0 |
| H4  | H | 0.0911945400000000 | 0.0682969900000000 | 0.0890775000000000 | 1.0 |
| H5  | H | 0.2504780900000000 | 0.0441351200000000 | 0.9112492300000000 | 1.0 |
| H6  | H | 0.2638513900000000 | 0.9100225900000000 | 0.0727437900000000 | 1.0 |
| H7  | H | 0.3475320100000000 | 0.1403950600000000 | 0.0611316600000000 | 1.0 |
| H8  | H | 0.3412060600000000 | 0.9316534000000000 | 0.9059395300000000 | 1.0 |
| H9  | H | 0.5004706100000000 | 0.9557389700000000 | 0.0838358500000000 | 1.0 |
| H10 | H | 0.5138504300000000 | 0.0897853100000000 | 0.9222850800000000 | 1.0 |
| H11 | H | 0.5974647100000000 | 0.8593812600000000 | 0.9340116800000000 | 1.0 |
| H12 | H | 0.5912730100000000 | 0.0683563900000000 | 0.0890426400000000 | 1.0 |
| H13 | H | 0.7504710000000000 | 0.0440730600000000 | 0.9112115300000000 | 1.0 |
| H14 | H | 0.7638645100000000 | 0.9099818500000000 | 0.0727137600000000 | 1.0 |
| H15 | H | 0.8474800500000000 | 0.1403606400000000 | 0.0611113200000000 | 1.0 |
| H16 | H | 0.8412483200000000 | 0.9313701800000000 | 0.9060082300000000 | 1.0 |

|     |   |                    |                    |                    |     |
|-----|---|--------------------|--------------------|--------------------|-----|
| C17 | C | 0.0413389600000000 | 0.9388647700000000 | 0.9769359300000000 | 1.0 |
| C18 | C | 0.9531785500000000 | 0.9666133500000000 | 0.0349555000000000 | 1.0 |
| C19 | C | 0.9542092400000000 | 0.0431513100000000 | 0.0204091600000000 | 1.0 |
| C20 | C | 0.0399059700000000 | 0.0468858500000000 | 0.9540477800000000 | 1.0 |
| C21 | C | 0.2913165100000000 | 0.0609829700000000 | 0.0181078700000000 | 1.0 |
| C22 | C | 0.2031714000000000 | 0.0332165600000000 | 0.9600923400000000 | 1.0 |
| C23 | C | 0.2042337500000000 | 0.9566817700000000 | 0.9746345900000000 | 1.0 |
| C24 | C | 0.2899144500000000 | 0.9529579700000000 | 0.0410108600000000 | 1.0 |
| C25 | C | 0.5413021000000000 | 0.9388385600000000 | 0.9769776500000000 | 1.0 |
| C26 | C | 0.4531780100000000 | 0.9666401500000000 | 0.0349837300000000 | 1.0 |
| C27 | C | 0.4542274600000000 | 0.0431718000000000 | 0.0204083800000000 | 1.0 |
| C28 | C | 0.5399020500000000 | 0.0468586300000000 | 0.9540296600000000 | 1.0 |
| C29 | C | 0.7913076000000000 | 0.0609444000000000 | 0.0180786300000000 | 1.0 |
| C30 | C | 0.7031703500000000 | 0.0331700500000000 | 0.9600594500000000 | 1.0 |
| C31 | C | 0.7042068200000000 | 0.9566355200000000 | 0.9746237300000000 | 1.0 |
| C32 | C | 0.7899142500000000 | 0.9529220400000000 | 0.0409847500000000 | 1.0 |
| O33 | O | 0.9957024900000000 | 0.9854623700000000 | 0.9216010200000000 | 1.0 |
| O34 | O | 0.0168299500000000 | 0.8730505600000000 | 0.9620811300000000 | 1.0 |
| O35 | O | 0.9998023900000000 | 0.0849102500000000 | 0.0730668700000000 | 1.0 |
| O36 | O | 0.2457039800000000 | 0.0143860600000000 | 0.0734455900000000 | 1.0 |
| O37 | O | 0.2667738700000000 | 0.1267944200000000 | 0.0329512300000000 | 1.0 |
| O38 | O | 0.2498913600000000 | 0.9149508800000000 | 0.9219678600000000 | 1.0 |
| O39 | O | 0.4956625800000000 | 0.9854242200000000 | 0.9216121800000000 | 1.0 |
| O40 | O | 0.5167424200000000 | 0.8730179400000000 | 0.9621966500000000 | 1.0 |
| O41 | O | 0.4998595700000000 | 0.0849503900000000 | 0.0730424200000000 | 1.0 |
| O42 | O | 0.7456831800000000 | 0.0143471700000000 | 0.0734169500000000 | 1.0 |
| O43 | O | 0.7667472500000000 | 0.1267580100000000 | 0.0329154800000000 | 1.0 |
| O44 | O | 0.7497596800000000 | 0.9148486300000000 | 0.9219788400000000 | 1.0 |

##### cif ends

furand\_OH\_24\_anti\_alt\_forbid Energy: -281.25811183

##### cif starts

data\_furand\_OH\_24\_anti\_alt\_forbid

\_publ\_section\_comment

;  
Andrew Reynoso, Bohan Xu, and Vincent H. Crespi  
;

\_cell\_length\_a 10.2143876071

\_cell\_length\_b 20.0

\_cell\_length\_c 20.0

\_cell\_angle\_alpha 90.0

\_cell\_angle\_beta 90.0

\_cell\_angle\_gamma 90.0

\_symmetry\_space\_group\_name\_H-M 'P 1'

\_symmetry\_Int\_Tables\_number 1

\_symmetry\_cell\_setting triclinic

loop

\_atom\_site\_label

\_atom\_site\_type\_symbol

\_atom\_site\_fract\_x

|     |   | _atom_site_fract_y |                    | _atom_site_fract_z |     | _atom_site_occupancy |  |
|-----|---|--------------------|--------------------|--------------------|-----|----------------------|--|
| H1  | H | 0.0671547600000000 | 0.8925569400000000 | 0.9362384300000000 | 1.0 |                      |  |
| H2  | H | 0.9508880200000000 | 0.0636734800000000 | 0.0505050900000000 | 1.0 |                      |  |
| H3  | H | 0.2093765400000000 | 0.1022654500000000 | 0.0313945800000000 | 1.0 |                      |  |
| H4  | H | 0.3255975000000000 | 0.9311542700000000 | 0.9171097400000000 | 1.0 |                      |  |
| H5  | H | 0.5667428000000000 | 0.8924368400000000 | 0.9366762400000000 | 1.0 |                      |  |
| H6  | H | 0.4515036200000000 | 0.0640541900000000 | 0.0504462800000000 | 1.0 |                      |  |
| H7  | H | 0.7097875300000000 | 0.1023661200000000 | 0.0309277600000000 | 1.0 |                      |  |
| H8  | H | 0.8250899100000000 | 0.9307612400000000 | 0.9171527000000000 | 1.0 |                      |  |
| H9  | H | 0.0336005400000000 | 0.9078396500000000 | 0.0797186200000000 | 1.0 |                      |  |
| H10 | H | 0.5333065600000000 | 0.9083946700000000 | 0.0801339300000000 | 1.0 |                      |  |
| H11 | H | 0.2915668800000000 | 0.8864465900000000 | 0.0700546100000000 | 1.0 |                      |  |
| H12 | H | 0.7914933500000000 | 0.8864779700000000 | 0.0702230300000000 | 1.0 |                      |  |
| H13 | H | 0.2428366600000000 | 0.0870038000000000 | 0.8879502900000000 | 1.0 |                      |  |
| H14 | H | 0.7432753700000000 | 0.0864327200000000 | 0.8874530700000000 | 1.0 |                      |  |
| H15 | H | 0.9850134400000000 | 0.1083669300000000 | 0.8975726500000000 | 1.0 |                      |  |
| H16 | H | 0.4850594100000000 | 0.1083232800000000 | 0.8973616500000000 | 1.0 |                      |  |
| C17 | C | 0.0757121300000000 | 0.0533165200000000 | 0.9601407600000000 | 1.0 |                      |  |
| C18 | C | 0.9536493300000000 | 0.0373283400000000 | 0.0024738800000000 | 1.0 |                      |  |
| C19 | C | 0.9529392500000000 | 0.9582461300000000 | 0.0054623300000000 | 1.0 |                      |  |
| C20 | C | 0.0753986000000000 | 0.9399281100000000 | 0.9637348000000000 | 1.0 |                      |  |
| C21 | C | 0.2011499200000000 | 0.0548867300000000 | 0.0039049300000000 | 1.0 |                      |  |
| C22 | C | 0.3235874700000000 | 0.0365778300000000 | 0.9621570200000000 | 1.0 |                      |  |
| C23 | C | 0.3228772300000000 | 0.9574922900000000 | 0.9651460300000000 | 1.0 |                      |  |
| C24 | C | 0.2008421100000000 | 0.9414936200000000 | 0.0075002400000000 | 1.0 |                      |  |
| C25 | C | 0.5757750700000000 | 0.0532895000000000 | 0.9599448000000000 | 1.0 |                      |  |
| C26 | C | 0.4537863100000000 | 0.0375720300000000 | 0.0024808600000000 | 1.0 |                      |  |
| C27 | C | 0.4528993500000000 | 0.9585004600000000 | 0.0056332600000000 | 1.0 |                      |  |
| C28 | C | 0.5752430200000000 | 0.9399175900000000 | 0.9639643300000000 | 1.0 |                      |  |
| C29 | C | 0.7013078000000000 | 0.0548903500000000 | 0.0036278500000000 | 1.0 |                      |  |
| C30 | C | 0.8236546000000000 | 0.0363198900000000 | 0.9619592100000000 | 1.0 |                      |  |
| C31 | C | 0.8227737000000000 | 0.9572468500000000 | 0.9651151100000000 | 1.0 |                      |  |
| C32 | C | 0.7007854600000000 | 0.9415121800000000 | 0.0076415700000000 | 1.0 |                      |  |
| O33 | O | 0.0725401600000000 | 0.1096515800000000 | 0.9193819800000000 | 1.0 |                      |  |
| O34 | O | 0.9458548900000000 | 0.9244134900000000 | 0.0677763300000000 | 1.0 |                      |  |
| O35 | O | 0.3306021300000000 | 0.0704173900000000 | 0.8998492300000000 | 1.0 |                      |  |
| O36 | O | 0.2040318300000000 | 0.8851598100000000 | 0.0482570900000000 | 1.0 |                      |  |
| O37 | O | 0.0857043200000000 | 0.9938287500000000 | 0.9169282500000000 | 1.0 |                      |  |
| O38 | O | 0.1908596300000000 | 0.0009885100000000 | 0.0507121900000000 | 1.0 |                      |  |
| O39 | O | 0.5727759800000000 | 0.1094615400000000 | 0.9189731800000000 | 1.0 |                      |  |
| O40 | O | 0.4455676100000000 | 0.9248610600000000 | 0.0680458200000000 | 1.0 |                      |  |
| O41 | O | 0.8310090500000000 | 0.0699642600000000 | 0.8995502200000000 | 1.0 |                      |  |
| O42 | O | 0.7037939400000000 | 0.8853265500000000 | 0.0485933400000000 | 1.0 |                      |  |
| O43 | O | 0.5855277300000000 | 0.9936316800000000 | 0.9169415000000000 | 1.0 |                      |  |
| O44 | O | 0.6910507100000000 | 0.0011724200000000 | 0.0506480500000000 | 1.0 |                      |  |

##### cif ends

furan\_OH\_24\_anti\_dir    Energy: -280.65652343

##### cif starts

data\_furan\_OH\_24\_anti\_dir

\_publ\_section\_comment

;  
Andrew Reynoso, Bohan Xu, and Vincent H. Crespi  
;

\_cell\_length\_a 9.3646826716  
\_cell\_length\_b 20.0  
\_cell\_length\_c 20.0  
\_cell\_angle\_alpha 90.0  
\_cell\_angle\_beta 90.0  
\_cell\_angle\_gamma 90.0

\_symmetry\_space\_group\_name\_H-M 'P 1'  
\_symmetry\_Int\_Tables\_number 1  
\_symmetry\_cell\_setting triclinic

loop\_  
\_atom\_site\_label  
\_atom\_site\_type\_symbol  
\_atom\_site\_fract\_x  
\_atom\_site\_fract\_y  
\_atom\_site\_fract\_z  
\_atom\_site\_occupancy

|     |   |                    |                    |                    |     |
|-----|---|--------------------|--------------------|--------------------|-----|
| H1  | H | 0.0006881200000000 | 0.0512614800000000 | 0.0682805100000000 | 1.0 |
| H2  | H | 0.0199402500000000 | 0.8846231400000000 | 0.9408501400000000 | 1.0 |
| H3  | H | 0.0696015600000000 | 0.1151764700000000 | 0.8967595500000000 | 1.0 |
| H4  | H | 0.0883020800000000 | 0.9464556000000000 | 0.0998118000000000 | 1.0 |
| H5  | H | 0.2507129300000000 | 0.0493939600000000 | 0.9196734600000000 | 1.0 |
| H6  | H | 0.2699484900000000 | 0.8860071000000000 | 0.0512517200000000 | 1.0 |
| H7  | H | 0.3195273900000000 | 0.1175690500000000 | 0.0895752100000000 | 1.0 |
| H8  | H | 0.3383190300000000 | 0.9438293500000000 | 0.8907819000000000 | 1.0 |
| H9  | H | 0.5007089800000000 | 0.0512482100000000 | 0.0682839400000000 | 1.0 |
| H10 | H | 0.5199522000000000 | 0.8846172000000000 | 0.9408473700000000 | 1.0 |
| H11 | H | 0.5695398200000000 | 0.1151755500000000 | 0.8967588200000000 | 1.0 |
| H12 | H | 0.5883002700000000 | 0.9464511700000000 | 0.0998169800000000 | 1.0 |
| H13 | H | 0.7506816500000000 | 0.0493930000000000 | 0.9196545900000000 | 1.0 |
| H14 | H | 0.7699374600000000 | 0.8860231500000000 | 0.0512565700000000 | 1.0 |
| H15 | H | 0.8195491200000000 | 0.1176117300000000 | 0.0895205400000000 | 1.0 |
| H16 | H | 0.8383247500000000 | 0.9438306600000000 | 0.8907792100000000 | 1.0 |
| C17 | C | 0.0362358600000000 | 0.0436959800000000 | 0.9600138100000000 | 1.0 |
| C18 | C | 0.9503868300000000 | 0.0289745700000000 | 0.0239635700000000 | 1.0 |
| C19 | C | 0.9536455300000000 | 0.9504320000000000 | 0.0265449400000000 | 1.0 |
| C20 | C | 0.0406038900000000 | 0.9337941200000000 | 0.9627886800000000 | 1.0 |
| C21 | C | 0.2862317800000000 | 0.0445487800000000 | 0.0280932800000000 | 1.0 |
| C22 | C | 0.2003948600000000 | 0.0282230500000000 | 0.9645290100000000 | 1.0 |
| C23 | C | 0.2036551200000000 | 0.9496353900000000 | 0.9639227600000000 | 1.0 |
| C24 | C | 0.2906034400000000 | 0.9346099700000000 | 0.0280787500000000 | 1.0 |
| C25 | C | 0.5362202100000000 | 0.0436903800000000 | 0.9600142300000000 | 1.0 |
| C26 | C | 0.4503918100000000 | 0.0289635400000000 | 0.0239700700000000 | 1.0 |
| C27 | C | 0.4536529200000000 | 0.9504216400000000 | 0.0265457800000000 | 1.0 |
| C28 | C | 0.5406067900000000 | 0.9337889200000000 | 0.9627868200000000 | 1.0 |
| C29 | C | 0.7862276400000000 | 0.0445614000000000 | 0.0280757500000000 | 1.0 |
| C30 | C | 0.7003840500000000 | 0.0282245200000000 | 0.9645167400000000 | 1.0 |
| C31 | C | 0.7036544900000000 | 0.9496378000000000 | 0.9639180400000000 | 1.0 |
| C32 | C | 0.7905978100000000 | 0.9346224500000000 | 0.0280774300000000 | 1.0 |
| O33 | O | 0.9942757300000000 | 0.9862240000000000 | 0.9171659100000000 | 1.0 |

|     |   |                    |                    |                    |     |
|-----|---|--------------------|--------------------|--------------------|-----|
| O34 | O | 0.9988893300000000 | 0.1038149700000000 | 0.9306784900000000 | 1.0 |
| O35 | O | 0.0037166000000000 | 0.9207166700000000 | 0.0862956100000000 | 1.0 |
| O36 | O | 0.2442772600000000 | 0.9881739500000000 | 0.0723706200000000 | 1.0 |
| O37 | O | 0.2488819100000000 | 0.1053894200000000 | 0.0559094900000000 | 1.0 |
| O38 | O | 0.2537461000000000 | 0.9184244400000000 | 0.9049347000000000 | 1.0 |
| O39 | O | 0.4942600100000000 | 0.9862177500000000 | 0.9171671100000000 | 1.0 |
| O40 | O | 0.4988478500000000 | 0.1038087000000000 | 0.9306844800000000 | 1.0 |
| O41 | O | 0.5037318400000000 | 0.9207040900000000 | 0.0862945500000000 | 1.0 |
| O42 | O | 0.7442665600000000 | 0.9881927600000000 | 0.0723613000000000 | 1.0 |
| O43 | O | 0.7488780700000000 | 0.1054107100000000 | 0.0558749800000000 | 1.0 |
| O44 | O | 0.7537556700000000 | 0.9184241200000000 | 0.9049329600000000 | 1.0 |

##### cif ends

furan\_OH\_24\_anti\_dir\_forbid Energy: -280.15632795

##### cif starts

data\_furan\_OH\_24\_anti\_dir\_forbid

\_publ\_section\_comment

;  
Andrew Reynoso, Bohan Xu, and Vincent H. Crespi  
;

\_cell\_length\_a 10.2017024367

\_cell\_length\_b 20.0

\_cell\_length\_c 20.0

\_cell\_angle\_alpha 90.0

\_cell\_angle\_beta 90.0

\_cell\_angle\_gamma 90.0

\_symmetry\_space\_group\_name\_H-M 'P 1'

\_symmetry\_Int\_Tables\_number 1

\_symmetry\_cell\_setting triclinic

loop\_

\_atom\_site\_label

\_atom\_site\_type\_symbol

\_atom\_site\_fract\_x

\_atom\_site\_fract\_y

\_atom\_site\_fract\_z

\_atom\_site\_occupancy

|     |   |                    |                    |                    |     |
|-----|---|--------------------|--------------------|--------------------|-----|
| H1  | H | 0.9984403600000000 | 0.0585023300000000 | 0.0664062200000000 | 1.0 |
| H2  | H | 0.1232398700000000 | 0.8999206500000000 | 0.9381807900000000 | 1.0 |
| H3  | H | 0.1893705700000000 | 0.1332437300000000 | 0.9261983800000000 | 1.0 |
| H4  | H | 0.0728198100000000 | 0.9379260400000000 | 0.1033700200000000 | 1.0 |
| H5  | H | 0.3761871100000000 | 0.0637309200000000 | 0.9300657600000000 | 1.0 |
| H6  | H | 0.2604937400000000 | 0.8945066400000000 | 0.0450299900000000 | 1.0 |
| H7  | H | 0.3373020400000000 | 0.1126068200000000 | 0.0850200000000000 | 1.0 |
| H8  | H | 0.4477598900000000 | 0.9446303400000000 | 0.8885391600000000 | 1.0 |
| H9  | H | 0.5084397700000000 | 0.0638209900000000 | 0.0664026500000000 | 1.0 |
| H10 | H | 0.6175553200000000 | 0.8949206600000000 | 0.9489649300000000 | 1.0 |
| H11 | H | 0.6878650500000000 | 0.1301937600000000 | 0.9212144800000000 | 1.0 |
| H12 | H | 0.5649620800000000 | 0.9418347100000000 | 0.1093990400000000 | 1.0 |
| H13 | H | 0.8814884100000000 | 0.0577453300000000 | 0.9246571100000000 | 1.0 |
| H14 | H | 0.7619336600000000 | 0.8984823200000000 | 0.0530370500000000 | 1.0 |



|     |   |                    |                    |                    |     |
|-----|---|--------------------|--------------------|--------------------|-----|
| H15 | H | 0.8465462000000000 | 0.1209173700000000 | 0.0695039300000000 | 1.0 |
| H16 | H | 0.9060216600000000 | 0.8780950900000000 | 0.9213960700000000 | 1.0 |
| C17 | C | 0.1243734500000000 | 0.0569680400000000 | 0.9765607900000000 | 1.0 |
| C18 | C | 0.0027577700000000 | 0.0362569600000000 | 0.0162588000000000 | 1.0 |
| C19 | C | 0.0066717100000000 | 0.9576193800000000 | 0.0150879900000000 | 1.0 |
| C20 | C | 0.1296414700000000 | 0.9436816000000000 | 0.9710825200000000 | 1.0 |
| C21 | C | 0.2513354300000000 | 0.0550278500000000 | 0.0208812800000000 | 1.0 |
| C22 | C | 0.3739445600000000 | 0.0383780700000000 | 0.9786809100000000 | 1.0 |
| C23 | C | 0.3756115700000000 | 0.9595072300000000 | 0.9768560400000000 | 1.0 |
| C24 | C | 0.2519674900000000 | 0.9411284300000000 | 0.0165289000000000 | 1.0 |
| C25 | C | 0.6234328900000000 | 0.0552517300000000 | 0.9736534900000000 | 1.0 |
| C26 | C | 0.5046345000000000 | 0.0385118900000000 | 0.0177123900000000 | 1.0 |
| C27 | C | 0.5055356200000000 | 0.9597046000000000 | 0.0193511200000000 | 1.0 |
| C28 | C | 0.6275942900000000 | 0.9415061400000000 | 0.9773998700000000 | 1.0 |
| C29 | C | 0.7532078700000000 | 0.0560936100000000 | 0.0156345900000000 | 1.0 |
| C30 | C | 0.8745232000000000 | 0.0352873600000000 | 0.9744934000000000 | 1.0 |
| C31 | C | 0.8733794800000000 | 0.9569062100000000 | 0.9765253000000000 | 1.0 |
| C32 | C | 0.7521076900000000 | 0.9426553100000000 | 0.0209072900000000 | 1.0 |
| O33 | O | 0.1387130200000000 | 0.0022447800000000 | 0.9292855300000000 | 1.0 |
| O34 | O | 0.1053135200000000 | 0.1165269200000000 | 0.9422191000000000 | 1.0 |
| O35 | O | 0.0024334800000000 | 0.9206157600000000 | 0.0750834200000000 | 1.0 |
| O36 | O | 0.2395889200000000 | 0.9958449800000000 | 0.0637982800000000 | 1.0 |
| O37 | O | 0.2546185200000000 | 0.1119504300000000 | 0.0604823000000000 | 1.0 |
| O38 | O | 0.3789256000000000 | 0.9245159600000000 | 0.9159085500000000 | 1.0 |
| O39 | O | 0.6335981100000000 | 0.9965042400000000 | 0.9301931200000000 | 1.0 |
| O40 | O | 0.6035588000000000 | 0.1117361000000000 | 0.9347499300000000 | 1.0 |
| O41 | O | 0.4954739500000000 | 0.9249178200000000 | 0.0804016500000000 | 1.0 |
| O42 | O | 0.7430094100000000 | 0.0010054900000000 | 0.0637298000000000 | 1.0 |
| O43 | O | 0.7596844500000000 | 0.1165248300000000 | 0.0495203600000000 | 1.0 |
| O44 | O | 0.8705014700000000 | 0.9227723700000000 | 0.9146111900000000 | 1.0 |

##### cif ends

furan\_OH\_24\_syn\_alt    Energy: -280.15150099

##### cif starts

data\_furan\_OH\_24\_syn\_alt

\_publ\_section\_comment

;  
Andrew Reynoso, Bohan Xu, and Vincent H. Crespi  
;

\_cell\_length\_a    10.3303278758

\_cell\_length\_b    20.0

\_cell\_length\_c    20.0

\_cell\_angle\_alpha    90.0

\_cell\_angle\_beta    90.0

\_cell\_angle\_gamma    90.0

\_symmetry\_space\_group\_name\_H-M    'P 1'

\_symmetry\_Int\_Tables\_number    1

\_symmetry\_cell\_setting    triclinic

loop\_

\_atom\_site\_label

|     | _atom_site_type_symbol | _atom_site_fract_x | _atom_site_fract_y | _atom_site_fract_z | _atom_site_occupancy |
|-----|------------------------|--------------------|--------------------|--------------------|----------------------|
| H1  | H                      | 0.1173934300000000 | 0.9343000800000000 | 0.9145131800000000 | 1.0                  |
| H2  | H                      | 0.9947463400000000 | 0.0955796000000000 | 0.0339343200000000 | 1.0                  |
| H3  | H                      | 0.0573636800000000 | 0.8718864500000000 | 0.0659103400000000 | 1.0                  |
| H4  | H                      | 0.1258253800000000 | 0.1108042000000000 | 0.9053820100000000 | 1.0                  |
| H5  | H                      | 0.3674187200000000 | 0.0558967900000000 | 0.9155403000000000 | 1.0                  |
| H6  | H                      | 0.2447499700000000 | 0.8926063600000000 | 0.0322034200000000 | 1.0                  |
| H7  | H                      | 0.3074302600000000 | 0.1157976500000000 | 0.0679036900000000 | 1.0                  |
| H8  | H                      | 0.3753916400000000 | 0.8795715100000000 | 0.9033764800000000 | 1.0                  |
| H9  | H                      | 0.6173971500000000 | 0.9343100400000000 | 0.9145077500000000 | 1.0                  |
| H10 | H                      | 0.4947285700000000 | 0.0955861800000000 | 0.0339202000000000 | 1.0                  |
| H11 | H                      | 0.5573842100000000 | 0.8719008500000000 | 0.0659025100000000 | 1.0                  |
| H12 | H                      | 0.6257842100000000 | 0.1108200400000000 | 0.9054051000000000 | 1.0                  |
| H13 | H                      | 0.8673962700000000 | 0.0559049500000000 | 0.9155640000000000 | 1.0                  |
| H14 | H                      | 0.7447461900000000 | 0.8925860900000000 | 0.0321849800000000 | 1.0                  |
| H15 | H                      | 0.8074621400000000 | 0.1157735000000000 | 0.0679307500000000 | 1.0                  |
| H16 | H                      | 0.8754277000000000 | 0.8795785000000000 | 0.9033812500000000 | 1.0                  |
| C17 | C                      | 0.9921432700000000 | 0.9401469500000000 | 0.0059959400000000 | 1.0                  |
| C18 | C                      | 0.1174991100000000 | 0.9556990000000000 | 0.9648864400000000 | 1.0                  |
| C19 | C                      | 0.1165798200000000 | 0.0337121900000000 | 0.9651484500000000 | 1.0                  |
| C20 | C                      | 0.9911555700000000 | 0.0476470500000000 | 0.0072193500000000 | 1.0                  |
| C21 | C                      | 0.2421500000000000 | 0.0484857600000000 | 0.0069160700000000 | 1.0                  |
| C22 | C                      | 0.3675104700000000 | 0.0336327500000000 | 0.9655398300000000 | 1.0                  |
| C23 | C                      | 0.3665710200000000 | 0.9556288100000000 | 0.9644778800000000 | 1.0                  |
| C24 | C                      | 0.2411488700000000 | 0.9409800900000000 | 0.0063060300000000 | 1.0                  |
| C25 | C                      | 0.4921436500000000 | 0.9401510000000000 | 0.0059895800000000 | 1.0                  |
| C26 | C                      | 0.6175028800000000 | 0.9557035200000000 | 0.9648832300000000 | 1.0                  |
| C27 | C                      | 0.6165892900000000 | 0.0337163700000000 | 0.9651572500000000 | 1.0                  |
| C28 | C                      | 0.4911513900000000 | 0.0476515500000000 | 0.0072094100000000 | 1.0                  |
| C29 | C                      | 0.7421466900000000 | 0.0484747400000000 | 0.0069420600000000 | 1.0                  |
| C30 | C                      | 0.8675040800000000 | 0.0336315700000000 | 0.9655591700000000 | 1.0                  |
| C31 | C                      | 0.8665699200000000 | 0.9556285200000000 | 0.9644855900000000 | 1.0                  |
| C32 | C                      | 0.7411449900000000 | 0.9409694100000000 | 0.0063040700000000 | 1.0                  |
| O33 | O                      | 0.9915574100000000 | 0.9935230600000000 | 0.0545146200000000 | 1.0                  |
| O34 | O                      | 0.9837062000000000 | 0.8774771400000000 | 0.0359495400000000 | 1.0                  |
| O35 | O                      | 0.1164356300000000 | 0.0625730400000000 | 0.9003402100000000 | 1.0                  |
| O36 | O                      | 0.2415576300000000 | 0.9942896000000000 | 0.0545202400000000 | 1.0                  |
| O37 | O                      | 0.2336807200000000 | 0.1106471000000000 | 0.0379220900000000 | 1.0                  |
| O38 | O                      | 0.3664133300000000 | 0.9279020500000000 | 0.8991763900000000 | 1.0                  |
| O39 | O                      | 0.4915467800000000 | 0.9935304300000000 | 0.0545074800000000 | 1.0                  |
| O40 | O                      | 0.4837145600000000 | 0.8774825900000000 | 0.0359472400000000 | 1.0                  |
| O41 | O                      | 0.6164835600000000 | 0.0625857300000000 | 0.9003529100000000 | 1.0                  |
| O42 | O                      | 0.7415455700000000 | 0.9942648800000000 | 0.0545323000000000 | 1.0                  |
| O43 | O                      | 0.7336815800000000 | 0.1106243500000000 | 0.0379683600000000 | 1.0                  |
| O44 | O                      | 0.8664161100000000 | 0.9279078200000000 | 0.8991827100000000 | 1.0                  |

##### cif ends

furand\_OH\_24\_syn\_alt\_forbid Energy: -277.63410235

##### cif starts

data\_furand\_OH\_24\_syn\_alt\_forbid

\_publ\_section\_comment  
;  
Andrew Reynoso, Bohan Xu, and Vincent H. Crespi  
;

\_cell\_length\_a 9.5554150447  
\_cell\_length\_b 20.0  
\_cell\_length\_c 20.0  
\_cell\_angle\_alpha 90.0  
\_cell\_angle\_beta 90.0  
\_cell\_angle\_gamma 90.0

\_symmetry\_space\_group\_name\_H-M 'P 1'  
\_symmetry\_Int\_Tables\_number 1  
\_symmetry\_cell\_setting triclinic

loop\_

\_atom\_site\_label  
\_atom\_site\_type\_symbol  
\_atom\_site\_fract\_x  
\_atom\_site\_fract\_y  
\_atom\_site\_fract\_z  
\_atom\_site\_occupancy

|     |   |                    |                    |                    |     |
|-----|---|--------------------|--------------------|--------------------|-----|
| H1  | H | 0.9008867300000000 | 0.0590195500000000 | 0.9171785000000000 | 1.0 |
| H2  | H | 0.8985670000000000 | 0.8992524200000000 | 0.0559938400000000 | 1.0 |
| H3  | H | 0.1555625100000000 | 0.1004485800000000 | 0.0502193800000000 | 1.0 |
| H4  | H | 0.1533046100000000 | 0.9329709000000000 | 0.9208057400000000 | 1.0 |
| H5  | H | 0.4009919700000000 | 0.0589936700000000 | 0.9171039500000000 | 1.0 |
| H6  | H | 0.3985910700000000 | 0.8993904000000000 | 0.0561144300000000 | 1.0 |
| H7  | H | 0.6555486500000000 | 0.1003199800000000 | 0.0503334000000000 | 1.0 |
| H8  | H | 0.6531766100000000 | 0.9329847800000000 | 0.9207218600000000 | 1.0 |
| H9  | H | 0.9617890000000000 | 0.9114690600000000 | 0.8792500700000000 | 1.0 |
| H10 | H | 0.8566662500000000 | 0.1254945000000000 | 0.0933797900000000 | 1.0 |
| H11 | H | 0.4616198500000000 | 0.9113797000000000 | 0.8793256900000000 | 1.0 |
| H12 | H | 0.3565863000000000 | 0.1257438800000000 | 0.0931554200000000 | 1.0 |
| H13 | H | 0.1975636800000000 | 0.8766979700000000 | 0.1005043300000000 | 1.0 |
| H14 | H | 0.6975944400000000 | 0.8764760900000000 | 0.1003164600000000 | 1.0 |
| H15 | H | 0.0927832400000000 | 0.0775195300000000 | 0.8741705500000000 | 1.0 |
| H16 | H | 0.5928903500000000 | 0.0776476300000000 | 0.8742529900000000 | 1.0 |
| C17 | C | 0.8625318600000000 | 0.0556934600000000 | 0.0263266700000000 | 1.0 |
| C18 | C | 0.9445195300000000 | 0.0367438500000000 | 0.9627571500000000 | 1.0 |
| C19 | C | 0.9438328500000000 | 0.9580535400000000 | 0.9649253400000000 | 1.0 |
| C20 | C | 0.8616242200000000 | 0.9443195000000000 | 0.0302404700000000 | 1.0 |
| C21 | C | 0.1925160500000000 | 0.0539794700000000 | 0.0270963900000000 | 1.0 |
| C22 | C | 0.1103402100000000 | 0.0365246300000000 | 0.9626712800000000 | 1.0 |
| C23 | C | 0.1096563200000000 | 0.9578310100000000 | 0.9650262100000000 | 1.0 |
| C24 | C | 0.1916226700000000 | 0.9425620800000000 | 0.0295807000000000 | 1.0 |
| C25 | C | 0.3625346100000000 | 0.0557952900000000 | 0.0262549600000000 | 1.0 |
| C26 | C | 0.4445405400000000 | 0.0367565200000000 | 0.9627215900000000 | 1.0 |
| C27 | C | 0.4438020600000000 | 0.9580711500000000 | 0.9649463100000000 | 1.0 |
| C28 | C | 0.3616443200000000 | 0.9444251900000000 | 0.0303054500000000 | 1.0 |
| C29 | C | 0.6925036400000000 | 0.0538799400000000 | 0.0271536600000000 | 1.0 |
| C30 | C | 0.6103631900000000 | 0.0365117800000000 | 0.9626867600000000 | 1.0 |
| C31 | C | 0.6096240000000000 | 0.9578163700000000 | 0.9649811900000000 | 1.0 |

|     |   |                    |                    |                    |     |
|-----|---|--------------------|--------------------|--------------------|-----|
| C32 | C | 0.6916153200000000 | 0.9424616300000000 | 0.0295021000000000 | 1.0 |
| O33 | O | 0.8967558600000000 | 0.0007513200000000 | 0.0702458200000000 | 1.0 |
| O34 | O | 0.9109706500000000 | 0.1159602600000000 | 0.0532064200000000 | 1.0 |
| O35 | O | 0.8864963700000000 | 0.9214894800000000 | 0.9103499000000000 | 1.0 |
| O36 | O | 0.1573630600000000 | 0.9999343700000000 | 0.0702689700000000 | 1.0 |
| O37 | O | 0.1677339300000000 | 0.0699530200000000 | 0.9061472600000000 | 1.0 |
| O38 | O | 0.1432153100000000 | 0.8839284500000000 | 0.0598671700000000 | 1.0 |
| O39 | O | 0.3967759700000000 | 0.0009096800000000 | 0.0702398300000000 | 1.0 |
| O40 | O | 0.4109912800000000 | 0.1160984100000000 | 0.0530410000000000 | 1.0 |
| O41 | O | 0.3863576000000000 | 0.9214662400000000 | 0.9104228700000000 | 1.0 |
| O42 | O | 0.6573489100000000 | 0.9997796800000000 | 0.0702585500000000 | 1.0 |
| O43 | O | 0.6678352300000000 | 0.0699861400000000 | 0.9062072000000000 | 1.0 |
| O44 | O | 0.6431769500000000 | 0.8837922400000000 | 0.0597128900000000 | 1.0 |

##### cif ends

furan\_OH\_24\_syn\_dir Energy: -281.52113358

##### cif starts

data\_furan\_OH\_24\_syn\_dir

\_publ\_section\_comment

;  
Andrew Reynoso, Bohan Xu, and Vincent H. Crespi  
;

\_cell\_length\_a 10.358880939

\_cell\_length\_b 20.0

\_cell\_length\_c 20.0

\_cell\_angle\_alpha 90.0

\_cell\_angle\_beta 90.0

\_cell\_angle\_gamma 90.0

\_symmetry\_space\_group\_name\_H-M 'P 1'

\_symmetry\_Int\_Tables\_number 1

\_symmetry\_cell\_setting triclinic

loop\_

\_atom\_site\_label

\_atom\_site\_type\_symbol

\_atom\_site\_fract\_x

\_atom\_site\_fract\_y

\_atom\_site\_fract\_z

\_atom\_site\_occupancy

|     |   |                    |                    |                    |     |
|-----|---|--------------------|--------------------|--------------------|-----|
| H1  | H | 0.0584406900000000 | 0.0419315600000000 | 0.9323993200000000 | 1.0 |
| H2  | H | 0.9329695600000000 | 0.8939210600000000 | 0.0691720000000000 | 1.0 |
| H3  | H | 0.8500166900000000 | 0.1247142600000000 | 0.0605388400000000 | 1.0 |
| H4  | H | 0.9745966600000000 | 0.8997144400000000 | 0.9206189500000000 | 1.0 |
| H5  | H | 0.3084881400000000 | 0.0419261000000000 | 0.9323900200000000 | 1.0 |
| H6  | H | 0.1829862700000000 | 0.8939427900000000 | 0.0691862800000000 | 1.0 |
| H7  | H | 0.1000034000000000 | 0.1247413600000000 | 0.0604633400000000 | 1.0 |
| H8  | H | 0.2245901700000000 | 0.8997065000000000 | 0.9206306100000000 | 1.0 |
| H9  | H | 0.5585332300000000 | 0.0419517800000000 | 0.9324222600000000 | 1.0 |
| H10 | H | 0.4329813600000000 | 0.8939467300000000 | 0.0691928600000000 | 1.0 |
| H11 | H | 0.3499751400000000 | 0.1247451000000000 | 0.0604582700000000 | 1.0 |
| H12 | H | 0.4745725000000000 | 0.8997298900000000 | 0.9206248900000000 | 1.0 |

|     |   |                    |                    |                    |     |
|-----|---|--------------------|--------------------|--------------------|-----|
| H13 | H | 0.8084356200000000 | 0.0419567700000000 | 0.9324320100000000 | 1.0 |
| H14 | H | 0.6829742300000000 | 0.8939089700000000 | 0.0691636800000000 | 1.0 |
| H15 | H | 0.5999947500000000 | 0.1247165100000000 | 0.0605459500000000 | 1.0 |
| H16 | H | 0.7245755900000000 | 0.8997408200000000 | 0.9206142400000000 | 1.0 |
| C17 | C | 0.9337175200000000 | 0.0462029100000000 | 0.0236155500000000 | 1.0 |
| C18 | C | 0.0583630400000000 | 0.0261271700000000 | 0.9849155300000000 | 1.0 |
| C19 | C | 0.0583742800000000 | 0.9479890100000000 | 0.9945532800000000 | 1.0 |
| C20 | C | 0.9331712900000000 | 0.9389438200000000 | 0.0377880100000000 | 1.0 |
| C21 | C | 0.1837162500000000 | 0.0462118900000000 | 0.0235854600000000 | 1.0 |
| C22 | C | 0.3083785100000000 | 0.0261287800000000 | 0.9849081000000000 | 1.0 |
| C23 | C | 0.3083788600000000 | 0.9479929700000000 | 0.9945555000000000 | 1.0 |
| C24 | C | 0.1831752700000000 | 0.9389577700000000 | 0.0377912100000000 | 1.0 |
| C25 | C | 0.4337137800000000 | 0.0462169000000000 | 0.0235973400000000 | 1.0 |
| C26 | C | 0.5583876300000000 | 0.0261373000000000 | 0.9849349700000000 | 1.0 |
| C27 | C | 0.5583757300000000 | 0.9479980200000000 | 0.9945576600000000 | 1.0 |
| C28 | C | 0.4331729700000000 | 0.9389603500000000 | 0.0377958700000000 | 1.0 |
| C29 | C | 0.6837154800000000 | 0.0462018100000000 | 0.0236404400000000 | 1.0 |
| C30 | C | 0.8083635800000000 | 0.0261353100000000 | 0.9849427300000000 | 1.0 |
| C31 | C | 0.8083705300000000 | 0.9479949900000000 | 0.9945550900000000 | 1.0 |
| C32 | C | 0.6831701200000000 | 0.9389391800000000 | 0.0377898100000000 | 1.0 |
| O33 | O | 0.9336104500000000 | 0.9976465600000000 | 0.0780009200000000 | 1.0 |
| O34 | O | 0.9389569800000000 | 0.1112983800000000 | 0.0477315100000000 | 1.0 |
| O35 | O | 0.0643021400000000 | 0.9072935900000000 | 0.9363011700000000 | 1.0 |
| O36 | O | 0.1836044100000000 | 0.9976737700000000 | 0.0779859700000000 | 1.0 |
| O37 | O | 0.1889492500000000 | 0.1113175500000000 | 0.0476738800000000 | 1.0 |
| O38 | O | 0.3142985700000000 | 0.9072910000000000 | 0.9363082500000000 | 1.0 |
| O39 | O | 0.4335933900000000 | 0.9976741900000000 | 0.0779938700000000 | 1.0 |
| O40 | O | 0.4389346200000000 | 0.1113204800000000 | 0.0476925100000000 | 1.0 |
| O41 | O | 0.5642849600000000 | 0.9073195500000000 | 0.9362941900000000 | 1.0 |
| O42 | O | 0.6835980900000000 | 0.9976334800000000 | 0.0780146500000000 | 1.0 |
| O43 | O | 0.6889485500000000 | 0.1112907500000000 | 0.0477751900000000 | 1.0 |
| O44 | O | 0.8142878700000000 | 0.9073247400000000 | 0.9362857800000000 | 1.0 |

##### cif ends

uran\_OH\_24\_syn\_dir\_forbid Energy: -278.78883921

##### cif starts

data\_uran\_OH\_24\_syn\_dir\_forbid

\_publ\_section\_comment

;

Andrew Reynoso, Bohan Xu, and Vincent H. Crespi

;

\_cell\_length\_a 9.6892293946

\_cell\_length\_b 20.0

\_cell\_length\_c 20.0

\_cell\_angle\_alpha 90.0

\_cell\_angle\_beta 90.0

\_cell\_angle\_gamma 90.0

\_symmetry\_space\_group\_name\_H-M 'P 1'

\_symmetry\_Int\_Tables\_number 1

\_symmetry\_cell\_setting triclinic

| loop_                  |   |                    |                    |                    |     |
|------------------------|---|--------------------|--------------------|--------------------|-----|
| _atom_site_label       |   |                    |                    |                    |     |
| _atom_site_type_symbol |   |                    |                    |                    |     |
| _atom_site_fract_x     |   |                    |                    |                    |     |
| _atom_site_fract_y     |   |                    |                    |                    |     |
| _atom_site_fract_z     |   |                    |                    |                    |     |
| _atom_site_occupancy   |   |                    |                    |                    |     |
| H1                     | H | 0.9006443500000000 | 0.0445231200000000 | 0.9116163200000000 | 1.0 |
| H2                     | H | 0.9036117200000000 | 0.9001691300000000 | 0.0678988700000000 | 1.0 |
| H3                     | H | 0.1479639400000000 | 0.0555537800000000 | 0.9194196100000000 | 1.0 |
| H4                     | H | 0.1654723100000000 | 0.8910428300000000 | 0.0537649100000000 | 1.0 |
| H5                     | H | 0.4001824300000000 | 0.0446450000000000 | 0.9118411600000000 | 1.0 |
| H6                     | H | 0.4036706200000000 | 0.8998607700000000 | 0.0676946400000000 | 1.0 |
| H7                     | H | 0.6475229000000000 | 0.0555880400000000 | 0.9192347800000000 | 1.0 |
| H8                     | H | 0.6654172100000000 | 0.8913571600000000 | 0.0539412600000000 | 1.0 |
| H9                     | H | 0.9862750000000000 | 0.8942628600000000 | 0.8939453900000000 | 1.0 |
| H10                    | H | 0.2495470400000000 | 0.9102843200000000 | 0.9043013200000000 | 1.0 |
| H11                    | H | 0.4864230800000000 | 0.8944222600000000 | 0.8938219600000000 | 1.0 |
| H12                    | H | 0.7496410800000000 | 0.9102521300000000 | 0.9044264600000000 | 1.0 |
| H13                    | H | 0.8134841700000000 | 0.1350175000000000 | 0.0633660500000000 | 1.0 |
| H14                    | H | 0.0508128900000000 | 0.1161314300000000 | 0.0603533900000000 | 1.0 |
| H15                    | H | 0.3132381700000000 | 0.1347074900000000 | 0.0638396100000000 | 1.0 |
| H16                    | H | 0.5509032600000000 | 0.1162626000000000 | 0.0603344900000000 | 1.0 |
| C17                    | C | 0.8555716400000000 | 0.0514198400000000 | 0.0216106400000000 | 1.0 |
| C18                    | C | 0.9393297100000000 | 0.0273187700000000 | 0.9601581800000000 | 1.0 |
| C19                    | C | 0.9490224600000000 | 0.9495334200000000 | 0.9702418000000000 | 1.0 |
| C20                    | C | 0.8688881000000000 | 0.9415117500000000 | 0.0360217500000000 | 1.0 |
| C21                    | C | 0.1841500700000000 | 0.0492837300000000 | 0.0283287200000000 | 1.0 |
| C22                    | C | 0.1041293300000000 | 0.0317839600000000 | 0.9640007500000000 | 1.0 |
| C23                    | C | 0.1150690100000000 | 0.9536840600000000 | 0.9654888500000000 | 1.0 |
| C24                    | C | 0.2000079500000000 | 0.9377540600000000 | 0.0302612000000000 | 1.0 |
| C25                    | C | 0.3555161800000000 | 0.0512418900000000 | 0.0218729000000000 | 1.0 |
| C26                    | C | 0.4391680800000000 | 0.0273523900000000 | 0.9602956200000000 | 1.0 |
| C27                    | C | 0.4489835000000000 | 0.9495538100000000 | 0.9702026800000000 | 1.0 |
| C28                    | C | 0.3688736400000000 | 0.9412978000000000 | 0.0359561800000000 | 1.0 |
| C29                    | C | 0.6842344900000000 | 0.0495228600000000 | 0.0281180700000000 | 1.0 |
| C30                    | C | 0.6039825600000000 | 0.0318750200000000 | 0.9639162100000000 | 1.0 |
| C31                    | C | 0.6150486100000000 | 0.9537810400000000 | 0.9654840000000000 | 1.0 |
| C32                    | C | 0.6999931500000000 | 0.9379980900000000 | 0.0303153800000000 | 1.0 |
| O33                    | O | 0.8953976900000000 | 0.0024830300000000 | 0.0706114500000000 | 1.0 |
| O34                    | O | 0.8961199700000000 | 0.1155600300000000 | 0.0408005300000000 | 1.0 |
| O35                    | O | 0.9027394200000000 | 0.9030680400000000 | 0.9217506300000000 | 1.0 |
| O36                    | O | 0.1584338900000000 | 0.9921318200000000 | 0.0710779000000000 | 1.0 |
| O37                    | O | 0.1529293500000000 | 0.1070661000000000 | 0.0627525200000000 | 1.0 |
| O38                    | O | 0.1482656800000000 | 0.9215637200000000 | 0.9050054600000000 | 1.0 |
| O39                    | O | 0.3953446200000000 | 0.0021622900000000 | 0.0707281800000000 | 1.0 |
| O40                    | O | 0.3959461500000000 | 0.1153252000000000 | 0.0412681900000000 | 1.0 |
| O41                    | O | 0.4027944600000000 | 0.9032228700000000 | 0.9215618800000000 | 1.0 |
| O42                    | O | 0.6585067400000000 | 0.9924868500000000 | 0.0710069500000000 | 1.0 |
| O43                    | O | 0.6531291600000000 | 0.1074089200000000 | 0.0623980700000000 | 1.0 |
| O44                    | O | 0.6483930600000000 | 0.9216219800000000 | 0.9050456300000000 | 1.0 |

##### cif ends

furan\_OH\_25\_anti\_dir    Energy: -281.84147509

##### cif starts

data\_furan\_OH\_25\_anti\_dir

\_publ\_section\_comment

;

Andrew Reynoso, Bohan Xu, and Vincent H. Crespi

;

\_cell\_length\_a 9.1865881381

\_cell\_length\_b 20.0

\_cell\_length\_c 20.0

\_cell\_angle\_alpha 90.0

\_cell\_angle\_beta 90.0

\_cell\_angle\_gamma 90.0

\_symmetry\_space\_group\_name\_H-M 'P 1'

\_symmetry\_Int\_Tables\_number 1

\_symmetry\_cell\_setting triclinic

loop\_

\_atom\_site\_label

\_atom\_site\_type\_symbol

\_atom\_site\_fract\_x

\_atom\_site\_fract\_y

\_atom\_site\_fract\_z

\_atom\_site\_occupancy

|     |   |                    |                    |                    |     |
|-----|---|--------------------|--------------------|--------------------|-----|
| H1  | H | 0.9473973900000000 | 0.0601359500000000 | 0.0679507400000000 | 1.0 |
| H2  | H | 0.9474077700000000 | 0.9402472300000000 | 0.0689172200000000 | 1.0 |
| H3  | H | 0.0179354200000000 | 0.1287360200000000 | 0.9008079800000000 | 1.0 |
| H4  | H | 0.0178714800000000 | 0.8689942200000000 | 0.9028425400000000 | 1.0 |
| H5  | H | 0.1974102900000000 | 0.0589207000000000 | 0.9207057700000000 | 1.0 |
| H6  | H | 0.1974113900000000 | 0.9390176600000000 | 0.9217247200000000 | 1.0 |
| H7  | H | 0.2680263400000000 | 0.1303332300000000 | 0.0866019500000000 | 1.0 |
| H8  | H | 0.2681393700000000 | 0.8704148100000000 | 0.0887696300000000 | 1.0 |
| H9  | H | 0.4474010800000000 | 0.0601309300000000 | 0.0679519200000000 | 1.0 |
| H10 | H | 0.4474038300000000 | 0.9402420500000000 | 0.0689185200000000 | 1.0 |
| H11 | H | 0.5178871700000000 | 0.1287165100000000 | 0.9007829200000000 | 1.0 |
| H12 | H | 0.5178990100000000 | 0.8689883900000000 | 0.9028522900000000 | 1.0 |
| H13 | H | 0.6974014400000000 | 0.0589189100000000 | 0.9207013900000000 | 1.0 |
| H14 | H | 0.6974156400000000 | 0.9390154900000000 | 0.9217280600000000 | 1.0 |
| H15 | H | 0.7680330900000000 | 0.1303456100000000 | 0.0865866900000000 | 1.0 |
| H16 | H | 0.7681534900000000 | 0.8704141400000000 | 0.0887652100000000 | 1.0 |
| C17 | C | 0.9775814700000000 | 0.0540797000000000 | 0.9593379100000000 | 1.0 |
| C18 | C | 0.8931726400000000 | 0.0385153900000000 | 0.0240930700000000 | 1.0 |
| C19 | C | 0.8931404000000000 | 0.9611527500000000 | 0.0247246100000000 | 1.0 |
| C20 | C | 0.9775273100000000 | 0.9445447600000000 | 0.9602124900000000 | 1.0 |
| C21 | C | 0.2275718000000000 | 0.0546574000000000 | 0.0294008700000000 | 1.0 |
| C22 | C | 0.1431777300000000 | 0.0380222800000000 | 0.9649097900000000 | 1.0 |
| C23 | C | 0.1431459500000000 | 0.9606627400000000 | 0.9655595300000000 | 1.0 |
| C24 | C | 0.2275238800000000 | 0.9451193200000000 | 0.0303356900000000 | 1.0 |
| C25 | C | 0.4775748600000000 | 0.0540759400000000 | 0.9593373900000000 | 1.0 |
| C26 | C | 0.3931722700000000 | 0.0385117500000000 | 0.0240945800000000 | 1.0 |
| C27 | C | 0.3931400100000000 | 0.9611487000000000 | 0.0247251100000000 | 1.0 |
| C28 | C | 0.4775305500000000 | 0.9445414600000000 | 0.9602139300000000 | 1.0 |
| C29 | C | 0.7275716100000000 | 0.0546616800000000 | 0.0293965300000000 | 1.0 |

|     |   |                    |                    |                    |     |
|-----|---|--------------------|--------------------|--------------------|-----|
| C30 | C | 0.6431744300000000 | 0.0380220400000000 | 0.9649074700000000 | 1.0 |
| C31 | C | 0.6431475000000000 | 0.9606628000000000 | 0.9655611400000000 | 1.0 |
| C32 | C | 0.7275246900000000 | 0.9451238700000000 | 0.0303381000000000 | 1.0 |
| O33 | O | 0.9323799500000000 | 0.9989573900000000 | 0.9152757400000000 | 1.0 |
| O34 | O | 0.9422631600000000 | 0.1159280600000000 | 0.9324549800000000 | 1.0 |
| O35 | O | 0.9421890400000000 | 0.8822929500000000 | 0.9342807600000000 | 1.0 |
| O36 | O | 0.1823816100000000 | 0.0002728600000000 | 0.0743707900000000 | 1.0 |
| O37 | O | 0.1922319600000000 | 0.1169396800000000 | 0.0552619700000000 | 1.0 |
| O38 | O | 0.1921933900000000 | 0.8832991600000000 | 0.0572942800000000 | 1.0 |
| O39 | O | 0.4323770500000000 | 0.9989522600000000 | 0.9152768400000000 | 1.0 |
| O40 | O | 0.4422480900000000 | 0.1159223000000000 | 0.9324518800000000 | 1.0 |
| O41 | O | 0.4422020700000000 | 0.8822886600000000 | 0.9342825000000000 | 1.0 |
| O42 | O | 0.6823839600000000 | 0.0002788300000000 | 0.0743693900000000 | 1.0 |
| O43 | O | 0.6922304900000000 | 0.1169452900000000 | 0.0552537500000000 | 1.0 |
| O44 | O | 0.6921930600000000 | 0.8833050800000000 | 0.0573000700000000 | 1.0 |

##### cif ends

furand\_OH\_25\_anti\_dir\_forbid Energy: -281.09276497

##### cif starts

data\_furand\_OH\_25\_anti\_dir\_forbid

\_publ\_section\_comment

;  
Andrew Reynoso, Bohan Xu, and Vincent H. Crespi  
;

\_cell\_length\_a 10.2149576753

\_cell\_length\_b 20.0

\_cell\_length\_c 20.0

\_cell\_angle\_alpha 90.0

\_cell\_angle\_beta 90.0

\_cell\_angle\_gamma 90.0

\_symmetry\_space\_group\_name\_H-M 'P 1'

\_symmetry\_Int\_Tables\_number 1

\_symmetry\_cell\_setting triclinic

loop\_

\_atom\_site\_label

\_atom\_site\_type\_symbol

\_atom\_site\_fract\_x

\_atom\_site\_fract\_y

\_atom\_site\_fract\_z

\_atom\_site\_occupancy

|     |   |                    |                    |                    |     |
|-----|---|--------------------|--------------------|--------------------|-----|
| H1  | H | 0.9682865700000000 | 0.0636691500000000 | 0.0603777600000000 | 1.0 |
| H2  | H | 0.9703815000000000 | 0.9356235000000000 | 0.0612421100000000 | 1.0 |
| H3  | H | 0.1537002600000000 | 0.1334568200000000 | 0.9203671200000000 | 1.0 |
| H4  | H | 0.0078604700000000 | 0.8834234600000000 | 0.9063777400000000 | 1.0 |
| H5  | H | 0.3417513700000000 | 0.0627392700000000 | 0.9238622700000000 | 1.0 |
| H6  | H | 0.3352043300000000 | 0.9340219600000000 | 0.9251998200000000 | 1.0 |
| H7  | H | 0.3023808300000000 | 0.1178258500000000 | 0.0745114200000000 | 1.0 |
| H8  | H | 0.3008434300000000 | 0.8825769000000000 | 0.0777020300000000 | 1.0 |
| H9  | H | 0.4701285900000000 | 0.0636029400000000 | 0.0608865800000000 | 1.0 |
| H10 | H | 0.4699148600000000 | 0.9350094000000000 | 0.0617144500000000 | 1.0 |



|     |   |                    |                    |                    |     |
|-----|---|--------------------|--------------------|--------------------|-----|
| H11 | H | 0.6276324100000000 | 0.1480790700000000 | 0.9503540600000000 | 1.0 |
| H12 | H | 0.5069440700000000 | 0.8819789300000000 | 0.9084683000000000 | 1.0 |
| H13 | H | 0.8402973900000000 | 0.0624576700000000 | 0.9225706200000000 | 1.0 |
| H14 | H | 0.8342562100000000 | 0.9333871000000000 | 0.9252796600000000 | 1.0 |
| H15 | H | 0.8077895800000000 | 0.1247453700000000 | 0.0643356300000000 | 1.0 |
| H16 | H | 0.8019813000000000 | 0.8836706300000000 | 0.0780688000000000 | 1.0 |
| C17 | C | 0.0886224500000000 | 0.0566336200000000 | 0.9698026100000000 | 1.0 |
| C18 | C | 0.9674423000000000 | 0.0383552600000000 | 0.0116288400000000 | 1.0 |
| C19 | C | 0.9679133300000000 | 0.9604664700000000 | 0.0122802500000000 | 1.0 |
| C20 | C | 0.0900400400000000 | 0.9421767300000000 | 0.9704905900000000 | 1.0 |
| C21 | C | 0.2153775900000000 | 0.0566979600000000 | 0.0140943600000000 | 1.0 |
| C22 | C | 0.3376414200000000 | 0.0378597900000000 | 0.9726948600000000 | 1.0 |
| C23 | C | 0.3371900000000000 | 0.9598935100000000 | 0.9736088500000000 | 1.0 |
| C24 | C | 0.2152296600000000 | 0.9423419400000000 | 0.0156246900000000 | 1.0 |
| C25 | C | 0.5886863200000000 | 0.0559395900000000 | 0.9691874000000000 | 1.0 |
| C26 | C | 0.4678615900000000 | 0.0379801700000000 | 0.0123092900000000 | 1.0 |
| C27 | C | 0.4677914100000000 | 0.9601392400000000 | 0.0128958300000000 | 1.0 |
| C28 | C | 0.5897377400000000 | 0.9421114800000000 | 0.9710634900000000 | 1.0 |
| C29 | C | 0.7158537800000000 | 0.0568764000000000 | 0.0127456900000000 | 1.0 |
| C30 | C | 0.8374673300000000 | 0.0378457800000000 | 0.9714456400000000 | 1.0 |
| C31 | C | 0.8370264300000000 | 0.9599214800000000 | 0.9733084200000000 | 1.0 |
| C32 | C | 0.7155252300000000 | 0.9430264200000000 | 0.0159507200000000 | 1.0 |
| O33 | O | 0.1036075300000000 | 0.9991713600000000 | 0.9256641900000000 | 1.0 |
| O34 | O | 0.0693174100000000 | 0.1143600600000000 | 0.9326768800000000 | 1.0 |
| O35 | O | 0.0869986700000000 | 0.8835316600000000 | 0.9336982900000000 | 1.0 |
| O36 | O | 0.2014264000000000 | 0.0003419000000000 | 0.0594897700000000 | 1.0 |
| O37 | O | 0.2199296400000000 | 0.1162231600000000 | 0.0499124100000000 | 1.0 |
| O38 | O | 0.2180183000000000 | 0.8844407000000000 | 0.0534805200000000 | 1.0 |
| O39 | O | 0.6019965500000000 | 0.9989071200000000 | 0.9255829200000000 | 1.0 |
| O40 | O | 0.5748943300000000 | 0.1129997200000000 | 0.9296317200000000 | 1.0 |
| O41 | O | 0.5875519300000000 | 0.8833184300000000 | 0.9346070300000000 | 1.0 |
| O42 | O | 0.7025956300000000 | 0.0016968800000000 | 0.0593336400000000 | 1.0 |
| O43 | O | 0.7198594500000000 | 0.1179376100000000 | 0.0465001400000000 | 1.0 |
| O44 | O | 0.7184329900000000 | 0.8856515200000000 | 0.0545124800000000 | 1.0 |

##### cif ends

uran\_OH\_25\_syn\_dir Energy: -282.58210605

##### cif starts

data\_uran\_OH\_25\_syn\_dir

\_publ\_section\_comment

;  
Andrew Reynoso, Bohan Xu, and Vincent H. Crespi  
;

\_cell\_length\_a 10.3785187722

\_cell\_length\_b 20.0

\_cell\_length\_c 20.0

\_cell\_angle\_alpha 90.0

\_cell\_angle\_beta 90.0

\_cell\_angle\_gamma 90.0

\_symmetry\_space\_group\_name\_H-M 'P 1'

\_symmetry\_Int\_Tables\_number 1

\_symmetry\_cell\_setting triclinic

loop\_

\_atom\_site\_label

\_atom\_site\_type\_symbol

\_atom\_site\_fract\_x

\_atom\_site\_fract\_y

\_atom\_site\_fract\_z

\_atom\_site\_occupancy

|     |   |                    |                    |                    |     |
|-----|---|--------------------|--------------------|--------------------|-----|
| H1  | H | 0.1149613600000000 | 0.0592742600000000 | 0.9161555200000000 | 1.0 |
| H2  | H | 0.1150068200000000 | 0.9329297200000000 | 0.9230151600000000 | 1.0 |
| H3  | H | 0.0731541400000000 | 0.1314775700000000 | 0.0477754400000000 | 1.0 |
| H4  | H | 0.9067214300000000 | 0.8753103100000000 | 0.0615480400000000 | 1.0 |
| H5  | H | 0.3650027600000000 | 0.0592713800000000 | 0.9161662500000000 | 1.0 |
| H6  | H | 0.3649063000000000 | 0.9329217900000000 | 0.9230228700000000 | 1.0 |
| H7  | H | 0.3231643900000000 | 0.1314771200000000 | 0.0477921000000000 | 1.0 |
| H8  | H | 0.1566918200000000 | 0.8753495300000000 | 0.0615885100000000 | 1.0 |
| H9  | H | 0.6149353100000000 | 0.0592567000000000 | 0.9161629400000000 | 1.0 |
| H10 | H | 0.6149461900000000 | 0.9329125900000000 | 0.9230079800000000 | 1.0 |
| H11 | H | 0.5731927600000000 | 0.1314457800000000 | 0.0477990000000000 | 1.0 |
| H12 | H | 0.4067075500000000 | 0.8753016200000000 | 0.0615596500000000 | 1.0 |
| H13 | H | 0.8649534500000000 | 0.0592641200000000 | 0.9161538700000000 | 1.0 |
| H14 | H | 0.8649783200000000 | 0.9329218600000000 | 0.9229985000000000 | 1.0 |
| H15 | H | 0.8231770600000000 | 0.1314610800000000 | 0.0477648400000000 | 1.0 |
| H16 | H | 0.6567310100000000 | 0.8752993900000000 | 0.0615550700000000 | 1.0 |
| C17 | C | 0.9896645000000000 | 0.0548212400000000 | 0.0070688900000000 | 1.0 |
| C18 | C | 0.1149394100000000 | 0.0375396700000000 | 0.9665420400000000 | 1.0 |
| C19 | C | 0.1149975100000000 | 0.9599956100000000 | 0.9707495300000000 | 1.0 |
| C20 | C | 0.9902604200000000 | 0.9471718800000000 | 0.0128917800000000 | 1.0 |
| C21 | C | 0.2396697100000000 | 0.0548359600000000 | 0.0070698300000000 | 1.0 |
| C22 | C | 0.3649459000000000 | 0.0375328000000000 | 0.9665512700000000 | 1.0 |
| C23 | C | 0.3649760200000000 | 0.9599884400000000 | 0.9707567700000000 | 1.0 |
| C24 | C | 0.2402533100000000 | 0.9471891500000000 | 0.0129173500000000 | 1.0 |
| C25 | C | 0.4896730700000000 | 0.0548093200000000 | 0.0070853800000000 | 1.0 |
| C26 | C | 0.6149322100000000 | 0.0375184000000000 | 0.9665477800000000 | 1.0 |
| C27 | C | 0.6149800500000000 | 0.9599742500000000 | 0.9707446100000000 | 1.0 |
| C28 | C | 0.4902527800000000 | 0.9471580500000000 | 0.0129012900000000 | 1.0 |
| C29 | C | 0.7396688000000000 | 0.0548073000000000 | 0.0070699200000000 | 1.0 |
| C30 | C | 0.8649352900000000 | 0.0375257100000000 | 0.9665387300000000 | 1.0 |
| C31 | C | 0.8649920500000000 | 0.9599815800000000 | 0.9707367200000000 | 1.0 |
| C32 | C | 0.7402600400000000 | 0.9471566600000000 | 0.0128897400000000 | 1.0 |
| O33 | O | 0.9899653800000000 | 0.0035799500000000 | 0.0577343000000000 | 1.0 |
| O34 | O | 0.9844465900000000 | 0.1187952100000000 | 0.0341685000000000 | 1.0 |
| O35 | O | 0.9954551400000000 | 0.8864802200000000 | 0.0467126300000000 | 1.0 |
| O36 | O | 0.2399620800000000 | 0.0036075900000000 | 0.0577450600000000 | 1.0 |
| O37 | O | 0.2344626400000000 | 0.1188166600000000 | 0.0341567800000000 | 1.0 |
| O38 | O | 0.2454333300000000 | 0.8865108100000000 | 0.0467576600000000 | 1.0 |
| O39 | O | 0.4899758200000000 | 0.0035632800000000 | 0.0577468200000000 | 1.0 |
| O40 | O | 0.4844783100000000 | 0.1187816900000000 | 0.0341878900000000 | 1.0 |
| O41 | O | 0.4954393600000000 | 0.8864633300000000 | 0.0467162100000000 | 1.0 |
| O42 | O | 0.7399775700000000 | 0.0035628300000000 | 0.0577347100000000 | 1.0 |
| O43 | O | 0.7344614600000000 | 0.1187809700000000 | 0.0341682800000000 | 1.0 |
| O44 | O | 0.7454573400000000 | 0.8864620300000000 | 0.0467047000000000 | 1.0 |

##### cif ends

furandiol\_25\_syn\_dir\_forbid Energy: -279.57929323

##### cif starts

data\_furandiol\_25\_syn\_dir\_forbid

\_publ\_section\_comment

;  
Andrew Reynoso, Bohan Xu, and Vincent H. Crespi  
;

\_cell\_length\_a 9.693403391

\_cell\_length\_b 20.0

\_cell\_length\_c 20.0

\_cell\_angle\_alpha 90.0

\_cell\_angle\_beta 90.0

\_cell\_angle\_gamma 90.0

\_symmetry\_space\_group\_name\_H-M 'P 1'

\_symmetry\_Int\_Tables\_number 1

\_symmetry\_cell\_setting triclinic

loop\_

\_atom\_site\_label

\_atom\_site\_type\_symbol

\_atom\_site\_fract\_x

\_atom\_site\_fract\_y

\_atom\_site\_fract\_z

\_atom\_site\_occupancy

|     |   |                    |                    |                    |     |
|-----|---|--------------------|--------------------|--------------------|-----|
| H1  | H | 0.9004706600000000 | 0.0548179000000000 | 0.9123270100000000 | 1.0 |
| H2  | H | 0.9047944700000000 | 0.9265388300000000 | 0.9217802700000000 | 1.0 |
| H3  | H | 0.1483470100000000 | 0.0644586600000000 | 0.9197834900000000 | 1.0 |
| H4  | H | 0.1526661400000000 | 0.9359682500000000 | 0.9140527900000000 | 1.0 |
| H5  | H | 0.3999633500000000 | 0.0548690900000000 | 0.9126090000000000 | 1.0 |
| H6  | H | 0.4052939000000000 | 0.9265880400000000 | 0.9215335900000000 | 1.0 |
| H7  | H | 0.6478415100000000 | 0.0644226400000000 | 0.9195561500000000 | 1.0 |
| H8  | H | 0.6531651100000000 | 0.9359487900000000 | 0.9143150300000000 | 1.0 |
| H9  | H | 0.8135876100000000 | 0.1353892400000000 | 0.0672810800000000 | 1.0 |
| H10 | H | 0.0505956100000000 | 0.1166505400000000 | 0.0627810800000000 | 1.0 |
| H11 | H | 0.3132812200000000 | 0.1348464000000000 | 0.0678500800000000 | 1.0 |
| H12 | H | 0.5506344300000000 | 0.1168338700000000 | 0.0627589100000000 | 1.0 |
| H13 | H | 0.0025590900000000 | 0.8785411800000000 | 0.0662428200000000 | 1.0 |
| H14 | H | 0.2394806200000000 | 0.8599238700000000 | 0.0713057400000000 | 1.0 |
| H15 | H | 0.5025192300000000 | 0.8783131100000000 | 0.0661657100000000 | 1.0 |
| H16 | H | 0.7398410400000000 | 0.8604870300000000 | 0.0718363300000000 | 1.0 |
| C17 | C | 0.8565715200000000 | 0.0536439800000000 | 0.0219893200000000 | 1.0 |
| C18 | C | 0.9398700900000000 | 0.0331612900000000 | 0.9589549500000000 | 1.0 |
| C19 | C | 0.9483652900000000 | 0.9555097300000000 | 0.9632879500000000 | 1.0 |
| C20 | C | 0.8687963200000000 | 0.9429474600000000 | 0.0294112000000000 | 1.0 |
| C21 | C | 0.1843501300000000 | 0.0511814000000000 | 0.0278569100000000 | 1.0 |
| C22 | C | 0.1047720300000000 | 0.0367115800000000 | 0.9621174500000000 | 1.0 |
| C23 | C | 0.1132559900000000 | 0.9589678000000000 | 0.9600316900000000 | 1.0 |
| C24 | C | 0.1965575500000000 | 0.9403124400000000 | 0.0236308300000000 | 1.0 |
| C25 | C | 0.3565220600000000 | 0.0532729800000000 | 0.0222943300000000 | 1.0 |
| C26 | C | 0.4397332800000000 | 0.0331019300000000 | 0.9591127400000000 | 1.0 |
| C27 | C | 0.4484809600000000 | 0.9554422400000000 | 0.9632180000000000 | 1.0 |

|     |   |                    |                    |                    |     |
|-----|---|--------------------|--------------------|--------------------|-----|
| C28 | C | 0.3686700000000000 | 0.9425388200000000 | 0.0291910300000000 | 1.0 |
| C29 | C | 0.6844637000000000 | 0.0515687500000000 | 0.0276293500000000 | 1.0 |
| C30 | C | 0.6046448000000000 | 0.0367806500000000 | 0.9620519000000000 | 1.0 |
| C31 | C | 0.6133933300000000 | 0.9590385400000000 | 0.9601758200000000 | 1.0 |
| C32 | C | 0.6966299600000000 | 0.9406881300000000 | 0.0239057800000000 | 1.0 |
| O33 | O | 0.8949038200000000 | 0.0025249300000000 | 0.0678528400000000 | 1.0 |
| O34 | O | 0.8965760500000000 | 0.1169803200000000 | 0.0442081400000000 | 1.0 |
| O35 | O | 0.9000734000000000 | 0.8871174000000000 | 0.0668482500000000 | 1.0 |
| O36 | O | 0.1582412000000000 | 0.9927374700000000 | 0.0679989300000000 | 1.0 |
| O37 | O | 0.1530641400000000 | 0.1080684300000000 | 0.0636767900000000 | 1.0 |
| O38 | O | 0.1565236200000000 | 0.8776475800000000 | 0.0476782300000000 | 1.0 |
| O39 | O | 0.3947617200000000 | 0.0019211300000000 | 0.0679257100000000 | 1.0 |
| O40 | O | 0.3963995000000000 | 0.1165047600000000 | 0.0448240500000000 | 1.0 |
| O41 | O | 0.3998911800000000 | 0.8865084600000000 | 0.0663477500000000 | 1.0 |
| O42 | O | 0.6583824700000000 | 0.9933209800000000 | 0.0680486300000000 | 1.0 |
| O43 | O | 0.6532537800000000 | 0.1086352300000000 | 0.0631830300000000 | 1.0 |
| O44 | O | 0.6567648200000000 | 0.8781255400000000 | 0.0482333300000000 | 1.0 |

##### cif ends

furan\_OH\_34\_anti\_dir Energy: -279.26594176

##### cif starts

data\_furan\_OH\_34\_anti\_dir

\_publ\_section\_comment

;  
Andrew Reynoso, Bohan Xu, and Vincent H. Crespi  
;

\_cell\_length\_a 9.5112955639

\_cell\_length\_b 20.0

\_cell\_length\_c 20.0

\_cell\_angle\_alpha 90.0

\_cell\_angle\_beta 90.0

\_cell\_angle\_gamma 90.0

\_symmetry\_space\_group\_name\_H-M 'P 1'

\_symmetry\_Int\_Tables\_number 1

\_symmetry\_cell\_setting triclinic

loop\_

\_atom\_site\_label

\_atom\_site\_type\_symbol

\_atom\_site\_fract\_x

\_atom\_site\_fract\_y

\_atom\_site\_fract\_z

\_atom\_site\_occupancy

|    |   |                    |                    |                    |     |
|----|---|--------------------|--------------------|--------------------|-----|
| H1 | H | 0.0319623900000000 | 0.0430859800000000 | 0.0843862100000000 | 1.0 |
|----|---|--------------------|--------------------|--------------------|-----|

|    |   |                    |                    |                    |     |
|----|---|--------------------|--------------------|--------------------|-----|
| H2 | H | 0.9582861800000000 | 0.1036938800000000 | 0.9245379000000000 | 1.0 |
|----|---|--------------------|--------------------|--------------------|-----|

|    |   |                    |                    |                    |     |
|----|---|--------------------|--------------------|--------------------|-----|
| H3 | H | 0.9657952800000000 | 0.8984313400000000 | 0.9255531300000000 | 1.0 |
|----|---|--------------------|--------------------|--------------------|-----|

|    |   |                    |                    |                    |     |
|----|---|--------------------|--------------------|--------------------|-----|
| H4 | H | 0.9021385500000000 | 0.9499004100000000 | 0.1090457100000000 | 1.0 |
|----|---|--------------------|--------------------|--------------------|-----|

|    |   |                    |                    |                    |     |
|----|---|--------------------|--------------------|--------------------|-----|
| H5 | H | 0.1521152400000000 | 0.0543913200000000 | 0.8550904600000000 | 1.0 |
|----|---|--------------------|--------------------|--------------------|-----|

|    |   |                    |                    |                    |     |
|----|---|--------------------|--------------------|--------------------|-----|
| H6 | H | 0.2157824500000000 | 0.1057171500000000 | 0.0385830000000000 | 1.0 |
|----|---|--------------------|--------------------|--------------------|-----|

|    |   |                    |                    |                    |     |
|----|---|--------------------|--------------------|--------------------|-----|
| H7 | H | 0.2082988500000000 | 0.9004462300000000 | 0.0395502500000000 | 1.0 |
|----|---|--------------------|--------------------|--------------------|-----|

|    |   |                    |                    |                    |     |
|----|---|--------------------|--------------------|--------------------|-----|
| H8 | H | 0.2819760800000000 | 0.9610990400000000 | 0.8797174000000000 | 1.0 |
|----|---|--------------------|--------------------|--------------------|-----|

|     |   |                    |                    |                    |     |
|-----|---|--------------------|--------------------|--------------------|-----|
| H9  | H | 0.5319936800000000 | 0.0430794900000000 | 0.0843714200000000 | 1.0 |
| H10 | H | 0.4582918000000000 | 0.1036709400000000 | 0.9245166100000000 | 1.0 |
| H11 | H | 0.4657895100000000 | 0.8984086400000000 | 0.9255695800000000 | 1.0 |
| H12 | H | 0.4021174900000000 | 0.9499215800000000 | 0.1090480800000000 | 1.0 |
| H13 | H | 0.6521399900000000 | 0.0543015000000000 | 0.8550725000000000 | 1.0 |
| H14 | H | 0.7157525700000000 | 0.1057181900000000 | 0.0385584900000000 | 1.0 |
| H15 | H | 0.7083223900000000 | 0.9004477600000000 | 0.0395693400000000 | 1.0 |
| H16 | H | 0.7819782200000000 | 0.9610639500000000 | 0.8797220000000000 | 1.0 |
| C17 | C | 0.9857433100000000 | 0.9464973100000000 | 0.9500046800000000 | 1.0 |
| C18 | C | 0.8954989600000000 | 0.9613492000000000 | 0.0127772100000000 | 1.0 |
| C19 | C | 0.8965956400000000 | 0.0416058500000000 | 0.0127193800000000 | 1.0 |
| C20 | C | 0.9826346700000000 | 0.0564110600000000 | 0.9494854100000000 | 1.0 |
| C21 | C | 0.2326429900000000 | 0.9477367700000000 | 0.0146170100000000 | 1.0 |
| C22 | C | 0.1466111900000000 | 0.9625559200000000 | 0.9513840000000000 | 1.0 |
| C23 | C | 0.1454936100000000 | 0.0428121100000000 | 0.9513501400000000 | 1.0 |
| C24 | C | 0.2357234400000000 | 0.0576547300000000 | 0.0141235400000000 | 1.0 |
| C25 | C | 0.4857398700000000 | 0.9464796300000000 | 0.9500117200000000 | 1.0 |
| C26 | C | 0.3954924900000000 | 0.9613450500000000 | 0.0127789700000000 | 1.0 |
| C27 | C | 0.3966013700000000 | 0.0416012800000000 | 0.0127153700000000 | 1.0 |
| C28 | C | 0.4826363300000000 | 0.0563944700000000 | 0.9494748600000000 | 1.0 |
| C29 | C | 0.7326492200000000 | 0.9477341100000000 | 0.0146238300000000 | 1.0 |
| C30 | C | 0.6466104400000000 | 0.9625365300000000 | 0.9513901600000000 | 1.0 |
| C31 | C | 0.6454930400000000 | 0.0427919800000000 | 0.9513377500000000 | 1.0 |
| C32 | C | 0.7357167400000000 | 0.0576520400000000 | 0.0141108200000000 | 1.0 |
| O33 | O | 0.9414372600000000 | 0.0006468700000000 | 0.9060479200000000 | 1.0 |
| O34 | O | 0.9528207400000000 | 0.9312923300000000 | 0.0708265300000000 | 1.0 |
| O35 | O | 0.9482804400000000 | 0.0697947800000000 | 0.0726526300000000 | 1.0 |
| O36 | O | 0.1914283100000000 | 0.0034923100000000 | 0.0580691400000000 | 1.0 |
| O37 | O | 0.1982776200000000 | 0.9343923300000000 | 0.8914339700000000 | 1.0 |
| O38 | O | 0.2028833500000000 | 0.0729020200000000 | 0.8933349000000000 | 1.0 |
| O39 | O | 0.4414390300000000 | 0.0006240600000000 | 0.9060458700000000 | 1.0 |
| O40 | O | 0.4527957000000000 | 0.9312947900000000 | 0.0708359200000000 | 1.0 |
| O41 | O | 0.4483104300000000 | 0.0697906700000000 | 0.0726431700000000 | 1.0 |
| O42 | O | 0.6914253300000000 | 0.0034952000000000 | 0.0580653000000000 | 1.0 |
| O43 | O | 0.6982843100000000 | 0.9343585600000000 | 0.8914470000000000 | 1.0 |
| O44 | O | 0.7028621300000000 | 0.0728603600000000 | 0.8933073600000000 | 1.0 |

##### cif ends

furand\_OH\_34\_anti\_dir\_forbid Energy: -279.60859765

##### cif starts

data\_furand\_OH\_34\_anti\_dir\_forbid

\_publ\_section\_comment

;  
Andrew Reynoso, Bohan Xu, and Vincent H. Crespi  
;

\_cell\_length\_a 10.1825661719

\_cell\_length\_b 20.0

\_cell\_length\_c 20.0

\_cell\_angle\_alpha 90.0

\_cell\_angle\_beta 90.0

\_cell\_angle\_gamma 90.0

\_symmetry\_space\_group\_name\_H-M 'P 1'  
\_symmetry\_Int\_Tables\_number 1  
\_symmetry\_cell\_setting triclinic

loop\_

\_atom\_site\_label  
\_atom\_site\_type\_symbol  
\_atom\_site\_fract\_x  
\_atom\_site\_fract\_y  
\_atom\_site\_fract\_z  
\_atom\_site\_occupancy

|     |   |                    |                    |                    |     |
|-----|---|--------------------|--------------------|--------------------|-----|
| H1  | H | 0.0608154200000000 | 0.0538383600000000 | 0.1029947800000000 | 1.0 |
| H2  | H | 0.1111026500000000 | 0.1014479600000000 | 0.9404020500000000 | 1.0 |
| H3  | H | 0.1118755600000000 | 0.8970484900000000 | 0.9414408800000000 | 1.0 |
| H4  | H | 0.9298281400000000 | 0.9485112100000000 | 0.1029962500000000 | 1.0 |
| H5  | H | 0.3060554400000000 | 0.0533819700000000 | 0.8825486200000000 | 1.0 |
| H6  | H | 0.2558403500000000 | 0.1016350800000000 | 0.0449500600000000 | 1.0 |
| H7  | H | 0.2549020100000000 | 0.8972271000000000 | 0.0446784800000000 | 1.0 |
| H8  | H | 0.4371079900000000 | 0.9480356400000000 | 0.8829911100000000 | 1.0 |
| H9  | H | 0.5605253600000000 | 0.0536792400000000 | 0.1030675100000000 | 1.0 |
| H10 | H | 0.6110841900000000 | 0.1014210700000000 | 0.9404012700000000 | 1.0 |
| H11 | H | 0.6119423900000000 | 0.8970162400000000 | 0.9415204100000000 | 1.0 |
| H12 | H | 0.4293513700000000 | 0.9483585700000000 | 0.1028956600000000 | 1.0 |
| H13 | H | 0.8058945200000000 | 0.0534316400000000 | 0.8826018700000000 | 1.0 |
| H14 | H | 0.7557970300000000 | 0.1016598300000000 | 0.0449557300000000 | 1.0 |
| H15 | H | 0.7549387900000000 | 0.8972594900000000 | 0.0447773200000000 | 1.0 |
| H16 | H | 0.9367978100000000 | 0.9480943000000000 | 0.8829638100000000 | 1.0 |
| C17 | C | 0.1208792500000000 | 0.9425207200000000 | 0.9717166000000000 | 1.0 |
| C18 | C | 0.9987894200000000 | 0.9597032600000000 | 0.0138006400000000 | 1.0 |
| C19 | C | 0.9988136200000000 | 0.0398070300000000 | 0.0132004300000000 | 1.0 |
| C20 | C | 0.1206972100000000 | 0.0562583000000000 | 0.9710661000000000 | 1.0 |
| C21 | C | 0.2459628100000000 | 0.9425931100000000 | 0.0142370100000000 | 1.0 |
| C22 | C | 0.3681006800000000 | 0.9596045200000000 | 0.9721301400000000 | 1.0 |
| C23 | C | 0.3680770700000000 | 0.0397096600000000 | 0.9723909300000000 | 1.0 |
| C24 | C | 0.2461945900000000 | 0.0563336900000000 | 0.0144580900000000 | 1.0 |
| C25 | C | 0.6208996000000000 | 0.9425037000000000 | 0.9717765700000000 | 1.0 |
| C26 | C | 0.4987592200000000 | 0.9596957800000000 | 0.0138108100000000 | 1.0 |
| C27 | C | 0.4987956900000000 | 0.0398011800000000 | 0.0132079800000000 | 1.0 |
| C28 | C | 0.6206916200000000 | 0.0562446800000000 | 0.9710838000000000 | 1.0 |
| C29 | C | 0.7459696000000000 | 0.9426072700000000 | 0.0143119500000000 | 1.0 |
| C30 | C | 0.8680811600000000 | 0.9596039100000000 | 0.9721703400000000 | 1.0 |
| C31 | C | 0.8680602500000000 | 0.0397098700000000 | 0.9724125800000000 | 1.0 |
| C32 | C | 0.7461792800000000 | 0.0563447600000000 | 0.0144829400000000 | 1.0 |
| O33 | O | 0.1268938400000000 | 0.9991875100000000 | 0.9258790100000000 | 1.0 |
| O34 | O | 0.9978578400000000 | 0.9269262600000000 | 0.0759556600000000 | 1.0 |
| O35 | O | 0.9907840400000000 | 0.0727200000000000 | 0.0752880500000000 | 1.0 |
| O36 | O | 0.2399648400000000 | 0.9994346100000000 | 0.0598631500000000 | 1.0 |
| O37 | O | 0.3691055900000000 | 0.9265491700000000 | 0.9101242500000000 | 1.0 |
| O38 | O | 0.3761289800000000 | 0.0723629100000000 | 0.9101642000000000 | 1.0 |
| O39 | O | 0.6269158900000000 | 0.9991540900000000 | 0.9259151400000000 | 1.0 |
| O40 | O | 0.4977304300000000 | 0.9269213400000000 | 0.0759653200000000 | 1.0 |
| O41 | O | 0.4907478600000000 | 0.0727104100000000 | 0.0752946000000000 | 1.0 |
| O42 | O | 0.7399533000000000 | 0.9994661600000000 | 0.0599073600000000 | 1.0 |
| O43 | O | 0.8690079300000000 | 0.9265292400000000 | 0.9101753900000000 | 1.0 |
| O44 | O | 0.8760906900000000 | 0.0723493800000000 | 0.9101777900000000 | 1.0 |

##### cif ends

  furan\_OH\_34\_syn\_dir   Energy: -280.31145483

##### cif starts

data\_furan\_OH\_34\_syn\_dir

\_publ\_section\_comment

;  
Andrew Reynoso, Bohan Xu, and Vincent H. Crespi  
;

\_cell\_length\_a  10.3420435685

\_cell\_length\_b  20.0

\_cell\_length\_c  20.0

\_cell\_angle\_alpha  90.0

\_cell\_angle\_beta  90.0

\_cell\_angle\_gamma  90.0

\_symmetry\_space\_group\_name\_H-M  'P 1'

\_symmetry\_Int\_Tables\_number 1

\_symmetry\_cell\_setting triclinic

loop\_

\_atom\_site\_label

\_atom\_site\_type\_symbol

\_atom\_site\_fract\_x

\_atom\_site\_fract\_y

\_atom\_site\_fract\_z

\_atom\_site\_occupancy

|     |   |                    |                    |                    |     |
|-----|---|--------------------|--------------------|--------------------|-----|
| H1  | H | 0.8398414200000000 | 0.0771288100000000 | 0.9179796300000000 | 1.0 |
| H2  | H | 0.0474479100000000 | 0.1033274100000000 | 0.0683138800000000 | 1.0 |
| H3  | H | 0.0478409700000000 | 0.8991929400000000 | 0.0654706800000000 | 1.0 |
| H4  | H | 0.0054445000000000 | 0.9296536200000000 | 0.9158984000000000 | 1.0 |
| H5  | H | 0.0898278200000000 | 0.0771056200000000 | 0.9179730200000000 | 1.0 |
| H6  | H | 0.2974556500000000 | 0.1033318700000000 | 0.0682979300000000 | 1.0 |
| H7  | H | 0.2978329300000000 | 0.8991978200000000 | 0.0654821000000000 | 1.0 |
| H8  | H | 0.2554509600000000 | 0.9296277500000000 | 0.9159139900000000 | 1.0 |
| H9  | H | 0.3398319600000000 | 0.0771017700000000 | 0.9179637600000000 | 1.0 |
| H10 | H | 0.5474328200000000 | 0.1033334500000000 | 0.0682967600000000 | 1.0 |
| H11 | H | 0.5478448500000000 | 0.8991985600000000 | 0.0654804900000000 | 1.0 |
| H12 | H | 0.5054495700000000 | 0.9296358000000000 | 0.9159098900000000 | 1.0 |
| H13 | H | 0.5898423200000000 | 0.0771062800000000 | 0.9179673200000000 | 1.0 |
| H14 | H | 0.7974343200000000 | 0.1033278900000000 | 0.0683129100000000 | 1.0 |
| H15 | H | 0.7978334100000000 | 0.8991941900000000 | 0.0654693000000000 | 1.0 |
| H16 | H | 0.7554376000000000 | 0.9296464500000000 | 0.9159018900000000 | 1.0 |
| C17 | C | 0.0477756100000000 | 0.9473243600000000 | 0.0390657300000000 | 1.0 |
| C18 | C | 0.9224809300000000 | 0.9618482800000000 | 0.9979835900000000 | 1.0 |
| C19 | C | 0.9228054900000000 | 0.0425805400000000 | 0.9991104700000000 | 1.0 |
| C20 | C | 0.0475121200000000 | 0.0559486200000000 | 0.0405784300000000 | 1.0 |
| C21 | C | 0.2977753200000000 | 0.9473254600000000 | 0.0390703900000000 | 1.0 |
| C22 | C | 0.1724817200000000 | 0.9618433300000000 | 0.9979876200000000 | 1.0 |
| C23 | C | 0.1728052400000000 | 0.0425761800000000 | 0.9991056300000000 | 1.0 |
| C24 | C | 0.2975139100000000 | 0.0559497600000000 | 0.0405684800000000 | 1.0 |
| C25 | C | 0.5477773300000000 | 0.9473268000000000 | 0.0390695400000000 | 1.0 |

|     |   |                    |                    |                    |     |
|-----|---|--------------------|--------------------|--------------------|-----|
| C26 | C | 0.4224812200000000 | 0.9618392000000000 | 0.9979880900000000 | 1.0 |
| C27 | C | 0.4228048500000000 | 0.0425724600000000 | 0.9990987500000000 | 1.0 |
| C28 | C | 0.5475070700000000 | 0.0559507800000000 | 0.0405683400000000 | 1.0 |
| C29 | C | 0.7977742900000000 | 0.9473251700000000 | 0.0390635500000000 | 1.0 |
| C30 | C | 0.6724795600000000 | 0.9618463100000000 | 0.9979850000000000 | 1.0 |
| C31 | C | 0.6728051900000000 | 0.0425791200000000 | 0.9991054000000000 | 1.0 |
| C32 | C | 0.7975079300000000 | 0.0559496200000000 | 0.0405771900000000 | 1.0 |
| O33 | O | 0.0476426000000000 | 0.0009826600000000 | 0.0868248100000000 | 1.0 |
| O34 | O | 0.9162042100000000 | 0.9318563000000000 | 0.9339996100000000 | 1.0 |
| O35 | O | 0.9290889100000000 | 0.0743690200000000 | 0.9359941000000000 | 1.0 |
| O36 | O | 0.2976464500000000 | 0.0009901600000000 | 0.0868222500000000 | 1.0 |
| O37 | O | 0.1662075700000000 | 0.9318349700000000 | 0.9340115000000000 | 1.0 |
| O38 | O | 0.1790795000000000 | 0.0743539100000000 | 0.9359843100000000 | 1.0 |
| O39 | O | 0.5476404700000000 | 0.0009912200000000 | 0.0868218300000000 | 1.0 |
| O40 | O | 0.4162109500000000 | 0.9318236200000000 | 0.9340148100000000 | 1.0 |
| O41 | O | 0.4290811800000000 | 0.0743457600000000 | 0.9359753900000000 | 1.0 |
| O42 | O | 0.7976400900000000 | 0.0009832600000000 | 0.0868230300000000 | 1.0 |
| O43 | O | 0.6661999400000000 | 0.9318429900000000 | 0.9340062000000000 | 1.0 |
| O44 | O | 0.6790874800000000 | 0.0743637200000000 | 0.9359877400000000 | 1.0 |

##### cif ends

furand\_OH\_34\_syn\_dir\_forbid Energy: -277.75423627

##### cif starts

data\_furand\_OH\_34\_syn\_dir\_forbid

\_publ\_section\_comment

;  
Andrew Reynoso, Bohan Xu, and Vincent H. Crespi  
;

\_cell\_length\_a 9.6929142679

\_cell\_length\_b 20.0

\_cell\_length\_c 20.0

\_cell\_angle\_alpha 90.0

\_cell\_angle\_beta 90.0

\_cell\_angle\_gamma 90.0

\_symmetry\_space\_group\_name\_H-M 'P 1'

\_symmetry\_Int\_Tables\_number 1

\_symmetry\_cell\_setting triclinic

loop\_

\_atom\_site\_label

\_atom\_site\_type\_symbol

\_atom\_site\_fract\_x

\_atom\_site\_fract\_y

\_atom\_site\_fract\_z

\_atom\_site\_occupancy

|    |   |                    |                    |                    |     |
|----|---|--------------------|--------------------|--------------------|-----|
| H1 | H | 0.9046607400000000 | 0.0949010400000000 | 0.0611477400000000 | 1.0 |
|----|---|--------------------|--------------------|--------------------|-----|

|    |   |                    |                    |                    |     |
|----|---|--------------------|--------------------|--------------------|-----|
| H2 | H | 0.8875292400000000 | 0.8931235000000000 | 0.0440084800000000 | 1.0 |
|----|---|--------------------|--------------------|--------------------|-----|

|    |   |                    |                    |                    |     |
|----|---|--------------------|--------------------|--------------------|-----|
| H3 | H | 0.1644051200000000 | 0.1030158300000000 | 0.0461871800000000 | 1.0 |
|----|---|--------------------|--------------------|--------------------|-----|

|    |   |                    |                    |                    |     |
|----|---|--------------------|--------------------|--------------------|-----|
| H4 | H | 0.1526568100000000 | 0.9008352200000000 | 0.0595919800000000 | 1.0 |
|----|---|--------------------|--------------------|--------------------|-----|

|    |   |                    |                    |                    |     |
|----|---|--------------------|--------------------|--------------------|-----|
| H5 | H | 0.4017824900000000 | 0.0953865600000000 | 0.0625648700000000 | 1.0 |
|----|---|--------------------|--------------------|--------------------|-----|

|    |   |                    |                    |                    |     |
|----|---|--------------------|--------------------|--------------------|-----|
| H6 | H | 0.3900514000000000 | 0.8937093900000000 | 0.0430134500000000 | 1.0 |
|----|---|--------------------|--------------------|--------------------|-----|



|     |   |                    |                    |                    |     |
|-----|---|--------------------|--------------------|--------------------|-----|
| H7  | H | 0.6669407900000000 | 0.1034226300000000 | 0.0473919800000000 | 1.0 |
| H8  | H | 0.6498187700000000 | 0.9011996800000000 | 0.0580172100000000 | 1.0 |
| H9  | H | 0.9853146300000000 | 0.0868659700000000 | 0.8837283400000000 | 1.0 |
| H10 | H | 0.2508920800000000 | 0.0730275300000000 | 0.8966281700000000 | 1.0 |
| H11 | H | 0.4835218900000000 | 0.0900635000000000 | 0.8852350400000000 | 1.0 |
| H12 | H | 0.7502566300000000 | 0.0738374600000000 | 0.8964599800000000 | 1.0 |
| H13 | H | 0.8042676000000000 | 0.9275549900000000 | 0.8941065600000000 | 1.0 |
| H14 | H | 0.0709575900000000 | 0.9115880100000000 | 0.8824774800000000 | 1.0 |
| H15 | H | 0.3035069700000000 | 0.9282445300000000 | 0.8944362300000000 | 1.0 |
| H16 | H | 0.5690911500000000 | 0.9149294600000000 | 0.8809837600000000 | 1.0 |
| C17 | C | 0.8694167300000000 | 0.0525895600000000 | 0.0306834700000000 | 1.0 |
| C18 | C | 0.9500564000000000 | 0.0407864400000000 | 0.9660480400000000 | 1.0 |
| C19 | C | 0.9389157400000000 | 0.9614667100000000 | 0.9603912900000000 | 1.0 |
| C20 | C | 0.8531600800000000 | 0.9411493400000000 | 0.0232865400000000 | 1.0 |
| C21 | C | 0.2005505500000000 | 0.0555714700000000 | 0.0248474100000000 | 1.0 |
| C22 | C | 0.1160803100000000 | 0.0359271500000000 | 0.9611472500000000 | 1.0 |
| C23 | C | 0.1048290900000000 | 0.9565384300000000 | 0.9655931600000000 | 1.0 |
| C24 | C | 0.1859487000000000 | 0.9440101100000000 | 0.0298296700000000 | 1.0 |
| C25 | C | 0.3684983400000000 | 0.0531374800000000 | 0.0315042700000000 | 1.0 |
| C26 | C | 0.4496362600000000 | 0.0425669200000000 | 0.9669232700000000 | 1.0 |
| C27 | C | 0.4383922800000000 | 0.9633543600000000 | 0.9600370200000000 | 1.0 |
| C28 | C | 0.3539213400000000 | 0.9417797900000000 | 0.0231198200000000 | 1.0 |
| C29 | C | 0.7013149200000000 | 0.0560936000000000 | 0.0251295900000000 | 1.0 |
| C30 | C | 0.6155634100000000 | 0.0378091300000000 | 0.9615997200000000 | 1.0 |
| C31 | C | 0.6044329000000000 | 0.9583505400000000 | 0.9647248300000000 | 1.0 |
| C32 | C | 0.6850830500000000 | 0.9444680400000000 | 0.0289365600000000 | 1.0 |
| O33 | O | 0.8958004900000000 | 0.9928252900000000 | 0.0682196600000000 | 1.0 |
| O34 | O | 0.9034510700000000 | 0.0820882200000000 | 0.9134631700000000 | 1.0 |
| O35 | O | 0.9066418300000000 | 0.9358065700000000 | 0.8972241600000000 | 1.0 |
| O36 | O | 0.1584809600000000 | 0.0028107400000000 | 0.0686337600000000 | 1.0 |
| O37 | O | 0.1493151600000000 | 0.0622061600000000 | 0.8983430800000000 | 1.0 |
| O38 | O | 0.1522642900000000 | 0.9158574300000000 | 0.9126165600000000 | 1.0 |
| O39 | O | 0.3959516000000000 | 0.9931817000000000 | 0.0685013800000000 | 1.0 |
| O40 | O | 0.4021891300000000 | 0.0848285900000000 | 0.9151994700000000 | 1.0 |
| O41 | O | 0.4050868100000000 | 0.9390289000000000 | 0.8964673100000000 | 1.0 |
| O42 | O | 0.6586702200000000 | 0.0029930900000000 | 0.0683721200000000 | 1.0 |
| O43 | O | 0.6478868000000000 | 0.0654604200000000 | 0.8992789300000000 | 1.0 |
| O44 | O | 0.6510192600000000 | 0.9187993500000000 | 0.9108111100000000 | 1.0 |

##### cif ends

furan\_OH\_3\_anti\_alt    Energy: -253.61421929

##### cif starts

data\_furan\_OH\_3\_anti\_alt

\_publ\_section\_comment

;  
Andrew Reynoso, Bohan Xu, and Vincent H. Crespi  
;

\_cell\_length\_a    9.3331811083

\_cell\_length\_b    20.0

\_cell\_length\_c    20.0

\_cell\_angle\_alpha    90.0

\_cell\_angle\_beta    90.0

\_cell\_angle\_gamma 90.0

\_symmetry\_space\_group\_name\_H-M 'P 1'

\_symmetry\_Int\_Tables\_number 1

\_symmetry\_cell\_setting triclinic

loop\_

\_atom\_site\_label

\_atom\_site\_type\_symbol

\_atom\_site\_fract\_x

\_atom\_site\_fract\_y

\_atom\_site\_fract\_z

\_atom\_site\_occupancy

|     |   |                    |                    |                    |     |
|-----|---|--------------------|--------------------|--------------------|-----|
| H1  | H | 0.0585747900000000 | 0.9556935100000000 | 0.0858879900000000 | 1.0 |
| H2  | H | 0.9750538000000000 | 0.0621824300000000 | 0.0742259100000000 | 1.0 |
| H3  | H | 0.9859425900000000 | 0.9249319100000000 | 0.9153134500000000 | 1.0 |
| H4  | H | 0.9894766600000000 | 0.1269771900000000 | 0.9499448400000000 | 1.0 |
| H5  | H | 0.3084885500000000 | 0.0773379800000000 | 0.8937945400000000 | 1.0 |
| H6  | H | 0.2250152500000000 | 0.9708436900000000 | 0.9054480400000000 | 1.0 |
| H7  | H | 0.2359675900000000 | 0.1080467000000000 | 0.0643988500000000 | 1.0 |
| H8  | H | 0.2394804100000000 | 0.9060123200000000 | 0.0297057500000000 | 1.0 |
| H9  | H | 0.5584918800000000 | 0.9556790800000000 | 0.0858974900000000 | 1.0 |
| H10 | H | 0.4750559600000000 | 0.0621555600000000 | 0.0742103200000000 | 1.0 |
| H11 | H | 0.4860321100000000 | 0.9249142300000000 | 0.9153016800000000 | 1.0 |
| H12 | H | 0.4894699800000000 | 0.1269606500000000 | 0.9499302400000000 | 1.0 |
| H13 | H | 0.8085110400000000 | 0.0773369900000000 | 0.8938115000000000 | 1.0 |
| H14 | H | 0.7250974000000000 | 0.9708308600000000 | 0.9054855400000000 | 1.0 |
| H15 | H | 0.7359541400000000 | 0.1080724100000000 | 0.0643999800000000 | 1.0 |
| H16 | H | 0.7394975500000000 | 0.9060314900000000 | 0.0297618000000000 | 1.0 |
| C17 | C | 0.0111199600000000 | 0.0757289600000000 | 0.9661852400000000 | 1.0 |
| C18 | C | 0.9251378900000000 | 0.0501760400000000 | 0.0260286300000000 | 1.0 |
| C19 | C | 0.9249175800000000 | 0.9721423900000000 | 0.0135876700000000 | 1.0 |
| C20 | C | 0.0111321600000000 | 0.9681527800000000 | 0.9469743800000000 | 1.0 |
| C21 | C | 0.2611371100000000 | 0.9572653500000000 | 0.0134859200000000 | 1.0 |
| C22 | C | 0.1751309700000000 | 0.9828390300000000 | 0.9536552500000000 | 1.0 |
| C23 | C | 0.1748967100000000 | 0.0608645100000000 | 0.9661193400000000 | 1.0 |
| C24 | C | 0.2611390400000000 | 0.0648353100000000 | 0.0327236100000000 | 1.0 |
| C25 | C | 0.5111224400000000 | 0.0757147800000000 | 0.9661741300000000 | 1.0 |
| C26 | C | 0.4251347100000000 | 0.0501566300000000 | 0.0260121900000000 | 1.0 |
| C27 | C | 0.4249142900000000 | 0.9721247900000000 | 0.0135616000000000 | 1.0 |
| C28 | C | 0.5111728000000000 | 0.9681388000000000 | 0.9469649400000000 | 1.0 |
| C29 | C | 0.7611421000000000 | 0.9572799200000000 | 0.0135258600000000 | 1.0 |
| C30 | C | 0.6751613500000000 | 0.9828348500000000 | 0.9536785500000000 | 1.0 |
| C31 | C | 0.6749033700000000 | 0.0608642300000000 | 0.9661263300000000 | 1.0 |
| C32 | C | 0.7611317700000000 | 0.0648533900000000 | 0.0327355600000000 | 1.0 |
| O33 | O | 0.9668204900000000 | 0.0291025100000000 | 0.9131217500000000 | 1.0 |
| O34 | O | 0.9776192300000000 | 0.9314118800000000 | 0.0661045700000000 | 1.0 |
| O35 | O | 0.2168766100000000 | 0.0038736600000000 | 0.0665696900000000 | 1.0 |
| O36 | O | 0.2276027800000000 | 0.1016243300000000 | 0.9136201800000000 | 1.0 |
| O37 | O | 0.4668576100000000 | 0.0290855800000000 | 0.9131065000000000 | 1.0 |
| O38 | O | 0.4775888900000000 | 0.9313883200000000 | 0.0660818800000000 | 1.0 |
| O39 | O | 0.7168666700000000 | 0.0039001800000000 | 0.0665953800000000 | 1.0 |
| O40 | O | 0.7276061900000000 | 0.1016212400000000 | 0.9136257500000000 | 1.0 |

##### cif ends

furandiol\_anti\_alt\_forbid Energy: -253.41862426

##### cif starts

data\_furandiol\_anti\_alt\_forbid

\_publ\_section\_comment

;  
Andrew Reynoso, Bohan Xu, and Vincent H. Crespi  
;

\_cell\_length\_a 10.1861150321

\_cell\_length\_b 20.0

\_cell\_length\_c 20.0

\_cell\_angle\_alpha 90.0

\_cell\_angle\_beta 90.0

\_cell\_angle\_gamma 90.0

\_symmetry\_space\_group\_name\_H-M 'P 1'

\_symmetry\_Int\_Tables\_number 1

\_symmetry\_cell\_setting triclinic

loop\_

\_atom\_site\_label

\_atom\_site\_type\_symbol

\_atom\_site\_fract\_x

\_atom\_site\_fract\_y

\_atom\_site\_fract\_z

\_atom\_site\_occupancy

|     |   |                    |                    |                    |     |
|-----|---|--------------------|--------------------|--------------------|-----|
| H1  | H | 0.0688815000000000 | 0.0972371900000000 | 0.9321359300000000 | 1.0 |
| H2  | H | 0.9514247100000000 | 0.9330891200000000 | 0.0555324500000000 | 1.0 |
| H3  | H | 0.0680438000000000 | 0.8932813300000000 | 0.9351679400000000 | 1.0 |
| H4  | H | 0.3282365400000000 | 0.0592760900000000 | 0.9166826700000000 | 1.0 |
| H5  | H | 0.2117882800000000 | 0.0990556500000000 | 0.0370781400000000 | 1.0 |
| H6  | H | 0.2109673800000000 | 0.8950984000000000 | 0.0400815100000000 | 1.0 |
| H7  | H | 0.5687515100000000 | 0.0969826900000000 | 0.9315799900000000 | 1.0 |
| H8  | H | 0.4509421800000000 | 0.9333388000000000 | 0.0555644500000000 | 1.0 |
| H9  | H | 0.5679853800000000 | 0.8930457800000000 | 0.9354917700000000 | 1.0 |
| H10 | H | 0.8289412000000000 | 0.0589508800000000 | 0.9165113500000000 | 1.0 |
| H11 | H | 0.7117032800000000 | 0.0992936300000000 | 0.0365253200000000 | 1.0 |
| H12 | H | 0.7108162500000000 | 0.8953474000000000 | 0.0404851400000000 | 1.0 |
| H13 | H | 0.2593542500000000 | 0.9386953200000000 | 0.8776336200000000 | 1.0 |
| H14 | H | 0.7591529300000000 | 0.9382266500000000 | 0.8778384000000000 | 1.0 |
| H15 | H | 0.0202028600000000 | 0.0536785900000000 | 0.0945453000000000 | 1.0 |
| H16 | H | 0.5210034200000000 | 0.0540536200000000 | 0.0942007400000000 | 1.0 |
| C17 | C | 0.0787766000000000 | 0.0519749300000000 | 0.9629230300000000 | 1.0 |
| C18 | C | 0.9558605500000000 | 0.0356485200000000 | 0.0056955400000000 | 1.0 |
| C19 | C | 0.9550916800000000 | 0.9565336400000000 | 0.0059602400000000 | 1.0 |
| C20 | C | 0.0765971400000000 | 0.9389562600000000 | 0.9651590000000000 | 1.0 |
| C21 | C | 0.2031761200000000 | 0.0533809200000000 | 0.0070846700000000 | 1.0 |
| C22 | C | 0.3246351800000000 | 0.0358083900000000 | 0.9662418000000000 | 1.0 |
| C23 | C | 0.3238524400000000 | 0.9567000200000000 | 0.9664659400000000 | 1.0 |
| C24 | C | 0.2010083100000000 | 0.9403608300000000 | 0.0093007700000000 | 1.0 |
| C25 | C | 0.5787712700000000 | 0.0518718500000000 | 0.9625756400000000 | 1.0 |
| C26 | C | 0.4559474300000000 | 0.0357484300000000 | 0.0055369000000000 | 1.0 |
| C27 | C | 0.4550041000000000 | 0.9566388500000000 | 0.0059349200000000 | 1.0 |

|     |   |                    |                    |                    |     |
|-----|---|--------------------|--------------------|--------------------|-----|
| C28 | C | 0.5765645500000000 | 0.9388527200000000 | 0.9652867900000000 | 1.0 |
| C29 | C | 0.7031553000000000 | 0.0534763300000000 | 0.0067407100000000 | 1.0 |
| C30 | C | 0.8247835900000000 | 0.0356762100000000 | 0.9661497800000000 | 1.0 |
| C31 | C | 0.8238592800000000 | 0.9565653800000000 | 0.9665826200000000 | 1.0 |
| C32 | C | 0.7009325500000000 | 0.9404496600000000 | 0.0094693400000000 | 1.0 |
| O33 | O | 0.9499475400000000 | 0.0714654700000000 | 0.0664146200000000 | 1.0 |
| O34 | O | 0.3296683100000000 | 0.9209170900000000 | 0.9057301600000000 | 1.0 |
| O35 | O | 0.0876877700000000 | 0.9950646400000000 | 0.9183544800000000 | 1.0 |
| O36 | O | 0.1921184800000000 | 0.9972652200000000 | 0.0538837900000000 | 1.0 |
| O37 | O | 0.4504653100000000 | 0.0717184200000000 | 0.0661745300000000 | 1.0 |
| O38 | O | 0.8295487300000000 | 0.9205736100000000 | 0.9059605100000000 | 1.0 |
| O39 | O | 0.5877183200000000 | 0.9947690700000000 | 0.9182546200000000 | 1.0 |
| O40 | O | 0.6919771200000000 | 0.9975629400000000 | 0.0537816600000000 | 1.0 |

##### cif ends

  furan\_OH\_3\_anti\_dir  Energy: -252.95958369

##### cif starts

data\_furan\_OH\_3\_anti\_dir

\_publ\_section\_comment

;  
Andrew Reynoso, Bohan Xu, and Vincent H. Crespi  
;

\_cell\_length\_a  9.3819349256

\_cell\_length\_b  20.0

\_cell\_length\_c  20.0

\_cell\_angle\_alpha  90.0

\_cell\_angle\_beta  90.0

\_cell\_angle\_gamma  90.0

\_symmetry\_space\_group\_name\_H-M  'P 1'

\_symmetry\_Int\_Tables\_number  1

\_symmetry\_cell\_setting  triclinic

loop\_

\_atom\_site\_label

\_atom\_site\_type\_symbol

\_atom\_site\_fract\_x

\_atom\_site\_fract\_y

\_atom\_site\_fract\_z

\_atom\_site\_occupancy

|     |   |                    |                    |                    |     |
|-----|---|--------------------|--------------------|--------------------|-----|
| H1  | H | 0.9453886000000000 | 0.0476889000000000 | 0.1222732800000000 | 1.0 |
| H2  | H | 0.9874759200000000 | 0.9322230300000000 | 0.0715533900000000 | 1.0 |
| H3  | H | 0.9968738900000000 | 0.0934930700000000 | 0.9392395900000000 | 1.0 |
| H4  | H | 0.9992664200000000 | 0.8890835400000000 | 0.9376513600000000 | 1.0 |
| H5  | H | 0.1953327200000000 | 0.0502760100000000 | 0.8717041800000000 | 1.0 |
| H6  | H | 0.2374801900000000 | 0.9337439000000000 | 0.9200944400000000 | 1.0 |
| H7  | H | 0.2468784100000000 | 0.0923409500000000 | 0.0555981300000000 | 1.0 |
| H8  | H | 0.2492631100000000 | 0.8879385800000000 | 0.0531133300000000 | 1.0 |
| H9  | H | 0.4453387600000000 | 0.0477414300000000 | 0.1222593300000000 | 1.0 |
| H10 | H | 0.4874792000000000 | 0.9322386700000000 | 0.0715544500000000 | 1.0 |
| H11 | H | 0.4969013000000000 | 0.0934911900000000 | 0.9392243800000000 | 1.0 |
| H12 | H | 0.4992463300000000 | 0.8890825800000000 | 0.9376557200000000 | 1.0 |

|     |   |                    |                    |                    |     |
|-----|---|--------------------|--------------------|--------------------|-----|
| H13 | H | 0.6954894200000000 | 0.0501960500000000 | 0.8716907100000000 | 1.0 |
| H14 | H | 0.7374706600000000 | 0.9337316700000000 | 0.9200919600000000 | 1.0 |
| H15 | H | 0.7468735500000000 | 0.0923308600000000 | 0.0556040300000000 | 1.0 |
| H16 | H | 0.7492582000000000 | 0.8879280200000000 | 0.0531068900000000 | 1.0 |
| C17 | C | 0.0239767700000000 | 0.9368374800000000 | 0.9621742200000000 | 1.0 |
| C18 | C | 0.9371968000000000 | 0.9516378000000000 | 0.0259636800000000 | 1.0 |
| C19 | C | 0.9335889800000000 | 0.0307042600000000 | 0.0266876100000000 | 1.0 |
| C20 | C | 0.0195143200000000 | 0.0455422400000000 | 0.9631567400000000 | 1.0 |
| C21 | C | 0.2739731500000000 | 0.9361725700000000 | 0.0295449500000000 | 1.0 |
| C22 | C | 0.1872014100000000 | 0.9522384200000000 | 0.9660615600000000 | 1.0 |
| C23 | C | 0.1835936900000000 | 0.0313080300000000 | 0.9669172500000000 | 1.0 |
| C24 | C | 0.2695158200000000 | 0.0448771400000000 | 0.0307270600000000 | 1.0 |
| C25 | C | 0.5239690000000000 | 0.9368364700000000 | 0.9621738800000000 | 1.0 |
| C26 | C | 0.4371996800000000 | 0.9516456400000000 | 0.0259645800000000 | 1.0 |
| C27 | C | 0.4335922800000000 | 0.0307128800000000 | 0.0266796400000000 | 1.0 |
| C28 | C | 0.5195234800000000 | 0.0455432400000000 | 0.9631473800000000 | 1.0 |
| C29 | C | 0.7739695700000000 | 0.9361638400000000 | 0.0295418300000000 | 1.0 |
| C30 | C | 0.6871991200000000 | 0.9522317700000000 | 0.9660599500000000 | 1.0 |
| C31 | C | 0.6836016700000000 | 0.0313004500000000 | 0.9669151200000000 | 1.0 |
| C32 | C | 0.7695148400000000 | 0.0448670700000000 | 0.0307289300000000 | 1.0 |
| O33 | O | 0.9790081800000000 | 0.9910726400000000 | 0.9185932700000000 | 1.0 |
| O34 | O | 0.9948236000000000 | 0.0640722500000000 | 0.0826754300000000 | 1.0 |
| O35 | O | 0.2290108000000000 | 0.9895323800000000 | 0.0741975000000000 | 1.0 |
| O36 | O | 0.2448557700000000 | 0.0657956900000000 | 0.9116181900000000 | 1.0 |
| O37 | O | 0.4790101100000000 | 0.9910702200000000 | 0.9185881700000000 | 1.0 |
| O38 | O | 0.4948334100000000 | 0.0640882100000000 | 0.0826618700000000 | 1.0 |
| O39 | O | 0.7290018400000000 | 0.9895205600000000 | 0.0741956200000000 | 1.0 |
| O40 | O | 0.7448789300000000 | 0.0657824600000000 | 0.9116156000000000 | 1.0 |

##### cif ends

furan\_OH\_3\_anti\_dir\_forbid Energy: -253.30472897

##### cif starts

data\_furan\_OH\_3\_anti\_dir\_forbid

\_publ\_section\_comment

;

Andrew Reynoso, Bohan Xu, and Vincent H. Crespi

;

\_cell\_length\_a 10.1855120923

\_cell\_length\_b 20.0

\_cell\_length\_c 20.0

\_cell\_angle\_alpha 90.0

\_cell\_angle\_beta 90.0

\_cell\_angle\_gamma 90.0

\_symmetry\_space\_group\_name\_H-M 'P 1'

\_symmetry\_Int\_Tables\_number 1

\_symmetry\_cell\_setting triclinic

loop\_

\_atom\_site\_label

\_atom\_site\_type\_symbol

\_atom\_site\_fract\_x

|     |   | _atom_site_fract_y |                    | _atom_site_fract_z |     | _atom_site_occupancy |  |
|-----|---|--------------------|--------------------|--------------------|-----|----------------------|--|
| H1  | H | 0.8993988300000000 | 0.0483439200000000 | 0.1154911400000000 | 1.0 |                      |  |
| H2  | H | 0.8296774200000000 | 0.9277500500000000 | 0.0736235200000000 | 1.0 |                      |  |
| H3  | H | 0.9485521700000000 | 0.0945001500000000 | 0.9538179100000000 | 1.0 |                      |  |
| H4  | H | 0.9466351500000000 | 0.8903063000000000 | 0.9519260600000000 | 1.0 |                      |  |
| H5  | H | 0.2729656900000000 | 0.0501545600000000 | 0.8968092700000000 | 1.0 |                      |  |
| H6  | H | 0.2061746500000000 | 0.9296974700000000 | 0.9348489100000000 | 1.0 |                      |  |
| H7  | H | 0.0915660200000000 | 0.0935091600000000 | 0.0578268100000000 | 1.0 |                      |  |
| H8  | H | 0.0894136500000000 | 0.8896606800000000 | 0.0556611000000000 | 1.0 |                      |  |
| H9  | H | 0.3990484000000000 | 0.0477944800000000 | 0.1156516800000000 | 1.0 |                      |  |
| H10 | H | 0.3302898800000000 | 0.9273772000000000 | 0.0735212700000000 | 1.0 |                      |  |
| H11 | H | 0.4481835800000000 | 0.0945610500000000 | 0.9540883700000000 | 1.0 |                      |  |
| H12 | H | 0.4469206000000000 | 0.8903677700000000 | 0.9515924000000000 | 1.0 |                      |  |
| H13 | H | 0.7723733800000000 | 0.0509499100000000 | 0.8968013200000000 | 1.0 |                      |  |
| H14 | H | 0.7066630900000000 | 0.9300981900000000 | 0.9346500000000000 | 1.0 |                      |  |
| H15 | H | 0.5911821500000000 | 0.0934146800000000 | 0.0581081800000000 | 1.0 |                      |  |
| H16 | H | 0.5898344000000000 | 0.8895721900000000 | 0.0552429000000000 | 1.0 |                      |  |
| C17 | C | 0.9549082900000000 | 0.9356701200000000 | 0.9827500400000000 | 1.0 |                      |  |
| C18 | C | 0.8335215300000000 | 0.9521748600000000 | 0.0245298500000000 | 1.0 |                      |  |
| C19 | C | 0.8357637900000000 | 0.0313429000000000 | 0.0262502000000000 | 1.0 |                      |  |
| C20 | C | 0.9575811400000000 | 0.0485126100000000 | 0.9832826800000000 | 1.0 |                      |  |
| C21 | C | 0.0810478500000000 | 0.9355255300000000 | 0.0255767100000000 | 1.0 |                      |  |
| C22 | C | 0.2034824400000000 | 0.9528411000000000 | 0.9846212500000000 | 1.0 |                      |  |
| C23 | C | 0.2042642600000000 | 0.0320476100000000 | 0.9852838300000000 | 1.0 |                      |  |
| C24 | C | 0.0819969700000000 | 0.0483395900000000 | 0.0271713100000000 | 1.0 |                      |  |
| C25 | C | 0.4550192600000000 | 0.9356541200000000 | 0.9825413200000000 | 1.0 |                      |  |
| C26 | C | 0.3336716500000000 | 0.9519191400000000 | 0.0244736700000000 | 1.0 |                      |  |
| C27 | C | 0.3357338800000000 | 0.0310798700000000 | 0.0263179500000000 | 1.0 |                      |  |
| C28 | C | 0.4574546900000000 | 0.0485014200000000 | 0.9834167800000000 | 1.0 |                      |  |
| C29 | C | 0.5812028700000000 | 0.9355314900000000 | 0.0253251700000000 | 1.0 |                      |  |
| C30 | C | 0.7035897000000000 | 0.9531133500000000 | 0.9844739400000000 | 1.0 |                      |  |
| C31 | C | 0.7041972400000000 | 0.0323301000000000 | 0.9853244100000000 | 1.0 |                      |  |
| C32 | C | 0.5818766500000000 | 0.0483335600000000 | 0.0273013900000000 | 1.0 |                      |  |
| O33 | O | 0.9630152100000000 | 0.9924213000000000 | 0.9371123500000000 | 1.0 |                      |  |
| O34 | O | 0.8288901500000000 | 0.0660316200000000 | 0.0874963100000000 | 1.0 |                      |  |
| O35 | O | 0.0725575900000000 | 0.9914339900000000 | 0.0722025300000000 | 1.0 |                      |  |
| O36 | O | 0.2043165700000000 | 0.0688560900000000 | 0.9252743400000000 | 1.0 |                      |  |
| O37 | O | 0.4629478800000000 | 0.9925468700000000 | 0.9370670600000000 | 1.0 |                      |  |
| O38 | O | 0.3286542600000000 | 0.0655946700000000 | 0.0876521500000000 | 1.0 |                      |  |
| O39 | O | 0.5726039500000000 | 0.9912761900000000 | 0.0721465300000000 | 1.0 |                      |  |
| O40 | O | 0.7038197200000000 | 0.0694029100000000 | 0.9254701500000000 | 1.0 |                      |  |

##### cif ends

furan\_OH\_3\_syn\_alt    Energy: -252.91312413

##### cif starts

data\_furan\_OH\_3\_syn\_alt

\_publ\_section\_comment

;  
 Andrew Reynoso, Bohan Xu, and Vincent H. Crespi  
 ;

\_cell\_length\_a 10.3103863324  
\_cell\_length\_b 20.0  
\_cell\_length\_c 20.0  
\_cell\_angle\_alpha 90.0  
\_cell\_angle\_beta 90.0  
\_cell\_angle\_gamma 90.0

\_symmetry\_space\_group\_name\_H-M 'P 1'  
\_symmetry\_Int\_Tables\_number 1  
\_symmetry\_cell\_setting triclinic

loop\_  
\_atom\_site\_label  
\_atom\_site\_type\_symbol  
\_atom\_site\_fract\_x  
\_atom\_site\_fract\_y  
\_atom\_site\_fract\_z  
\_atom\_site\_occupancy

|     |   |                    |                    |                    |     |
|-----|---|--------------------|--------------------|--------------------|-----|
| H1  | H | 0.1097447700000000 | 0.9551254900000000 | 0.8874437700000000 | 1.0 |
| H2  | H | 0.1083005700000000 | 0.0537792400000000 | 0.9415915300000000 | 1.0 |
| H3  | H | 0.9845978000000000 | 0.8835429900000000 | 0.0511392700000000 | 1.0 |
| H4  | H | 0.9820736500000000 | 0.0870586900000000 | 0.0602728300000000 | 1.0 |
| H5  | H | 0.3601595300000000 | 0.0305058200000000 | 0.8908718400000000 | 1.0 |
| H6  | H | 0.3582498200000000 | 0.9273622100000000 | 0.9358881400000000 | 1.0 |
| H7  | H | 0.2344418500000000 | 0.0870438600000000 | 0.0602999300000000 | 1.0 |
| H8  | H | 0.2319880800000000 | 0.8835299400000000 | 0.0510945300000000 | 1.0 |
| H9  | H | 0.6084054300000000 | 0.9551109700000000 | 0.8874485400000000 | 1.0 |
| H10 | H | 0.6083603800000000 | 0.0537643300000000 | 0.9415918500000000 | 1.0 |
| H11 | H | 0.4845070000000000 | 0.8835313200000000 | 0.0511080200000000 | 1.0 |
| H12 | H | 0.4820957900000000 | 0.0870428900000000 | 0.0603008000000000 | 1.0 |
| H13 | H | 0.8594966900000000 | 0.0304314800000000 | 0.8908504500000000 | 1.0 |
| H14 | H | 0.8583926900000000 | 0.9273193400000000 | 0.9359121900000000 | 1.0 |
| H15 | H | 0.7346003900000000 | 0.0870514400000000 | 0.0602645000000000 | 1.0 |
| H16 | H | 0.7320868100000000 | 0.8835356100000000 | 0.0511329000000000 | 1.0 |
| C17 | C | 0.9837151800000000 | 0.0402716400000000 | 0.0315814400000000 | 1.0 |
| C18 | C | 0.1082849600000000 | 0.0281301000000000 | 0.9901393400000000 | 1.0 |
| C19 | C | 0.1082681700000000 | 0.9495917900000000 | 0.9857968700000000 | 1.0 |
| C20 | C | 0.9829032000000000 | 0.9327091200000000 | 0.0267509700000000 | 1.0 |
| C21 | C | 0.2336688800000000 | 0.9327033000000000 | 0.0267225100000000 | 1.0 |
| C22 | C | 0.3582702500000000 | 0.9485319500000000 | 0.9865542600000000 | 1.0 |
| C23 | C | 0.3582638500000000 | 0.0271500100000000 | 0.9893192800000000 | 1.0 |
| C24 | C | 0.2328580200000000 | 0.0402674300000000 | 0.0315920900000000 | 1.0 |
| C25 | C | 0.4837183700000000 | 0.0402694600000000 | 0.0315875000000000 | 1.0 |
| C26 | C | 0.6083103700000000 | 0.0281204400000000 | 0.9901458100000000 | 1.0 |
| C27 | C | 0.6083080500000000 | 0.9495773600000000 | 0.9858095700000000 | 1.0 |
| C28 | C | 0.4828788200000000 | 0.9327015900000000 | 0.0267282700000000 | 1.0 |
| C29 | C | 0.7337173000000000 | 0.9326996200000000 | 0.0267414700000000 | 1.0 |
| C30 | C | 0.8583138100000000 | 0.9485096800000000 | 0.9865649300000000 | 1.0 |
| C31 | C | 0.8583158000000000 | 0.0271277700000000 | 0.9892945400000000 | 1.0 |
| C32 | C | 0.7329191100000000 | 0.0402668500000000 | 0.0315728700000000 | 1.0 |
| O33 | O | 0.9833181200000000 | 0.9843513300000000 | 0.0767823700000000 | 1.0 |
| O34 | O | 0.1079444900000000 | 0.9197845900000000 | 0.9206789700000000 | 1.0 |
| O35 | O | 0.2332679800000000 | 0.9843312600000000 | 0.0767720100000000 | 1.0 |
| O36 | O | 0.3579143700000000 | 0.0627131800000000 | 0.9271477300000000 | 1.0 |
| O37 | O | 0.4832921100000000 | 0.9843335400000000 | 0.0767710000000000 | 1.0 |

|     |   |                    |                    |                    |     |
|-----|---|--------------------|--------------------|--------------------|-----|
| O38 | O | 0.6082874300000000 | 0.9197600300000000 | 0.9206944000000000 | 1.0 |
| O39 | O | 0.7333239600000000 | 0.9843467100000000 | 0.0767727000000000 | 1.0 |
| O40 | O | 0.8581848500000000 | 0.0626701300000000 | 0.9271184200000000 | 1.0 |

##### cif ends

furan\_OH\_3\_syn\_alt\_forbid Energy: -250.62340893

##### cif starts

data\_furan\_OH\_3\_syn\_alt\_forbid

\_publ\_section\_comment

;  
Andrew Reynoso, Bohan Xu, and Vincent H. Crespi  
;

\_cell\_length\_a 9.5040464651

\_cell\_length\_b 20.0

\_cell\_length\_c 20.0

\_cell\_angle\_alpha 90.0

\_cell\_angle\_beta 90.0

\_cell\_angle\_gamma 90.0

\_symmetry\_space\_group\_name\_H-M 'P 1'

\_symmetry\_Int\_Tables\_number 1

\_symmetry\_cell\_setting triclinic

loop\_

\_atom\_site\_label

\_atom\_site\_type\_symbol

\_atom\_site\_fract\_x

\_atom\_site\_fract\_y

\_atom\_site\_fract\_z

\_atom\_site\_occupancy

|     |   |                    |                    |                    |     |
|-----|---|--------------------|--------------------|--------------------|-----|
| H1  | H | 0.8956869100000000 | 0.1017199600000000 | 0.0650435300000000 | 1.0 |
| H2  | H | 0.8946637800000000 | 0.9356446700000000 | 0.9330011300000000 | 1.0 |
| H3  | H | 0.8951533800000000 | 0.8995226700000000 | 0.0684794900000000 | 1.0 |
| H4  | H | 0.1507659900000000 | 0.1015295600000000 | 0.0640903100000000 | 1.0 |
| H5  | H | 0.1512157800000000 | 0.0595587100000000 | 0.9303056800000000 | 1.0 |
| H6  | H | 0.1502104700000000 | 0.8993680100000000 | 0.0694216400000000 | 1.0 |
| H7  | H | 0.3956970900000000 | 0.1016833300000000 | 0.0650686300000000 | 1.0 |
| H8  | H | 0.3947023500000000 | 0.9356420100000000 | 0.9329828600000000 | 1.0 |
| H9  | H | 0.3951341500000000 | 0.8994860000000000 | 0.0684518800000000 | 1.0 |
| H10 | H | 0.6507623700000000 | 0.1015571400000000 | 0.0640643900000000 | 1.0 |
| H11 | H | 0.6511982600000000 | 0.0595514100000000 | 0.9302940200000000 | 1.0 |
| H12 | H | 0.6502281100000000 | 0.8993993700000000 | 0.0694593500000000 | 1.0 |
| H13 | H | 0.9569546500000000 | 0.0770905200000000 | 0.8863463300000000 | 1.0 |
| H14 | H | 0.4568841200000000 | 0.0770484700000000 | 0.8863332500000000 | 1.0 |
| H15 | H | 0.0891304800000000 | 0.9165226000000000 | 0.8896878300000000 | 1.0 |
| H16 | H | 0.5891973500000000 | 0.9164933600000000 | 0.8897021500000000 | 1.0 |
| C17 | C | 0.8587395800000000 | 0.0557481200000000 | 0.0407020100000000 | 1.0 |
| C18 | C | 0.9404641900000000 | 0.0384876900000000 | 0.9760323200000000 | 1.0 |
| C19 | C | 0.9387154600000000 | 0.9597075300000000 | 0.9776649000000000 | 1.0 |
| C20 | C | 0.8577265300000000 | 0.9443665100000000 | 0.0422659700000000 | 1.0 |
| C21 | C | 0.1881903800000000 | 0.0555870400000000 | 0.0398526100000000 | 1.0 |
| C22 | C | 0.1071831600000000 | 0.0374602900000000 | 0.9759783100000000 | 1.0 |



|     |   |                    |                    |                    |     |
|-----|---|--------------------|--------------------|--------------------|-----|
| C23 | C | 0.1054386700000000 | 0.9586992400000000 | 0.9777499300000000 | 1.0 |
| C24 | C | 0.1871780700000000 | 0.9442422800000000 | 0.0431079200000000 | 1.0 |
| C25 | C | 0.3587438000000000 | 0.0557205500000000 | 0.0407129600000000 | 1.0 |
| C26 | C | 0.4404644400000000 | 0.0384777300000000 | 0.9760358900000000 | 1.0 |
| C27 | C | 0.4387272600000000 | 0.9596968800000000 | 0.9776573900000000 | 1.0 |
| C28 | C | 0.3577196900000000 | 0.9443391900000000 | 0.0422484200000000 | 1.0 |
| C29 | C | 0.6881929000000000 | 0.0556087800000000 | 0.0398395400000000 | 1.0 |
| C30 | C | 0.6071833100000000 | 0.0374592400000000 | 0.9759728100000000 | 1.0 |
| C31 | C | 0.6054509700000000 | 0.9586948100000000 | 0.9777601400000000 | 1.0 |
| C32 | C | 0.6871827400000000 | 0.9442626800000000 | 0.0431272300000000 | 1.0 |
| O33 | O | 0.8927667100000000 | 0.0010045900000000 | 0.0832646700000000 | 1.0 |
| O34 | O | 0.8835367400000000 | 0.0734748300000000 | 0.9200152500000000 | 1.0 |
| O35 | O | 0.1531288900000000 | 0.0007847700000000 | 0.0832620800000000 | 1.0 |
| O36 | O | 0.1623650500000000 | 0.9213328100000000 | 0.9232956800000000 | 1.0 |
| O37 | O | 0.3927652400000000 | 0.0009642400000000 | 0.0832613200000000 | 1.0 |
| O38 | O | 0.3835185000000000 | 0.0734776200000000 | 0.9200320800000000 | 1.0 |
| O39 | O | 0.6531277800000000 | 0.0008165800000000 | 0.0832631500000000 | 1.0 |
| O40 | O | 0.6624041800000000 | 0.9213123600000000 | 0.9233221600000000 | 1.0 |

##### cif ends

furan\_OH\_3\_syn\_dir Energy: -253.82632444

##### cif starts

data\_furan\_OH\_3\_syn\_dir

\_publ\_section\_comment

;  
Andrew Reynoso, Bohan Xu, and Vincent H. Crespi  
;

\_cell\_length\_a 10.3253948843

\_cell\_length\_b 20.0

\_cell\_length\_c 20.0

\_cell\_angle\_alpha 90.0

\_cell\_angle\_beta 90.0

\_cell\_angle\_gamma 90.0

\_symmetry\_space\_group\_name\_H-M 'P 1'

\_symmetry\_Int\_Tables\_number 1

\_symmetry\_cell\_setting triclinic

loop\_

\_atom\_site\_label

\_atom\_site\_type\_symbol

\_atom\_site\_fract\_x

\_atom\_site\_fract\_y

\_atom\_site\_fract\_z

\_atom\_site\_occupancy

|    |   |                    |                    |                    |     |
|----|---|--------------------|--------------------|--------------------|-----|
| H1 | H | 0.9965532600000000 | 0.0970425300000000 | 0.9204706100000000 | 1.0 |
|----|---|--------------------|--------------------|--------------------|-----|

|    |   |                    |                    |                    |     |
|----|---|--------------------|--------------------|--------------------|-----|
| H2 | H | 0.0808954900000000 | 0.9556890200000000 | 0.9271471800000000 | 1.0 |
|----|---|--------------------|--------------------|--------------------|-----|

|    |   |                    |                    |                    |     |
|----|---|--------------------|--------------------|--------------------|-----|
| H3 | H | 0.9555647600000000 | 0.0976417700000000 | 0.0699807000000000 | 1.0 |
|----|---|--------------------|--------------------|--------------------|-----|

|    |   |                    |                    |                    |     |
|----|---|--------------------|--------------------|--------------------|-----|
| H4 | H | 0.9558628100000000 | 0.8964474900000000 | 0.0376891200000000 | 1.0 |
|----|---|--------------------|--------------------|--------------------|-----|

|    |   |                    |                    |                    |     |
|----|---|--------------------|--------------------|--------------------|-----|
| H5 | H | 0.2465262200000000 | 0.0969650800000000 | 0.9204130800000000 | 1.0 |
|----|---|--------------------|--------------------|--------------------|-----|

|    |   |                    |                    |                    |     |
|----|---|--------------------|--------------------|--------------------|-----|
| H6 | H | 0.3310171900000000 | 0.9556206500000000 | 0.9272264300000000 | 1.0 |
|----|---|--------------------|--------------------|--------------------|-----|

|    |   |                    |                    |                    |     |
|----|---|--------------------|--------------------|--------------------|-----|
| H7 | H | 0.2055521500000000 | 0.0976801000000000 | 0.0699484600000000 | 1.0 |
|----|---|--------------------|--------------------|--------------------|-----|

|     |   |                    |                    |                    |     |
|-----|---|--------------------|--------------------|--------------------|-----|
| H8  | H | 0.2057814900000000 | 0.8964712400000000 | 0.0377380300000000 | 1.0 |
| H9  | H | 0.4965254600000000 | 0.0969332300000000 | 0.9203954400000000 | 1.0 |
| H10 | H | 0.5808515800000000 | 0.9555618100000000 | 0.9272902500000000 | 1.0 |
| H11 | H | 0.4555725900000000 | 0.0977841200000000 | 0.0698603400000000 | 1.0 |
| H12 | H | 0.4557640900000000 | 0.8965315400000000 | 0.0379329000000000 | 1.0 |
| H13 | H | 0.7466198800000000 | 0.0969266400000000 | 0.9203718500000000 | 1.0 |
| H14 | H | 0.8306840700000000 | 0.9556278600000000 | 0.9272122000000000 | 1.0 |
| H15 | H | 0.7055394200000000 | 0.0977840600000000 | 0.0698547300000000 | 1.0 |
| H16 | H | 0.7058688200000000 | 0.8965306300000000 | 0.0379290600000000 | 1.0 |
| C17 | C | 0.9558458900000000 | 0.9478510000000000 | 0.0183044600000000 | 1.0 |
| C18 | C | 0.0807994700000000 | 0.9685583800000000 | 0.9805375500000000 | 1.0 |
| C19 | C | 0.0809209200000000 | 0.0468549100000000 | 0.9929879700000000 | 1.0 |
| C20 | C | 0.9557495300000000 | 0.0542269100000000 | 0.0364324100000000 | 1.0 |
| C21 | C | 0.2058266300000000 | 0.9478655400000000 | 0.0183288000000000 | 1.0 |
| C22 | C | 0.3308274800000000 | 0.9685425100000000 | 0.9806040100000000 | 1.0 |
| C23 | C | 0.3309191400000000 | 0.0468527200000000 | 0.9929801500000000 | 1.0 |
| C24 | C | 0.2057457300000000 | 0.0542458100000000 | 0.0364246700000000 | 1.0 |
| C25 | C | 0.4558221500000000 | 0.9478964500000000 | 0.0184464400000000 | 1.0 |
| C26 | C | 0.5807862800000000 | 0.9685185400000000 | 0.9806588400000000 | 1.0 |
| C27 | C | 0.5809172800000000 | 0.0468373300000000 | 0.9929665500000000 | 1.0 |
| C28 | C | 0.4557488800000000 | 0.0543001600000000 | 0.0363998200000000 | 1.0 |
| C29 | C | 0.7058445300000000 | 0.9478944500000000 | 0.0184414500000000 | 1.0 |
| C30 | C | 0.8307485200000000 | 0.9685401000000000 | 0.9805921700000000 | 1.0 |
| C31 | C | 0.8309216200000000 | 0.0468467400000000 | 0.9929824600000000 | 1.0 |
| C32 | C | 0.7057434800000000 | 0.0542984400000000 | 0.0363970000000000 | 1.0 |
| O33 | O | 0.9559552700000000 | 0.9937784600000000 | 0.0743580700000000 | 1.0 |
| O34 | O | 0.0866953600000000 | 0.0893601300000000 | 0.9359326700000000 | 1.0 |
| O35 | O | 0.2059201300000000 | 0.9938110500000000 | 0.0743697200000000 | 1.0 |
| O36 | O | 0.3366706600000000 | 0.0893011600000000 | 0.9358816700000000 | 1.0 |
| O37 | O | 0.4559228200000000 | 0.9939199300000000 | 0.0744271500000000 | 1.0 |
| O38 | O | 0.5866811200000000 | 0.0892163600000000 | 0.9358149600000000 | 1.0 |
| O39 | O | 0.7059554400000000 | 0.9939167900000000 | 0.0744224400000000 | 1.0 |
| O40 | O | 0.8367386300000000 | 0.0893022500000000 | 0.9358888300000000 | 1.0 |

##### cif ends

furan\_OH\_3\_syn\_dir\_forbid Energy: -251.17472924

##### cif starts

data\_furan\_OH\_3\_syn\_dir\_forbid

\_publ\_section\_comment

;  
Andrew Reynoso, Bohan Xu, and Vincent H. Crespi  
;

\_cell\_length\_a 9.563840576

\_cell\_length\_b 20.0

\_cell\_length\_c 20.0

\_cell\_angle\_alpha 90.0

\_cell\_angle\_beta 90.0

\_cell\_angle\_gamma 90.0

\_symmetry\_space\_group\_name\_H-M 'P 1'

\_symmetry\_Int\_Tables\_number 1

\_symmetry\_cell\_setting triclinic

```

loop_
_atom_site_label
_atom_site_type_symbol
_atom_site_fract_x
_atom_site_fract_y
_atom_site_fract_z
_atom_site_occupancy
H1  H  0.8982570200000000  0.1076137800000000  0.0536065800000000  1.0
H2  H  0.9007436700000000  0.9323812800000000  0.9350053000000000  1.0
H3  H  0.9179749300000000  0.9065937500000000  0.0751174000000000  1.0
H4  H  0.1642909100000000  0.0856870500000000  0.0765811400000000  1.0
H5  H  0.1519946500000000  0.9400028900000000  0.9208791900000000  1.0
H6  H  0.1633219700000000  0.8852218600000000  0.0495155900000000  1.0
H7  H  0.4070355100000000  0.0893622900000000  0.0616972400000000  1.0
H8  H  0.4258911100000000  0.9237843900000000  0.9281743200000000  1.0
H9  H  0.4030040500000000  0.8870798500000000  0.0632898900000000  1.0
H10 H  0.6540537700000000  0.1016693200000000  0.0583851300000000  1.0
H11 H  0.6759483100000000  0.9294407700000000  0.9349707100000000  1.0
H12 H  0.6739393700000000  0.9002110400000000  0.0735239500000000  1.0
H13 H  0.8169456900000000  0.0697104100000000  0.9038314500000000  1.0
H14 H  0.0829731300000000  0.0918256000000000  0.9013458900000000  1.0
H15 H  0.3094977400000000  0.0705871600000000  0.9116284100000000  1.0
H16 H  0.5697930200000000  0.0746560300000000  0.8909736400000000  1.0
C17 C  0.8640017000000000  0.0588434800000000  0.0343940100000000  1.0
C18 C  0.9487929600000000  0.0363316300000000  0.9726643100000000  1.0
C19 C  0.9514007100000000  0.9581471900000000  0.9768678700000000  1.0
C20 C  0.8770650000000000  0.9477786600000000  0.0446230600000000  1.0
C21 C  0.1960993700000000  0.0437585200000000  0.0446868500000000  1.0
C22 C  0.1151414000000000  0.0372535100000000  0.9787583400000000  1.0
C23 C  0.1181949300000000  0.9584252300000000  0.9699541000000000  1.0
C24 C  0.2024644800000000  0.9335077400000000  0.0311169700000000  1.0
C25 C  0.3668194200000000  0.0438270500000000  0.0378902200000000  1.0
C26 C  0.4486053600000000  0.0264955400000000  0.9717000800000000  1.0
C27 C  0.4600533000000000  0.9484395400000000  0.9743909200000000  1.0
C28 C  0.3722362400000000  0.9324442400000000  0.0360400500000000  1.0
C29 C  0.6947430300000000  0.0550714400000000  0.0368479600000000  1.0
C30 C  0.6166340900000000  0.0320540500000000  0.9738483500000000  1.0
C31 C  0.6266882200000000  0.9536091200000000  0.9781763500000000  1.0
C32 C  0.7068141400000000  0.9441798700000000  0.0446544800000000  1.0
O33 O  0.9067959200000000  0.0087802000000000  0.0807381600000000  1.0
O34 O  0.9210421700000000  0.0655421200000000  0.9098953700000000  1.0
O35 O  0.1652808200000000  0.9833726500000000  0.0795541100000000  1.0
O36 O  0.1652630400000000  0.0841928300000000  0.9311251600000000  1.0
O37 O  0.4048426500000000  0.9882033000000000  0.0787278000000000  1.0
O38 O  0.4097805100000000  0.0542448400000000  0.9098715900000000  1.0
O39 O  0.6667972400000000  0.0022727100000000  0.0825877800000000  1.0
O40 O  0.6594431800000000  0.0664090100000000  0.9155184500000000  1.0

```

##### cif ends

thiophene\_CF3\_24\_anti\_alt Energy: -348.47878378

##### cif starts

data\_thiophene\_CF3\_24\_anti\_alt

\_publ\_section\_comment  
;  
Andrew Reynoso, Bohan Xu, and Vincent H. Crespi  
;

\_cell\_length\_a 10.7508855096  
\_cell\_length\_b 20.0  
\_cell\_length\_c 20.0  
\_cell\_angle\_alpha 90.0  
\_cell\_angle\_beta 90.0  
\_cell\_angle\_gamma 90.0

\_symmetry\_space\_group\_name\_H-M 'P 1'  
\_symmetry\_Int\_Tables\_number 1  
\_symmetry\_cell\_setting triclinic

loop\_

\_atom\_site\_label  
\_atom\_site\_type\_symbol  
\_atom\_site\_fract\_x  
\_atom\_site\_fract\_y  
\_atom\_site\_fract\_z  
\_atom\_site\_occupancy

|     |   |                    |                    |                    |     |
|-----|---|--------------------|--------------------|--------------------|-----|
| H1  | H | 0.0130284200000000 | 0.9362231800000000 | 0.0617722400000000 | 1.0 |
| H2  | H | 0.1169114500000000 | 0.0983551800000000 | 0.9310699000000000 | 1.0 |
| H3  | H | 0.4207334900000000 | 0.0586475400000000 | 0.9140018300000000 | 1.0 |
| H4  | H | 0.3040888700000000 | 0.9027825300000000 | 0.0476835500000000 | 1.0 |
| H5  | H | 0.5045545700000000 | 0.9410808200000000 | 0.0614867500000000 | 1.0 |
| H6  | H | 0.6198281700000000 | 0.1001408000000000 | 0.9310384400000000 | 1.0 |
| H7  | H | 0.9200887100000000 | 0.0478122700000000 | 0.9094412200000000 | 1.0 |
| H8  | H | 0.7956306700000000 | 0.8999614900000000 | 0.0508678800000000 | 1.0 |
| C9  | C | 0.1503774900000000 | 0.9284379100000000 | 0.9780216800000000 | 1.0 |
| C10 | C | 0.0255993300000000 | 0.9556762400000000 | 0.0110788400000000 | 1.0 |
| C11 | C | 0.0266782100000000 | 0.0346373000000000 | 0.0073665800000000 | 1.0 |
| C12 | C | 0.1445322600000000 | 0.0555241900000000 | 0.9616531800000000 | 1.0 |
| C13 | C | 0.1489167100000000 | 0.8480204300000000 | 0.9754024300000000 | 1.0 |
| C14 | C | 0.0218048800000000 | 0.0712571500000000 | 0.0796572800000000 | 1.0 |
| C15 | C | 0.2791209900000000 | 0.0703254200000000 | 0.9950252100000000 | 1.0 |
| C16 | C | 0.4013149100000000 | 0.0389400500000000 | 0.9640012000000000 | 1.0 |
| C17 | C | 0.3967157100000000 | 0.9606179200000000 | 0.9664137800000000 | 1.0 |
| C18 | C | 0.2800011700000000 | 0.9442392700000000 | 0.0143633500000000 | 1.0 |
| C19 | C | 0.3034635500000000 | 0.1492211000000000 | 0.9905444900000000 | 1.0 |
| C20 | C | 0.3982999800000000 | 0.9269615900000000 | 0.8927964100000000 | 1.0 |
| C21 | C | 0.6449377400000000 | 0.9296066200000000 | 0.9804038800000000 | 1.0 |
| C22 | C | 0.5237117500000000 | 0.9609260300000000 | 0.0114633600000000 | 1.0 |
| C23 | C | 0.5288818000000000 | 0.0394118800000000 | 0.0093494600000000 | 1.0 |
| C24 | C | 0.6449030500000000 | 0.0568651200000000 | 0.9617534800000000 | 1.0 |
| C25 | C | 0.6204879300000000 | 0.8501754800000000 | 0.9809544300000000 | 1.0 |
| C26 | C | 0.5280581100000000 | 0.0747987300000000 | 0.0813500600000000 | 1.0 |
| C27 | C | 0.7822602200000000 | 0.0669085400000000 | 0.9921085000000000 | 1.0 |
| C28 | C | 0.9002621100000000 | 0.0311312600000000 | 0.9605922900000000 | 1.0 |
| C29 | C | 0.8934693000000000 | 0.9529107900000000 | 0.9689704900000000 | 1.0 |
| C30 | C | 0.7763027000000000 | 0.9414008700000000 | 0.0167197800000000 | 1.0 |
| C31 | C | 0.8131134100000000 | 0.1440513400000000 | 0.9824285900000000 | 1.0 |
| C32 | C | 0.8904374400000000 | 0.8998857100000000 | 0.9099402000000000 | 1.0 |

|     |   |                    |                    |                    |     |
|-----|---|--------------------|--------------------|--------------------|-----|
| F33 | F | 0.2614276500000000 | 0.8203106500000000 | 0.9914344800000000 | 1.0 |
| F34 | F | 0.0288809300000000 | 0.0269061300000000 | 0.1312889800000000 | 1.0 |
| F35 | F | 0.0712901400000000 | 0.8266277200000000 | 0.0256873000000000 | 1.0 |
| F36 | F | 0.1155111900000000 | 0.8174031800000000 | 0.9184225300000000 | 1.0 |
| F37 | F | 0.1168049200000000 | 0.1155228200000000 | 0.0873314900000000 | 1.0 |
| F38 | F | 0.9213078200000000 | 0.1110510200000000 | 0.0948891700000000 | 1.0 |
| F39 | F | 0.4269653600000000 | 0.1640601700000000 | 0.9806079900000000 | 1.0 |
| F40 | F | 0.3960950800000000 | 0.9735285300000000 | 0.8428807900000000 | 1.0 |
| F41 | F | 0.2475565000000000 | 0.1719819200000000 | 0.9327962300000000 | 1.0 |
| F42 | F | 0.2639956800000000 | 0.1893040800000000 | 0.0399477100000000 | 1.0 |
| F43 | F | 0.4979434100000000 | 0.8873637900000000 | 0.8782543300000000 | 1.0 |
| F44 | F | 0.3014271200000000 | 0.8844222300000000 | 0.8805479000000000 | 1.0 |
| F45 | F | 0.6799338300000000 | 0.8230011400000000 | 0.0356621700000000 | 1.0 |
| F46 | F | 0.5329127700000000 | 0.0298051300000000 | 0.1326452400000000 | 1.0 |
| F47 | F | 0.4981214100000000 | 0.8355984600000000 | 0.9925670300000000 | 1.0 |
| F48 | F | 0.6560637200000000 | 0.8136668300000000 | 0.9280311300000000 | 1.0 |
| F49 | F | 0.6247128500000000 | 0.1179917200000000 | 0.0898822600000000 | 1.0 |
| F50 | F | 0.4278522200000000 | 0.1144716900000000 | 0.0957987400000000 | 1.0 |
| F51 | F | 0.9372008100000000 | 0.1594494500000000 | 0.9823978600000000 | 1.0 |
| F52 | F | 0.9862402000000000 | 0.9021521000000000 | 0.8660627100000000 | 1.0 |
| F53 | F | 0.7769449700000000 | 0.1593796500000000 | 0.9177138300000000 | 1.0 |
| F54 | F | 0.7566016500000000 | 0.1884241100000000 | 0.0224863900000000 | 1.0 |
| F55 | F | 0.8916508800000000 | 0.8390744400000000 | 0.9412142700000000 | 1.0 |
| F56 | F | 0.7909780200000000 | 0.8969441300000000 | 0.8675691000000000 | 1.0 |
| S57 | S | 0.1538753500000000 | 0.9866941500000000 | 0.9042734600000000 | 1.0 |
| S58 | S | 0.2736738400000000 | 0.0149789900000000 | 0.0700829100000000 | 1.0 |
| S59 | S | 0.6513195500000000 | 0.9874219800000000 | 0.9051239500000000 | 1.0 |
| S60 | S | 0.7746836300000000 | 0.0140256400000000 | 0.0694367700000000 | 1.0 |

##### cif ends

thiophene\_CF3\_24\_anti\_dir    Energy: -351.89582864

##### cif starts

data\_thiophene\_CF3\_24\_anti\_dir

\_publ\_section\_comment

;  
Andrew Reynoso, Bohan Xu, and Vincent H. Crespi  
;

\_cell\_length\_a    10.1527634121

\_cell\_length\_b    20.0

\_cell\_length\_c    20.0

\_cell\_angle\_alpha    90.0

\_cell\_angle\_beta    90.0

\_cell\_angle\_gamma    90.0

\_symmetry\_space\_group\_name\_H-M    'P 1'

\_symmetry\_Int\_Tables\_number 1

\_symmetry\_cell\_setting triclinic

loop\_

\_atom\_site\_label

\_atom\_site\_type\_symbol

\_atom\_site\_fract\_x

|     |   | _atom_site_fract_y |                    |                      |     |
|-----|---|--------------------|--------------------|----------------------|-----|
|     |   |                    | _atom_site_fract_z |                      |     |
|     |   |                    |                    | _atom_site_occupancy |     |
| H1  | H | 0.0710814600000000 | 0.0953340100000000 | 0.9128373500000000   | 1.0 |
| H2  | H | 0.0293707500000000 | 0.9873343200000000 | 0.0890718600000000   | 1.0 |
| H3  | H | 0.3210735200000000 | 0.1280192000000000 | 0.9832288200000000   | 1.0 |
| H4  | H | 0.2793324000000000 | 0.9236826800000000 | 0.9521136700000000   | 1.0 |
| H5  | H | 0.5710421200000000 | 0.0953002300000000 | 0.9128500100000000   | 1.0 |
| H6  | H | 0.5293050700000000 | 0.9873217400000000 | 0.0891128800000000   | 1.0 |
| H7  | H | 0.8210555300000000 | 0.1280250800000000 | 0.9832003100000000   | 1.0 |
| H8  | H | 0.7793292400000000 | 0.9236784700000000 | 0.9521439700000000   | 1.0 |
| C9  | C | 0.9887958100000000 | 0.0592634700000000 | 0.0071603200000000   | 1.0 |
| C10 | C | 0.9889811800000000 | 0.9864236800000000 | 0.0384776900000000   | 1.0 |
| C11 | C | 0.0827455600000000 | 0.9428935300000000 | 0.9908297900000000   | 1.0 |
| C12 | C | 0.0628978700000000 | 0.8662039600000000 | 0.9914284700000000   | 1.0 |
| C13 | C | 0.0245012900000000 | 0.1228437000000000 | 0.0542842300000000   | 1.0 |
| C14 | C | 0.0847139600000000 | 0.0532774100000000 | 0.9464903300000000   | 1.0 |
| C15 | C | 0.3347188500000000 | 0.0751799100000000 | 0.9936701400000000   | 1.0 |
| C16 | C | 0.2388025900000000 | 0.0326756300000000 | 0.9499658100000000   | 1.0 |
| C17 | C | 0.2389640900000000 | 0.9617672700000000 | 0.9854391500000000   | 1.0 |
| C18 | C | 0.3327420900000000 | 0.9701013400000000 | 0.0494414800000000   | 1.0 |
| C19 | C | 0.3129050500000000 | 0.9201775400000000 | 0.1076681900000000   | 1.0 |
| C20 | C | 0.2745260100000000 | 0.0375979300000000 | 0.8709891700000000   | 1.0 |
| C21 | C | 0.5846965300000000 | 0.0532528100000000 | 0.9465108000000000   | 1.0 |
| C22 | C | 0.4887902100000000 | 0.0592481700000000 | 0.0071860300000000   | 1.0 |
| C23 | C | 0.4889677800000000 | 0.9864107100000000 | 0.0385075100000000   | 1.0 |
| C24 | C | 0.5827649000000000 | 0.9428815600000000 | 0.9908767800000000   | 1.0 |
| C25 | C | 0.5629632700000000 | 0.8661903600000000 | 0.9915320700000000   | 1.0 |
| C26 | C | 0.5244955500000000 | 0.1228269500000000 | 0.0543106300000000   | 1.0 |
| C27 | C | 0.8347134200000000 | 0.0751877400000000 | 0.9936532200000000   | 1.0 |
| C28 | C | 0.7387866600000000 | 0.0326641800000000 | 0.9499731300000000   | 1.0 |
| C29 | C | 0.7389704800000000 | 0.9617682700000000 | 0.9854651500000000   | 1.0 |
| C30 | C | 0.8327732500000000 | 0.9701232800000000 | 0.0494490300000000   | 1.0 |
| C31 | C | 0.8129847100000000 | 0.9202191200000000 | 0.1076945900000000   | 1.0 |
| C32 | C | 0.7744751700000000 | 0.0375674100000000 | 0.8709918000000000   | 1.0 |
| F33 | F | 0.9298664700000000 | 0.1719710300000000 | 0.0557063400000000   | 1.0 |
| F34 | F | 0.9424230400000000 | 0.8486290600000000 | 0.9661478800000000   | 1.0 |
| F35 | F | 0.1532967600000000 | 0.8345992700000000 | 0.9520472900000000   | 1.0 |
| F36 | F | 0.0718814100000000 | 0.8392505300000000 | 0.0532610200000000   | 1.0 |
| F37 | F | 0.0472834700000000 | 0.1086103500000000 | 0.1194436500000000   | 1.0 |
| F38 | F | 0.1315098400000000 | 0.1567559700000000 | 0.0293492700000000   | 1.0 |
| F39 | F | 0.2972056000000000 | 0.9785679100000000 | 0.8399187300000000   | 1.0 |
| F40 | F | 0.4032263900000000 | 0.9299198200000000 | 0.1572442000000000   | 1.0 |
| F41 | F | 0.1923925400000000 | 0.9281346300000000 | 0.1373570900000000   | 1.0 |
| F42 | F | 0.3219731100000000 | 0.8555326000000000 | 0.0883977400000000   | 1.0 |
| F43 | F | 0.8815305300000000 | 0.0784431900000000 | 0.8610735500000000   | 1.0 |
| F44 | F | 0.6798736900000000 | 0.0681526800000000 | 0.8325044100000000   | 1.0 |
| F45 | F | 0.4298531700000000 | 0.1719491300000000 | 0.0557484300000000   | 1.0 |
| F46 | F | 0.4425323300000000 | 0.8485765500000000 | 0.9662269900000000   | 1.0 |
| F47 | F | 0.6534316200000000 | 0.8345553000000000 | 0.9522196300000000   | 1.0 |
| F48 | F | 0.5718825100000000 | 0.8393033200000000 | 0.0533963900000000   | 1.0 |
| F49 | F | 0.5472992400000000 | 0.1085873700000000 | 0.1194670100000000   | 1.0 |
| F50 | F | 0.6314858100000000 | 0.1567464500000000 | 0.0293659100000000   | 1.0 |
| F51 | F | 0.7971530900000000 | 0.9785311900000000 | 0.8399335900000000   | 1.0 |
| F52 | F | 0.8220665600000000 | 0.8555716800000000 | 0.0884400600000000   | 1.0 |

|     |   |                    |                    |                    |     |
|-----|---|--------------------|--------------------|--------------------|-----|
| F53 | F | 0.9033362200000000 | 0.9299836900000000 | 0.1572529800000000 | 1.0 |
| F54 | F | 0.6924914400000000 | 0.9281748600000000 | 0.1374034100000000 | 1.0 |
| F55 | F | 0.1799543500000000 | 0.0682013800000000 | 0.8324985300000000 | 1.0 |
| F56 | F | 0.3815985300000000 | 0.0784644100000000 | 0.8610954400000000 | 1.0 |
| S57 | S | 0.5303201000000000 | 0.9739536900000000 | 0.9097574400000000 | 1.0 |
| S58 | S | 0.2803261600000000 | 0.0521550800000000 | 0.0779808300000000 | 1.0 |
| S59 | S | 0.0303368600000000 | 0.9739959900000000 | 0.9097150800000000 | 1.0 |
| S60 | S | 0.7803575700000000 | 0.0521805300000000 | 0.0779732900000000 | 1.0 |

##### cif ends

thiophene\_CF3\_24\_anti\_dir\_forbid    Energy: -352.65923848

##### cif starts

data\_thiophene\_CF3\_24\_anti\_dir\_forbid

\_publ\_section\_comment

;  
Andrew Reynoso, Bohan Xu, and Vincent H. Crespi  
;

\_cell\_length\_a    10.6553936354

\_cell\_length\_b    20.0

\_cell\_length\_c    20.0

\_cell\_angle\_alpha    90.0

\_cell\_angle\_beta    90.0

\_cell\_angle\_gamma    90.0

\_symmetry\_space\_group\_name\_H-M    'P 1'

\_symmetry\_Int\_Tables\_number 1

\_symmetry\_cell\_setting triclinic

loop\_

\_atom\_site\_label

\_atom\_site\_type\_symbol

\_atom\_site\_fract\_x

\_atom\_site\_fract\_y

\_atom\_site\_fract\_z

\_atom\_site\_occupancy

|     |   |                    |                    |                    |     |
|-----|---|--------------------|--------------------|--------------------|-----|
| H1  | H | 0.4417714900000000 | 0.0481641900000000 | 0.0699013300000000 | 1.0 |
| H2  | H | 0.5570726600000000 | 0.8830916500000000 | 0.9478074100000000 | 1.0 |
| H3  | H | 0.8193683800000000 | 0.0548960800000000 | 0.9319325400000000 | 1.0 |
| H4  | H | 0.7082672200000000 | 0.8764102100000000 | 0.0317579000000000 | 1.0 |
| H5  | H | 0.9518952700000000 | 0.0522543400000000 | 0.0663908300000000 | 1.0 |
| H6  | H | 0.0621492300000000 | 0.8767290100000000 | 0.9616276400000000 | 1.0 |
| H7  | H | 0.3267588300000000 | 0.0470212900000000 | 0.9289503200000000 | 1.0 |
| H8  | H | 0.2076411200000000 | 0.8804069300000000 | 0.0475584000000000 | 1.0 |
| C9  | C | 0.5690143000000000 | 0.0557034200000000 | 0.9811308000000000 | 1.0 |
| C10 | C | 0.4494915400000000 | 0.0268779500000000 | 0.0198744800000000 | 1.0 |
| C11 | C | 0.4534683200000000 | 0.9472354400000000 | 0.0195947700000000 | 1.0 |
| C12 | C | 0.5701275100000000 | 0.9300401500000000 | 0.9741802900000000 | 1.0 |
| C13 | C | 0.5492087500000000 | 0.1247830700000000 | 0.9465810900000000 | 1.0 |
| C14 | C | 0.4535444500000000 | 0.9057239900000000 | 0.0879769900000000 | 1.0 |
| C15 | C | 0.7017345600000000 | 0.0525604600000000 | 0.0238415400000000 | 1.0 |
| C16 | C | 0.8197084900000000 | 0.0296907200000000 | 0.9802640400000000 | 1.0 |
| C17 | C | 0.8182563300000000 | 0.9501732100000000 | 0.9754622600000000 | 1.0 |

|     |   |                    |                    |                    |     |
|-----|---|--------------------|--------------------|--------------------|-----|
| C18 | C | 0.6970487100000000 | 0.9269631300000000 | 0.0131996700000000 | 1.0 |
| C19 | C | 0.7231061900000000 | 0.1158310400000000 | 0.0678369400000000 | 1.0 |
| C20 | C | 0.8242931500000000 | 0.9155566700000000 | 0.9035971600000000 | 1.0 |
| C21 | C | 0.0701390400000000 | 0.0521966900000000 | 0.9749954800000000 | 1.0 |
| C22 | C | 0.9512280100000000 | 0.0286267400000000 | 0.0172820700000000 | 1.0 |
| C23 | C | 0.9511731300000000 | 0.9490095300000000 | 0.0196248600000000 | 1.0 |
| C24 | C | 0.0730721800000000 | 0.9267477400000000 | 0.9817716100000000 | 1.0 |
| C25 | C | 0.0502605900000000 | 0.1168458800000000 | 0.9327736200000000 | 1.0 |
| C26 | C | 0.9441152300000000 | 0.9119356300000000 | 0.0906173500000000 | 1.0 |
| C27 | C | 0.2016919700000000 | 0.0536983600000000 | 0.0187756000000000 | 1.0 |
| C28 | C | 0.3207919900000000 | 0.0258753700000000 | 0.9791087800000000 | 1.0 |
| C29 | C | 0.3176322000000000 | 0.9457479800000000 | 0.9811249500000000 | 1.0 |
| C30 | C | 0.1976375200000000 | 0.9282663800000000 | 0.0230461000000000 | 1.0 |
| C31 | C | 0.2207083900000000 | 0.1217673800000000 | 0.0554892600000000 | 1.0 |
| C32 | C | 0.3246437500000000 | 0.8949449800000000 | 0.9202873300000000 | 1.0 |
| F33 | F | 0.5168183500000000 | 0.1743357700000000 | 0.9892241700000000 | 1.0 |
| F34 | F | 0.4325863400000000 | 0.9440419000000000 | 0.1426143700000000 | 1.0 |
| F35 | F | 0.6566687400000000 | 0.1436553900000000 | 0.9143052200000000 | 1.0 |
| F36 | F | 0.4581146100000000 | 0.1231240800000000 | 0.8984444100000000 | 1.0 |
| F37 | F | 0.3646306900000000 | 0.8561305700000000 | 0.0881396100000000 | 1.0 |
| F38 | F | 0.5603459700000000 | 0.8695349100000000 | 0.1013064700000000 | 1.0 |
| F39 | F | 0.7622578700000000 | 0.1696883300000000 | 0.0325339100000000 | 1.0 |
| F40 | F | 0.8345935000000000 | 0.9590510300000000 | 0.8521582300000000 | 1.0 |
| F41 | F | 0.6152761700000000 | 0.1325000100000000 | 0.1007401900000000 | 1.0 |
| F42 | F | 0.8106094300000000 | 0.1057552700000000 | 0.1169440200000000 | 1.0 |
| F43 | F | 0.9195059300000000 | 0.8699257500000000 | 0.8971646200000000 | 1.0 |
| F44 | F | 0.7208920000000000 | 0.8767059200000000 | 0.8897712900000000 | 1.0 |
| F45 | F | 0.0104558800000000 | 0.1697731900000000 | 0.9692380900000000 | 1.0 |
| F46 | F | 0.9351947000000000 | 0.9537981400000000 | 0.1434770400000000 | 1.0 |
| F47 | F | 0.1589599800000000 | 0.1343279300000000 | 0.9011241600000000 | 1.0 |
| F48 | F | 0.9639249500000000 | 0.1082243200000000 | 0.8828276700000000 | 1.0 |
| F49 | F | 0.8478126200000000 | 0.8668192900000000 | 0.0958228500000000 | 1.0 |
| F50 | F | 0.0460999900000000 | 0.8716928800000000 | 0.1033256600000000 | 1.0 |
| F51 | F | 0.2564878400000000 | 0.1721645700000000 | 0.0146545500000000 | 1.0 |
| F52 | F | 0.3918669800000000 | 0.9153895700000000 | 0.8666290500000000 | 1.0 |
| F53 | F | 0.1118133400000000 | 0.1403700100000000 | 0.0864779700000000 | 1.0 |
| F54 | F | 0.3086680000000000 | 0.1184560900000000 | 0.1052026500000000 | 1.0 |
| F55 | F | 0.3796531700000000 | 0.8373254300000000 | 0.9446861700000000 | 1.0 |
| F56 | F | 0.2148761600000000 | 0.8719056900000000 | 0.8933725500000000 | 1.0 |
| S57 | S | 0.5796701800000000 | 0.9966265600000000 | 0.9124113500000000 | 1.0 |
| S58 | S | 0.6882868000000000 | 0.9843963000000000 | 0.0835913300000000 | 1.0 |
| S59 | S | 0.0855582000000000 | 0.9858821700000000 | 0.9130452200000000 | 1.0 |
| S60 | S | 0.1886741300000000 | 0.9926233300000000 | 0.0864037800000000 | 1.0 |

##### cif ends

thiophene\_CF3\_24\_syn\_alt Energy: -351.79934301

##### cif starts

data\_thiophene\_CF3\_24\_syn\_alt

\_publ\_section\_comment

;  
Andrew Reynoso, Bohan Xu, and Vincent H. Crespi

;



\_cell\_length\_a 10.9682630415  
\_cell\_length\_b 20.0  
\_cell\_length\_c 20.0  
\_cell\_angle\_alpha 90.0  
\_cell\_angle\_beta 90.0  
\_cell\_angle\_gamma 90.0

\_symmetry\_space\_group\_name\_H-M 'P 1'  
\_symmetry\_Int\_Tables\_number 1  
\_symmetry\_cell\_setting triclinic

loop\_  
\_atom\_site\_label  
\_atom\_site\_type\_symbol  
\_atom\_site\_fract\_x  
\_atom\_site\_fract\_y  
\_atom\_site\_fract\_z  
\_atom\_site\_occupancy

|     |   |                    |                    |                    |     |
|-----|---|--------------------|--------------------|--------------------|-----|
| H1  | H | 0.0664552300000000 | 0.9399733200000000 | 0.9347104400000000 | 1.0 |
| H2  | H | 0.9462590600000000 | 0.1157960200000000 | 0.0265635600000000 | 1.0 |
| H3  | H | 0.3165338800000000 | 0.0589485800000000 | 0.9316278600000000 | 1.0 |
| H4  | H | 0.1963596600000000 | 0.8880750700000000 | 0.0324168300000000 | 1.0 |
| H5  | H | 0.5664681300000000 | 0.9399249900000000 | 0.9347870500000000 | 1.0 |
| H6  | H | 0.4464189600000000 | 0.1158398100000000 | 0.0265289600000000 | 1.0 |
| H7  | H | 0.8164034900000000 | 0.0588455200000000 | 0.9316930200000000 | 1.0 |
| H8  | H | 0.6963169800000000 | 0.8879584300000000 | 0.0324689500000000 | 1.0 |
| C9  | C | 0.9554732600000000 | 0.9453072000000000 | 0.0279687800000000 | 1.0 |
| C10 | C | 0.0725491100000000 | 0.9631009000000000 | 0.9838832500000000 | 1.0 |
| C11 | C | 0.0730718000000000 | 0.0413400200000000 | 0.9808290900000000 | 1.0 |
| C12 | C | 0.9489121600000000 | 0.0624575400000000 | 0.0158760900000000 | 1.0 |
| C13 | C | 0.9646095500000000 | 0.8763339500000000 | 0.0632101000000000 | 1.0 |
| C14 | C | 0.0851039400000000 | 0.0741214300000000 | 0.9106168100000000 | 1.0 |
| C15 | C | 0.2054241900000000 | 0.0584192400000000 | 0.0249785900000000 | 1.0 |
| C16 | C | 0.3225714200000000 | 0.0383957600000000 | 0.9819353900000000 | 1.0 |
| C17 | C | 0.3231155800000000 | 0.9601085800000000 | 0.9829426600000000 | 1.0 |
| C18 | C | 0.1989464100000000 | 0.9407916200000000 | 0.0189816500000000 | 1.0 |
| C19 | C | 0.2144847000000000 | 0.1291655400000000 | 0.0565252500000000 | 1.0 |
| C20 | C | 0.3352739800000000 | 0.9238217400000000 | 0.9144912900000000 | 1.0 |
| C21 | C | 0.4554198600000000 | 0.9453444000000000 | 0.0279919900000000 | 1.0 |
| C22 | C | 0.5725657600000000 | 0.9630521000000000 | 0.9839565600000000 | 1.0 |
| C23 | C | 0.5731817800000000 | 0.0412973700000000 | 0.9808933400000000 | 1.0 |
| C24 | C | 0.4489822600000000 | 0.0624939300000000 | 0.0158642000000000 | 1.0 |
| C25 | C | 0.4643557300000000 | 0.8763793300000000 | 0.0632575600000000 | 1.0 |
| C26 | C | 0.5853757200000000 | 0.0740113500000000 | 0.9106466700000000 | 1.0 |
| C27 | C | 0.7054296300000000 | 0.0583119000000000 | 0.0250857600000000 | 1.0 |
| C28 | C | 0.8225286900000000 | 0.0383052000000000 | 0.9819993700000000 | 1.0 |
| C29 | C | 0.8231199700000000 | 0.9600109800000000 | 0.9830017700000000 | 1.0 |
| C30 | C | 0.6989425700000000 | 0.9406855000000000 | 0.0190606100000000 | 1.0 |
| C31 | C | 0.7145130900000000 | 0.1290105400000000 | 0.0567336000000000 | 1.0 |
| C32 | C | 0.8352230500000000 | 0.9236933400000000 | 0.9145557600000000 | 1.0 |
| F33 | F | 0.8549094900000000 | 0.8513543500000000 | 0.0831692200000000 | 1.0 |
| F34 | F | 0.1528049200000000 | 0.0374638400000000 | 0.8666550000000000 | 1.0 |
| F35 | F | 0.0178715500000000 | 0.8283748500000000 | 0.0246985600000000 | 1.0 |
| F36 | F | 0.0335404900000000 | 0.8806201200000000 | 0.1203182000000000 | 1.0 |
| F37 | F | 0.9763745400000000 | 0.0856504100000000 | 0.8796114000000000 | 1.0 |

|     |   |                    |                    |                    |     |
|-----|---|--------------------|--------------------|--------------------|-----|
| F38 | F | 0.1391120300000000 | 0.1356232700000000 | 0.9151938300000000 | 1.0 |
| F39 | F | 0.2828891900000000 | 0.1278343600000000 | 0.1139623800000000 | 1.0 |
| F40 | F | 0.4031807400000000 | 0.9582175900000000 | 0.8688161200000000 | 1.0 |
| F41 | F | 0.2682772200000000 | 0.1749543000000000 | 0.0156594000000000 | 1.0 |
| F42 | F | 0.1047336600000000 | 0.1553221100000000 | 0.0748099500000000 | 1.0 |
| F43 | F | 0.3891221200000000 | 0.8625944900000000 | 0.9221800400000000 | 1.0 |
| F44 | F | 0.2266031400000000 | 0.9108320200000000 | 0.8840048800000000 | 1.0 |
| F45 | F | 0.6526336100000000 | 0.0371225100000000 | 0.8666751400000000 | 1.0 |
| F46 | F | 0.5173466500000000 | 0.8283409600000000 | 0.0247362900000000 | 1.0 |
| F47 | F | 0.5334085500000000 | 0.8806087900000000 | 0.1203264300000000 | 1.0 |
| F48 | F | 0.4766705900000000 | 0.0858198200000000 | 0.8797213300000000 | 1.0 |
| F49 | F | 0.6399590400000000 | 0.1353682000000000 | 0.9151190000000000 | 1.0 |
| F50 | F | 0.7832111200000000 | 0.1276291700000000 | 0.1140652700000000 | 1.0 |
| F51 | F | 0.9027155400000000 | 0.9581749200000000 | 0.8687687300000000 | 1.0 |
| F52 | F | 0.7679769200000000 | 0.1749091600000000 | 0.0158651200000000 | 1.0 |
| F53 | F | 0.6047859000000000 | 0.1550437900000000 | 0.0752457200000000 | 1.0 |
| F54 | F | 0.8894869800000000 | 0.8625703100000000 | 0.9222215400000000 | 1.0 |
| F55 | F | 0.7265066000000000 | 0.9104548400000000 | 0.8842283700000000 | 1.0 |
| F56 | F | 0.3546007000000000 | 0.8515369200000000 | 0.0832977800000000 | 1.0 |
| S57 | S | 0.9584490100000000 | 0.0130199300000000 | 0.0899089100000000 | 1.0 |
| S58 | S | 0.2084486600000000 | 0.9940098400000000 | 0.0903510200000000 | 1.0 |
| S59 | S | 0.4584278700000000 | 0.0130811800000000 | 0.0899122300000000 | 1.0 |
| S60 | S | 0.7084250900000000 | 0.9938660800000000 | 0.0904473200000000 | 1.0 |

##### cif ends

thiophene\_CF3\_24\_syn\_dir\_break Energy: -350.99988001

##### cif starts

data\_thiophene\_CF3\_24\_syn\_dir\_break

\_publ\_section\_comment

;

Andrew Reynoso, Bohan Xu, and Vincent H. Crespi

;

\_cell\_length\_a 14.6999464474

\_cell\_length\_b 20.0

\_cell\_length\_c 20.0

\_cell\_angle\_alpha 90.0

\_cell\_angle\_beta 90.0

\_cell\_angle\_gamma 90.0

\_symmetry\_space\_group\_name\_H-M 'P 1'

\_symmetry\_Int\_Tables\_number 1

\_symmetry\_cell\_setting triclinic

loop\_

\_atom\_site\_label

\_atom\_site\_type\_symbol

\_atom\_site\_fract\_x

\_atom\_site\_fract\_y

\_atom\_site\_fract\_z

\_atom\_site\_occupancy

|    |   |                    |                    |                    |     |
|----|---|--------------------|--------------------|--------------------|-----|
| H1 | H | 0.1696330700000000 | 0.0044933900000000 | 0.9244043900000000 | 1.0 |
| H2 | H | 0.0801641300000000 | 0.8771858600000000 | 0.0896771300000000 | 1.0 |

|     |   |                    |                    |                    |     |
|-----|---|--------------------|--------------------|--------------------|-----|
| H3  | H | 0.3230913700000000 | 0.0695625700000000 | 0.9577182700000000 | 1.0 |
| H4  | H | 0.2831172900000000 | 0.8809613000000000 | 0.0575206400000000 | 1.0 |
| H5  | H | 0.4670352800000000 | 0.0830761500000000 | 0.9509866100000000 | 1.0 |
| H6  | H | 0.4465334200000000 | 0.8933118200000000 | 0.0235798800000000 | 1.0 |
| H7  | H | 0.9480993300000000 | 0.9446129500000000 | 0.9081840400000000 | 1.0 |
| H8  | H | 0.6235477300000000 | 0.9299007900000000 | 0.0606438000000000 | 1.0 |
| C9  | C | 0.0392560800000000 | 0.0055816600000000 | 0.9795113500000000 | 1.0 |
| C10 | C | 0.1468157800000000 | 0.9964085700000000 | 0.9757558700000000 | 1.0 |
| C11 | C | 0.1622462700000000 | 0.9222584100000000 | 0.0010278700000000 | 1.0 |
| C12 | C | 0.0696005900000000 | 0.9106570800000000 | 0.0470139500000000 | 1.0 |
| C13 | C | 0.9946243100000000 | 0.0680813900000000 | 0.9462714700000000 | 1.0 |
| C14 | C | 0.1645298600000000 | 0.8584526800000000 | 0.9540019900000000 | 1.0 |
| C15 | C | 0.2127629000000000 | 0.0408232900000000 | 0.0281091600000000 | 1.0 |
| C16 | C | 0.3169489900000000 | 0.0402650900000000 | 0.0037799100000000 | 1.0 |
| C17 | C | 0.3354831000000000 | 0.9641188400000000 | 0.9904092400000000 | 1.0 |
| C18 | C | 0.2570859800000000 | 0.9278531300000000 | 0.0363950000000000 | 1.0 |
| C19 | C | 0.1804960900000000 | 0.1133532500000000 | 0.0439090300000000 | 1.0 |
| C20 | C | 0.3396386500000000 | 0.9509546700000000 | 0.9130672200000000 | 1.0 |
| C21 | C | 0.4062915300000000 | 0.0606783400000000 | 0.0505295300000000 | 1.0 |
| C22 | C | 0.4917846200000000 | 0.0623822200000000 | 0.9986918000000000 | 1.0 |
| C23 | C | 0.5192576900000000 | 0.9864538100000000 | 0.9924697700000000 | 1.0 |
| C24 | C | 0.4333569500000000 | 0.9471444700000000 | 0.0196844200000000 | 1.0 |
| C25 | C | 0.4059395000000000 | 0.1213925000000000 | 0.0991385900000000 | 1.0 |
| C26 | C | 0.5706106900000000 | 0.9641995100000000 | 0.9259430500000000 | 1.0 |
| C27 | C | 0.5777513000000000 | 0.0992279300000000 | 0.0205743600000000 | 1.0 |
| C28 | C | 0.9886996600000000 | 0.9440365200000000 | 0.9533397000000000 | 1.0 |
| C29 | C | 0.9957916300000000 | 0.8929360800000000 | 0.9964636700000000 | 1.0 |
| C30 | C | 0.5955921000000000 | 0.9776147100000000 | 0.0441270400000000 | 1.0 |
| C31 | C | 0.6123690700000000 | 0.1635895800000000 | 0.9957667500000000 | 1.0 |
| C32 | C | 0.9325189000000000 | 0.8337917000000000 | 0.9943354700000000 | 1.0 |
| F33 | F | 0.0562224600000000 | 0.1143873100000000 | 0.9254813100000000 | 1.0 |
| F34 | F | 0.1252370100000000 | 0.8645321100000000 | 0.8929647600000000 | 1.0 |
| F35 | F | 0.9477723300000000 | 0.0510751800000000 | 0.8894152800000000 | 1.0 |
| F36 | F | 0.9329261400000000 | 0.0977085200000000 | 0.9873195000000000 | 1.0 |
| F37 | F | 0.2508016500000000 | 0.8351725300000000 | 0.9441177000000000 | 1.0 |
| F38 | F | 0.1221740500000000 | 0.8060103000000000 | 0.9861219800000000 | 1.0 |
| F39 | F | 0.2109930800000000 | 0.1341039400000000 | 0.1041522400000000 | 1.0 |
| F40 | F | 0.3770629400000000 | 0.0053221700000000 | 0.8821861300000000 | 1.0 |
| F41 | F | 0.2132780100000000 | 0.1559879800000000 | 0.9961173400000000 | 1.0 |
| F42 | F | 0.0892414500000000 | 0.1233720100000000 | 0.0469194400000000 | 1.0 |
| F43 | F | 0.3925794100000000 | 0.8970602700000000 | 0.8988759500000000 | 1.0 |
| F44 | F | 0.2604632900000000 | 0.9417638500000000 | 0.8786631100000000 | 1.0 |
| F45 | F | 0.4891290900000000 | 0.1345952900000000 | 0.1258644600000000 | 1.0 |
| F46 | F | 0.6557874100000000 | 0.9914478200000000 | 0.9230011400000000 | 1.0 |
| F47 | F | 0.3777765800000000 | 0.1778524000000000 | 0.0680069800000000 | 1.0 |
| F48 | F | 0.3529696500000000 | 0.1097926000000000 | 0.1538886700000000 | 1.0 |
| F49 | F | 0.5817006200000000 | 0.8960128100000000 | 0.9287759700000000 | 1.0 |
| F50 | F | 0.5330500500000000 | 0.9791345700000000 | 0.8661466100000000 | 1.0 |
| F51 | F | 0.6330764400000000 | 0.1628831800000000 | 0.9277426600000000 | 1.0 |
| F52 | F | 0.9406184600000000 | 0.7958402800000000 | 0.9380673900000000 | 1.0 |
| F53 | F | 0.5529750300000000 | 0.2160599400000000 | 0.0026803300000000 | 1.0 |
| F54 | F | 0.6913304600000000 | 0.1804657800000000 | 0.0281196600000000 | 1.0 |
| F55 | F | 0.9434661700000000 | 0.7928197700000000 | 0.0481600200000000 | 1.0 |
| F56 | F | 0.8441905700000000 | 0.8560080300000000 | 0.9955229400000000 | 1.0 |
| S57 | S | 0.0243451400000000 | 0.9927715900000000 | 0.0716547800000000 | 1.0 |

|     |   |                    |                    |                    |     |
|-----|---|--------------------|--------------------|--------------------|-----|
| S58 | S | 0.2276928100000000 | 0.9875395400000000 | 0.1016370600000000 | 1.0 |
| S59 | S | 0.4299304400000000 | 0.9850947000000000 | 0.1019216400000000 | 1.0 |
| S60 | S | 0.6514440800000000 | 0.0472751700000000 | 0.0577577500000000 | 1.0 |

##### cif ends

thiophene\_CF3\_3\_anti\_alt Energy: -282.93285794

##### cif starts

data\_thiophene\_CF3\_3\_anti\_alt

\_publ\_section\_comment

;  
Andrew Reynoso, Bohan Xu, and Vincent H. Crespi  
;

\_cell\_length\_a 9.9827034593  
\_cell\_length\_b 20.0  
\_cell\_length\_c 20.0  
\_cell\_angle\_alpha 90.0  
\_cell\_angle\_beta 90.0  
\_cell\_angle\_gamma 90.0

\_symmetry\_space\_group\_name\_H-M 'P 1'  
\_symmetry\_Int\_Tables\_number 1  
\_symmetry\_cell\_setting triclinic

loop\_  
\_atom\_site\_label  
\_atom\_site\_type\_symbol  
\_atom\_site\_fract\_x  
\_atom\_site\_fract\_y  
\_atom\_site\_fract\_z  
\_atom\_site\_occupancy

|     |   |                    |                    |                    |     |
|-----|---|--------------------|--------------------|--------------------|-----|
| H1  | H | 0.0833707200000000 | 0.9305505900000000 | 0.9058721800000000 | 1.0 |
| H2  | H | 0.0326294100000000 | 0.0440713300000000 | 0.0819118400000000 | 1.0 |
| H3  | H | 0.0626679700000000 | 0.1358811700000000 | 0.9894045100000000 | 1.0 |
| H4  | H | 0.7825889200000000 | 0.9959169600000000 | 0.8945858500000000 | 1.0 |
| H5  | H | 0.3333675700000000 | 0.1094953700000000 | 0.0705939600000000 | 1.0 |
| H6  | H | 0.2826434100000000 | 0.9959143000000000 | 0.8945950200000000 | 1.0 |
| H7  | H | 0.3126605600000000 | 0.9041382500000000 | 0.9871452000000000 | 1.0 |
| H8  | H | 0.8126559000000000 | 0.9041291500000000 | 0.9871047900000000 | 1.0 |
| H9  | H | 0.5833308300000000 | 0.9305394400000000 | 0.9059093000000000 | 1.0 |
| H10 | H | 0.5326149500000000 | 0.0441080300000000 | 0.0819242200000000 | 1.0 |
| H11 | H | 0.5626778800000000 | 0.1358896500000000 | 0.9893973900000000 | 1.0 |
| H12 | H | 0.8333937900000000 | 0.1094651900000000 | 0.0706051000000000 | 1.0 |
| C13 | C | 0.0908066300000000 | 0.9737137000000000 | 0.9395268300000000 | 1.0 |
| C14 | C | 0.9920496000000000 | 0.9684674400000000 | 0.0026157300000000 | 1.0 |
| C15 | C | 0.9954761400000000 | 0.0424398300000000 | 0.0303140400000000 | 1.0 |
| C16 | C | 0.0849813300000000 | 0.0831914500000000 | 0.9833669700000000 | 1.0 |
| C17 | C | 0.0271982200000000 | 0.9074567600000000 | 0.0520236500000000 | 1.0 |
| C18 | C | 0.3408105100000000 | 0.0663157300000000 | 0.0369593800000000 | 1.0 |
| C19 | C | 0.2420509800000000 | 0.0715385600000000 | 0.9738659600000000 | 1.0 |
| C20 | C | 0.2454640000000000 | 0.9975591800000000 | 0.9461878900000000 | 1.0 |
| C21 | C | 0.3349685100000000 | 0.9568298400000000 | 0.9931568000000000 | 1.0 |
| C22 | C | 0.2771683200000000 | 0.1325066600000000 | 0.9244020500000000 | 1.0 |

|     |   |                    |                    |                    |     |
|-----|---|--------------------|--------------------|--------------------|-----|
| C23 | C | 0.5907895400000000 | 0.9737115800000000 | 0.9395517300000000 | 1.0 |
| C24 | C | 0.4920410100000000 | 0.9684853500000000 | 0.0026475800000000 | 1.0 |
| C25 | C | 0.4954652400000000 | 0.0424620500000000 | 0.0303257000000000 | 1.0 |
| C26 | C | 0.5849795100000000 | 0.0831974600000000 | 0.9833714500000000 | 1.0 |
| C27 | C | 0.5271760200000000 | 0.9075125300000000 | 0.0521002500000000 | 1.0 |
| C28 | C | 0.7771719000000000 | 0.1325033900000000 | 0.9244087200000000 | 1.0 |
| C29 | C | 0.8408242800000000 | 0.0662943900000000 | 0.0369596200000000 | 1.0 |
| C30 | C | 0.7420492800000000 | 0.0715337000000000 | 0.9738704100000000 | 1.0 |
| C31 | C | 0.7454483600000000 | 0.9975576500000000 | 0.9461856700000000 | 1.0 |
| C32 | C | 0.8349736000000000 | 0.9568159800000000 | 0.9931326500000000 | 1.0 |
| F33 | F | 0.8005994200000000 | 0.1155793600000000 | 0.8596802900000000 | 1.0 |
| F34 | F | 0.9287098100000000 | 0.8594107700000000 | 0.0559302500000000 | 1.0 |
| F35 | F | 0.0508256700000000 | 0.9243160100000000 | 0.1167475200000000 | 1.0 |
| F36 | F | 0.1350306600000000 | 0.8714042500000000 | 0.0294832600000000 | 1.0 |
| F37 | F | 0.6787192400000000 | 0.1805715800000000 | 0.9205362000000000 | 1.0 |
| F38 | F | 0.1787174700000000 | 0.1805756300000000 | 0.9205386000000000 | 1.0 |
| F39 | F | 0.3005828300000000 | 0.1155830000000000 | 0.8596720200000000 | 1.0 |
| F40 | F | 0.3851152400000000 | 0.1685449500000000 | 0.9468182900000000 | 1.0 |
| F41 | F | 0.8851091300000000 | 0.1685429800000000 | 0.9468316100000000 | 1.0 |
| F42 | F | 0.4287313800000000 | 0.8594411000000000 | 0.0559808800000000 | 1.0 |
| F43 | F | 0.5506408700000000 | 0.9244287100000000 | 0.1168246900000000 | 1.0 |
| F44 | F | 0.6350967400000000 | 0.8714728000000000 | 0.0296519100000000 | 1.0 |
| S45 | S | 0.0307124500000000 | 0.0497761600000000 | 0.9009789000000000 | 1.0 |
| S46 | S | 0.2807100700000000 | 0.9902712000000000 | 0.0755352600000000 | 1.0 |
| S47 | S | 0.5306994600000000 | 0.0497701000000000 | 0.9009895600000000 | 1.0 |
| S48 | S | 0.7807481500000000 | 0.9902382500000000 | 0.0755230800000000 | 1.0 |

##### cif ends

thiophene\_CF3\_3\_anti\_alt\_forbid    Energy: -283.70958727

##### cif starts

data\_thiophene\_CF3\_3\_anti\_alt\_forbid

\_publ\_section\_comment

;

Andrew Reynoso, Bohan Xu, and Vincent H. Crespi

;

\_cell\_length\_a    10.5039611319

\_cell\_length\_b    20.0

\_cell\_length\_c    20.0

\_cell\_angle\_alpha    90.0

\_cell\_angle\_beta    90.0

\_cell\_angle\_gamma    90.0

\_symmetry\_space\_group\_name\_H-M    'P 1'

\_symmetry\_Int\_Tables\_number    1

\_symmetry\_cell\_setting    triclinic

loop\_

\_atom\_site\_label

\_atom\_site\_type\_symbol

\_atom\_site\_fract\_x

\_atom\_site\_fract\_y

\_atom\_site\_fract\_z

|     | atom | site               | occupancy          |                    |     |  |  |
|-----|------|--------------------|--------------------|--------------------|-----|--|--|
| H1  | H    | 0.0687708600000000 | 0.1059904700000000 | 0.9380932100000000 | 1.0 |  |  |
| H2  | H    | 0.9548704200000000 | 0.9391304200000000 | 0.0623730300000000 | 1.0 |  |  |
| H3  | H    | 0.0587259300000000 | 0.8841060800000000 | 0.9513137300000000 | 1.0 |  |  |
| H4  | H    | 0.3286539900000000 | 0.0497328800000000 | 0.9126042700000000 | 1.0 |  |  |
| H5  | H    | 0.2248345500000000 | 0.1047330300000000 | 0.0237037100000000 | 1.0 |  |  |
| H6  | H    | 0.2148749900000000 | 0.8828483300000000 | 0.0368781200000000 | 1.0 |  |  |
| H7  | H    | 0.5687369300000000 | 0.1060434300000000 | 0.9380977500000000 | 1.0 |  |  |
| H8  | H    | 0.4549950100000000 | 0.9391162400000000 | 0.0623218000000000 | 1.0 |  |  |
| H9  | H    | 0.5588039700000000 | 0.8841593200000000 | 0.9511949600000000 | 1.0 |  |  |
| H10 | H    | 0.8287298900000000 | 0.0497324200000000 | 0.9125754300000000 | 1.0 |  |  |
| H11 | H    | 0.7248919600000000 | 0.1047536700000000 | 0.0236454200000000 | 1.0 |  |  |
| H12 | H    | 0.7147966000000000 | 0.8828737200000000 | 0.0368414000000000 | 1.0 |  |  |
| C13 | C    | 0.9486401800000000 | 0.0947403300000000 | 0.0596381100000000 | 1.0 |  |  |
| C14 | C    | 0.3349071100000000 | 0.8941984000000000 | 0.9152540700000000 | 1.0 |  |  |
| C15 | C    | 0.4486980300000000 | 0.0947009000000000 | 0.0596704500000000 | 1.0 |  |  |
| C16 | C    | 0.8349738200000000 | 0.8941122200000000 | 0.9153219200000000 | 1.0 |  |  |
| C17 | C    | 0.0790129500000000 | 0.0570264900000000 | 0.9625088200000000 | 1.0 |  |  |
| C18 | C    | 0.9561632900000000 | 0.0387034700000000 | 0.0042899200000000 | 1.0 |  |  |
| C19 | C    | 0.9585469300000000 | 0.9588384100000000 | 0.0112566800000000 | 1.0 |  |  |
| C20 | C    | 0.0763625100000000 | 0.9337186300000000 | 0.9714014400000000 | 1.0 |  |  |
| C21 | C    | 0.2072296900000000 | 0.0551258400000000 | 0.0035979000000000 | 1.0 |  |  |
| C22 | C    | 0.3250378100000000 | 0.0300300600000000 | 0.9637227600000000 | 1.0 |  |  |
| C23 | C    | 0.3274227700000000 | 0.9501677900000000 | 0.9706659200000000 | 1.0 |  |  |
| C24 | C    | 0.2046043000000000 | 0.9318169100000000 | 0.0124723100000000 | 1.0 |  |  |
| C25 | C    | 0.5790070700000000 | 0.0570654100000000 | 0.9624816600000000 | 1.0 |  |  |
| C26 | C    | 0.4561846000000000 | 0.0387052400000000 | 0.0042792200000000 | 1.0 |  |  |
| C27 | C    | 0.4585829000000000 | 0.9588381500000000 | 0.0112082800000000 | 1.0 |  |  |
| C28 | C    | 0.5763942300000000 | 0.9337578000000000 | 0.9713232300000000 | 1.0 |  |  |
| C29 | C    | 0.7072502800000000 | 0.0551450600000000 | 0.0035529000000000 | 1.0 |  |  |
| C30 | C    | 0.8250675100000000 | 0.0300266400000000 | 0.9636925200000000 | 1.0 |  |  |
| C31 | C    | 0.8274566900000000 | 0.9501619800000000 | 0.9706594300000000 | 1.0 |  |  |
| C32 | C    | 0.7045874600000000 | 0.9318423600000000 | 0.0124315600000000 | 1.0 |  |  |
| F33 | F    | 0.9068026900000000 | 0.1519896900000000 | 0.0268069200000000 | 1.0 |  |  |
| F34 | F    | 0.5612452100000000 | 0.1143284700000000 | 0.0878534000000000 | 1.0 |  |  |
| F35 | F    | 0.3714737100000000 | 0.0857407300000000 | 0.1131440800000000 | 1.0 |  |  |
| F36 | F    | 0.4066331100000000 | 0.1519528200000000 | 0.0269231700000000 | 1.0 |  |  |
| F37 | F    | 0.4119559900000000 | 0.9032664800000000 | 0.8617345300000000 | 1.0 |  |  |
| F38 | F    | 0.2223416000000000 | 0.8744889000000000 | 0.8871414100000000 | 1.0 |  |  |
| F39 | F    | 0.3772107800000000 | 0.8369556100000000 | 0.9479302500000000 | 1.0 |  |  |
| F40 | F    | 0.9124753200000000 | 0.9029118200000000 | 0.8619278600000000 | 1.0 |  |  |
| F41 | F    | 0.7224727300000000 | 0.8745911100000000 | 0.8870176100000000 | 1.0 |  |  |
| F42 | F    | 0.8766958900000000 | 0.8368537000000000 | 0.9481826400000000 | 1.0 |  |  |
| F43 | F    | 0.0611499100000000 | 0.1143007200000000 | 0.0879051900000000 | 1.0 |  |  |
| F44 | F    | 0.8712187400000000 | 0.0858879100000000 | 0.1130542300000000 | 1.0 |  |  |
| S45 | S    | 0.0870377200000000 | 0.9928193300000000 | 0.9004656300000000 | 1.0 |  |  |
| S46 | S    | 0.1965819500000000 | 0.9960150600000000 | 0.0745250900000000 | 1.0 |  |  |
| S47 | S    | 0.5870678400000000 | 0.9928884100000000 | 0.9004124300000000 | 1.0 |  |  |
| S48 | S    | 0.6965719400000000 | 0.9960407200000000 | 0.0744835200000000 | 1.0 |  |  |

##### cif ends

thiophene\_CF3\_3\_anti\_dir    Energy: -282.61511051

##### cif starts

data\_thiophene\_CF3\_3\_anti\_dir

\_publ\_section\_comment  
;  
Andrew Reynoso, Bohan Xu, and Vincent H. Crespi  
;

\_cell\_length\_a 10.0071427757  
\_cell\_length\_b 20.0  
\_cell\_length\_c 20.0  
\_cell\_angle\_alpha 90.0  
\_cell\_angle\_beta 90.0  
\_cell\_angle\_gamma 90.0

\_symmetry\_space\_group\_name\_H-M 'P 1'  
\_symmetry\_Int\_Tables\_number 1  
\_symmetry\_cell\_setting triclinic

loop\_

\_atom\_site\_label  
\_atom\_site\_type\_symbol  
\_atom\_site\_fract\_x  
\_atom\_site\_fract\_y  
\_atom\_site\_fract\_z  
\_atom\_site\_occupancy

|     |   |                    |                    |                    |     |
|-----|---|--------------------|--------------------|--------------------|-----|
| H1  | H | 0.0429233200000000 | 0.0921376400000000 | 0.9504420800000000 | 1.0 |
| H2  | H | 0.0036418600000000 | 0.9208422200000000 | 0.0686835400000000 | 1.0 |
| H3  | H | 0.0469553100000000 | 0.8701061600000000 | 0.9459293400000000 | 1.0 |
| H4  | H | 0.2928630800000000 | 0.0915964700000000 | 0.0319832400000000 | 1.0 |
| H5  | H | 0.2536222800000000 | 0.9218413600000000 | 0.9115306300000000 | 1.0 |
| H6  | H | 0.2970165700000000 | 0.8695287800000000 | 0.0336112800000000 | 1.0 |
| H7  | H | 0.7536856800000000 | 0.9218774900000000 | 0.9115517300000000 | 1.0 |
| H8  | H | 0.5428957600000000 | 0.0921547400000000 | 0.9504453300000000 | 1.0 |
| H9  | H | 0.5036584300000000 | 0.9208354300000000 | 0.0686603700000000 | 1.0 |
| H10 | H | 0.5470199900000000 | 0.8701251600000000 | 0.9458982200000000 | 1.0 |
| H11 | H | 0.7969607000000000 | 0.8695580500000000 | 0.0336453100000000 | 1.0 |
| H12 | H | 0.7929128700000000 | 0.0916257500000000 | 0.0320003800000000 | 1.0 |
| C13 | C | 0.0588053900000000 | 0.0403254600000000 | 0.9642746100000000 | 1.0 |
| C14 | C | 0.9648935900000000 | 0.0209201800000000 | 0.0234727000000000 | 1.0 |
| C15 | C | 0.9675125400000000 | 0.9418149300000000 | 0.0213001200000000 | 1.0 |
| C16 | C | 0.0619363900000000 | 0.9222024000000000 | 0.9615604100000000 | 1.0 |
| C17 | C | 0.0000393100000000 | 0.0588584200000000 | 0.0927163400000000 | 1.0 |
| C18 | C | 0.7500470900000000 | 0.0601905000000000 | 0.8893031000000000 | 1.0 |
| C19 | C | 0.3087866900000000 | 0.0399716700000000 | 0.0174753800000000 | 1.0 |
| C20 | C | 0.2148854000000000 | 0.0213280700000000 | 0.9580347900000000 | 1.0 |
| C21 | C | 0.2175102800000000 | 0.9422018400000000 | 0.9591849800000000 | 1.0 |
| C22 | C | 0.3119634000000000 | 0.9218257700000000 | 0.0186535500000000 | 1.0 |
| C23 | C | 0.2500163100000000 | 0.0601610300000000 | 0.8892844200000000 | 1.0 |
| C24 | C | 0.5587996700000000 | 0.0403411600000000 | 0.9642733000000000 | 1.0 |
| C25 | C | 0.4648765600000000 | 0.0209174700000000 | 0.0234610700000000 | 1.0 |
| C26 | C | 0.4675249200000000 | 0.9418114100000000 | 0.0212785400000000 | 1.0 |
| C27 | C | 0.5619688900000000 | 0.9222178800000000 | 0.9615449800000000 | 1.0 |
| C28 | C | 0.4999902400000000 | 0.0588593200000000 | 0.0927065800000000 | 1.0 |
| C29 | C | 0.8088030600000000 | 0.0399971300000000 | 0.0174924000000000 | 1.0 |
| C30 | C | 0.7148973800000000 | 0.0213576400000000 | 0.9580502300000000 | 1.0 |
| C31 | C | 0.7175290800000000 | 0.9422295500000000 | 0.9591986000000000 | 1.0 |

|     |   |                    |                    |                    |     |
|-----|---|--------------------|--------------------|--------------------|-----|
| C32 | C | 0.8119454300000000 | 0.9218500700000000 | 0.0186800300000000 | 1.0 |
| F33 | F | 0.8578252800000000 | 0.1018592100000000 | 0.8973247400000000 | 1.0 |
| F34 | F | 0.1077177900000000 | 0.1006835500000000 | 0.0851966500000000 | 1.0 |
| F35 | F | 0.0233710100000000 | 0.0185495700000000 | 0.1460984200000000 | 1.0 |
| F36 | F | 0.9026435000000000 | 0.1020522700000000 | 0.1149697000000000 | 1.0 |
| F37 | F | 0.6527193900000000 | 0.1037319100000000 | 0.8676568900000000 | 1.0 |
| F38 | F | 0.1526323100000000 | 0.1036513900000000 | 0.8676004300000000 | 1.0 |
| F39 | F | 0.2732947400000000 | 0.0205399600000000 | 0.8353848800000000 | 1.0 |
| F40 | F | 0.3577196900000000 | 0.1018751100000000 | 0.8973292900000000 | 1.0 |
| F41 | F | 0.7732138800000000 | 0.0205699900000000 | 0.8353909300000000 | 1.0 |
| F42 | F | 0.4025823000000000 | 0.1020578100000000 | 0.1149408600000000 | 1.0 |
| F43 | F | 0.6076761100000000 | 0.1006824000000000 | 0.0851999700000000 | 1.0 |
| F44 | F | 0.5232806100000000 | 0.0185529200000000 | 0.1460927000000000 | 1.0 |
| S45 | S | 0.0030928500000000 | 0.9807329200000000 | 0.8991563800000000 | 1.0 |
| S46 | S | 0.2531080200000000 | 0.9795320400000000 | 0.0818159800000000 | 1.0 |
| S47 | S | 0.5031255700000000 | 0.9807528000000000 | 0.8991459300000000 | 1.0 |
| S48 | S | 0.7531056500000000 | 0.9795684200000000 | 0.0818352300000000 | 1.0 |

##### cif ends

thiophene\_CF3\_3\_anti\_dir\_forbid    Energy: -283.59338762

##### cif starts

data\_thiophene\_CF3\_3\_anti\_dir\_forbid

\_publ\_section\_comment

;  
Andrew Reynoso, Bohan Xu, and Vincent H. Crespi  
;

\_cell\_length\_a    10.5319456145

\_cell\_length\_b    20.0

\_cell\_length\_c    20.0

\_cell\_angle\_alpha    90.0

\_cell\_angle\_beta    90.0

\_cell\_angle\_gamma    90.0

\_symmetry\_space\_group\_name\_H-M    'P 1'

\_symmetry\_Int\_Tables\_number 1

\_symmetry\_cell\_setting triclinic

loop\_

\_atom\_site\_label

\_atom\_site\_type\_symbol

\_atom\_site\_fract\_x

\_atom\_site\_fract\_y

\_atom\_site\_fract\_z

\_atom\_site\_occupancy

|    |   |                    |                    |                    |     |
|----|---|--------------------|--------------------|--------------------|-----|
| H1 | H | 0.0263598600000000 | 0.1286664800000000 | 0.9617198300000000 | 1.0 |
| H2 | H | 0.1394012000000000 | 0.0689061200000000 | 0.0665147700000000 | 1.0 |
| H3 | H | 0.3529136300000000 | 0.1214700200000000 | 0.0404844400000000 | 1.0 |
| H4 | H | 0.2480729700000000 | 0.0755133100000000 | 0.9251999100000000 | 1.0 |
| H5 | H | 0.5263329700000000 | 0.1286688500000000 | 0.9617434100000000 | 1.0 |
| H6 | H | 0.6394174200000000 | 0.0688727300000000 | 0.0665046200000000 | 1.0 |
| H7 | H | 0.8528920400000000 | 0.1214957300000000 | 0.0404342500000000 | 1.0 |
| H8 | H | 0.7480276800000000 | 0.0755129100000000 | 0.9251742900000000 | 1.0 |



|     |   |                    |                    |                    |     |
|-----|---|--------------------|--------------------|--------------------|-----|
| H9  | H | 0.0188849300000000 | 0.9070329800000000 | 0.9412945800000000 | 1.0 |
| H10 | H | 0.3725408900000000 | 0.8996245600000000 | 0.0280736400000000 | 1.0 |
| H11 | H | 0.5188403000000000 | 0.9070423700000000 | 0.9412408600000000 | 1.0 |
| H12 | H | 0.8725382200000000 | 0.8996457100000000 | 0.0280888500000000 | 1.0 |
| C13 | C | 0.0076366400000000 | 0.0772697100000000 | 0.9787190800000000 | 1.0 |
| C14 | C | 0.1283751200000000 | 0.0487480000000000 | 0.0158406700000000 | 1.0 |
| C15 | C | 0.1260317100000000 | 0.9692560100000000 | 0.0126744200000000 | 1.0 |
| C16 | C | 0.0070878700000000 | 0.9538195500000000 | 0.9683126500000000 | 1.0 |
| C17 | C | 0.3744932700000000 | 0.0735857900000000 | 0.0158997800000000 | 1.0 |
| C18 | C | 0.2559421800000000 | 0.0500627300000000 | 0.9735606800000000 | 1.0 |
| C19 | C | 0.2584628700000000 | 0.9699408400000000 | 0.9702621800000000 | 1.0 |
| C20 | C | 0.3807236000000000 | 0.9500311000000000 | 0.0090781800000000 | 1.0 |
| C21 | C | 0.5076287100000000 | 0.0772652900000000 | 0.9787283100000000 | 1.0 |
| C22 | C | 0.6283774200000000 | 0.0487316600000000 | 0.0158249000000000 | 1.0 |
| C23 | C | 0.6260330100000000 | 0.9692384500000000 | 0.0126341400000000 | 1.0 |
| C24 | C | 0.5070621600000000 | 0.9538179400000000 | 0.9682801200000000 | 1.0 |
| C25 | C | 0.8744799400000000 | 0.0736039800000000 | 0.0158681400000000 | 1.0 |
| C26 | C | 0.7559368800000000 | 0.0500652400000000 | 0.9735350900000000 | 1.0 |
| C27 | C | 0.7584871100000000 | 0.9699447200000000 | 0.9702368000000000 | 1.0 |
| C28 | C | 0.8807243700000000 | 0.9500471600000000 | 0.0090811200000000 | 1.0 |
| C29 | C | 0.1277603600000000 | 0.9267575700000000 | 0.0805184800000000 | 1.0 |
| C30 | C | 0.2505102000000000 | 0.9217184000000000 | 0.9077430300000000 | 1.0 |
| C31 | C | 0.6277715400000000 | 0.9266992200000000 | 0.0804552200000000 | 1.0 |
| C32 | C | 0.7505554700000000 | 0.9217691100000000 | 0.9076842200000000 | 1.0 |
| F33 | F | 0.1345463100000000 | 0.9648412500000000 | 0.1365230500000000 | 1.0 |
| F34 | F | 0.7257942400000000 | 0.8817985500000000 | 0.0842572500000000 | 1.0 |
| F35 | F | 0.5246281000000000 | 0.8854818600000000 | 0.0891931500000000 | 1.0 |
| F36 | F | 0.6346534000000000 | 0.9647443700000000 | 0.1364804300000000 | 1.0 |
| F37 | F | 0.3616977000000000 | 0.9069850100000000 | 0.8758137500000000 | 1.0 |
| F38 | F | 0.1713599900000000 | 0.9382653500000000 | 0.8569321600000000 | 1.0 |
| F39 | F | 0.2094650600000000 | 0.8607439100000000 | 0.9324175300000000 | 1.0 |
| F40 | F | 0.8617989600000000 | 0.9068944700000000 | 0.8758693800000000 | 1.0 |
| F41 | F | 0.6717052500000000 | 0.9385015800000000 | 0.8568077100000000 | 1.0 |
| F42 | F | 0.7091338600000000 | 0.8608204200000000 | 0.9322457300000000 | 1.0 |
| F43 | F | 0.2258251300000000 | 0.8818896600000000 | 0.0843806800000000 | 1.0 |
| F44 | F | 0.0246411300000000 | 0.8855195900000000 | 0.0892460400000000 | 1.0 |
| S45 | S | 0.9991348200000000 | 0.0229651700000000 | 0.9071398400000000 | 1.0 |
| S46 | S | 0.3842315100000000 | 0.0089536500000000 | 0.0791076800000000 | 1.0 |
| S47 | S | 0.4990718000000000 | 0.0229845700000000 | 0.9071333000000000 | 1.0 |
| S48 | S | 0.8841900800000000 | 0.0089966800000000 | 0.0790947100000000 | 1.0 |

##### cif ends

thiophene\_CF3\_3\_syn\_alt    Energy: -283.12924317

##### cif starts

data\_thiophene\_CF3\_3\_syn\_alt

\_publ\_section\_comment

;  
Andrew Reynoso, Bohan Xu, and Vincent H. Crespi  
;

\_cell\_length\_a    10.6664895099

\_cell\_length\_b    20.0

\_cell\_length\_c    20.0

\_cell\_angle\_alpha 90.0  
\_cell\_angle\_beta 90.0  
\_cell\_angle\_gamma 90.0

\_symmetry\_space\_group\_name\_H-M 'P 1'  
\_symmetry\_Int\_Tables\_number 1  
\_symmetry\_cell\_setting triclinic

loop\_

\_atom\_site\_label  
\_atom\_site\_type\_symbol  
\_atom\_site\_fract\_x  
\_atom\_site\_fract\_y  
\_atom\_site\_fract\_z  
\_atom\_site\_occupancy

|     |   |                    |                    |                    |     |
|-----|---|--------------------|--------------------|--------------------|-----|
| H1  | H | 0.0510656800000000 | 0.8980356400000000 | 0.0562427600000000 | 1.0 |
| H2  | H | 0.1941487600000000 | 0.0576990000000000 | 0.9370954500000000 | 1.0 |
| H3  | H | 0.0596331900000000 | 0.1180851400000000 | 0.0275979600000000 | 1.0 |
| H4  | H | 0.9439902700000000 | 0.9407251400000000 | 0.9373503100000000 | 1.0 |
| H5  | H | 0.3009167900000000 | 0.1006579100000000 | 0.0560317800000000 | 1.0 |
| H6  | H | 0.4442008600000000 | 0.9408013800000000 | 0.9372064400000000 | 1.0 |
| H7  | H | 0.3095890000000000 | 0.8805603200000000 | 0.0277879500000000 | 1.0 |
| H8  | H | 0.8096890600000000 | 0.8806829800000000 | 0.0282507600000000 | 1.0 |
| H9  | H | 0.5507988800000000 | 0.8979795400000000 | 0.0562330500000000 | 1.0 |
| H10 | H | 0.6940157000000000 | 0.0575789100000000 | 0.9370994900000000 | 1.0 |
| H11 | H | 0.5596271000000000 | 0.1180330600000000 | 0.0276830100000000 | 1.0 |
| H12 | H | 0.8008855400000000 | 0.1008608000000000 | 0.0558298000000000 | 1.0 |
| C13 | C | 0.0535160000000000 | 0.9469675700000000 | 0.0314563500000000 | 1.0 |
| C14 | C | 0.1767667400000000 | 0.9584401300000000 | 0.9865538600000000 | 1.0 |
| C15 | C | 0.1829157100000000 | 0.0369985300000000 | 0.9869706400000000 | 1.0 |
| C16 | C | 0.0566066700000000 | 0.0638004800000000 | 0.0197118100000000 | 1.0 |
| C17 | C | 0.1628229600000000 | 0.9222152500000000 | 0.9184315700000000 | 1.0 |
| C18 | C | 0.9128077100000000 | 0.0761688600000000 | 0.9182730800000000 | 1.0 |
| C19 | C | 0.3034420400000000 | 0.0516856700000000 | 0.0313305900000000 | 1.0 |
| C20 | C | 0.4267670000000000 | 0.0401275700000000 | 0.9865159300000000 | 1.0 |
| C21 | C | 0.4329265200000000 | 0.9615672300000000 | 0.9870542600000000 | 1.0 |
| C22 | C | 0.3066043700000000 | 0.9348419300000000 | 0.0198143600000000 | 1.0 |
| C23 | C | 0.4128696200000000 | 0.0762546600000000 | 0.9183345700000000 | 1.0 |
| C24 | C | 0.5534143000000000 | 0.9469216100000000 | 0.0314752400000000 | 1.0 |
| C25 | C | 0.6768217200000000 | 0.9583941800000000 | 0.9867077900000000 | 1.0 |
| C26 | C | 0.6828899400000000 | 0.0369610500000000 | 0.9870150800000000 | 1.0 |
| C27 | C | 0.5566013000000000 | 0.0637526100000000 | 0.0197647500000000 | 1.0 |
| C28 | C | 0.6630332400000000 | 0.9220691700000000 | 0.9186200000000000 | 1.0 |
| C29 | C | 0.8034431400000000 | 0.0517989300000000 | 0.0312985200000000 | 1.0 |
| C30 | C | 0.9267640600000000 | 0.0401453600000000 | 0.9865058700000000 | 1.0 |
| C31 | C | 0.9328972000000000 | 0.9615763700000000 | 0.9871714300000000 | 1.0 |
| C32 | C | 0.8066405700000000 | 0.9349290800000000 | 0.0200782900000000 | 1.0 |
| F33 | F | 0.1030575900000000 | 0.8616893200000000 | 0.9270849600000000 | 1.0 |
| F34 | F | 0.2745515600000000 | 0.9064468800000000 | 0.8890807700000000 | 1.0 |
| F35 | F | 0.0975454400000000 | 0.9567464900000000 | 0.8708499600000000 | 1.0 |
| F36 | F | 0.8527497400000000 | 0.1366395500000000 | 0.9267238500000000 | 1.0 |
| F37 | F | 0.3530011800000000 | 0.1367628300000000 | 0.9268905900000000 | 1.0 |
| F38 | F | 0.3477173300000000 | 0.0416390400000000 | 0.8707583100000000 | 1.0 |
| F39 | F | 0.5246109500000000 | 0.0920414500000000 | 0.8890186300000000 | 1.0 |
| F40 | F | 0.0245169900000000 | 0.0920111300000000 | 0.8889537300000000 | 1.0 |

|     |   |                    |                    |                    |     |
|-----|---|--------------------|--------------------|--------------------|-----|
| F41 | F | 0.8477640300000000 | 0.0414243800000000 | 0.8707509000000000 | 1.0 |
| F42 | F | 0.6029164200000000 | 0.8616433300000000 | 0.9272838300000000 | 1.0 |
| F43 | F | 0.7747961600000000 | 0.9060711700000000 | 0.8894291800000000 | 1.0 |
| F44 | F | 0.5981339100000000 | 0.9566314400000000 | 0.8709134200000000 | 1.0 |
| S45 | S | 0.0553625900000000 | 0.0176098900000000 | 0.0950325200000000 | 1.0 |
| S46 | S | 0.3051606900000000 | 0.9811427600000000 | 0.0950639400000000 | 1.0 |
| S47 | S | 0.5550778700000000 | 0.0175253500000000 | 0.0950645600000000 | 1.0 |
| S48 | S | 0.8052458700000000 | 0.9814853200000000 | 0.0951822500000000 | 1.0 |

##### cif ends

thiophene\_CF3\_3\_syn\_alt\_forbid    Energy: -280.77032659

##### cif starts

data\_thiophene\_CF3\_3\_syn\_alt\_forbid

\_publ\_section\_comment

;  
Andrew Reynoso, Bohan Xu, and Vincent H. Crespi  
;

\_cell\_length\_a    9.9930559885

\_cell\_length\_b    20.0

\_cell\_length\_c    20.0

\_cell\_angle\_alpha    90.0

\_cell\_angle\_beta    90.0

\_cell\_angle\_gamma    90.0

\_symmetry\_space\_group\_name\_H-M    'P 1'

\_symmetry\_Int\_Tables\_number 1

\_symmetry\_cell\_setting triclinic

loop\_

\_atom\_site\_label

\_atom\_site\_type\_symbol

\_atom\_site\_fract\_x

\_atom\_site\_fract\_y

\_atom\_site\_fract\_z

\_atom\_site\_occupancy

|     |   |                    |                    |                    |     |
|-----|---|--------------------|--------------------|--------------------|-----|
| H1  | H | 0.0229102700000000 | 0.1281434100000000 | 0.0268625800000000 | 1.0 |
| H2  | H | 0.9803311500000000 | 0.0455604200000000 | 0.9272585700000000 | 1.0 |
| H3  | H | 0.0247786000000000 | 0.9168196800000000 | 0.0968143600000000 | 1.0 |
| H4  | H | 0.2524201000000000 | 0.1326803600000000 | 0.0353284000000000 | 1.0 |
| H5  | H | 0.2406672600000000 | 0.9417263700000000 | 0.9521475800000000 | 1.0 |
| H6  | H | 0.2518963000000000 | 0.9171101100000000 | 0.0886766700000000 | 1.0 |
| H7  | H | 0.5203007800000000 | 0.0825171600000000 | 0.0829206500000000 | 1.0 |
| H8  | H | 0.5340189400000000 | 0.0472671900000000 | 0.9486395700000000 | 1.0 |
| H9  | H | 0.5216824600000000 | 0.8636045800000000 | 0.0462438700000000 | 1.0 |
| H10 | H | 0.7474487500000000 | 0.0833540600000000 | 0.0924982400000000 | 1.0 |
| H11 | H | 0.7894185500000000 | 0.9445236500000000 | 0.9309143100000000 | 1.0 |
| H12 | H | 0.7510102900000000 | 0.8680782600000000 | 0.0357246900000000 | 1.0 |
| C13 | C | 0.0564027200000000 | 0.0758954200000000 | 0.0278741400000000 | 1.0 |
| C14 | C | 0.9659495000000000 | 0.0344867800000000 | 0.9802556700000000 | 1.0 |
| C15 | C | 0.9683974000000000 | 0.9577035700000000 | 0.9951758100000000 | 1.0 |
| C16 | C | 0.0504970700000000 | 0.9584228800000000 | 0.0636331800000000 | 1.0 |
| C17 | C | 0.0191856000000000 | 0.9020676400000000 | 0.9470063500000000 | 1.0 |

|     |   |                    |                    |                    |     |
|-----|---|--------------------|--------------------|--------------------|-----|
| C18 | C | 0.2269231300000000 | 0.0795011100000000 | 0.0312851700000000 | 1.0 |
| C19 | C | 0.3200032500000000 | 0.0419918900000000 | 0.9808597500000000 | 1.0 |
| C20 | C | 0.2941062100000000 | 0.9659136500000000 | 0.9925087400000000 | 1.0 |
| C21 | C | 0.2177620300000000 | 0.9607372400000000 | 0.0602676700000000 | 1.0 |
| C22 | C | 0.3028587400000000 | 0.0735304600000000 | 0.9110832000000000 | 1.0 |
| C23 | C | 0.5553228000000000 | 0.0369014900000000 | 0.0581446500000000 | 1.0 |
| C24 | C | 0.4799388000000000 | 0.0263731900000000 | 0.9906774200000000 | 1.0 |
| C25 | C | 0.4541301500000000 | 0.9495949500000000 | 0.9844739500000000 | 1.0 |
| C26 | C | 0.5465239000000000 | 0.9163525600000000 | 0.0380233900000000 | 1.0 |
| C27 | C | 0.4763794500000000 | 0.9135803500000000 | 0.9167386200000000 | 1.0 |
| C28 | C | 0.7222135600000000 | 0.0397370100000000 | 0.0619020200000000 | 1.0 |
| C29 | C | 0.8033750800000000 | 0.0365114700000000 | 0.9933696800000000 | 1.0 |
| C30 | C | 0.8054083200000000 | 0.9588235300000000 | 0.9829988800000000 | 1.0 |
| C31 | C | 0.7166712100000000 | 0.9201713800000000 | 0.0337040900000000 | 1.0 |
| C32 | C | 0.7528769400000000 | 0.0901720000000000 | 0.9428341800000000 | 1.0 |
| F33 | F | 0.4889018500000000 | 0.8458368200000000 | 0.9272305600000000 | 1.0 |
| F34 | F | 0.9192385900000000 | 0.8587179400000000 | 0.9284679900000000 | 1.0 |
| F35 | F | 0.1122036900000000 | 0.8604968700000000 | 0.9761123300000000 | 1.0 |
| F36 | F | 0.7046775700000000 | 0.0645554100000000 | 0.8843246900000000 | 1.0 |
| F37 | F | 0.3757119000000000 | 0.9201877800000000 | 0.8713292200000000 | 1.0 |
| F38 | F | 0.5905254000000000 | 0.9334936200000000 | 0.8848317000000000 | 1.0 |
| F39 | F | 0.6569729600000000 | 0.1319209700000000 | 0.9691161800000000 | 1.0 |
| F40 | F | 0.0717947100000000 | 0.9256276600000000 | 0.8885183800000000 | 1.0 |
| F41 | F | 0.3208904000000000 | 0.1415786900000000 | 0.9159271500000000 | 1.0 |
| F42 | F | 0.1784800100000000 | 0.0641041600000000 | 0.8843429700000000 | 1.0 |
| F43 | F | 0.3913716900000000 | 0.0523337200000000 | 0.8638144400000000 | 1.0 |
| F44 | F | 0.8528533300000000 | 0.1337505200000000 | 0.9246380600000000 | 1.0 |
| S45 | S | 0.0037420200000000 | 0.0368555800000000 | 0.1045129900000000 | 1.0 |
| S46 | S | 0.2703831000000000 | 0.0365533900000000 | 0.1060096900000000 | 1.0 |
| S47 | S | 0.5026882900000000 | 0.9647003600000000 | 0.1092847200000000 | 1.0 |
| S48 | S | 0.7697212000000000 | 0.9640753300000000 | 0.1075953800000000 | 1.0 |

##### cif ends

thiophene\_CF3\_3\_syn\_dir Energy: -278.88864879

##### cif starts

data\_thiophene\_CF3\_3\_syn\_dir

\_publ\_section\_comment

;  
Andrew Reynoso, Bohan Xu, and Vincent H. Crespi  
;

\_cell\_length\_a 10.8135292146

\_cell\_length\_b 20.0

\_cell\_length\_c 20.0

\_cell\_angle\_alpha 90.0

\_cell\_angle\_beta 90.0

\_cell\_angle\_gamma 90.0

\_symmetry\_space\_group\_name\_H-M 'P 1'

\_symmetry\_Int\_Tables\_number 1

\_symmetry\_cell\_setting triclinic

loop\_

|     | _atom_site_label       |                    |                    |                    |     |
|-----|------------------------|--------------------|--------------------|--------------------|-----|
|     | _atom_site_type_symbol |                    |                    |                    |     |
|     | _atom_site_fract_x     |                    |                    |                    |     |
|     | _atom_site_fract_y     |                    |                    |                    |     |
|     | _atom_site_fract_z     |                    |                    |                    |     |
|     | _atom_site_occupancy   |                    |                    |                    |     |
| H1  | H                      | 0.0984382600000000 | 0.9207808400000000 | 0.9394270200000000 | 1.0 |
| H2  | H                      | 0.9796794600000000 | 0.8647443600000000 | 0.0433195800000000 | 1.0 |
| H3  | H                      | 0.0177950300000000 | 0.0825490000000000 | 0.0716957800000000 | 1.0 |
| H4  | H                      | 0.3707088100000000 | 0.9415670800000000 | 0.9306175900000000 | 1.0 |
| H5  | H                      | 0.2542857300000000 | 0.8513968400000000 | 0.0088955400000000 | 1.0 |
| H6  | H                      | 0.2282753900000000 | 0.0540152800000000 | 0.0939770700000000 | 1.0 |
| H7  | H                      | 0.6434952400000000 | 0.9208369700000000 | 0.9392859000000000 | 1.0 |
| H8  | H                      | 0.4875712400000000 | 0.8513540100000000 | 0.0085332400000000 | 1.0 |
| H9  | H                      | 0.5135990200000000 | 0.0537924300000000 | 0.0940879800000000 | 1.0 |
| H10 | H                      | 0.8710445100000000 | 0.9349711100000000 | 0.9422817900000000 | 1.0 |
| H11 | H                      | 0.7621476400000000 | 0.8646692700000000 | 0.0431315800000000 | 1.0 |
| H12 | H                      | 0.7240025300000000 | 0.0824457600000000 | 0.0717750500000000 | 1.0 |
| C13 | C                      | 0.0004854900000000 | 0.0342552500000000 | 0.0480355100000000 | 1.0 |
| C14 | C                      | 0.1240539500000000 | 0.0110384300000000 | 0.0034657300000000 | 1.0 |
| C15 | C                      | 0.1148673800000000 | 0.9341636900000000 | 0.9918117200000000 | 1.0 |
| C16 | C                      | 0.9921265700000000 | 0.9180407100000000 | 0.0318464500000000 | 1.0 |
| C17 | C                      | 0.1310262000000000 | 0.0359642600000000 | 0.9289151100000000 | 1.0 |
| C18 | C                      | 0.2423720200000000 | 0.0140395500000000 | 0.0574922700000000 | 1.0 |
| C19 | C                      | 0.3709192300000000 | 0.0169981200000000 | 0.0194743800000000 | 1.0 |
| C20 | C                      | 0.3708738100000000 | 0.9420323200000000 | 0.9850413100000000 | 1.0 |
| C21 | C                      | 0.2482151800000000 | 0.9059367500000000 | 0.0144078600000000 | 1.0 |
| C22 | C                      | 0.3709735500000000 | 0.0927027900000000 | 0.9898671300000000 | 1.0 |
| C23 | C                      | 0.4994291000000000 | 0.0139065300000000 | 0.0575105200000000 | 1.0 |
| C24 | C                      | 0.6177689700000000 | 0.0109981600000000 | 0.0034551100000000 | 1.0 |
| C25 | C                      | 0.6269985800000000 | 0.9341477600000000 | 0.9916812200000000 | 1.0 |
| C26 | C                      | 0.4936451800000000 | 0.9058774200000000 | 0.0142092000000000 | 1.0 |
| C27 | C                      | 0.6107272200000000 | 0.0359554300000000 | 0.9288896100000000 | 1.0 |
| C28 | C                      | 0.7413316400000000 | 0.0341828300000000 | 0.0480547800000000 | 1.0 |
| C29 | C                      | 0.8708983100000000 | 0.0298630800000000 | 0.0091113300000000 | 1.0 |
| C30 | C                      | 0.8709385900000000 | 0.9477852400000000 | 0.9955696300000000 | 1.0 |
| C31 | C                      | 0.7496923400000000 | 0.9179809700000000 | 0.0317329600000000 | 1.0 |
| C32 | C                      | 0.8708280600000000 | 0.0996583000000000 | 0.9658165200000000 | 1.0 |
| F33 | F                      | 0.1374730100000000 | 0.1015591400000000 | 0.9149840000000000 | 1.0 |
| F34 | F                      | 0.0275070800000000 | 0.0127200500000000 | 0.8956018800000000 | 1.0 |
| F35 | F                      | 0.2268071600000000 | 0.0065073200000000 | 0.8943515600000000 | 1.0 |
| F36 | F                      | 0.4700306000000000 | 0.1282543100000000 | 0.0145875300000000 | 1.0 |
| F37 | F                      | 0.2719823000000000 | 0.1283154200000000 | 0.0145874000000000 | 1.0 |
| F38 | F                      | 0.3709255700000000 | 0.1021369100000000 | 0.9234402400000000 | 1.0 |
| F39 | F                      | 0.6041859300000000 | 0.1015371200000000 | 0.9149197800000000 | 1.0 |
| F40 | F                      | 0.5149562100000000 | 0.0064442200000000 | 0.8943543000000000 | 1.0 |
| F41 | F                      | 0.7142675400000000 | 0.0127532100000000 | 0.8955744000000000 | 1.0 |
| F42 | F                      | 0.9691308300000000 | 0.1389580200000000 | 0.9850513300000000 | 1.0 |
| F43 | F                      | 0.7724209300000000 | 0.1388811800000000 | 0.9850455900000000 | 1.0 |
| F44 | F                      | 0.8708609400000000 | 0.1001998900000000 | 0.8985213300000000 | 1.0 |
| S45 | S                      | 0.0005701300000000 | 0.9696551400000000 | 0.1085540700000000 | 1.0 |
| S46 | S                      | 0.2416829700000000 | 0.9326574600000000 | 0.0996324700000000 | 1.0 |
| S47 | S                      | 0.5001609800000000 | 0.9323642400000000 | 0.0994816100000000 | 1.0 |
| S48 | S                      | 0.7411630700000000 | 0.9694873900000000 | 0.1085031500000000 | 1.0 |

##### cif ends

thiophene\_OH\_25\_CF3\_3\_anti\_alt Energy: -332.99243298

##### cif starts

data\_thiophene\_OH\_25\_CF3\_3\_anti\_alt

\_publ\_section\_comment

;  
Andrew Reynoso, Bohan Xu, and Vincent H. Crespi  
;

\_cell\_length\_a 10.0704213604  
\_cell\_length\_b 20.0  
\_cell\_length\_c 20.0  
\_cell\_angle\_alpha 90.0  
\_cell\_angle\_beta 90.0  
\_cell\_angle\_gamma 90.0

\_symmetry\_space\_group\_name\_H-M 'P 1'  
\_symmetry\_Int\_Tables\_number 1  
\_symmetry\_cell\_setting triclinic

loop\_  
\_atom\_site\_label  
\_atom\_site\_type\_symbol  
\_atom\_site\_fract\_x  
\_atom\_site\_fract\_y  
\_atom\_site\_fract\_z  
\_atom\_site\_occupancy  
H1 H 0.0238206700000000 0.0785050500000000 0.0704041000000000 1.0  
H2 H 0.1444112500000000 0.8717049100000000 0.9565095700000000 1.0  
H3 H 0.0911301100000000 0.1740171400000000 0.9246953200000000 1.0  
H4 H 0.2823457200000000 0.9695706900000000 0.9096089300000000 1.0  
H5 H 0.4136689300000000 0.1743297000000000 0.0190408900000000 1.0  
H6 H 0.3203484500000000 0.8776395900000000 0.0635492100000000 1.0  
H7 H 0.5382831000000000 0.0743972800000000 0.0682499600000000 1.0  
H8 H 0.6427424600000000 0.8637630000000000 0.9643814600000000 1.0  
H9 H 0.5942744600000000 0.1632866700000000 0.9165751000000000 1.0  
H10 H 0.7820201700000000 0.9583725400000000 0.9124067300000000 1.0  
H11 H 0.9082162700000000 0.1723708200000000 0.0085341200000000 1.0  
H12 H 0.8209186700000000 0.8810341500000000 0.0729622700000000 1.0  
C13 C 0.0923716800000000 0.9638169300000000 0.9579496700000000 1.0  
C14 C 0.9945277900000000 0.9784744900000000 0.0216932900000000 1.0  
C15 C 0.9970428600000000 0.0567716900000000 0.0219073600000000 1.0  
C16 C 0.0904418600000000 0.0839856300000000 0.9662019600000000 1.0  
C17 C 0.0276772700000000 0.9321496300000000 0.0857039000000000 1.0  
C18 C 0.3495891000000000 0.0842095300000000 0.0204658700000000 1.0  
C19 C 0.2485325700000000 0.0690106500000000 0.9582394000000000 1.0  
C20 C 0.2476828900000000 0.9907270100000000 0.9570136000000000 1.0  
C21 C 0.3317338000000000 0.9642378500000000 0.0162767000000000 1.0  
C22 C 0.2802517100000000 0.1158753500000000 0.8937506600000000 1.0  
C23 C 0.5907864600000000 0.9558660900000000 0.9596492600000000 1.0  
C24 C 0.4925130200000000 0.9751149900000000 0.0224028300000000 1.0  
C25 C 0.5005341900000000 0.0531272500000000 0.0215258700000000 1.0  
C26 C 0.5863647400000000 0.0764011800000000 0.9614369600000000 1.0

|     |   |                    |                    |                    |     |
|-----|---|--------------------|--------------------|--------------------|-----|
| C27 | C | 0.5224743400000000 | 0.9301696700000000 | 0.0877224000000000 | 1.0 |
| C28 | C | 0.8419706700000000 | 0.0833161200000000 | 0.0131390000000000 | 1.0 |
| C29 | C | 0.7429607900000000 | 0.0598381800000000 | 0.9521694400000000 | 1.0 |
| C30 | C | 0.7447301300000000 | 0.9828193300000000 | 0.9577970200000000 | 1.0 |
| C31 | C | 0.8307026400000000 | 0.9632936900000000 | 0.0183417600000000 | 1.0 |
| C32 | C | 0.7744200000000000 | 0.0883555600000000 | 0.8782548000000000 | 1.0 |
| O33 | O | 0.0830215400000000 | 0.8997002400000000 | 0.9309337300000000 | 1.0 |
| O34 | O | 0.0597665500000000 | 0.1520947300000000 | 0.9651816800000000 | 1.0 |
| O35 | O | 0.3478646300000000 | 0.1495079600000000 | 0.0451184500000000 | 1.0 |
| O36 | O | 0.2894800800000000 | 0.8982826300000000 | 0.0222835600000000 | 1.0 |
| O37 | O | 0.5817350200000000 | 0.8900612900000000 | 0.9369257500000000 | 1.0 |
| O38 | O | 0.5538402200000000 | 0.1435587100000000 | 0.9562246200000000 | 1.0 |
| O39 | O | 0.8295564400000000 | 0.1510033300000000 | 0.0283851600000000 | 1.0 |
| O40 | O | 0.7922677500000000 | 0.8974570300000000 | 0.0294807100000000 | 1.0 |
| F41 | F | 0.0375029800000000 | 0.8673369800000000 | 0.0632329300000000 | 1.0 |
| F42 | F | 0.9272026700000000 | 0.9298004400000000 | 0.1333227700000000 | 1.0 |
| F43 | F | 0.1356531100000000 | 0.9413481300000000 | 0.1250128800000000 | 1.0 |
| F44 | F | 0.3083502900000000 | 0.1792322000000000 | 0.9165557400000000 | 1.0 |
| F45 | F | 0.1736706300000000 | 0.1270199600000000 | 0.8509666400000000 | 1.0 |
| F46 | F | 0.3784575900000000 | 0.0999802900000000 | 0.8506386400000000 | 1.0 |
| F47 | F | 0.5416609700000000 | 0.8651657000000000 | 0.0670835600000000 | 1.0 |
| F48 | F | 0.4179780300000000 | 0.9242932300000000 | 0.1325334300000000 | 1.0 |
| F49 | F | 0.6254415300000000 | 0.9447720500000000 | 0.1286494000000000 | 1.0 |
| F50 | F | 0.8762094200000000 | 0.1334166300000000 | 0.8776533300000000 | 1.0 |
| F51 | F | 0.6719570500000000 | 0.1262587600000000 | 0.8493179000000000 | 1.0 |
| F52 | F | 0.7980308700000000 | 0.0416355400000000 | 0.8309061500000000 | 1.0 |
| S53 | S | 0.0335347800000000 | 0.0239088600000000 | 0.8973922900000000 | 1.0 |
| S54 | S | 0.2816756500000000 | 0.0296950900000000 | 0.0825608300000000 | 1.0 |
| S55 | S | 0.5268694700000000 | 0.0113560500000000 | 0.8962633500000000 | 1.0 |
| S56 | S | 0.7785502800000000 | 0.0314792700000000 | 0.0798959900000000 | 1.0 |

##### cif ends

thiophene\_OH\_25\_CF3\_3\_anti\_alt\_forbid Energy: -333.16867726

##### cif starts

data\_thiophene\_OH\_25\_CF3\_3\_anti\_alt\_forbid

\_publ\_section\_comment

;  
Andrew Reynoso, Bohan Xu, and Vincent H. Crespi  
;

\_cell\_length\_a 10.7061719578

\_cell\_length\_b 20.0

\_cell\_length\_c 20.0

\_cell\_angle\_alpha 90.0

\_cell\_angle\_beta 90.0

\_cell\_angle\_gamma 90.0

\_symmetry\_space\_group\_name\_H-M 'P 1'

\_symmetry\_Int\_Tables\_number 1

\_symmetry\_cell\_setting triclinic

loop\_

\_atom\_site\_label

|     | _atom_site_type_symbol | _atom_site_fract_x | _atom_site_fract_y | _atom_site_fract_z | _atom_site_occupancy |
|-----|------------------------|--------------------|--------------------|--------------------|----------------------|
| H1  | H                      | 0.9494772600000000 | 0.9336060500000000 | 0.0565205000000000 | 1.0                  |
| H2  | H                      | 0.3352999700000000 | 0.0575033100000000 | 0.9146810200000000 | 1.0                  |
| H3  | H                      | 0.4497016900000000 | 0.9335454800000000 | 0.0564723800000000 | 1.0                  |
| H4  | H                      | 0.8354214100000000 | 0.0575409100000000 | 0.9146242000000000 | 1.0                  |
| H5  | H                      | 0.1725702200000000 | 0.8392956000000000 | 0.0196317700000000 | 1.0                  |
| H6  | H                      | 0.6728448800000000 | 0.8392789600000000 | 0.0193900100000000 | 1.0                  |
| H7  | H                      | 0.1123609700000000 | 0.1517916800000000 | 0.9515981900000000 | 1.0                  |
| H8  | H                      | 0.6123358300000000 | 0.1518056300000000 | 0.9515124000000000 | 1.0                  |
| H9  | H                      | 0.1007767600000000 | 0.8552484300000000 | 0.9093828300000000 | 1.0                  |
| H10 | H                      | 0.6008529600000000 | 0.8554239000000000 | 0.9090520100000000 | 1.0                  |
| H11 | H                      | 0.1838828800000000 | 0.1357553000000000 | 0.0619528000000000 | 1.0                  |
| H12 | H                      | 0.6838806000000000 | 0.1358282000000000 | 0.0617902800000000 | 1.0                  |
| C13 | C                      | 0.9542517300000000 | 0.0881065000000000 | 0.0693741500000000 | 1.0                  |
| C14 | C                      | 0.3305514100000000 | 0.9030136800000000 | 0.9018294800000000 | 1.0                  |
| C15 | C                      | 0.4543612400000000 | 0.0880749800000000 | 0.0693636800000000 | 1.0                  |
| C16 | C                      | 0.8307166400000000 | 0.9030585800000000 | 0.9017481300000000 | 1.0                  |
| C17 | C                      | 0.0752374300000000 | 0.0586991600000000 | 0.9620647700000000 | 1.0                  |
| C18 | C                      | 0.9553326600000000 | 0.0377650100000000 | 0.0067966300000000 | 1.0                  |
| C19 | C                      | 0.9585290400000000 | 0.9579252400000000 | 0.0075769700000000 | 1.0                  |
| C20 | C                      | 0.0787052700000000 | 0.9326918900000000 | 0.9686811400000000 | 1.0                  |
| C21 | C                      | 0.2062131200000000 | 0.0584024200000000 | 0.0025880500000000 | 1.0                  |
| C22 | C                      | 0.3263639700000000 | 0.0331990200000000 | 0.9636382800000000 | 1.0                  |
| C23 | C                      | 0.3295641700000000 | 0.9533565200000000 | 0.9643967500000000 | 1.0                  |
| C24 | C                      | 0.2097212300000000 | 0.9323875900000000 | 0.0091764900000000 | 1.0                  |
| C25 | C                      | 0.5751969100000000 | 0.0587153700000000 | 0.9620009800000000 | 1.0                  |
| C26 | C                      | 0.4553741700000000 | 0.0377358100000000 | 0.0067860300000000 | 1.0                  |
| C27 | C                      | 0.4585902500000000 | 0.9578860800000000 | 0.0075300500000000 | 1.0                  |
| C28 | C                      | 0.5787465400000000 | 0.9327154500000000 | 0.9685430100000000 | 1.0                  |
| C29 | C                      | 0.7062250600000000 | 0.0584261100000000 | 0.0024878100000000 | 1.0                  |
| C30 | C                      | 0.8264066400000000 | 0.0332253500000000 | 0.9635716200000000 | 1.0                  |
| C31 | C                      | 0.8296329900000000 | 0.9533839600000000 | 0.9643368500000000 | 1.0                  |
| C32 | C                      | 0.7097304000000000 | 0.9324139300000000 | 0.0090620100000000 | 1.0                  |
| O33 | O                      | 0.0614908100000000 | 0.1189209600000000 | 0.9271604800000000 | 1.0                  |
| O34 | O                      | 0.0573931600000000 | 0.8653297100000000 | 0.9510967900000000 | 1.0                  |
| O35 | O                      | 0.2273932400000000 | 0.1257528300000000 | 0.0202572800000000 | 1.0                  |
| O36 | O                      | 0.2234884000000000 | 0.8721535900000000 | 0.0440573200000000 | 1.0                  |
| O37 | O                      | 0.5613565900000000 | 0.1189480400000000 | 0.9271261000000000 | 1.0                  |
| O38 | O                      | 0.5576014500000000 | 0.8653702300000000 | 0.9508357100000000 | 1.0                  |
| O39 | O                      | 0.7274490700000000 | 0.1257812700000000 | 0.0201229200000000 | 1.0                  |
| O40 | O                      | 0.7234581400000000 | 0.8721763000000000 | 0.0439412900000000 | 1.0                  |
| F41 | F                      | 0.4221907600000000 | 0.9075003600000000 | 0.8552715600000000 | 1.0                  |
| F42 | F                      | 0.2255590200000000 | 0.9022418100000000 | 0.8603716500000000 | 1.0                  |
| F43 | F                      | 0.3315618000000000 | 0.8392498000000000 | 0.9265906300000000 | 1.0                  |
| F44 | F                      | 0.9225996000000000 | 0.9074068900000000 | 0.8553135400000000 | 1.0                  |
| F45 | F                      | 0.7259204000000000 | 0.9024908400000000 | 0.8601646400000000 | 1.0                  |
| F46 | F                      | 0.8313253300000000 | 0.8392704300000000 | 0.9264662200000000 | 1.0                  |
| F47 | F                      | 0.0590830300000000 | 0.0887147500000000 | 0.1109409900000000 | 1.0                  |
| F48 | F                      | 0.8624026500000000 | 0.0837294500000000 | 0.1158122800000000 | 1.0                  |
| F49 | F                      | 0.9535746500000000 | 0.1518971700000000 | 0.0446596900000000 | 1.0                  |
| F50 | F                      | 0.5592859900000000 | 0.0887688300000000 | 0.1108663800000000 | 1.0                  |



|     |   |                    |                    |                    |     |
|-----|---|--------------------|--------------------|--------------------|-----|
| F51 | F | 0.3626316200000000 | 0.0836325900000000 | 0.1158574600000000 | 1.0 |
| F52 | F | 0.4535049300000000 | 0.1518631700000000 | 0.0446426200000000 | 1.0 |
| S53 | S | 0.0861007200000000 | 0.9955920000000000 | 0.8994858400000000 | 1.0 |
| S54 | S | 0.1988860900000000 | 0.9954869000000000 | 0.0717625500000000 | 1.0 |
| S55 | S | 0.5860061500000000 | 0.9956400700000000 | 0.8993965300000000 | 1.0 |
| S56 | S | 0.6988900500000000 | 0.9954990200000000 | 0.0716635800000000 | 1.0 |

##### cif ends

thiophene\_OH\_25\_CF3\_3\_anti\_dir    Energy: -332.17139158

##### cif starts

data\_thiophene\_OH\_25\_CF3\_3\_anti\_dir

\_publ\_section\_comment

;  
Andrew Reynoso, Bohan Xu, and Vincent H. Crespi  
;

\_cell\_length\_a    10.0957153095

\_cell\_length\_b    20.0

\_cell\_length\_c    20.0

\_cell\_angle\_alpha    90.0

\_cell\_angle\_beta    90.0

\_cell\_angle\_gamma    90.0

\_symmetry\_space\_group\_name\_H-M    'P 1'

\_symmetry\_Int\_Tables\_number 1

\_symmetry\_cell\_setting triclinic

loop\_

\_atom\_site\_label

\_atom\_site\_type\_symbol

\_atom\_site\_fract\_x

\_atom\_site\_fract\_y

\_atom\_site\_fract\_z

\_atom\_site\_occupancy

|     |   |                    |                    |                    |     |
|-----|---|--------------------|--------------------|--------------------|-----|
| H1  | H | 0.0047475600000000 | 0.9241128700000000 | 0.0723895800000000 | 1.0 |
| H2  | H | 0.0471566100000000 | 0.1179883800000000 | 0.8998599400000000 | 1.0 |
| H3  | H | 0.1491643100000000 | 0.8330696900000000 | 0.9798749400000000 | 1.0 |
| H4  | H | 0.2547202600000000 | 0.9242156300000000 | 0.9081055900000000 | 1.0 |
| H5  | H | 0.2972699800000000 | 0.1178862200000000 | 0.0808661600000000 | 1.0 |
| H6  | H | 0.3991369600000000 | 0.8330363000000000 | 0.0004971000000000 | 1.0 |
| H7  | H | 0.5047286800000000 | 0.9240942600000000 | 0.0723847200000000 | 1.0 |
| H8  | H | 0.5471092200000000 | 0.1179724500000000 | 0.8998544700000000 | 1.0 |
| H9  | H | 0.6492003900000000 | 0.8330742900000000 | 0.9799080100000000 | 1.0 |
| H10 | H | 0.7547558600000000 | 0.9242239800000000 | 0.9081244000000000 | 1.0 |
| H11 | H | 0.7973023100000000 | 0.1179093700000000 | 0.0808688800000000 | 1.0 |
| H12 | H | 0.8991188500000000 | 0.8330461100000000 | 0.0005416400000000 | 1.0 |
| C13 | C | 0.0538422400000000 | 0.0412856900000000 | 0.9604502400000000 | 1.0 |
| C14 | C | 0.9690506900000000 | 0.0234067400000000 | 0.0244322600000000 | 1.0 |
| C15 | C | 0.9776742800000000 | 0.9456360700000000 | 0.0238389800000000 | 1.0 |
| C16 | C | 0.0765806400000000 | 0.9216434900000000 | 0.9669489200000000 | 1.0 |
| C17 | C | 0.0034068000000000 | 0.0680827700000000 | 0.0901009100000000 | 1.0 |
| C18 | C | 0.3038573800000000 | 0.0412408100000000 | 0.0202007400000000 | 1.0 |
| C19 | C | 0.2190393500000000 | 0.0234468300000000 | 0.9561991300000000 | 1.0 |

|     |   |                    |                    |                    |     |
|-----|---|--------------------|--------------------|--------------------|-----|
| C20 | C | 0.2276644600000000 | 0.9456747900000000 | 0.9566869900000000 | 1.0 |
| C21 | C | 0.3265904100000000 | 0.9216058100000000 | 0.0135410700000000 | 1.0 |
| C22 | C | 0.2533521000000000 | 0.0682044500000000 | 0.8905830100000000 | 1.0 |
| C23 | C | 0.5538352800000000 | 0.0412804400000000 | 0.9604541300000000 | 1.0 |
| C24 | C | 0.4690410300000000 | 0.0233951100000000 | 0.0244324900000000 | 1.0 |
| C25 | C | 0.4776738900000000 | 0.9456247700000000 | 0.0238344500000000 | 1.0 |
| C26 | C | 0.5766042000000000 | 0.9216401100000000 | 0.9669531900000000 | 1.0 |
| C27 | C | 0.5033766300000000 | 0.0680721500000000 | 0.0901046600000000 | 1.0 |
| C28 | C | 0.8038586400000000 | 0.0412572000000000 | 0.0202101500000000 | 1.0 |
| C29 | C | 0.7190399900000000 | 0.0234563800000000 | 0.9562114900000000 | 1.0 |
| C30 | C | 0.7276781500000000 | 0.9456828700000000 | 0.9567028700000000 | 1.0 |
| C31 | C | 0.8265904000000000 | 0.9216207900000000 | 0.0135632200000000 | 1.0 |
| C32 | C | 0.7533503100000000 | 0.0682228600000000 | 0.8905989400000000 | 1.0 |
| O33 | O | 0.0171361700000000 | 0.1049372500000000 | 0.9442492700000000 | 1.0 |
| O34 | O | 0.0661071700000000 | 0.8509945200000000 | 0.9606033300000000 | 1.0 |
| O35 | O | 0.2671691500000000 | 0.1048730400000000 | 0.0364788300000000 | 1.0 |
| O36 | O | 0.3161044800000000 | 0.8509479100000000 | 0.0198064100000000 | 1.0 |
| O37 | O | 0.5171068600000000 | 0.1049272700000000 | 0.9442497100000000 | 1.0 |
| O38 | O | 0.5661606400000000 | 0.8509898400000000 | 0.9606073900000000 | 1.0 |
| O39 | O | 0.7671803300000000 | 0.1048925200000000 | 0.0364869600000000 | 1.0 |
| O40 | O | 0.8160944100000000 | 0.8509632200000000 | 0.0198522600000000 | 1.0 |
| F41 | F | 0.0165797800000000 | 0.1332059000000000 | 0.0720209900000000 | 1.0 |
| F42 | F | 0.1093735100000000 | 0.0536116500000000 | 0.1292775200000000 | 1.0 |
| F43 | F | 0.9027155300000000 | 0.0684869600000000 | 0.1377121000000000 | 1.0 |
| F44 | F | 0.2664909900000000 | 0.1333089500000000 | 0.9087274700000000 | 1.0 |
| F45 | F | 0.1526582900000000 | 0.0686465600000000 | 0.8429726200000000 | 1.0 |
| F46 | F | 0.3593205400000000 | 0.0537779200000000 | 0.8513888600000000 | 1.0 |
| F47 | F | 0.5165141100000000 | 0.1331977200000000 | 0.0720245100000000 | 1.0 |
| F48 | F | 0.6093482500000000 | 0.0536191800000000 | 0.1292832800000000 | 1.0 |
| F49 | F | 0.4026811900000000 | 0.0684580800000000 | 0.1377132600000000 | 1.0 |
| F50 | F | 0.7664640000000000 | 0.1333260700000000 | 0.9087510200000000 | 1.0 |
| F51 | F | 0.6526630300000000 | 0.0686611200000000 | 0.8429849900000000 | 1.0 |
| F52 | F | 0.8593268200000000 | 0.0538100700000000 | 0.8514052800000000 | 1.0 |
| S53 | S | 0.0062525600000000 | 0.9685549100000000 | 0.8990248000000000 | 1.0 |
| S54 | S | 0.2562728300000000 | 0.9684225200000000 | 0.0815303300000000 | 1.0 |
| S55 | S | 0.5062778500000000 | 0.9685454700000000 | 0.8990250500000000 | 1.0 |
| S56 | S | 0.7562804200000000 | 0.9684474000000000 | 0.0815445400000000 | 1.0 |

##### cif ends

thiophene\_OH\_25\_CF3\_3\_anti\_dir\_forbid    Energy: -332.48136637

##### cif starts

data\_thiophene\_OH\_25\_CF3\_3\_anti\_dir\_forbid

\_publ\_section\_comment

;  
Andrew Reynoso, Bohan Xu, and Vincent H. Crespi  
;

\_cell\_length\_a    10.7418825822

\_cell\_length\_b    20.0

\_cell\_length\_c    20.0

\_cell\_angle\_alpha    90.0

\_cell\_angle\_beta    90.0

\_cell\_angle\_gamma    90.0

\_symmetry\_space\_group\_name\_H-M 'P 1'

\_symmetry\_Int\_Tables\_number 1

\_symmetry\_cell\_setting triclinic

loop\_

\_atom\_site\_label

\_atom\_site\_type\_symbol

\_atom\_site\_fract\_x

\_atom\_site\_fract\_y

\_atom\_site\_fract\_z

\_atom\_site\_occupancy

|     |   |                    |                    |                    |     |
|-----|---|--------------------|--------------------|--------------------|-----|
| H1  | H | 0.1417320700000000 | 0.0627745800000000 | 0.0686415600000000 | 1.0 |
| H2  | H | 0.2493823300000000 | 0.0729821600000000 | 0.9292925900000000 | 1.0 |
| H3  | H | 0.6416999200000000 | 0.0629208900000000 | 0.0686117900000000 | 1.0 |
| H4  | H | 0.7493349700000000 | 0.0731373900000000 | 0.9292745000000000 | 1.0 |
| H5  | H | 0.9551741200000000 | 0.8567283700000000 | 0.9454904200000000 | 1.0 |
| H6  | H | 0.4556290500000000 | 0.8566318900000000 | 0.9454125800000000 | 1.0 |
| H7  | H | 0.4068860400000000 | 0.8538067400000000 | 0.0505045000000000 | 1.0 |
| H8  | H | 0.9064944500000000 | 0.8539509400000000 | 0.0505468700000000 | 1.0 |
| H9  | H | 0.9856130800000000 | 0.1531418400000000 | 0.9291763400000000 | 1.0 |
| H10 | H | 0.4097021800000000 | 0.1569387500000000 | 0.0405609900000000 | 1.0 |
| H11 | H | 0.4852262600000000 | 0.1530439600000000 | 0.9290969200000000 | 1.0 |
| H12 | H | 0.9098973900000000 | 0.1569785400000000 | 0.0405935000000000 | 1.0 |
| C13 | C | 0.0086964900000000 | 0.0716196300000000 | 0.9834747400000000 | 1.0 |
| C14 | C | 0.1295444000000000 | 0.0423698200000000 | 0.0182831300000000 | 1.0 |
| C15 | C | 0.1255523100000000 | 0.9639094500000000 | 0.0142460200000000 | 1.0 |
| C16 | C | 0.0068773700000000 | 0.9447348900000000 | 0.9692876300000000 | 1.0 |
| C17 | C | 0.3732146200000000 | 0.0652036600000000 | 0.0207981000000000 | 1.0 |
| C18 | C | 0.2552324200000000 | 0.0440403600000000 | 0.9757283700000000 | 1.0 |
| C19 | C | 0.2552750900000000 | 0.9649793900000000 | 0.9670795900000000 | 1.0 |
| C20 | C | 0.3730292000000000 | 0.9386155600000000 | 0.0059607500000000 | 1.0 |
| C21 | C | 0.5085844000000000 | 0.0715874900000000 | 0.9834662400000000 | 1.0 |
| C22 | C | 0.6295311400000000 | 0.0424655200000000 | 0.0182737900000000 | 1.0 |
| C23 | C | 0.6256313800000000 | 0.9640083500000000 | 0.0142957200000000 | 1.0 |
| C24 | C | 0.5070810500000000 | 0.9446475000000000 | 0.9694871600000000 | 1.0 |
| C25 | C | 0.8732411200000000 | 0.0652786400000000 | 0.0207550900000000 | 1.0 |
| C26 | C | 0.7551958300000000 | 0.0441598700000000 | 0.9756833100000000 | 1.0 |
| C27 | C | 0.7551821200000000 | 0.9651036100000000 | 0.9669930800000000 | 1.0 |
| C28 | C | 0.8729312600000000 | 0.9387226500000000 | 0.0058432200000000 | 1.0 |
| C29 | C | 0.1274226600000000 | 0.9289257300000000 | 0.0884413600000000 | 1.0 |
| C30 | C | 0.2522557100000000 | 0.9268290700000000 | 0.8948587600000000 | 1.0 |
| C31 | C | 0.6276222600000000 | 0.9290258200000000 | 0.0884978900000000 | 1.0 |
| C32 | C | 0.7521095100000000 | 0.9270424600000000 | 0.8946601300000000 | 1.0 |
| O33 | O | 0.0314647800000000 | 0.1407003300000000 | 0.9694419400000000 | 1.0 |
| O34 | O | 0.3483359700000000 | 0.1240984000000000 | 0.0564548000000000 | 1.0 |
| O35 | O | 0.5311704000000000 | 0.1406720000000000 | 0.9693526700000000 | 1.0 |
| O36 | O | 0.8484054300000000 | 0.1241721900000000 | 0.0564177200000000 | 1.0 |
| O37 | O | 0.0286518100000000 | 0.8851984900000000 | 0.9375519300000000 | 1.0 |
| O38 | O | 0.3516076700000000 | 0.8699326800000000 | 0.0153575600000000 | 1.0 |
| O39 | O | 0.5294324400000000 | 0.8850011700000000 | 0.9380739100000000 | 1.0 |
| O40 | O | 0.8514866900000000 | 0.8700301300000000 | 0.0152583700000000 | 1.0 |
| F41 | F | 0.3576688300000000 | 0.9353416900000000 | 0.8570494600000000 | 1.0 |
| F42 | F | 0.1614369200000000 | 0.9440767200000000 | 0.8513040500000000 | 1.0 |
| F43 | F | 0.2464013200000000 | 0.8592992800000000 | 0.9036388300000000 | 1.0 |

|     |   |                    |                    |                    |     |
|-----|---|--------------------|--------------------|--------------------|-----|
| F44 | F | 0.8570121400000000 | 0.9361814900000000 | 0.8566142200000000 | 1.0 |
| F45 | F | 0.6606392900000000 | 0.9438570700000000 | 0.8513188300000000 | 1.0 |
| F46 | F | 0.7473737600000000 | 0.8594688400000000 | 0.9033306400000000 | 1.0 |
| F47 | F | 0.2243631300000000 | 0.8902854300000000 | 0.1080550600000000 | 1.0 |
| F48 | F | 0.0295359300000000 | 0.8836612200000000 | 0.0975833100000000 | 1.0 |
| F49 | F | 0.1159054700000000 | 0.9747589000000000 | 0.1379922300000000 | 1.0 |
| F50 | F | 0.7245827700000000 | 0.8903895100000000 | 0.1081186500000000 | 1.0 |
| F51 | F | 0.5297631900000000 | 0.8837558200000000 | 0.0976490900000000 | 1.0 |
| F52 | F | 0.6161027700000000 | 0.9748739300000000 | 0.1380307000000000 | 1.0 |
| S53 | S | 0.9984159200000000 | 0.0216075400000000 | 0.9100450100000000 | 1.0 |
| S54 | S | 0.3787863200000000 | 0.9954443200000000 | 0.0796485000000000 | 1.0 |
| S55 | S | 0.4982993100000000 | 0.0214903400000000 | 0.9100776100000000 | 1.0 |
| S56 | S | 0.8787615900000000 | 0.9954878400000000 | 0.0795599900000000 | 1.0 |

##### cif ends

thiophene\_OH\_25\_CF3\_3\_syn\_alt    Energy: -335.99839965

##### cif starts

data\_thiophene\_OH\_25\_CF3\_3\_syn\_alt

\_publ\_section\_comment

;  
Andrew Reynoso, Bohan Xu, and Vincent H. Crespi  
;

\_cell\_length\_a    10.6654832138

\_cell\_length\_b    20.0

\_cell\_length\_c    20.0

\_cell\_angle\_alpha    90.0

\_cell\_angle\_beta    90.0

\_cell\_angle\_gamma    90.0

\_symmetry\_space\_group\_name\_H-M    'P 1'

\_symmetry\_Int\_Tables\_number 1

\_symmetry\_cell\_setting triclinic

loop\_

\_atom\_site\_label

\_atom\_site\_type\_symbol

\_atom\_site\_fract\_x

\_atom\_site\_fract\_y

\_atom\_site\_fract\_z

\_atom\_site\_occupancy

|     |   |                    |                    |                    |     |
|-----|---|--------------------|--------------------|--------------------|-----|
| H1  | H | 0.1909225400000000 | 0.0592037000000000 | 0.9332166300000000 | 1.0 |
| H2  | H | 0.9718488200000000 | 0.8620055500000000 | 0.0532339100000000 | 1.0 |
| H3  | H | 0.9825602400000000 | 0.1484093000000000 | 0.0424065000000000 | 1.0 |
| H4  | H | 0.4409575100000000 | 0.9391983600000000 | 0.9330607800000000 | 1.0 |
| H5  | H | 0.2218694300000000 | 0.1361014500000000 | 0.0535076900000000 | 1.0 |
| H6  | H | 0.2325137100000000 | 0.8497182900000000 | 0.0420396200000000 | 1.0 |
| H7  | H | 0.6908758400000000 | 0.0591705400000000 | 0.9332260800000000 | 1.0 |
| H8  | H | 0.4717815800000000 | 0.8619512400000000 | 0.0531017500000000 | 1.0 |
| H9  | H | 0.4825543800000000 | 0.1483701900000000 | 0.0424948400000000 | 1.0 |
| H10 | H | 0.9408822600000000 | 0.9391571700000000 | 0.9331308200000000 | 1.0 |
| H11 | H | 0.7218810700000000 | 0.1361726800000000 | 0.0534258600000000 | 1.0 |
| H12 | H | 0.7324883500000000 | 0.8497999800000000 | 0.0422662400000000 | 1.0 |

|     |   |                    |                    |                    |     |
|-----|---|--------------------|--------------------|--------------------|-----|
| C13 | C | 0.0533779100000000 | 0.9447588900000000 | 0.0261551600000000 | 1.0 |
| C14 | C | 0.1761281400000000 | 0.9592677400000000 | 0.9811841000000000 | 1.0 |
| C15 | C | 0.1813789000000000 | 0.0369796700000000 | 0.9826019500000000 | 1.0 |
| C16 | C | 0.0553298300000000 | 0.0632251800000000 | 0.0163246800000000 | 1.0 |
| C17 | C | 0.1631892800000000 | 0.9242423700000000 | 0.9116498400000000 | 1.0 |
| C18 | C | 0.3033655600000000 | 0.0533930400000000 | 0.0262716100000000 | 1.0 |
| C19 | C | 0.4261445200000000 | 0.0390002100000000 | 0.9812954100000000 | 1.0 |
| C20 | C | 0.4313855300000000 | 0.9612833000000000 | 0.9825073200000000 | 1.0 |
| C21 | C | 0.3053113600000000 | 0.9349574900000000 | 0.0161520500000000 | 1.0 |
| C22 | C | 0.4132260300000000 | 0.0742120300000000 | 0.9118550000000000 | 1.0 |
| C23 | C | 0.5533376300000000 | 0.9447441600000000 | 0.0261550900000000 | 1.0 |
| C24 | C | 0.6761503600000000 | 0.9592557800000000 | 0.9812395100000000 | 1.0 |
| C25 | C | 0.6813723400000000 | 0.0369718500000000 | 0.9826245000000000 | 1.0 |
| C26 | C | 0.5553274800000000 | 0.0632063600000000 | 0.0163537400000000 | 1.0 |
| C27 | C | 0.6632766600000000 | 0.9241933600000000 | 0.9117131200000000 | 1.0 |
| C28 | C | 0.8033767600000000 | 0.0534367100000000 | 0.0262655800000000 | 1.0 |
| C29 | C | 0.9261443400000000 | 0.0389999700000000 | 0.9812919500000000 | 1.0 |
| C30 | C | 0.9313753500000000 | 0.9612811700000000 | 0.9825622000000000 | 1.0 |
| C31 | C | 0.8053146300000000 | 0.9349957700000000 | 0.0162604400000000 | 1.0 |
| C32 | C | 0.9131970200000000 | 0.0741510400000000 | 0.9118218700000000 | 1.0 |
| O33 | O | 0.0574580500000000 | 0.8813208200000000 | 0.0538217000000000 | 1.0 |
| O34 | O | 0.0629358400000000 | 0.1334476000000000 | 0.0232517100000000 | 1.0 |
| O35 | O | 0.3074494900000000 | 0.1167526100000000 | 0.0541202200000000 | 1.0 |
| O36 | O | 0.3128804300000000 | 0.8647176900000000 | 0.0229007600000000 | 1.0 |
| O37 | O | 0.5573614000000000 | 0.8812993700000000 | 0.0538166100000000 | 1.0 |
| O38 | O | 0.5629166500000000 | 0.1334264200000000 | 0.0233098700000000 | 1.0 |
| O39 | O | 0.8074719600000000 | 0.1168346600000000 | 0.0540381800000000 | 1.0 |
| O40 | O | 0.8128790800000000 | 0.8647686100000000 | 0.0231345000000000 | 1.0 |
| F41 | F | 0.1010604800000000 | 0.8645594800000000 | 0.9170283600000000 | 1.0 |
| F42 | F | 0.2749780900000000 | 0.9088814700000000 | 0.8825048300000000 | 1.0 |
| F43 | F | 0.0997116800000000 | 0.9616594500000000 | 0.8655320800000000 | 1.0 |
| F44 | F | 0.3512045900000000 | 0.1339076600000000 | 0.9174091600000000 | 1.0 |
| F45 | F | 0.3496528300000000 | 0.0369458200000000 | 0.8656479800000000 | 1.0 |
| F46 | F | 0.5249946400000000 | 0.0896100800000000 | 0.8827179700000000 | 1.0 |
| F47 | F | 0.6009899800000000 | 0.8645573500000000 | 0.9170849200000000 | 1.0 |
| F48 | F | 0.7750753200000000 | 0.9087217600000000 | 0.8826372500000000 | 1.0 |
| F49 | F | 0.5999832100000000 | 0.9616343600000000 | 0.8655414400000000 | 1.0 |
| F50 | F | 0.8510574100000000 | 0.1338178200000000 | 0.9173090300000000 | 1.0 |
| F51 | F | 0.8497022500000000 | 0.0368095100000000 | 0.8656453400000000 | 1.0 |
| F52 | F | 0.0249498200000000 | 0.0895875600000000 | 0.8826892900000000 | 1.0 |
| S53 | S | 0.0554728600000000 | 0.0171438700000000 | 0.0925078800000000 | 1.0 |
| S54 | S | 0.3053884700000000 | 0.9808545100000000 | 0.0924341500000000 | 1.0 |
| S55 | S | 0.5553387800000000 | 0.0170905100000000 | 0.0925157800000000 | 1.0 |
| S56 | S | 0.8054333400000000 | 0.9810071400000000 | 0.0924768400000000 | 1.0 |

##### cif ends

thiophene\_OH\_25\_CF3\_3\_syn\_alt\_forbid Energy: -333.23688094

##### cif starts

data\_thiophene\_OH\_25\_CF3\_3\_syn\_alt\_forbid

\_publ\_section\_comment

;  
 Andrew Reynoso, Bohan Xu, and Vincent H. Crespi  
 ;

\_cell\_length\_a 10.2205537459  
\_cell\_length\_b 20.0  
\_cell\_length\_c 20.0  
\_cell\_angle\_alpha 90.0  
\_cell\_angle\_beta 90.0  
\_cell\_angle\_gamma 90.0

\_symmetry\_space\_group\_name\_H-M 'P 1'  
\_symmetry\_Int\_Tables\_number 1  
\_symmetry\_cell\_setting triclinic

loop\_  
\_atom\_site\_label  
\_atom\_site\_type\_symbol  
\_atom\_site\_fract\_x  
\_atom\_site\_fract\_y  
\_atom\_site\_fract\_z  
\_atom\_site\_occupancy

|     |   |                    |                    |                    |     |
|-----|---|--------------------|--------------------|--------------------|-----|
| H1  | H | 0.9796343200000000 | 0.0513931500000000 | 0.9286284700000000 | 1.0 |
| H2  | H | 0.2575133400000000 | 0.9329367800000000 | 0.9474405700000000 | 1.0 |
| H3  | H | 0.5244753400000000 | 0.0483488200000000 | 0.9445829600000000 | 1.0 |
| H4  | H | 0.7699711900000000 | 0.9425589800000000 | 0.9318145400000000 | 1.0 |
| H5  | H | 0.1857602600000000 | 0.1634665300000000 | 0.0494136800000000 | 1.0 |
| H6  | H | 0.4291709700000000 | 0.8497815800000000 | 0.0713712500000000 | 1.0 |
| H7  | H | 0.6713789400000000 | 0.1317675400000000 | 0.0954076800000000 | 1.0 |
| H8  | H | 0.9287918300000000 | 0.8691803900000000 | 0.0749108800000000 | 1.0 |
| H9  | H | 0.9302245900000000 | 0.1443599400000000 | 0.0565195500000000 | 1.0 |
| H10 | H | 0.4299391700000000 | 0.1250386700000000 | 0.0649245900000000 | 1.0 |
| H11 | H | 0.6941873800000000 | 0.8308663700000000 | 0.0575588300000000 | 1.0 |
| H12 | H | 0.1723740400000000 | 0.8678104500000000 | 0.0969679500000000 | 1.0 |
| C13 | C | 0.0457156200000000 | 0.0702564100000000 | 0.0312918800000000 | 1.0 |
| C14 | C | 0.9576870000000000 | 0.0354590100000000 | 0.9795698100000000 | 1.0 |
| C15 | C | 0.9583195400000000 | 0.9584638300000000 | 0.9873371800000000 | 1.0 |
| C16 | C | 0.0368894100000000 | 0.9483966300000000 | 0.0539689900000000 | 1.0 |
| C17 | C | 0.0117887700000000 | 0.9145386000000000 | 0.9290646000000000 | 1.0 |
| C18 | C | 0.2309541700000000 | 0.0712457200000000 | 0.0319437000000000 | 1.0 |
| C19 | C | 0.3180532000000000 | 0.0364562000000000 | 0.9790626000000000 | 1.0 |
| C20 | C | 0.3027290400000000 | 0.9598490800000000 | 0.9885191800000000 | 1.0 |
| C21 | C | 0.2260564300000000 | 0.9488760700000000 | 0.0536628600000000 | 1.0 |
| C22 | C | 0.2964664300000000 | 0.0680289900000000 | 0.9092741000000000 | 1.0 |
| C23 | C | 0.5464149000000000 | 0.0447310700000000 | 0.0541233800000000 | 1.0 |
| C24 | C | 0.4760333500000000 | 0.0263981400000000 | 0.9876424700000000 | 1.0 |
| C25 | C | 0.4616279700000000 | 0.9489320400000000 | 0.9844195900000000 | 1.0 |
| C26 | C | 0.5468034800000000 | 0.9202968100000000 | 0.0424108100000000 | 1.0 |
| C27 | C | 0.4971657200000000 | 0.9125350600000000 | 0.9171534100000000 | 1.0 |
| C28 | C | 0.7251916600000000 | 0.0489319600000000 | 0.0560796100000000 | 1.0 |
| C29 | C | 0.7986637000000000 | 0.0381362300000000 | 0.9886216100000000 | 1.0 |
| C30 | C | 0.7971575800000000 | 0.9605356800000000 | 0.9814146500000000 | 1.0 |
| C31 | C | 0.7189041700000000 | 0.9250100000000000 | 0.0375235900000000 | 1.0 |
| C32 | C | 0.7525508600000000 | 0.0882382200000000 | 0.9332442600000000 | 1.0 |
| O33 | O | 0.0197406800000000 | 0.1389384800000000 | 0.0387522100000000 | 1.0 |
| O34 | O | 0.0134789500000000 | 0.8895898800000000 | 0.0888979400000000 | 1.0 |
| O35 | O | 0.2669285500000000 | 0.1385522000000000 | 0.0388096600000000 | 1.0 |
| O36 | O | 0.2571957600000000 | 0.8880478800000000 | 0.0828401400000000 | 1.0 |

|     |   |                    |                    |                    |     |
|-----|---|--------------------|--------------------|--------------------|-----|
| O37 | O | 0.5142849300000000 | 0.1065906900000000 | 0.0813873700000000 | 1.0 |
| O38 | O | 0.5223943000000000 | 0.8530154000000000 | 0.0586301300000000 | 1.0 |
| O39 | O | 0.7566680400000000 | 0.1098201200000000 | 0.0855388000000000 | 1.0 |
| O40 | O | 0.7681026700000000 | 0.8591852900000000 | 0.0430607600000000 | 1.0 |
| F41 | F | 0.3737079100000000 | 0.1232626400000000 | 0.9012744700000000 | 1.0 |
| F42 | F | 0.1713414000000000 | 0.0892152700000000 | 0.8986846400000000 | 1.0 |
| F43 | F | 0.3259802700000000 | 0.0253705200000000 | 0.8582830300000000 | 1.0 |
| F44 | F | 0.8487359800000000 | 0.1327813400000000 | 0.9162876400000000 | 1.0 |
| F45 | F | 0.6508095100000000 | 0.1284996700000000 | 0.9522052300000000 | 1.0 |
| F46 | F | 0.7175179200000000 | 0.0568827900000000 | 0.8753921100000000 | 1.0 |
| F47 | F | 0.0875001200000000 | 0.9503471400000000 | 0.8853609600000000 | 1.0 |
| F48 | F | 0.9171708900000000 | 0.8856123100000000 | 0.8906517300000000 | 1.0 |
| F49 | F | 0.0861294000000000 | 0.8624164900000000 | 0.9520751600000000 | 1.0 |
| F50 | F | 0.5491885100000000 | 0.9543200500000000 | 0.8703462900000000 | 1.0 |
| F51 | F | 0.3928970500000000 | 0.8815505600000000 | 0.8879396700000000 | 1.0 |
| F52 | F | 0.5882352200000000 | 0.8632114500000000 | 0.9265338300000000 | 1.0 |
| S53 | S | 0.0082935900000000 | 0.0231904400000000 | 0.1043850800000000 | 1.0 |
| S54 | S | 0.2606293700000000 | 0.0228551000000000 | 0.1055242300000000 | 1.0 |
| S55 | S | 0.5080820200000000 | 0.9745441200000000 | 0.1108000800000000 | 1.0 |
| S56 | S | 0.7641423800000000 | 0.9756992800000000 | 0.1088668500000000 | 1.0 |

##### cif ends

thiophene\_OH\_25\_CH3\_3\_anti\_alt    Energy: -332.11508248

##### cif starts

data\_thiophene\_OH\_25\_CH3\_3\_anti\_alt

\_publ\_section\_comment

;

Andrew Reynoso, Bohan Xu, and Vincent H. Crespi

;

\_cell\_length\_a    9.9254593075

\_cell\_length\_b    20.0

\_cell\_length\_c    20.0

\_cell\_angle\_alpha    90.0

\_cell\_angle\_beta    90.0

\_cell\_angle\_gamma    90.0

\_symmetry\_space\_group\_name\_H-M    'P 1'

\_symmetry\_Int\_Tables\_number 1

\_symmetry\_cell\_setting triclinic

loop\_

\_atom\_site\_label

\_atom\_site\_type\_symbol

\_atom\_site\_fract\_x

\_atom\_site\_fract\_y

\_atom\_site\_fract\_z

\_atom\_site\_occupancy

|    |   |                    |                    |                    |     |
|----|---|--------------------|--------------------|--------------------|-----|
| H1 | H | 0.0806977300000000 | 0.9559715000000000 | 0.1063833600000000 | 1.0 |
|----|---|--------------------|--------------------|--------------------|-----|

|    |   |                    |                    |                    |     |
|----|---|--------------------|--------------------|--------------------|-----|
| H2 | H | 0.9887421800000000 | 0.0776630800000000 | 0.0650900200000000 | 1.0 |
|----|---|--------------------|--------------------|--------------------|-----|

|    |   |                    |                    |                    |     |
|----|---|--------------------|--------------------|--------------------|-----|
| H3 | H | 0.1176440100000000 | 0.8703299300000000 | 0.9605421000000000 | 1.0 |
|----|---|--------------------|--------------------|--------------------|-----|

|    |   |                    |                    |                    |     |
|----|---|--------------------|--------------------|--------------------|-----|
| H4 | H | 0.0781369300000000 | 0.1669460300000000 | 0.9230400200000000 | 1.0 |
|----|---|--------------------|--------------------|--------------------|-----|

|    |   |                    |                    |                    |     |
|----|---|--------------------|--------------------|--------------------|-----|
| H5 | H | 0.9104465800000000 | 0.9424333800000000 | 0.1224962100000000 | 1.0 |
|----|---|--------------------|--------------------|--------------------|-----|

|     |   |                    |                    |                    |     |
|-----|---|--------------------|--------------------|--------------------|-----|
| H6  | H | 0.0056288000000000 | 0.8861227800000000 | 0.0699335600000000 | 1.0 |
| H7  | H | 0.3311282200000000 | 0.0871117000000000 | 0.8723735800000000 | 1.0 |
| H8  | H | 0.2387333200000000 | 0.9650939800000000 | 0.9134272800000000 | 1.0 |
| H9  | H | 0.3677481400000000 | 0.1723997800000000 | 0.0179163500000000 | 1.0 |
| H10 | H | 0.3281026200000000 | 0.8758067700000000 | 0.0555001100000000 | 1.0 |
| H11 | H | 0.1607991200000000 | 0.1001005500000000 | 0.8559363400000000 | 1.0 |
| H12 | H | 0.2549686700000000 | 0.1567367700000000 | 0.9086112500000000 | 1.0 |
| H13 | H | 0.5809575600000000 | 0.9557809500000000 | 0.1062463700000000 | 1.0 |
| H14 | H | 0.4887741100000000 | 0.0776473200000000 | 0.0650855100000000 | 1.0 |
| H15 | H | 0.6176617000000000 | 0.8703260200000000 | 0.9605099200000000 | 1.0 |
| H16 | H | 0.5781262100000000 | 0.1669466900000000 | 0.9230462200000000 | 1.0 |
| H17 | H | 0.4106698300000000 | 0.9425230600000000 | 0.1225392900000000 | 1.0 |
| H18 | H | 0.5053094500000000 | 0.8860518600000000 | 0.0698988600000000 | 1.0 |
| H19 | H | 0.8311433600000000 | 0.0871308500000000 | 0.8723738300000000 | 1.0 |
| H20 | H | 0.7387290400000000 | 0.9650961300000000 | 0.9134089200000000 | 1.0 |
| H21 | H | 0.8677059700000000 | 0.1724074500000000 | 0.0179193300000000 | 1.0 |
| H22 | H | 0.8282002200000000 | 0.8757969200000000 | 0.0554336500000000 | 1.0 |
| H23 | H | 0.6608060200000000 | 0.1000954200000000 | 0.8559235100000000 | 1.0 |
| H24 | H | 0.7549287600000000 | 0.1567423500000000 | 0.9086066500000000 | 1.0 |
| C25 | C | 0.0441112200000000 | 0.9593239100000000 | 0.9591333800000000 | 1.0 |
| C26 | C | 0.9463839900000000 | 0.9785571700000000 | 0.0200563100000000 | 1.0 |
| C27 | C | 0.9477927800000000 | 0.0566234800000000 | 0.0185593100000000 | 1.0 |
| C28 | C | 0.0370921900000000 | 0.0794412600000000 | 0.9602978800000000 | 1.0 |
| C29 | C | 0.9877644600000000 | 0.9388292400000000 | 0.0834613300000000 | 1.0 |
| C30 | C | 0.2941341000000000 | 0.0834329300000000 | 0.0193924900000000 | 1.0 |
| C31 | C | 0.1963950500000000 | 0.0642057300000000 | 0.9584757800000000 | 1.0 |
| C32 | C | 0.1977930600000000 | 0.9861328600000000 | 0.9599599900000000 | 1.0 |
| C33 | C | 0.2871016200000000 | 0.9633090100000000 | 0.0182180500000000 | 1.0 |
| C34 | C | 0.2377957500000000 | 0.1039649100000000 | 0.8951007600000000 | 1.0 |
| C35 | C | 0.5441099200000000 | 0.9593159900000000 | 0.9591168000000000 | 1.0 |
| C36 | C | 0.4464004000000000 | 0.9785420100000000 | 0.0200483100000000 | 1.0 |
| C37 | C | 0.4478113600000000 | 0.0566104900000000 | 0.0185572000000000 | 1.0 |
| C38 | C | 0.5370911600000000 | 0.0794335500000000 | 0.9602908000000000 | 1.0 |
| C39 | C | 0.4878106000000000 | 0.9387901200000000 | 0.0834305400000000 | 1.0 |
| C40 | C | 0.7941109900000000 | 0.0834357200000000 | 0.0193851800000000 | 1.0 |
| C41 | C | 0.6963902200000000 | 0.0642042100000000 | 0.9584644400000000 | 1.0 |
| C42 | C | 0.6977956400000000 | 0.9861318200000000 | 0.9599442600000000 | 1.0 |
| C43 | C | 0.7871100700000000 | 0.9633087800000000 | 0.0181990800000000 | 1.0 |
| C44 | C | 0.7377910900000000 | 0.1039684200000000 | 0.8950924300000000 | 1.0 |
| O45 | O | 0.0367148100000000 | 0.8912808900000000 | 0.9419888600000000 | 1.0 |
| O46 | O | 0.0045235200000000 | 0.1463080500000000 | 0.9479977700000000 | 1.0 |
| O47 | O | 0.2868114100000000 | 0.1514856700000000 | 0.0365072700000000 | 1.0 |
| O48 | O | 0.2545448800000000 | 0.8964406100000000 | 0.0305003200000000 | 1.0 |
| O49 | O | 0.5367244600000000 | 0.8912760400000000 | 0.9419653900000000 | 1.0 |
| O50 | O | 0.5045108300000000 | 0.1463008600000000 | 0.9479962100000000 | 1.0 |
| O51 | O | 0.7867575700000000 | 0.1514903900000000 | 0.0364944100000000 | 1.0 |
| O52 | O | 0.7545972500000000 | 0.8964322500000000 | 0.0304664600000000 | 1.0 |
| S53 | S | 0.9878516400000000 | 0.0142976800000000 | 0.8917121300000000 | 1.0 |
| S54 | S | 0.2379214900000000 | 0.0284587900000000 | 0.0868287300000000 | 1.0 |
| S55 | S | 0.4878440500000000 | 0.0142947900000000 | 0.8917028700000000 | 1.0 |
| S56 | S | 0.7378807000000000 | 0.0284578100000000 | 0.0868177000000000 | 1.0 |

##### cif ends

thiophene\_OH\_25\_CH3\_3\_anti\_alt\_forbid    Energy: -332.59006642



```
##### cif starts
data_thiophene_OH_25_CH3_3_anti_alt_forbid

_publ_section_comment
;
Andrew Reynoso, Bohan Xu, and Vincent H. Crespi
;
```

```
_cell_length_a 10.5079899295
_cell_length_b 20.0
_cell_length_c 20.0
_cell_angle_alpha 90.0
_cell_angle_beta 90.0
_cell_angle_gamma 90.0
```

```
_symmetry_space_group_name_H-M 'P 1'
_symmetry_Int_Tables_number 1
_symmetry_cell_setting triclinic
```

```
loop_
_atom_site_label
_atom_site_type_symbol
_atom_site_fract_x
_atom_site_fract_y
_atom_site_fract_z
_atom_site_occupancy
H1 H 0.9542017200000000 0.9329886700000000 0.0512495100000000 1.0
H2 H 0.3323212700000000 0.0616883900000000 0.9155952100000000 1.0
H3 H 0.4540575600000000 0.9329845200000000 0.0512613500000000 1.0
H4 H 0.8321950400000000 0.0616831700000000 0.9156321000000000 1.0
H5 H 0.1586757800000000 0.8422436100000000 0.0188107400000000 1.0
H6 H 0.6584930200000000 0.8422678500000000 0.0192003700000000 1.0
H7 H 0.1277541700000000 0.1524239900000000 0.9480086400000000 1.0
H8 H 0.6276209100000000 0.1524451500000000 0.9483950700000000 1.0
H9 H 0.4092127500000000 0.9295035200000000 0.8640146200000000 1.0
H10 H 0.2445328700000000 0.9244746600000000 0.8664710900000000 1.0
H11 H 0.3400694300000000 0.8629189300000000 0.9090643500000000 1.0
H12 H 0.9091241100000000 0.9294868200000000 0.8640276900000000 1.0
H13 H 0.7444492500000000 0.9243828300000000 0.8665406200000000 1.0
H14 H 0.8401213800000000 0.8628972900000000 0.9091341400000000 1.0
H15 H 0.0419240600000000 0.0702120200000000 0.1003581700000000 1.0
H16 H 0.8772346200000000 0.0652322900000000 0.1027969600000000 1.0
H17 H 0.9464709800000000 0.1317677100000000 0.0577126900000000 1.0
H18 H 0.5417875700000000 0.0700986200000000 0.1004205800000000 1.0
H19 H 0.3770813700000000 0.0652842200000000 0.1027584000000000 1.0
H20 H 0.4466261900000000 0.1317634700000000 0.0577306200000000 1.0
H21 H 0.1334814500000000 0.8575664500000000 0.9102629200000000 1.0
H22 H 0.6335290100000000 0.8573833100000000 0.9105470400000000 1.0
H23 H 0.1530023100000000 0.1371005100000000 0.0565565900000000 1.0
H24 H 0.6529954000000000 0.1369156400000000 0.0568376400000000 1.0
C25 C 0.9565136300000000 0.0785346000000000 0.0701497400000000 1.0
C26 C 0.3299629900000000 0.9161559600000000 0.8966659900000000 1.0
C27 C 0.4564734000000000 0.0785177500000000 0.0701610400000000 1.0
C28 C 0.8299292100000000 0.9161241600000000 0.8967093000000000 1.0
C29 C 0.0745730100000000 0.0610596900000000 0.9622760600000000 1.0
```

|     |   |                    |                    |                    |     |
|-----|---|--------------------|--------------------|--------------------|-----|
| C30 | C | 0.9572960700000000 | 0.0376915800000000 | 0.0049461900000000 | 1.0 |
| C31 | C | 0.9597466500000000 | 0.9583774000000000 | 0.0026398600000000 | 1.0 |
| C32 | C | 0.0798658400000000 | 0.9349716500000000 | 0.9627036800000000 | 1.0 |
| C33 | C | 0.2065810100000000 | 0.0596962300000000 | 0.0041132800000000 | 1.0 |
| C34 | C | 0.3267231000000000 | 0.0362885900000000 | 0.9641994800000000 | 1.0 |
| C35 | C | 0.3291569200000000 | 0.9569750700000000 | 0.9618861400000000 | 1.0 |
| C36 | C | 0.2118566500000000 | 0.9336106200000000 | 0.0045426700000000 | 1.0 |
| C37 | C | 0.5746068100000000 | 0.0610266100000000 | 0.9623068400000000 | 1.0 |
| C38 | C | 0.4572812400000000 | 0.0376833200000000 | 0.0049527800000000 | 1.0 |
| C39 | C | 0.4597081500000000 | 0.9583721300000000 | 0.0026535900000000 | 1.0 |
| C40 | C | 0.5798467000000000 | 0.9349300700000000 | 0.9627564900000000 | 1.0 |
| C41 | C | 0.7065586800000000 | 0.0596546100000000 | 0.0041803300000000 | 1.0 |
| C42 | C | 0.8266911400000000 | 0.0362828300000000 | 0.9642380100000000 | 1.0 |
| C43 | C | 0.8291475800000000 | 0.9569633900000000 | 0.9619175900000000 | 1.0 |
| C44 | C | 0.7118747900000000 | 0.9335734600000000 | 0.0045813900000000 | 1.0 |
| O45 | O | 0.0550726900000000 | 0.1248690400000000 | 0.9343564600000000 | 1.0 |
| O46 | O | 0.0603356100000000 | 0.8689399500000000 | 0.9383033700000000 | 1.0 |
| O47 | O | 0.2261393300000000 | 0.1257230900000000 | 0.0285107700000000 | 1.0 |
| O48 | O | 0.2313164200000000 | 0.8698105900000000 | 0.0324971700000000 | 1.0 |
| O49 | O | 0.5552753200000000 | 0.1248333400000000 | 0.9343497500000000 | 1.0 |
| O50 | O | 0.5602136400000000 | 0.8689002700000000 | 0.9384046300000000 | 1.0 |
| O51 | O | 0.7260028900000000 | 0.1256818400000000 | 0.0286398300000000 | 1.0 |
| O52 | O | 0.7314847400000000 | 0.8697643700000000 | 0.0324866600000000 | 1.0 |
| S53 | S | 0.0879867600000000 | 0.9997829300000000 | 0.8951153800000000 | 1.0 |
| S54 | S | 0.1984196500000000 | 0.9948845200000000 | 0.0717036200000000 | 1.0 |
| S55 | S | 0.5880396900000000 | 0.9997502100000000 | 0.8951570500000000 | 1.0 |
| S56 | S | 0.6984315100000000 | 0.9948452200000000 | 0.0717516000000000 | 1.0 |

##### cif ends

thiophene\_OH\_25\_CH3\_3\_anti\_dir    Energy: -332.54755135

##### cif starts

data\_thiophene\_OH\_25\_CH3\_3\_anti\_dir

\_publ\_section\_comment

;  
Andrew Reynoso, Bohan Xu, and Vincent H. Crespi  
;

\_cell\_length\_a    9.8148991557

\_cell\_length\_b    20.0

\_cell\_length\_c    20.0

\_cell\_angle\_alpha    90.0

\_cell\_angle\_beta    90.0

\_cell\_angle\_gamma    90.0

\_symmetry\_space\_group\_name\_H-M    'P 1'

\_symmetry\_Int\_Tables\_number    1

\_symmetry\_cell\_setting    triclinic

loop\_

\_atom\_site\_label

\_atom\_site\_type\_symbol

\_atom\_site\_fract\_x

\_atom\_site\_fract\_y

|     |   | _atom_site_fract_z |                      |                    |     |  |
|-----|---|--------------------|----------------------|--------------------|-----|--|
|     |   |                    | _atom_site_occupancy |                    |     |  |
| H1  | H | 0.0301531800000000 | 0.0210220700000000   | 0.1280785900000000 | 1.0 |  |
| H2  | H | 0.0204510800000000 | 0.9235884700000000   | 0.0662962100000000 | 1.0 |  |
| H3  | H | 0.9741683200000000 | 0.1254224800000000   | 0.9698807700000000 | 1.0 |  |
| H4  | H | 0.1432421800000000 | 0.8310666700000000   | 0.9692796000000000 | 1.0 |  |
| H5  | H | 0.1191499800000000 | 0.0841819300000000   | 0.0839928100000000 | 1.0 |  |
| H6  | H | 0.9462396100000000 | 0.0942765100000000   | 0.1018987800000000 | 1.0 |  |
| H7  | H | 0.2813172200000000 | 0.0168340100000000   | 0.8474210500000000 | 1.0 |  |
| H8  | H | 0.2703964800000000 | 0.9213424300000000   | 0.9118017200000000 | 1.0 |  |
| H9  | H | 0.2240124100000000 | 0.1257994700000000   | 0.0024480800000000 | 1.0 |  |
| H10 | H | 0.3933706100000000 | 0.8316338900000000   | 0.0113446300000000 | 1.0 |  |
| H11 | H | 0.1955372500000000 | 0.0904291000000000   | 0.8710000500000000 | 1.0 |  |
| H12 | H | 0.3684693600000000 | 0.0818354600000000   | 0.8896930200000000 | 1.0 |  |
| H13 | H | 0.5306035800000000 | 0.0208246700000000   | 0.1280614900000000 | 1.0 |  |
| H14 | H | 0.5204047400000000 | 0.9235121700000000   | 0.0662940300000000 | 1.0 |  |
| H15 | H | 0.4740484500000000 | 0.1253810500000000   | 0.9699950400000000 | 1.0 |  |
| H16 | H | 0.6433731300000000 | 0.8310704400000000   | 0.9692650500000000 | 1.0 |  |
| H17 | H | 0.6186212500000000 | 0.0843604600000000   | 0.0840375500000000 | 1.0 |  |
| H18 | H | 0.4456558200000000 | 0.0938853200000000   | 0.1021860900000000 | 1.0 |  |
| H19 | H | 0.7810485100000000 | 0.0169319200000000   | 0.8474346000000000 | 1.0 |  |
| H20 | H | 0.7704553400000000 | 0.9213911500000000   | 0.9118371600000000 | 1.0 |  |
| H21 | H | 0.7239024900000000 | 0.1258219300000000   | 0.0025057400000000 | 1.0 |  |
| H22 | H | 0.8934359100000000 | 0.8317017200000000   | 0.0113806500000000 | 1.0 |  |
| H23 | H | 0.6955827900000000 | 0.0905788200000000   | 0.8711394600000000 | 1.0 |  |
| H24 | H | 0.8685219900000000 | 0.0818150800000000   | 0.8897214700000000 | 1.0 |  |
| C25 | C | 0.0714750900000000 | 0.0409626000000000   | 0.9600836700000000 | 1.0 |  |
| C26 | C | 0.9803341000000000 | 0.0216453300000000   | 0.0205208800000000 | 1.0 |  |
| C27 | C | 0.9823210100000000 | 0.9441463500000000   | 0.0188884900000000 | 1.0 |  |
| C28 | C | 0.0773879000000000 | 0.9213171400000000   | 0.9608162700000000 | 1.0 |  |
| C29 | C | 0.0226242800000000 | 0.0571359700000000   | 0.0873863900000000 | 1.0 |  |
| C30 | C | 0.3214433500000000 | 0.0416919200000000   | 0.0146598100000000 | 1.0 |  |
| C31 | C | 0.2303206200000000 | 0.0206543700000000   | 0.9547926200000000 | 1.0 |  |
| C32 | C | 0.2323011700000000 | 0.9432372500000000   | 0.9586156800000000 | 1.0 |  |
| C33 | C | 0.3274036100000000 | 0.9220654500000000   | 0.0172946100000000 | 1.0 |  |
| C34 | C | 0.2725486000000000 | 0.0541872200000000   | 0.8869103500000000 | 1.0 |  |
| C35 | C | 0.5714525400000000 | 0.0409571300000000   | 0.9601413400000000 | 1.0 |  |
| C36 | C | 0.4802830900000000 | 0.0215834200000000   | 0.0205558800000000 | 1.0 |  |
| C37 | C | 0.4822994900000000 | 0.9440876800000000   | 0.0188873700000000 | 1.0 |  |
| C38 | C | 0.5774342700000000 | 0.9213067000000000   | 0.9608243400000000 | 1.0 |  |
| C39 | C | 0.5224331400000000 | 0.0570208600000000   | 0.0874762300000000 | 1.0 |  |
| C40 | C | 0.8214475500000000 | 0.0417471600000000   | 0.0146879700000000 | 1.0 |  |
| C41 | C | 0.7303039500000000 | 0.0206899800000000   | 0.9548338400000000 | 1.0 |  |
| C42 | C | 0.7323254200000000 | 0.9432716900000000   | 0.9586505200000000 | 1.0 |  |
| C43 | C | 0.8274345900000000 | 0.9221204800000000   | 0.0173287500000000 | 1.0 |  |
| C44 | C | 0.7725018300000000 | 0.0542531900000000   | 0.8869656300000000 | 1.0 |  |
| O45 | O | 0.0587920200000000 | 0.1102587900000000   | 0.9480038800000000 | 1.0 |  |
| O46 | O | 0.0610253900000000 | 0.8514600300000000   | 0.9498631600000000 | 1.0 |  |
| O47 | O | 0.3086350200000000 | 0.1112871900000000   | 0.0247723500000000 | 1.0 |  |
| O48 | O | 0.3111379600000000 | 0.8525385100000000   | 0.0301884900000000 | 1.0 |  |
| O49 | O | 0.5586788800000000 | 0.1102497200000000   | 0.9480892300000000 | 1.0 |  |
| O50 | O | 0.5611597000000000 | 0.8514508600000000   | 0.9498337600000000 | 1.0 |  |
| O51 | O | 0.8085740600000000 | 0.1113369300000000   | 0.0248041100000000 | 1.0 |  |
| O52 | O | 0.8112084300000000 | 0.8525977100000000   | 0.0302471500000000 | 1.0 |  |
| S53 | S | 0.0160723700000000 | 0.9758043100000000   | 0.8925935700000000 | 1.0 |  |

|     |   |                    |                    |                    |     |
|-----|---|--------------------|--------------------|--------------------|-----|
| S54 | S | 0.2660107600000000 | 0.9784231900000000 | 0.0839632900000000 | 1.0 |
| S55 | S | 0.5161032700000000 | 0.9758026600000000 | 0.8926192000000000 | 1.0 |
| S56 | S | 0.7660976100000000 | 0.9784942400000000 | 0.0839938100000000 | 1.0 |

##### cif ends

thiophene\_OH\_25\_CH3\_3\_anti\_dir\_forbid    Energy: -332.71149236

##### cif starts

data\_thiophene\_OH\_25\_CH3\_3\_anti\_dir\_forbid

\_publ\_section\_comment

;  
Andrew Reynoso, Bohan Xu, and Vincent H. Crespi  
;

\_cell\_length\_a    10.5056454463

\_cell\_length\_b    20.0

\_cell\_length\_c    20.0

\_cell\_angle\_alpha    90.0

\_cell\_angle\_beta    90.0

\_cell\_angle\_gamma    90.0

\_symmetry\_space\_group\_name\_H-M    'P 1'

\_symmetry\_Int\_Tables\_number 1

\_symmetry\_cell\_setting triclinic

loop\_

\_atom\_site\_label

\_atom\_site\_type\_symbol

\_atom\_site\_fract\_x

\_atom\_site\_fract\_y

\_atom\_site\_fract\_z

\_atom\_site\_occupancy

|     |   |                    |                    |                    |     |
|-----|---|--------------------|--------------------|--------------------|-----|
| H1  | H | 0.1339433000000000 | 0.0655636300000000 | 0.0627305200000000 | 1.0 |
| H2  | H | 0.2484544200000000 | 0.0661194700000000 | 0.9232804000000000 | 1.0 |
| H3  | H | 0.6339666200000000 | 0.0653525500000000 | 0.0627731300000000 | 1.0 |
| H4  | H | 0.7484167900000000 | 0.0658306200000000 | 0.9232755300000000 | 1.0 |
| H5  | H | 0.9434476400000000 | 0.8661531600000000 | 0.9211364400000000 | 1.0 |
| H6  | H | 0.4439709900000000 | 0.8669837600000000 | 0.9195014000000000 | 1.0 |
| H7  | H | 0.4385470400000000 | 0.8537484000000000 | 0.0304888100000000 | 1.0 |
| H8  | H | 0.9404018500000000 | 0.8543706600000000 | 0.0330881600000000 | 1.0 |
| H9  | H | 0.3396127800000000 | 0.9318863600000000 | 0.8763747400000000 | 1.0 |
| H10 | H | 0.1748002100000000 | 0.9354199000000000 | 0.8757819200000000 | 1.0 |
| H11 | H | 0.2470102900000000 | 0.8689556300000000 | 0.9193619400000000 | 1.0 |
| H12 | H | 0.8403054000000000 | 0.9311476400000000 | 0.8768058000000000 | 1.0 |
| H13 | H | 0.6755453800000000 | 0.9354041200000000 | 0.8757626700000000 | 1.0 |
| H14 | H | 0.7464068400000000 | 0.8687267100000000 | 0.9196671600000000 | 1.0 |
| H15 | H | 0.1430982700000000 | 0.8693795800000000 | 0.0673623200000000 | 1.0 |
| H16 | H | 0.0388708300000000 | 0.9269788900000000 | 0.1075137100000000 | 1.0 |
| H17 | H | 0.2037295200000000 | 0.9385110600000000 | 0.1116283800000000 | 1.0 |
| H18 | H | 0.6435762500000000 | 0.8692481900000000 | 0.0672864700000000 | 1.0 |
| H19 | H | 0.5381478800000000 | 0.9262577800000000 | 0.1071549800000000 | 1.0 |
| H20 | H | 0.7028582600000000 | 0.9386195400000000 | 0.1117760000000000 | 1.0 |
| H21 | H | 0.9603033500000000 | 0.1619951900000000 | 0.9613349900000000 | 1.0 |
| H22 | H | 0.4035247800000000 | 0.1466611900000000 | 0.0713018200000000 | 1.0 |

|     |   |                    |                    |                    |     |
|-----|---|--------------------|--------------------|--------------------|-----|
| H23 | H | 0.4608864000000000 | 0.1620777500000000 | 0.9617853800000000 | 1.0 |
| H24 | H | 0.9032819100000000 | 0.1469419700000000 | 0.0709486600000000 | 1.0 |
| C25 | C | 0.0088597900000000 | 0.0699784900000000 | 0.9734787500000000 | 1.0 |
| C26 | C | 0.1263944300000000 | 0.0421496100000000 | 0.0132420900000000 | 1.0 |
| C27 | C | 0.1247823600000000 | 0.9630545800000000 | 0.0135441900000000 | 1.0 |
| C28 | C | 0.0053043700000000 | 0.9435406500000000 | 0.9711636800000000 | 1.0 |
| C29 | C | 0.3729489700000000 | 0.0692736000000000 | 0.0127044300000000 | 1.0 |
| C30 | C | 0.2552493600000000 | 0.0424233500000000 | 0.9726433200000000 | 1.0 |
| C31 | C | 0.2567515500000000 | 0.9633559300000000 | 0.9725652600000000 | 1.0 |
| C32 | C | 0.3762570000000000 | 0.9429780800000000 | 0.0147430500000000 | 1.0 |
| C33 | C | 0.5089842700000000 | 0.0699542700000000 | 0.9734966600000000 | 1.0 |
| C34 | C | 0.6263923100000000 | 0.0419970500000000 | 0.0132622800000000 | 1.0 |
| C35 | C | 0.6246773200000000 | 0.9628881700000000 | 0.0135185700000000 | 1.0 |
| C36 | C | 0.5052565000000000 | 0.9435812900000000 | 0.9709685300000000 | 1.0 |
| C37 | C | 0.8728390700000000 | 0.0692863400000000 | 0.0126986900000000 | 1.0 |
| C38 | C | 0.7552541200000000 | 0.0422480000000000 | 0.9726858100000000 | 1.0 |
| C39 | C | 0.7568392000000000 | 0.9631717100000000 | 0.9727143000000000 | 1.0 |
| C40 | C | 0.8763511300000000 | 0.9429466600000000 | 0.0149698300000000 | 1.0 |
| C41 | C | 0.1266982700000000 | 0.9223342800000000 | 0.0787596300000000 | 1.0 |
| C42 | C | 0.2556856200000000 | 0.9224160800000000 | 0.9074511600000000 | 1.0 |
| C43 | C | 0.6263934900000000 | 0.9221205500000000 | 0.0786978800000000 | 1.0 |
| C44 | C | 0.7559385900000000 | 0.9221280500000000 | 0.9076682400000000 | 1.0 |
| O45 | O | 0.0331036300000000 | 0.1342062500000000 | 0.9481426300000000 | 1.0 |
| O46 | O | 0.3447784500000000 | 0.1353677000000000 | 0.0352067700000000 | 1.0 |
| O47 | O | 0.5333084200000000 | 0.1341887100000000 | 0.9482168000000000 | 1.0 |
| O48 | O | 0.8443491000000000 | 0.1354017900000000 | 0.0350152400000000 | 1.0 |
| O49 | O | 0.0212605700000000 | 0.8778904400000000 | 0.9452719600000000 | 1.0 |
| O50 | O | 0.3627596700000000 | 0.8792950800000000 | 0.0432350500000000 | 1.0 |
| O51 | O | 0.5207765700000000 | 0.8779010400000000 | 0.9449020800000000 | 1.0 |
| O52 | O | 0.8626945300000000 | 0.8793010900000000 | 0.0435137000000000 | 1.0 |
| S53 | S | 0.9961747300000000 | 0.0091534000000000 | 0.9047528000000000 | 1.0 |
| S54 | S | 0.3860507400000000 | 0.0101064600000000 | 0.0813985600000000 | 1.0 |
| S55 | S | 0.4964468200000000 | 0.0092211300000000 | 0.9046703200000000 | 1.0 |
| S56 | S | 0.8859524200000000 | 0.0102594900000000 | 0.0815191300000000 | 1.0 |

##### cif ends

thiophene\_OH\_25\_CH3\_3\_syn\_alt    Energy: -332.72987661

##### cif starts

data\_thiophene\_OH\_25\_CH3\_3\_syn\_alt

\_publ\_section\_comment

;  
Andrew Reynoso, Bohan Xu, and Vincent H. Crespi  
;

\_cell\_length\_a    10.3846356575

\_cell\_length\_b    20.0

\_cell\_length\_c    20.0

\_cell\_angle\_alpha    90.0

\_cell\_angle\_beta    90.0

\_cell\_angle\_gamma    90.0

\_symmetry\_space\_group\_name\_H-M    'P 1'

\_symmetry\_Int\_Tables\_number    1

\_symmetry\_cell\_setting triclinic

loop\_

\_atom\_site\_label

\_atom\_site\_type\_symbol

\_atom\_site\_fract\_x

\_atom\_site\_fract\_y

\_atom\_site\_fract\_z

\_atom\_site\_occupancy

|     |   |                    |                    |                    |     |
|-----|---|--------------------|--------------------|--------------------|-----|
| H1  | H | 0.0871962200000000 | 0.9520404100000000 | 0.8779952400000000 | 1.0 |
| H2  | H | 0.1704988800000000 | 0.0629814800000000 | 0.9314620300000000 | 1.0 |
| H3  | H | 0.1268844700000000 | 0.8592869300000000 | 0.0487650100000000 | 1.0 |
| H4  | H | 0.1273964300000000 | 0.1435299200000000 | 0.0504568600000000 | 1.0 |
| H5  | H | 0.2561490700000000 | 0.9466104400000000 | 0.8795267900000000 | 1.0 |
| H6  | H | 0.1625104000000000 | 0.8785802000000000 | 0.9090199600000000 | 1.0 |
| H7  | H | 0.5062591100000000 | 0.0594605200000000 | 0.8807974900000000 | 1.0 |
| H8  | H | 0.4204900100000000 | 0.9420611400000000 | 0.9301872700000000 | 1.0 |
| H9  | H | 0.3766986200000000 | 0.1431692000000000 | 0.0518634600000000 | 1.0 |
| H10 | H | 0.3773386500000000 | 0.8589693400000000 | 0.0473971600000000 | 1.0 |
| H11 | H | 0.3372765600000000 | 0.0543980900000000 | 0.8791872200000000 | 1.0 |
| H12 | H | 0.4131160700000000 | 0.1269822600000000 | 0.9118571100000000 | 1.0 |
| H13 | H | 0.5872770700000000 | 0.9518246100000000 | 0.8781480700000000 | 1.0 |
| H14 | H | 0.6703924700000000 | 0.0630821700000000 | 0.9316839300000000 | 1.0 |
| H15 | H | 0.6268450700000000 | 0.8592271100000000 | 0.0485887900000000 | 1.0 |
| H16 | H | 0.6274145500000000 | 0.1434584000000000 | 0.0505624800000000 | 1.0 |
| H17 | H | 0.7562734300000000 | 0.9468257000000000 | 0.8796211300000000 | 1.0 |
| H18 | H | 0.6632931100000000 | 0.8785720000000000 | 0.9091677300000000 | 1.0 |
| H19 | H | 0.0061837600000000 | 0.0594646600000000 | 0.8807931000000000 | 1.0 |
| H20 | H | 0.9204136000000000 | 0.9419492500000000 | 0.9303461300000000 | 1.0 |
| H21 | H | 0.8769874200000000 | 0.1432608100000000 | 0.0515755300000000 | 1.0 |
| H22 | H | 0.8775022900000000 | 0.8590442500000000 | 0.0475317900000000 | 1.0 |
| H23 | H | 0.8372292100000000 | 0.0541211800000000 | 0.8791429800000000 | 1.0 |
| H24 | H | 0.9126298500000000 | 0.1268719800000000 | 0.9117351200000000 | 1.0 |
| C25 | C | 0.0447642600000000 | 0.9413845400000000 | 0.0180208600000000 | 1.0 |
| C26 | C | 0.1697855000000000 | 0.9623621500000000 | 0.9787068100000000 | 1.0 |
| C27 | C | 0.1699681500000000 | 0.0410857000000000 | 0.9819386800000000 | 1.0 |
| C28 | C | 0.0445908900000000 | 0.0619629300000000 | 0.0189442600000000 | 1.0 |
| C29 | C | 0.1688245700000000 | 0.9333738100000000 | 0.9073461900000000 | 1.0 |
| C30 | C | 0.2946380600000000 | 0.0617808900000000 | 0.0192370300000000 | 1.0 |
| C31 | C | 0.4197770200000000 | 0.0416253400000000 | 0.9796198600000000 | 1.0 |
| C32 | C | 0.4199173000000000 | 0.9628656300000000 | 0.9811204800000000 | 1.0 |
| C33 | C | 0.2944950600000000 | 0.9411740700000000 | 0.0176043700000000 | 1.0 |
| C34 | C | 0.4190604200000000 | 0.0722305800000000 | 0.9089354500000000 | 1.0 |
| C35 | C | 0.5446274700000000 | 0.9413425100000000 | 0.0179805900000000 | 1.0 |
| C36 | C | 0.6698291400000000 | 0.9624031800000000 | 0.9788242400000000 | 1.0 |
| C37 | C | 0.6699274500000000 | 0.0410688100000000 | 0.9821025000000000 | 1.0 |
| C38 | C | 0.5444622300000000 | 0.0618987100000000 | 0.0191044800000000 | 1.0 |
| C39 | C | 0.6691177000000000 | 0.9333766700000000 | 0.9074787300000000 | 1.0 |
| C40 | C | 0.7947232400000000 | 0.0617694000000000 | 0.0193621000000000 | 1.0 |
| C41 | C | 0.9198243700000000 | 0.0416001600000000 | 0.9796148700000000 | 1.0 |
| C42 | C | 0.9199978700000000 | 0.9628652700000000 | 0.9812308700000000 | 1.0 |
| C43 | C | 0.7945858200000000 | 0.9412584600000000 | 0.0178339900000000 | 1.0 |
| C44 | C | 0.9188763100000000 | 0.0721250600000000 | 0.9088939000000000 | 1.0 |
| O45 | O | 0.0390628700000000 | 0.8735169600000000 | 0.0351905400000000 | 1.0 |
| O46 | O | 0.0391295200000000 | 0.1294087400000000 | 0.0374880100000000 | 1.0 |

|     |   |                    |                    |                    |     |
|-----|---|--------------------|--------------------|--------------------|-----|
| O47 | O | 0.2889617300000000 | 0.1292589700000000 | 0.0378603300000000 | 1.0 |
| O48 | O | 0.2890983100000000 | 0.8733526300000000 | 0.0347221400000000 | 1.0 |
| O49 | O | 0.5390344600000000 | 0.8734463100000000 | 0.0350084700000000 | 1.0 |
| O50 | O | 0.5390994400000000 | 0.1293090800000000 | 0.0377483500000000 | 1.0 |
| O51 | O | 0.7890911100000000 | 0.1292817300000000 | 0.0378550300000000 | 1.0 |
| O52 | O | 0.7891794900000000 | 0.8734460800000000 | 0.0349819800000000 | 1.0 |
| S53 | S | 0.0451327400000000 | 0.0008396700000000 | 0.0937055200000000 | 1.0 |
| S54 | S | 0.2945232600000000 | 0.0007157400000000 | 0.0937271100000000 | 1.0 |
| S55 | S | 0.5443436500000000 | 0.0006842800000000 | 0.0936770300000000 | 1.0 |
| S56 | S | 0.7949466100000000 | 0.0008210100000000 | 0.0936568100000000 | 1.0 |

##### cif ends

thiophene\_OH\_25\_CH3\_3\_syn\_alt\_forbid    Energy: -329.73826428

##### cif starts

data\_thiophene\_OH\_25\_CH3\_3\_syn\_alt\_forbid

\_publ\_section\_comment

;  
Andrew Reynoso, Bohan Xu, and Vincent H. Crespi  
;

\_cell\_length\_a    10.2149932017

\_cell\_length\_b    20.0

\_cell\_length\_c    20.0

\_cell\_angle\_alpha    90.0

\_cell\_angle\_beta    90.0

\_cell\_angle\_gamma    90.0

\_symmetry\_space\_group\_name\_H-M    'P 1'

\_symmetry\_Int\_Tables\_number 1

\_symmetry\_cell\_setting triclinic

loop\_

\_atom\_site\_label

\_atom\_site\_type\_symbol

\_atom\_site\_fract\_x

\_atom\_site\_fract\_y

\_atom\_site\_fract\_z

\_atom\_site\_occupancy

|     |   |                    |                    |                    |     |
|-----|---|--------------------|--------------------|--------------------|-----|
| H1  | H | 0.9854223200000000 | 0.0558189500000000 | 0.9305513000000000 | 1.0 |
| H2  | H | 0.2574580200000000 | 0.9323754800000000 | 0.9514476100000000 | 1.0 |
| H3  | H | 0.5168301200000000 | 0.0593411800000000 | 0.9490396500000000 | 1.0 |
| H4  | H | 0.7881873100000000 | 0.9329560800000000 | 0.9340883100000000 | 1.0 |
| H5  | H | 0.1862374000000000 | 0.1655252600000000 | 0.0528217700000000 | 1.0 |
| H6  | H | 0.4255865100000000 | 0.8525760000000000 | 0.0660223200000000 | 1.0 |
| H7  | H | 0.6775536600000000 | 0.1306665900000000 | 0.0923109900000000 | 1.0 |
| H8  | H | 0.9309520900000000 | 0.8729663300000000 | 0.0765793600000000 | 1.0 |
| H9  | H | 0.9259572500000000 | 0.1438170000000000 | 0.0555572400000000 | 1.0 |
| H10 | H | 0.4331048400000000 | 0.1247300300000000 | 0.0724024800000000 | 1.0 |
| H11 | H | 0.6866796200000000 | 0.8315913600000000 | 0.0622616400000000 | 1.0 |
| H12 | H | 0.1777300500000000 | 0.8686466900000000 | 0.1015781600000000 | 1.0 |
| H13 | H | 0.3017849200000000 | 0.1201649100000000 | 0.9106317200000000 | 1.0 |
| H14 | H | 0.1813179200000000 | 0.0578730900000000 | 0.8964096700000000 | 1.0 |
| H15 | H | 0.3462296500000000 | 0.0432580800000000 | 0.8726150600000000 | 1.0 |

|     |   |                    |                    |                    |     |
|-----|---|--------------------|--------------------|--------------------|-----|
| H16 | H | 0.8196602000000000 | 0.0728180100000000 | 0.8840857900000000 | 1.0 |
| H17 | H | 0.7131713200000000 | 0.1193000100000000 | 0.9359803700000000 | 1.0 |
| H18 | H | 0.6624449900000000 | 0.0416367500000000 | 0.9007461700000000 | 1.0 |
| H19 | H | 0.1100288900000000 | 0.9459256100000000 | 0.9037871100000000 | 1.0 |
| H20 | H | 0.9537768900000000 | 0.9123451400000000 | 0.8896501900000000 | 1.0 |
| H21 | H | 0.0624336600000000 | 0.8702804800000000 | 0.9440425700000000 | 1.0 |
| H22 | H | 0.5931256100000000 | 0.9308937100000000 | 0.9001952900000000 | 1.0 |
| H23 | H | 0.4282904800000000 | 0.9439337000000000 | 0.8753346600000000 | 1.0 |
| H24 | H | 0.4729668800000000 | 0.8692894500000000 | 0.9174908600000000 | 1.0 |
| C25 | C | 0.0476982800000000 | 0.0722998700000000 | 0.0336283800000000 | 1.0 |
| C26 | C | 0.9620715200000000 | 0.0370220400000000 | 0.9808659700000000 | 1.0 |
| C27 | C | 0.9724236600000000 | 0.9598139300000000 | 0.9874351500000000 | 1.0 |
| C28 | C | 0.0478419500000000 | 0.9497813400000000 | 0.0550287400000000 | 1.0 |
| C29 | C | 0.0286698400000000 | 0.9200543100000000 | 0.9282892800000000 | 1.0 |
| C30 | C | 0.2269173800000000 | 0.0728987200000000 | 0.0344616000000000 | 1.0 |
| C31 | C | 0.3121006400000000 | 0.0380877300000000 | 0.9807705900000000 | 1.0 |
| C32 | C | 0.3027921700000000 | 0.9613310300000000 | 0.9915024000000000 | 1.0 |
| C33 | C | 0.2260862500000000 | 0.9501847500000000 | 0.0569214000000000 | 1.0 |
| C34 | C | 0.2836854100000000 | 0.0659838500000000 | 0.9110361200000000 | 1.0 |
| C35 | C | 0.5467909200000000 | 0.0457164600000000 | 0.0553379400000000 | 1.0 |
| C36 | C | 0.4705098300000000 | 0.0323594300000000 | 0.9901801900000000 | 1.0 |
| C37 | C | 0.4614205700000000 | 0.9548086000000000 | 0.9832088100000000 | 1.0 |
| C38 | C | 0.5463444900000000 | 0.9225433800000000 | 0.0389293000000000 | 1.0 |
| C39 | C | 0.4907051800000000 | 0.9234672400000000 | 0.9150607300000000 | 1.0 |
| C40 | C | 0.7251880800000000 | 0.0471084000000000 | 0.0514844000000000 | 1.0 |
| C41 | C | 0.8004841000000000 | 0.0322361600000000 | 0.9848953400000000 | 1.0 |
| C42 | C | 0.8109013600000000 | 0.9550883000000000 | 0.9830846300000000 | 1.0 |
| C43 | C | 0.7250704700000000 | 0.9231922300000000 | 0.0375817100000000 | 1.0 |
| C44 | C | 0.7449434900000000 | 0.0683065700000000 | 0.9233263900000000 | 1.0 |
| O45 | O | 0.0181794900000000 | 0.1410872600000000 | 0.0405393100000000 | 1.0 |
| O46 | O | 0.0202343800000000 | 0.8894492300000000 | 0.0873178600000000 | 1.0 |
| O47 | O | 0.2659902000000000 | 0.1403978300000000 | 0.0404080900000000 | 1.0 |
| O48 | O | 0.2610746800000000 | 0.8894317700000000 | 0.0865479900000000 | 1.0 |
| O49 | O | 0.5199436000000000 | 0.1071850300000000 | 0.0859643100000000 | 1.0 |
| O50 | O | 0.5170331400000000 | 0.8542587200000000 | 0.0495885300000000 | 1.0 |
| O51 | O | 0.7601866900000000 | 0.1098779200000000 | 0.0761088300000000 | 1.0 |
| O52 | O | 0.7652312600000000 | 0.8561420500000000 | 0.0470746100000000 | 1.0 |
| S53 | S | 0.0082814500000000 | 0.0246850000000000 | 0.1064509500000000 | 1.0 |
| S54 | S | 0.2638882200000000 | 0.0253929100000000 | 0.1084623000000000 | 1.0 |
| S55 | S | 0.5102080900000000 | 0.9733496500000000 | 0.1101187800000000 | 1.0 |
| S56 | S | 0.7660099600000000 | 0.9754444900000000 | 0.1077163300000000 | 1.0 |

##### cif ends

thiophene\_OH\_CF3\_245\_syn\_dir\_break    Energy: -333.68562954

##### cif starts

data\_thiophene\_OH\_CF3\_245\_syn\_dir\_break

\_publ\_section\_comment

;  
Andrew Reynoso, Bohan Xu, and Vincent H. Crespi  
;

\_cell\_length\_a    10.7026195698

\_cell\_length\_b    20.0



\_cell\_length\_c 20.0  
\_cell\_angle\_alpha 90.0  
\_cell\_angle\_beta 90.0  
\_cell\_angle\_gamma 90.0

\_symmetry\_space\_group\_name\_H-M 'P 1'  
\_symmetry\_Int\_Tables\_number 1  
\_symmetry\_cell\_setting triclinic

loop\_

\_atom\_site\_label  
\_atom\_site\_type\_symbol  
\_atom\_site\_fract\_x  
\_atom\_site\_fract\_y  
\_atom\_site\_fract\_z  
\_atom\_site\_occupancy

|     |   |                    |                    |                    |     |
|-----|---|--------------------|--------------------|--------------------|-----|
| H1  | H | 0.1261189800000000 | 0.8907796200000000 | 0.9623004800000000 | 1.0 |
| H2  | H | 0.9557948300000000 | 0.0831523700000000 | 0.1821042900000000 | 1.0 |
| H3  | H | 0.0579774600000000 | 0.8422030200000000 | 0.0529799300000000 | 1.0 |
| H4  | H | 0.3719241400000000 | 0.9001237600000000 | 0.9484081500000000 | 1.0 |
| H5  | H | 0.1743054800000000 | 0.1119855800000000 | 0.9092743000000000 | 1.0 |
| H6  | H | 0.3307351600000000 | 0.8848963900000000 | 0.0964110700000000 | 1.0 |
| H7  | H | 0.6504163500000000 | 0.9323282900000000 | 0.9442312900000000 | 1.0 |
| H8  | H | 0.5269338600000000 | 0.1382169200000000 | 0.0328449300000000 | 1.0 |
| H9  | H | 0.5945440500000000 | 0.8525913100000000 | 0.0606125500000000 | 1.0 |
| H10 | H | 0.8817307100000000 | 0.9772388900000000 | 0.9608301100000000 | 1.0 |
| H11 | H | 0.7289879800000000 | 0.1310021600000000 | 0.1160331600000000 | 1.0 |
| H12 | H | 0.8454526100000000 | 0.8531901200000000 | 0.0509723100000000 | 1.0 |
| C13 | C | 0.8848619400000000 | 0.0145884500000000 | 0.1245454100000000 | 1.0 |
| C14 | C | 0.1510819400000000 | 0.9944479500000000 | 0.9372019900000000 | 1.0 |
| C15 | C | 0.1339860100000000 | 0.9402807500000000 | 0.9864716600000000 | 1.0 |
| C16 | C | 0.0038999300000000 | 0.9350362400000000 | 0.0379876900000000 | 1.0 |
| C17 | C | 0.0917315100000000 | 0.9892593200000000 | 0.8725057500000000 | 1.0 |
| C18 | C | 0.2540371600000000 | 0.0405705000000000 | 0.9565970800000000 | 1.0 |
| C19 | C | 0.3938534900000000 | 0.0101379000000000 | 0.9531064200000000 | 1.0 |
| C20 | C | 0.3810758700000000 | 0.9406773900000000 | 0.9851640400000000 | 1.0 |
| C21 | C | 0.2533626000000000 | 0.9440955500000000 | 0.0289221800000000 | 1.0 |
| C22 | C | 0.4284248600000000 | 0.0018264300000000 | 0.8776318200000000 | 1.0 |
| C23 | C | 0.4931161800000000 | 0.0499865900000000 | 0.0014411700000000 | 1.0 |
| C24 | C | 0.6370389200000000 | 0.0330568200000000 | 0.9918246900000000 | 1.0 |
| C25 | C | 0.6370162800000000 | 0.9549895800000000 | 0.9935532700000000 | 1.0 |
| C26 | C | 0.5051115600000000 | 0.9309379800000000 | 0.0263688000000000 | 1.0 |
| C27 | C | 0.6933654500000000 | 0.0689339600000000 | 0.9273061300000000 | 1.0 |
| C28 | C | 0.7195805000000000 | 0.0546568100000000 | 0.0553365500000000 | 1.0 |
| C29 | C | 0.8671665000000000 | 0.0420224000000000 | 0.0528962600000000 | 1.0 |
| C30 | C | 0.8801416300000000 | 0.9724312600000000 | 0.0154193400000000 | 1.0 |
| C31 | C | 0.7516739000000000 | 0.9354286100000000 | 0.0369571600000000 | 1.0 |
| C32 | C | 0.9484717500000000 | 0.1066569300000000 | 0.0400576400000000 | 1.0 |
| O33 | O | 0.8759018000000000 | 0.0596154900000000 | 0.1782831900000000 | 1.0 |
| O34 | O | 0.9814245000000000 | 0.8634870900000000 | 0.0367200600000000 | 1.0 |
| O35 | O | 0.2564826000000000 | 0.1037012800000000 | 0.9285508000000000 | 1.0 |
| O36 | O | 0.2468988000000000 | 0.8958837900000000 | 0.0802690200000000 | 1.0 |
| O37 | O | 0.4617982600000000 | 0.1152850900000000 | 0.0070634200000000 | 1.0 |
| O38 | O | 0.5072592800000000 | 0.8664482900000000 | 0.0524089100000000 | 1.0 |
| O39 | O | 0.6752825600000000 | 0.1147533800000000 | 0.0799589900000000 | 1.0 |

|     |   |                    |                    |                    |     |
|-----|---|--------------------|--------------------|--------------------|-----|
| O40 | O | 0.7548372200000000 | 0.8677316100000000 | 0.0457389600000000 | 1.0 |
| F41 | F | 0.1155895700000000 | 0.0417905000000000 | 0.8300688100000000 | 1.0 |
| F42 | F | 0.9582283300000000 | 0.9857987800000000 | 0.8747824000000000 | 1.0 |
| F43 | F | 0.1151127300000000 | 0.9306843000000000 | 0.8349975600000000 | 1.0 |
| F44 | F | 0.4662015300000000 | 0.0590518200000000 | 0.8480199800000000 | 1.0 |
| F45 | F | 0.3319592200000000 | 0.9786303600000000 | 0.8409719700000000 | 1.0 |
| F46 | F | 0.5197843100000000 | 0.9536674300000000 | 0.8676838900000000 | 1.0 |
| F47 | F | 0.6280254900000000 | 0.1247458000000000 | 0.9114320800000000 | 1.0 |
| F48 | F | 0.6997899200000000 | 0.0287239700000000 | 0.8733256400000000 | 1.0 |
| F49 | F | 0.8123645100000000 | 0.0909456100000000 | 0.9366764100000000 | 1.0 |
| F50 | F | 0.0287601700000000 | 0.1183663800000000 | 0.0927256200000000 | 1.0 |
| F51 | F | 0.8770322600000000 | 0.1636470600000000 | 0.0381849500000000 | 1.0 |
| F52 | F | 0.0175204200000000 | 0.1067313700000000 | 0.9843769400000000 | 1.0 |
| S53 | S | 0.0158969000000000 | 0.9594032900000000 | 0.1280861000000000 | 1.0 |
| S54 | S | 0.2379760500000000 | 0.0344444300000000 | 0.0537728700000000 | 1.0 |
| S55 | S | 0.4808881400000000 | 0.9996976500000000 | 0.0881484400000000 | 1.0 |
| S56 | S | 0.7104984500000000 | 0.9841741200000000 | 0.1192573900000000 | 1.0 |

##### cif ends

thiophene\_OH\_CH3\_245\_syn\_dir    Energy: -330.88433736

##### cif starts

data\_thiophene\_OH\_CH3\_245\_syn\_dir

\_publ\_section\_comment

;  
Andrew Reynoso, Bohan Xu, and Vincent H. Crespi  
;

\_cell\_length\_a    10.6737226891

\_cell\_length\_b    20.0

\_cell\_length\_c    20.0

\_cell\_angle\_alpha    90.0

\_cell\_angle\_beta    90.0

\_cell\_angle\_gamma    90.0

\_symmetry\_space\_group\_name\_H-M    'P 1'

\_symmetry\_Int\_Tables\_number 1

\_symmetry\_cell\_setting triclinic

loop\_

\_atom\_site\_label

\_atom\_site\_type\_symbol

\_atom\_site\_fract\_x

\_atom\_site\_fract\_y

\_atom\_site\_fract\_z

\_atom\_site\_occupancy

|    |   |                    |                    |                    |     |
|----|---|--------------------|--------------------|--------------------|-----|
| H1 | H | 0.0912759200000000 | 0.0209459900000000 | 0.8734347700000000 | 1.0 |
| H2 | H | 0.1119493400000000 | 0.9179753600000000 | 0.9496349100000000 | 1.0 |
| H3 | H | 0.0477976600000000 | 0.1302186400000000 | 0.0450501600000000 | 1.0 |
| H4 | H | 0.8961406300000000 | 0.8396353900000000 | 0.0554428200000000 | 1.0 |
| H5 | H | 0.0199838500000000 | 0.0923805900000000 | 0.9100550800000000 | 1.0 |
| H6 | H | 0.1808306100000000 | 0.0874719700000000 | 0.9070429400000000 | 1.0 |
| H7 | H | 0.4561152500000000 | 0.0118065100000000 | 0.8957952800000000 | 1.0 |
| H8 | H | 0.3280493600000000 | 0.9182448900000000 | 0.9497904800000000 | 1.0 |

|     |   |                    |                    |                    |     |
|-----|---|--------------------|--------------------|--------------------|-----|
| H9  | H | 0.1403075600000000 | 0.8545709800000000 | 0.0790784300000000 | 1.0 |
| H10 | H | 0.2942755800000000 | 0.0085507600000000 | 0.8858798400000000 | 1.0 |
| H11 | H | 0.3680915900000000 | 0.0869101100000000 | 0.8992452300000000 | 1.0 |
| H12 | H | 0.2998847100000000 | 0.1348421300000000 | 0.0448531100000000 | 1.0 |
| H13 | H | 0.6046997100000000 | 0.0714776400000000 | 0.8956706400000000 | 1.0 |
| H14 | H | 0.5848114100000000 | 0.9333522700000000 | 0.9314544200000000 | 1.0 |
| H15 | H | 0.5403062900000000 | 0.1145108100000000 | 0.0851692400000000 | 1.0 |
| H16 | H | 0.4006630900000000 | 0.8386812800000000 | 0.0575629700000000 | 1.0 |
| H17 | H | 0.5189454000000000 | 0.1161626300000000 | 0.9560830500000000 | 1.0 |
| H18 | H | 0.6809863600000000 | 0.1171196600000000 | 0.9596376300000000 | 1.0 |
| H19 | H | 0.9055955000000000 | 0.0143410600000000 | 0.8867295200000000 | 1.0 |
| H20 | H | 0.8679108400000000 | 0.9203613200000000 | 0.9368235500000000 | 1.0 |
| H21 | H | 0.6418495400000000 | 0.8279530700000000 | 0.0266025600000000 | 1.0 |
| H22 | H | 0.7443557500000000 | 0.0153168400000000 | 0.8951693000000000 | 1.0 |
| H23 | H | 0.8300192100000000 | 0.0910185500000000 | 0.9051940900000000 | 1.0 |
| H24 | H | 0.8142791100000000 | 0.1063499600000000 | 0.0789229300000000 | 1.0 |
| C25 | C | 0.9738847900000000 | 0.0434983500000000 | 0.0240282500000000 | 1.0 |
| C26 | C | 0.0983865900000000 | 0.0245269500000000 | 0.9849991600000000 | 1.0 |
| C27 | C | 0.1012234000000000 | 0.9466850200000000 | 0.9963607400000000 | 1.0 |
| C28 | C | 0.9722018800000000 | 0.9252851400000000 | 0.0313911900000000 | 1.0 |
| C29 | C | 0.0973918400000000 | 0.0571054600000000 | 0.9145989500000000 | 1.0 |
| C30 | C | 0.2238834800000000 | 0.0503014200000000 | 0.0211456100000000 | 1.0 |
| C31 | C | 0.3514712500000000 | 0.0209071400000000 | 0.9888554300000000 | 1.0 |
| C32 | C | 0.3434879700000000 | 0.9444270500000000 | 0.9976245800000000 | 1.0 |
| C33 | C | 0.2225565600000000 | 0.9333286400000000 | 0.0418444900000000 | 1.0 |
| C34 | C | 0.3686533400000000 | 0.0340508800000000 | 0.9135244800000000 | 1.0 |
| C35 | C | 0.4695936800000000 | 0.0380273400000000 | 0.0382420100000000 | 1.0 |
| C36 | C | 0.5984327000000000 | 0.0251498500000000 | 0.9995013100000000 | 1.0 |
| C37 | C | 0.5947191400000000 | 0.9470536100000000 | 0.9845459000000000 | 1.0 |
| C38 | C | 0.4748890700000000 | 0.9216004200000000 | 0.0266962300000000 | 1.0 |
| C39 | C | 0.6012959900000000 | 0.0846858300000000 | 0.9484899800000000 | 1.0 |
| C40 | C | 0.7248309000000000 | 0.0301598100000000 | 0.0407185300000000 | 1.0 |
| C41 | C | 0.8456281600000000 | 0.0171705200000000 | 0.9892846500000000 | 1.0 |
| C42 | C | 0.8531855800000000 | 0.9402754100000000 | 0.9876108000000000 | 1.0 |
| C43 | C | 0.7227361900000000 | 0.9139027600000000 | 0.0151886300000000 | 1.0 |
| C44 | C | 0.8300019400000000 | 0.0372869100000000 | 0.9153629000000000 | 1.0 |
| O45 | O | 0.9626833000000000 | 0.1126951400000000 | 0.0366386100000000 | 1.0 |
| O46 | O | 0.9812785000000000 | 0.8583780300000000 | 0.0525586900000000 | 1.0 |
| O47 | O | 0.2206297300000000 | 0.1211581100000000 | 0.0235027900000000 | 1.0 |
| O48 | O | 0.2269429100000000 | 0.8707812600000000 | 0.0723644500000000 | 1.0 |
| O49 | O | 0.4594808200000000 | 0.1033355400000000 | 0.0645038600000000 | 1.0 |
| O50 | O | 0.4803146700000000 | 0.8518139800000000 | 0.0365000600000000 | 1.0 |
| O51 | O | 0.7272926300000000 | 0.0894455900000000 | 0.0765602900000000 | 1.0 |
| O52 | O | 0.7250824700000000 | 0.8434445900000000 | 0.0115196600000000 | 1.0 |
| S53 | S | 0.9675808400000000 | 0.9895172800000000 | 0.0996282100000000 | 1.0 |
| S54 | S | 0.2238394300000000 | 0.0104605000000000 | 0.1016945500000000 | 1.0 |
| S55 | S | 0.4718893100000000 | 0.9730793100000000 | 0.1033344400000000 | 1.0 |
| S56 | S | 0.7262868400000000 | 0.9490283400000000 | 0.0979510400000000 | 1.0 |

##### cif ends
